# Supplementary material for: Defining and Evaluating Network Communities based on Ground-truth
Source: arXiv:1205.6233 source file (2012-11-06)
Supplement: Supplementary file 1 [file 070appendix.tex]

\begin{figure}[!h]
	\centering
	\subfigure[Sep.	(LJ)]{\includegraphics[width=0.15\textwidth]{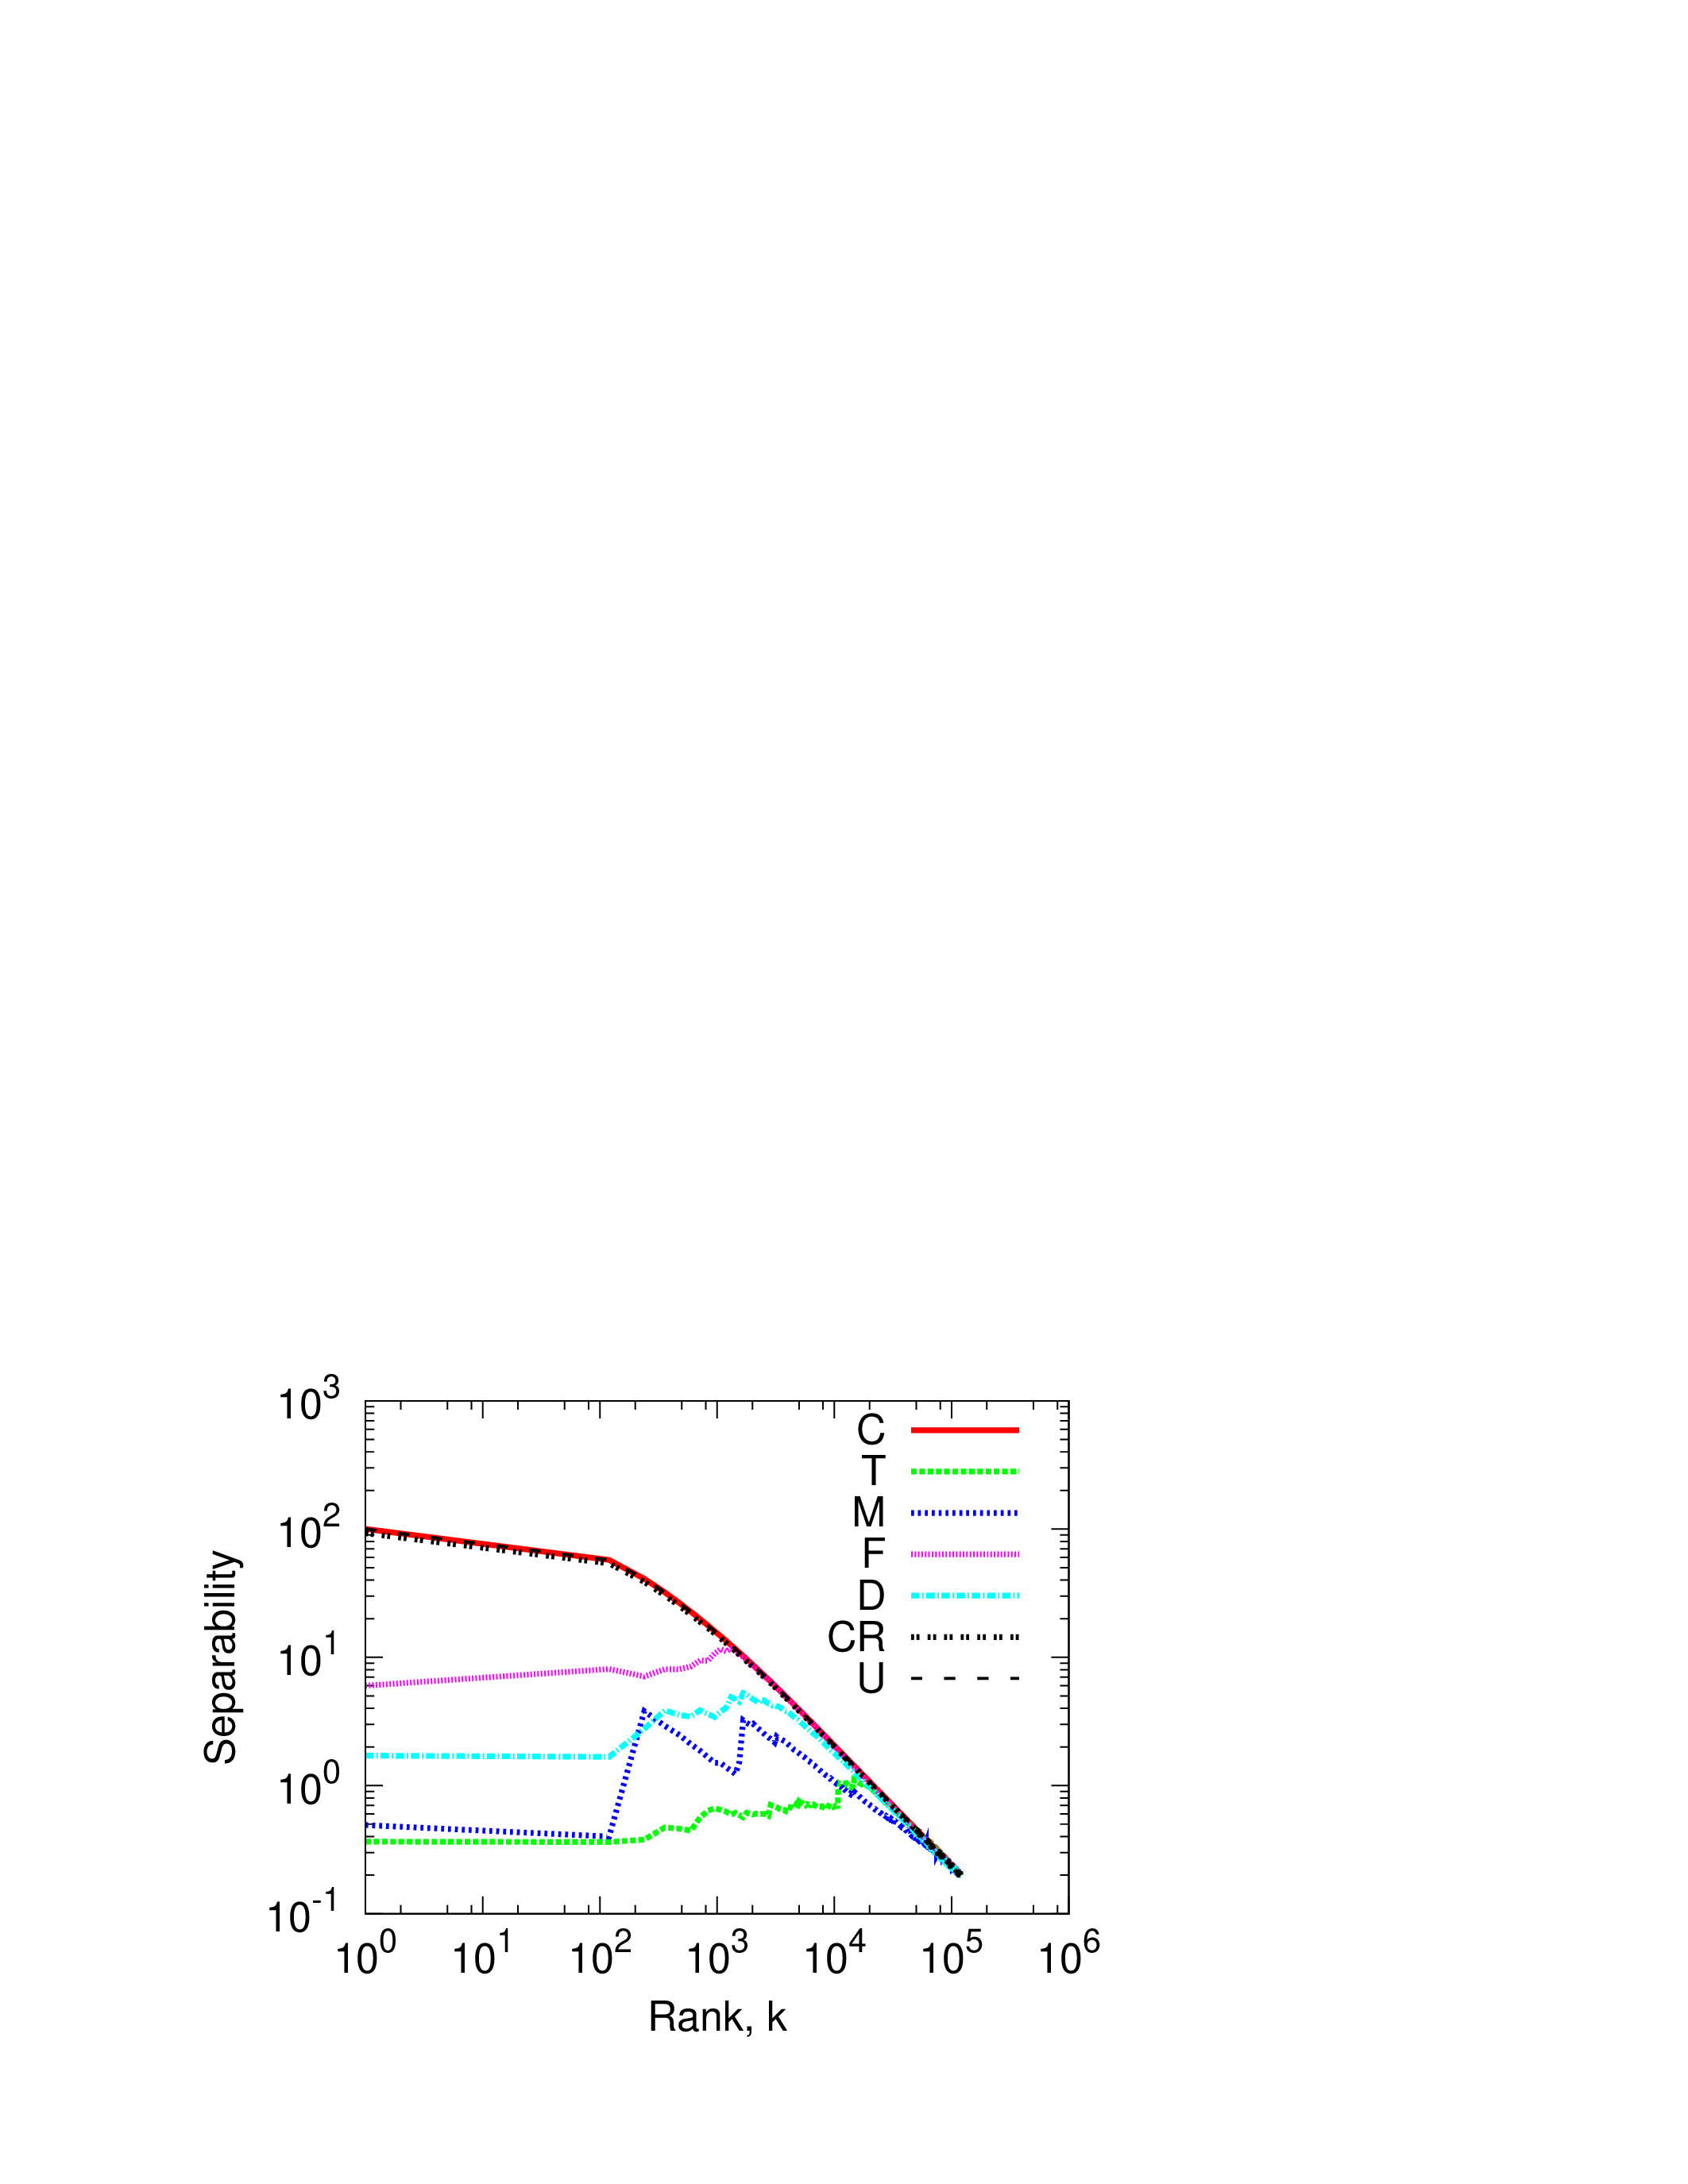}}
	\subfigure[Sep.	(FS)]{\includegraphics[width=0.15\textwidth]{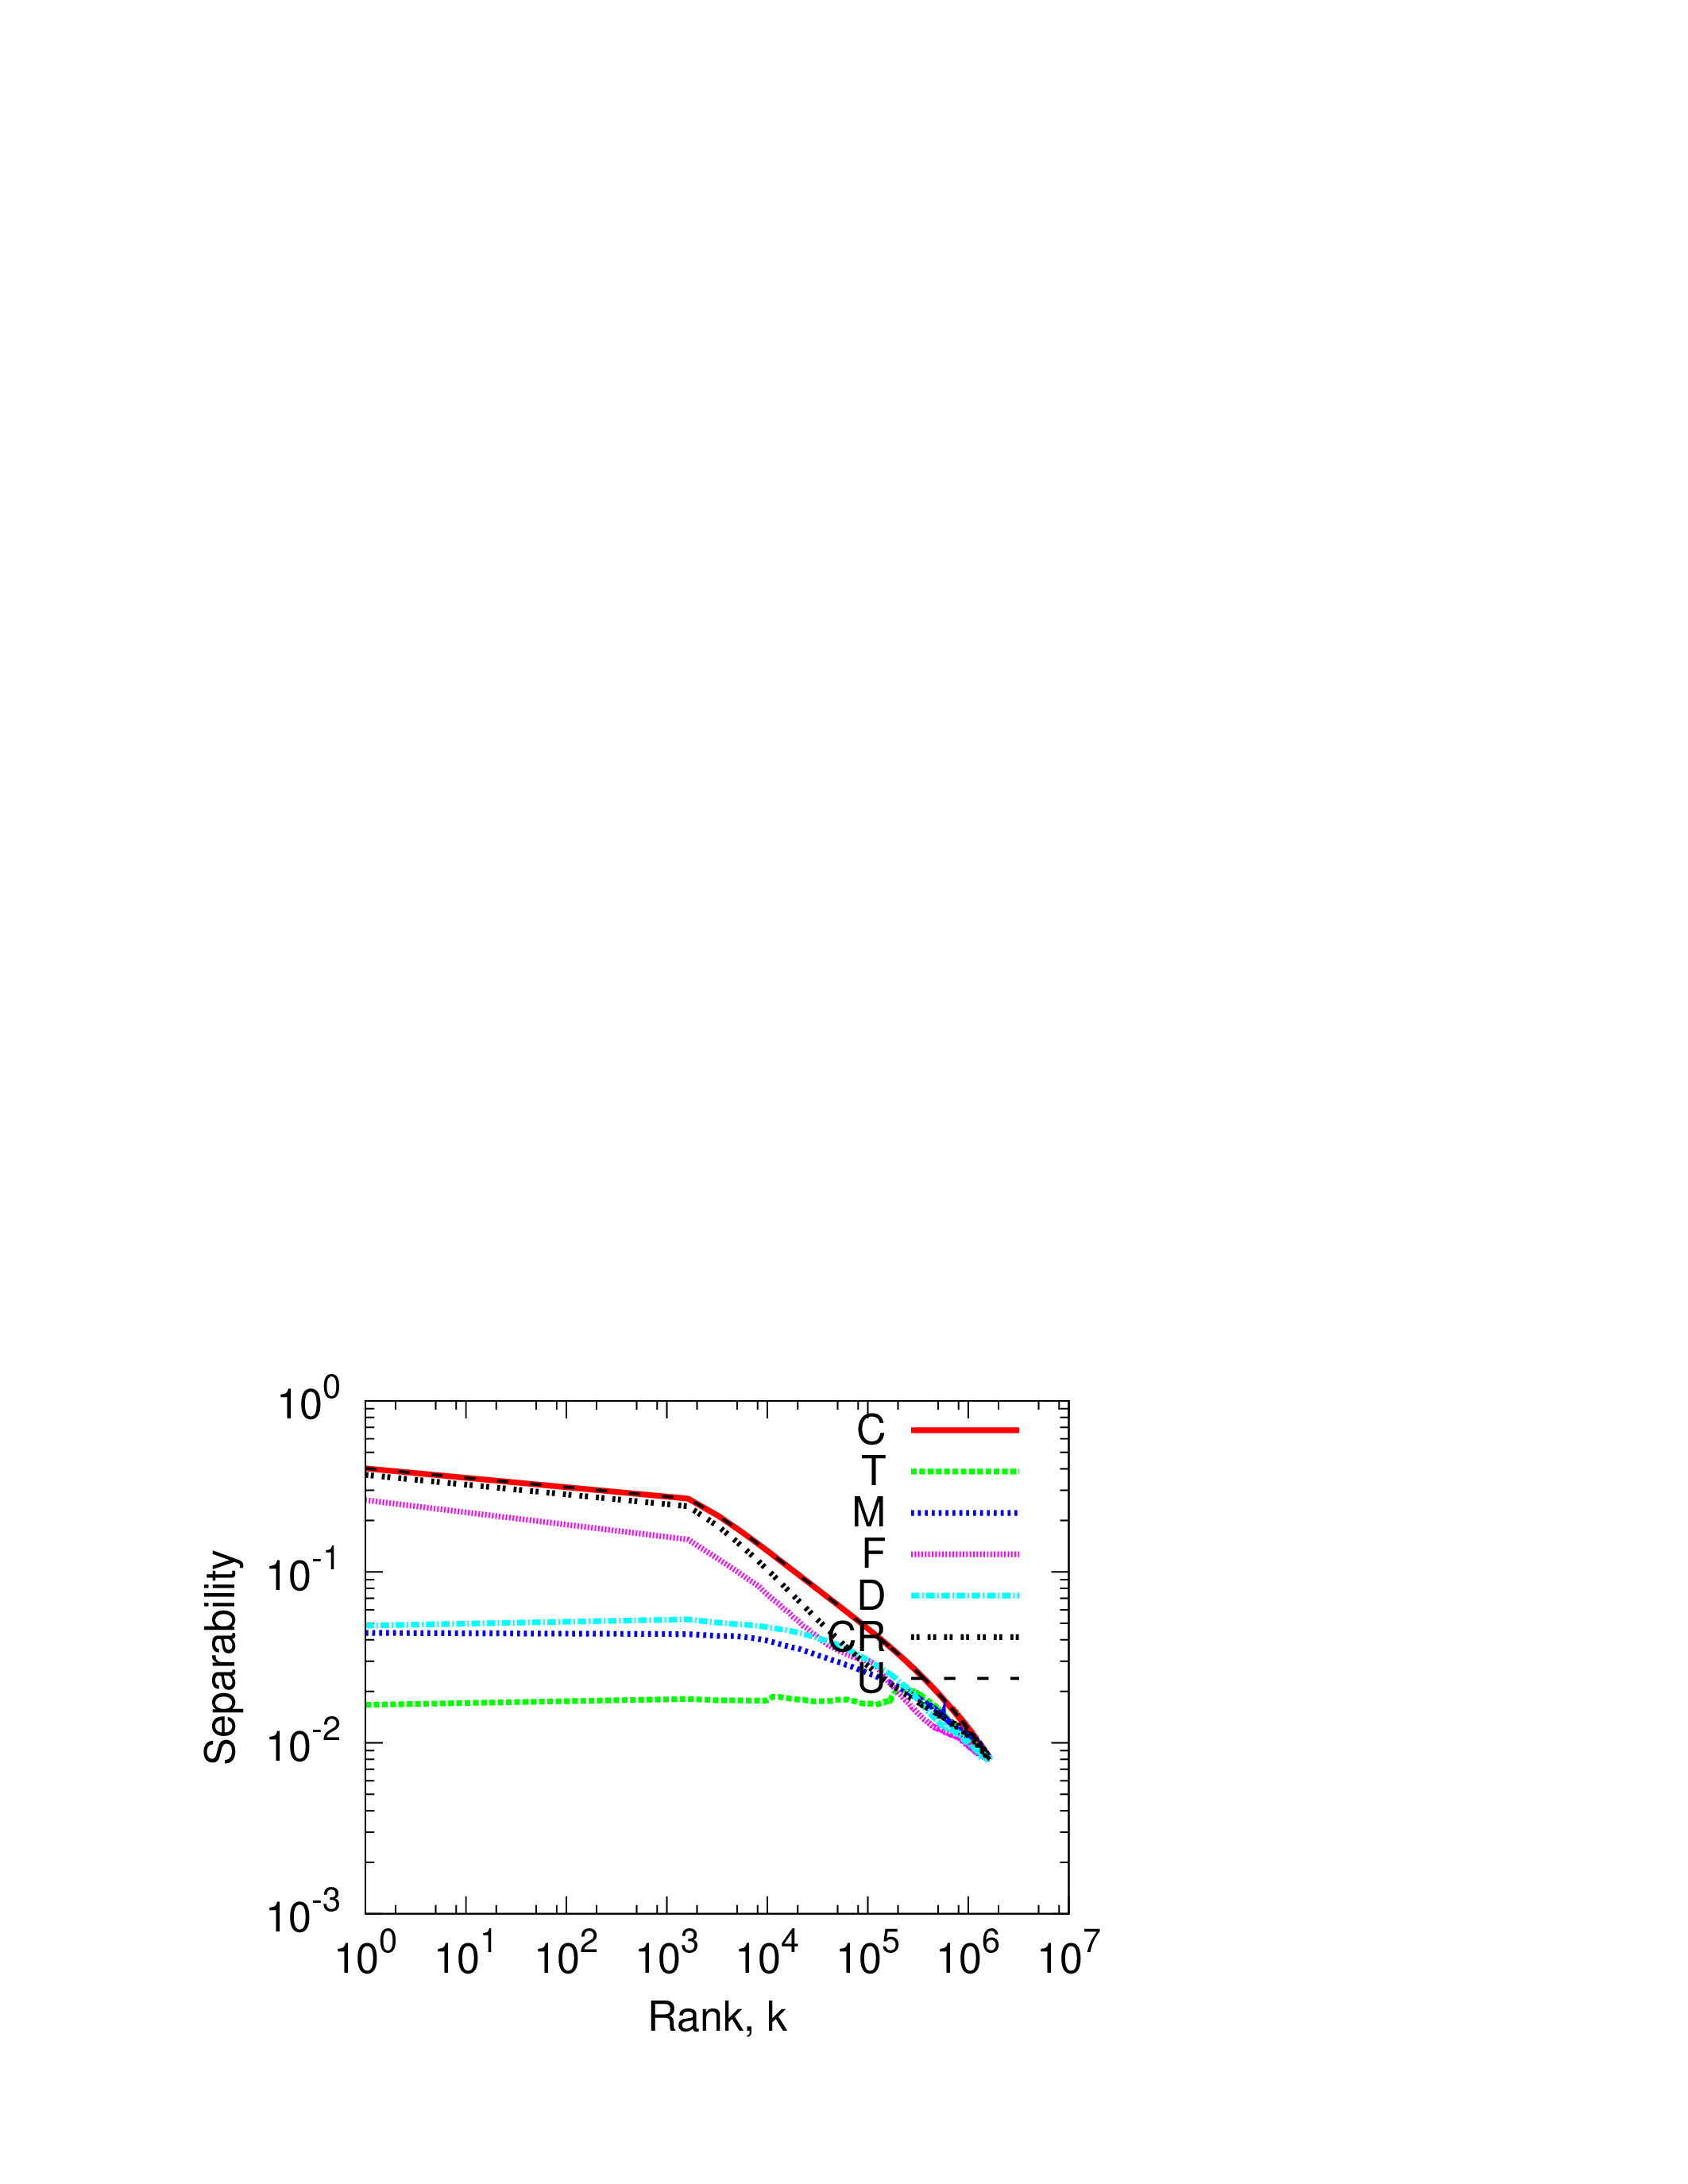}}
	\subfigure[Sep.	(Orkut)]{\includegraphics[width=0.15\textwidth]{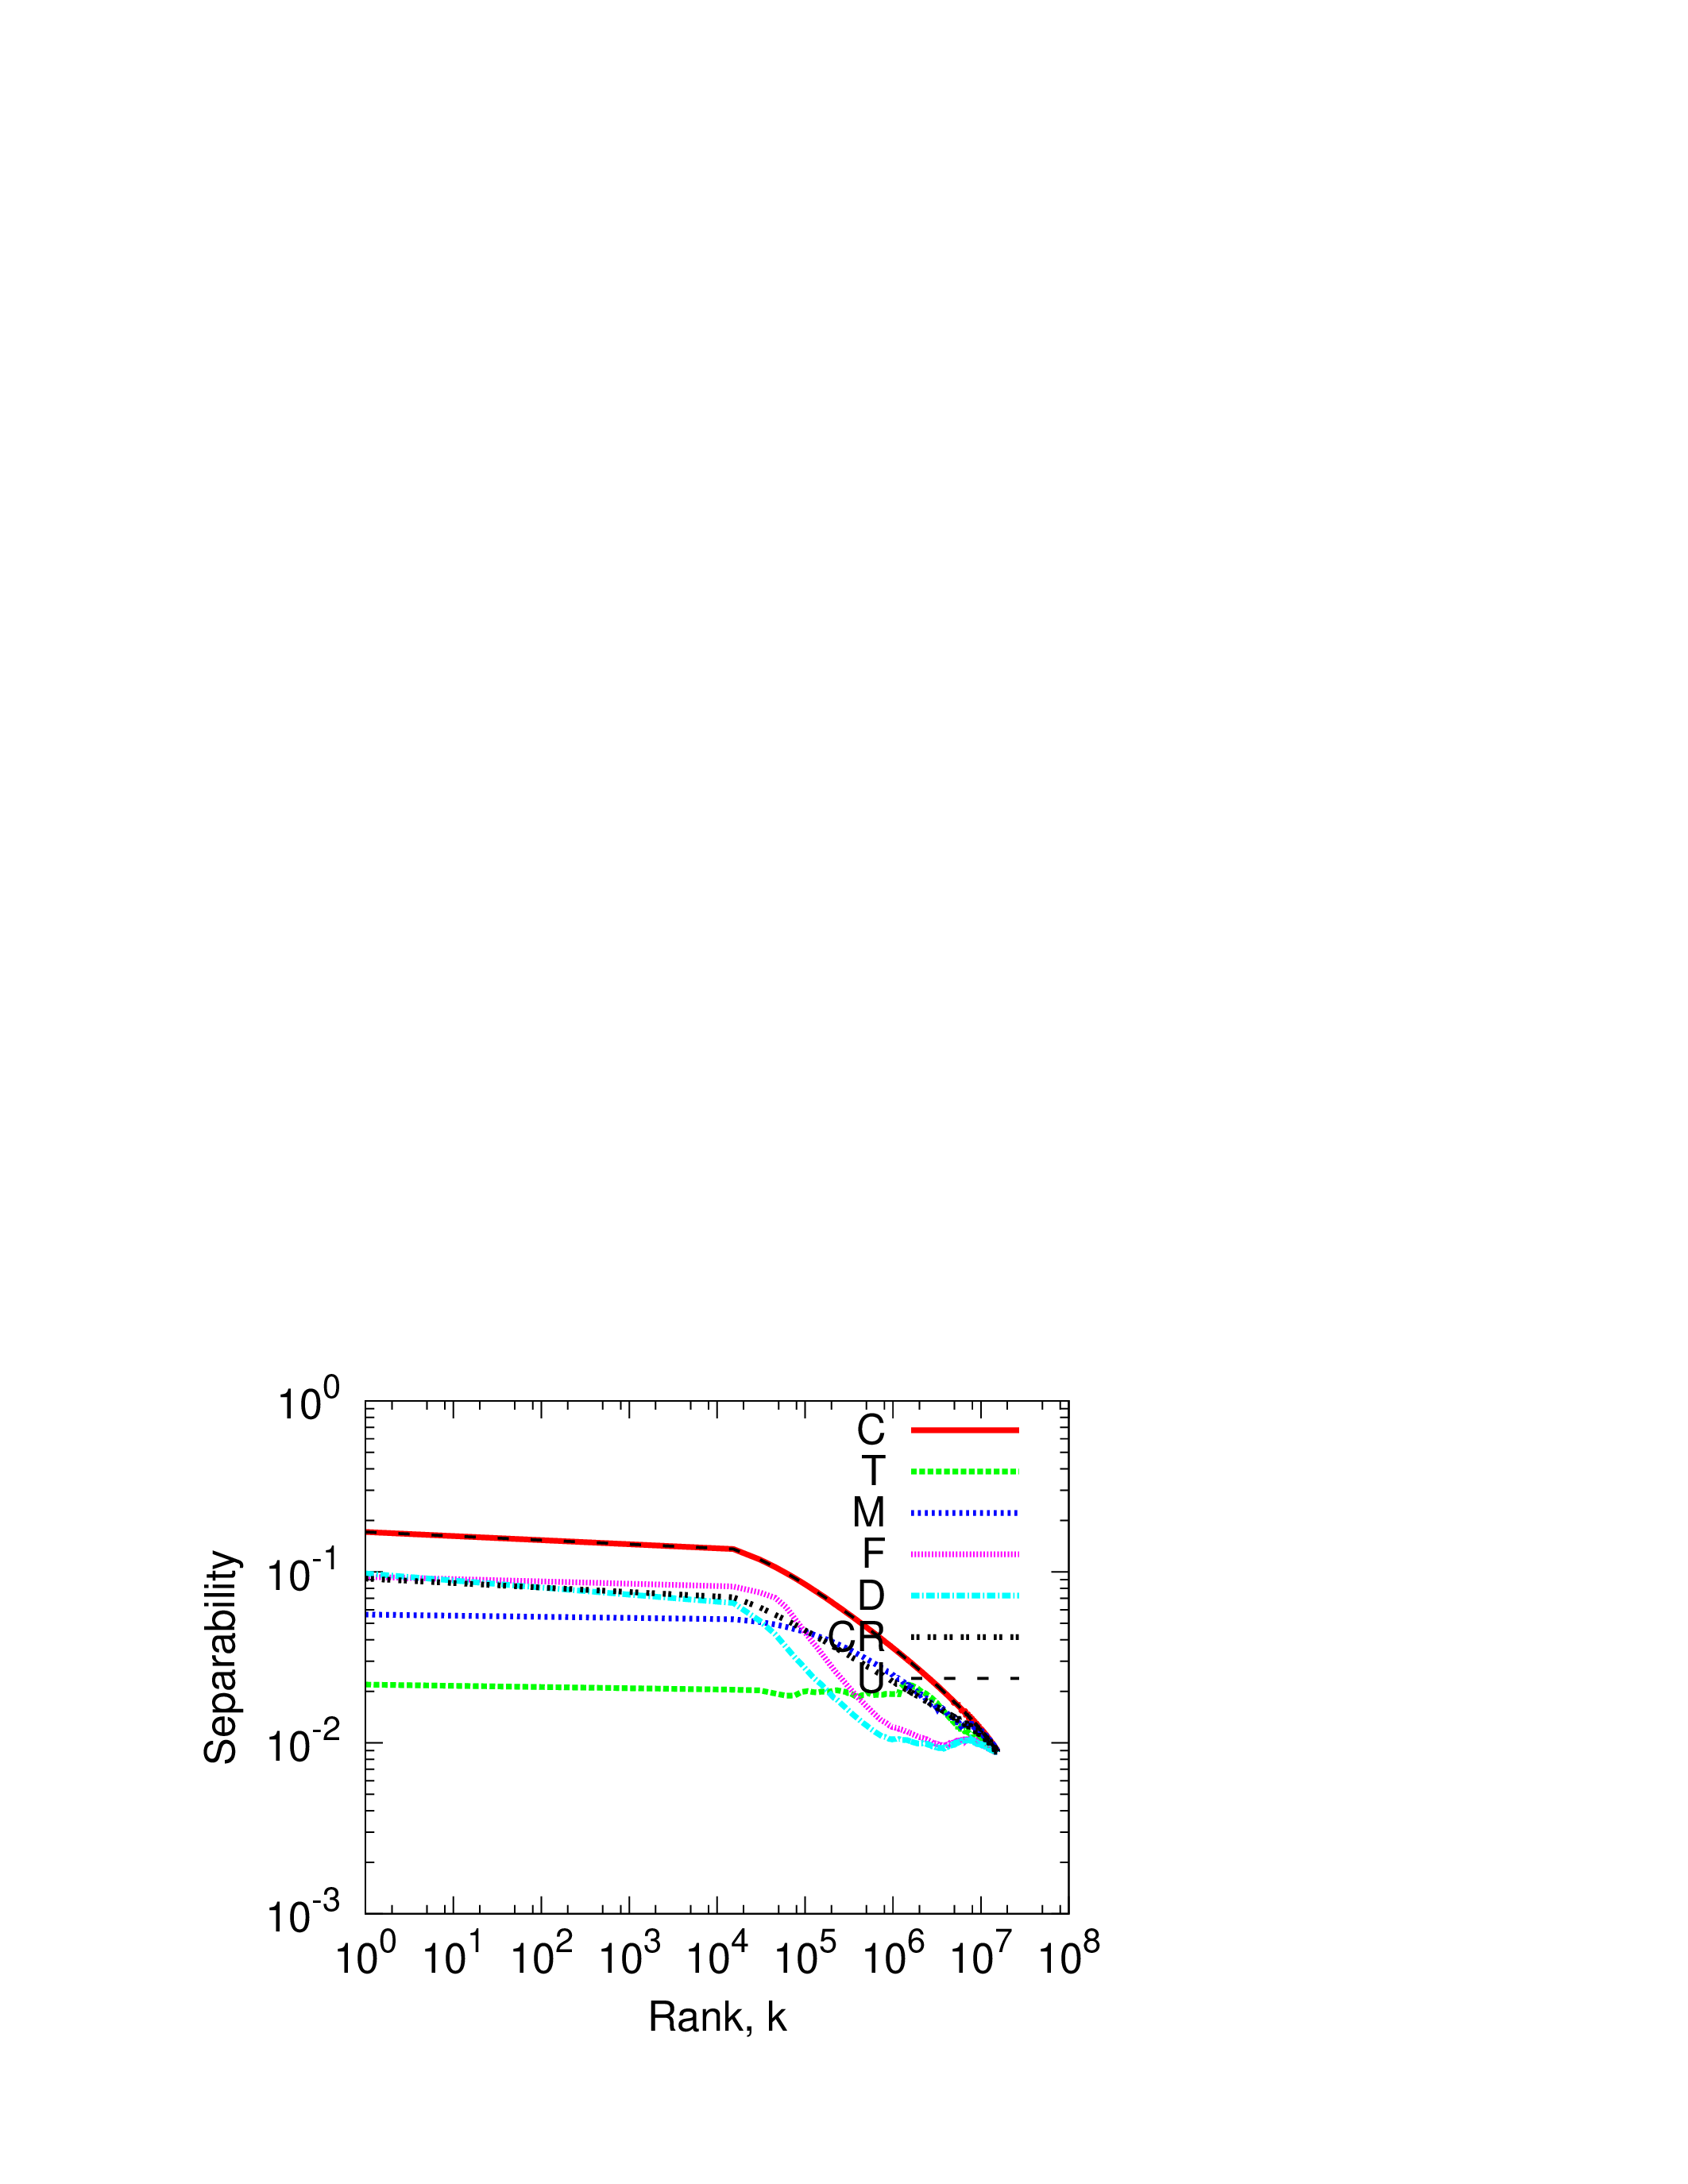}}
	\subfigure[Sep.	(Ning)]{\includegraphics[width=0.15\textwidth]{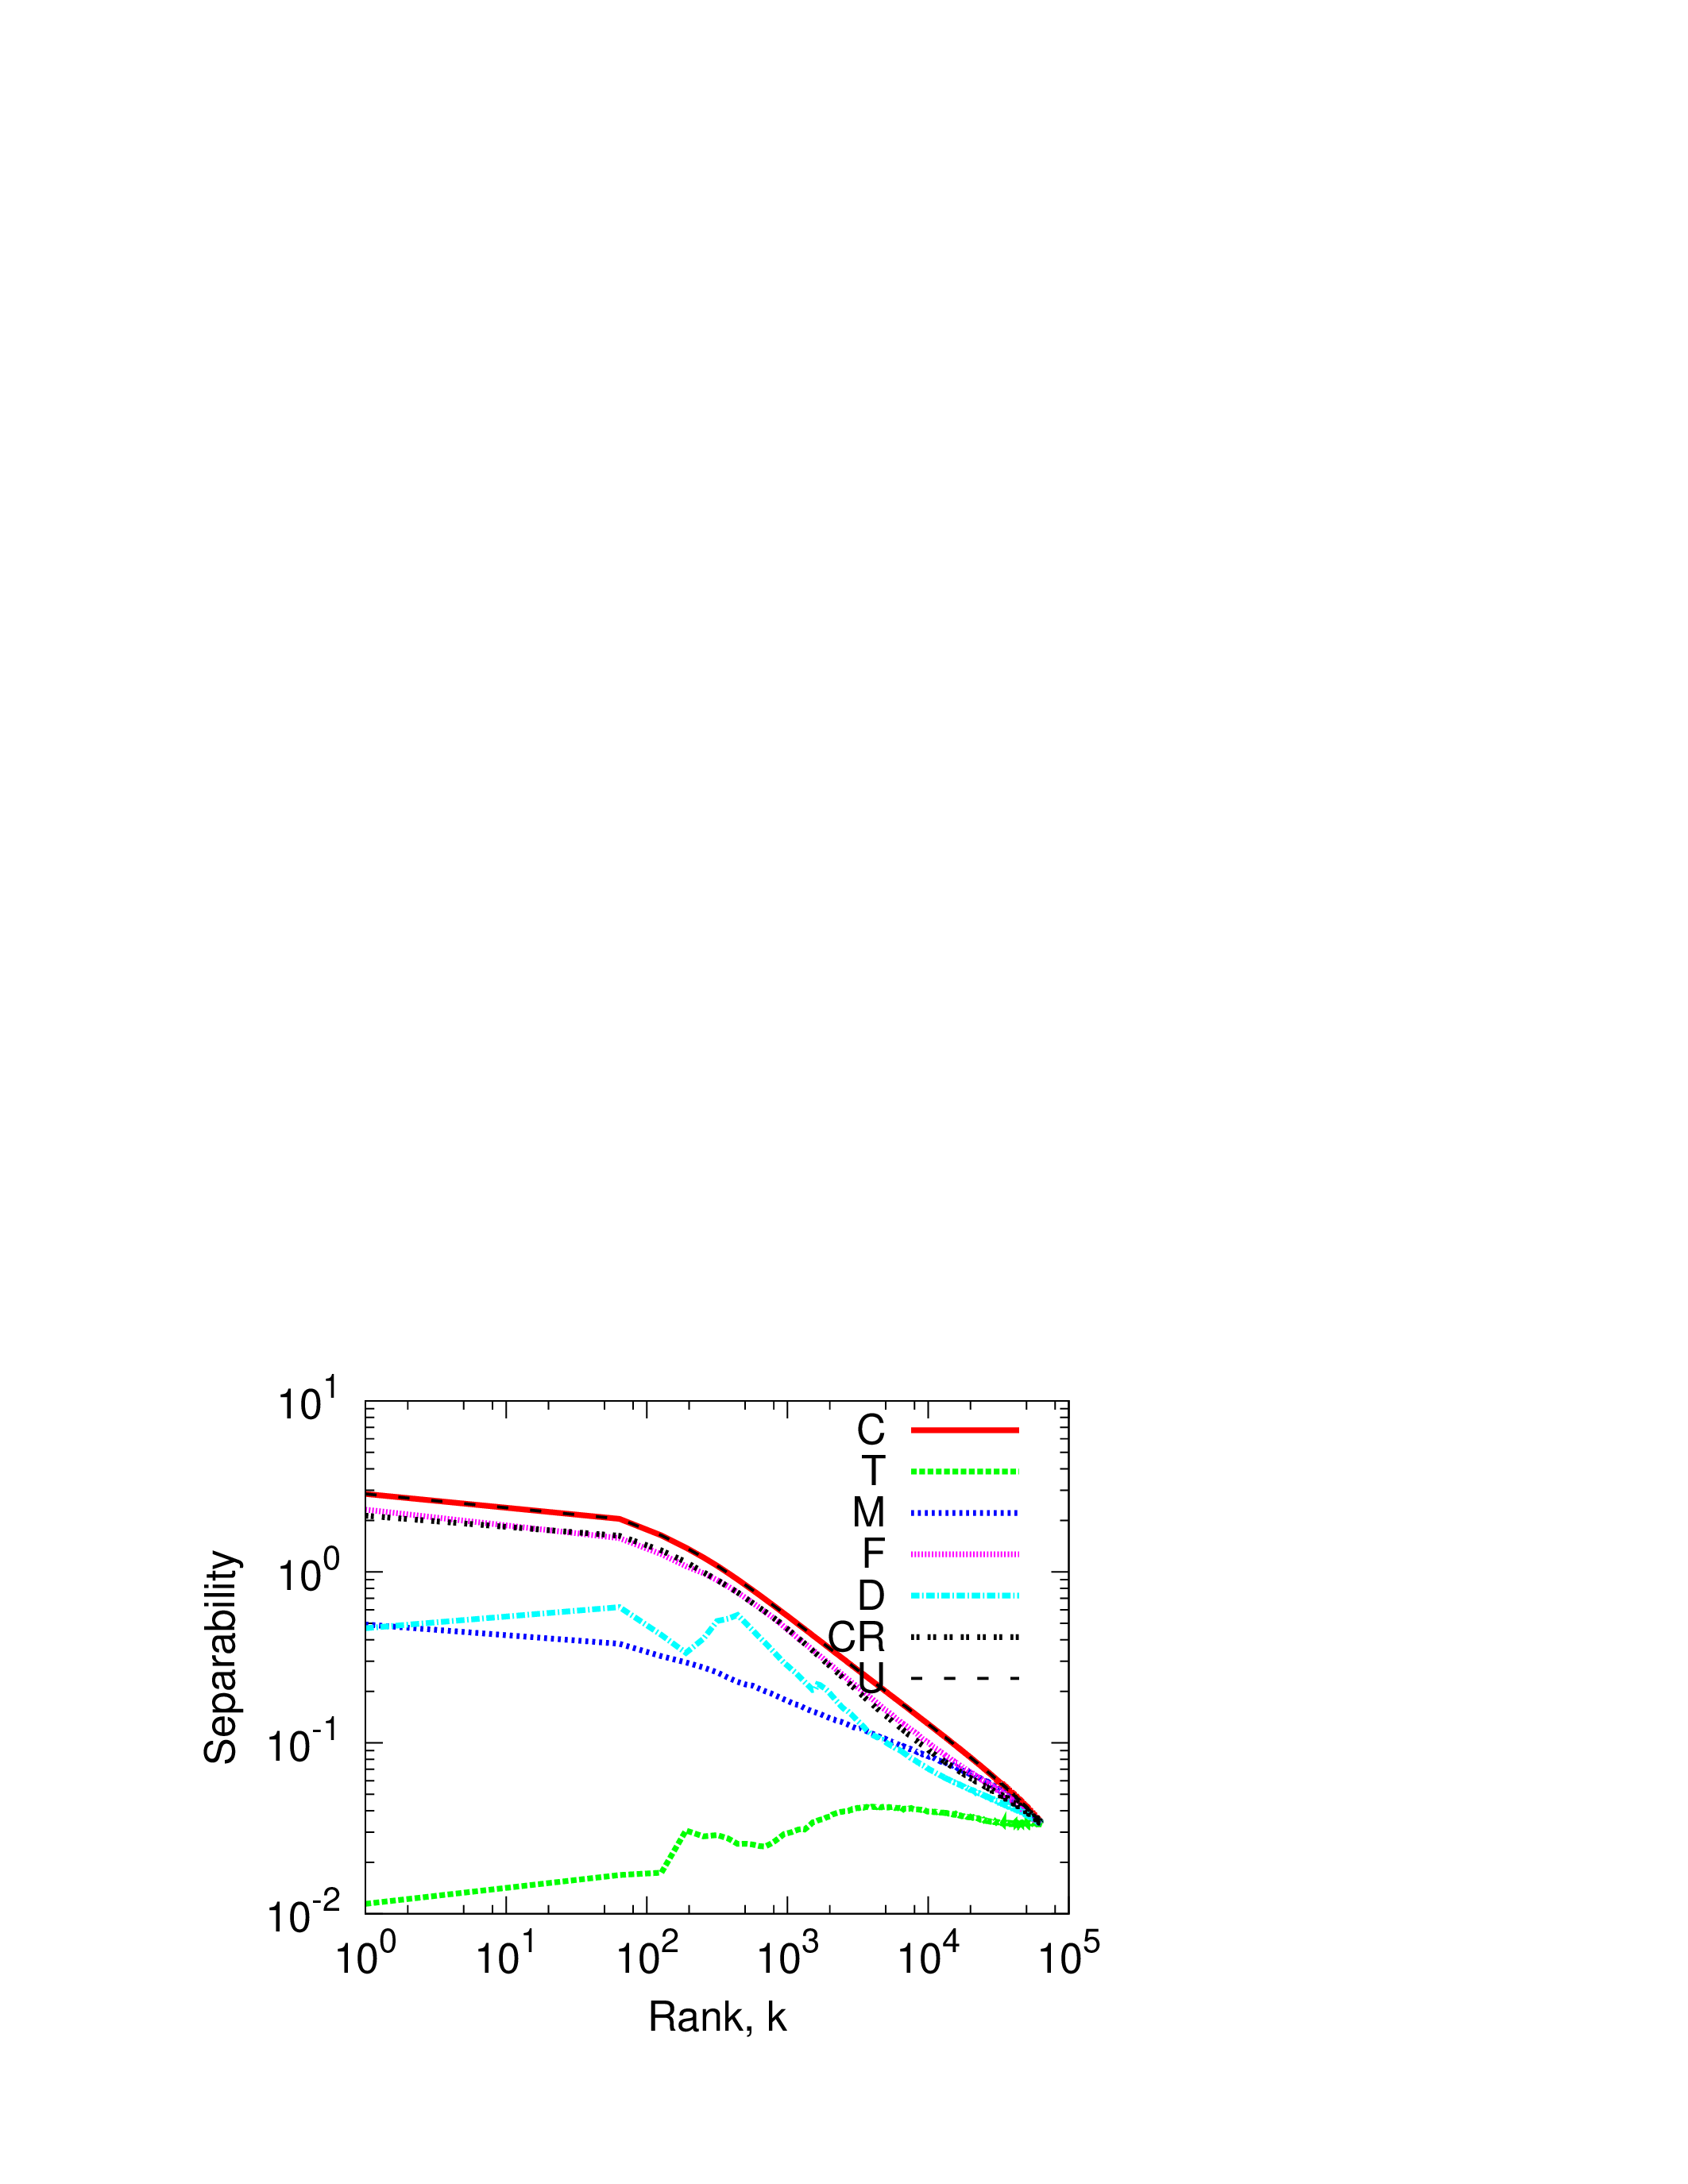}}
	\subfigure[Sep.	(Amazon)]{\includegraphics[width=0.15\textwidth]{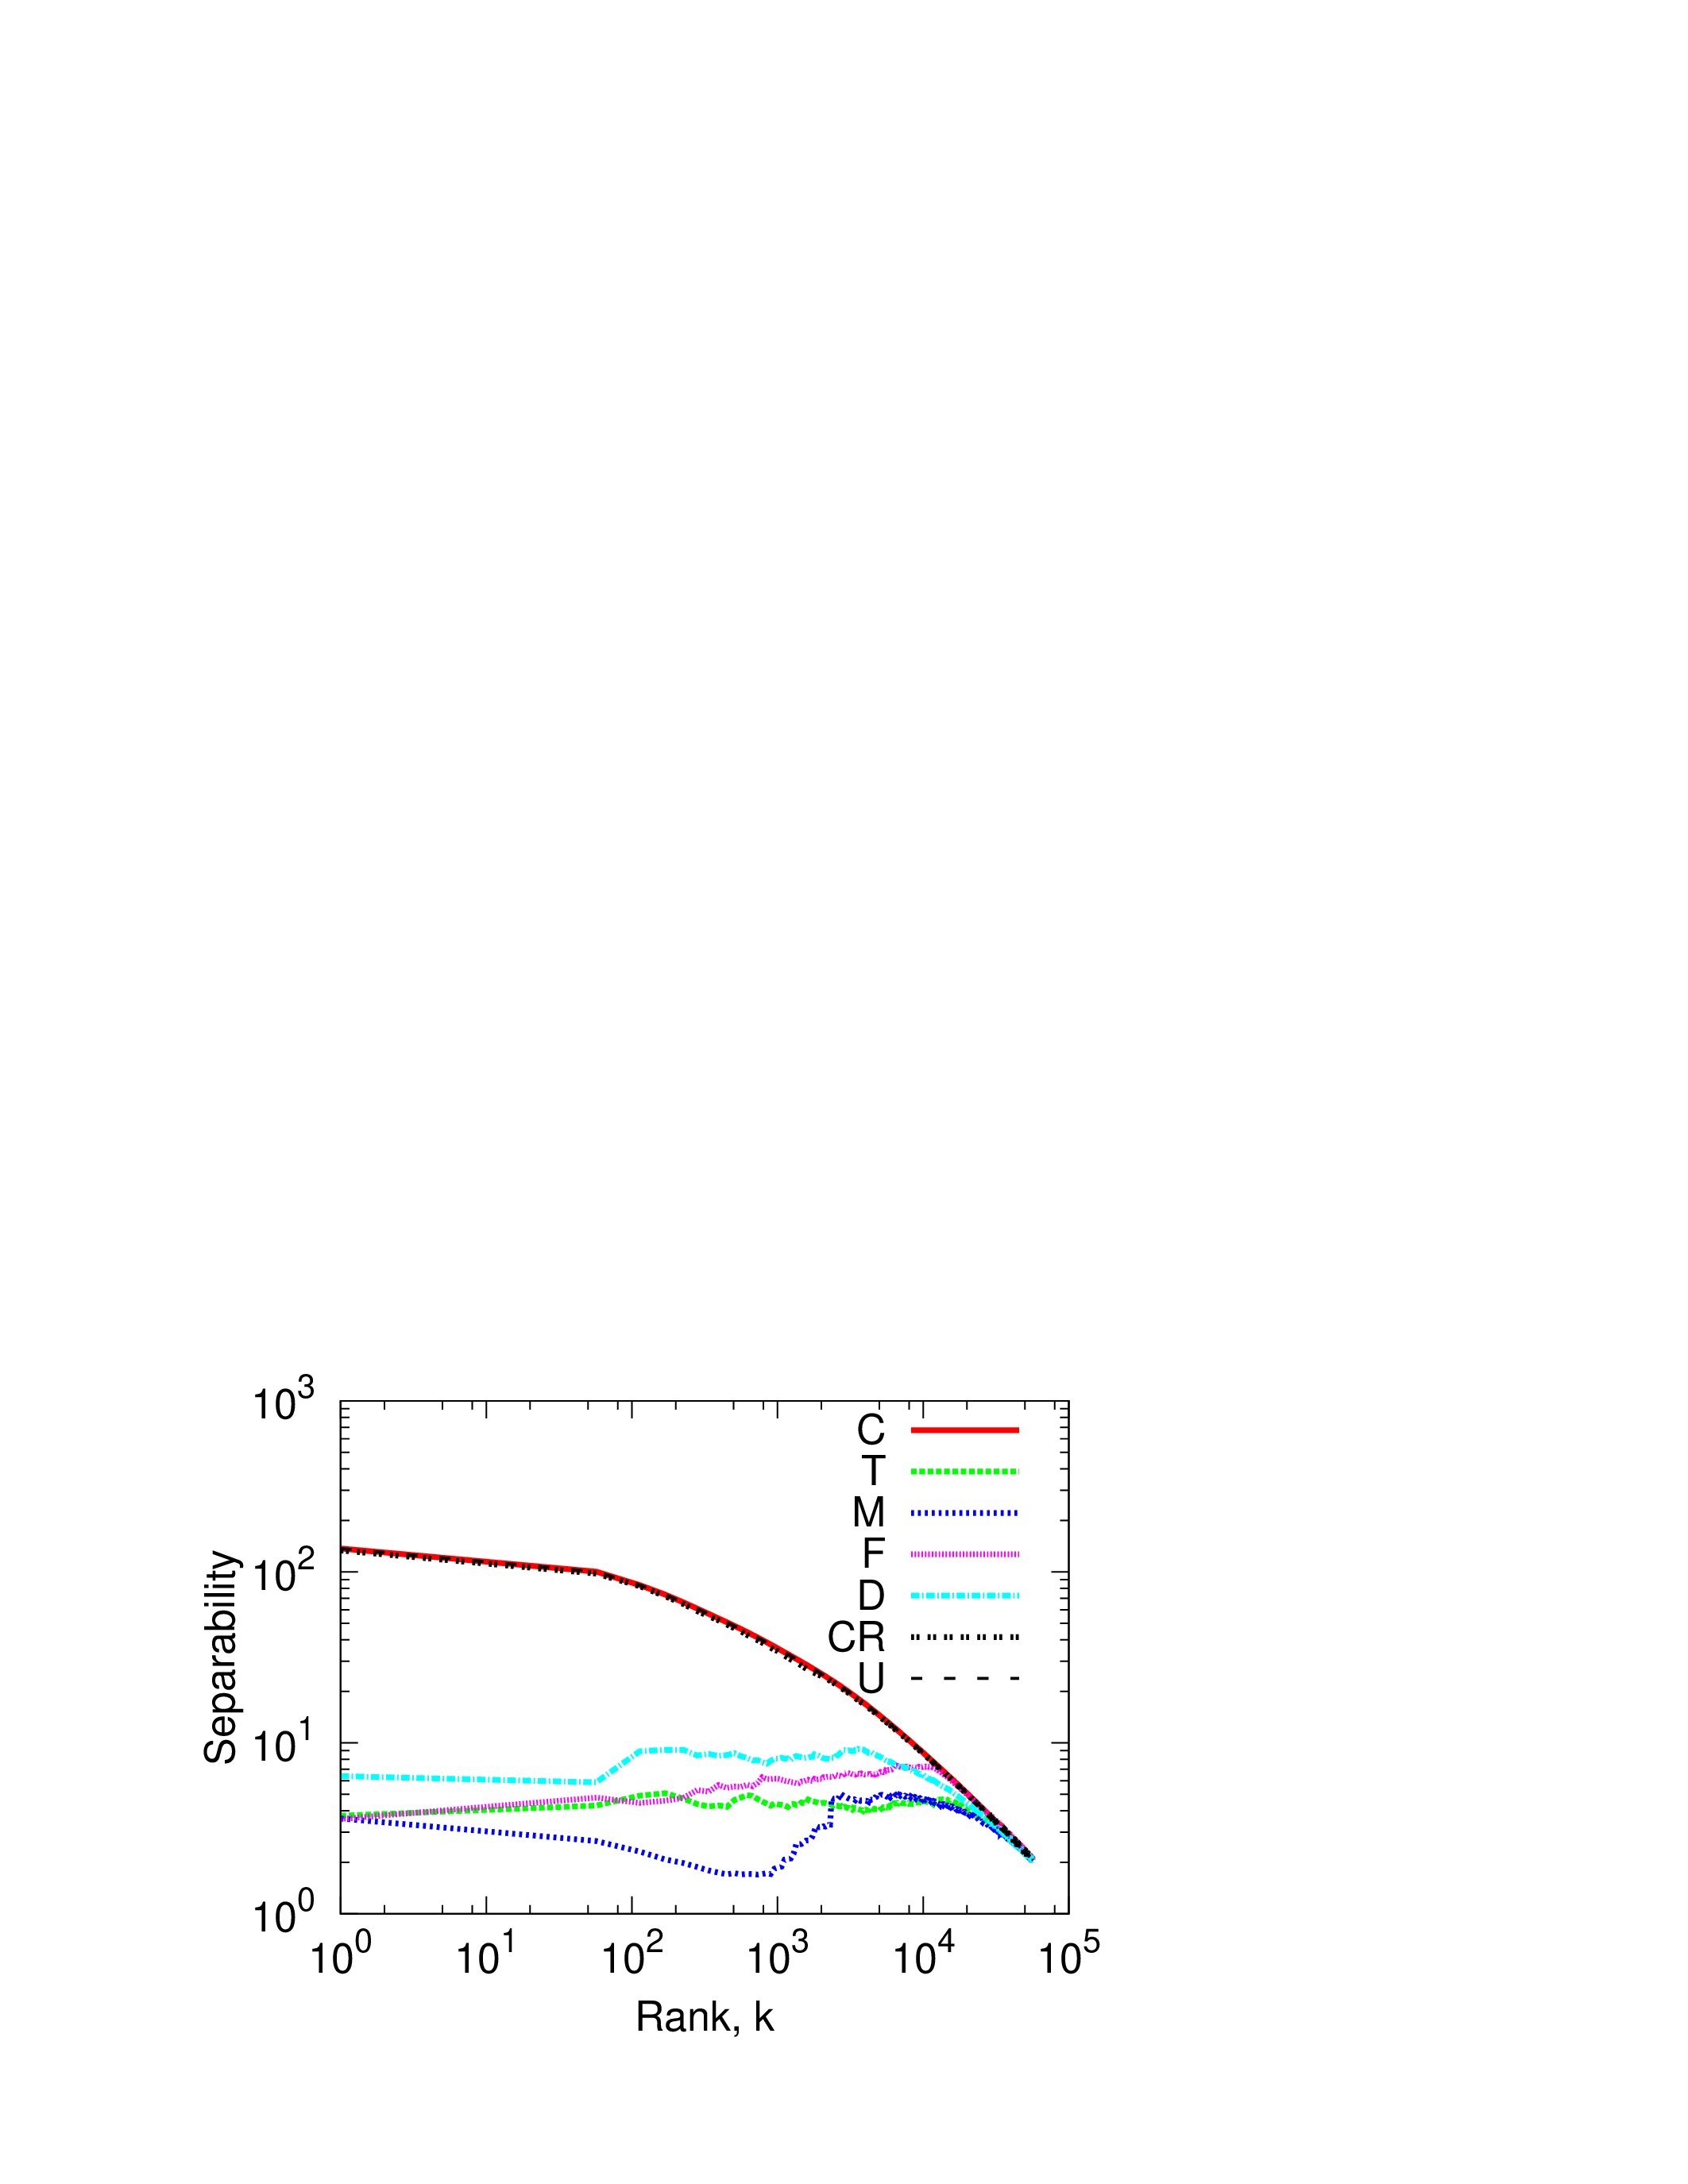}}
	\subfigure[Sep.	(DBLP)]{\includegraphics[width=0.15\textwidth]{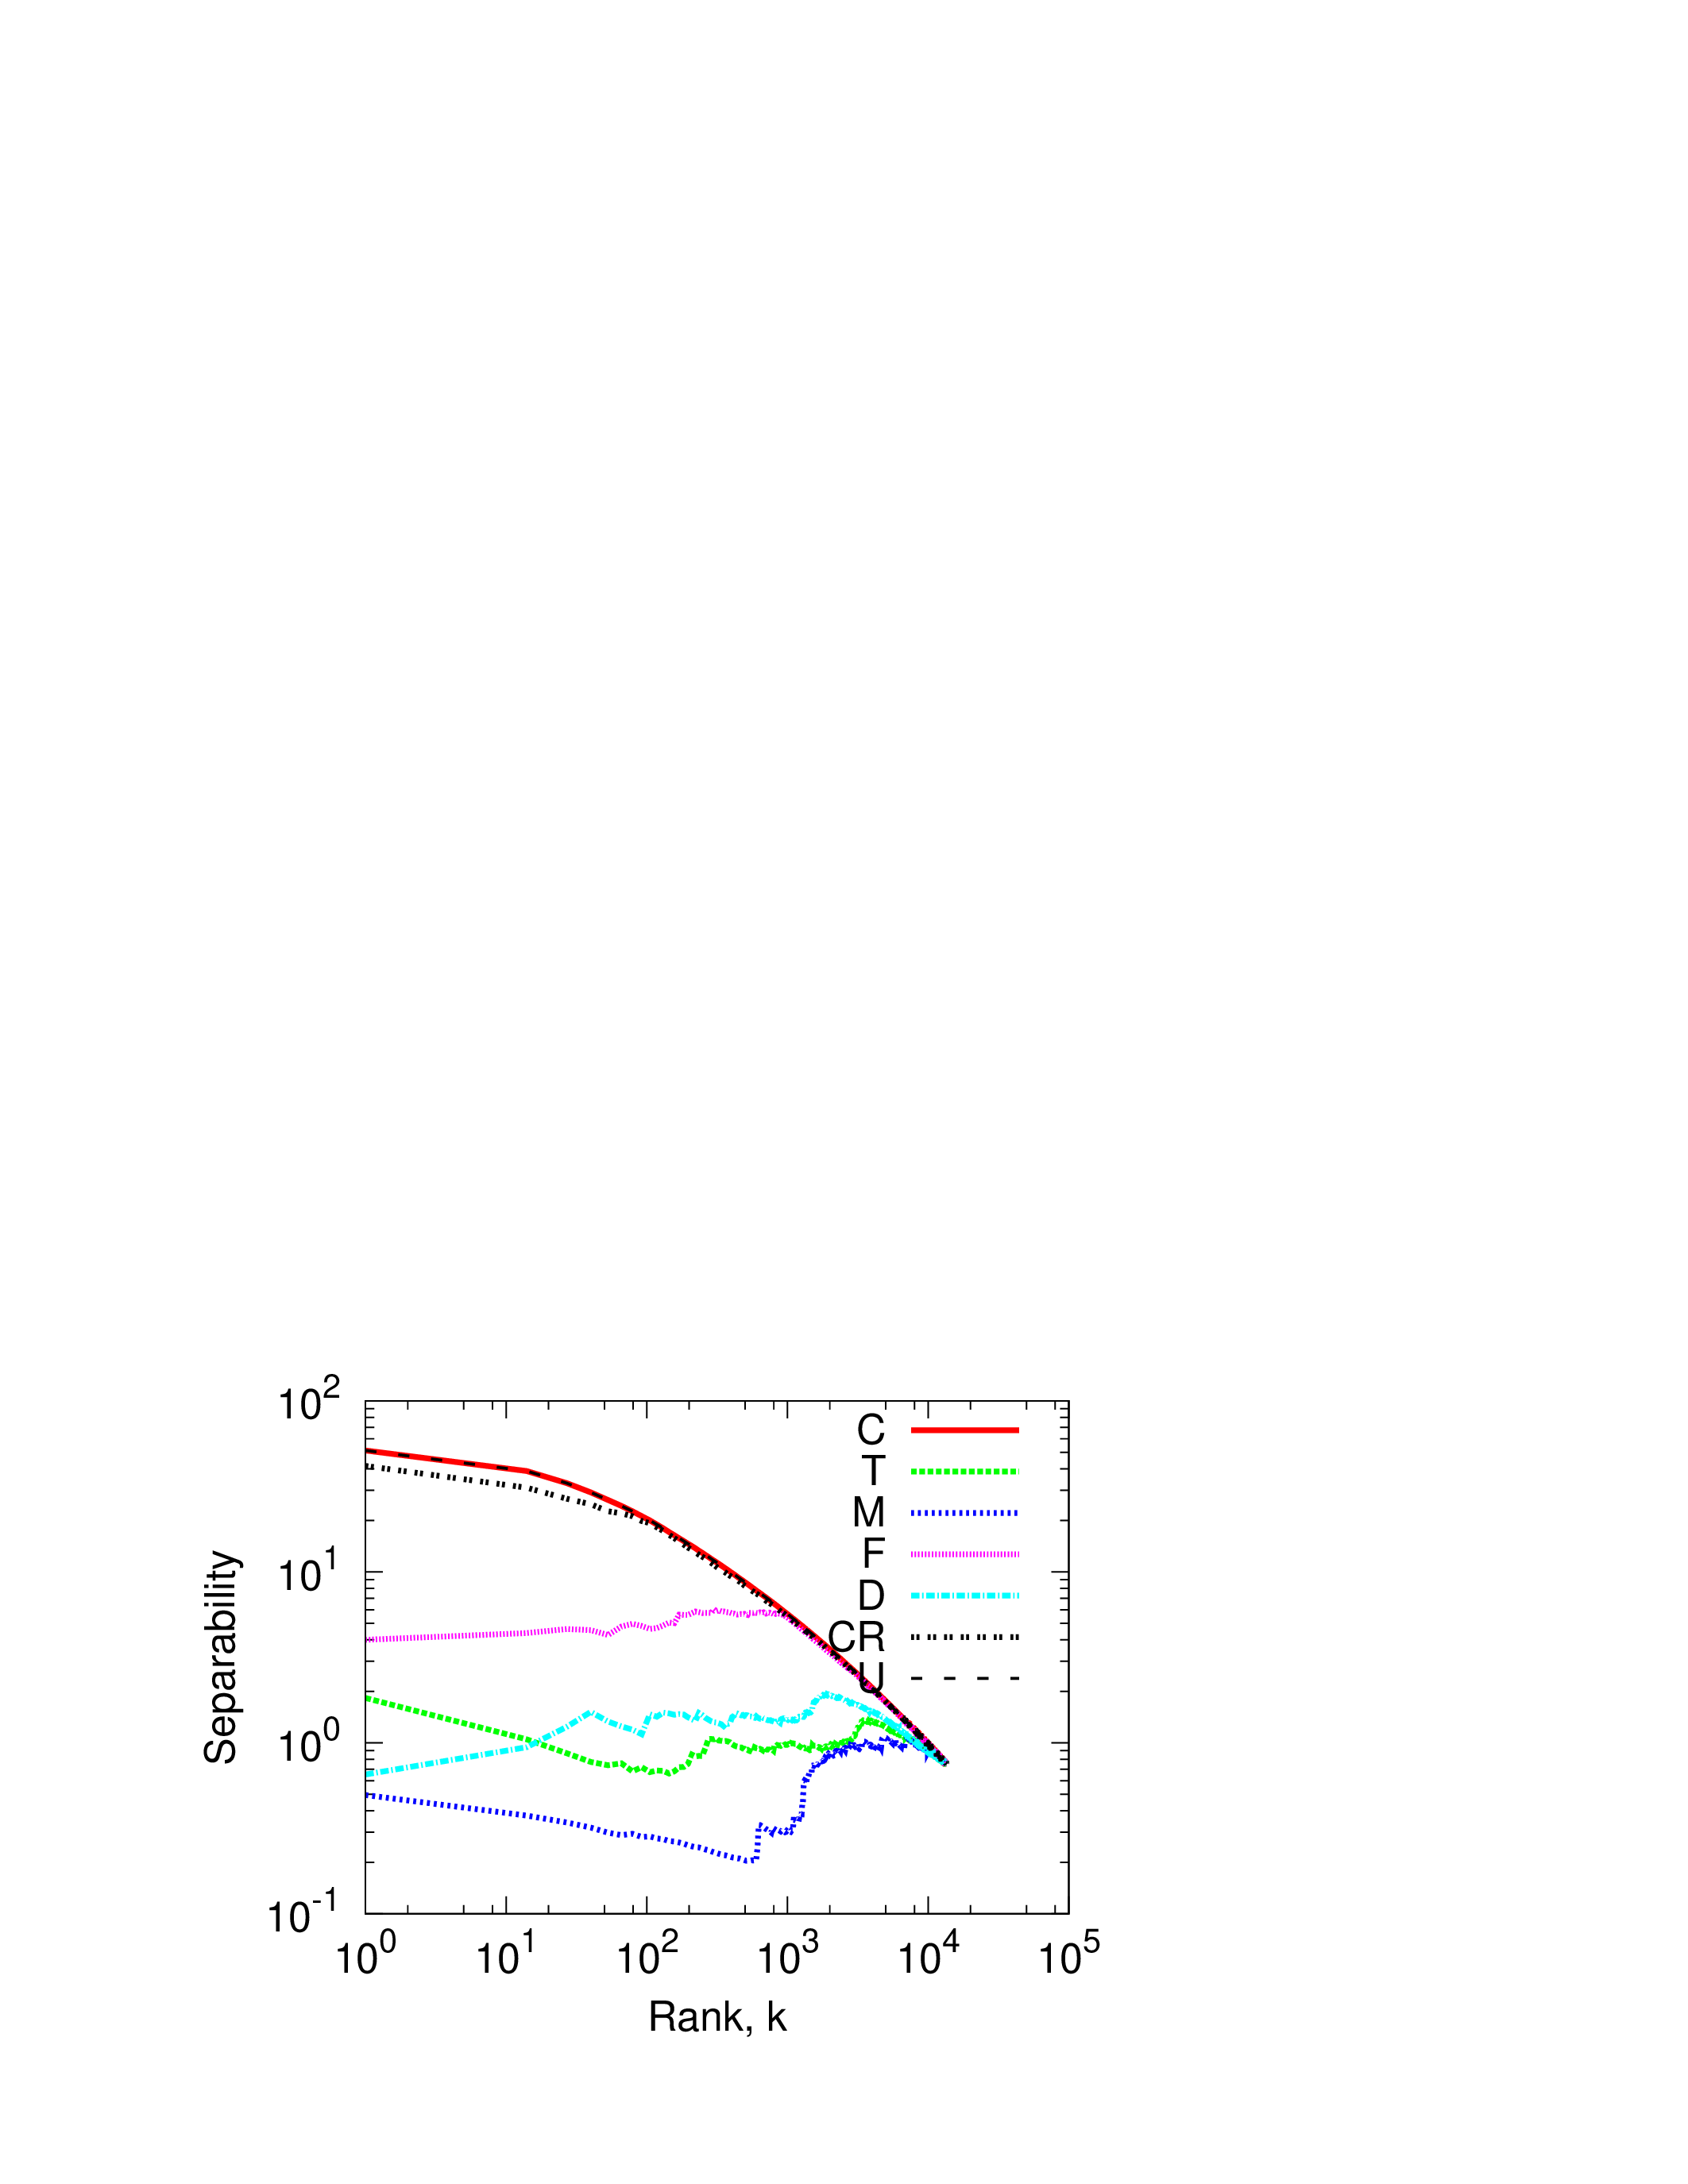}}
	\subfigure[Density	(LJ)]{\includegraphics[width=0.15\textwidth]{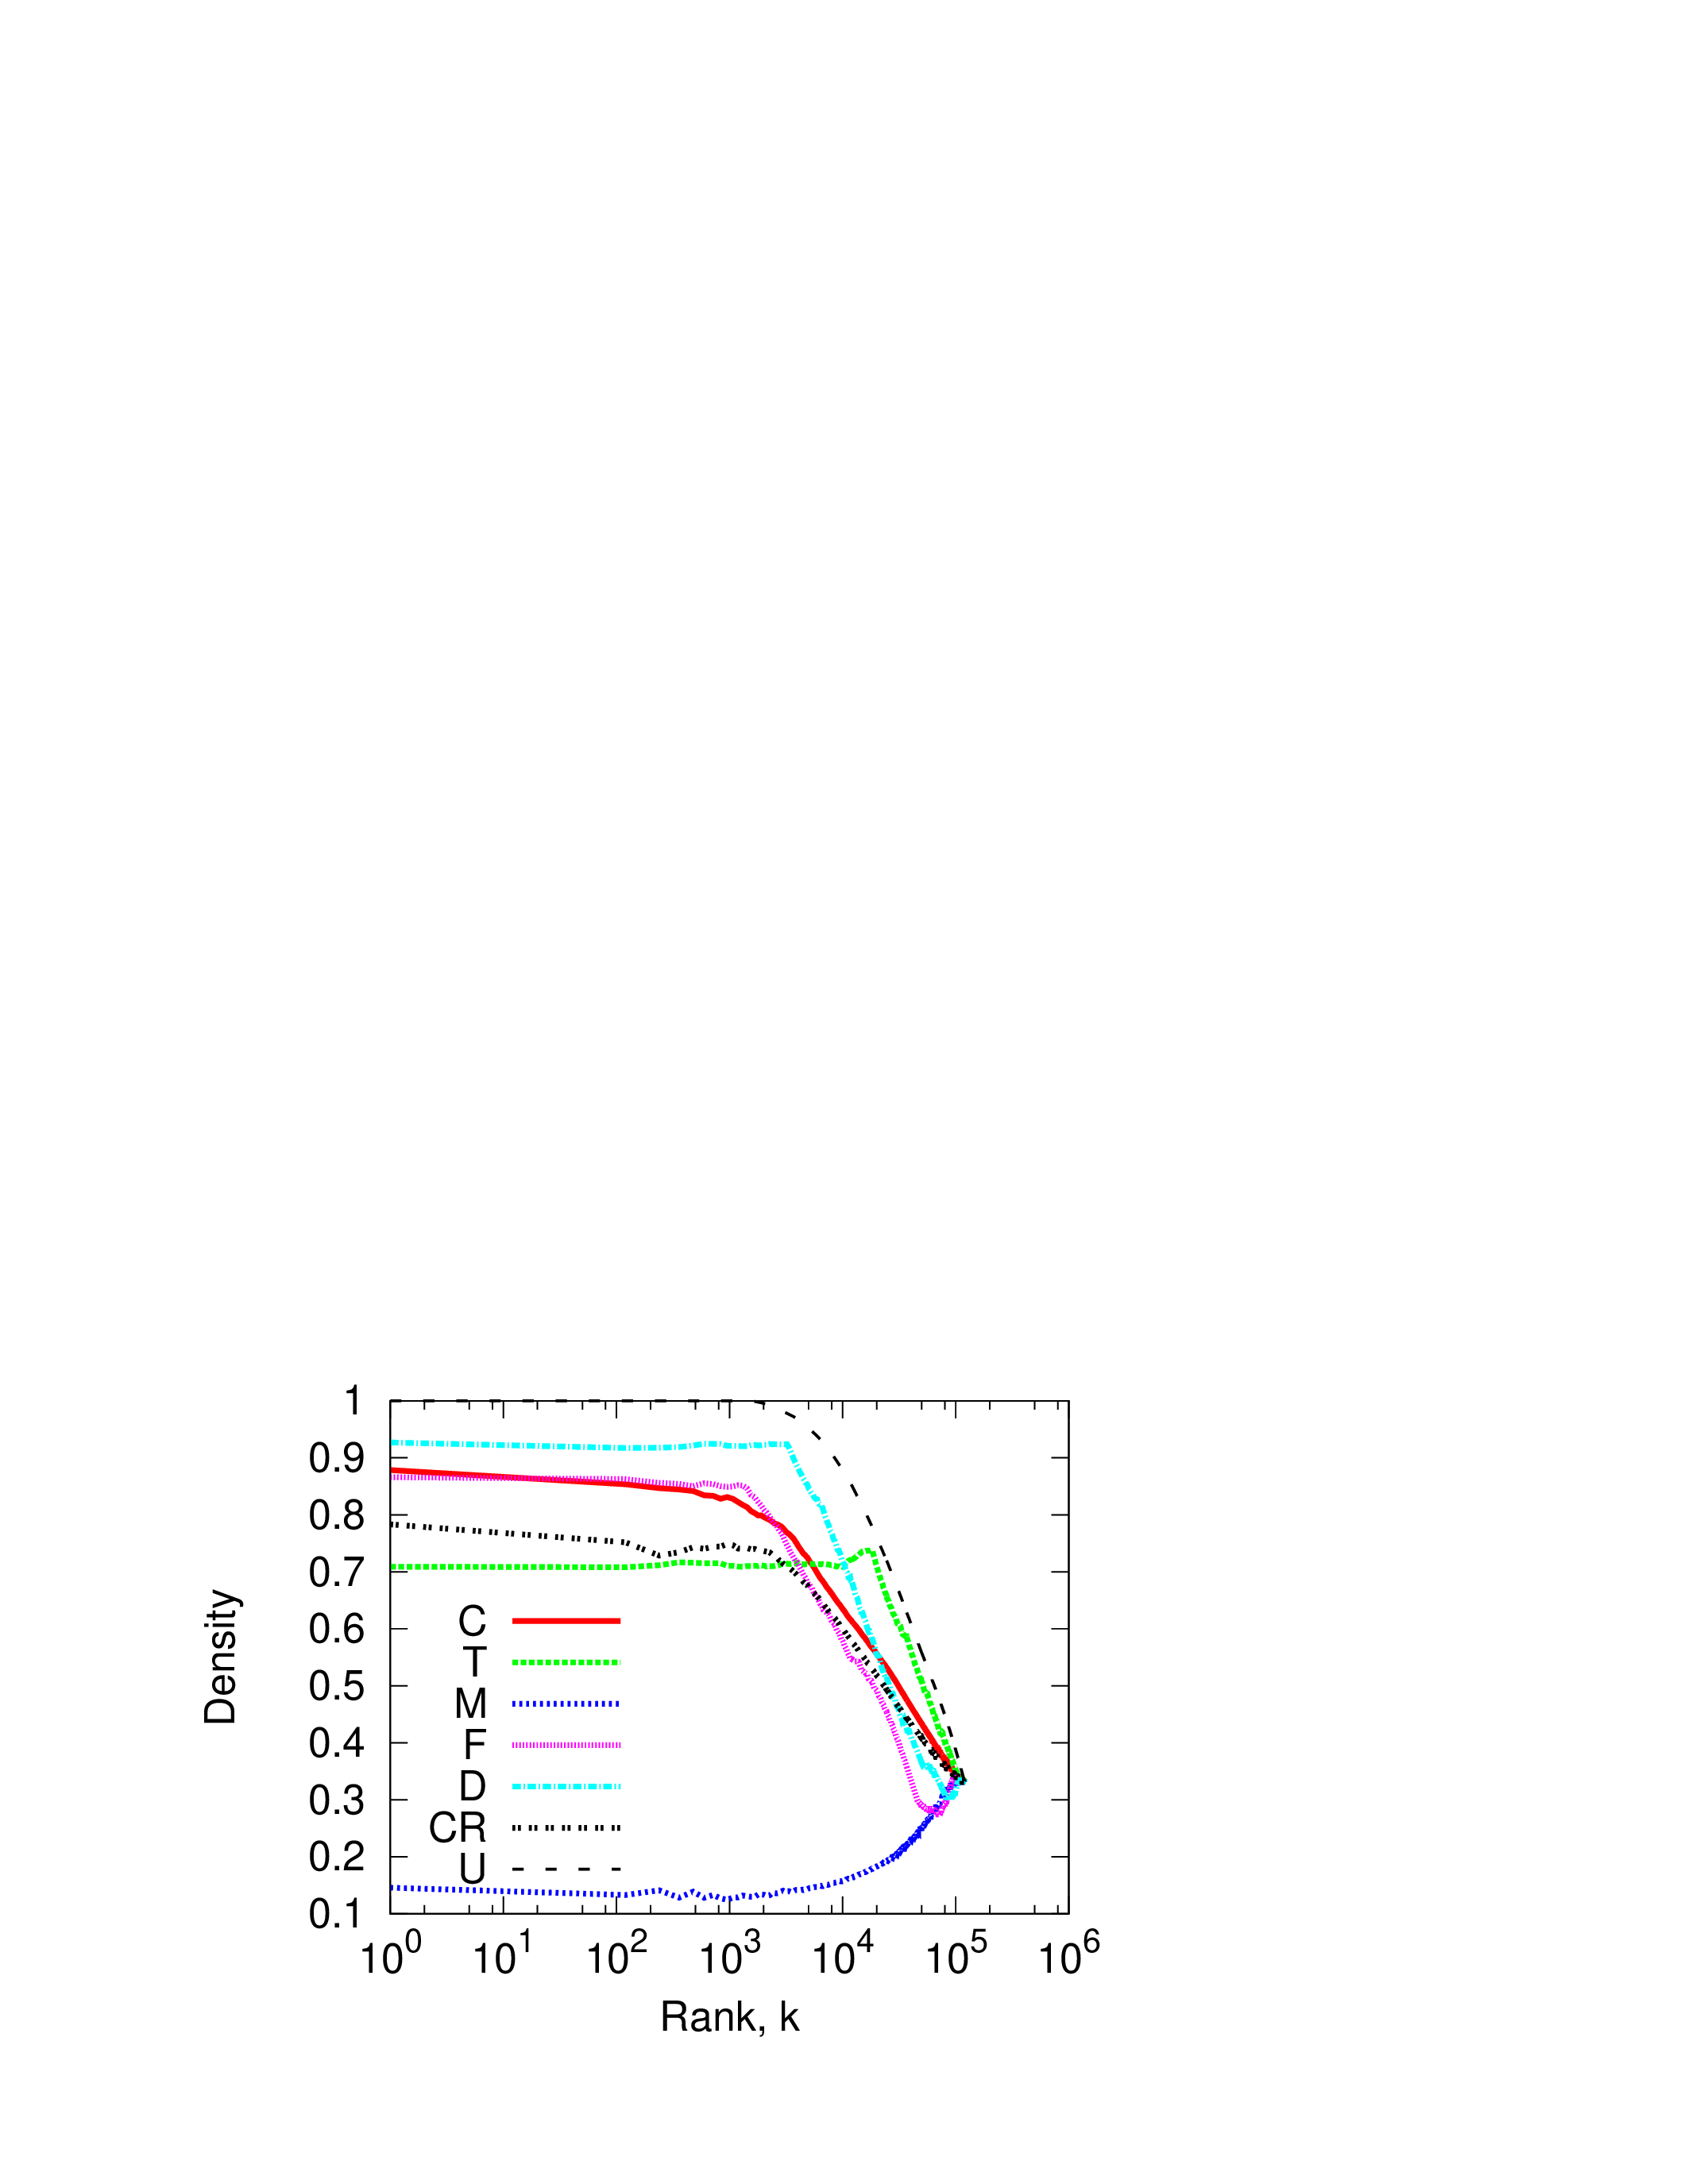}}
	\subfigure[Density	(FS)]{\includegraphics[width=0.15\textwidth]{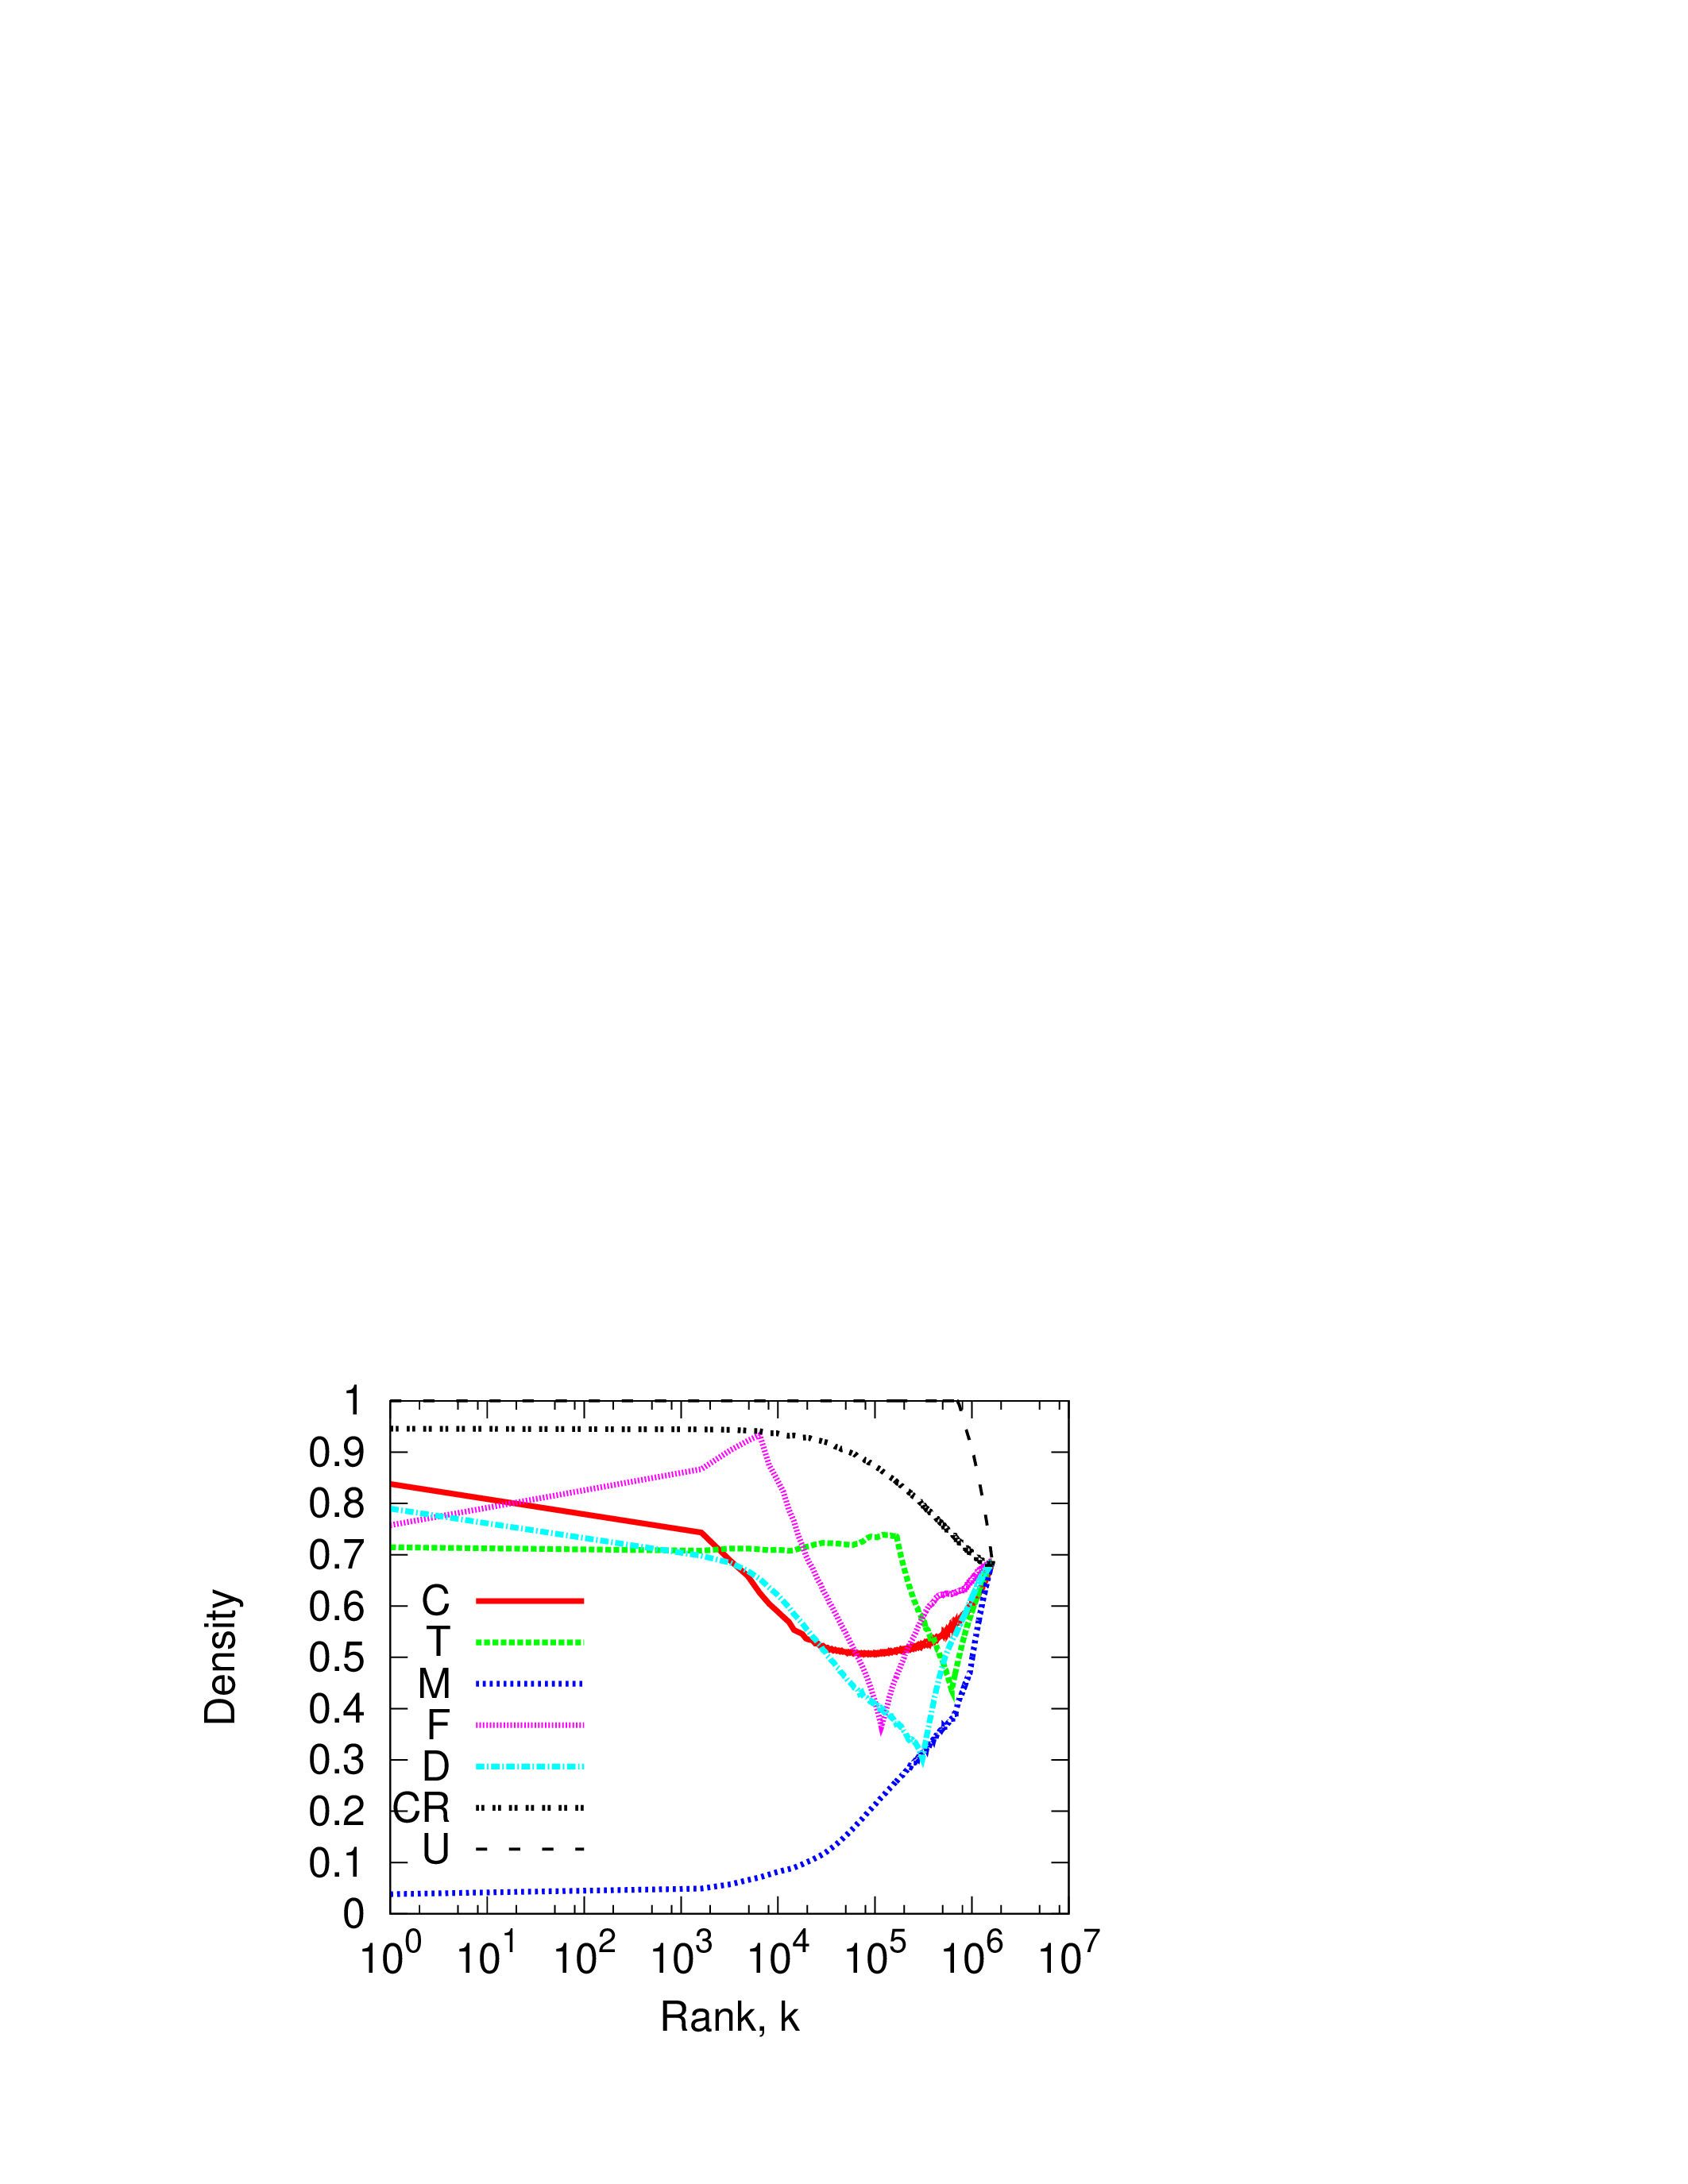}}
	\subfigure[Density	(Orkut)]{\includegraphics[width=0.15\textwidth]{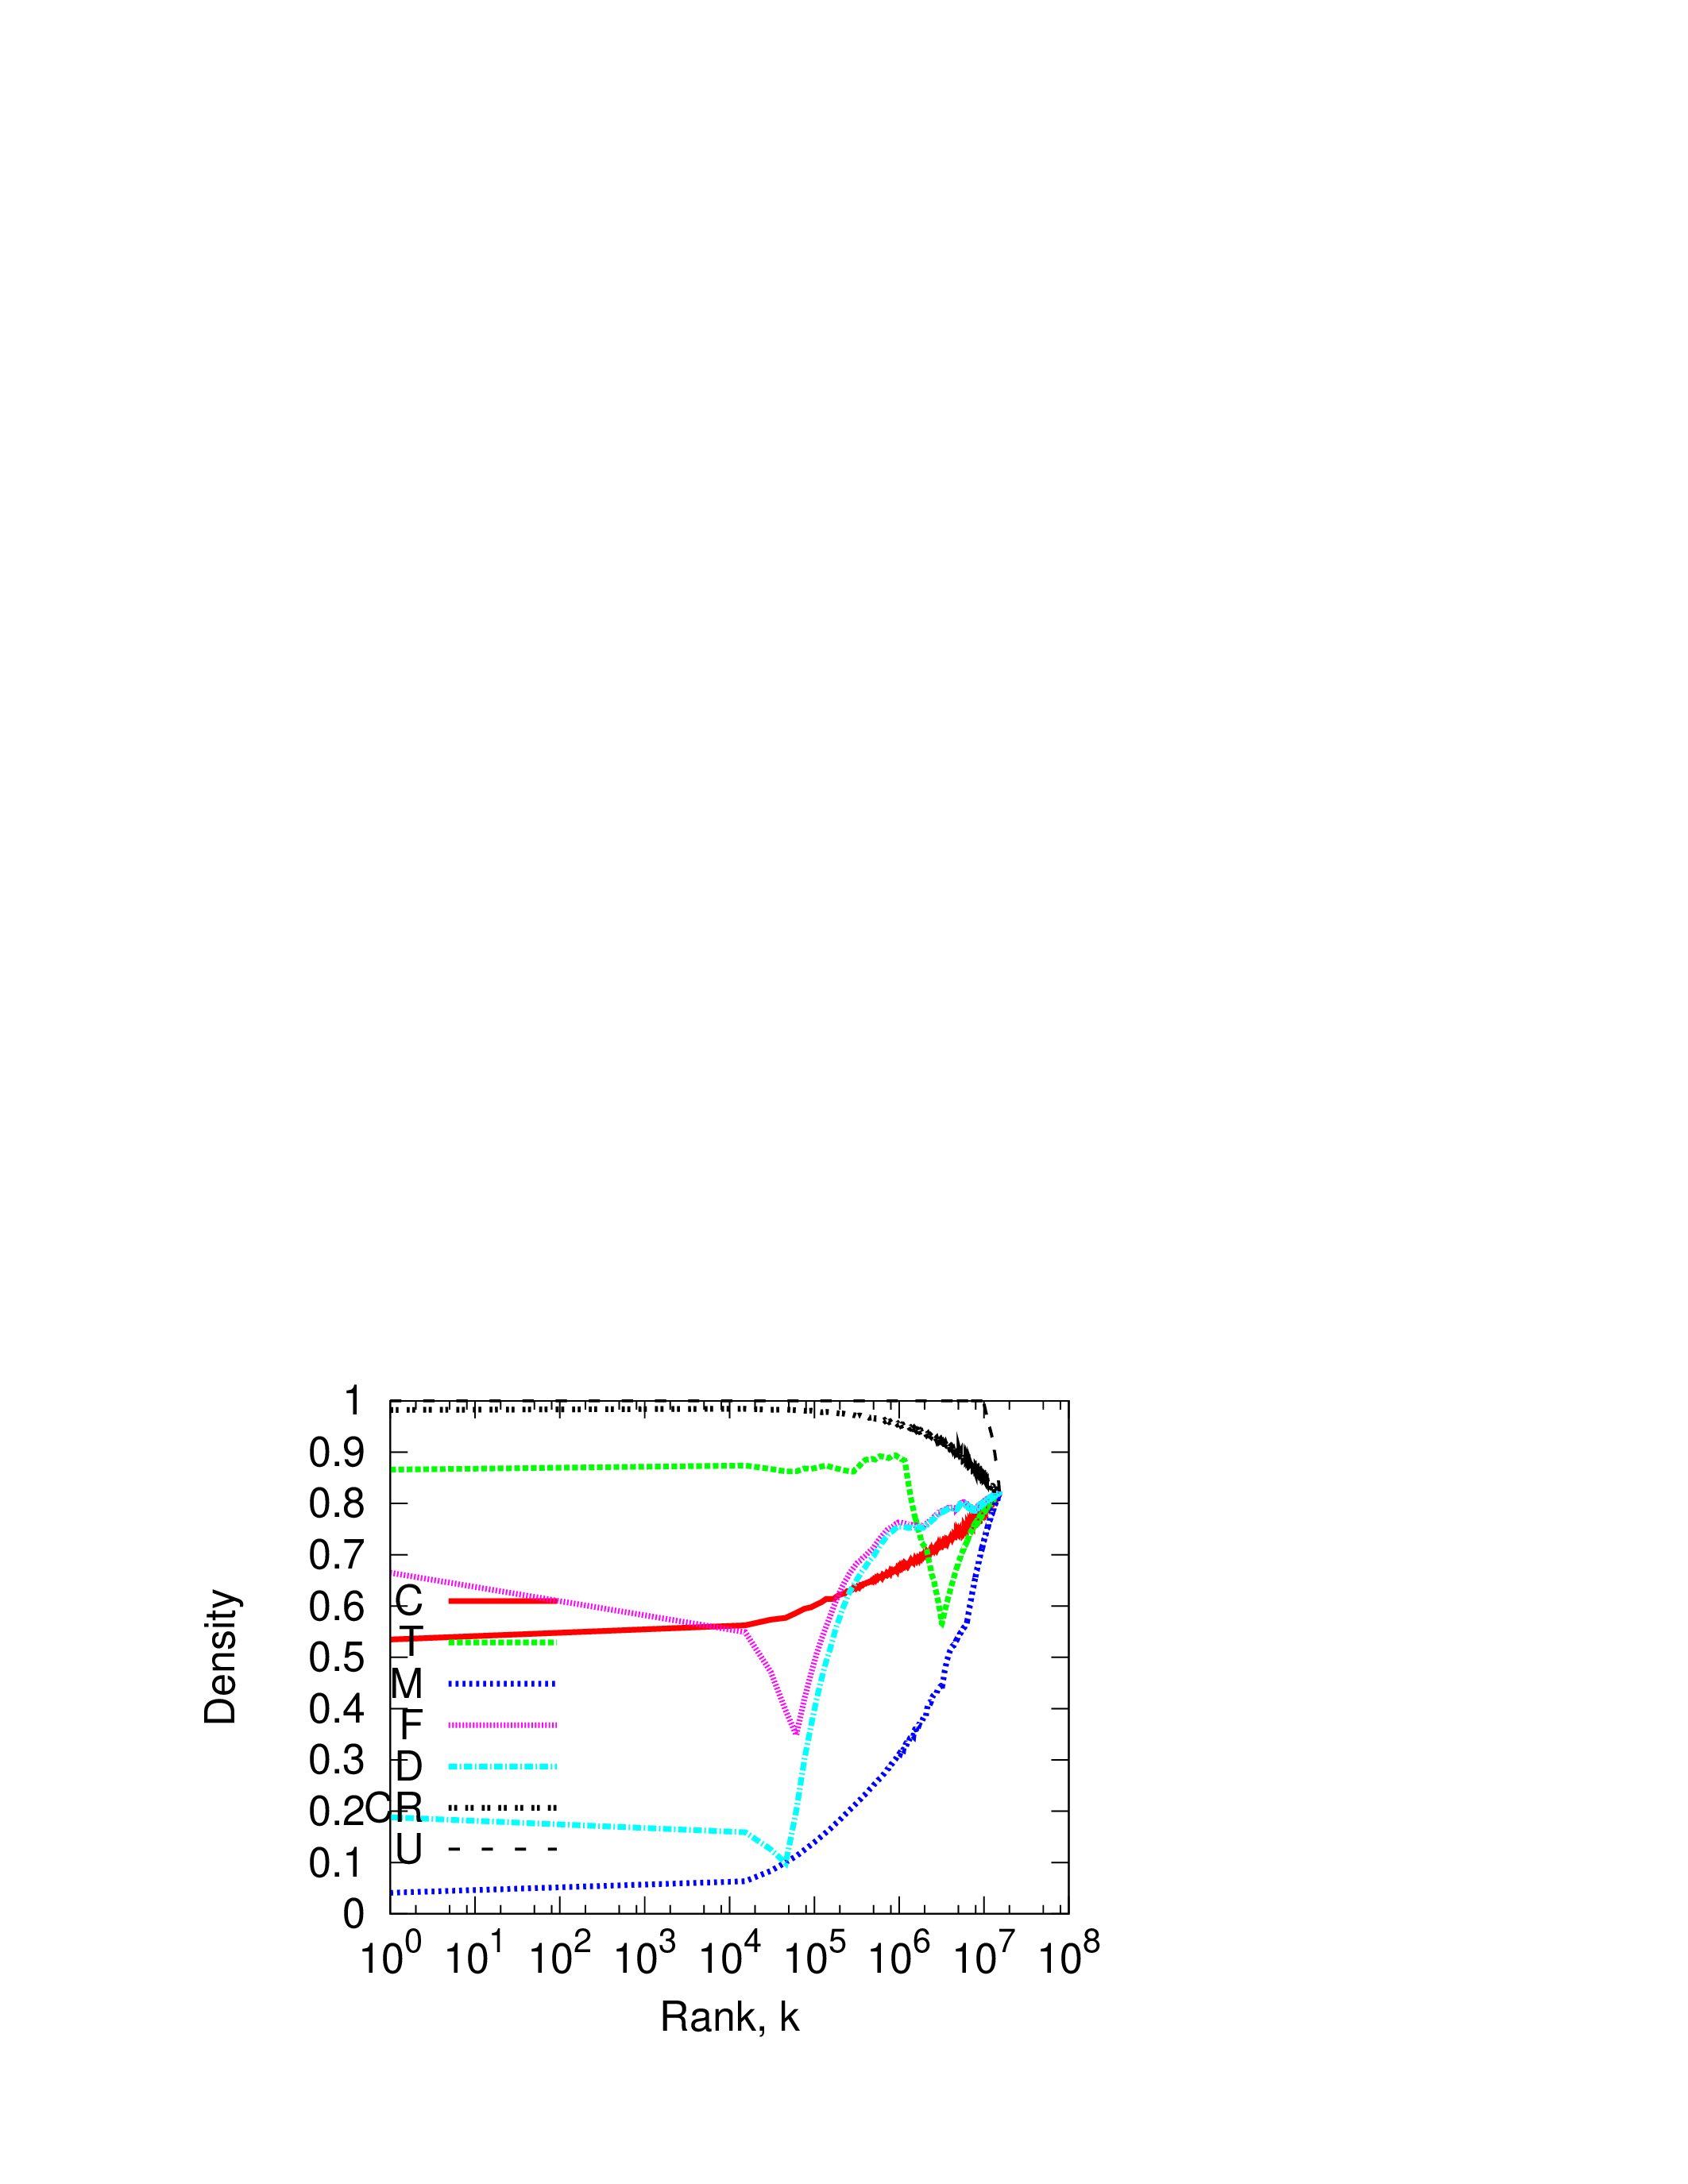}}
	\subfigure[Density	(Ning)]{\includegraphics[width=0.15\textwidth]{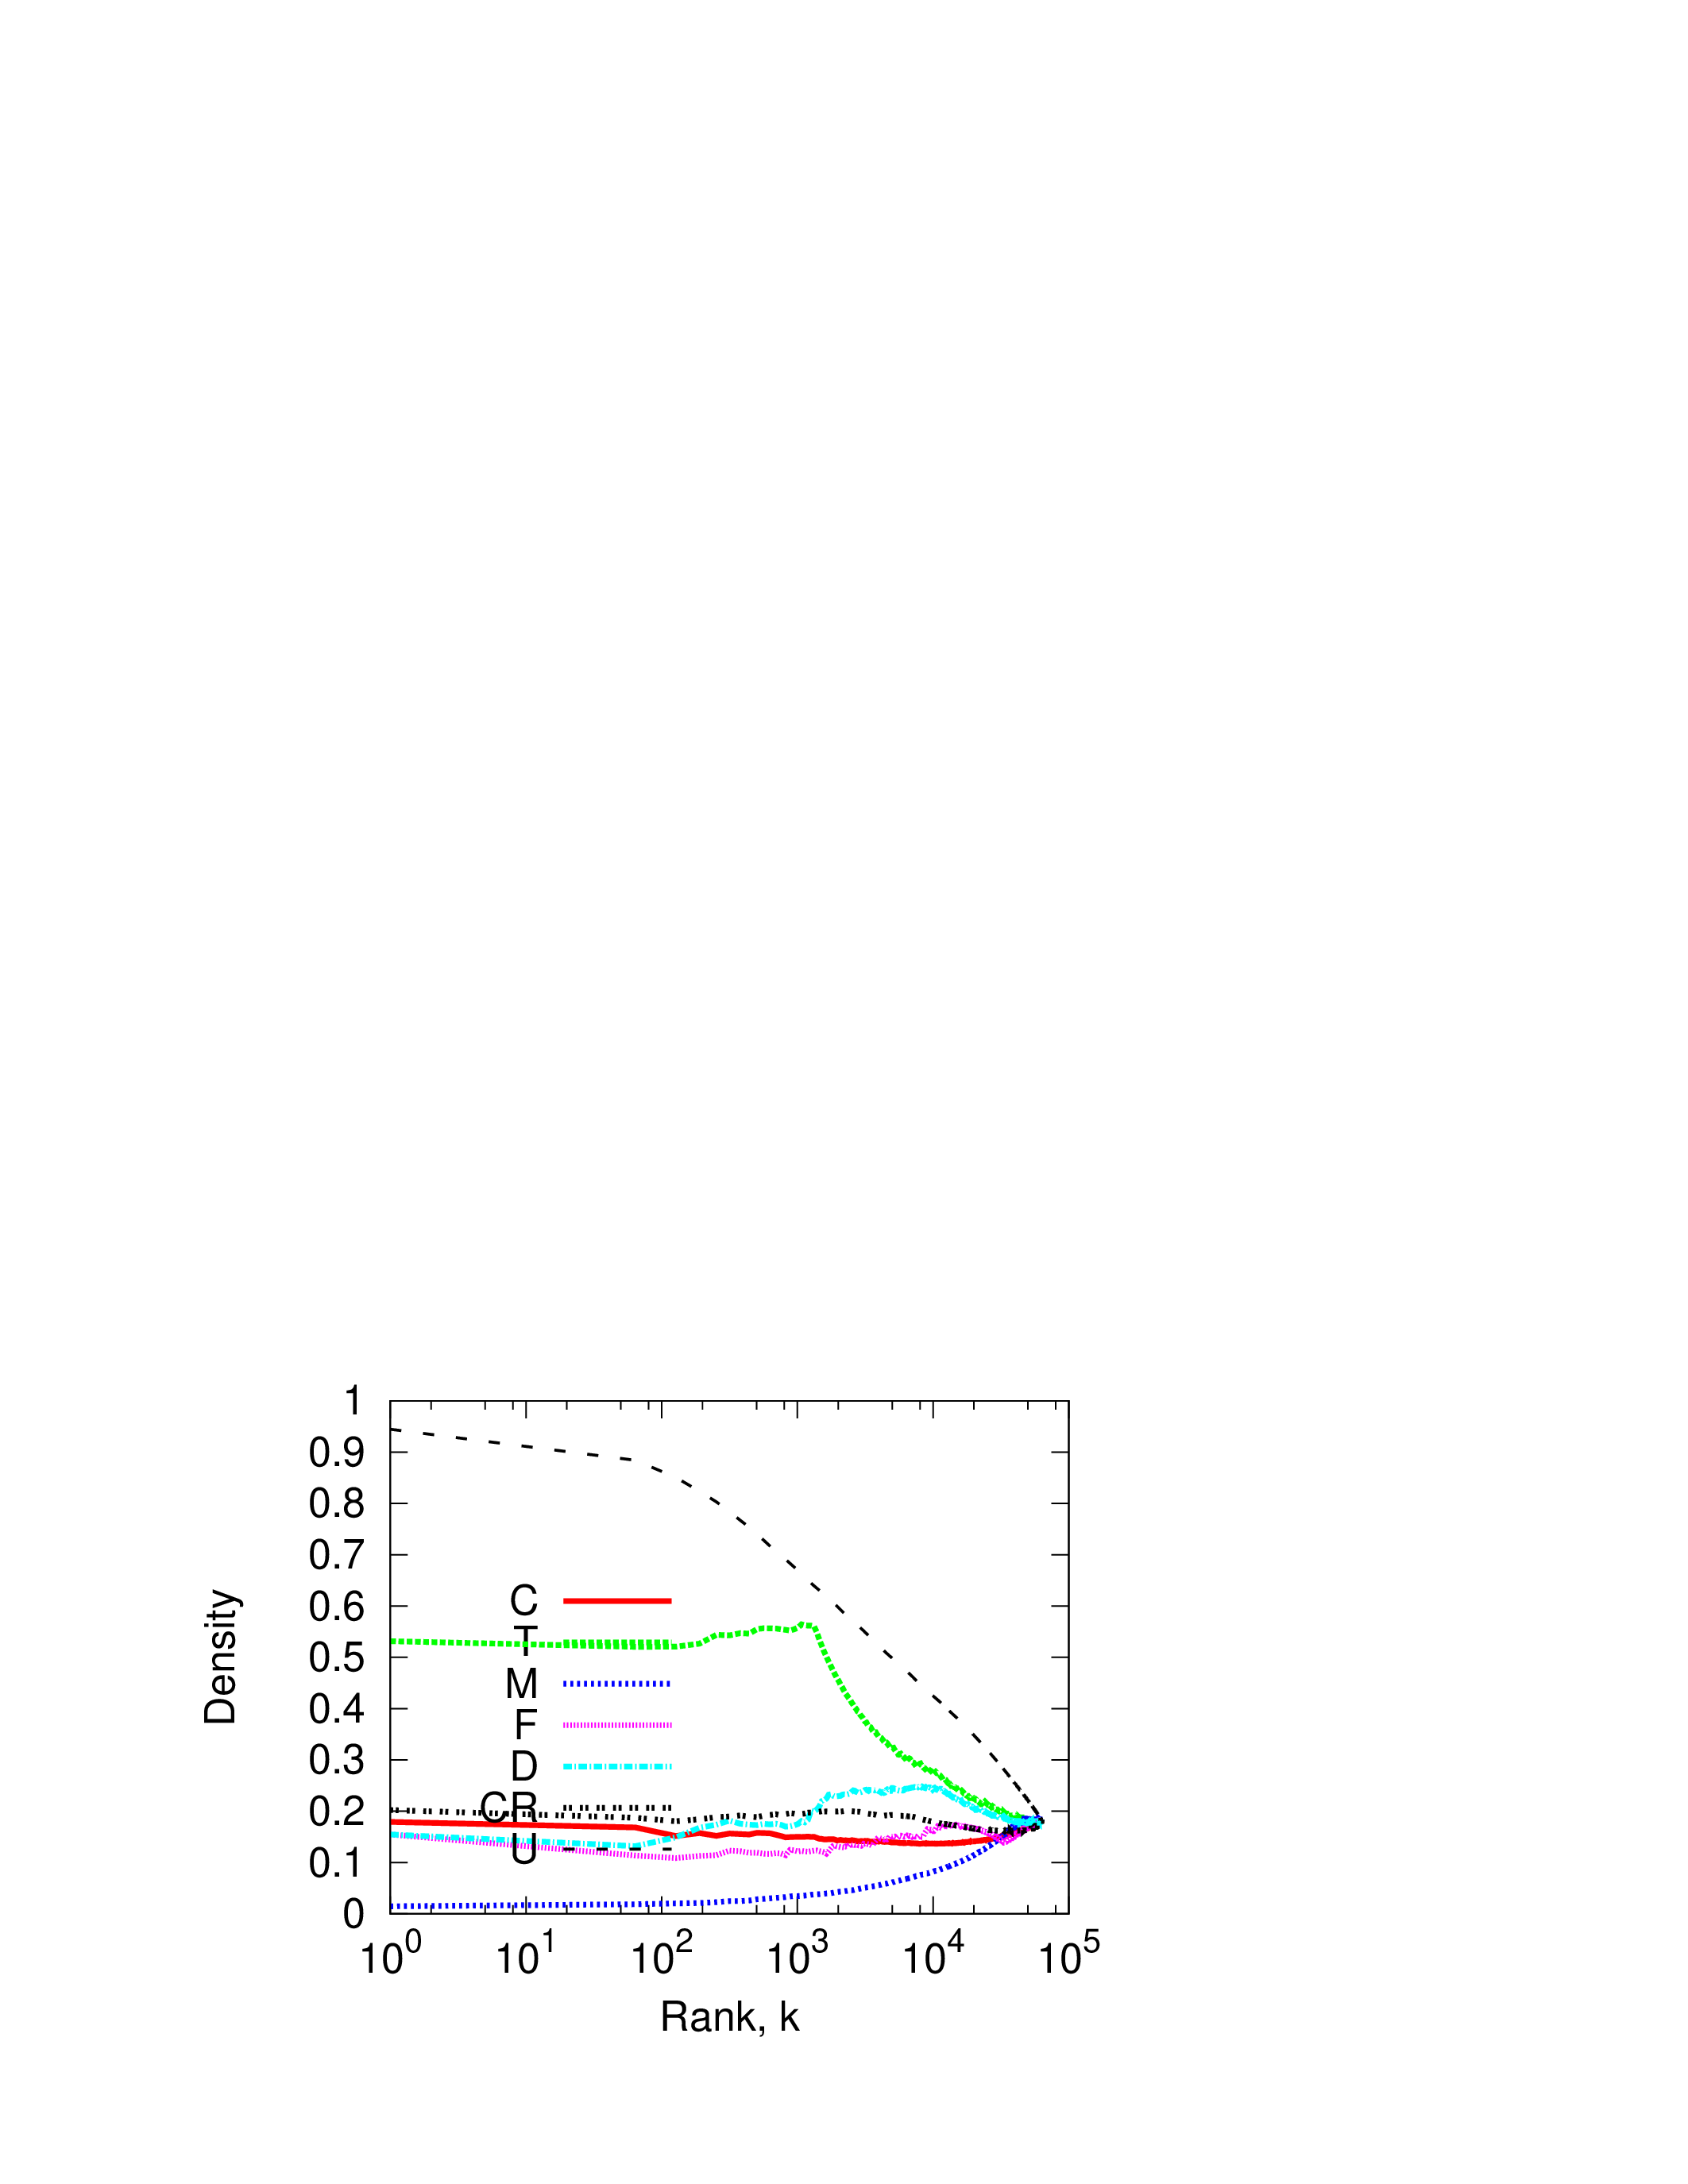}}
	\subfigure[Density	(Amazon)]{\includegraphics[width=0.15\textwidth]{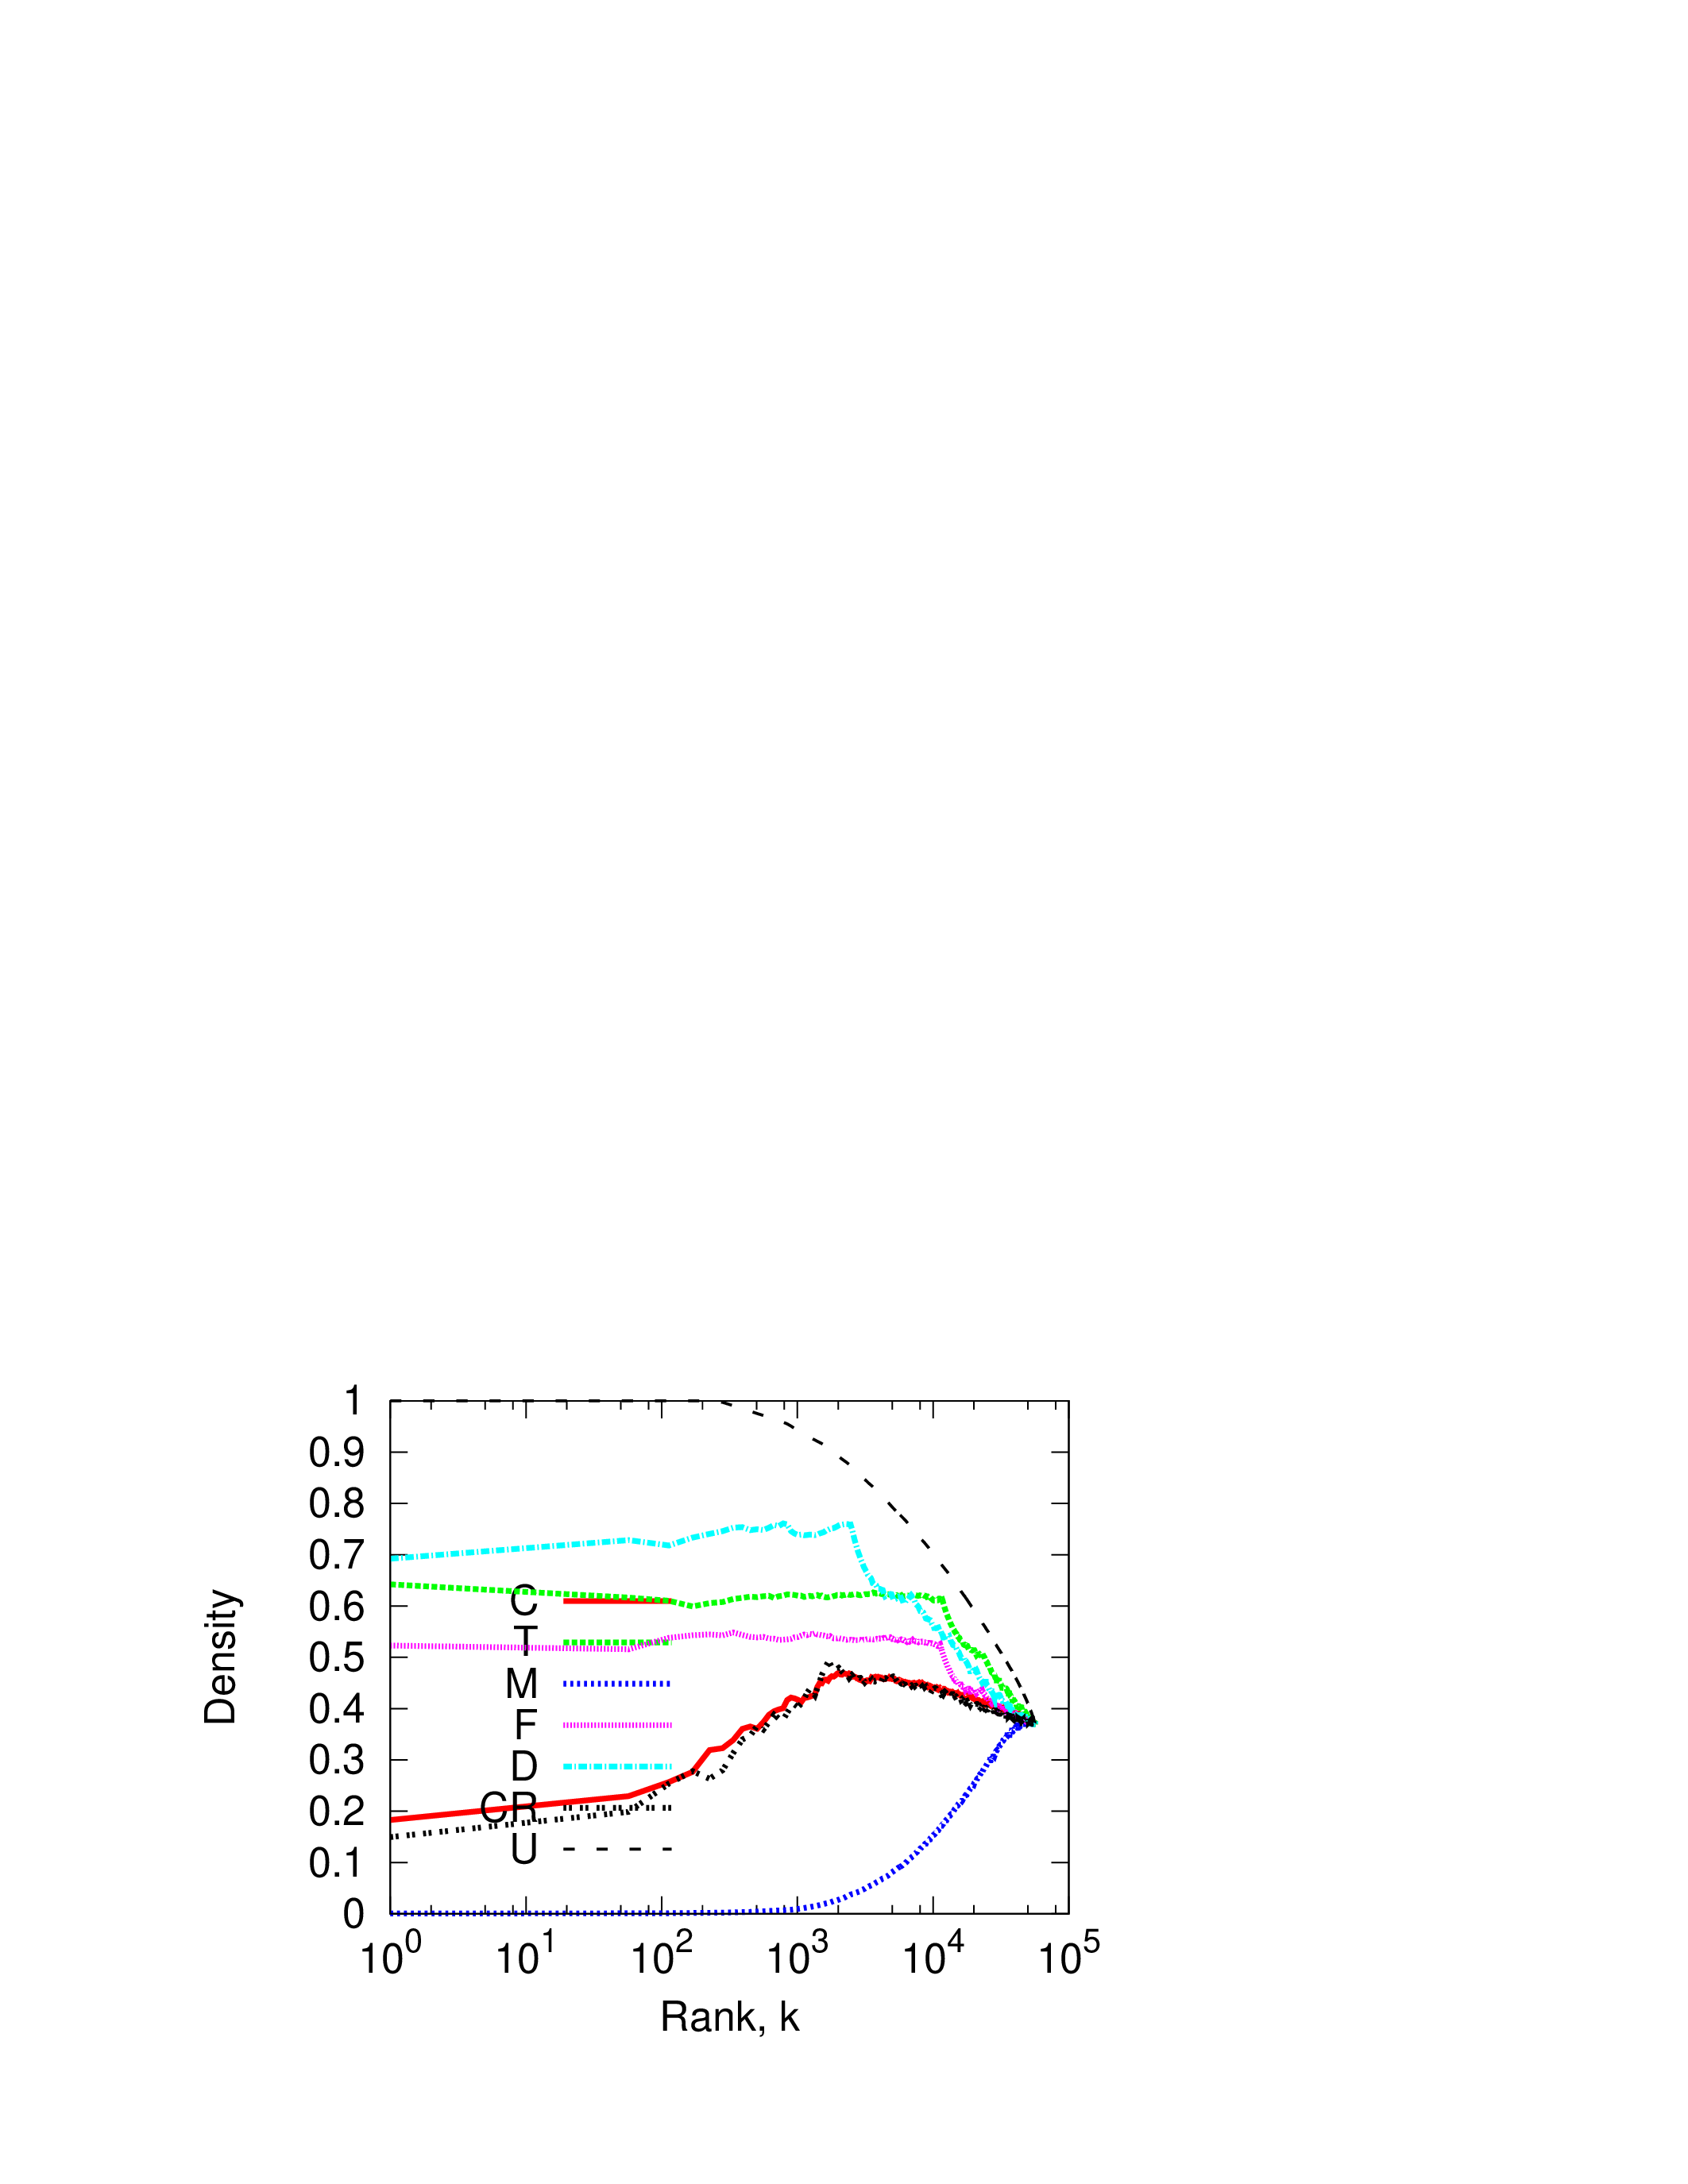}}
	\subfigure[Density	(DBLP)]{\includegraphics[width=0.15\textwidth]{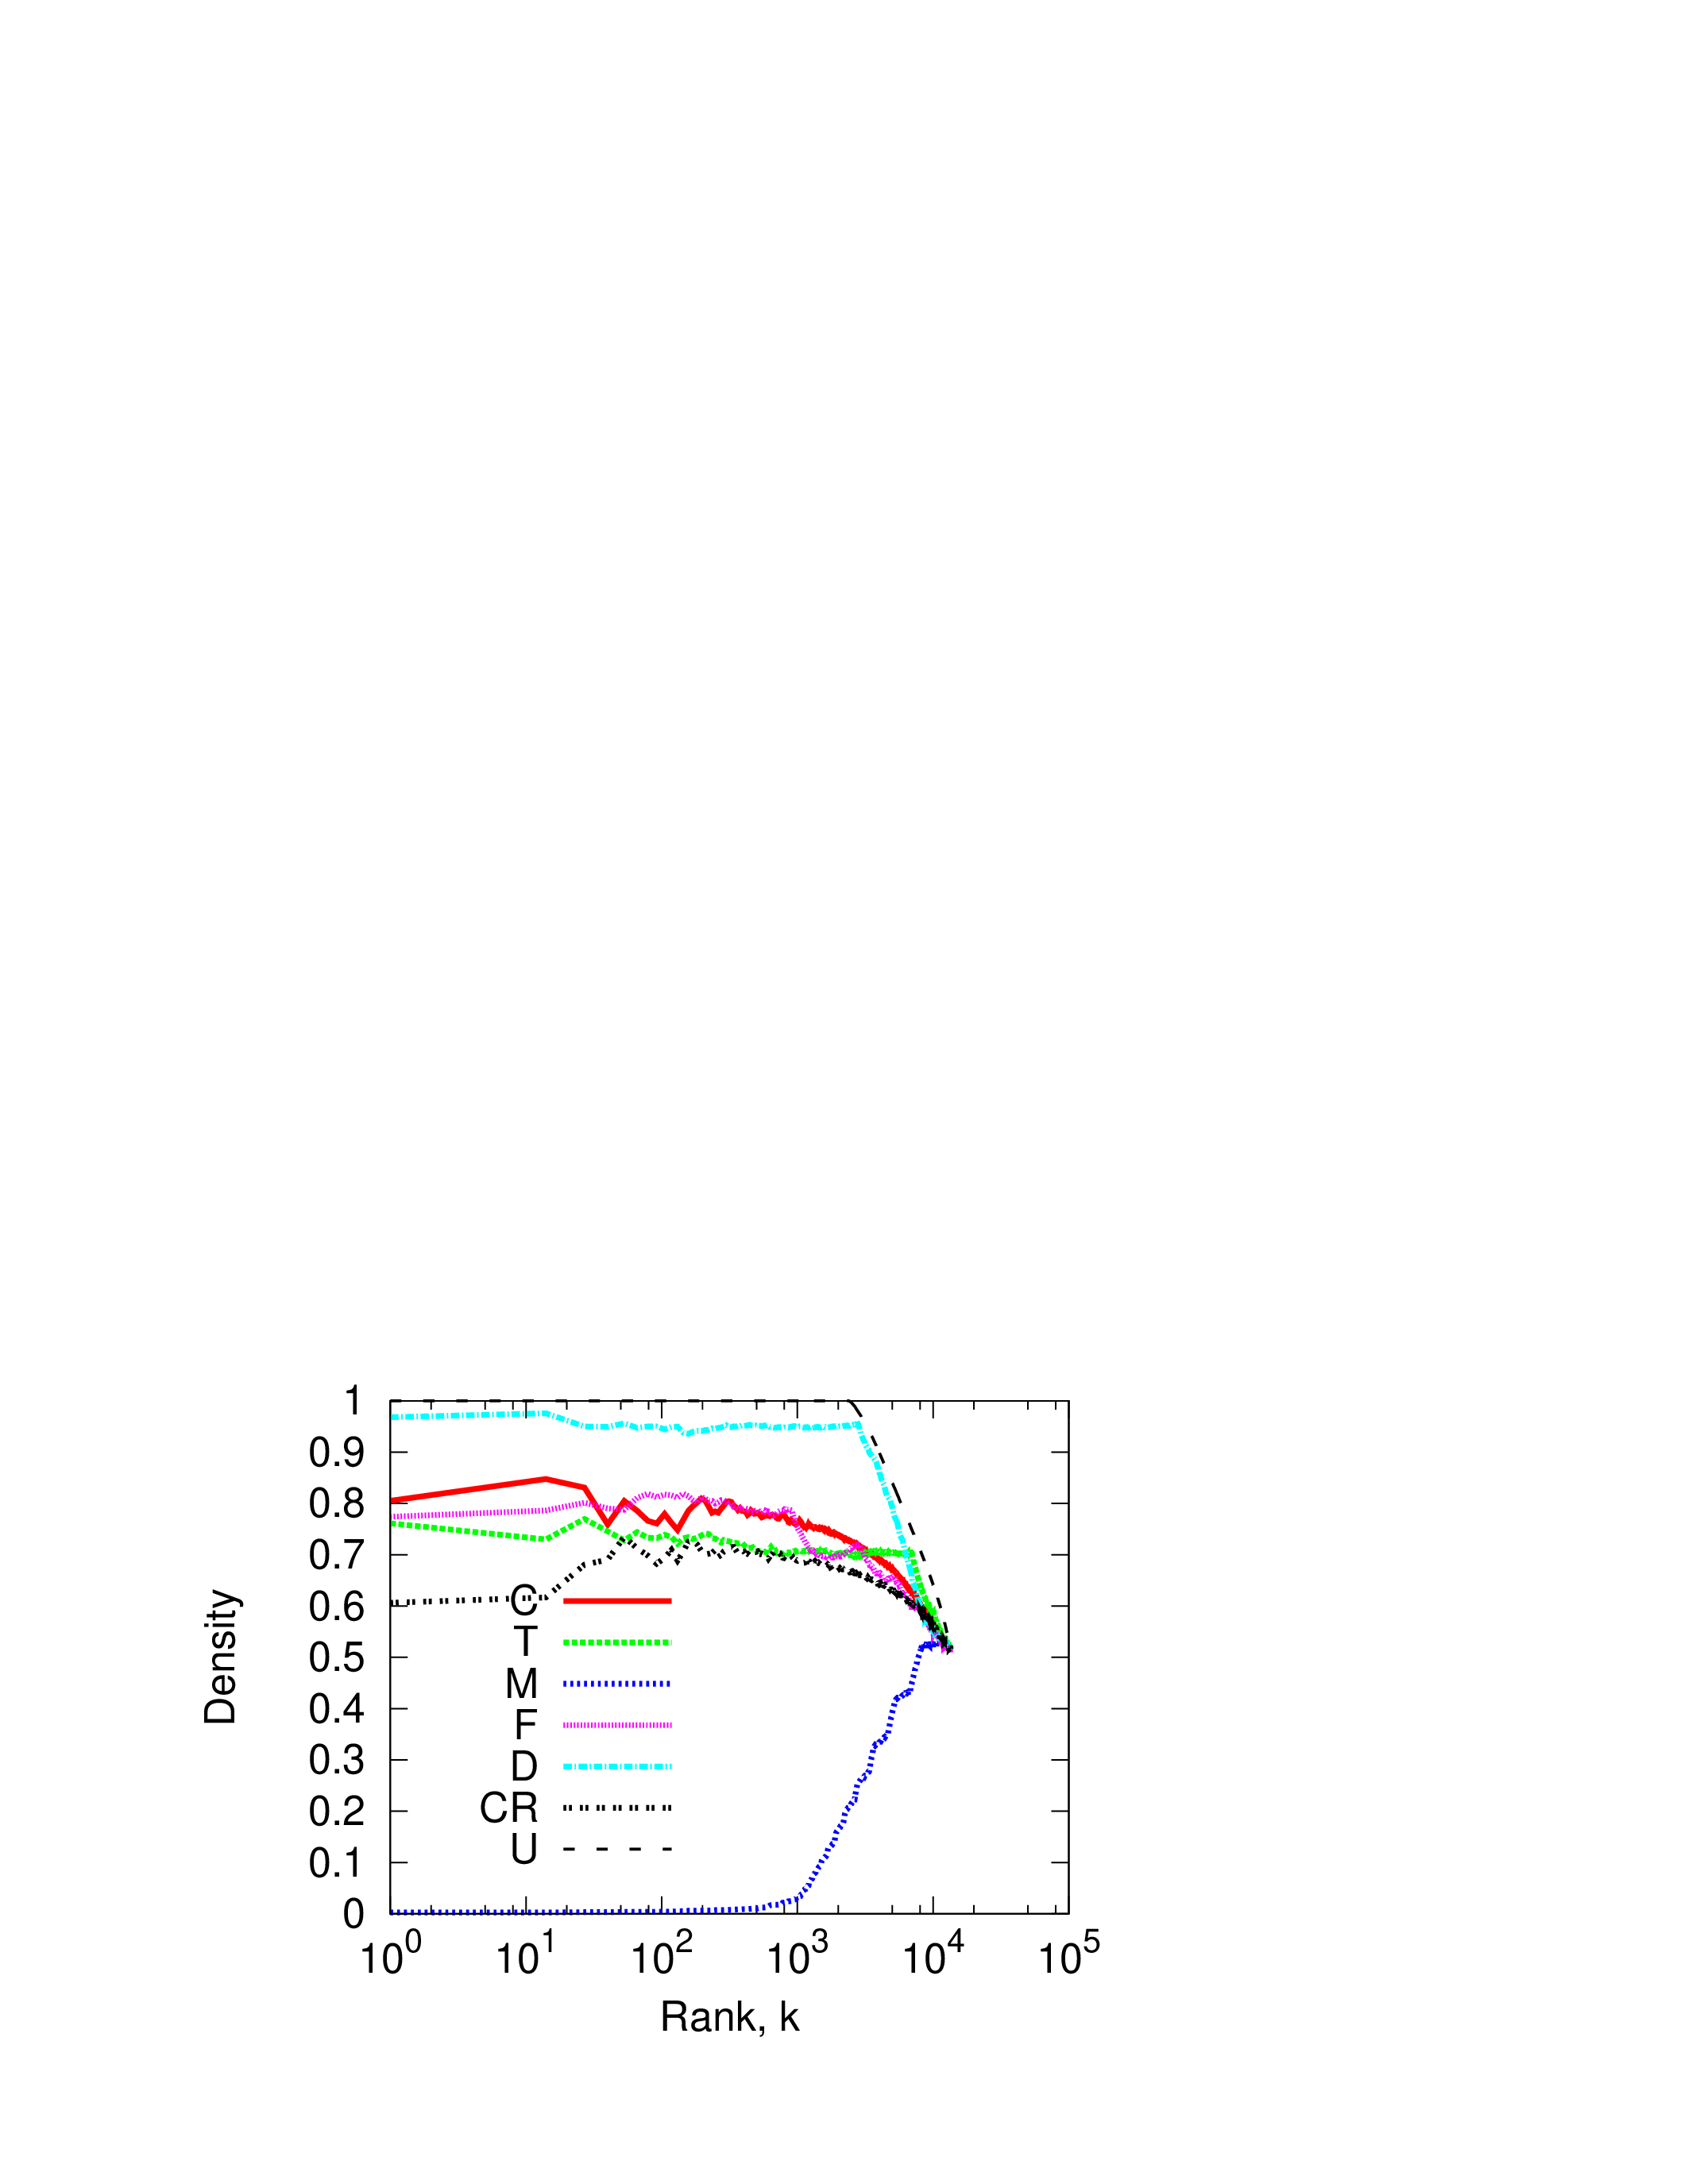}}
	\subfigure[Coh.	 (LJ)]{\includegraphics[width=0.15\textwidth]{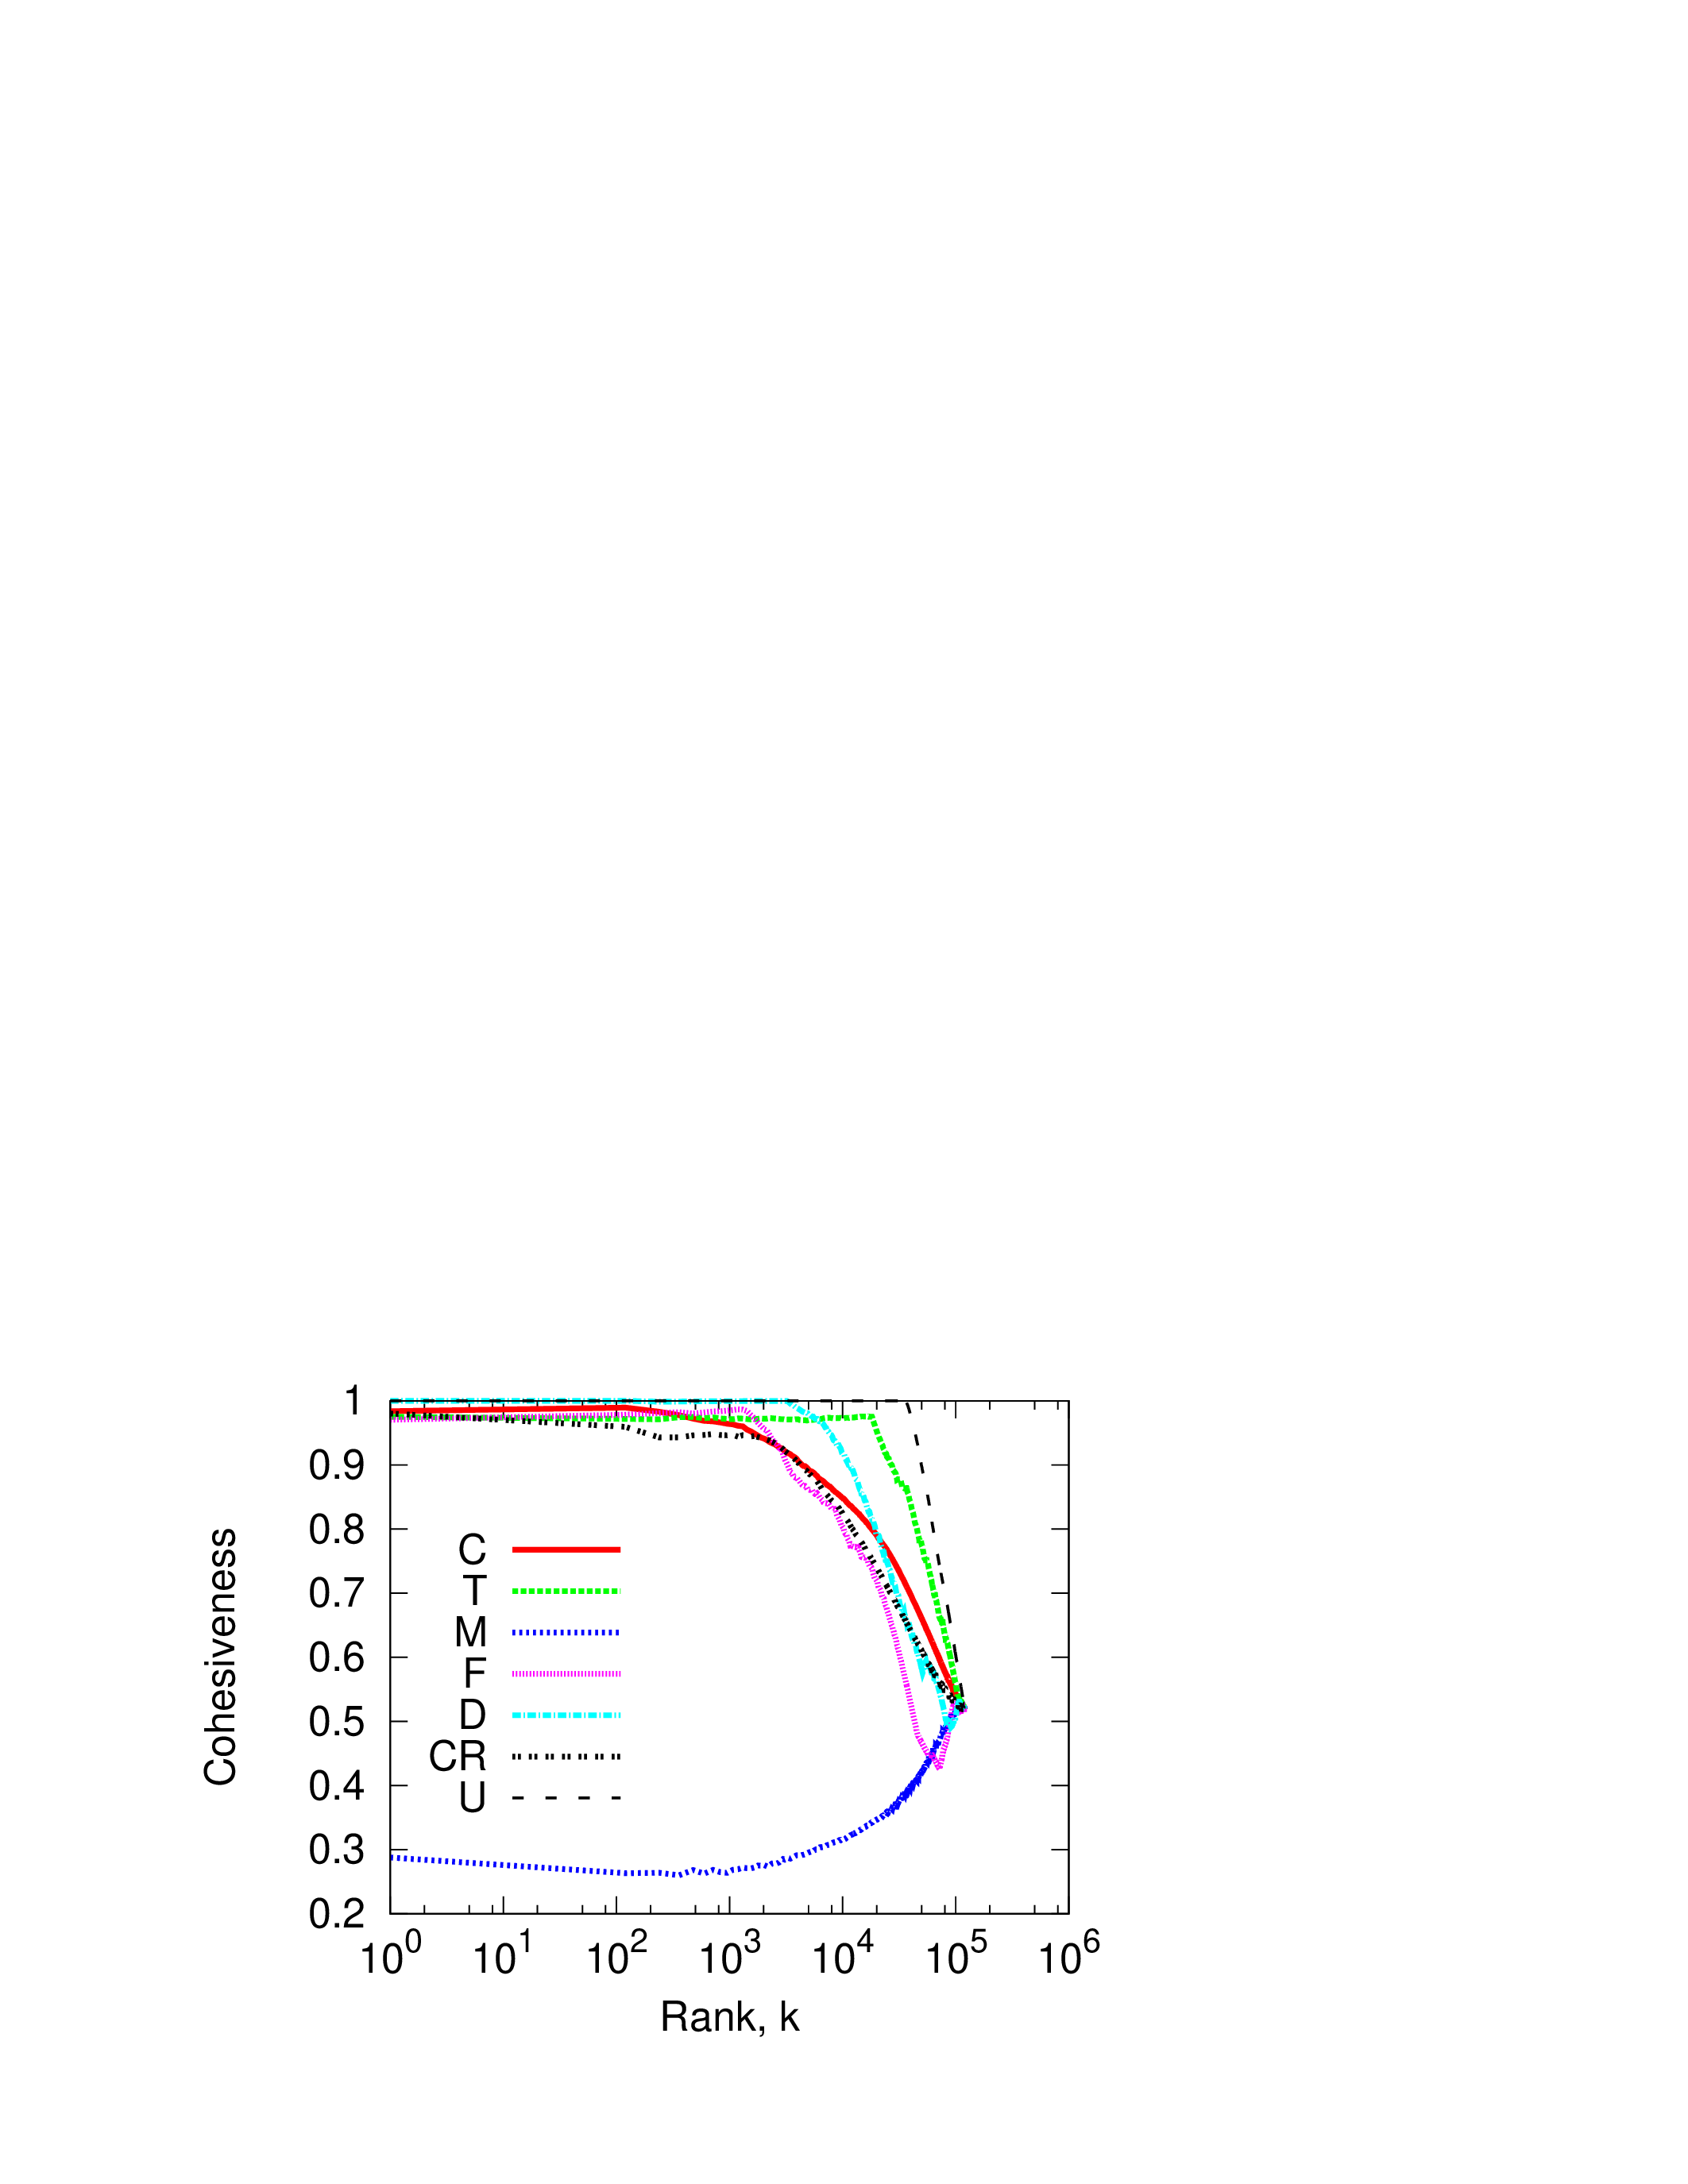}}
	\subfigure[Coh.	 (FS)]{\includegraphics[width=0.15\textwidth]{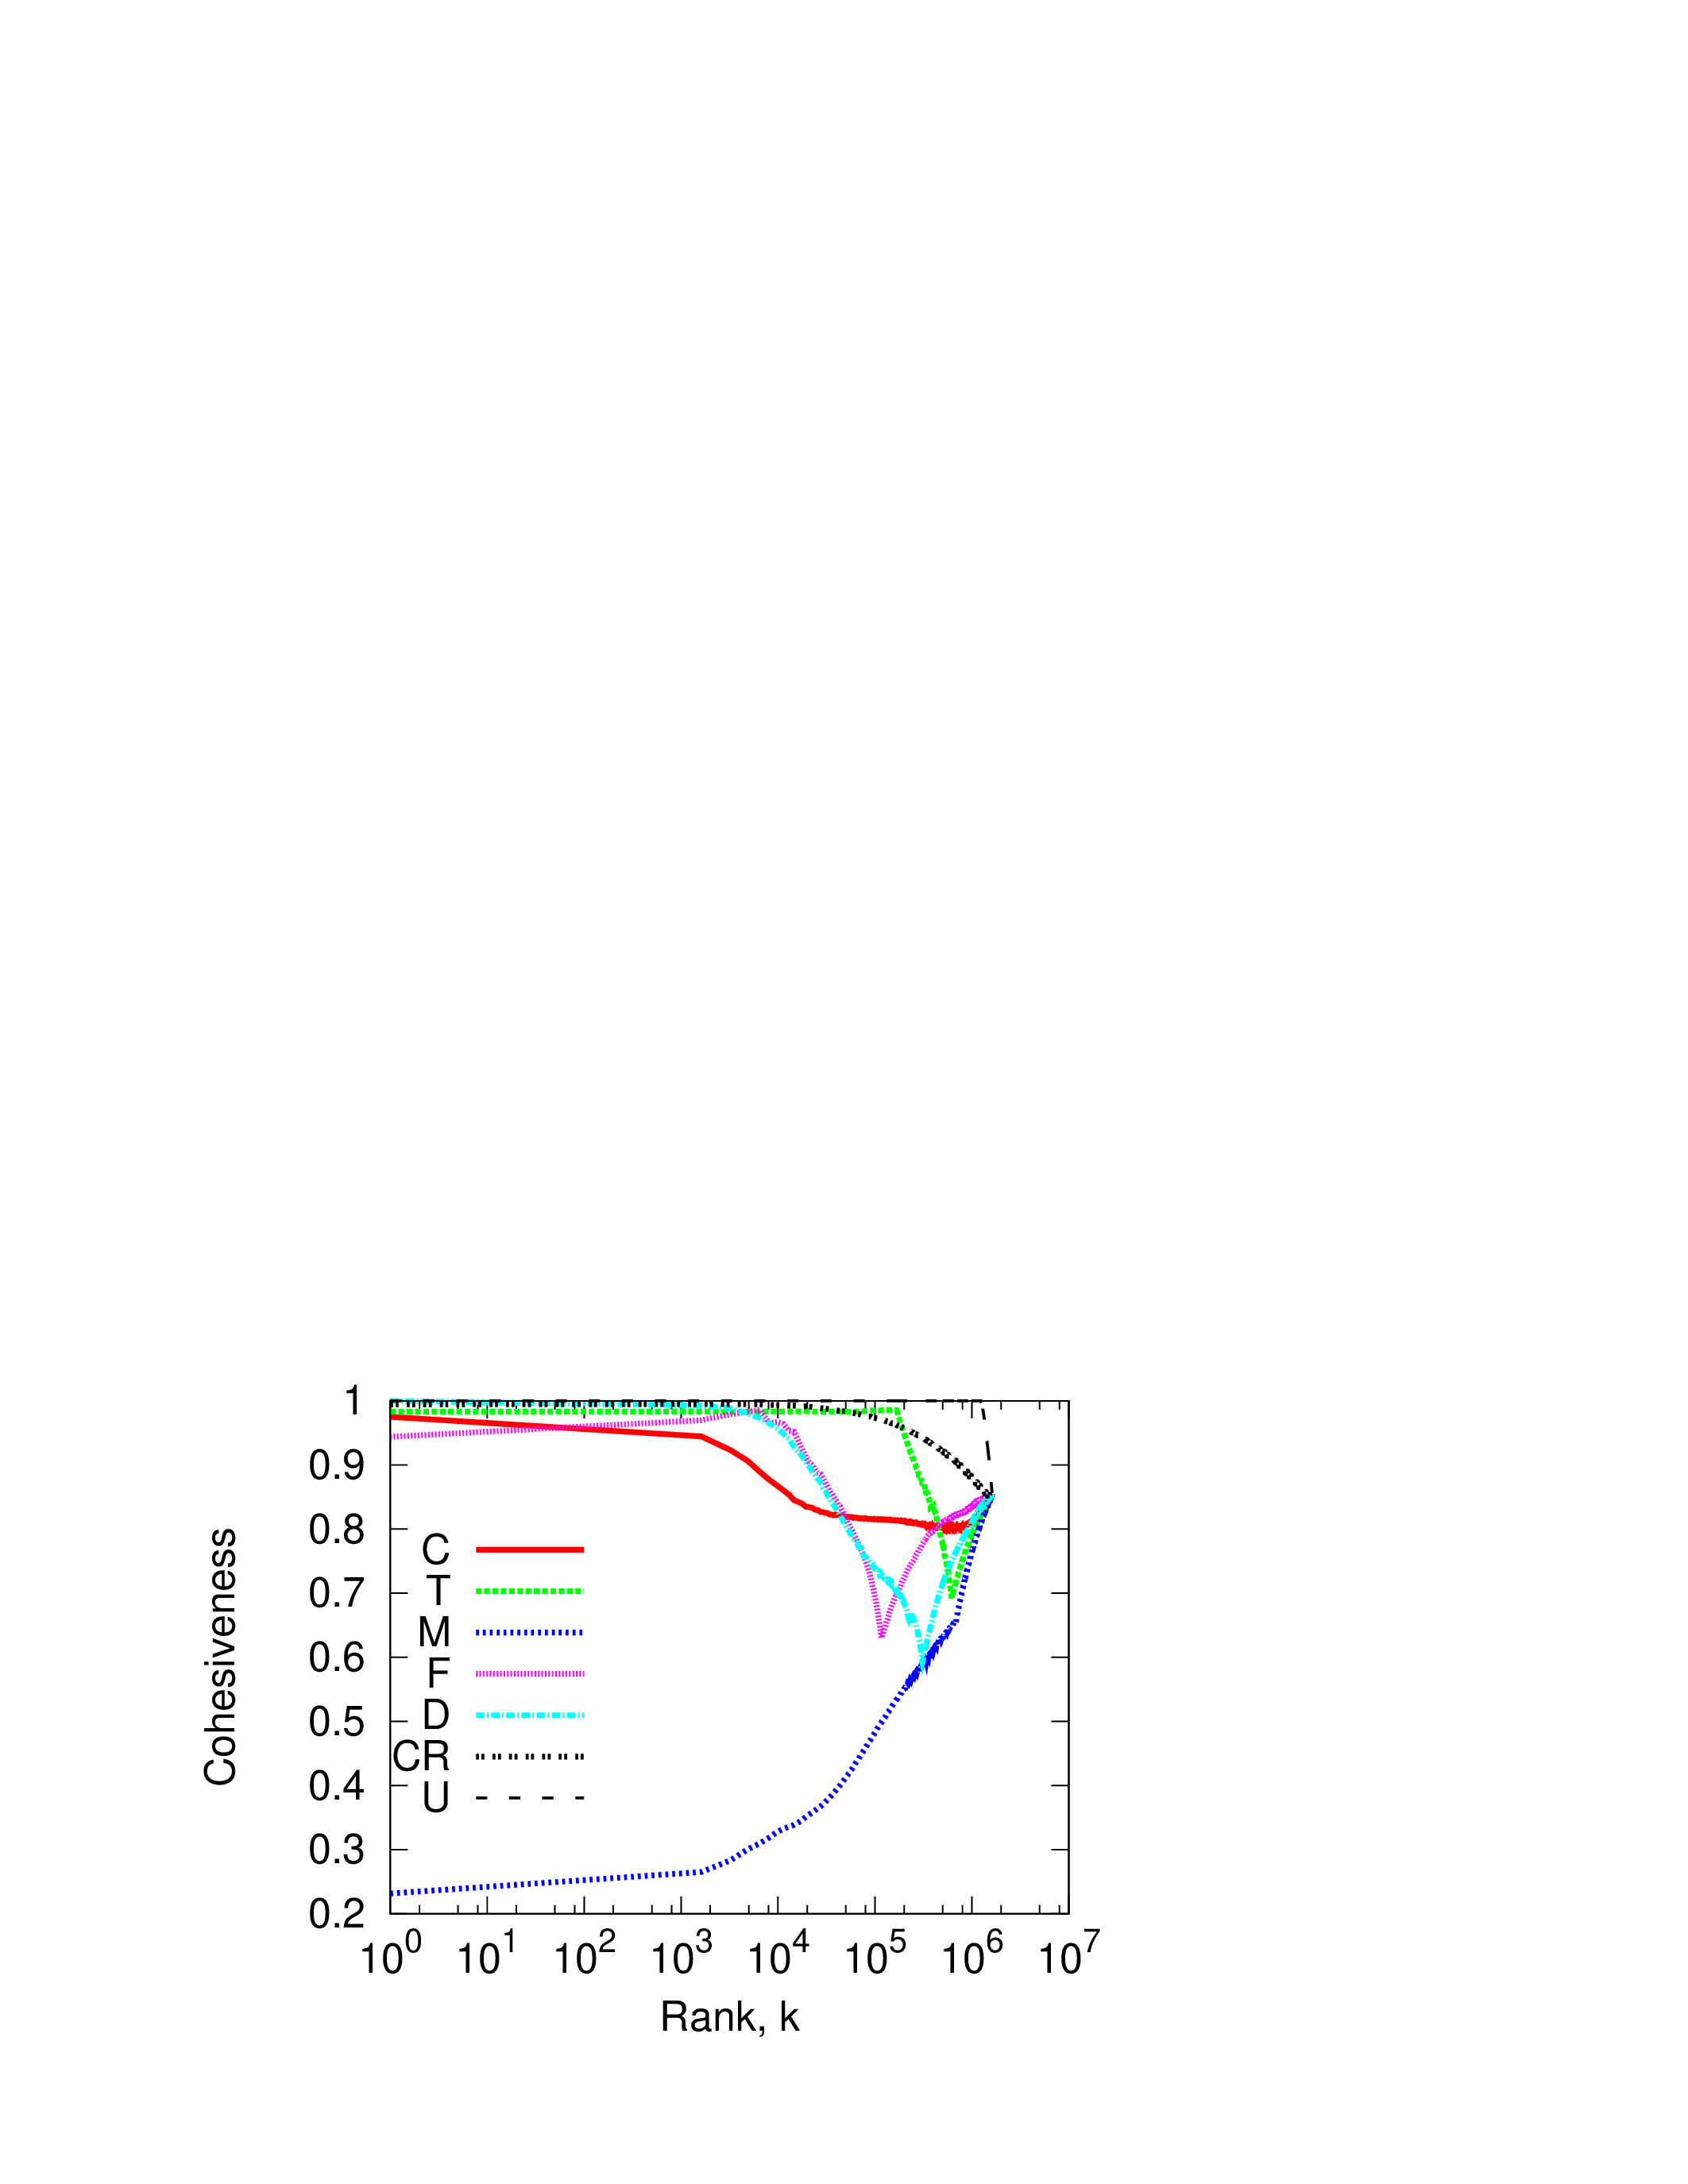}}
	\subfigure[Coh.	(Orkut)]{\includegraphics[width=0.15\textwidth]{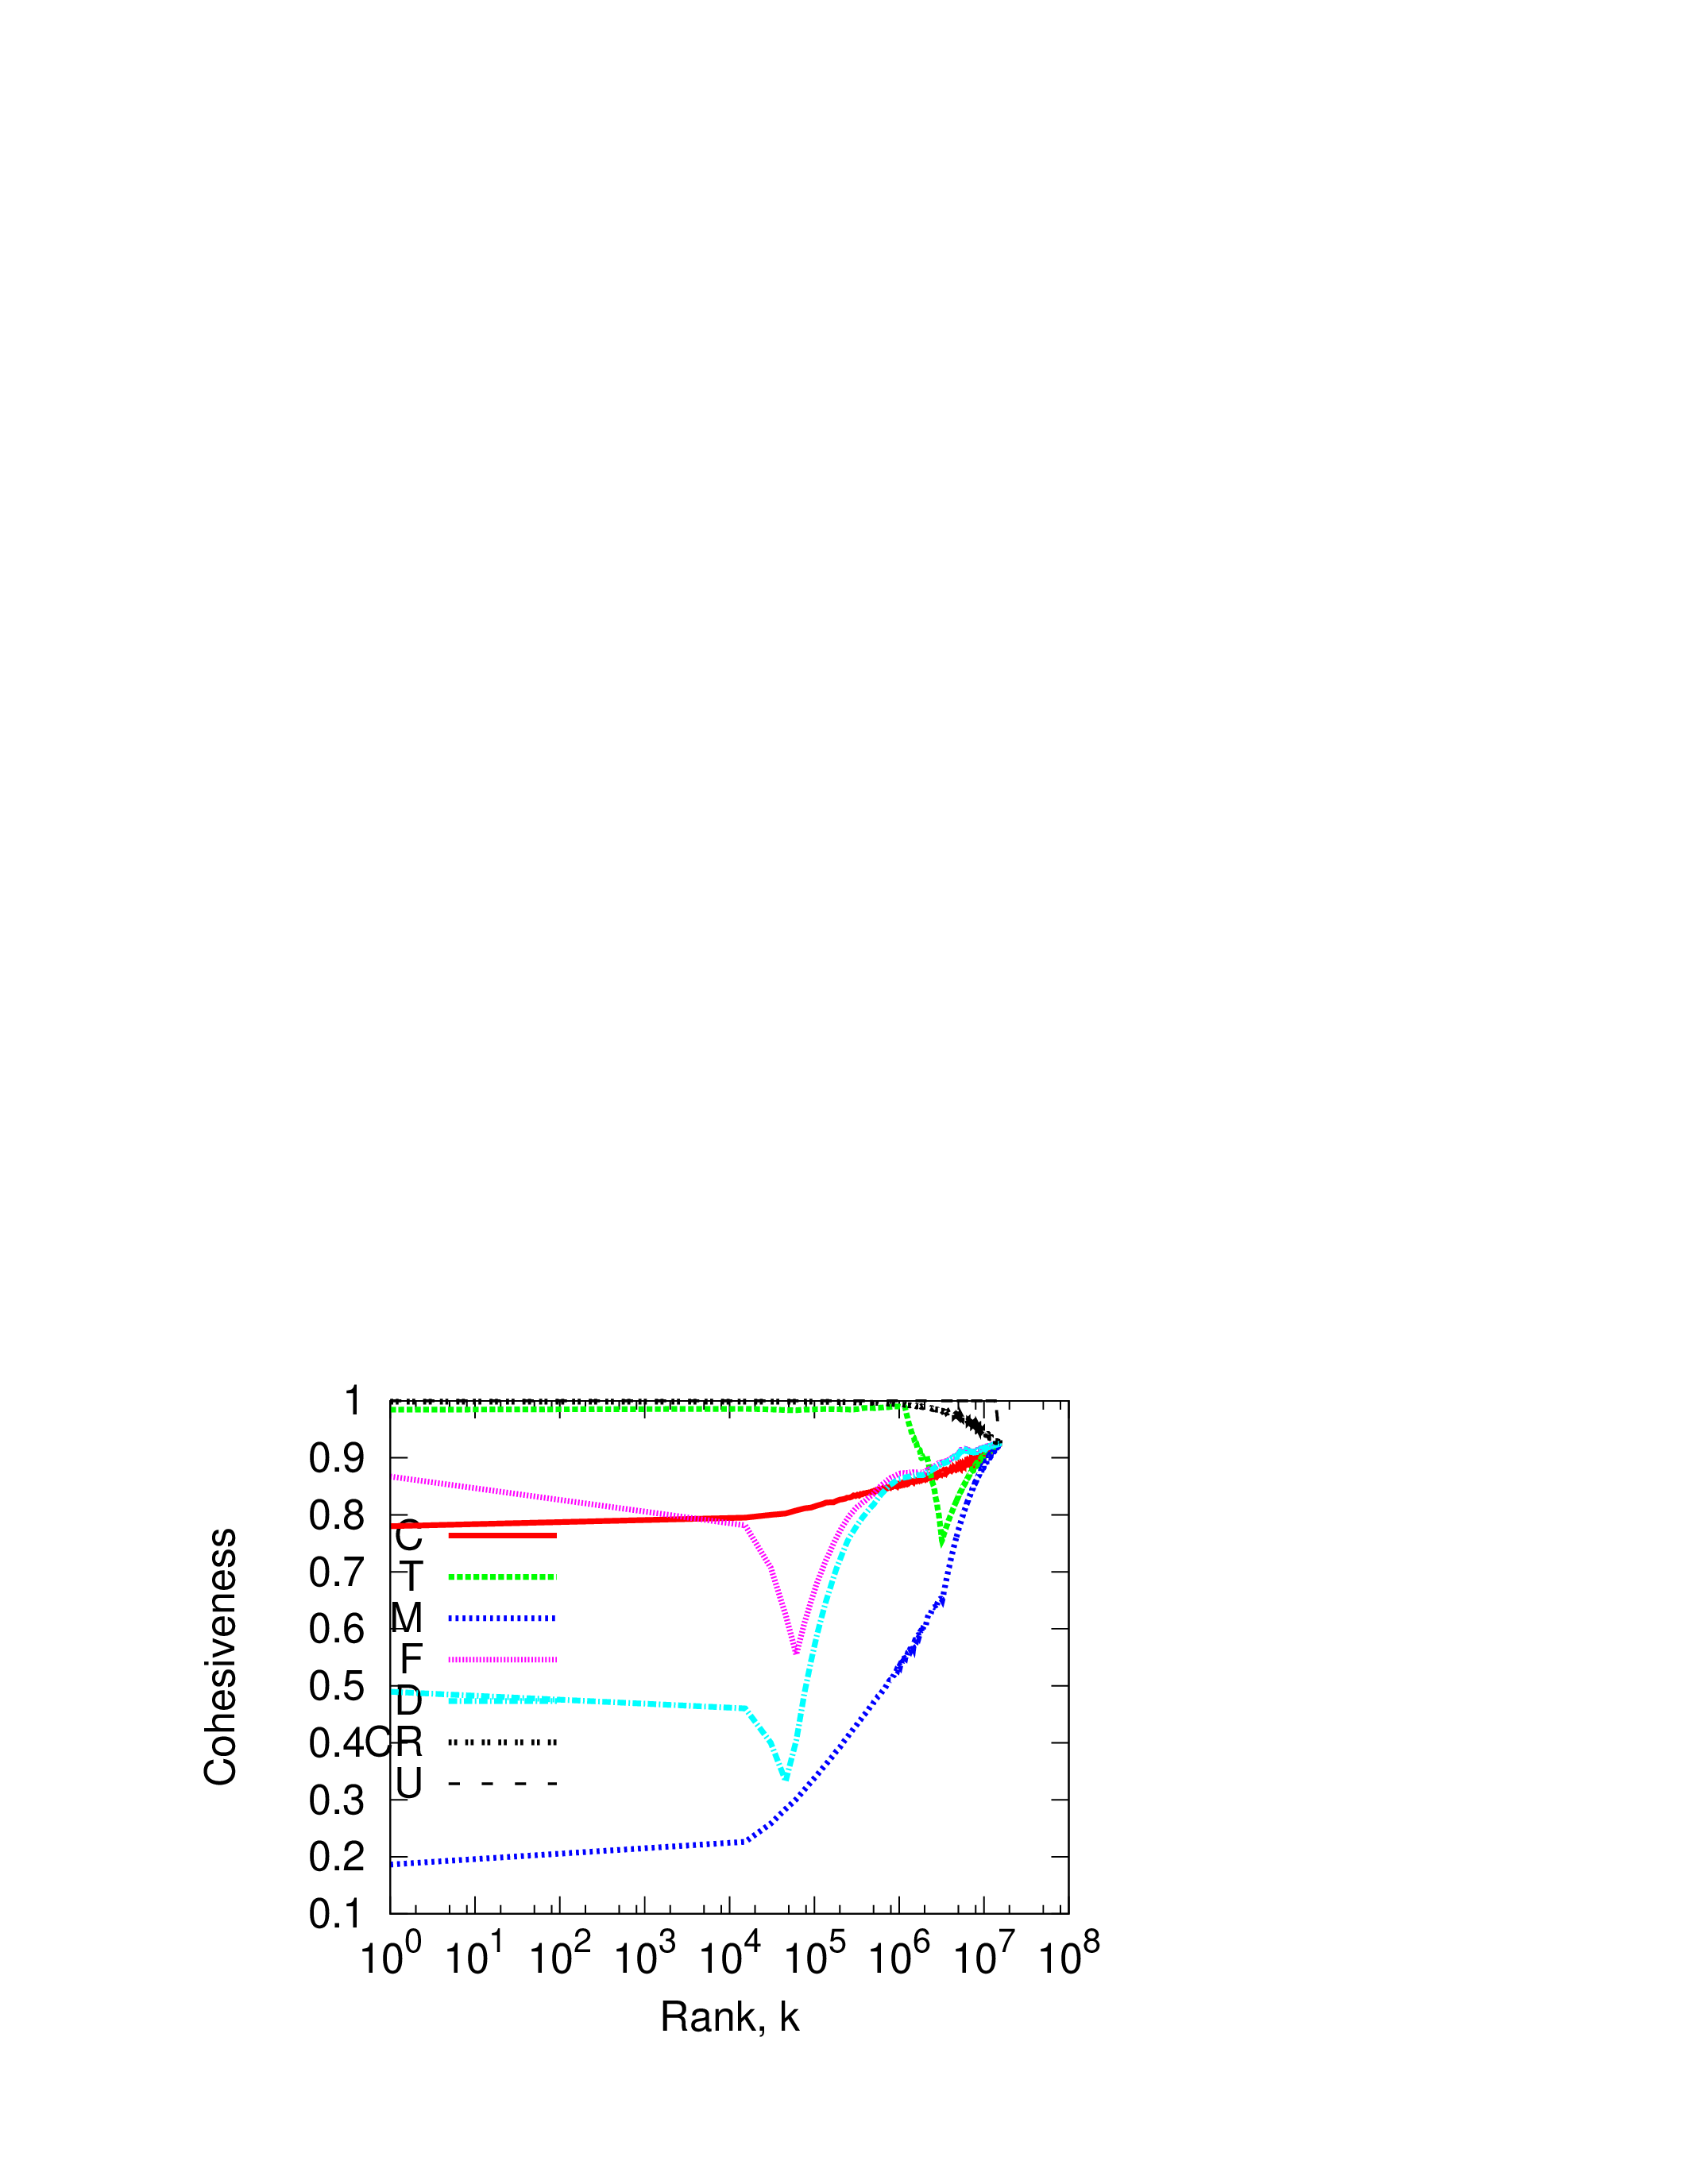}}
	\subfigure[Coh.	(Ning)]{\includegraphics[width=0.15\textwidth]{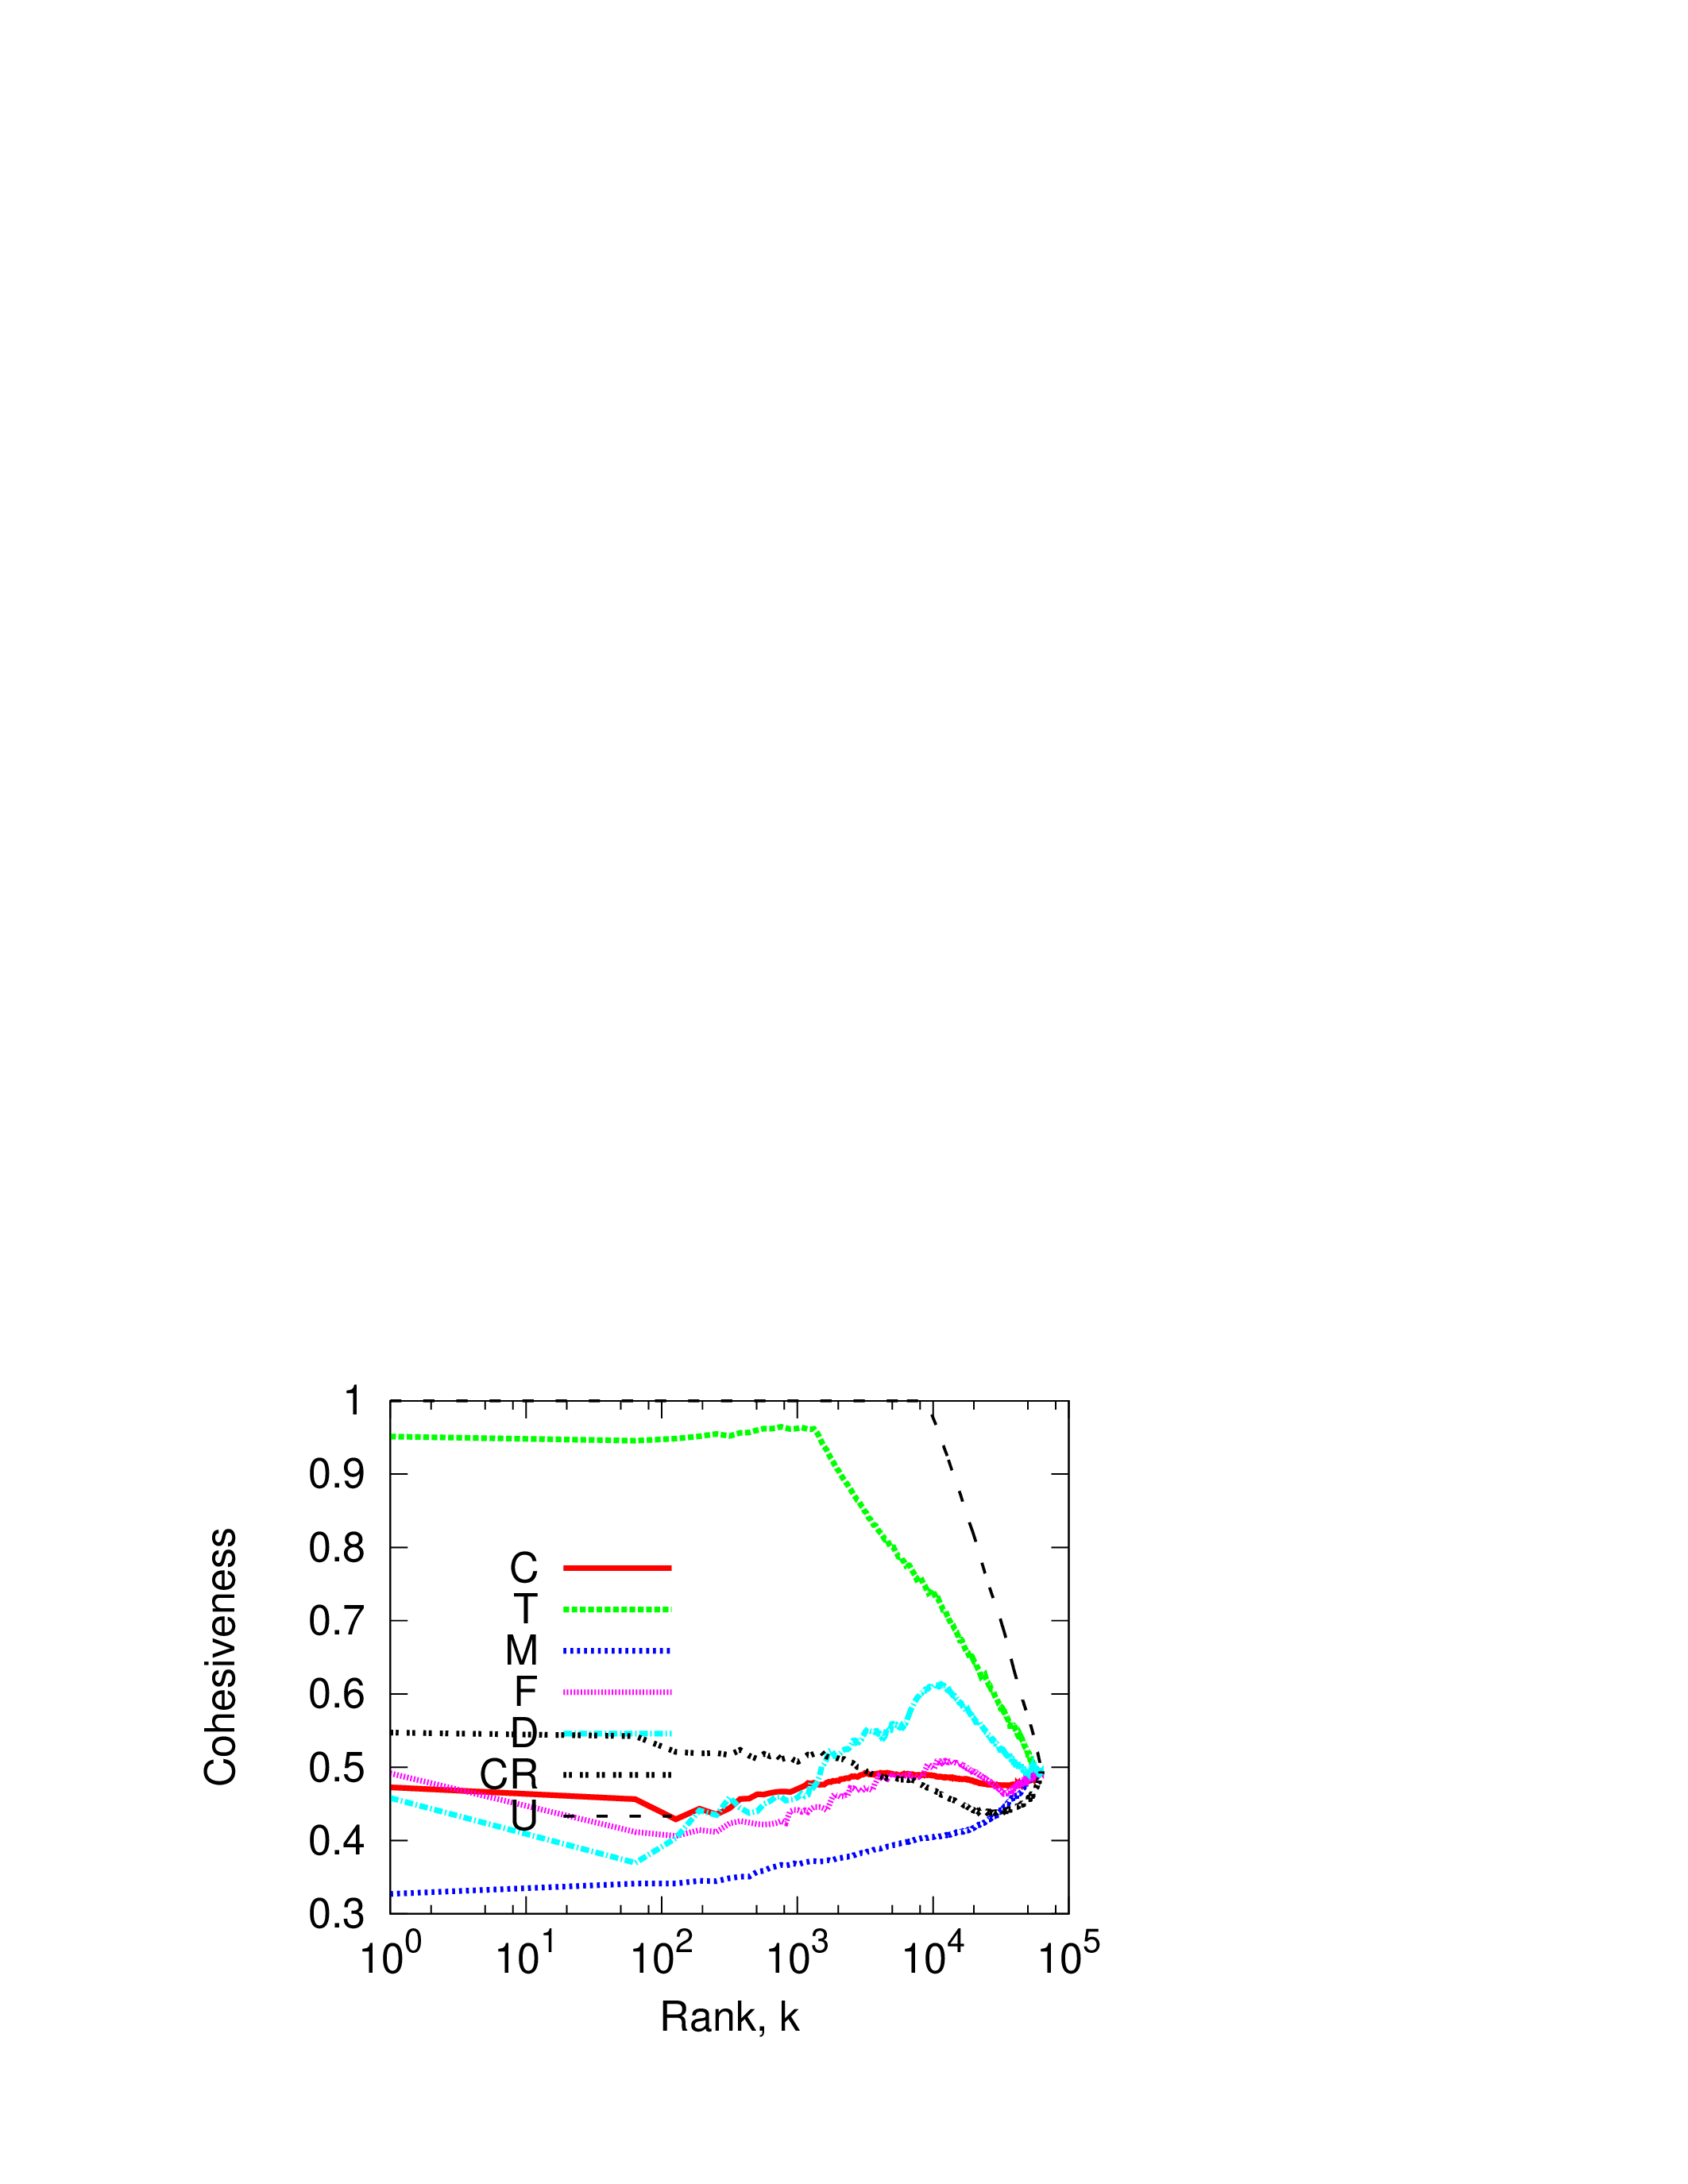}}
	\subfigure[Coh.	 (Amazon)]{\includegraphics[width=0.15\textwidth]{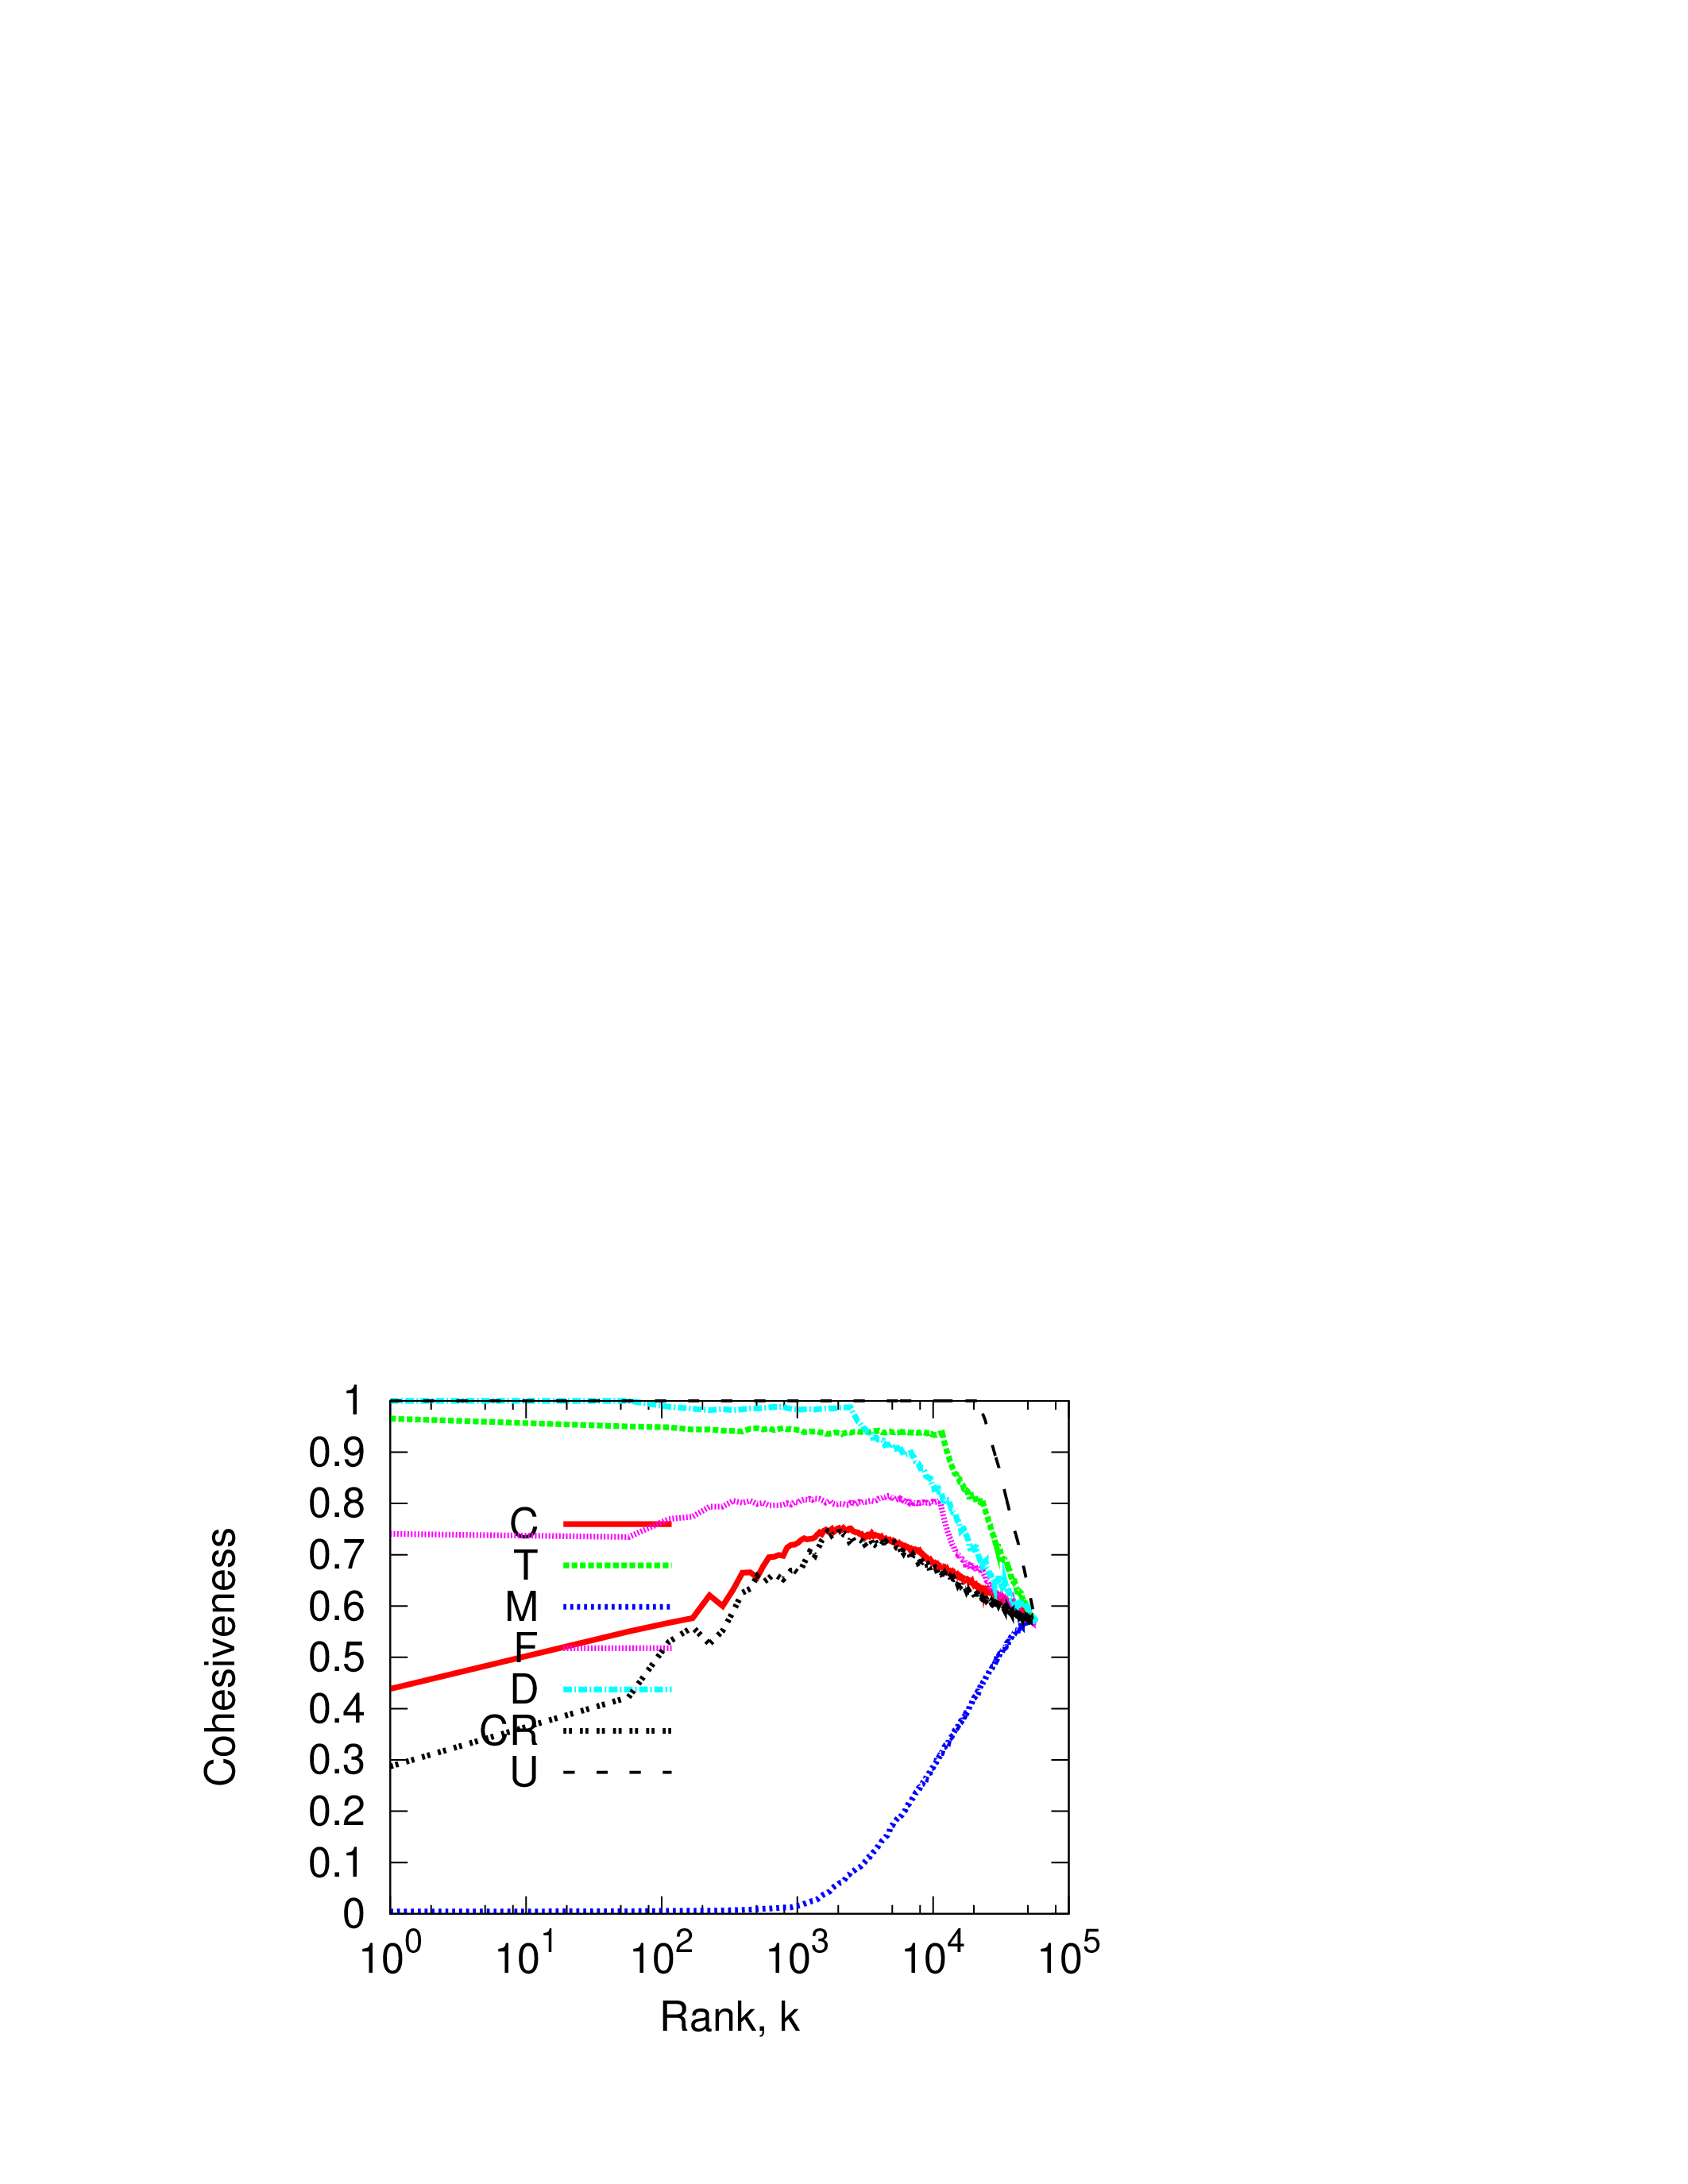}}
	\subfigure[Coh.	(DBLP)]{\includegraphics[width=0.15\textwidth]{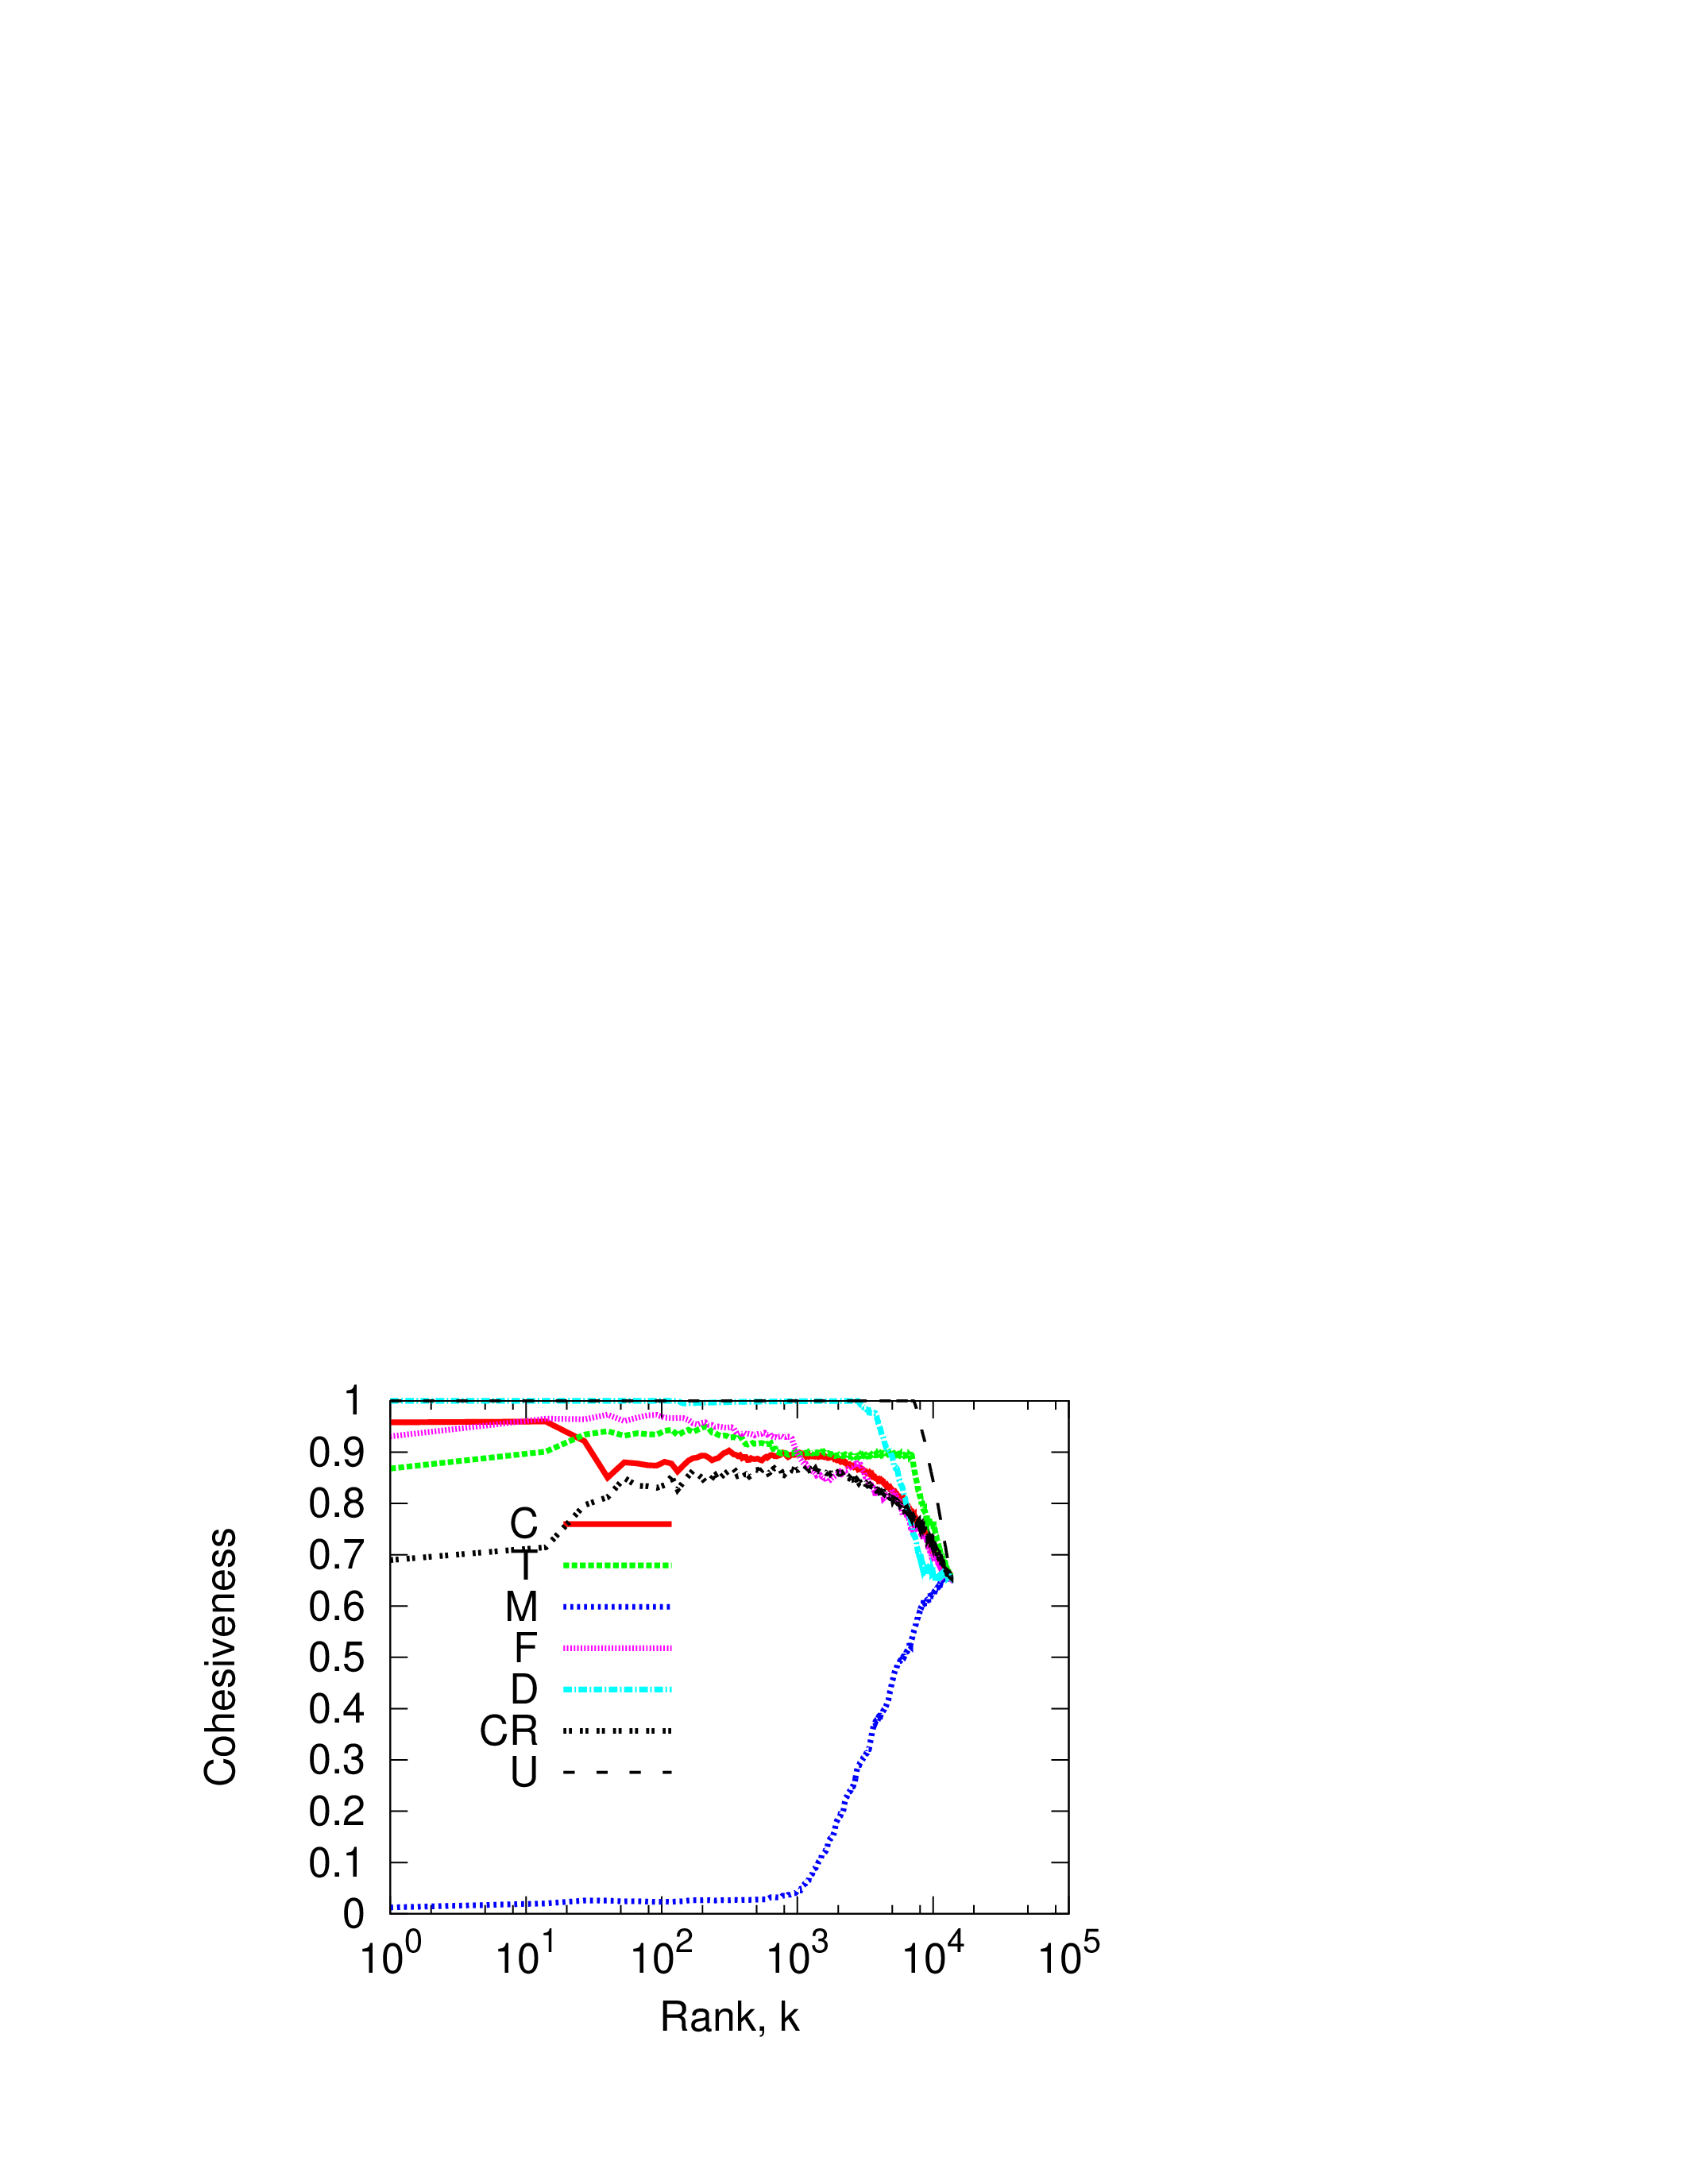}}
	\subfigure[CCF	(LJ)]{\includegraphics[width=0.15\textwidth]{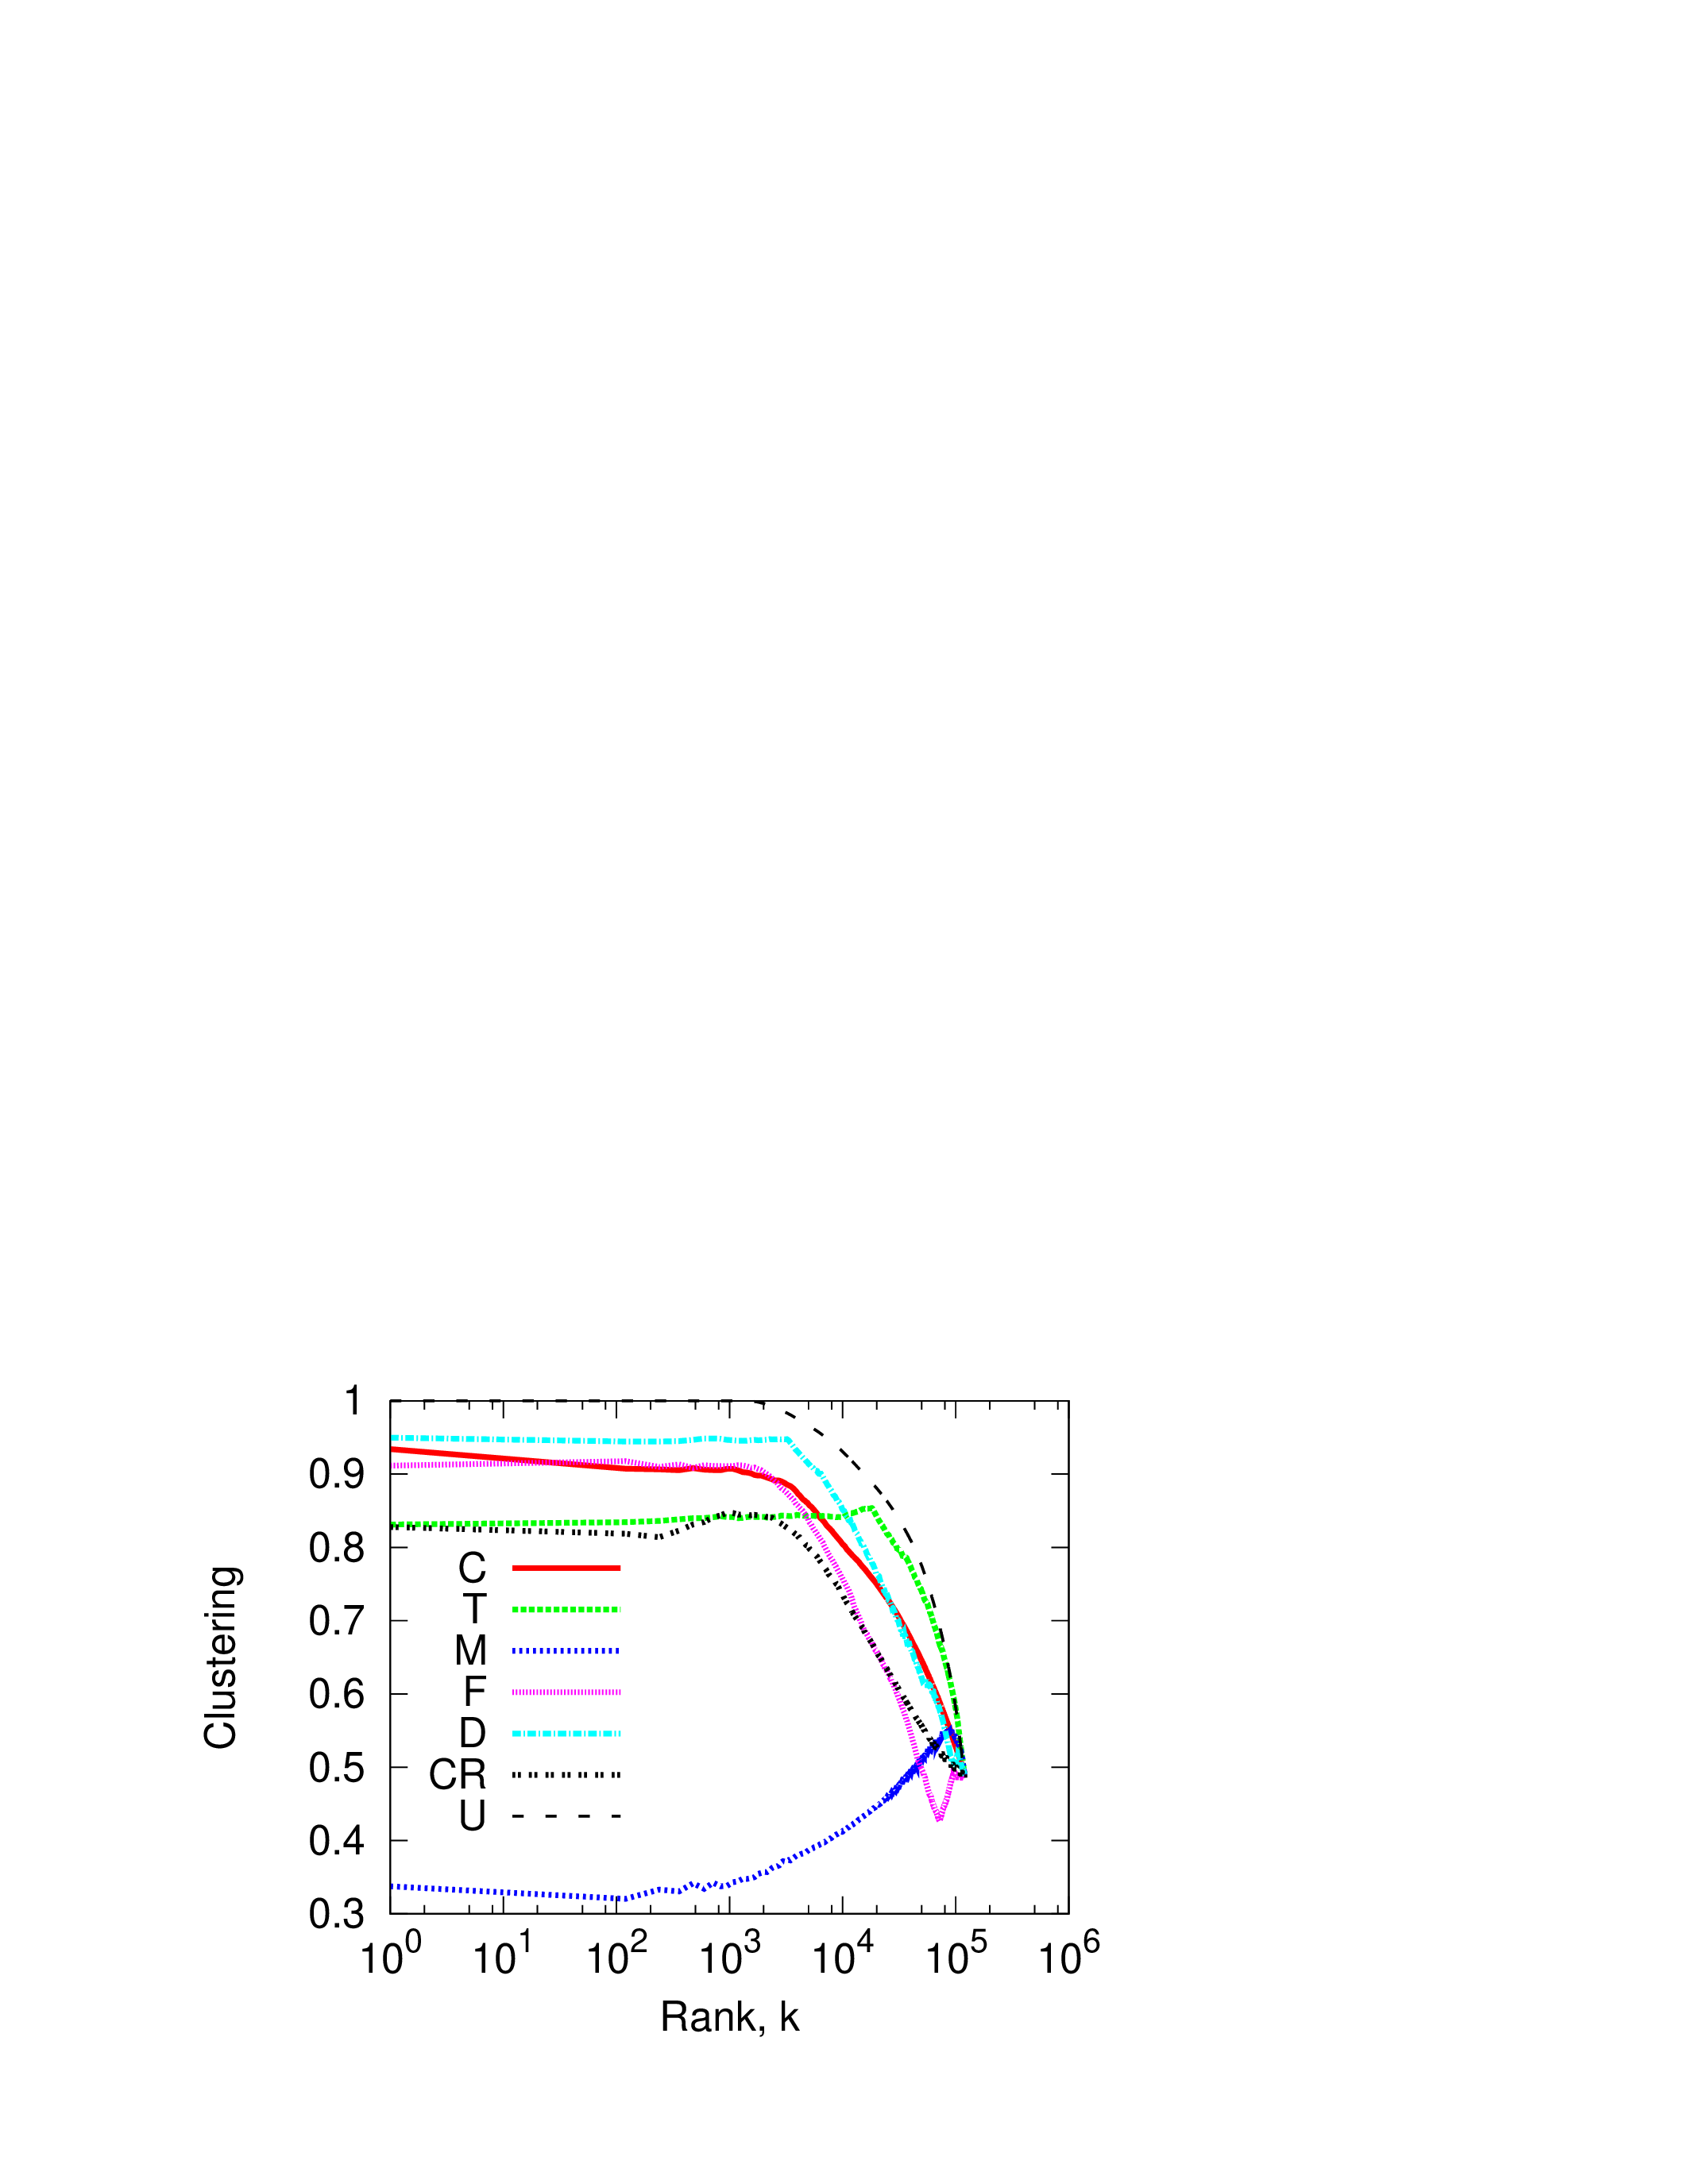}}
	\subfigure[CCF	(FS)]{\includegraphics[width=0.15\textwidth]{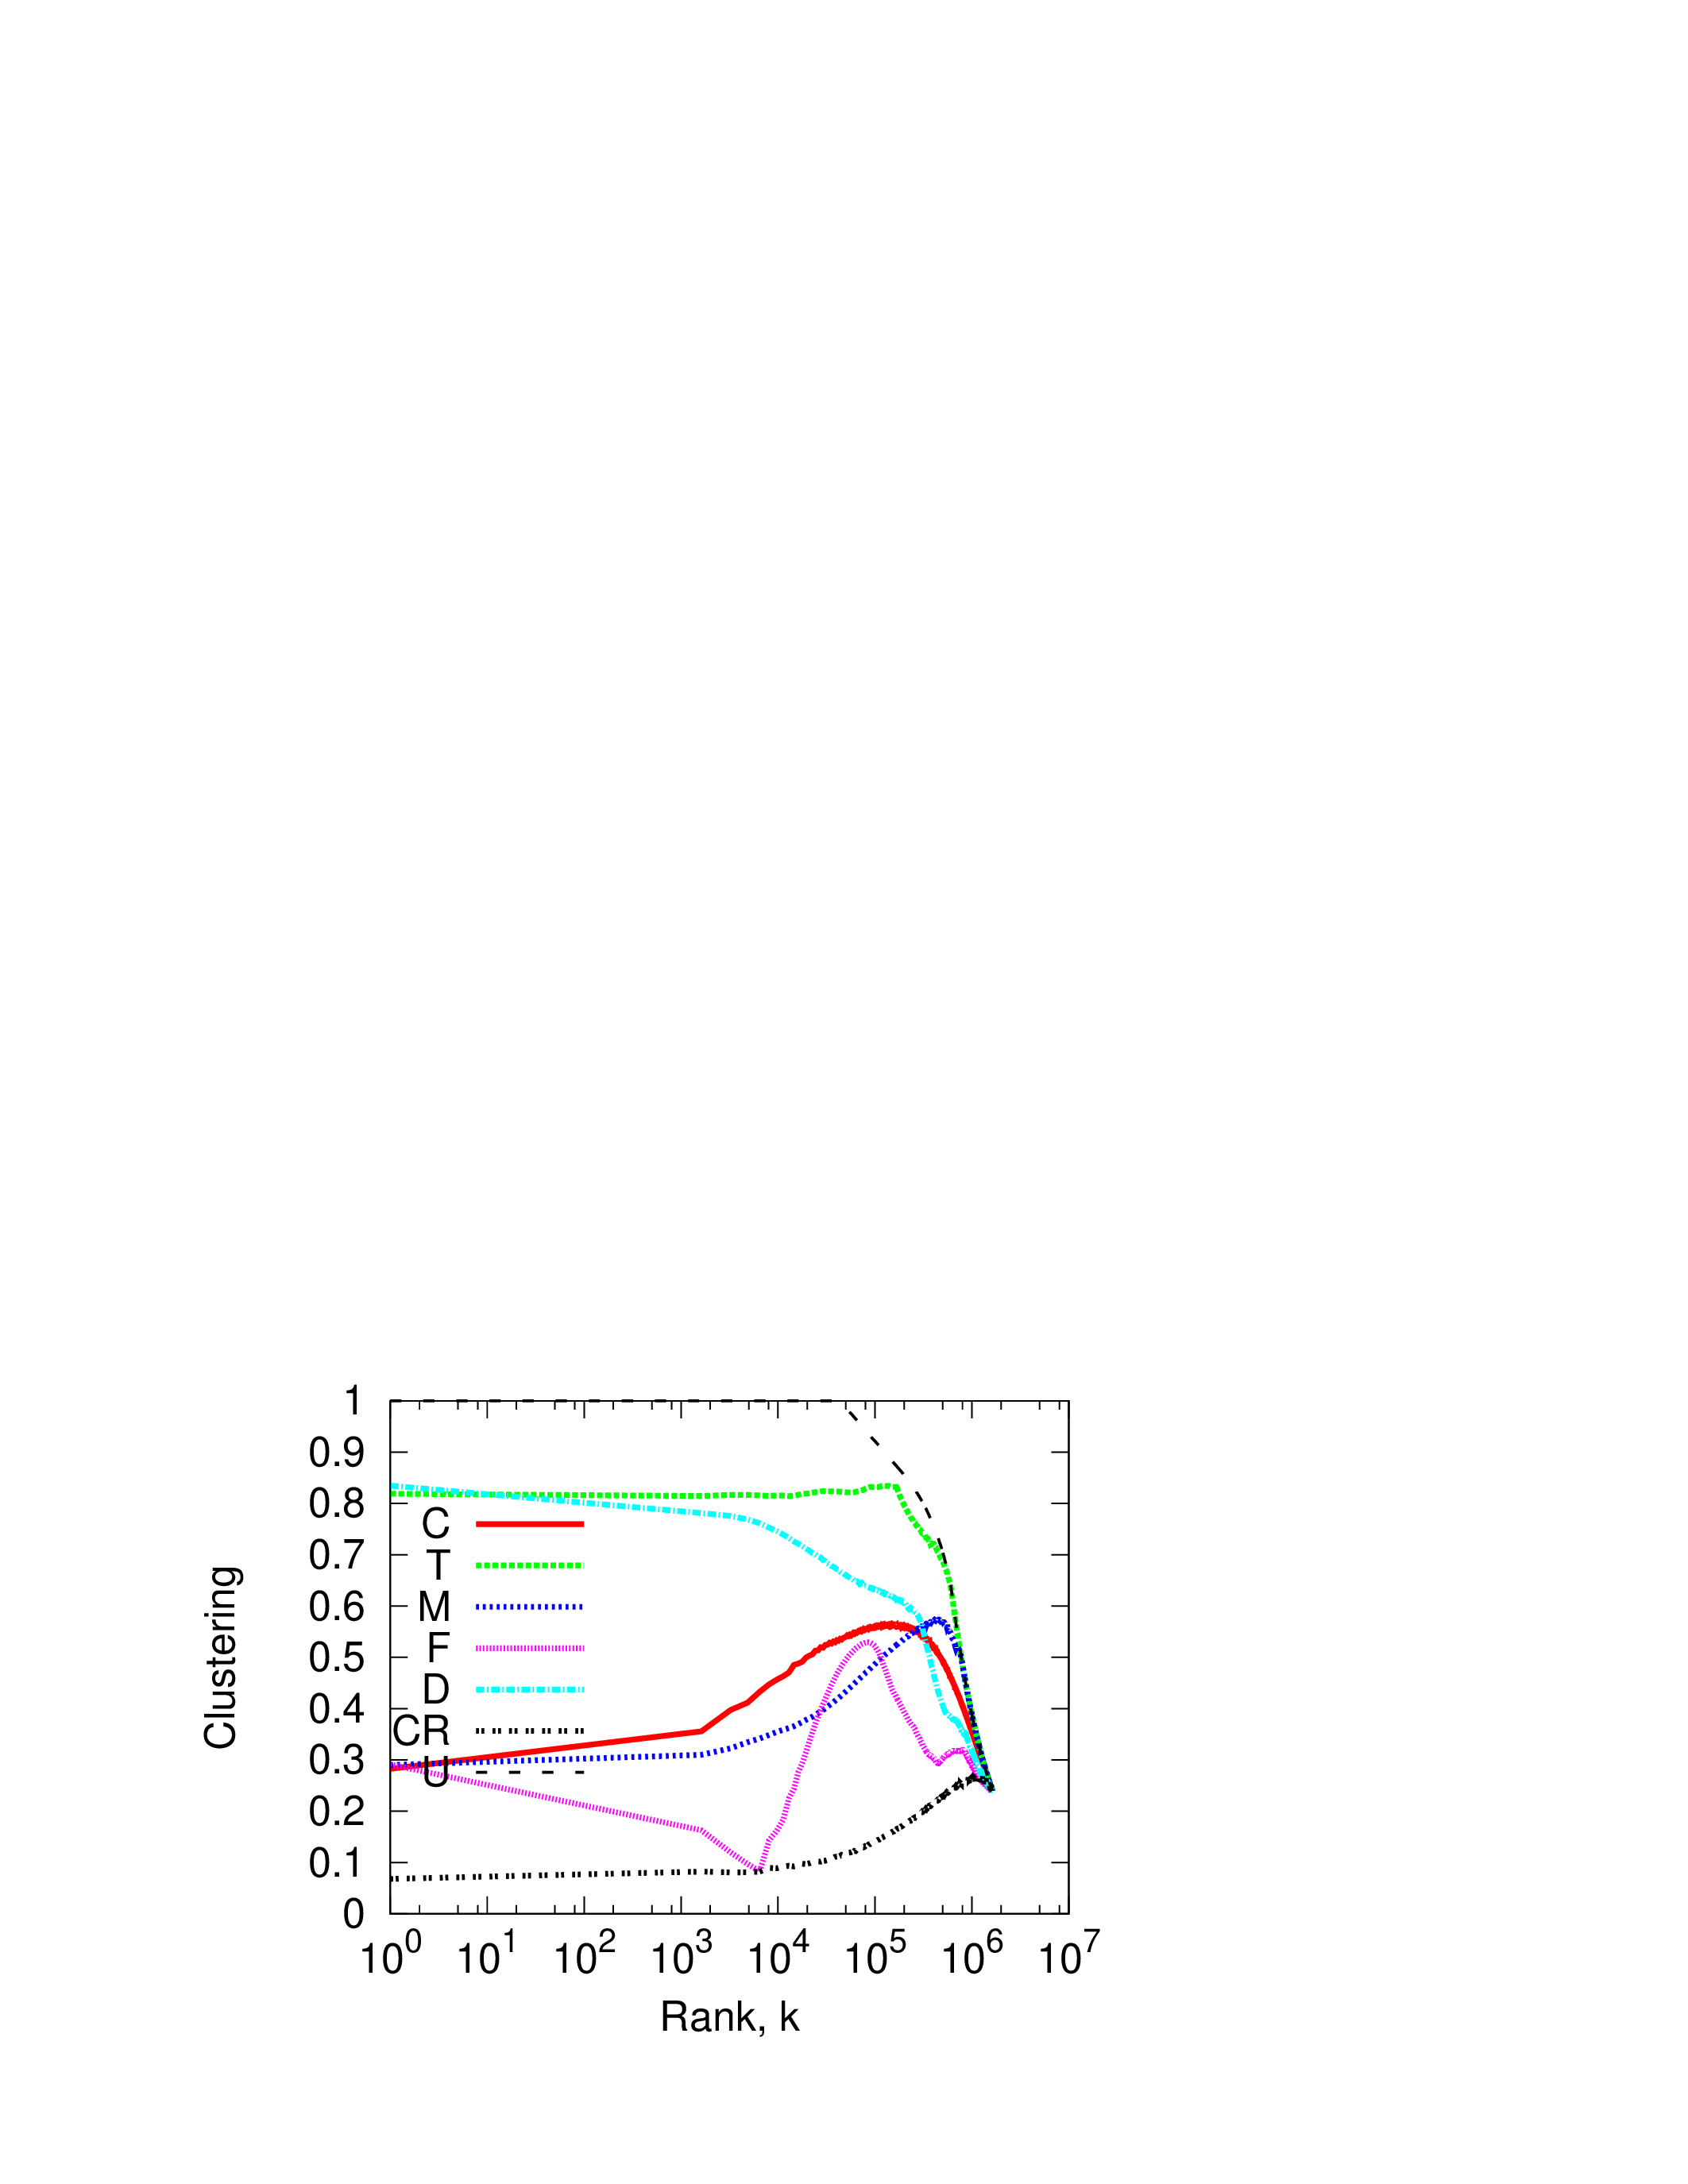}}
	\subfigure[CCF	(Orkut)]{\includegraphics[width=0.15\textwidth]{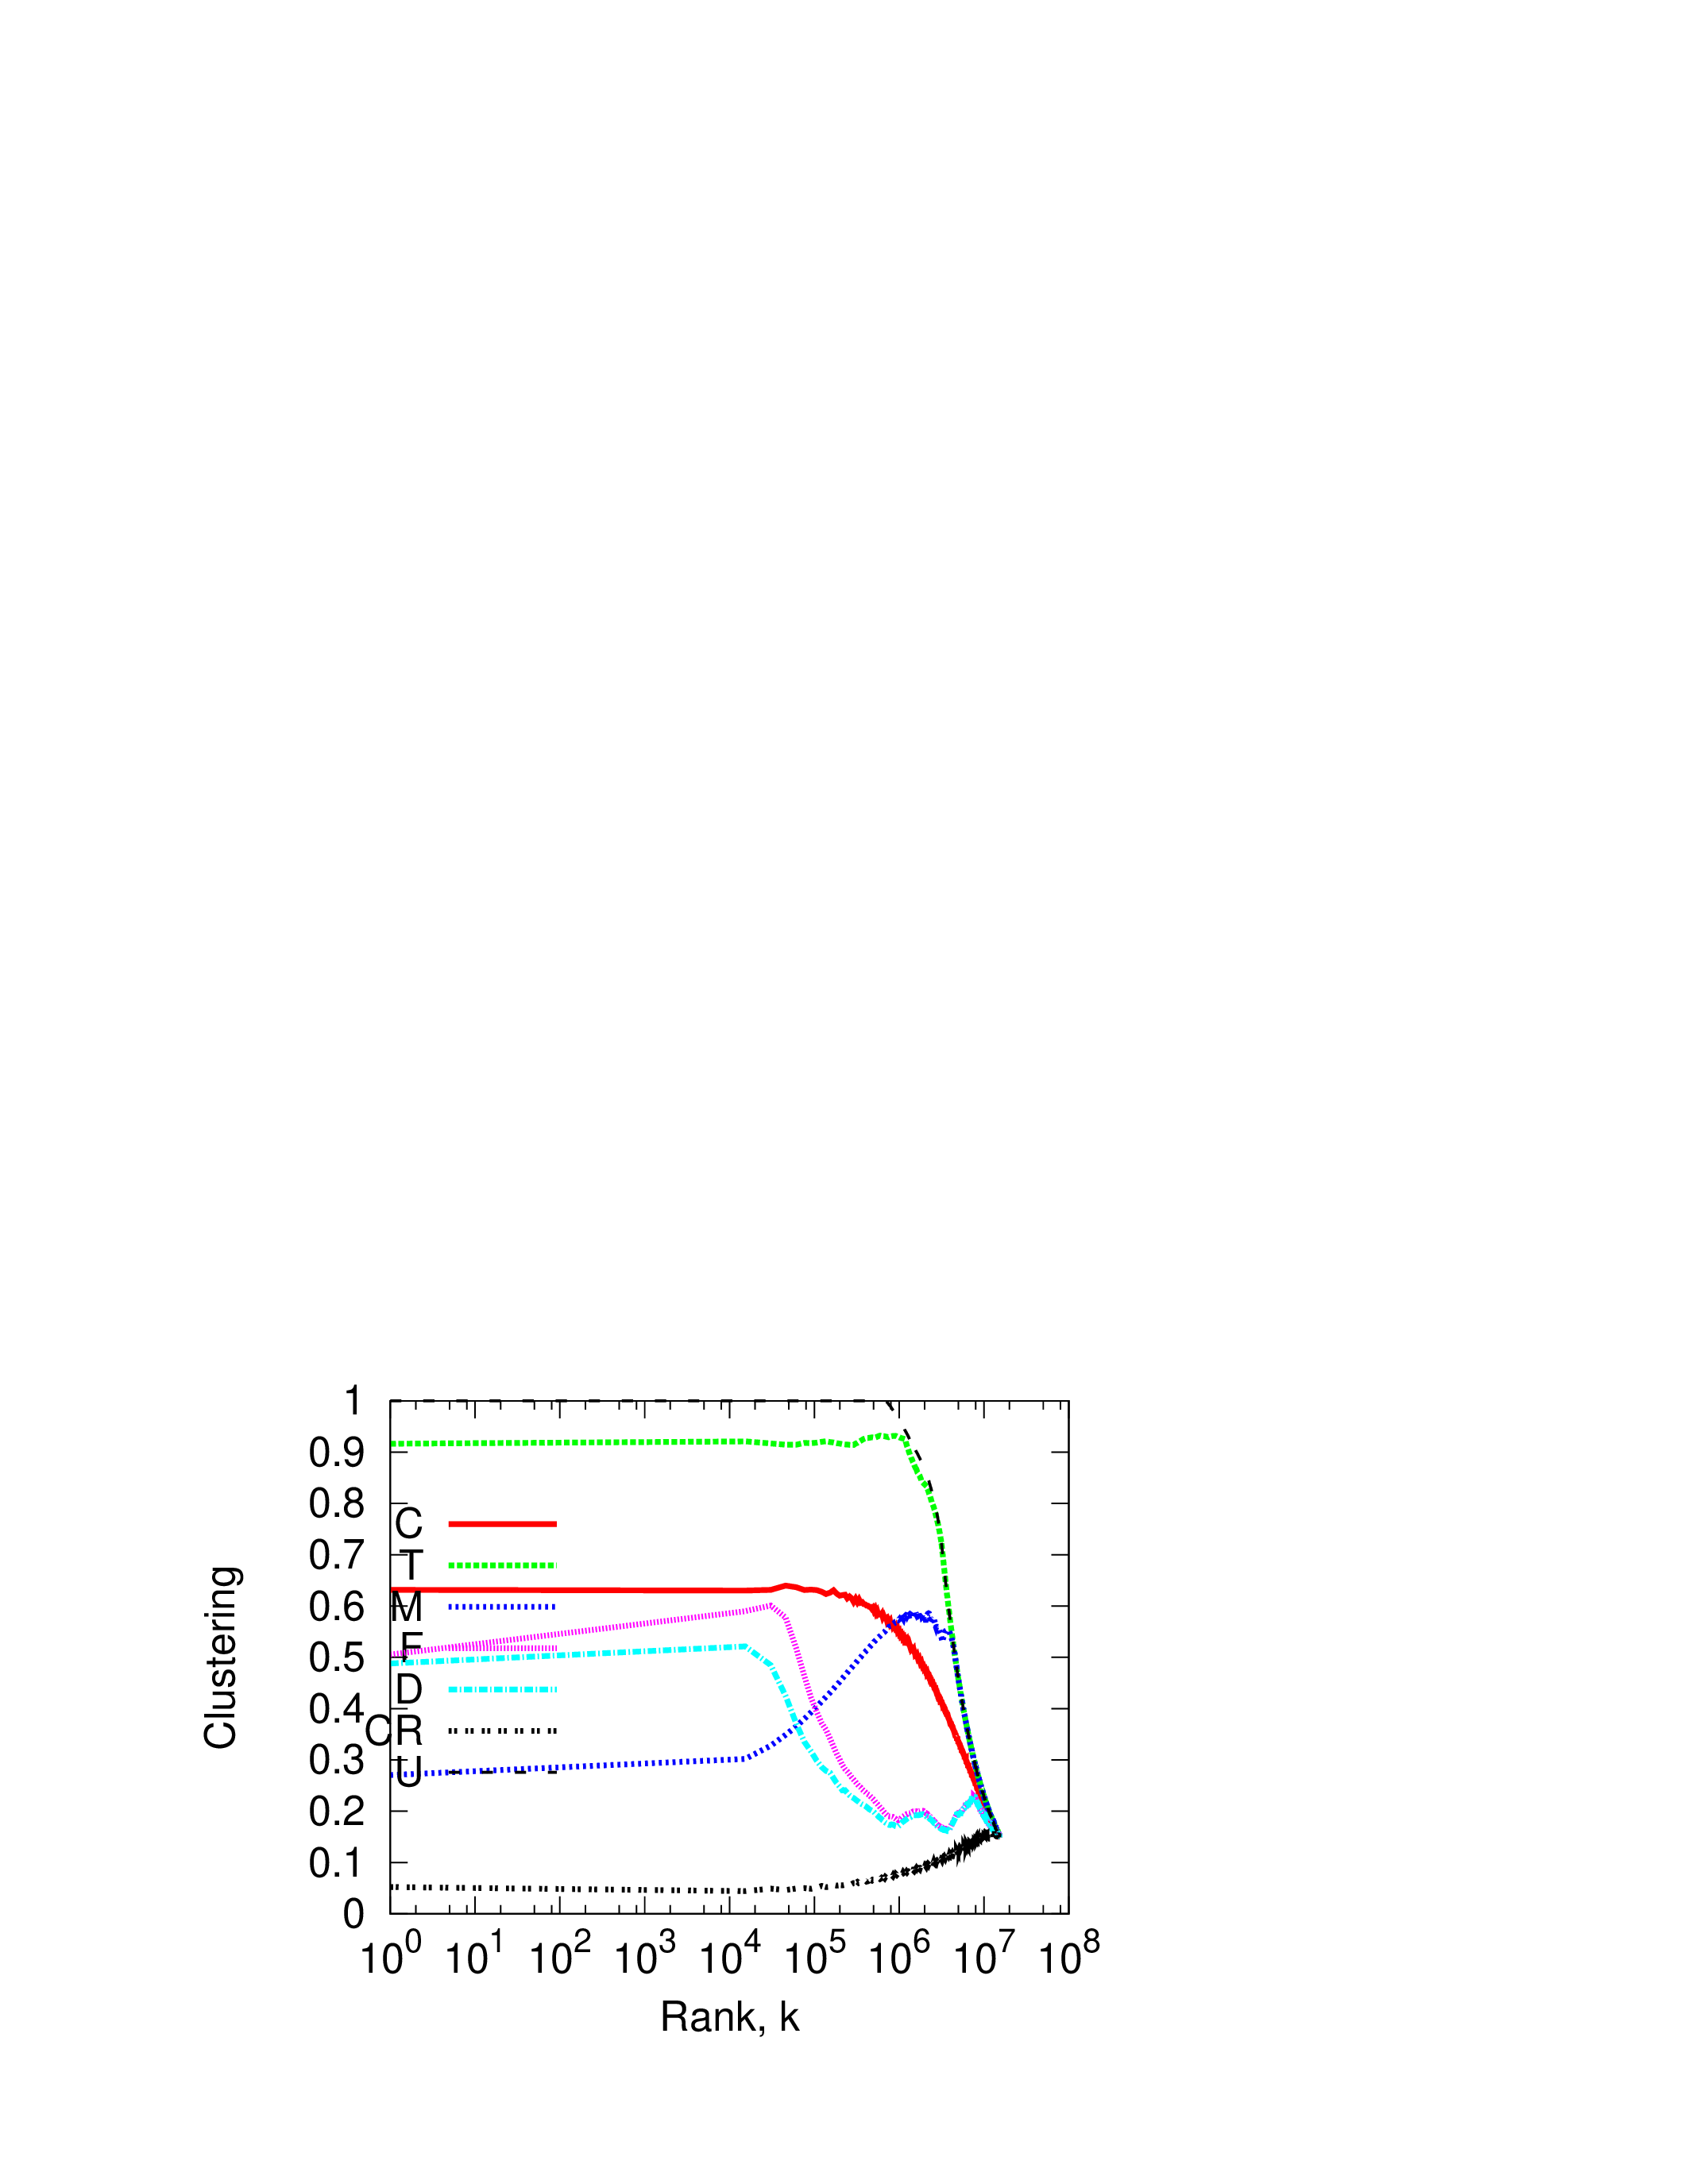}}
	\subfigure[CCF	(Ning)]{\includegraphics[width=0.15\textwidth]{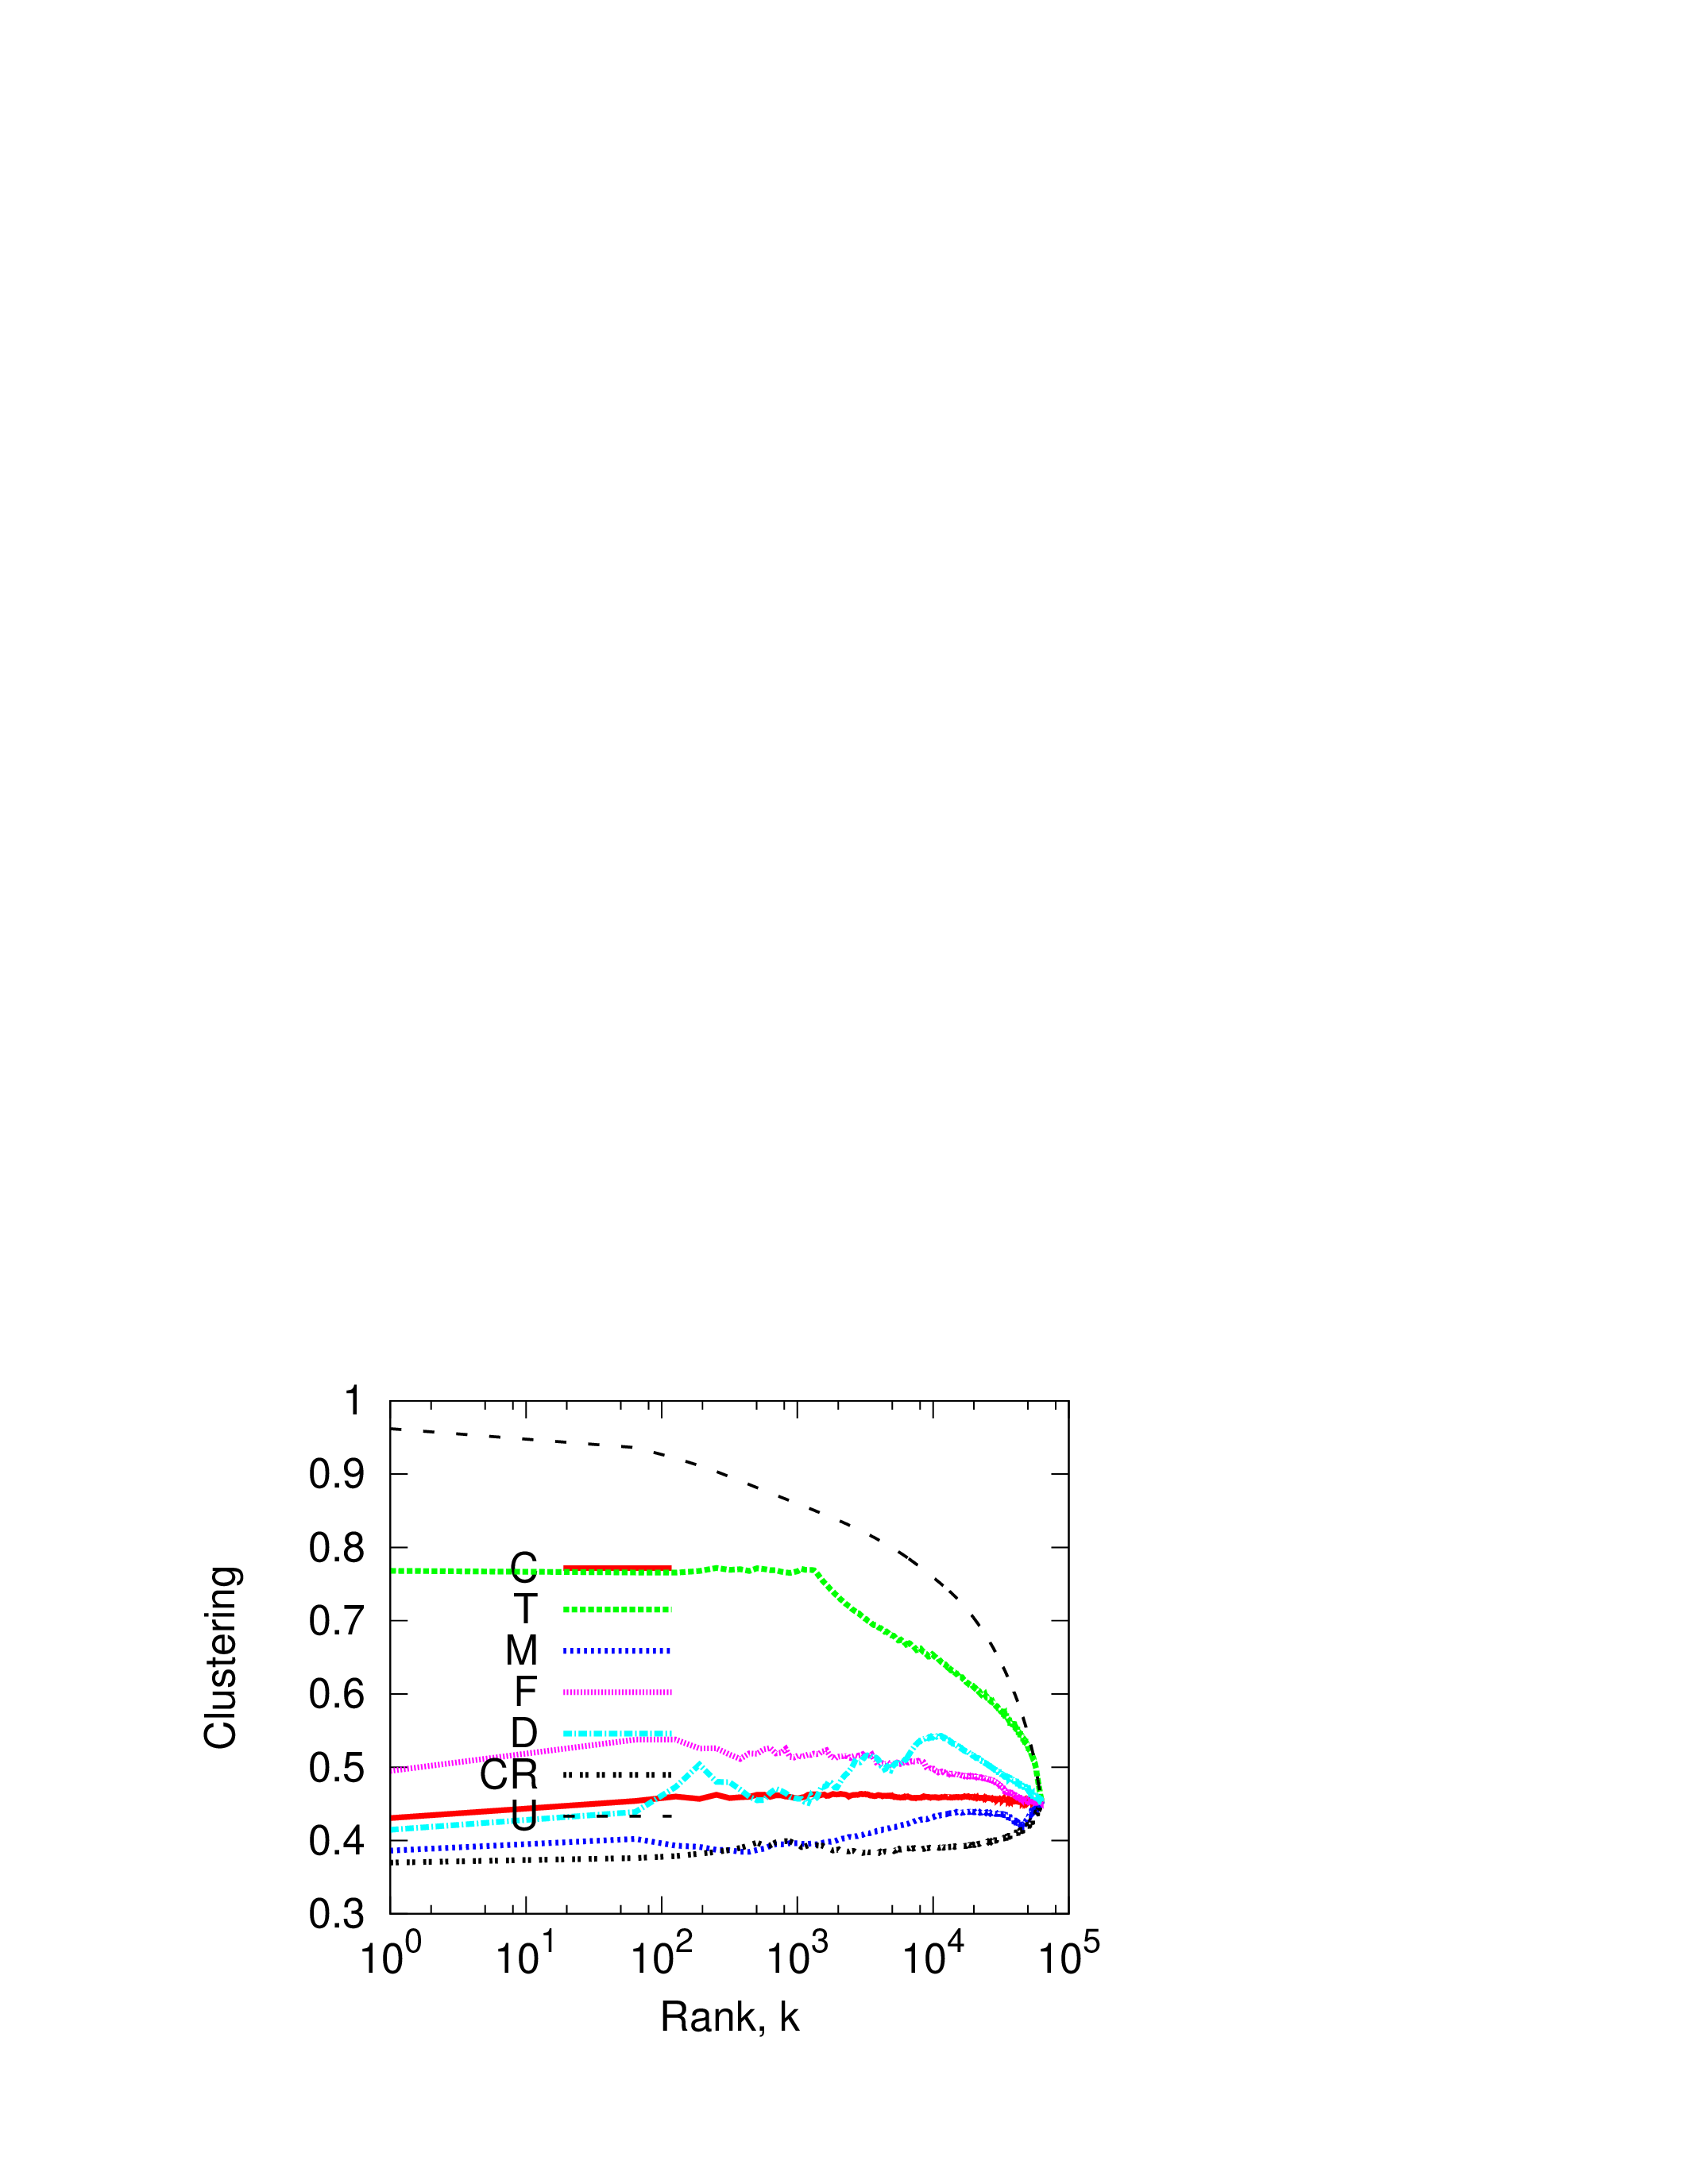}}
	\subfigure[CCF	(Amazon)]{\includegraphics[width=0.15\textwidth]{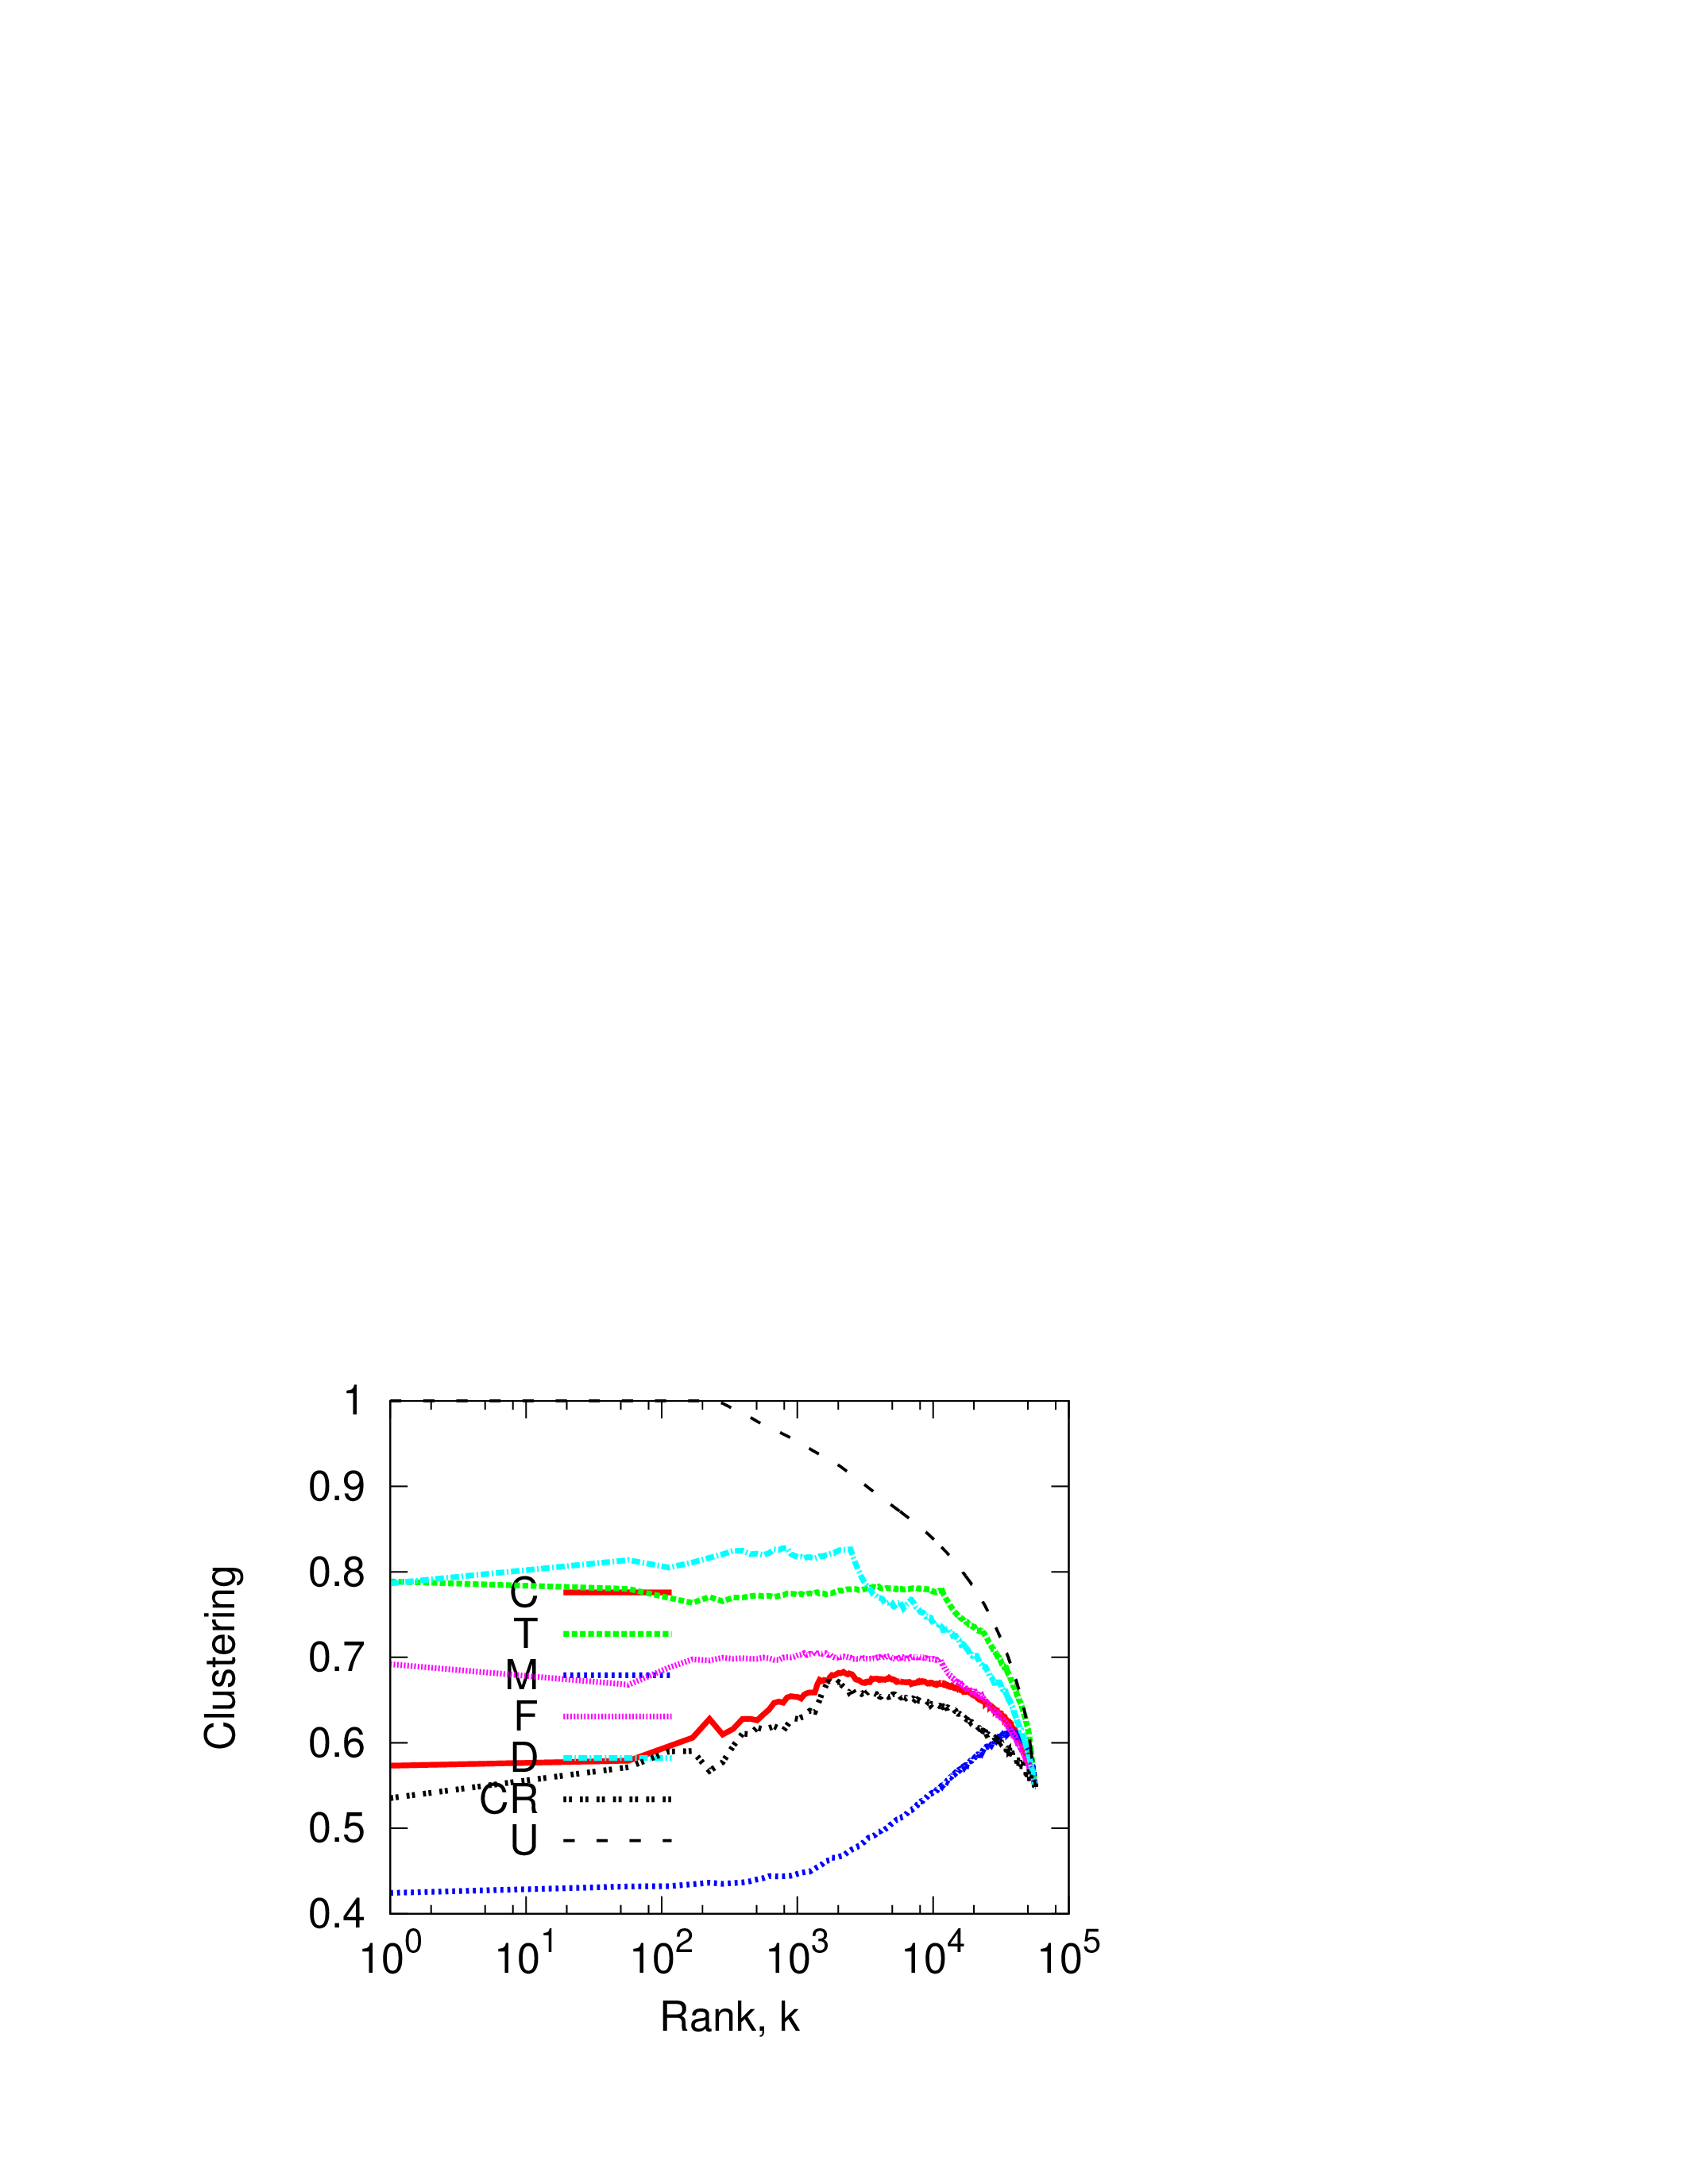}}
	\subfigure[CCF	(DBLP)]{\includegraphics[width=0.15\textwidth]{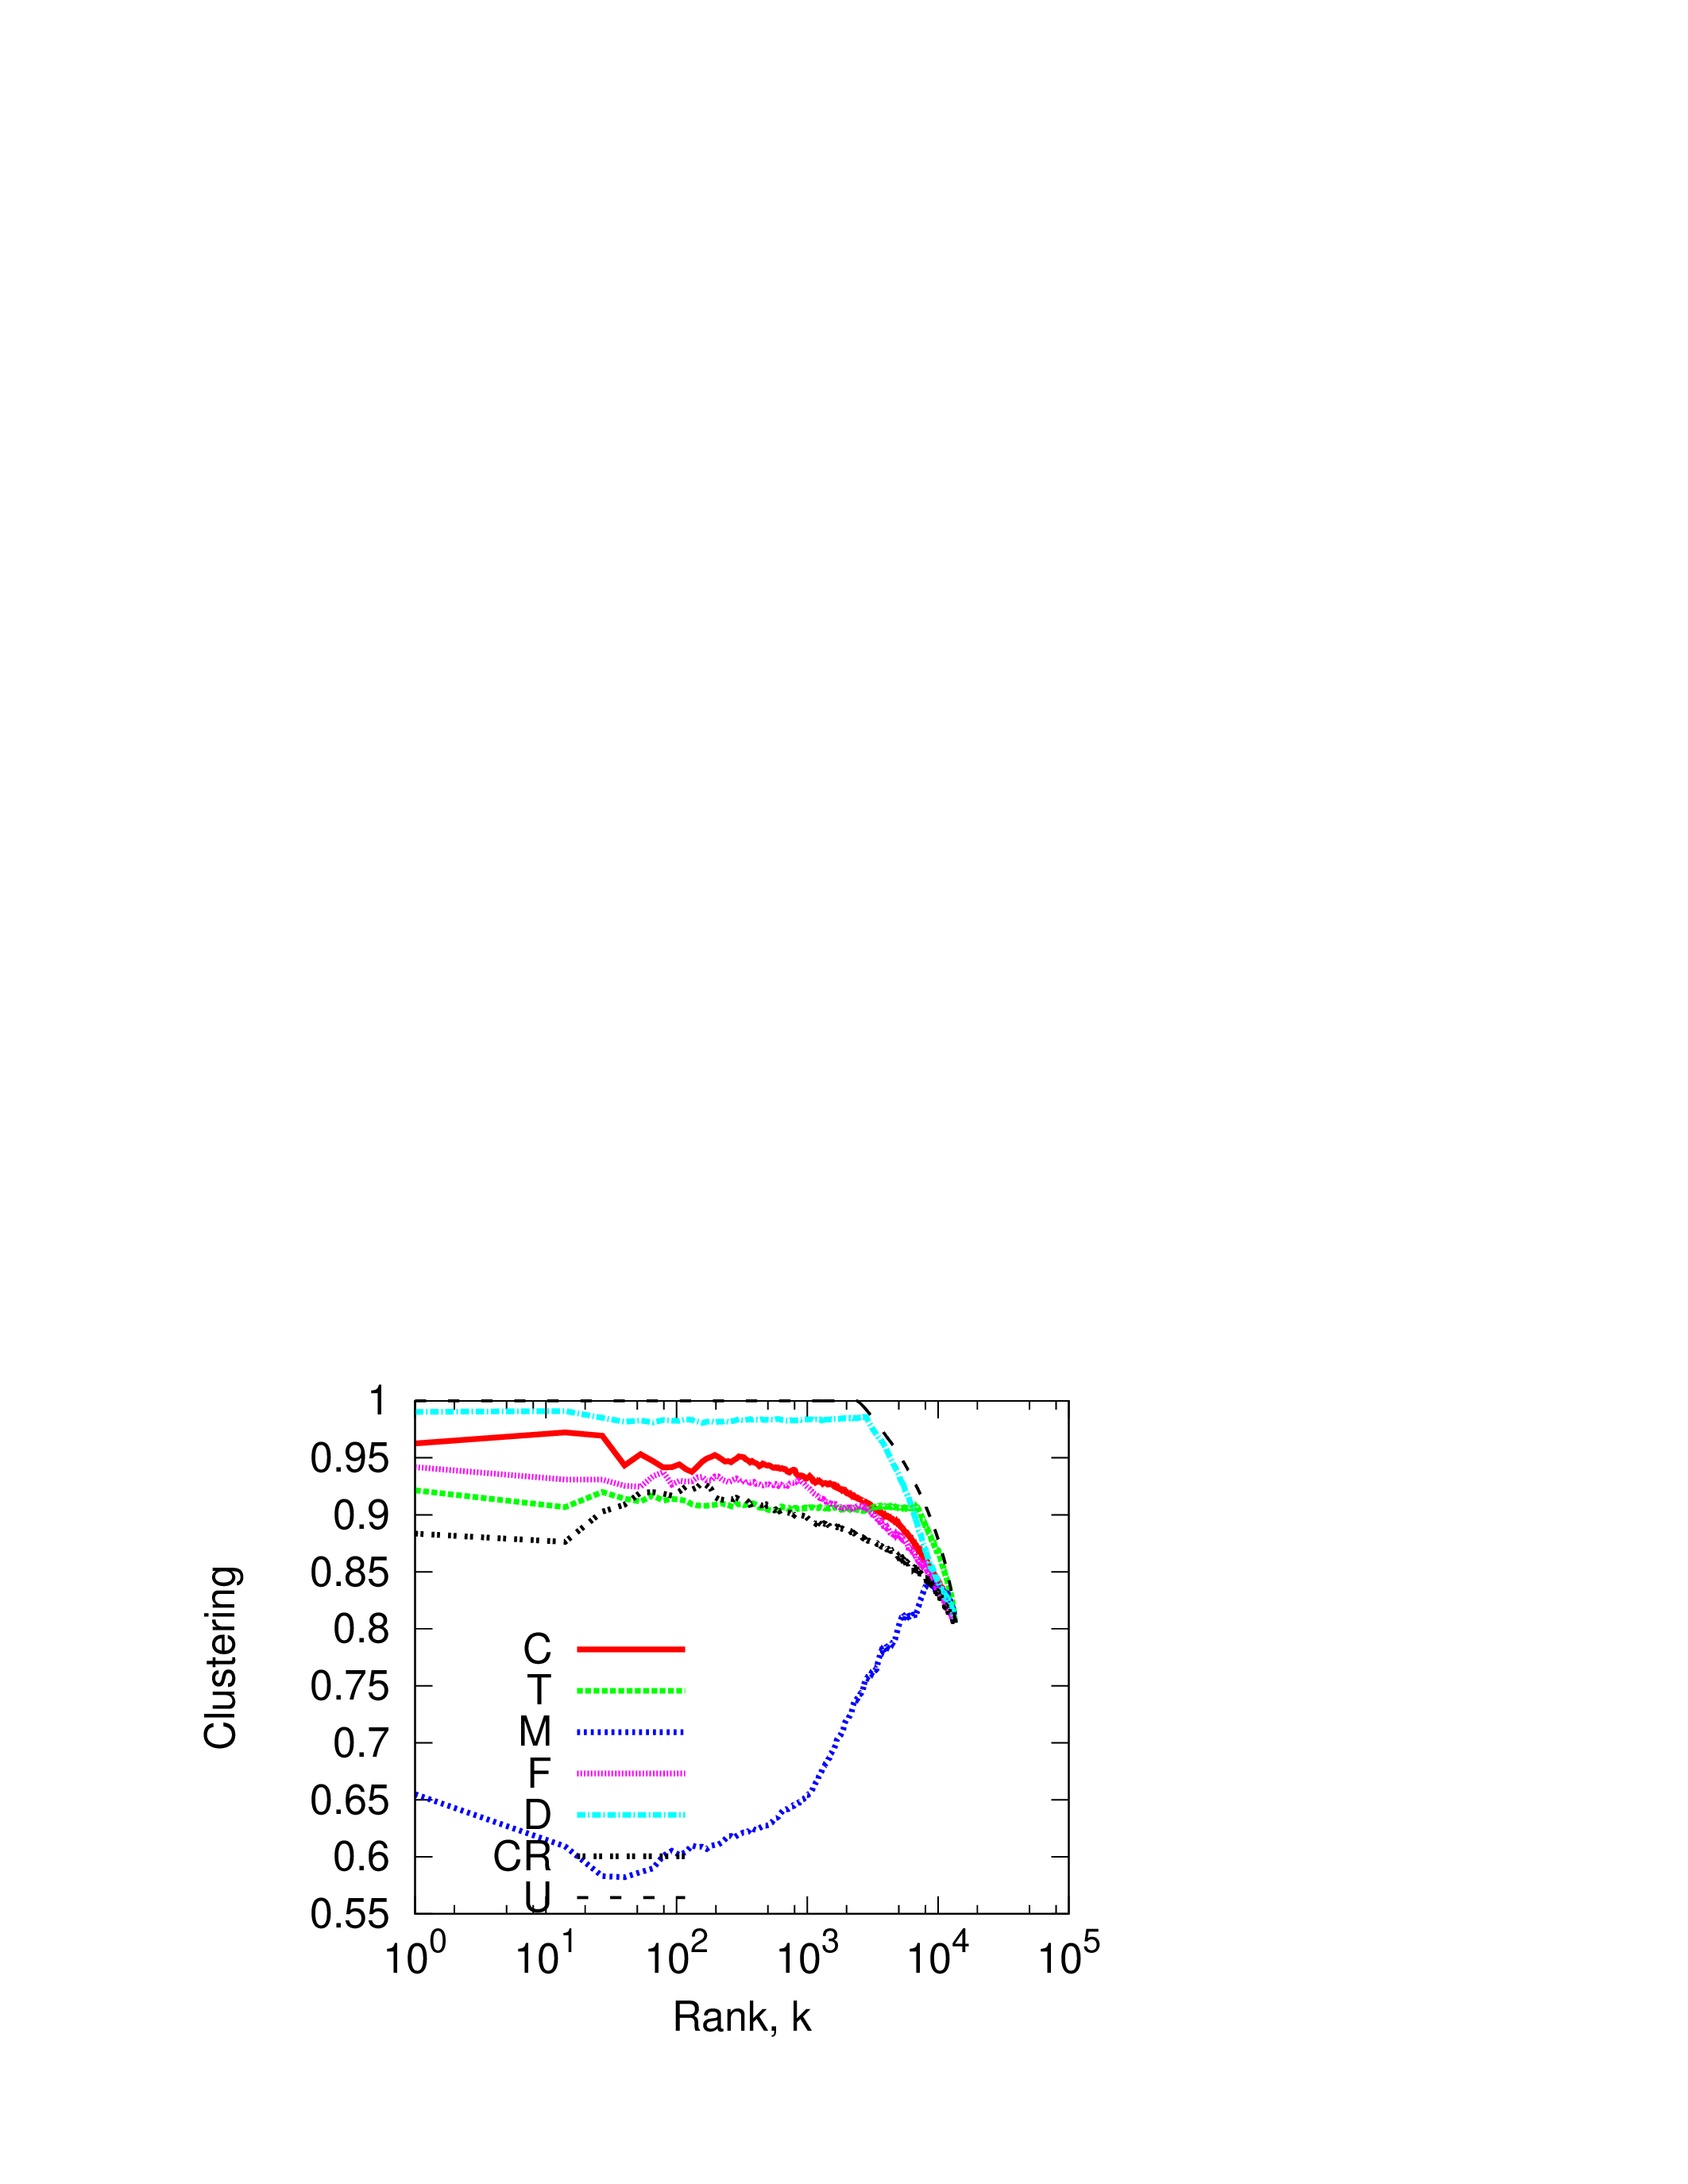}}
	\caption{Average metrics of	top	k	communities	by the scores. Sep.: Separability, Coh.: Cohesiveness.}
\label{fig:All.rank.AvgPath}
\vspace{-5mm}
\end{figure}

\begin{figure}[!h]
	\centering
	\subfigure[NS	(LJ)]{\includegraphics[width=0.15\textwidth]{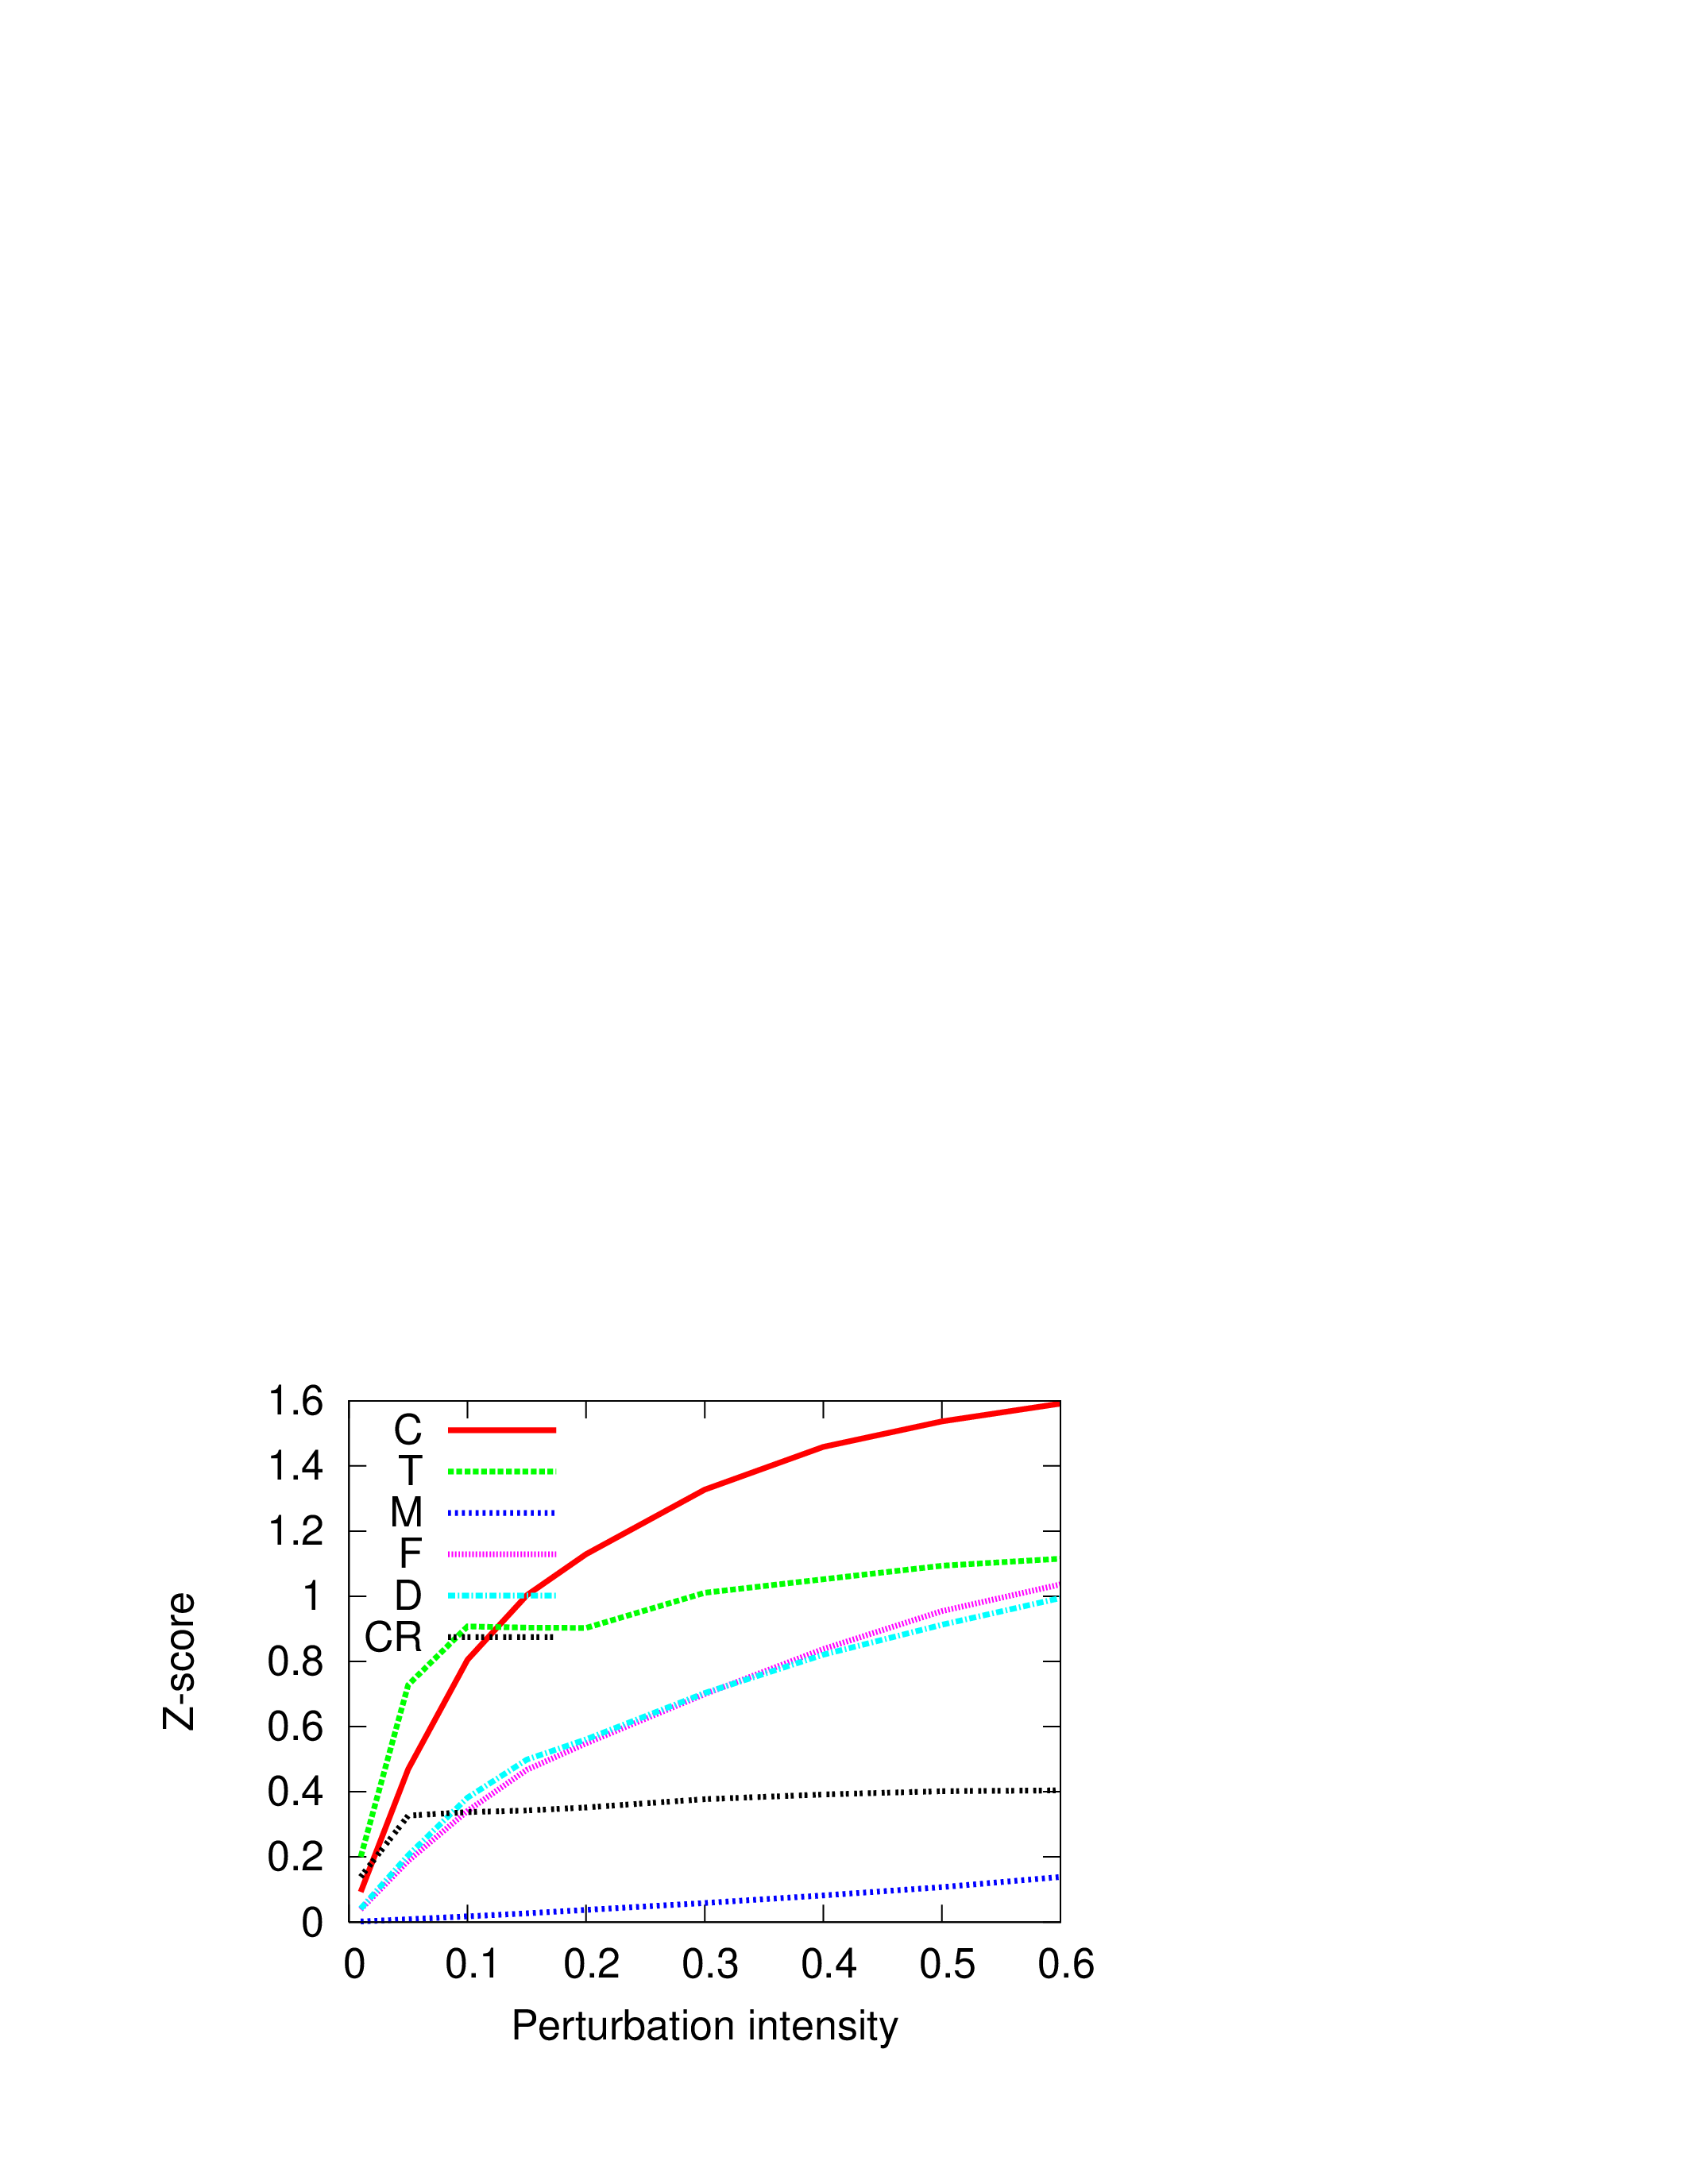}}
	\subfigure[NS	(FS)]{\includegraphics[width=0.15\textwidth]{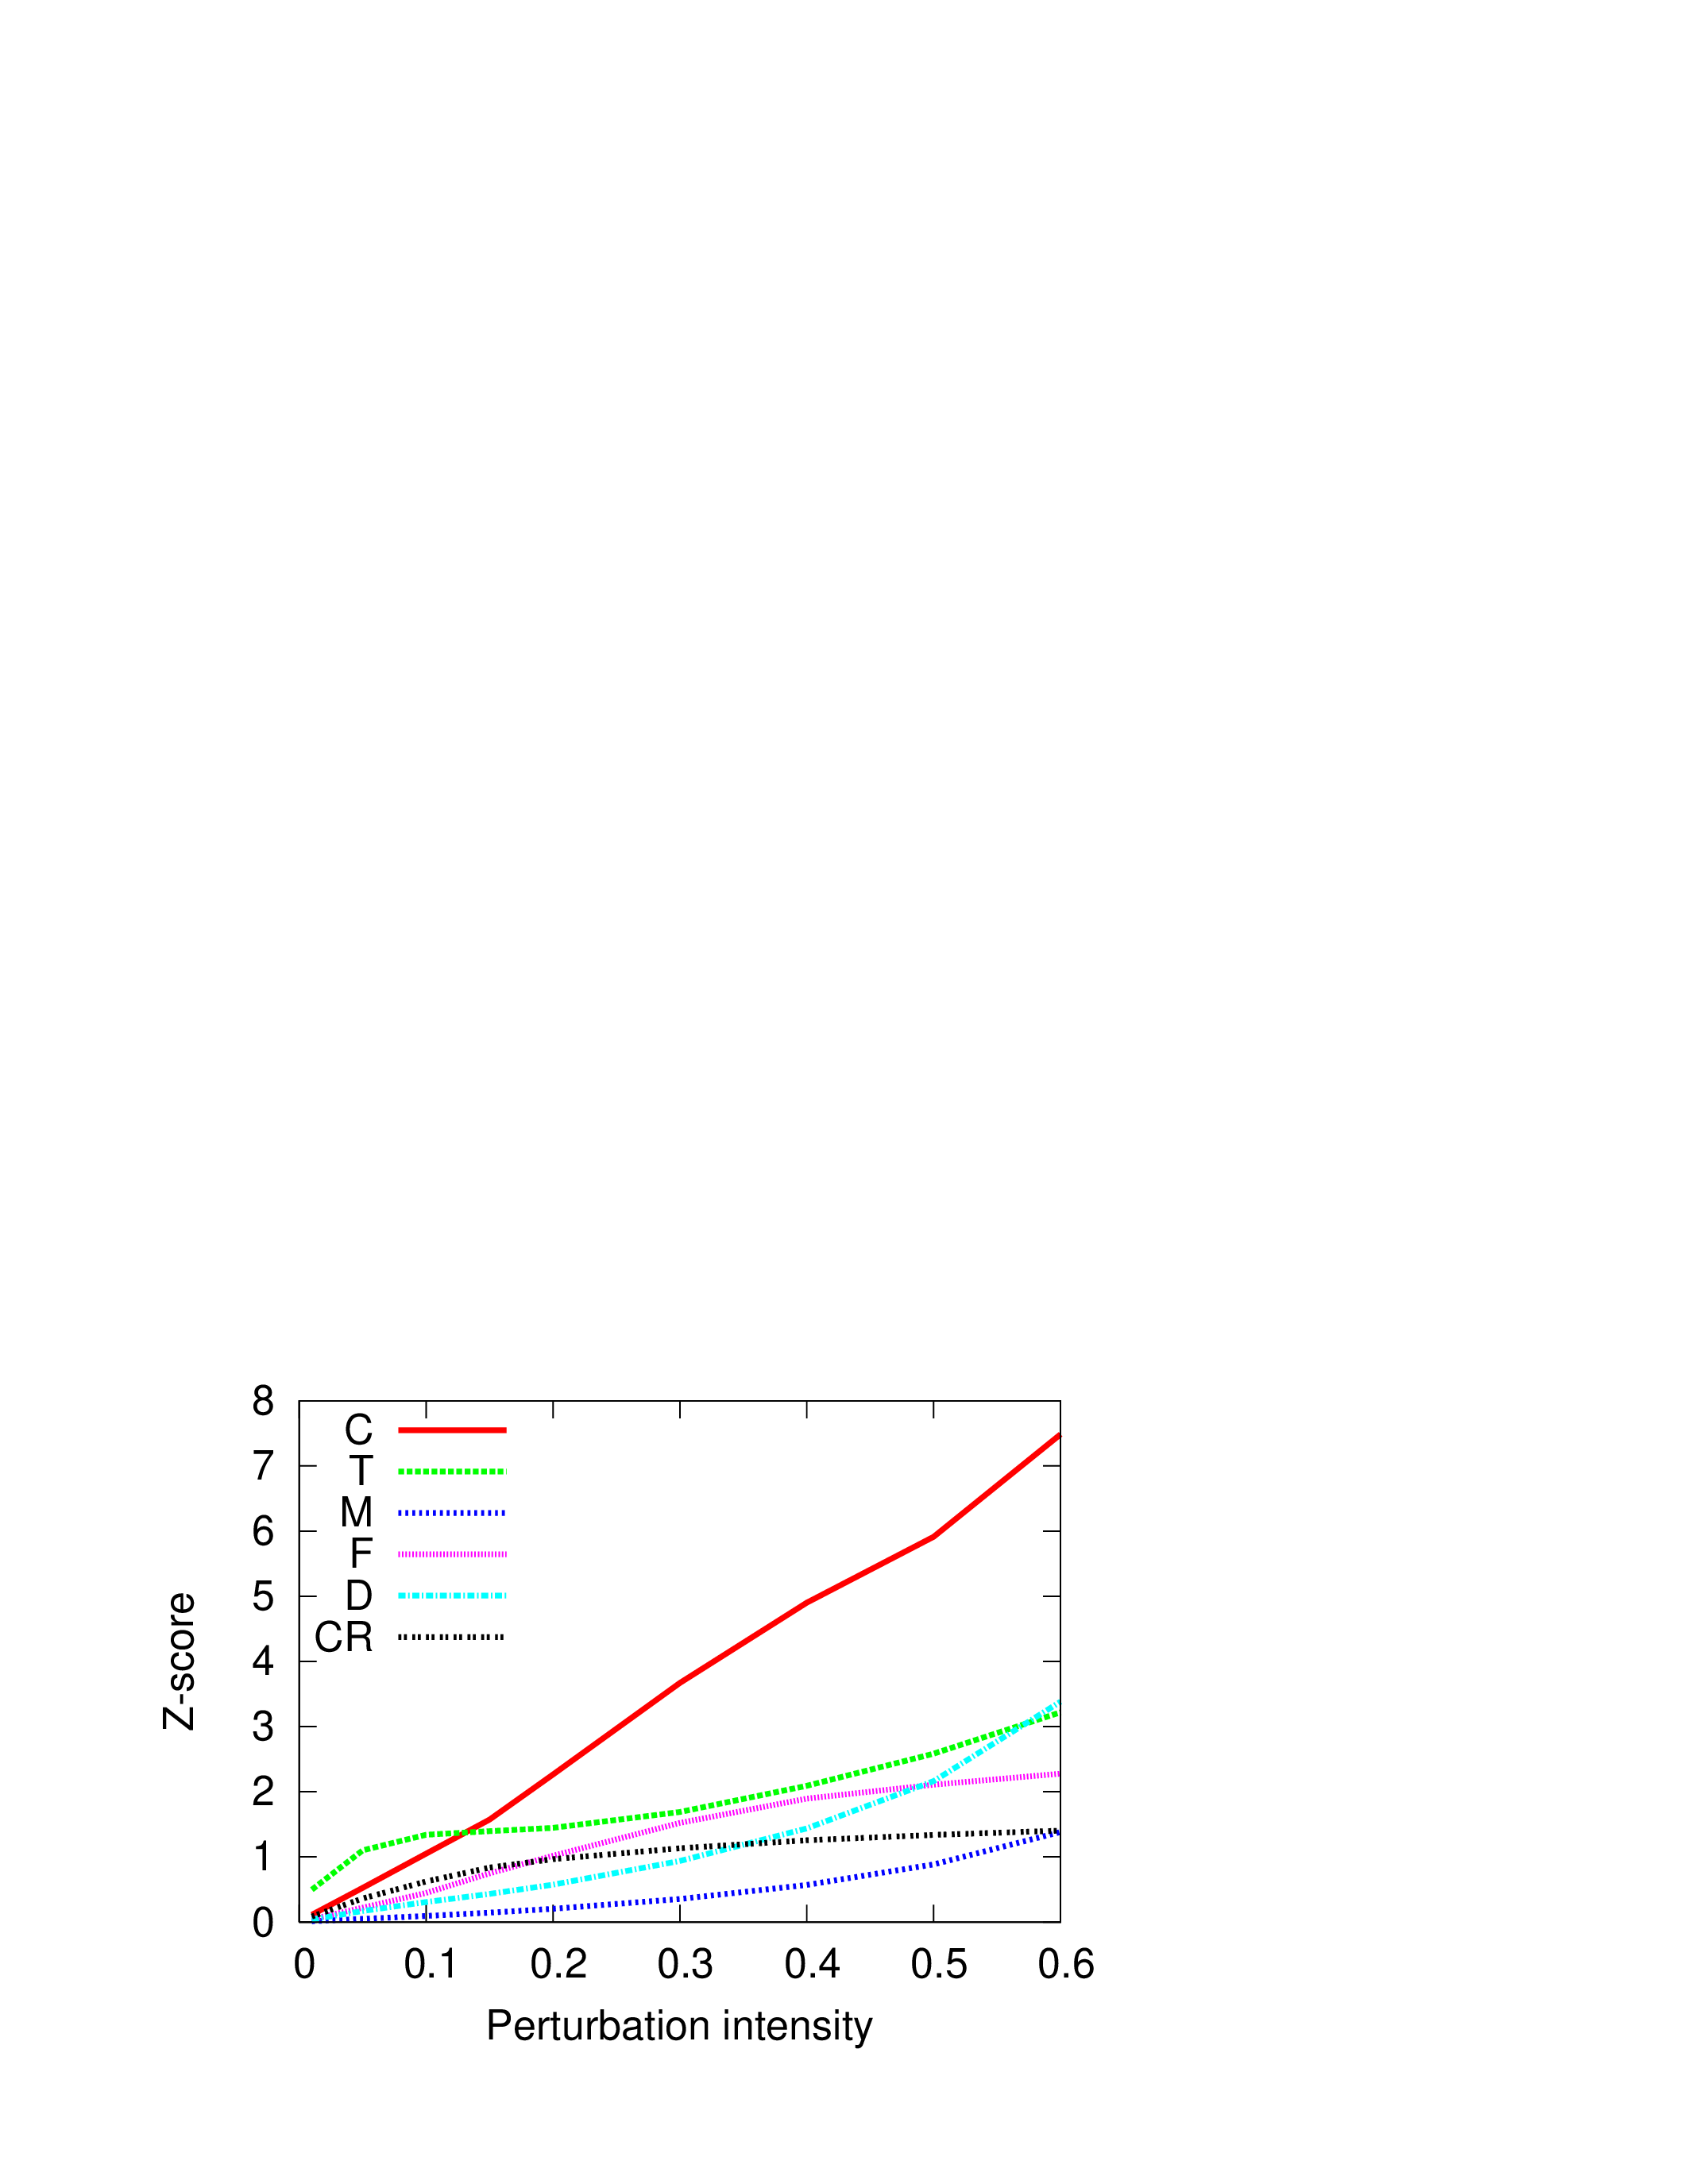}}
	\subfigure[NS	(Orkut)]{\includegraphics[width=0.15\textwidth]{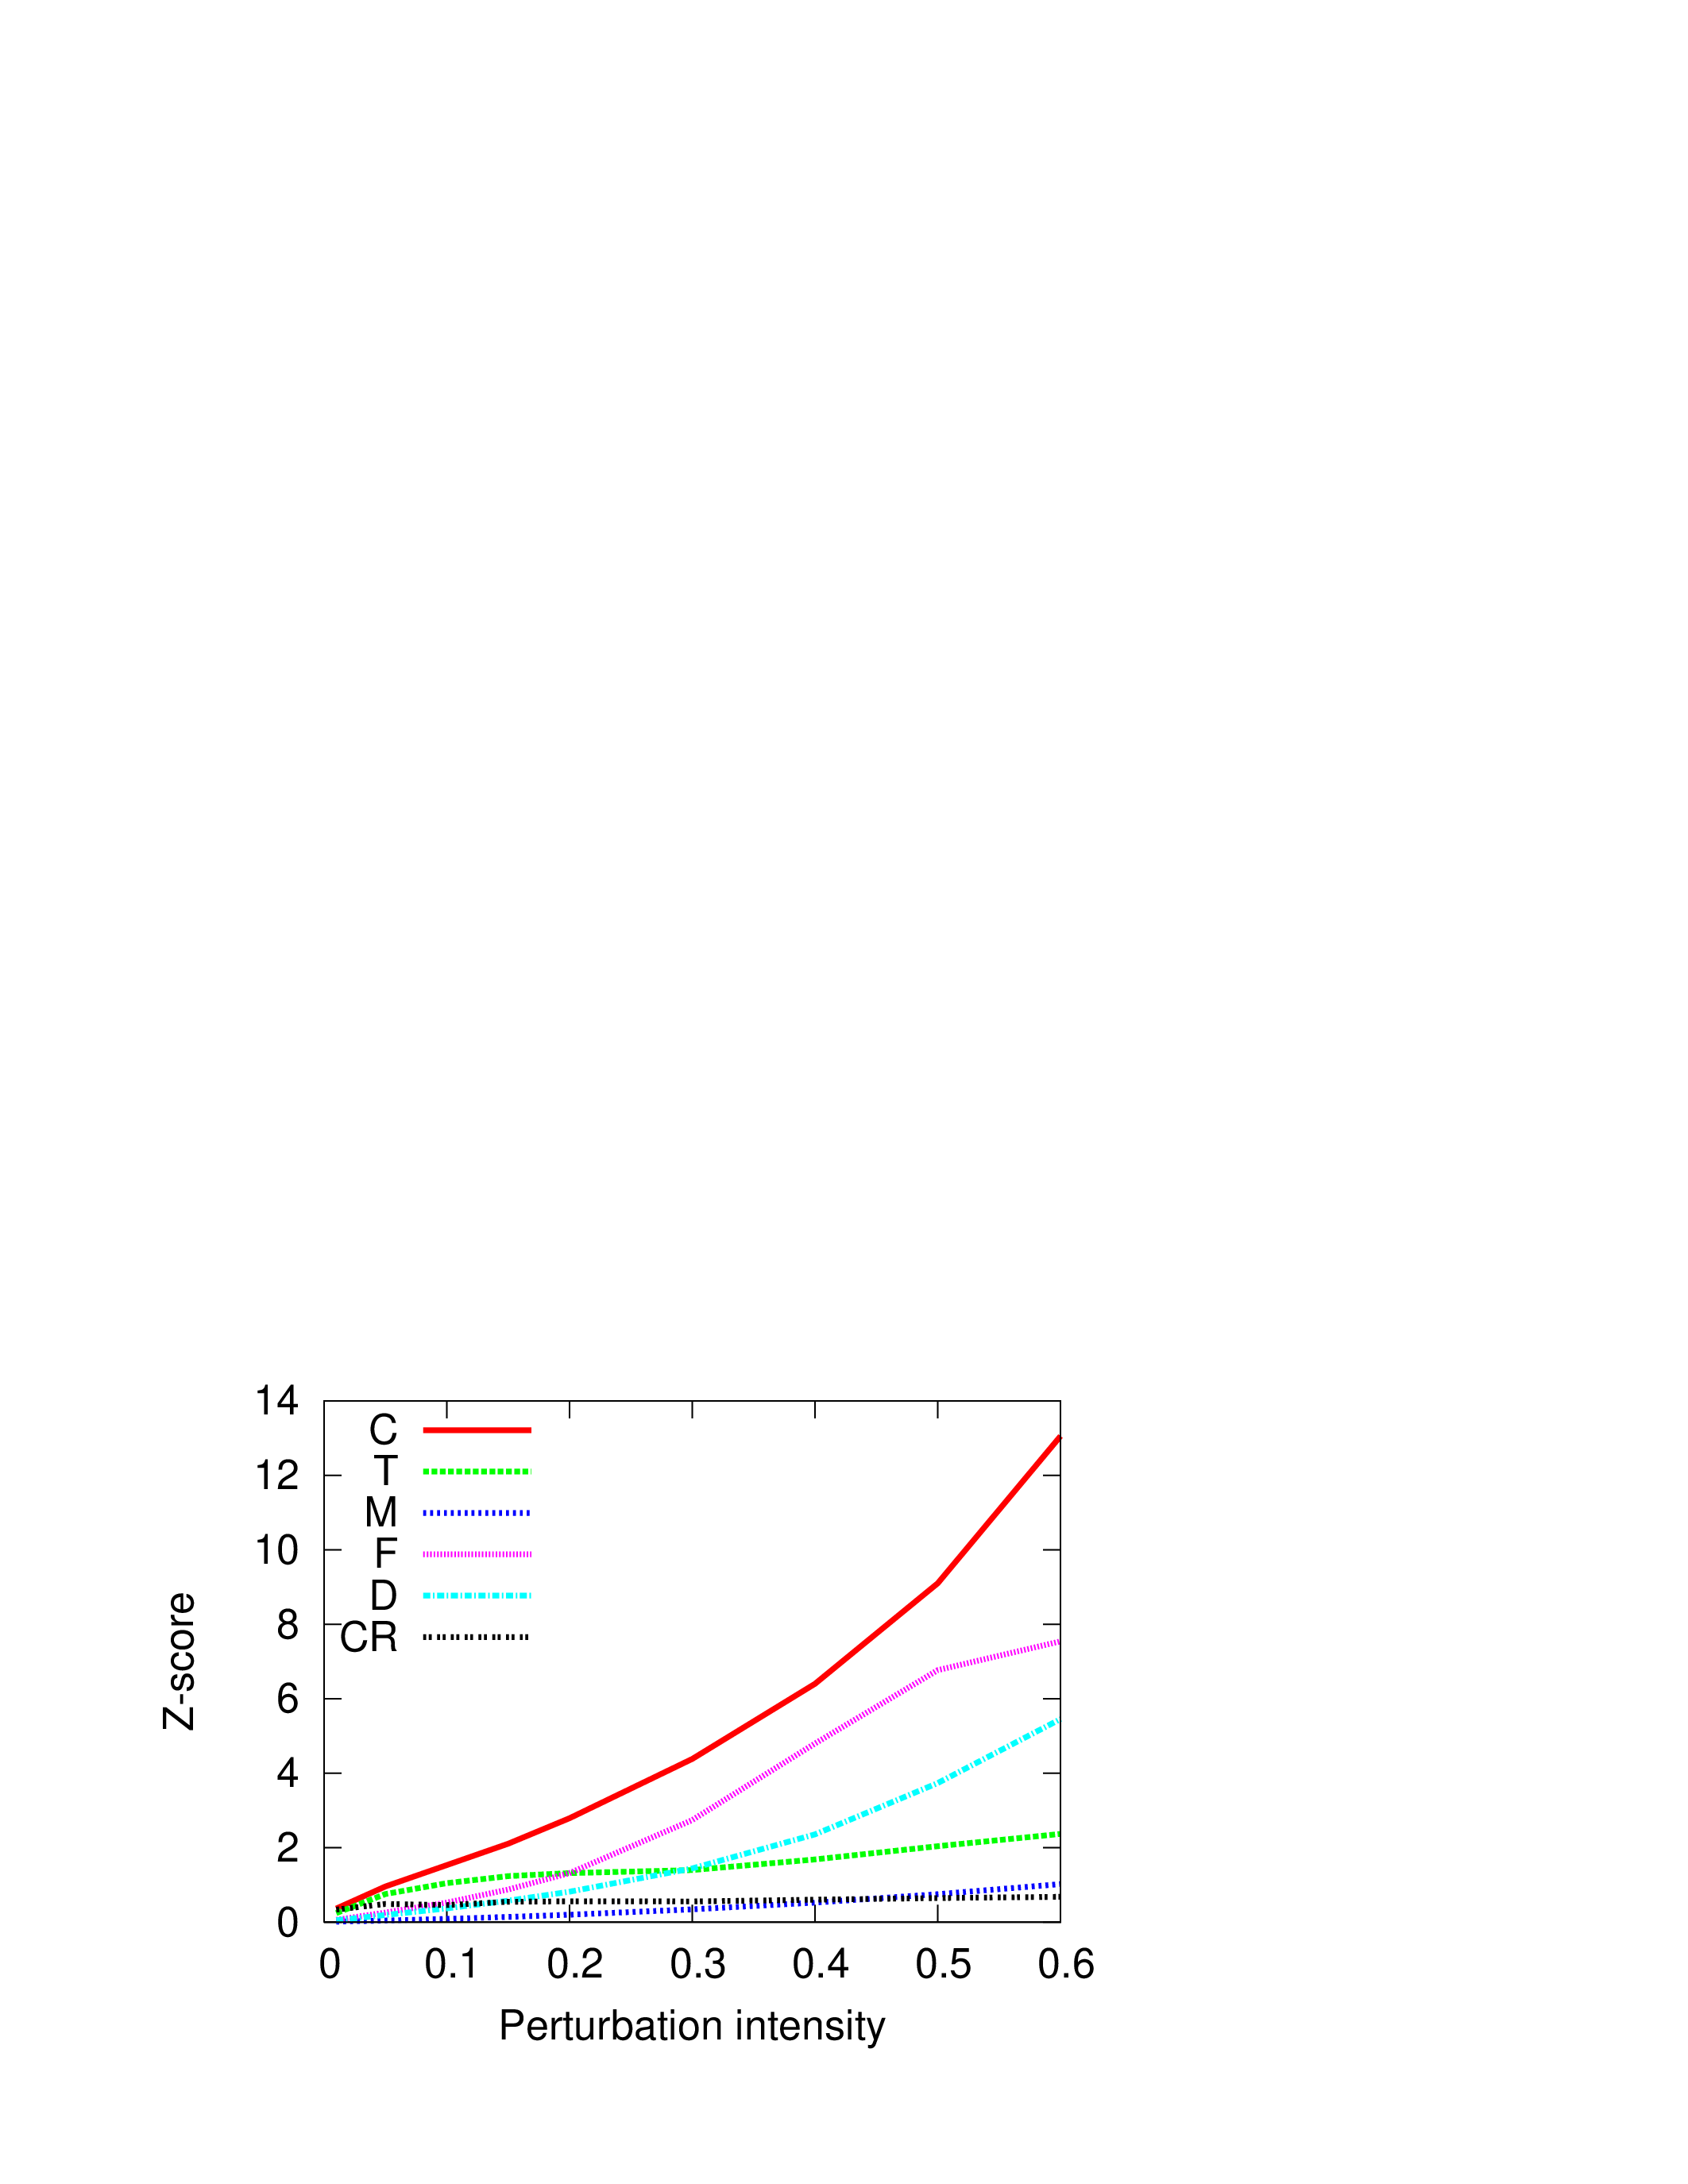}}
	\subfigure[NS	(Ning)]{\includegraphics[width=0.15\textwidth]{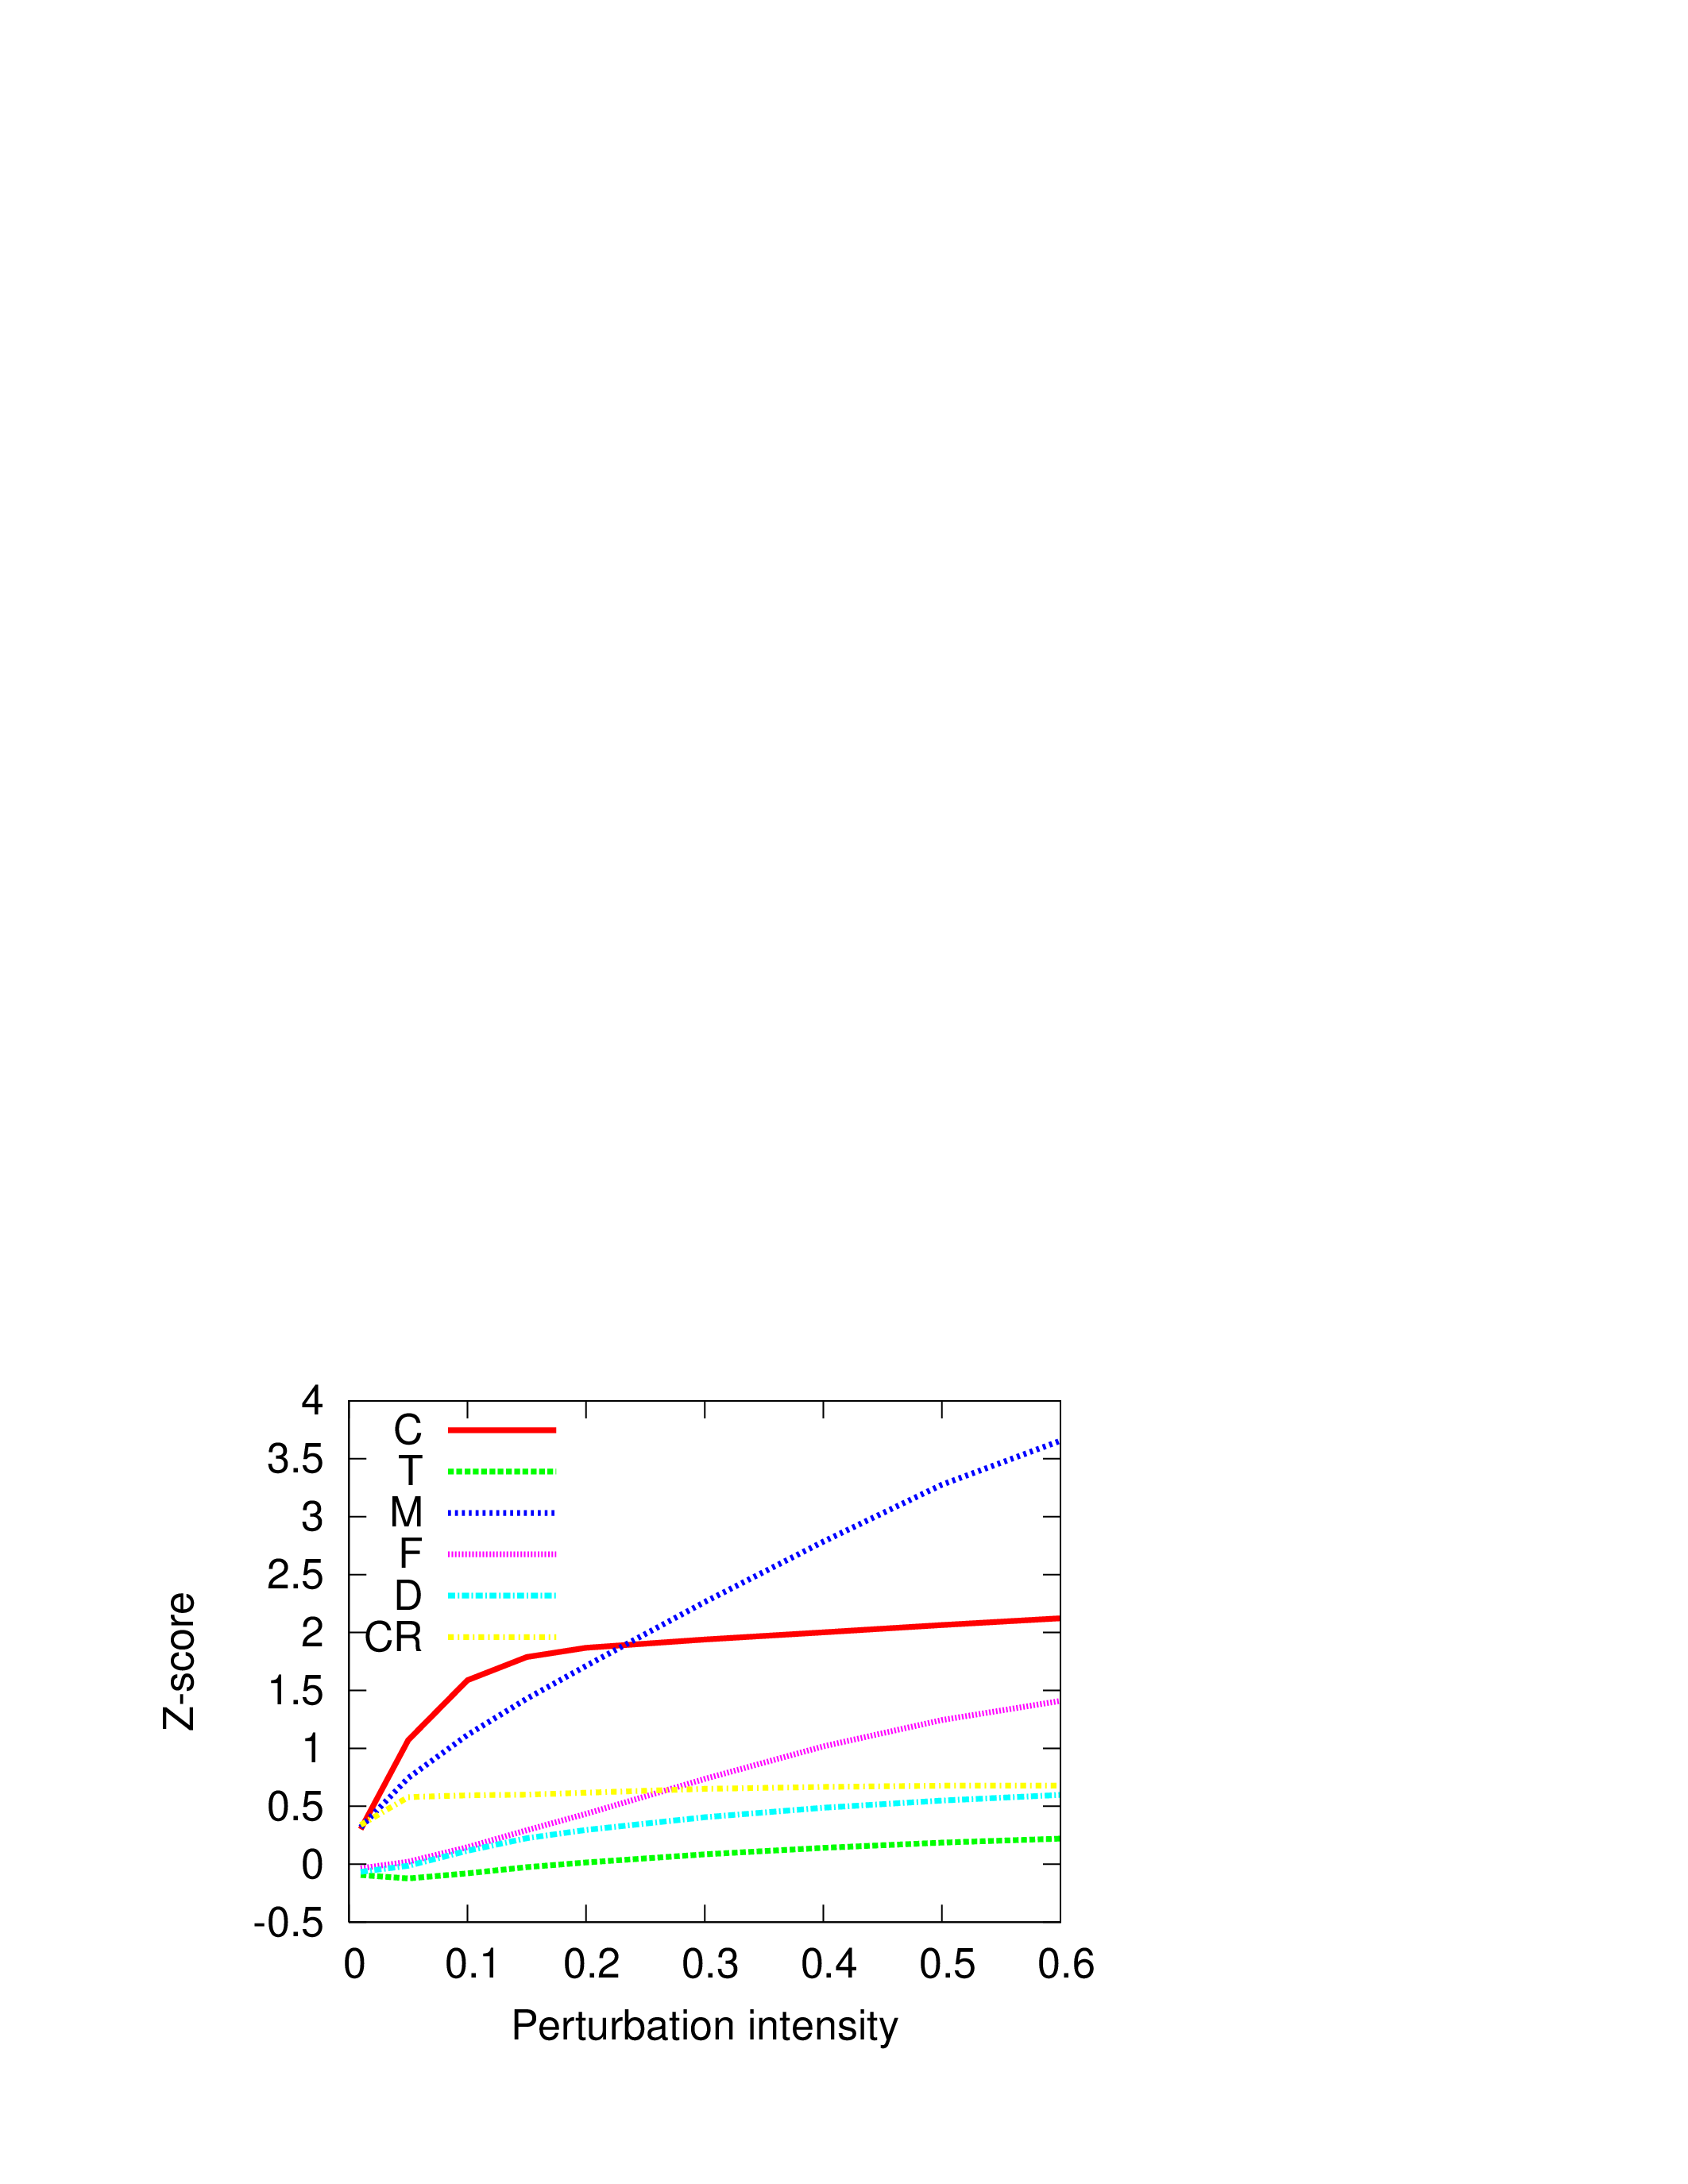}}
	\subfigure[NS	(Amazon)]{\includegraphics[width=0.15\textwidth]{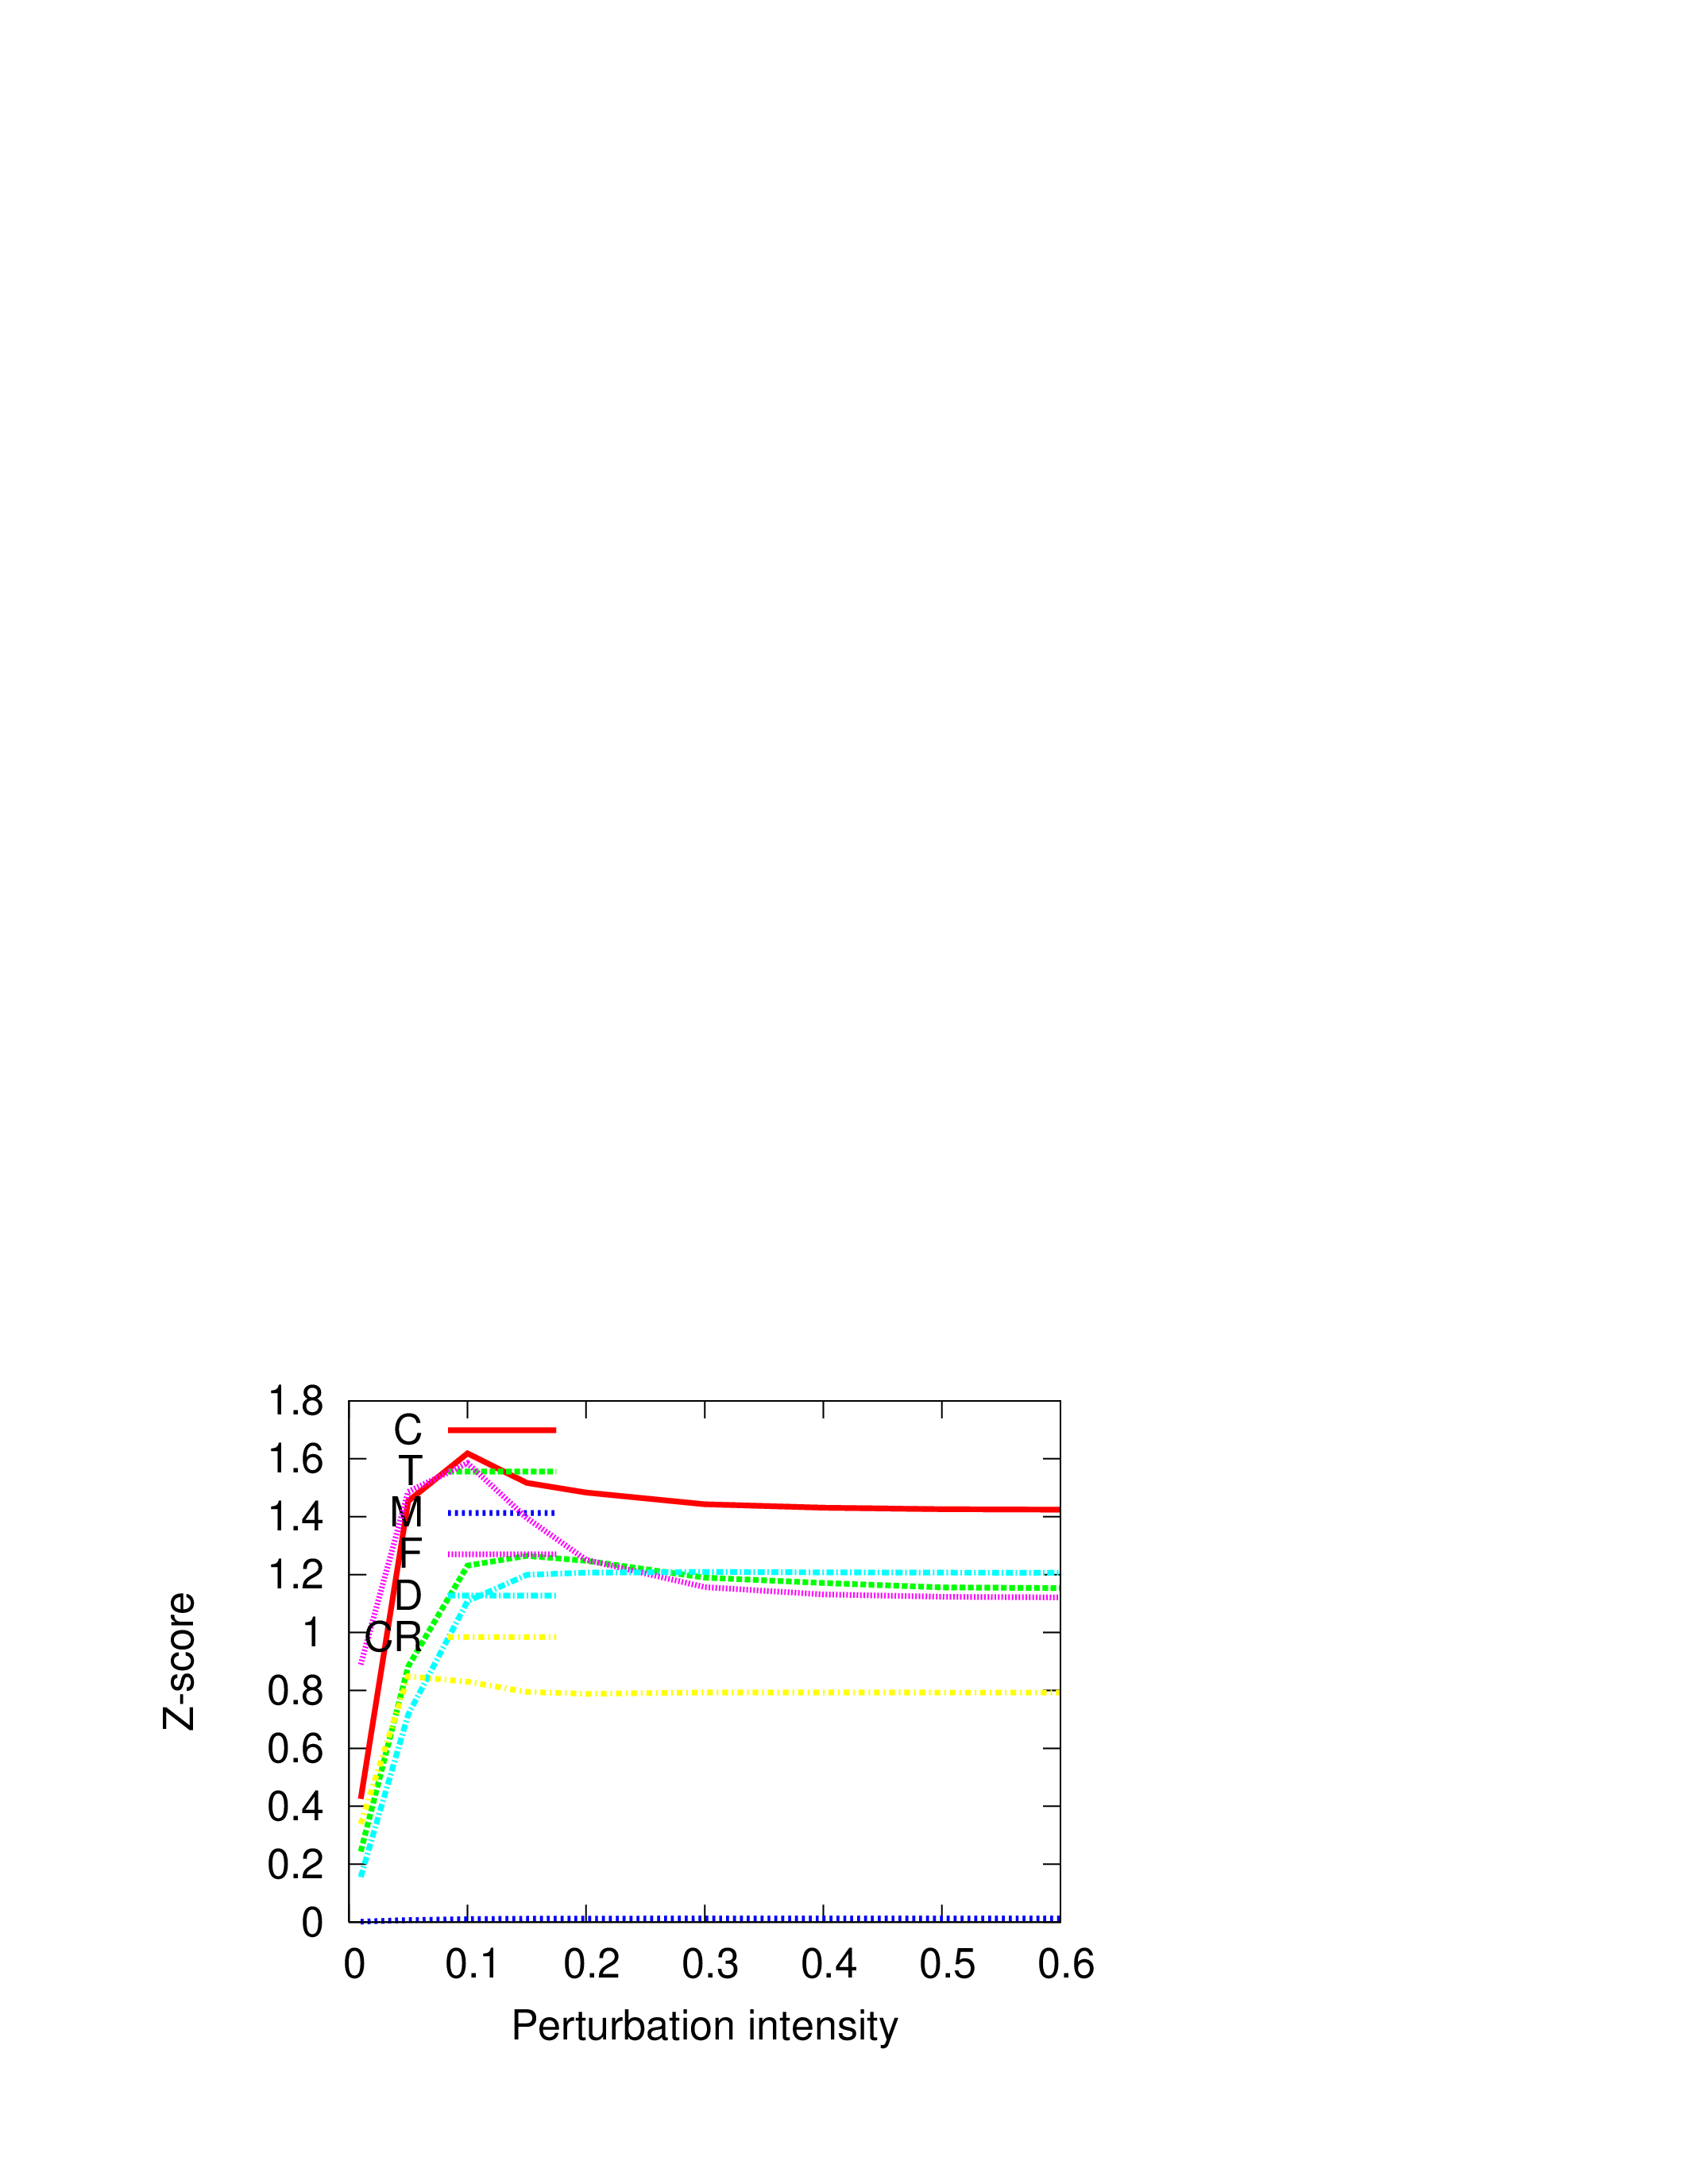}}
	\subfigure[NS	(DBLP)]{\includegraphics[width=0.15\textwidth]{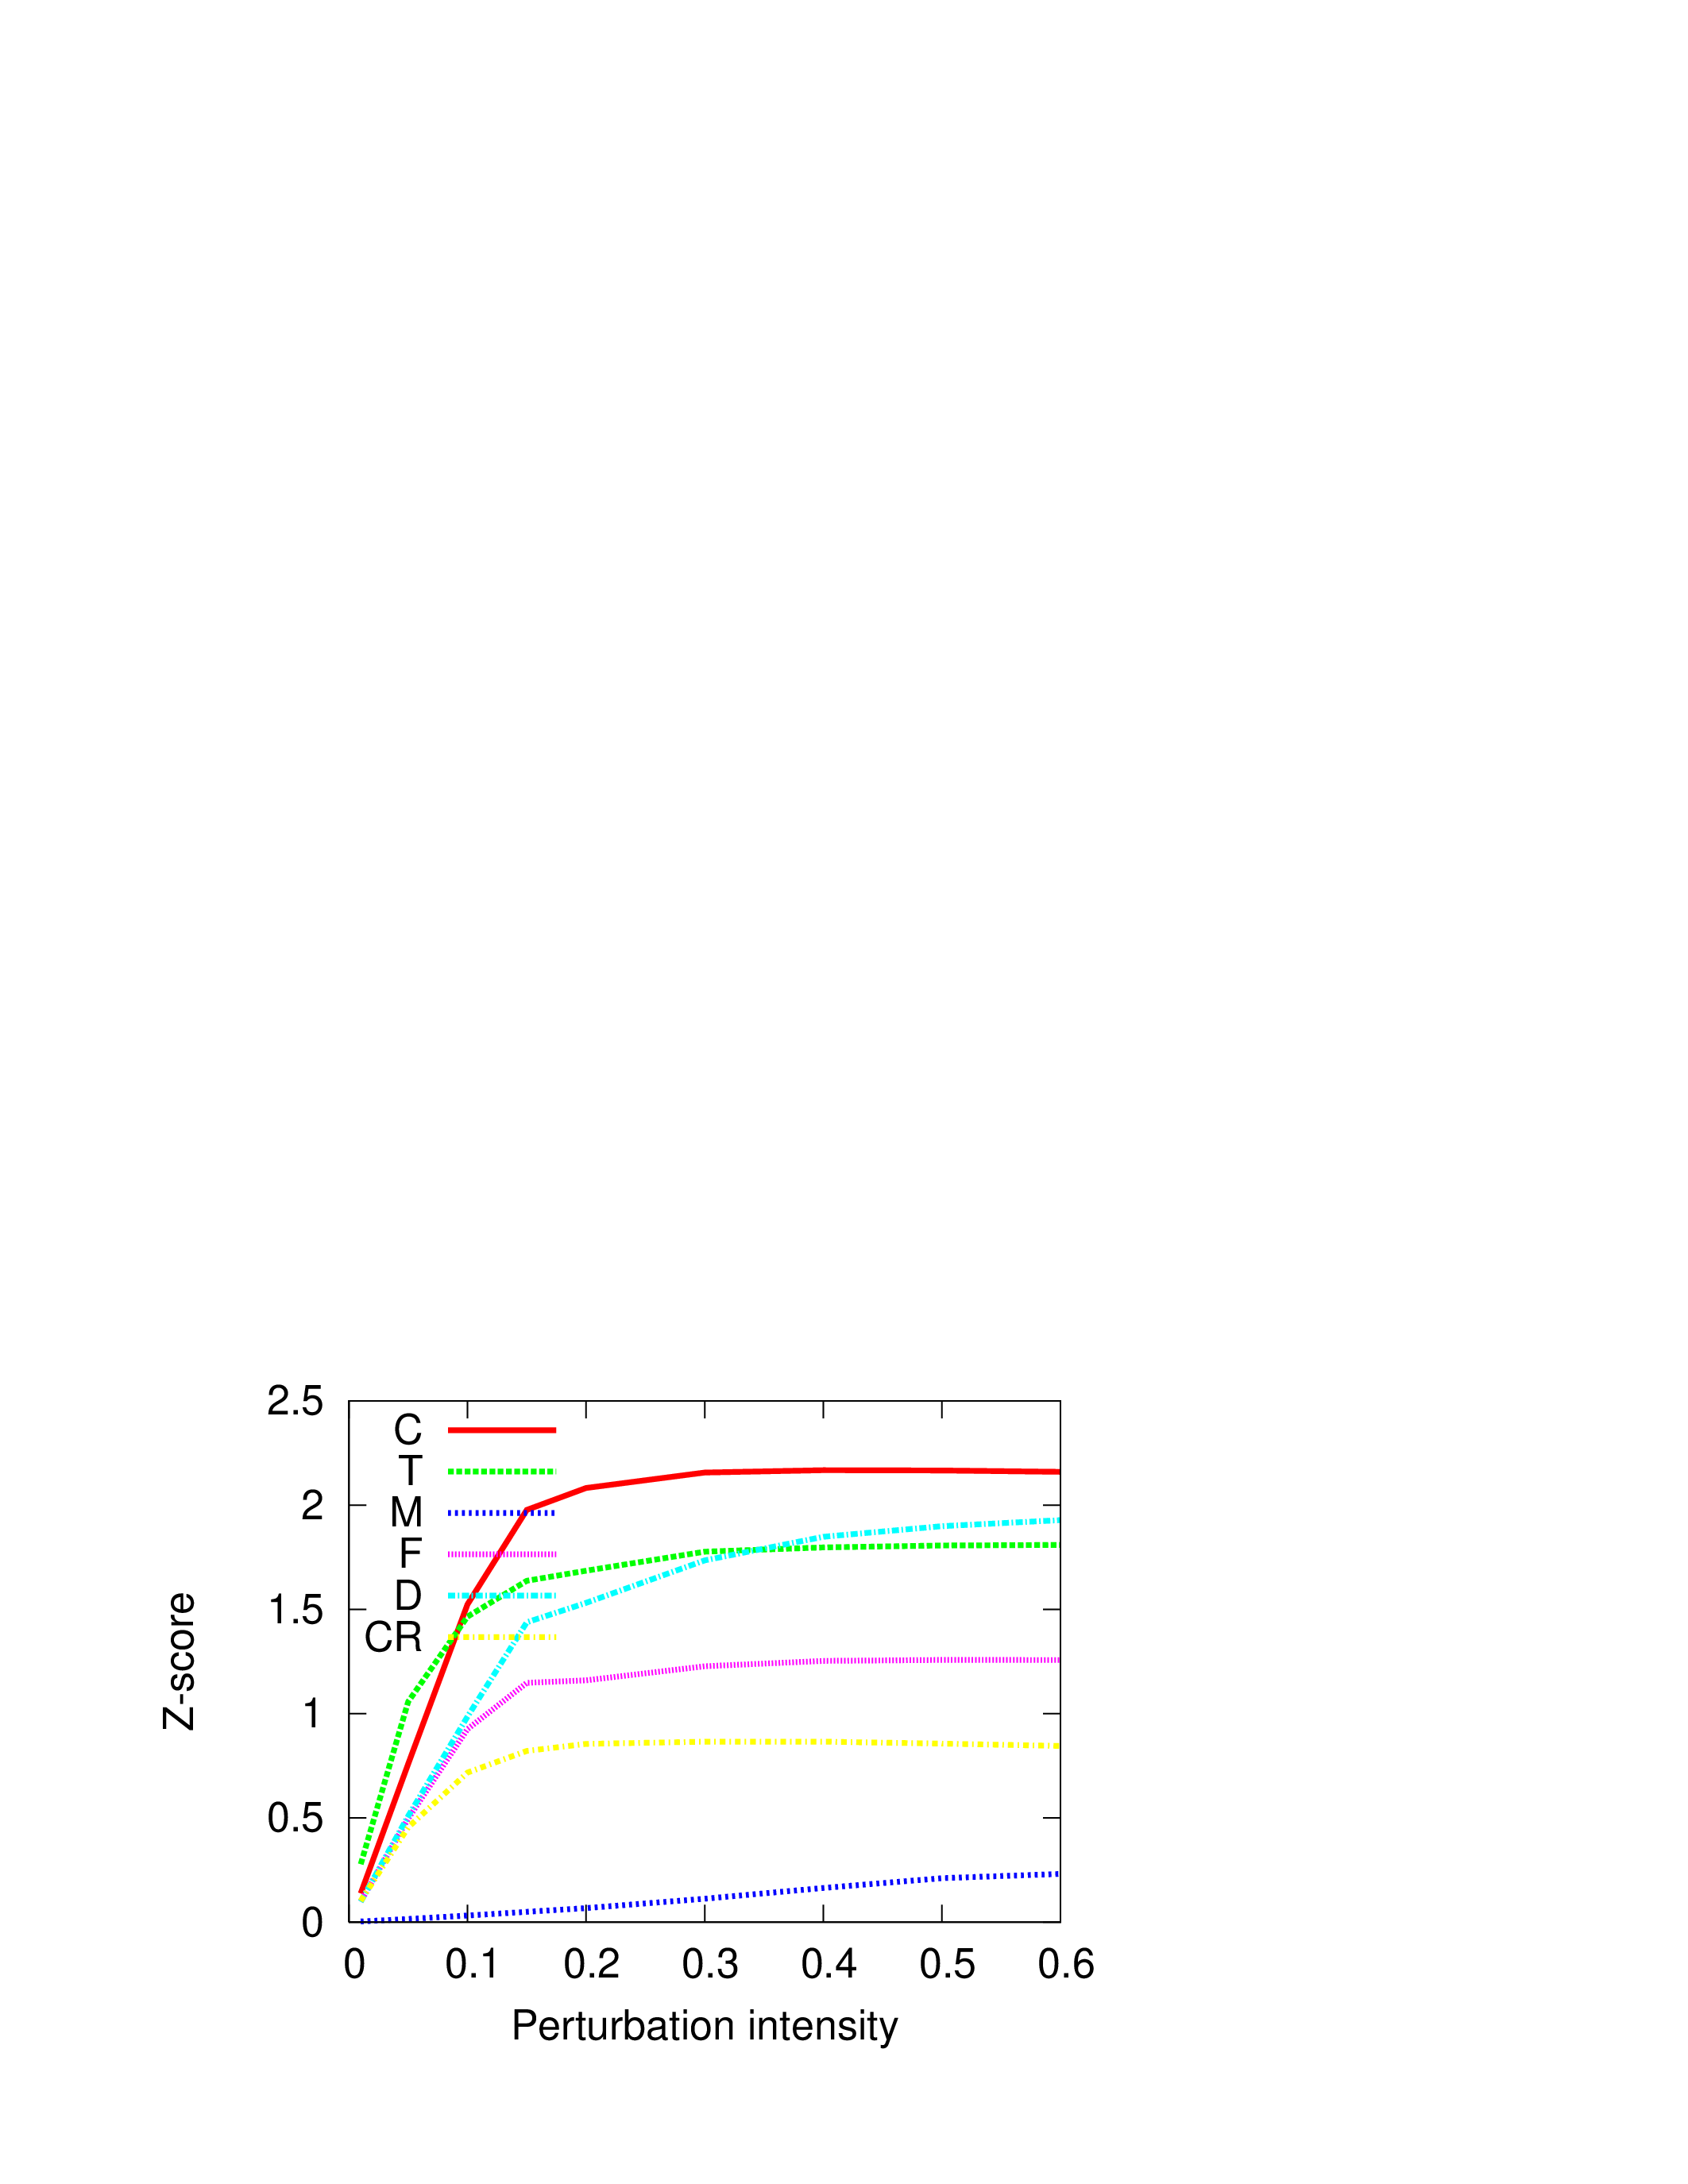}}
	\subfigure[RA	(LJ)]{\includegraphics[width=0.15\textwidth]{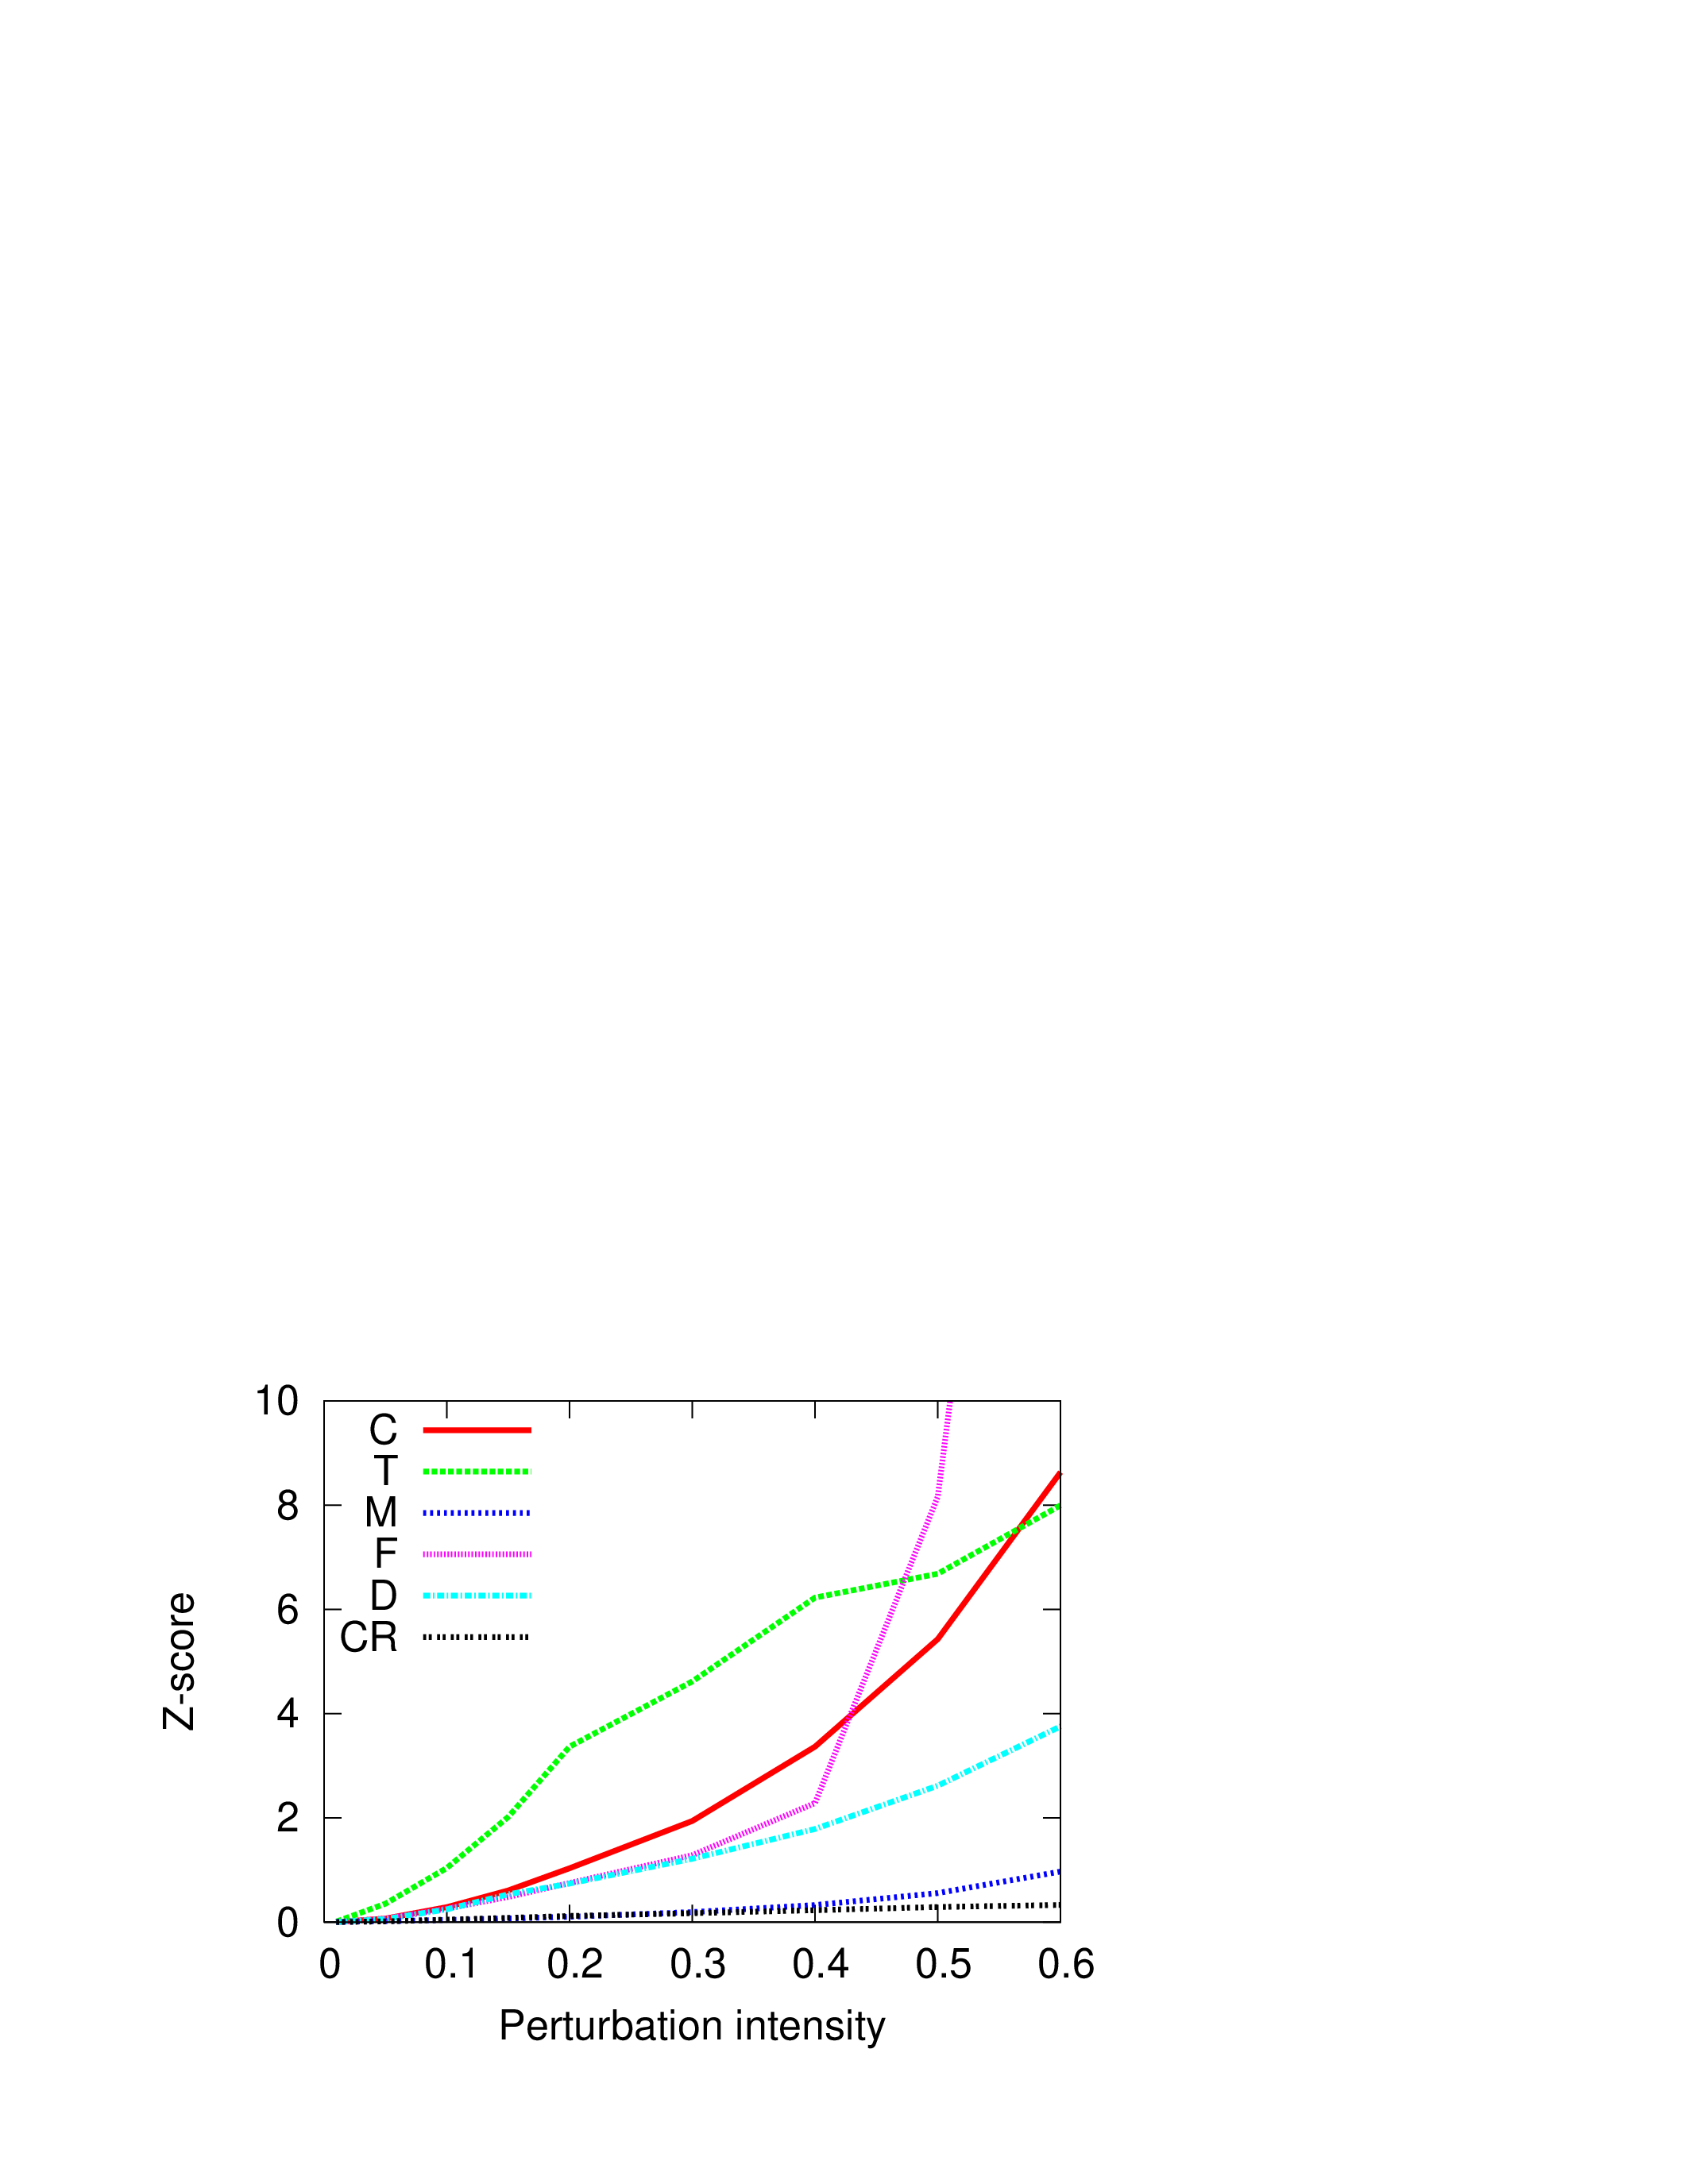}}
	\subfigure[RA	(FS)]{\includegraphics[width=0.15\textwidth]{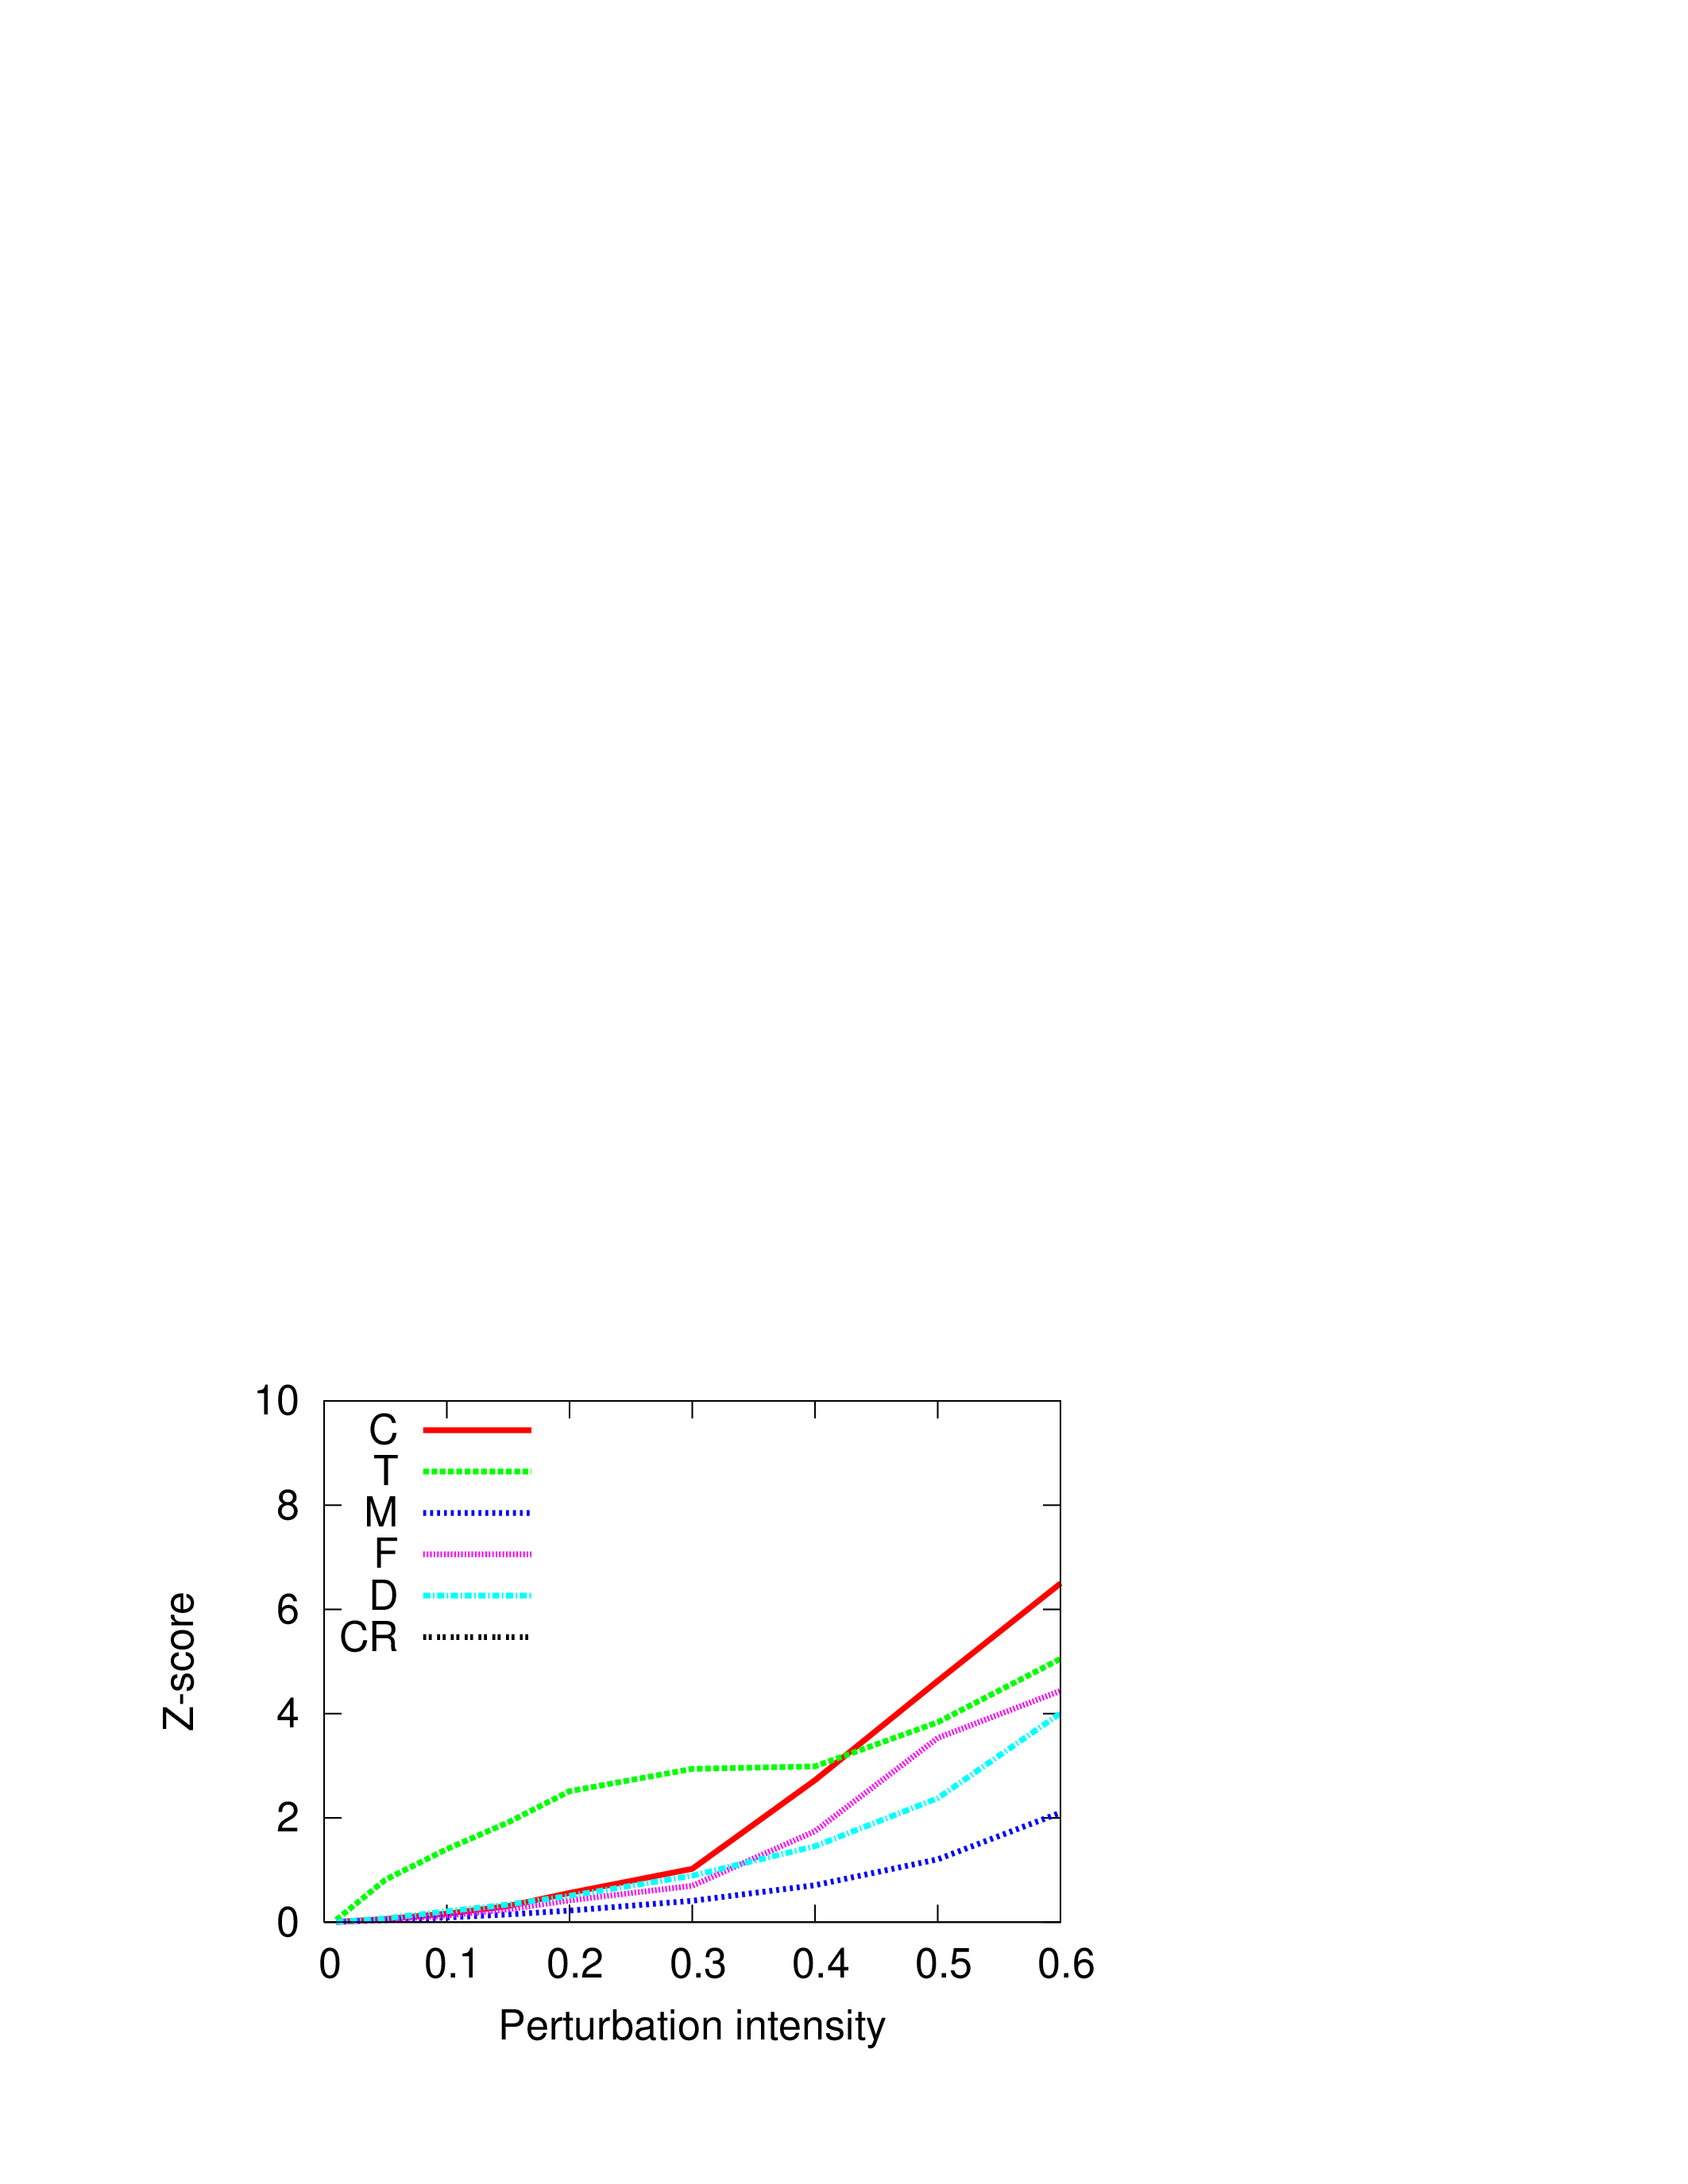}}
	\subfigure[RA	(Orkut)]{\includegraphics[width=0.15\textwidth]{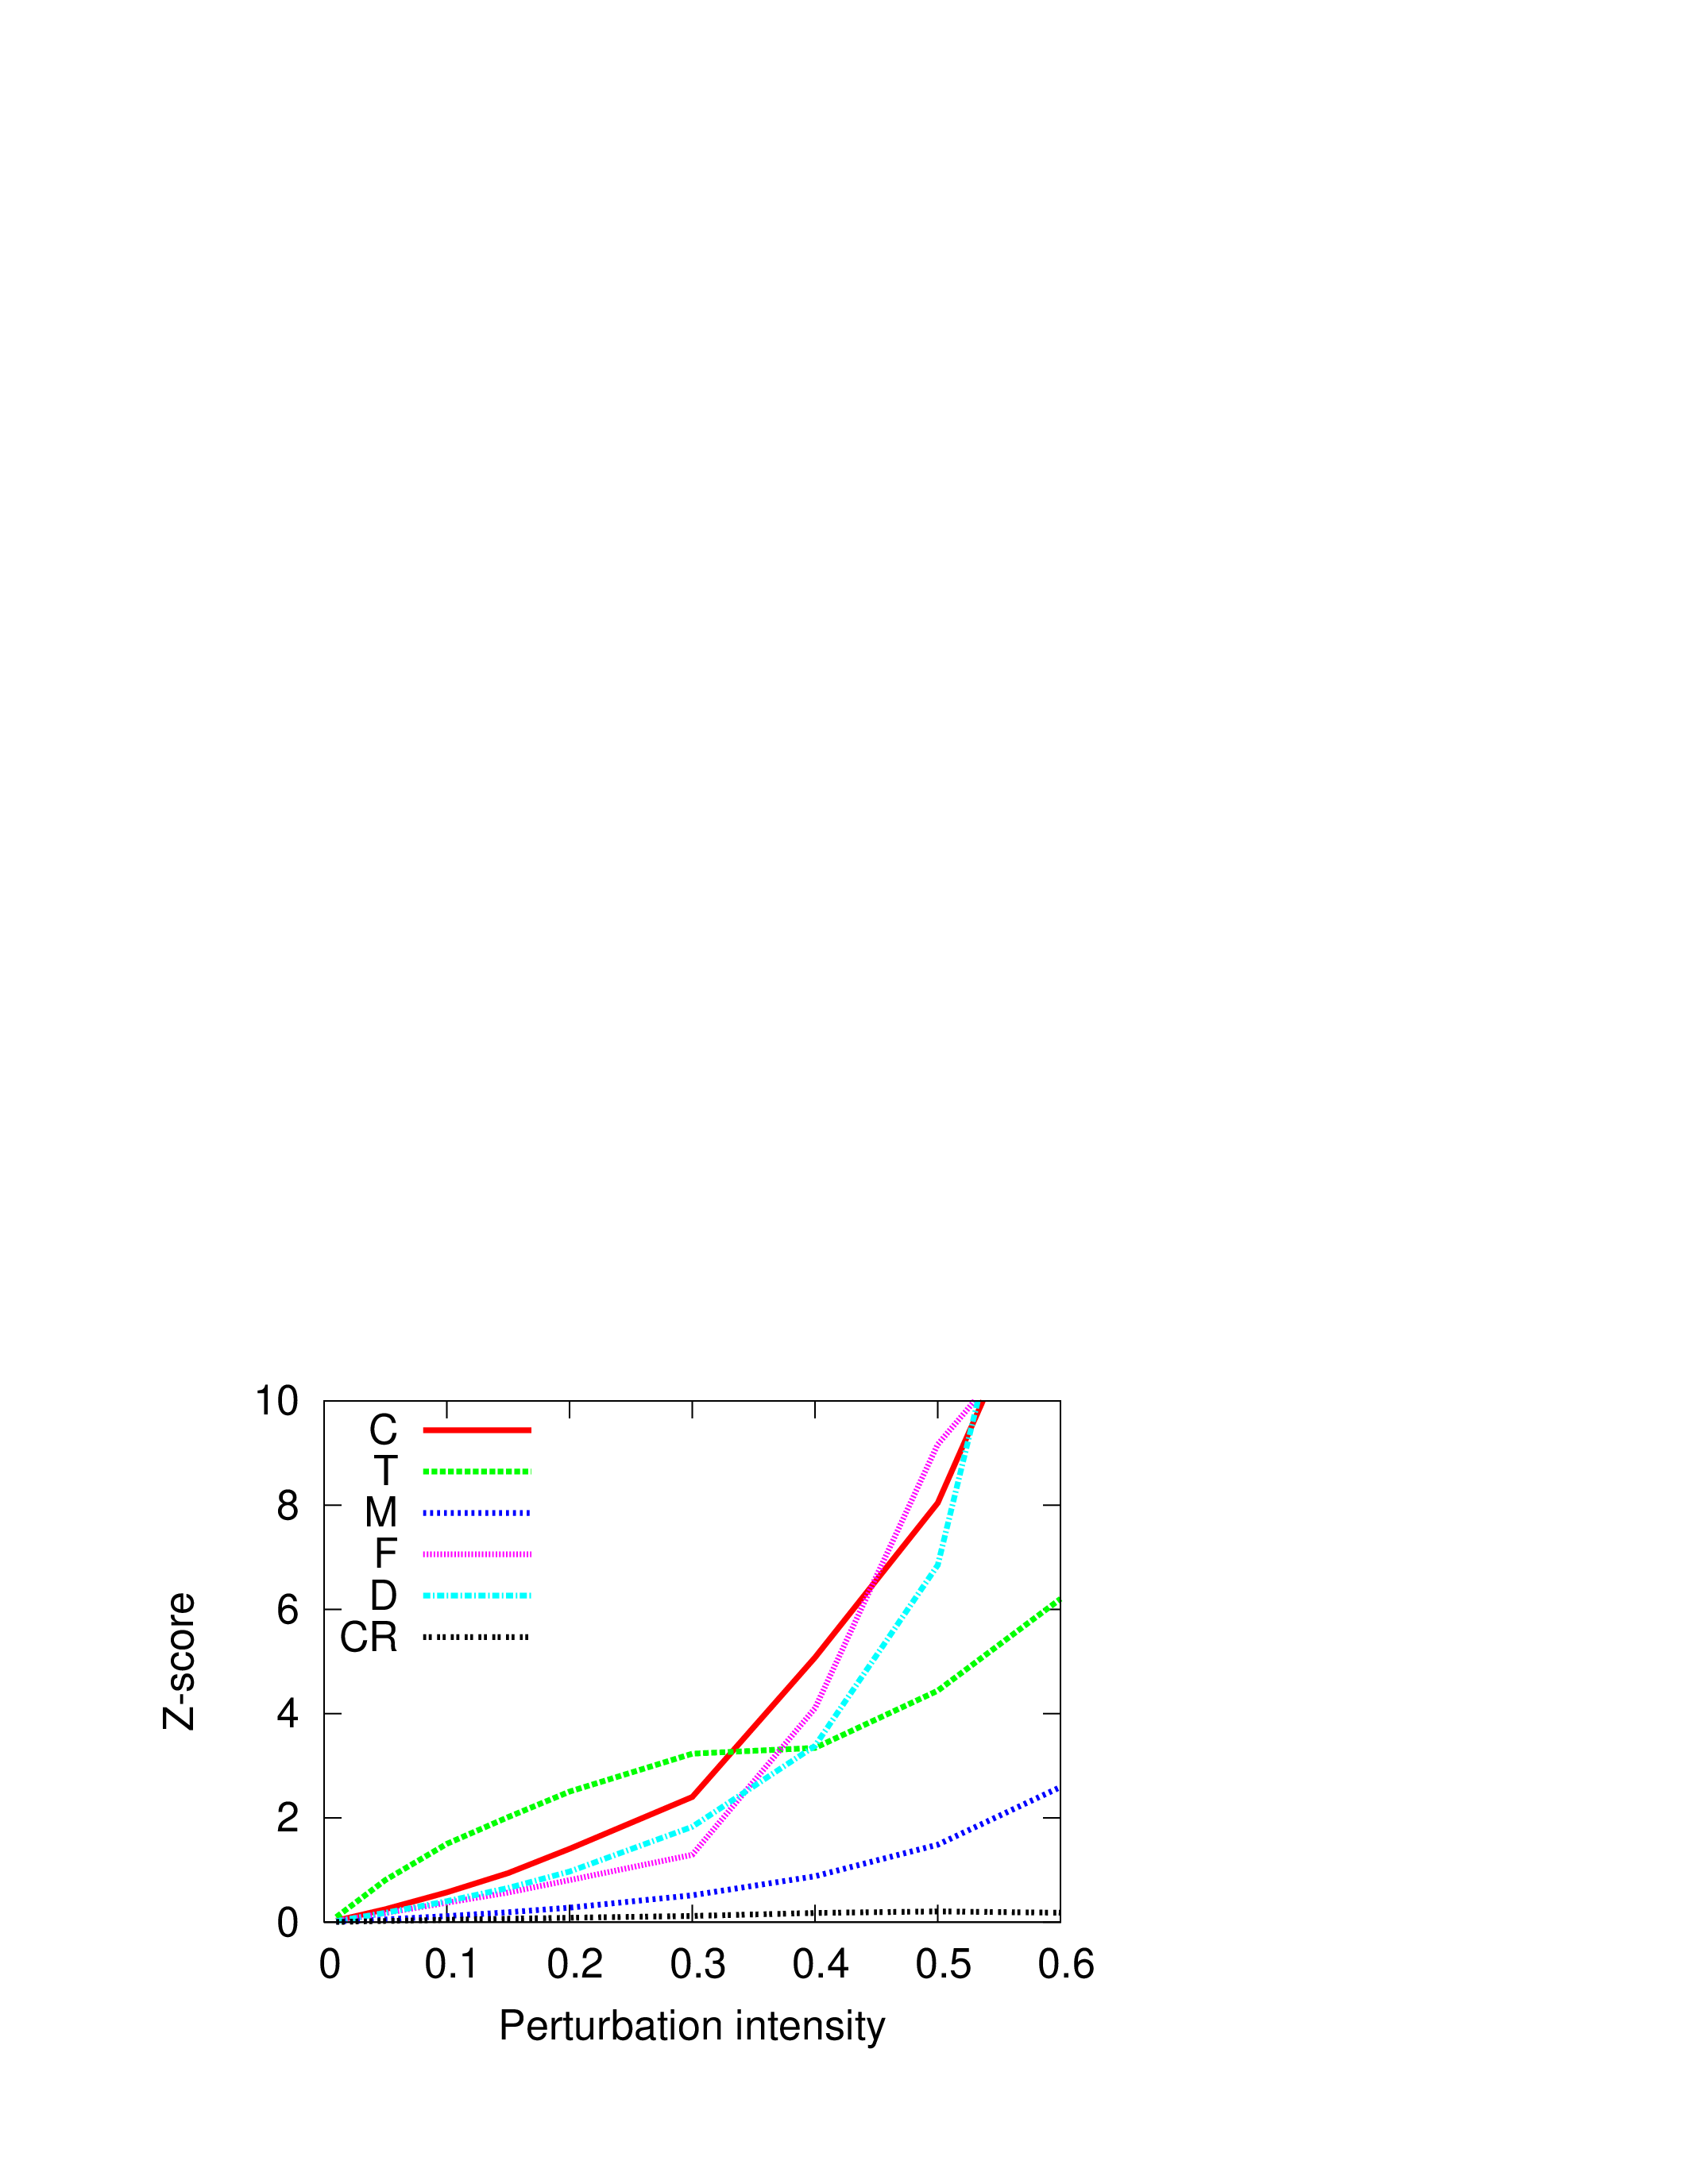}}
	\subfigure[RA	(Ning)]{\includegraphics[width=0.15\textwidth]{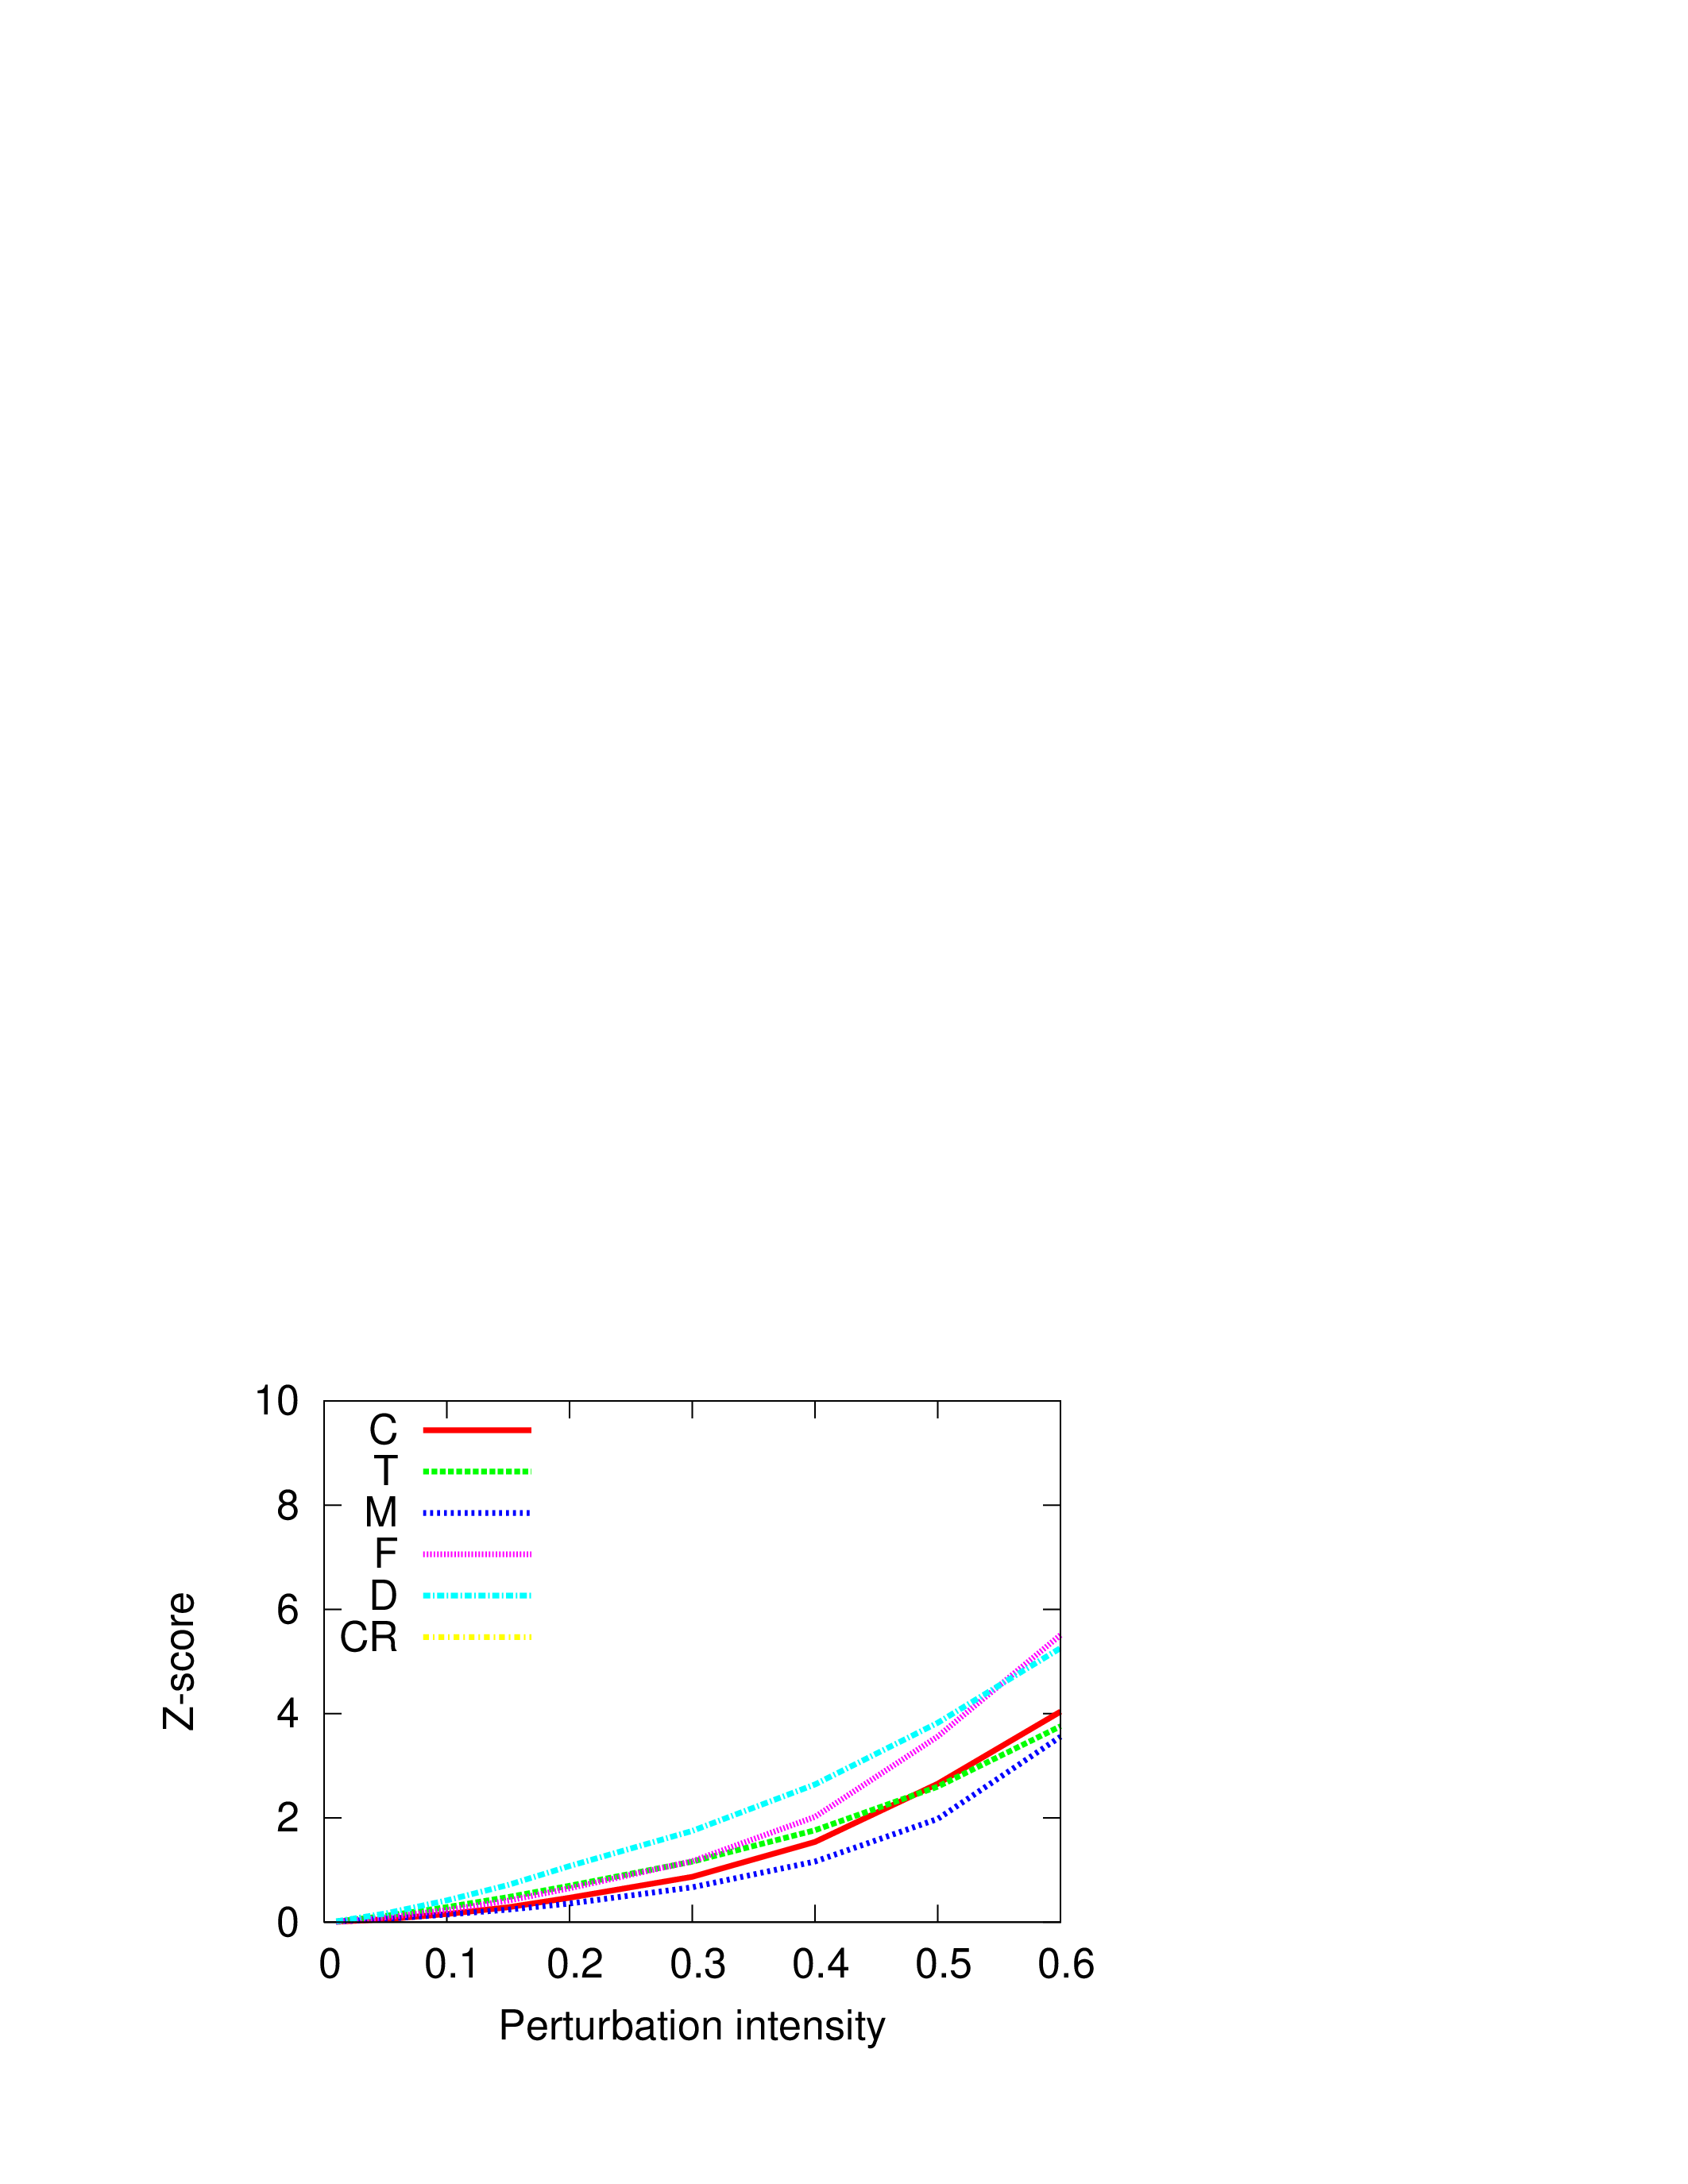}}
	\subfigure[RA	(Amazon)]{\includegraphics[width=0.15\textwidth]{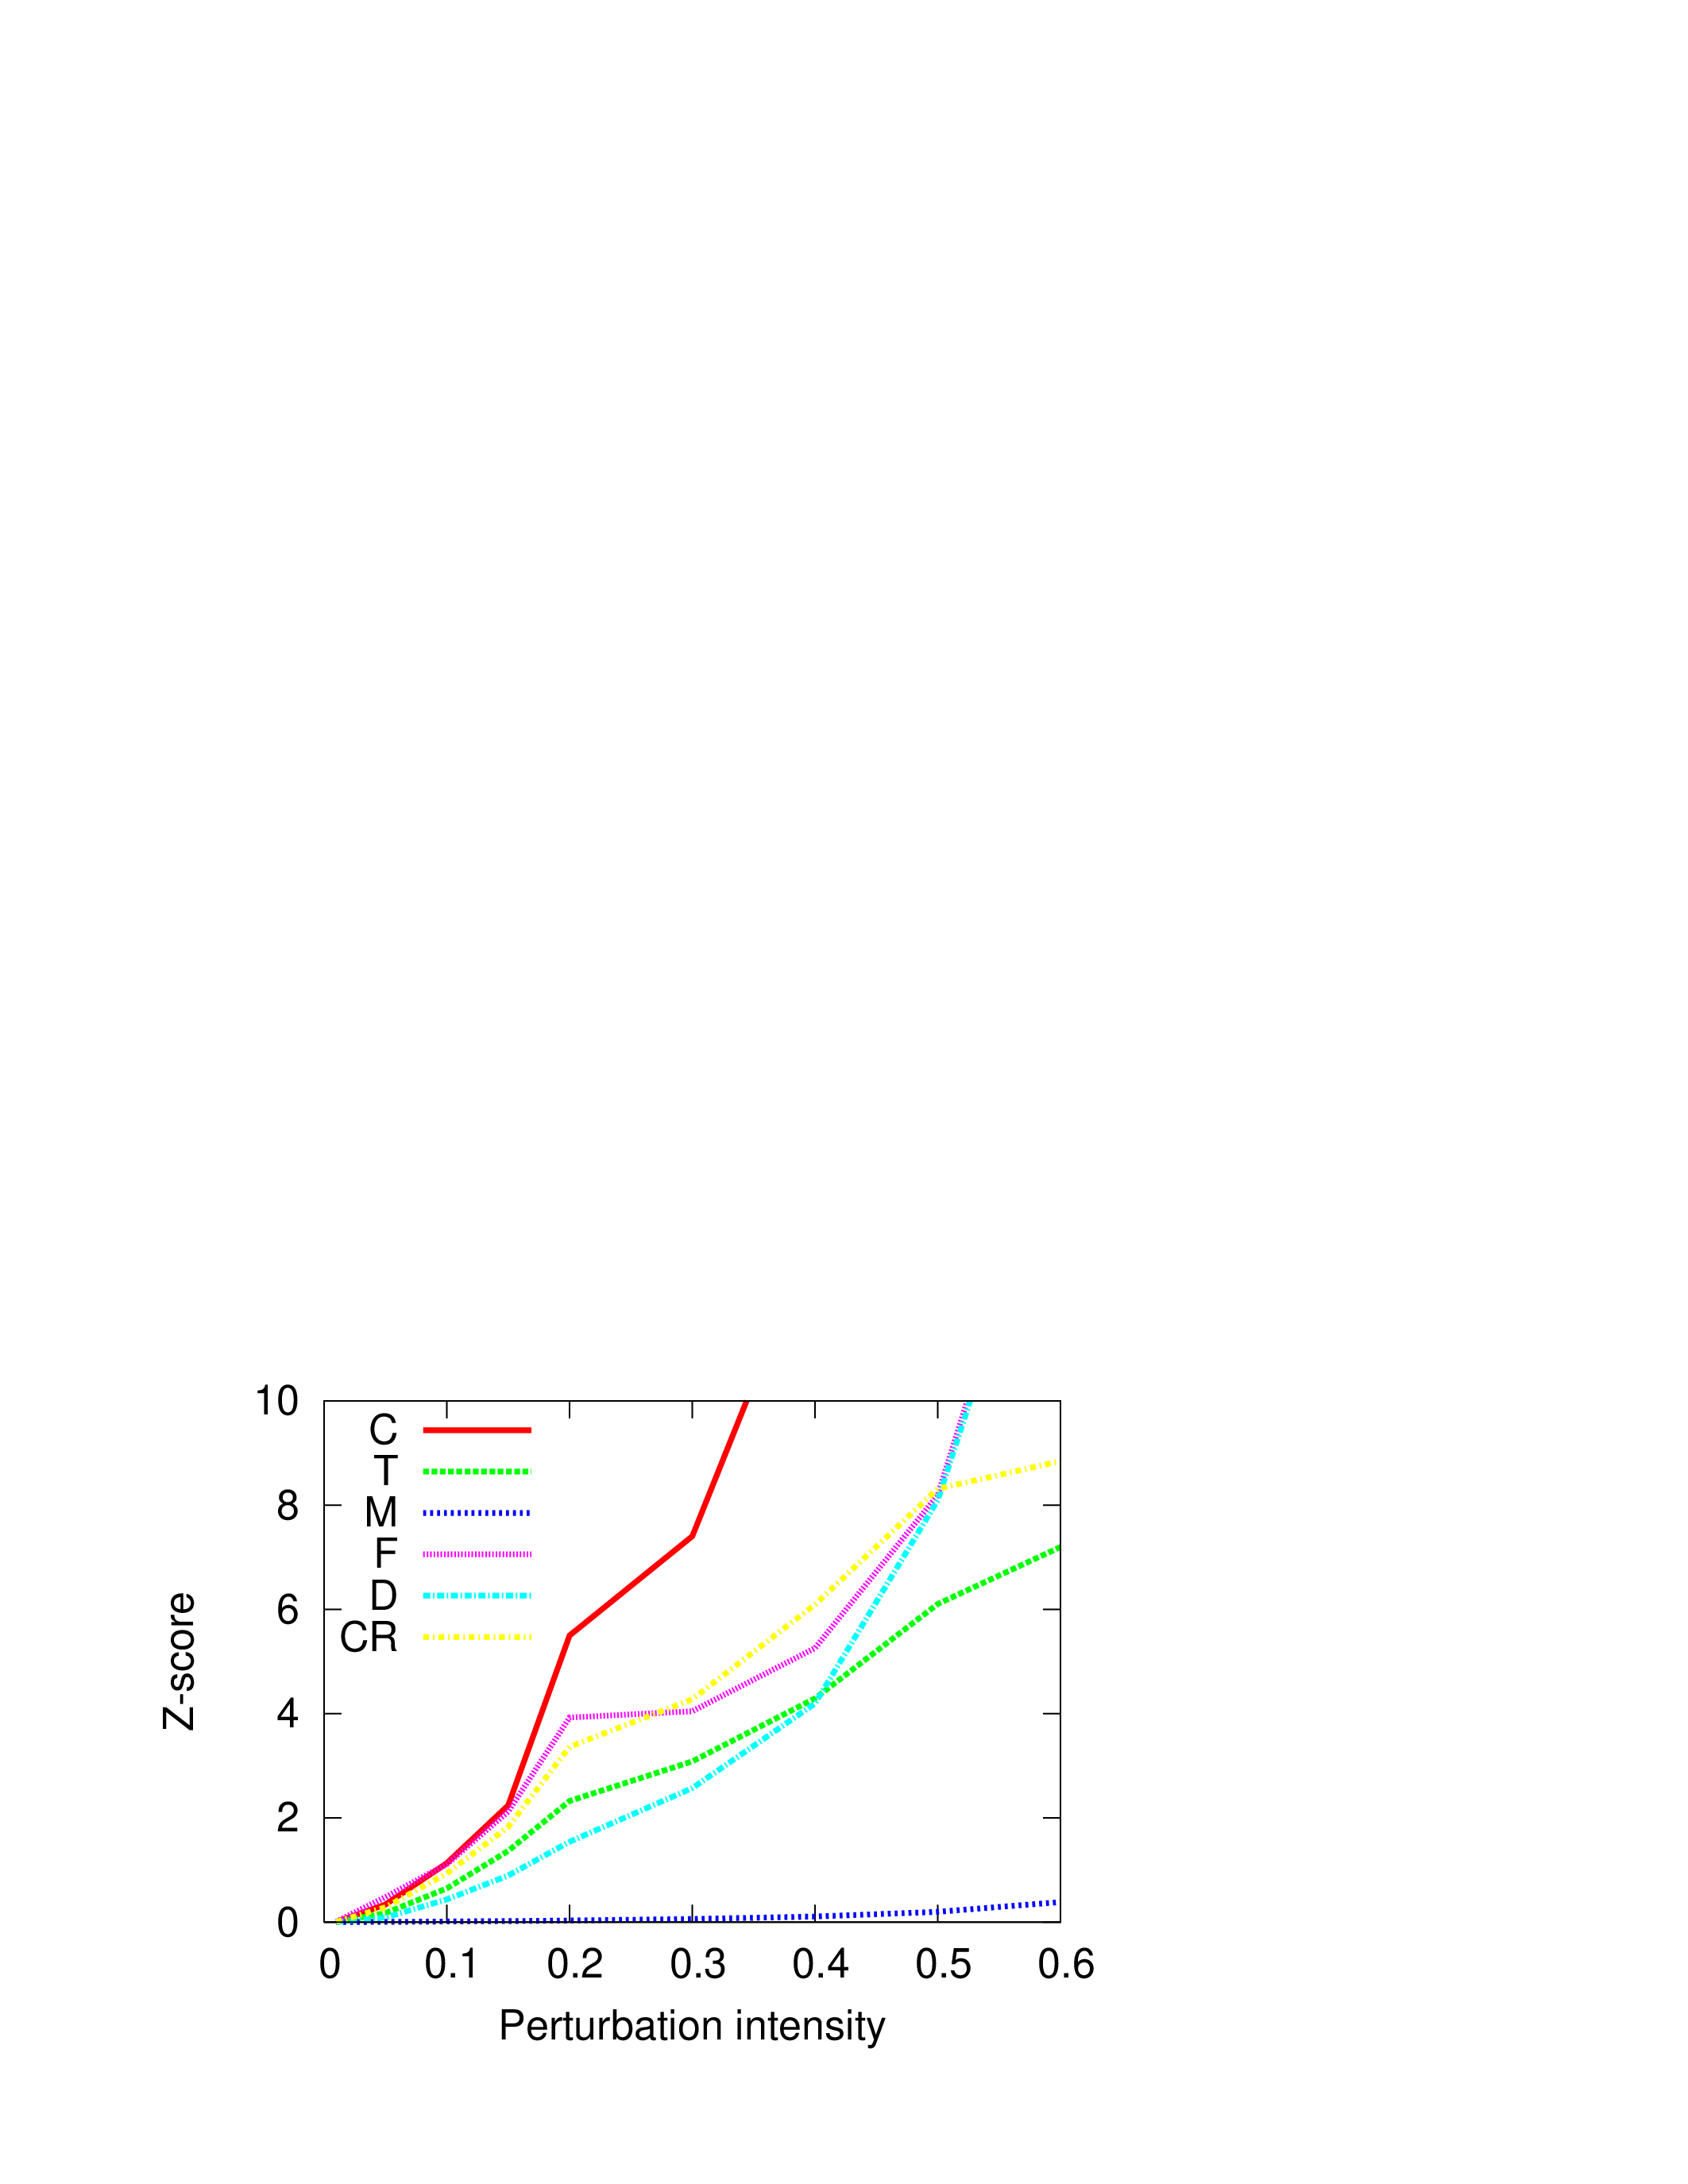}}
	\subfigure[RA	(DBLP)]{\includegraphics[width=0.15\textwidth]{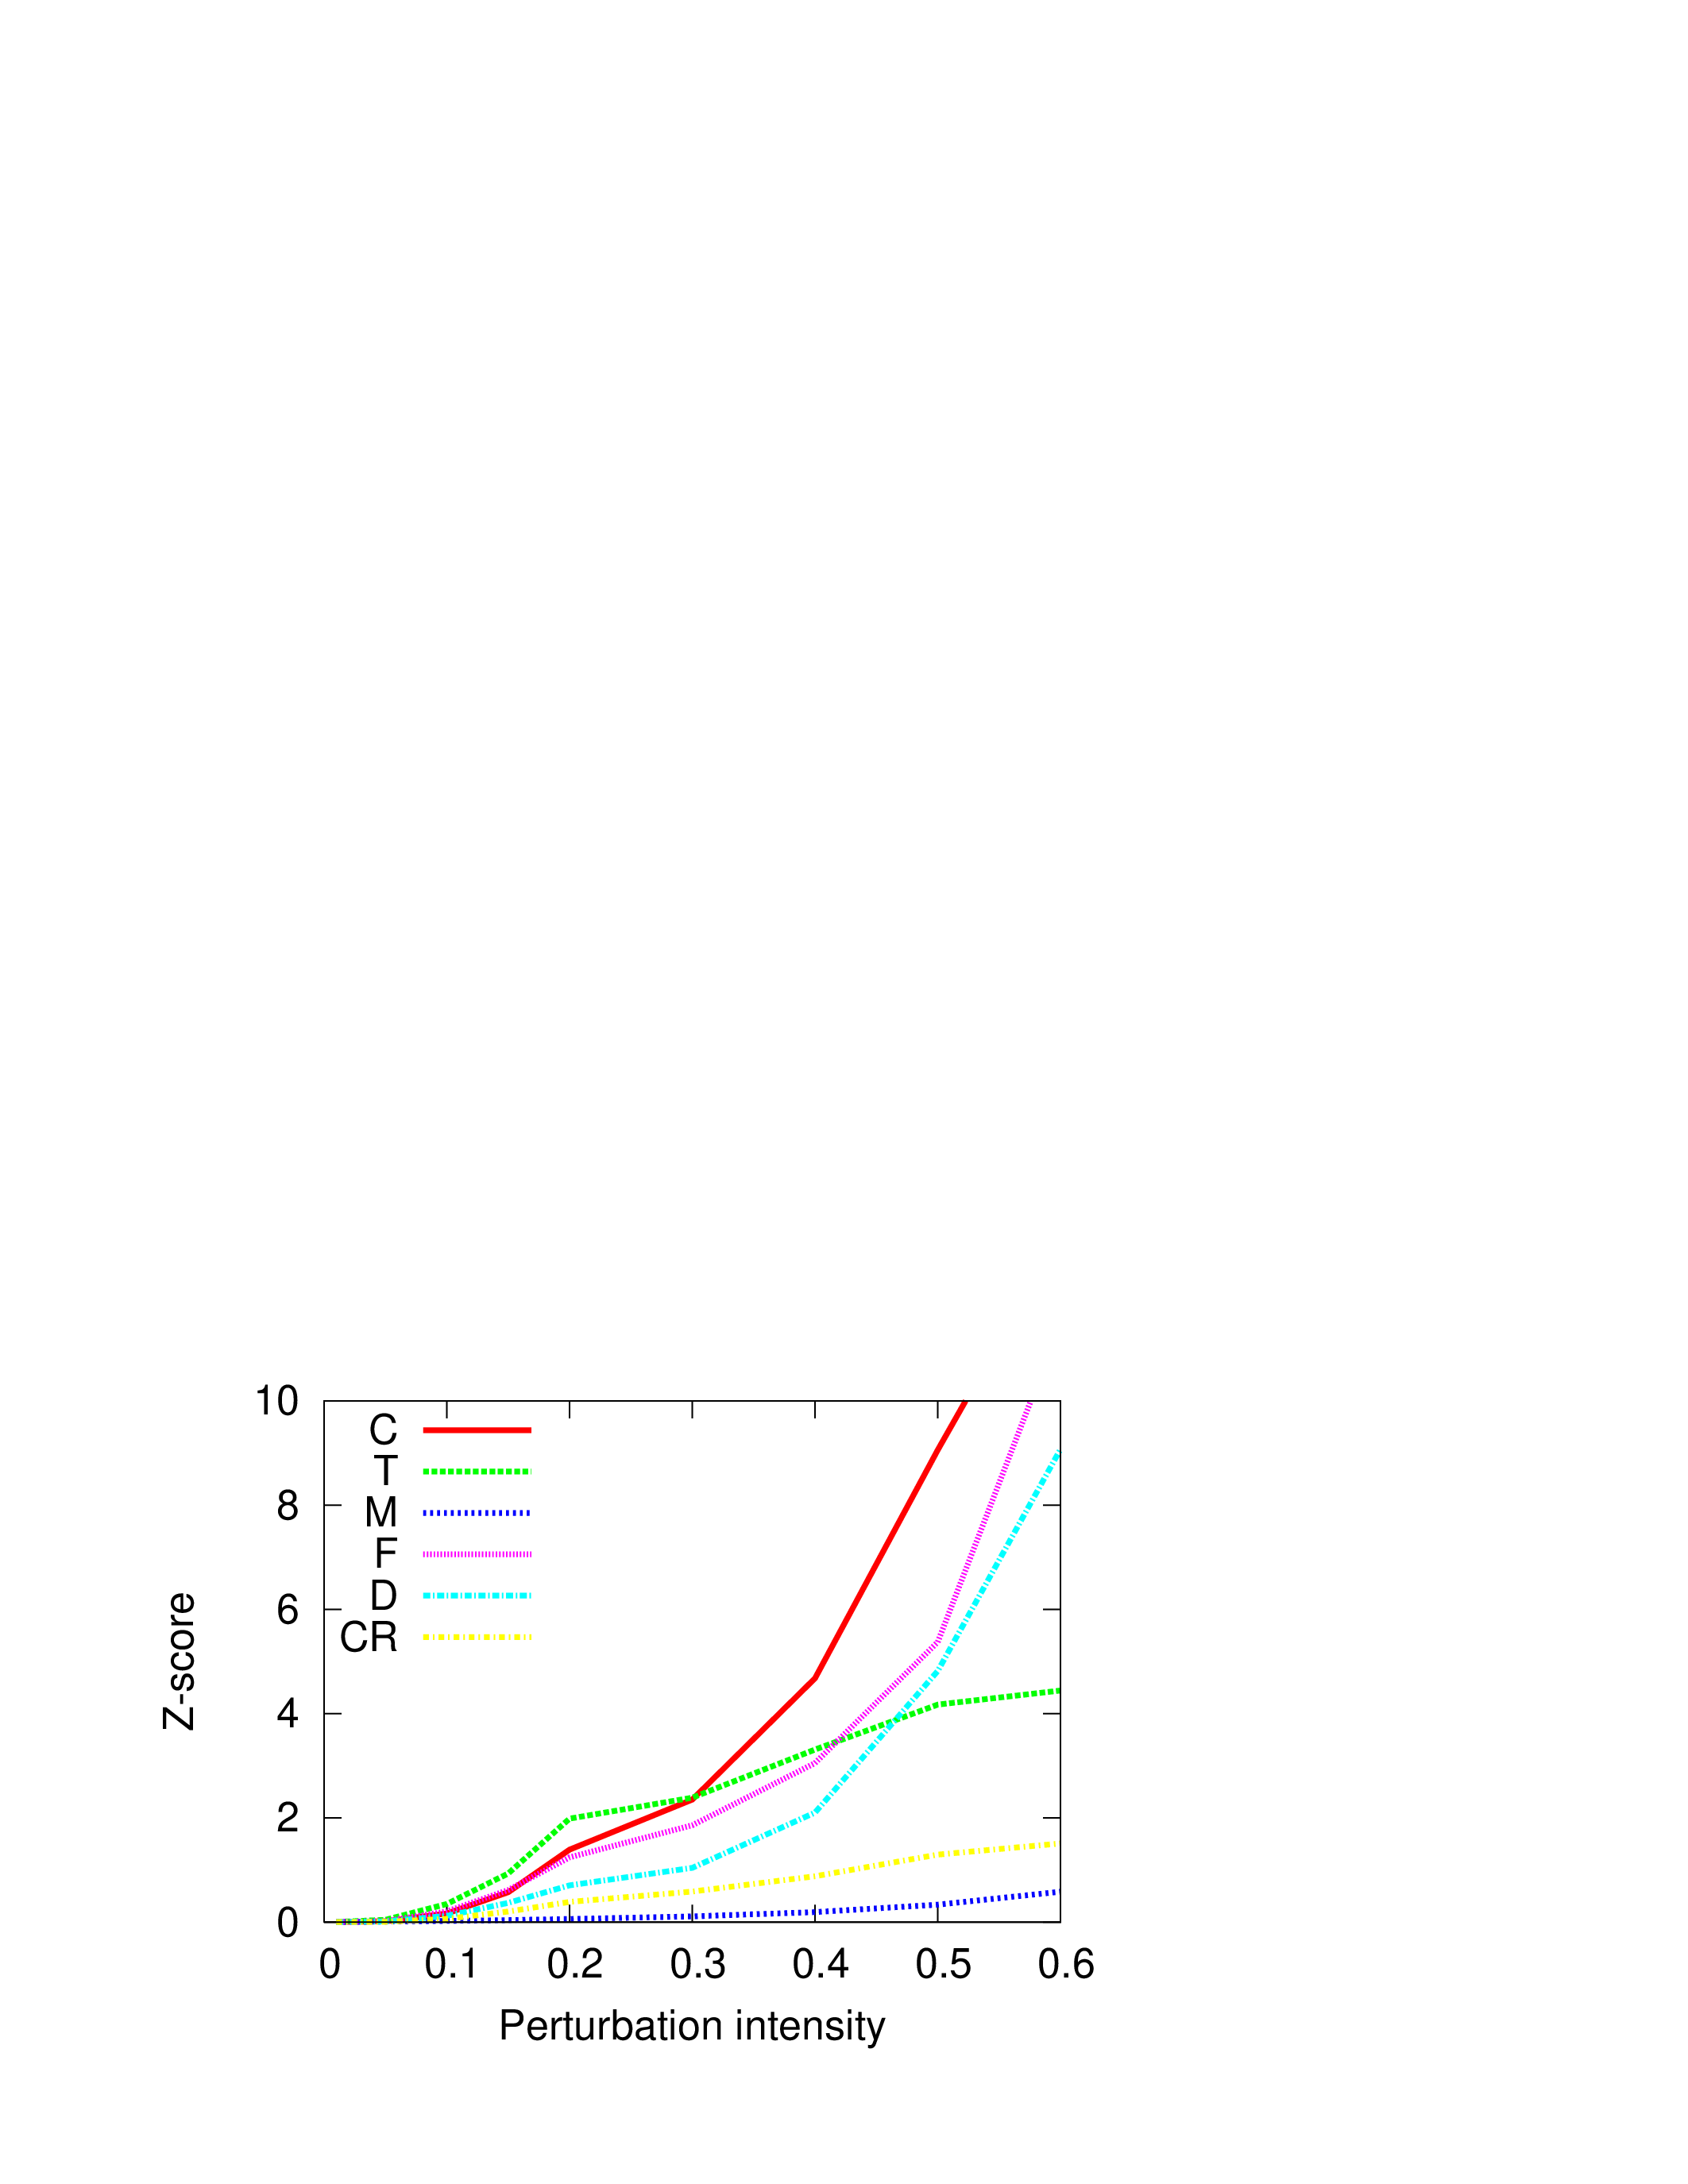}}
	\subfigure[EX	(LJ)]{\includegraphics[width=0.15\textwidth]{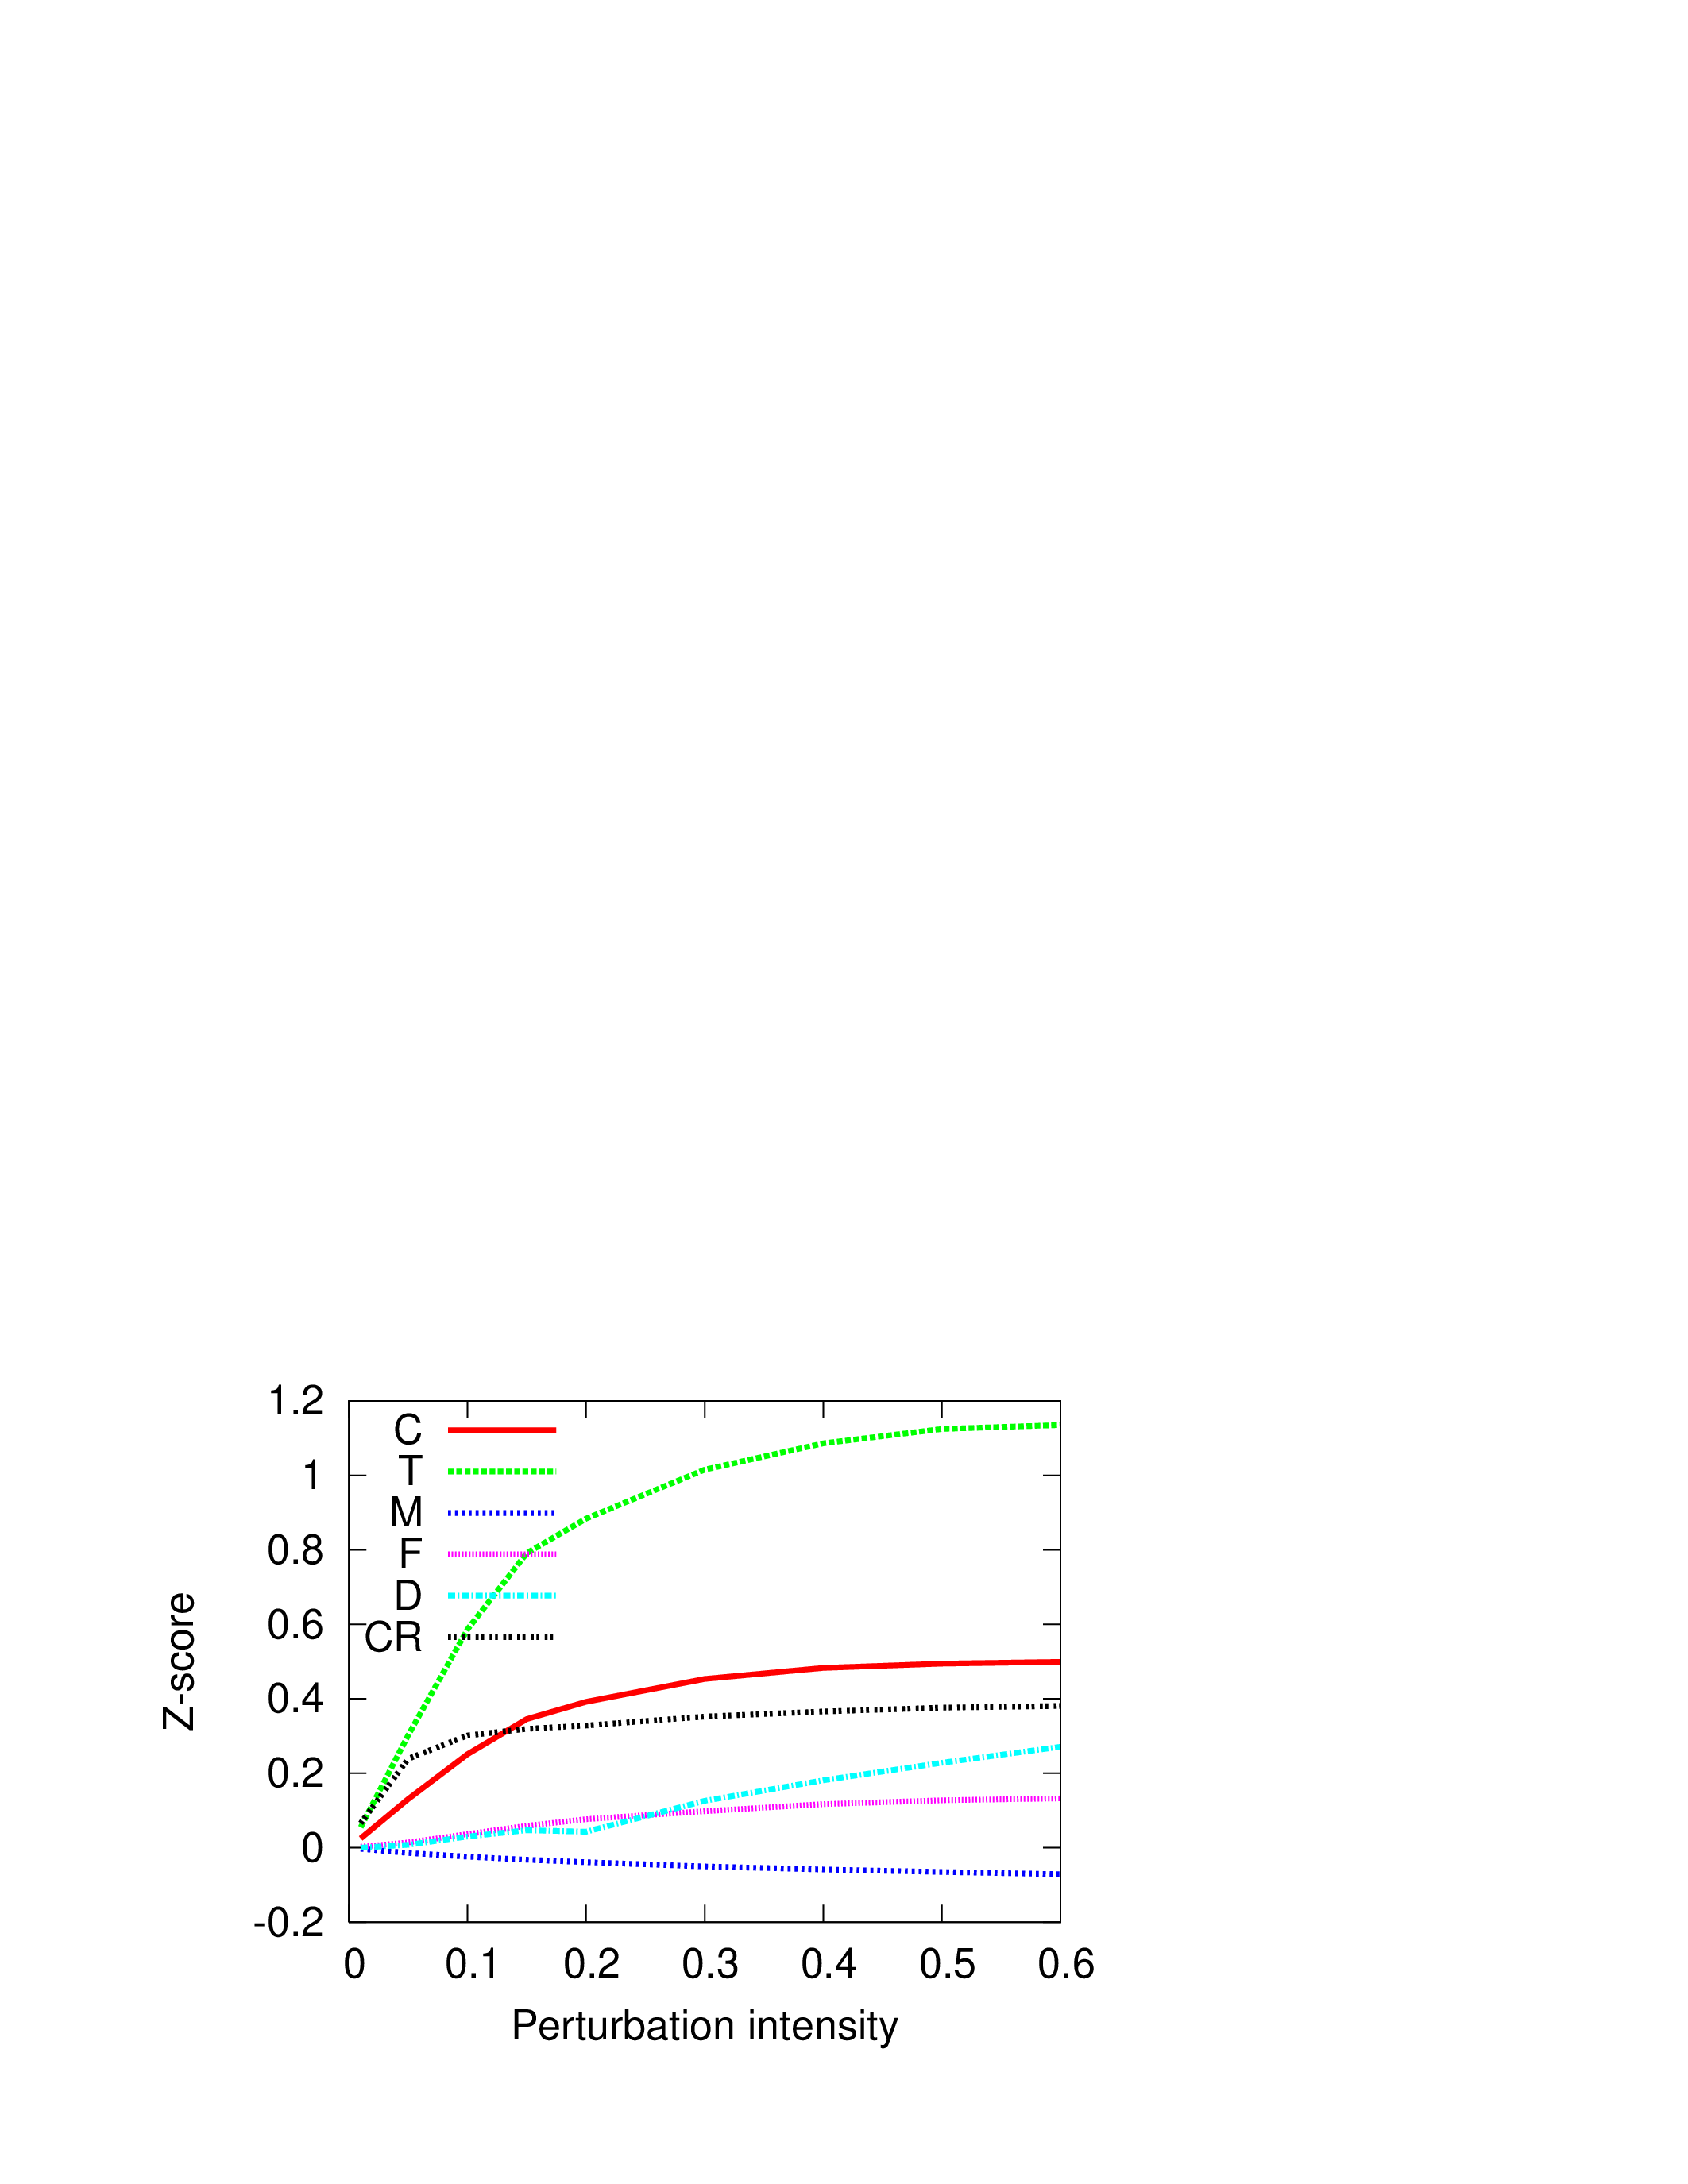}}
	\subfigure[EX	(FS)]{\includegraphics[width=0.15\textwidth]{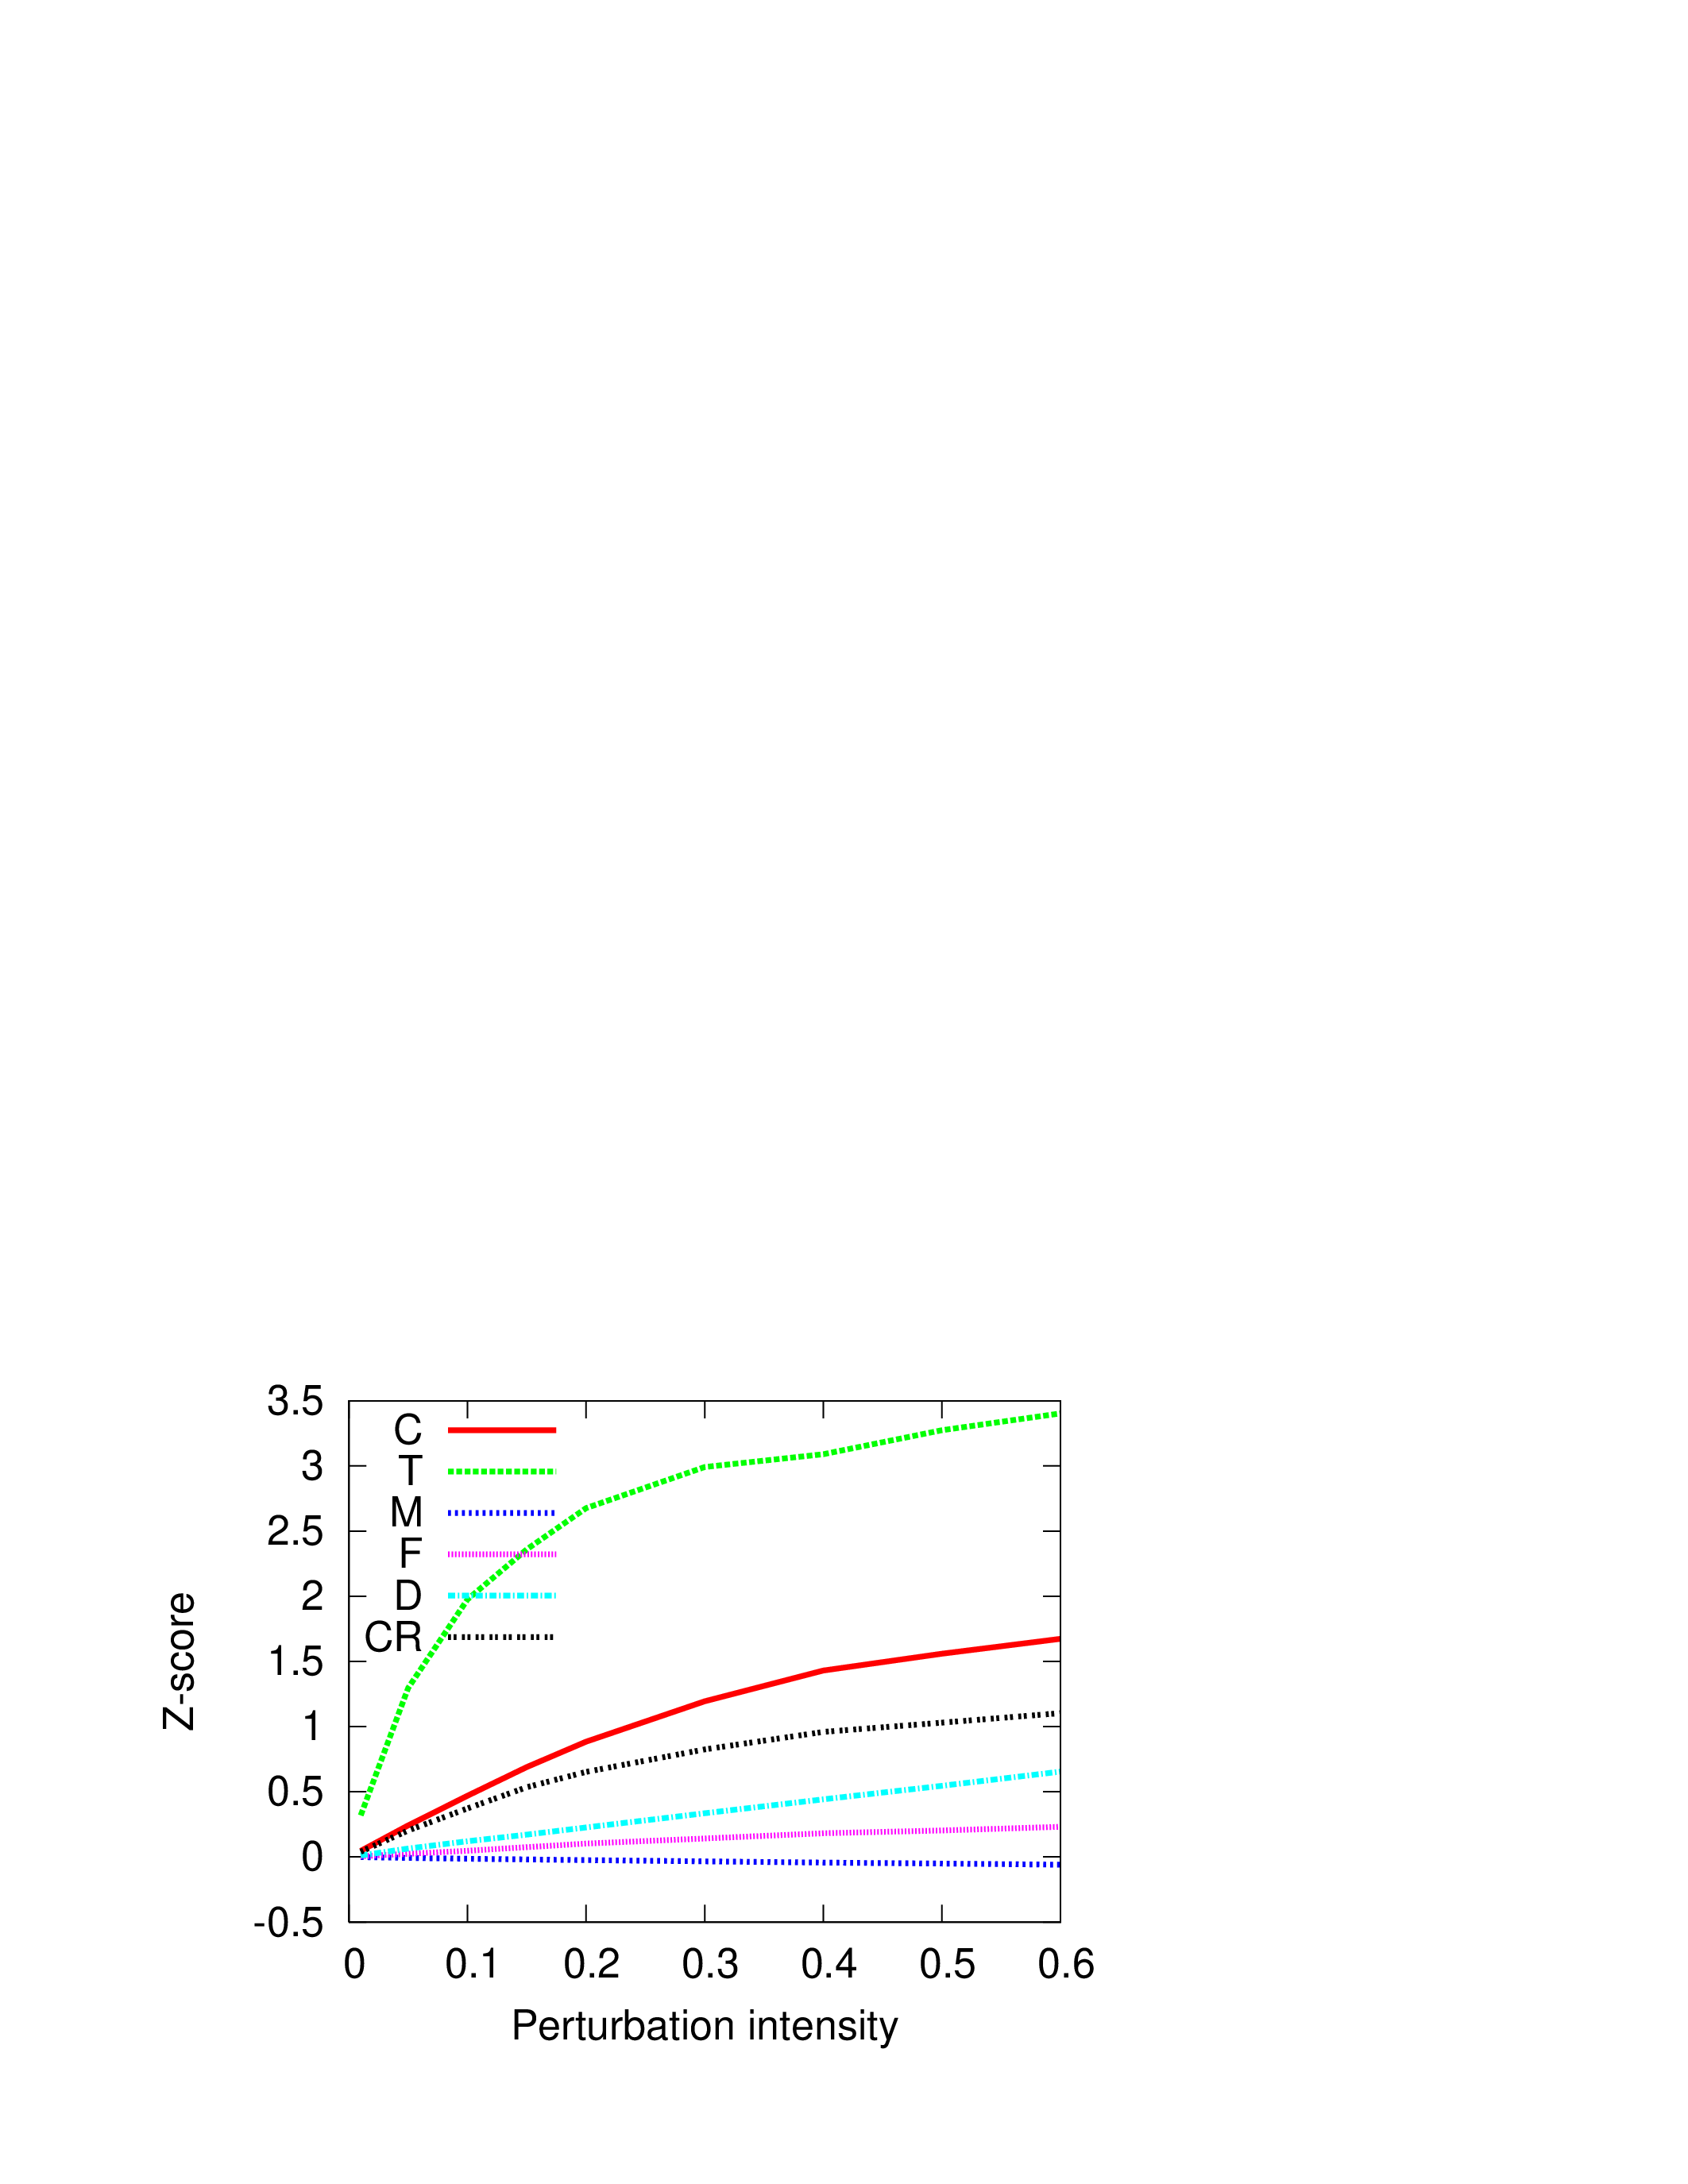}}
	\subfigure[EX	(Orkut)]{\includegraphics[width=0.15\textwidth]{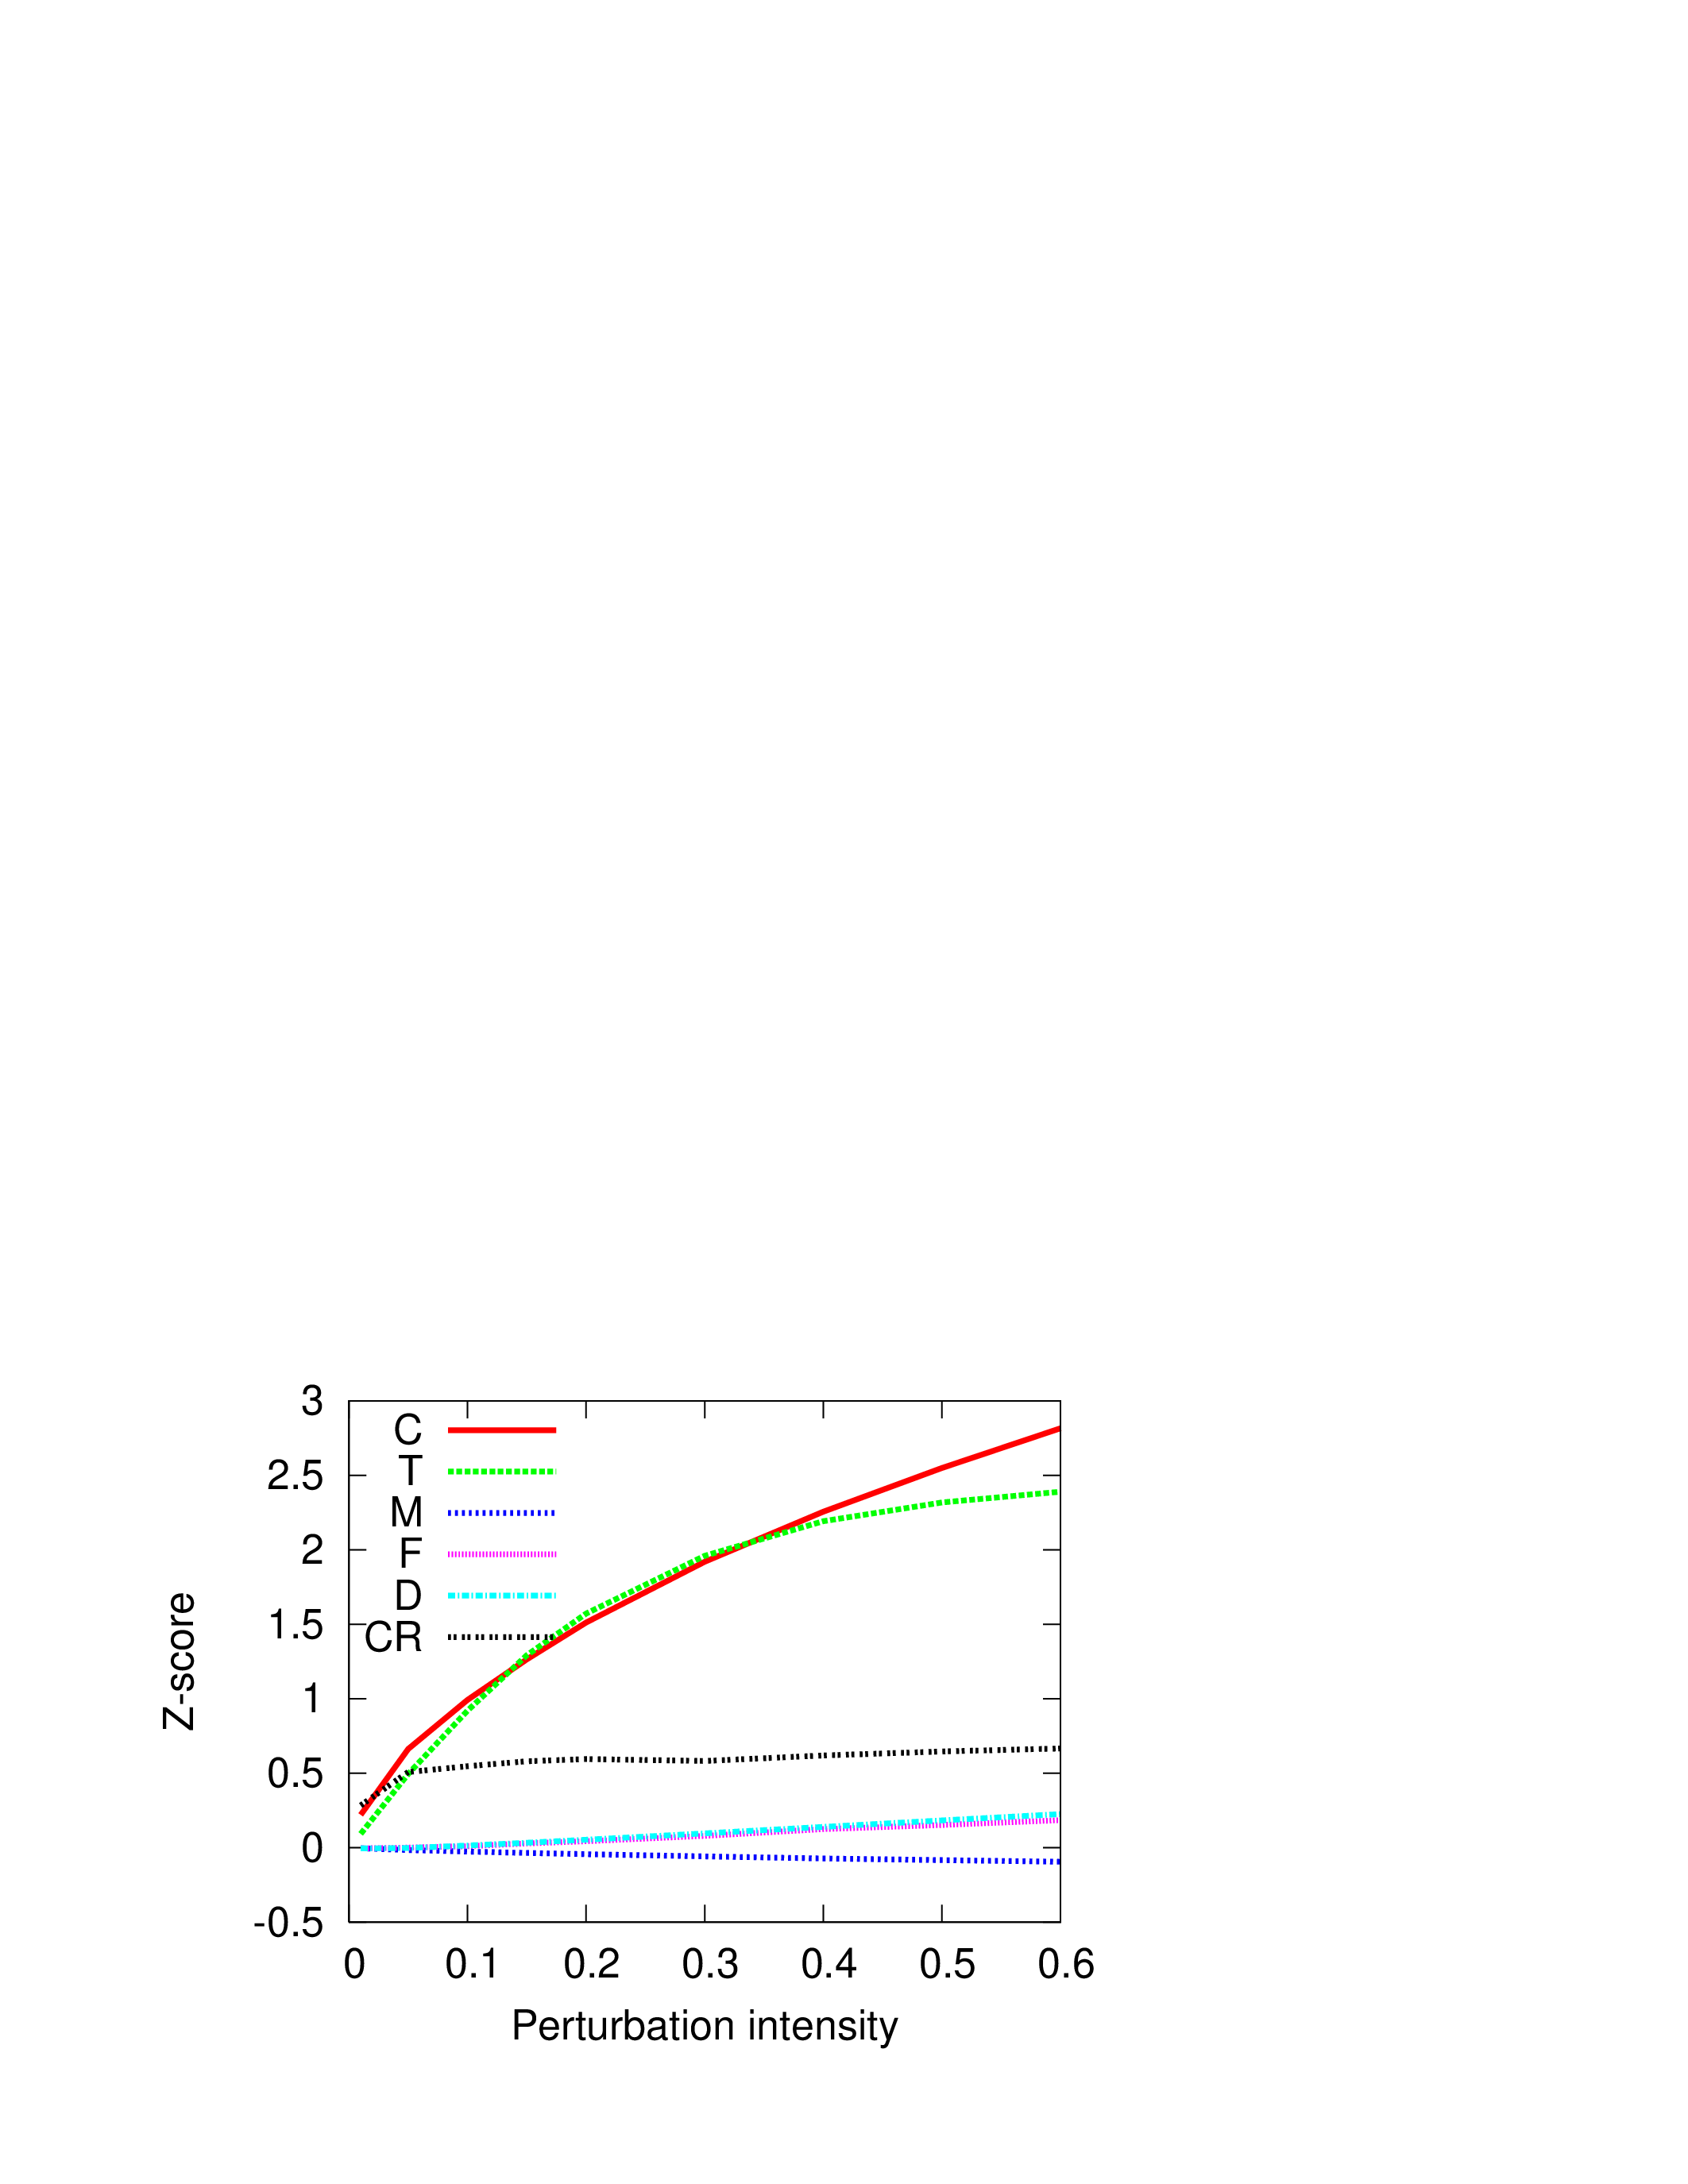}}
	\subfigure[EX	(Ning)]{\includegraphics[width=0.15\textwidth]{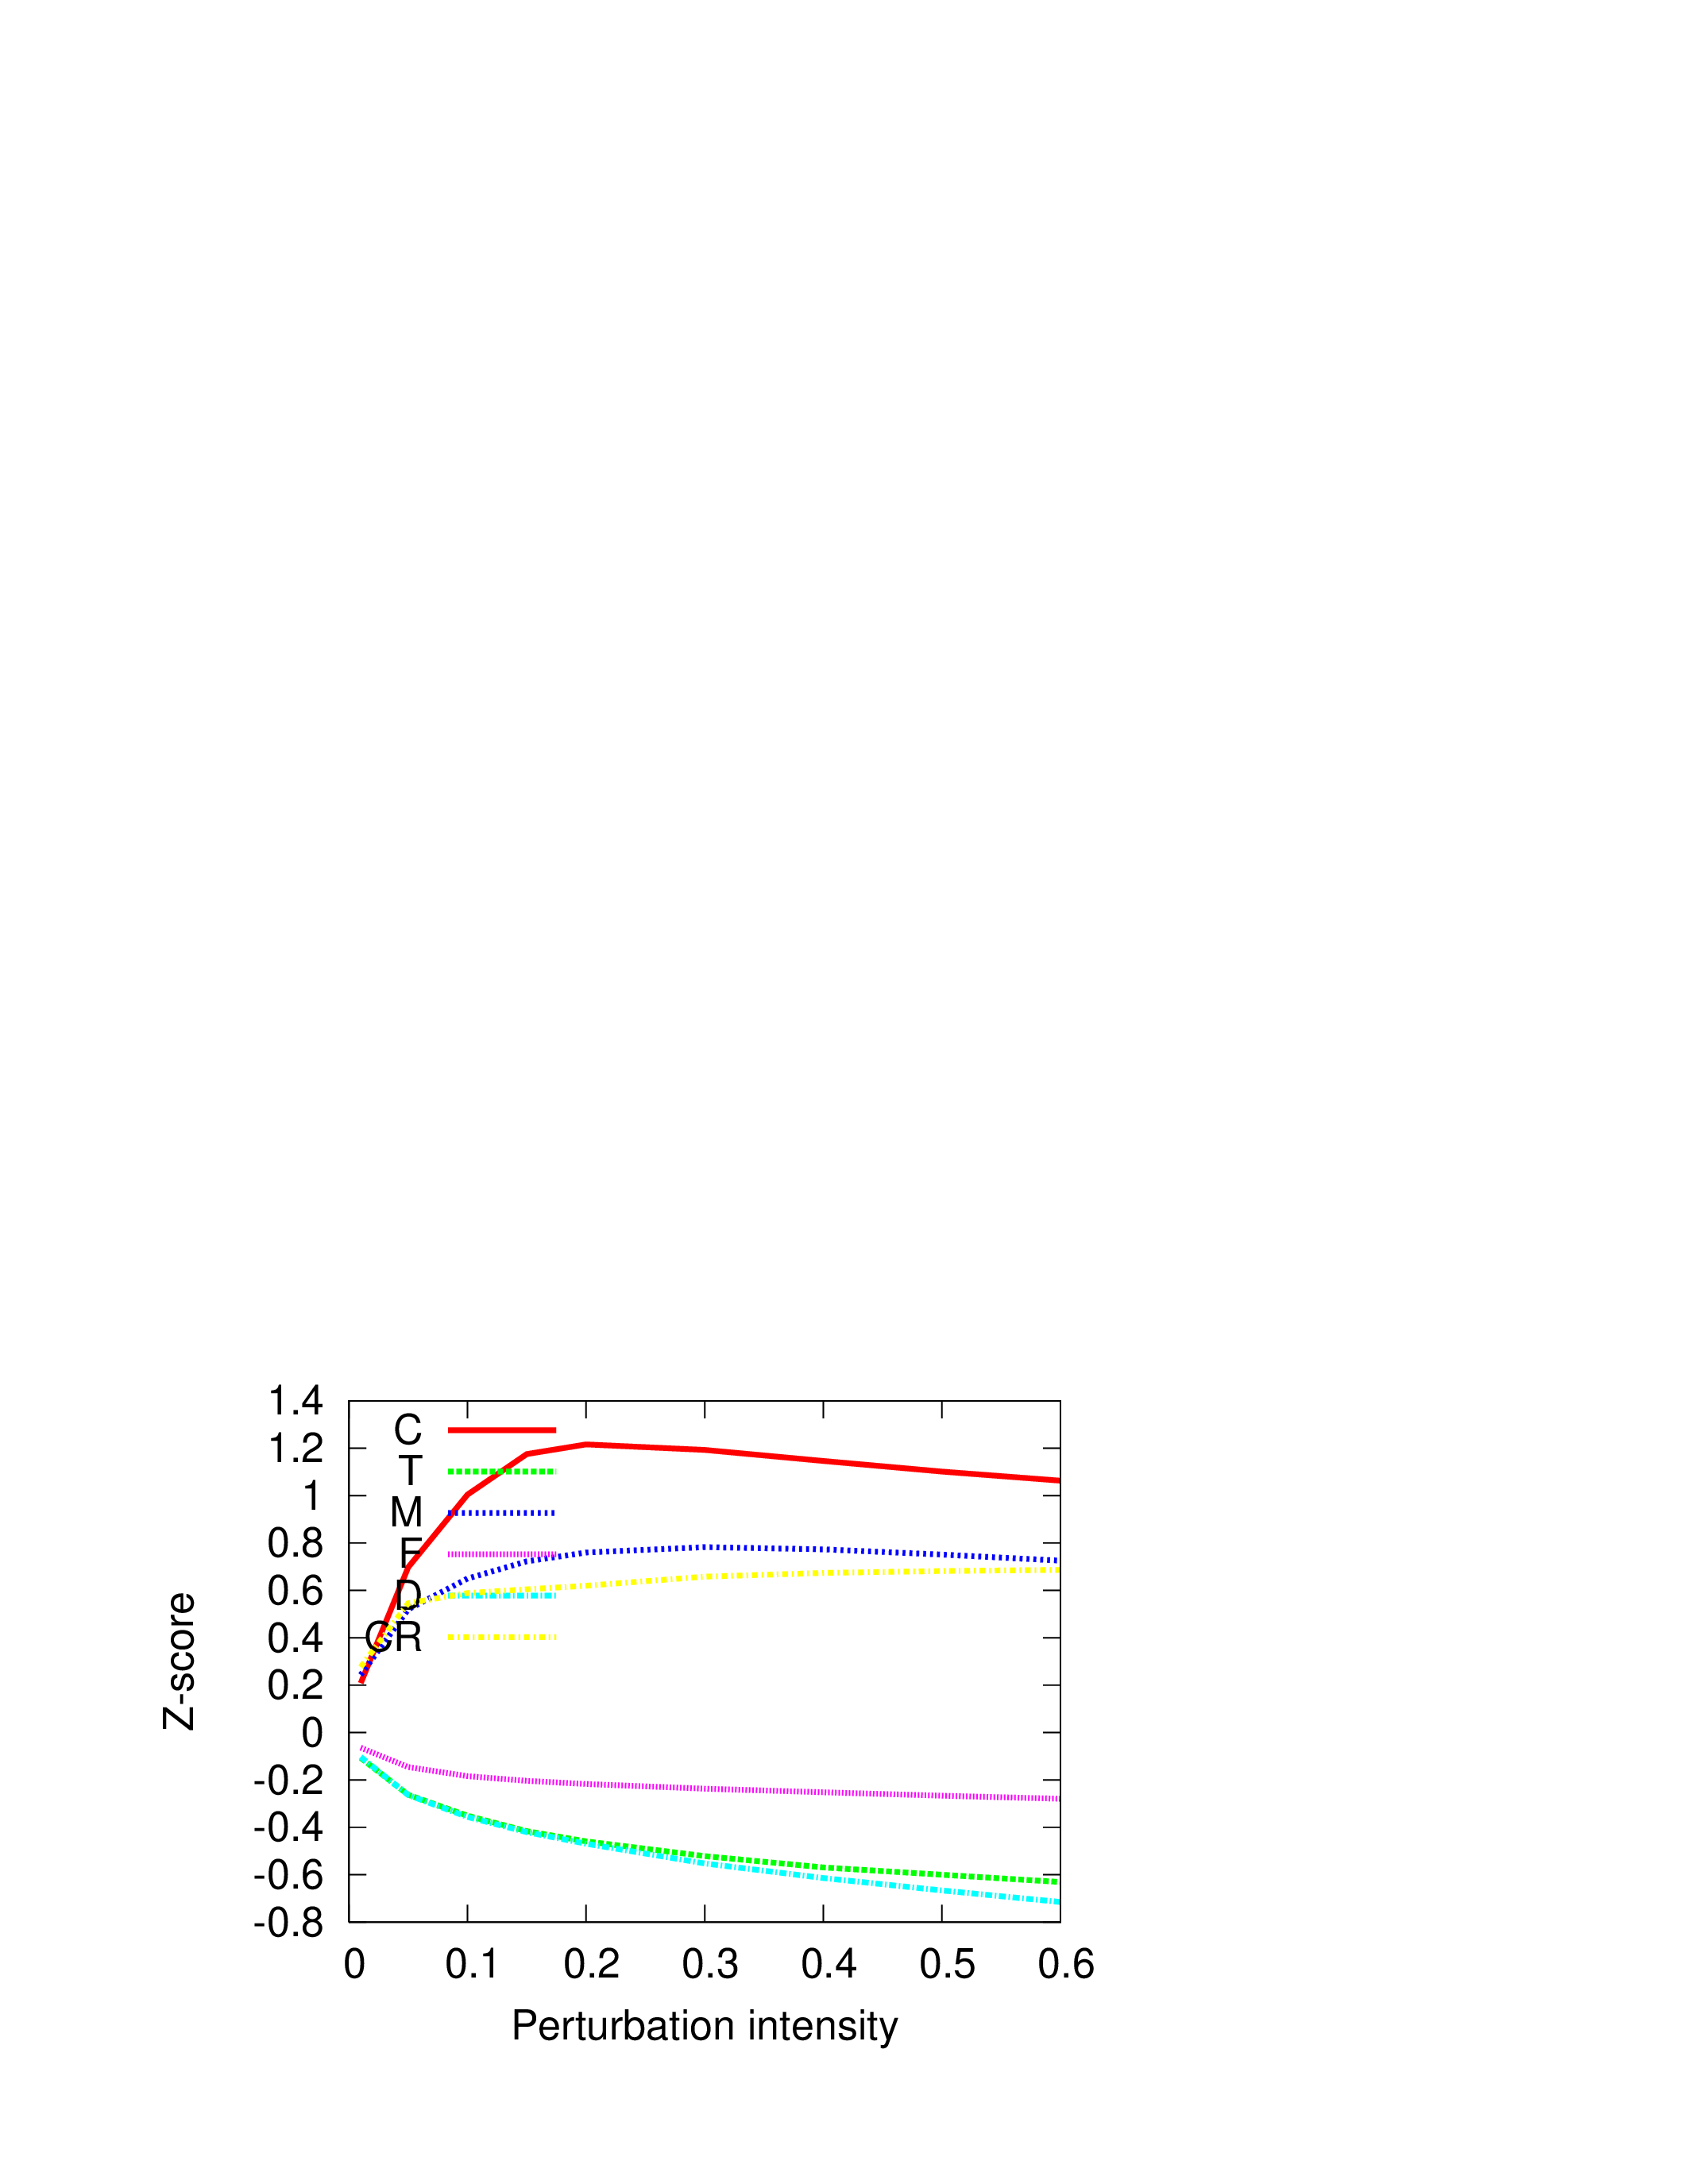}}
	\subfigure[EX	(Amazon)]{\includegraphics[width=0.15\textwidth]{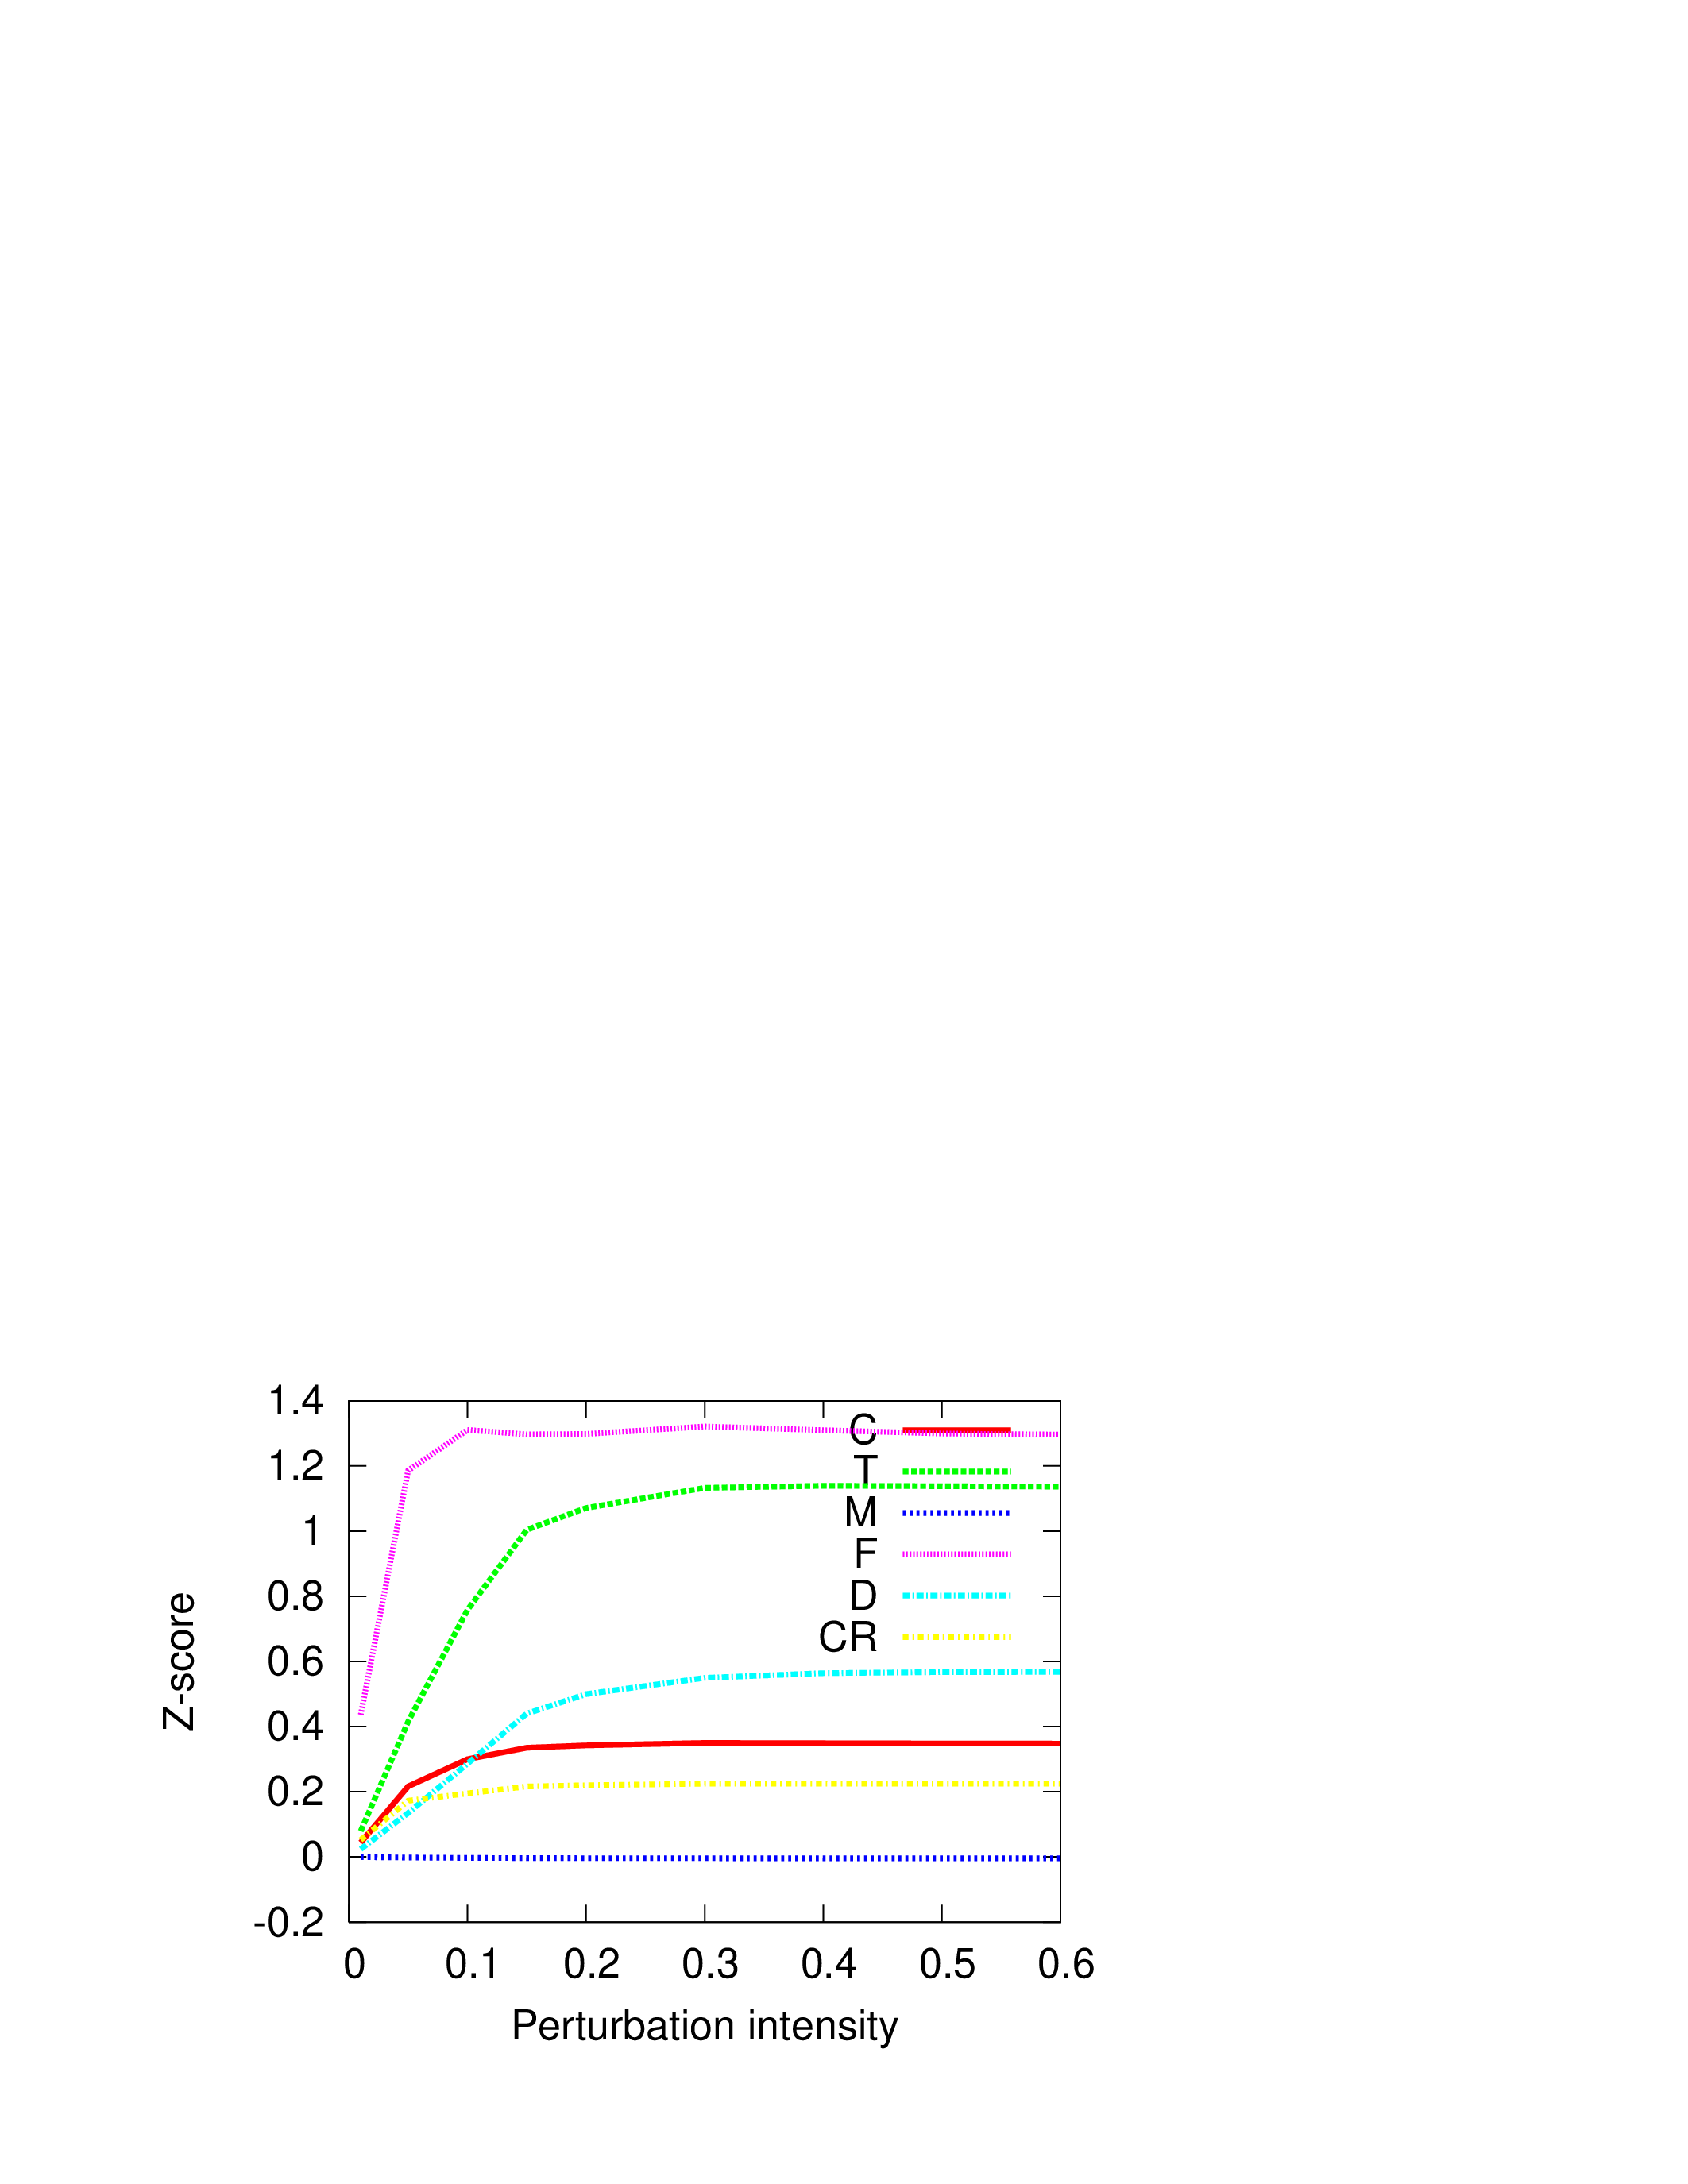}}
	\subfigure[EX	(DBLP)]{\includegraphics[width=0.15\textwidth]{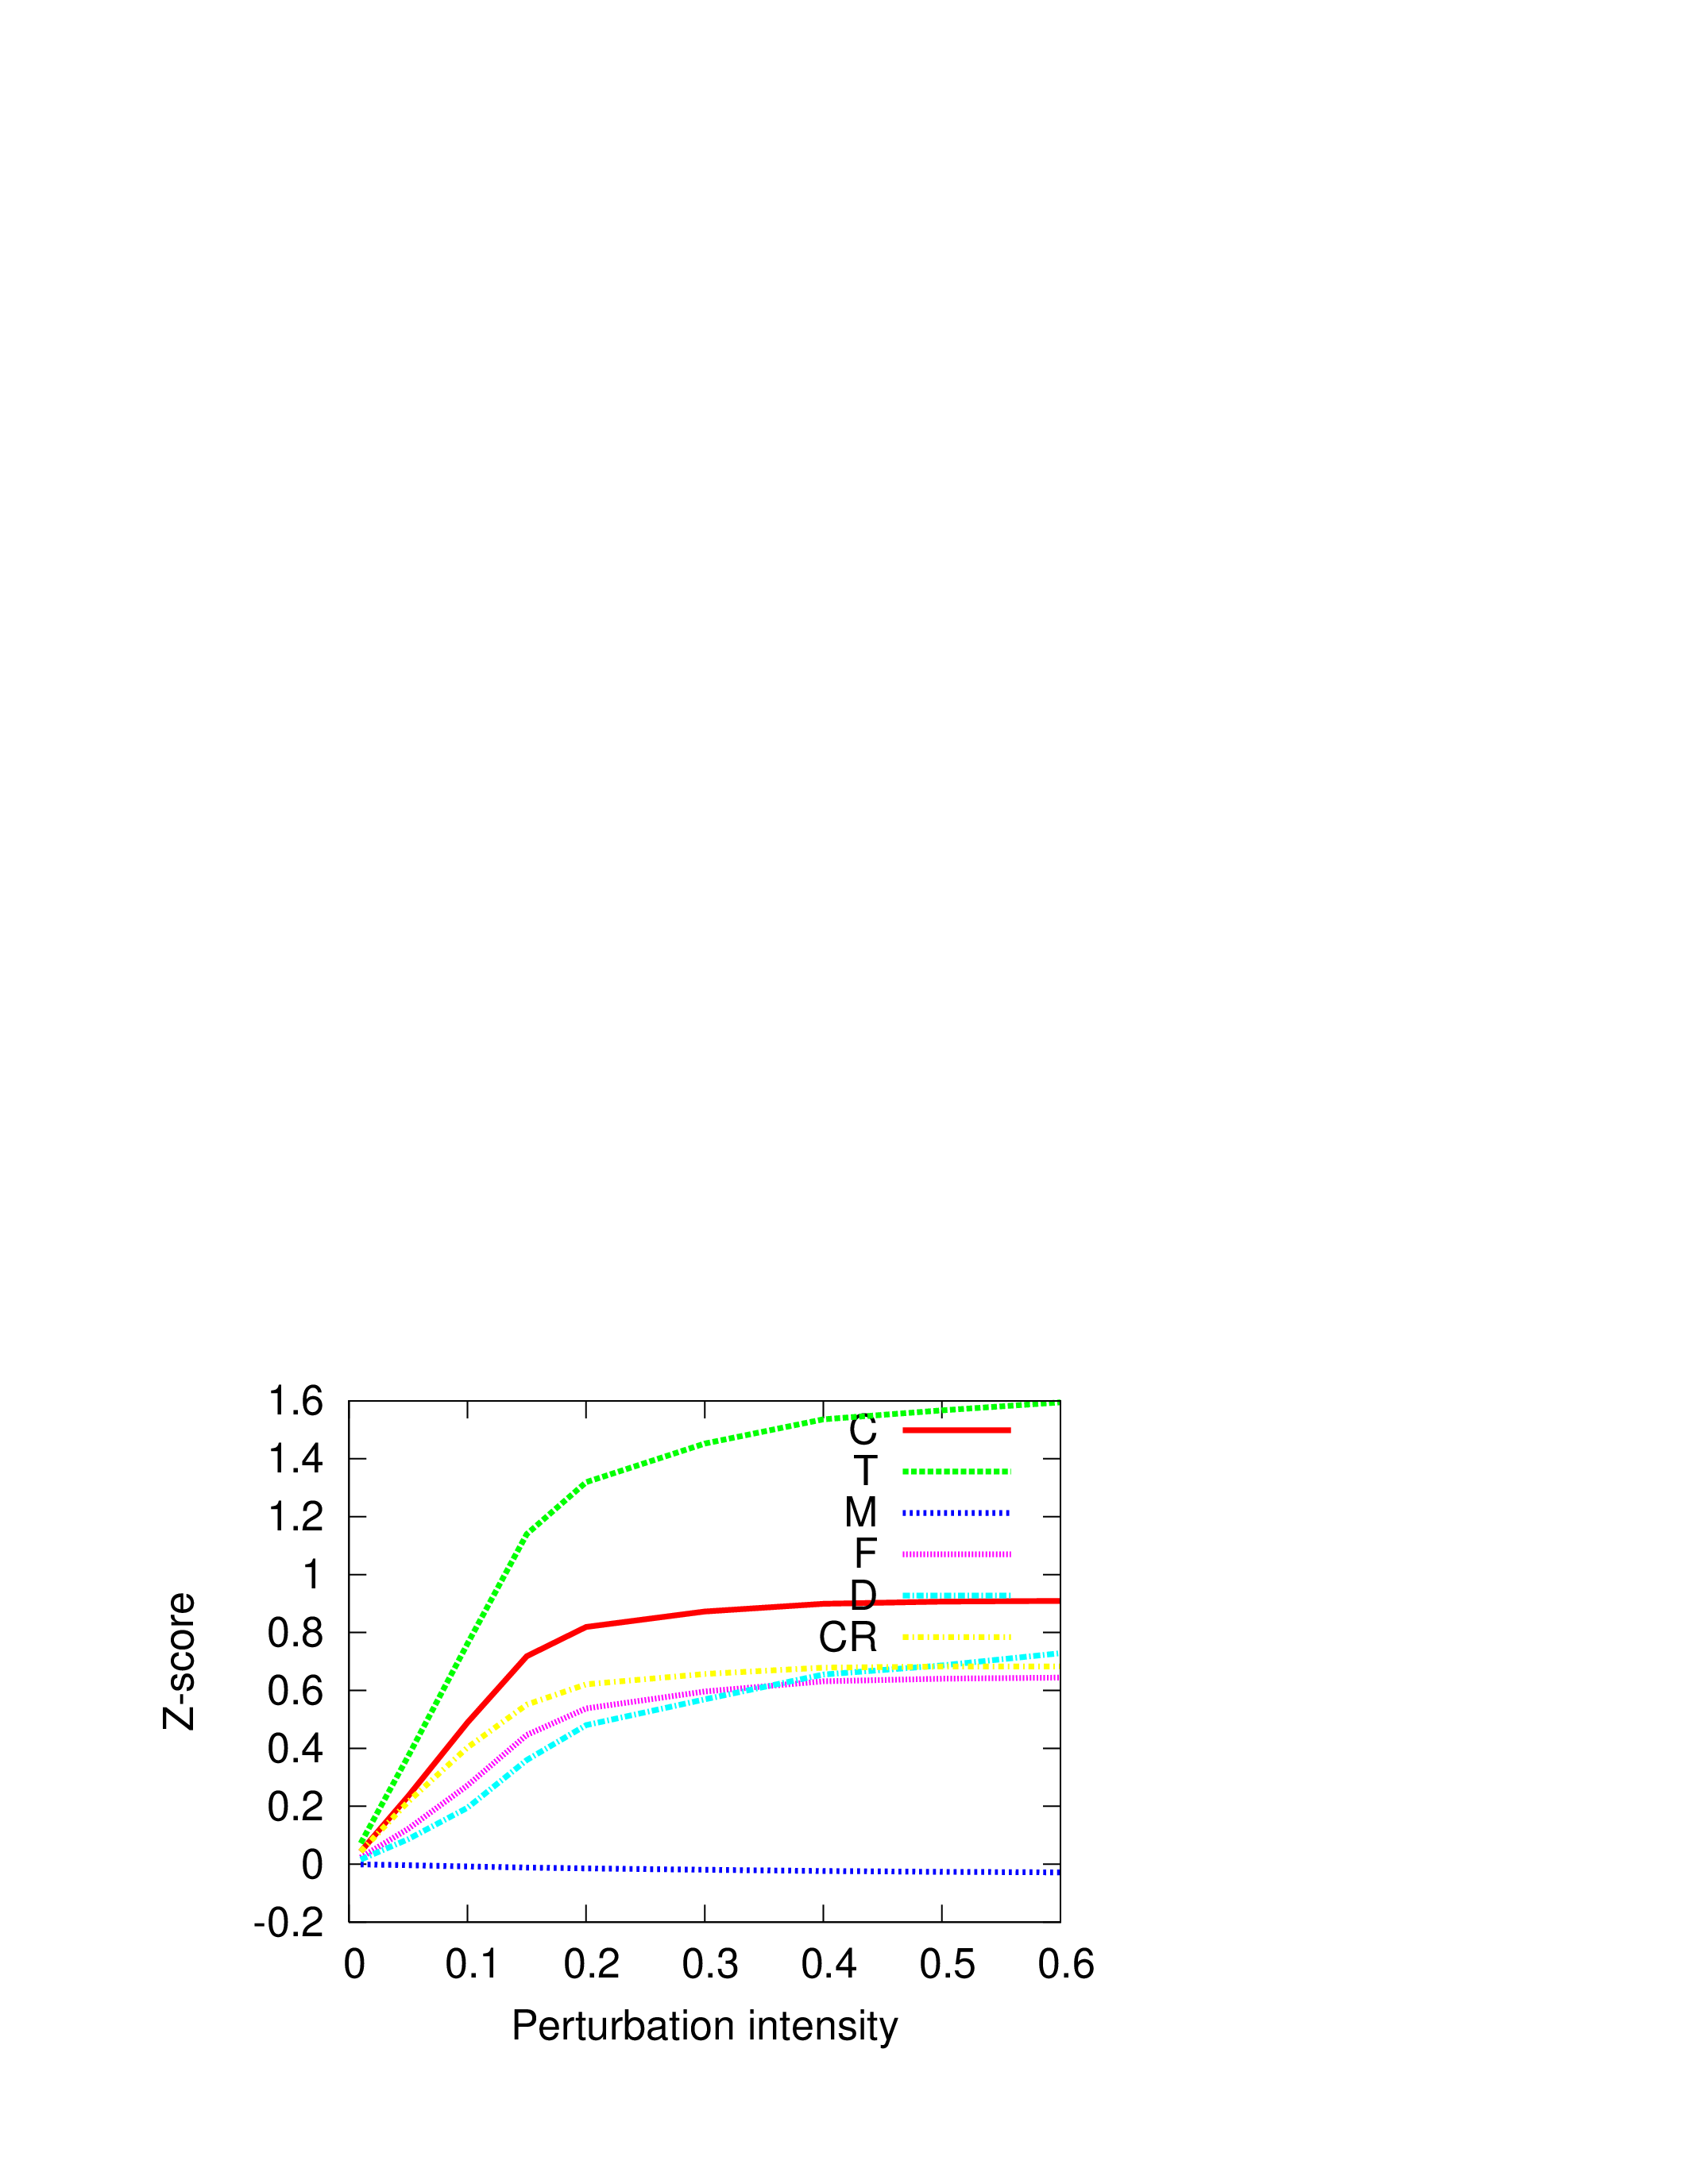}}
	\subfigure[SH	(LJ)]{\includegraphics[width=0.15\textwidth]{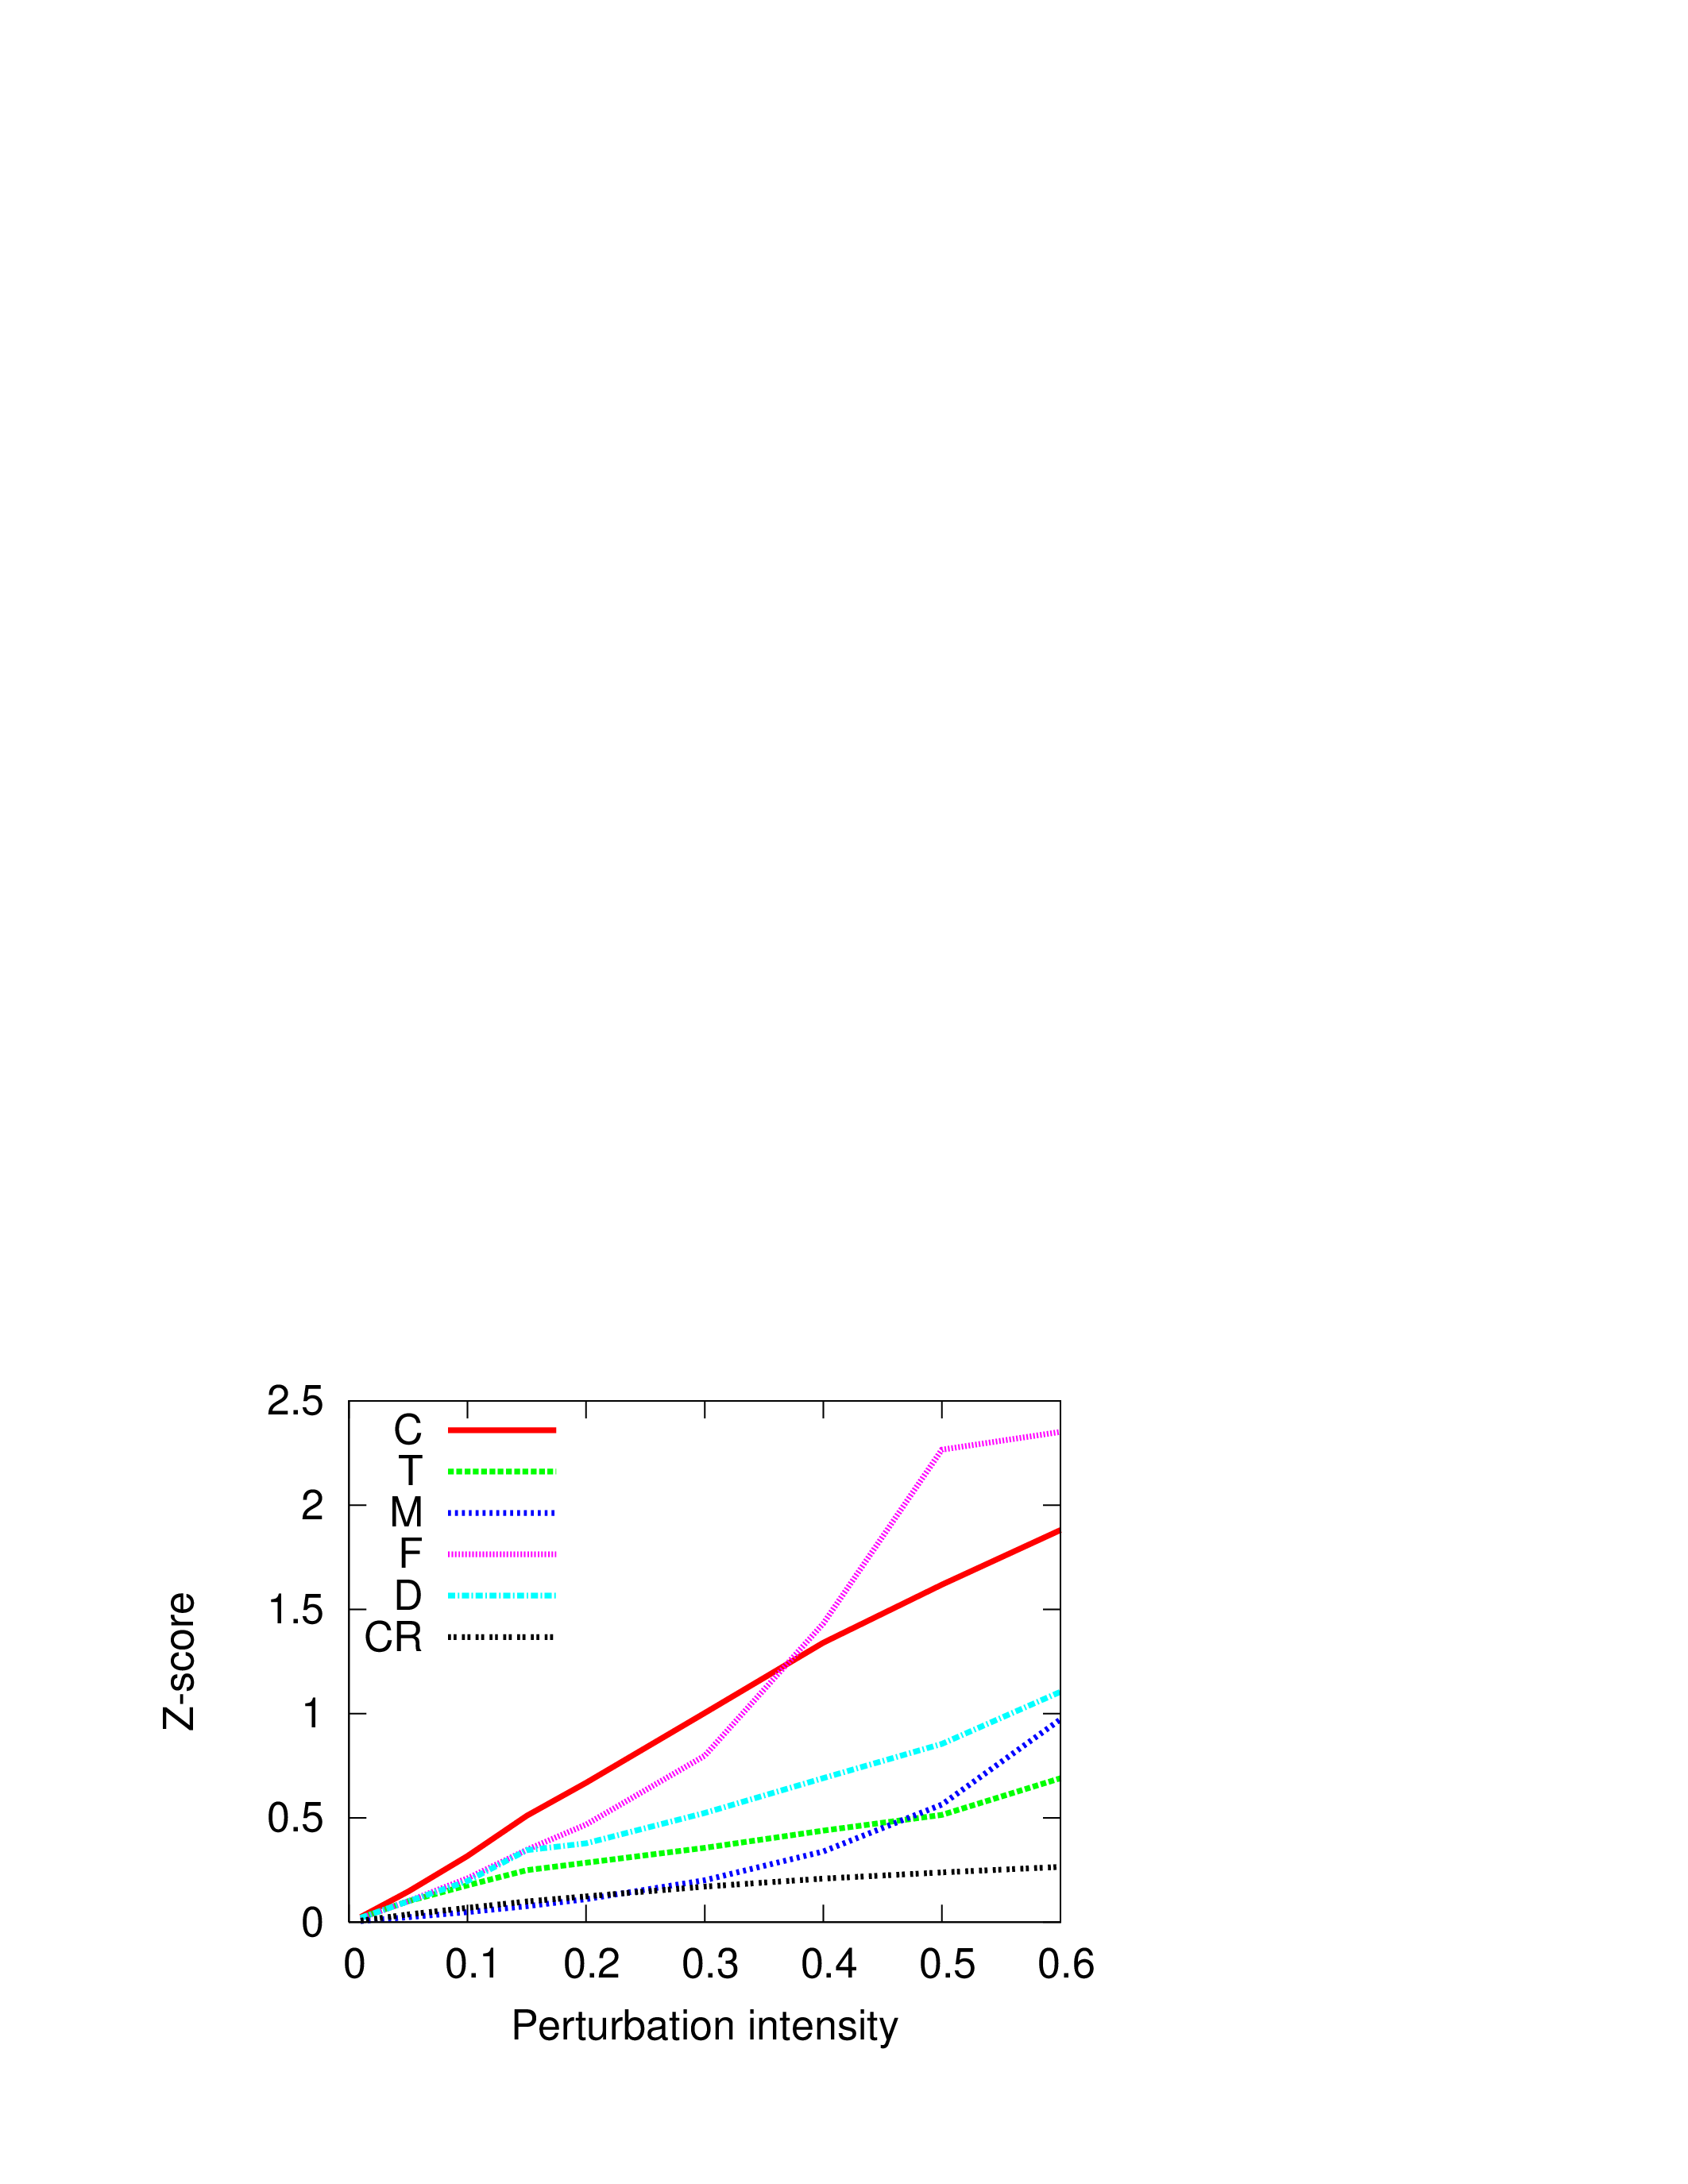}}
	\subfigure[SH	(FS)]{\includegraphics[width=0.15\textwidth]{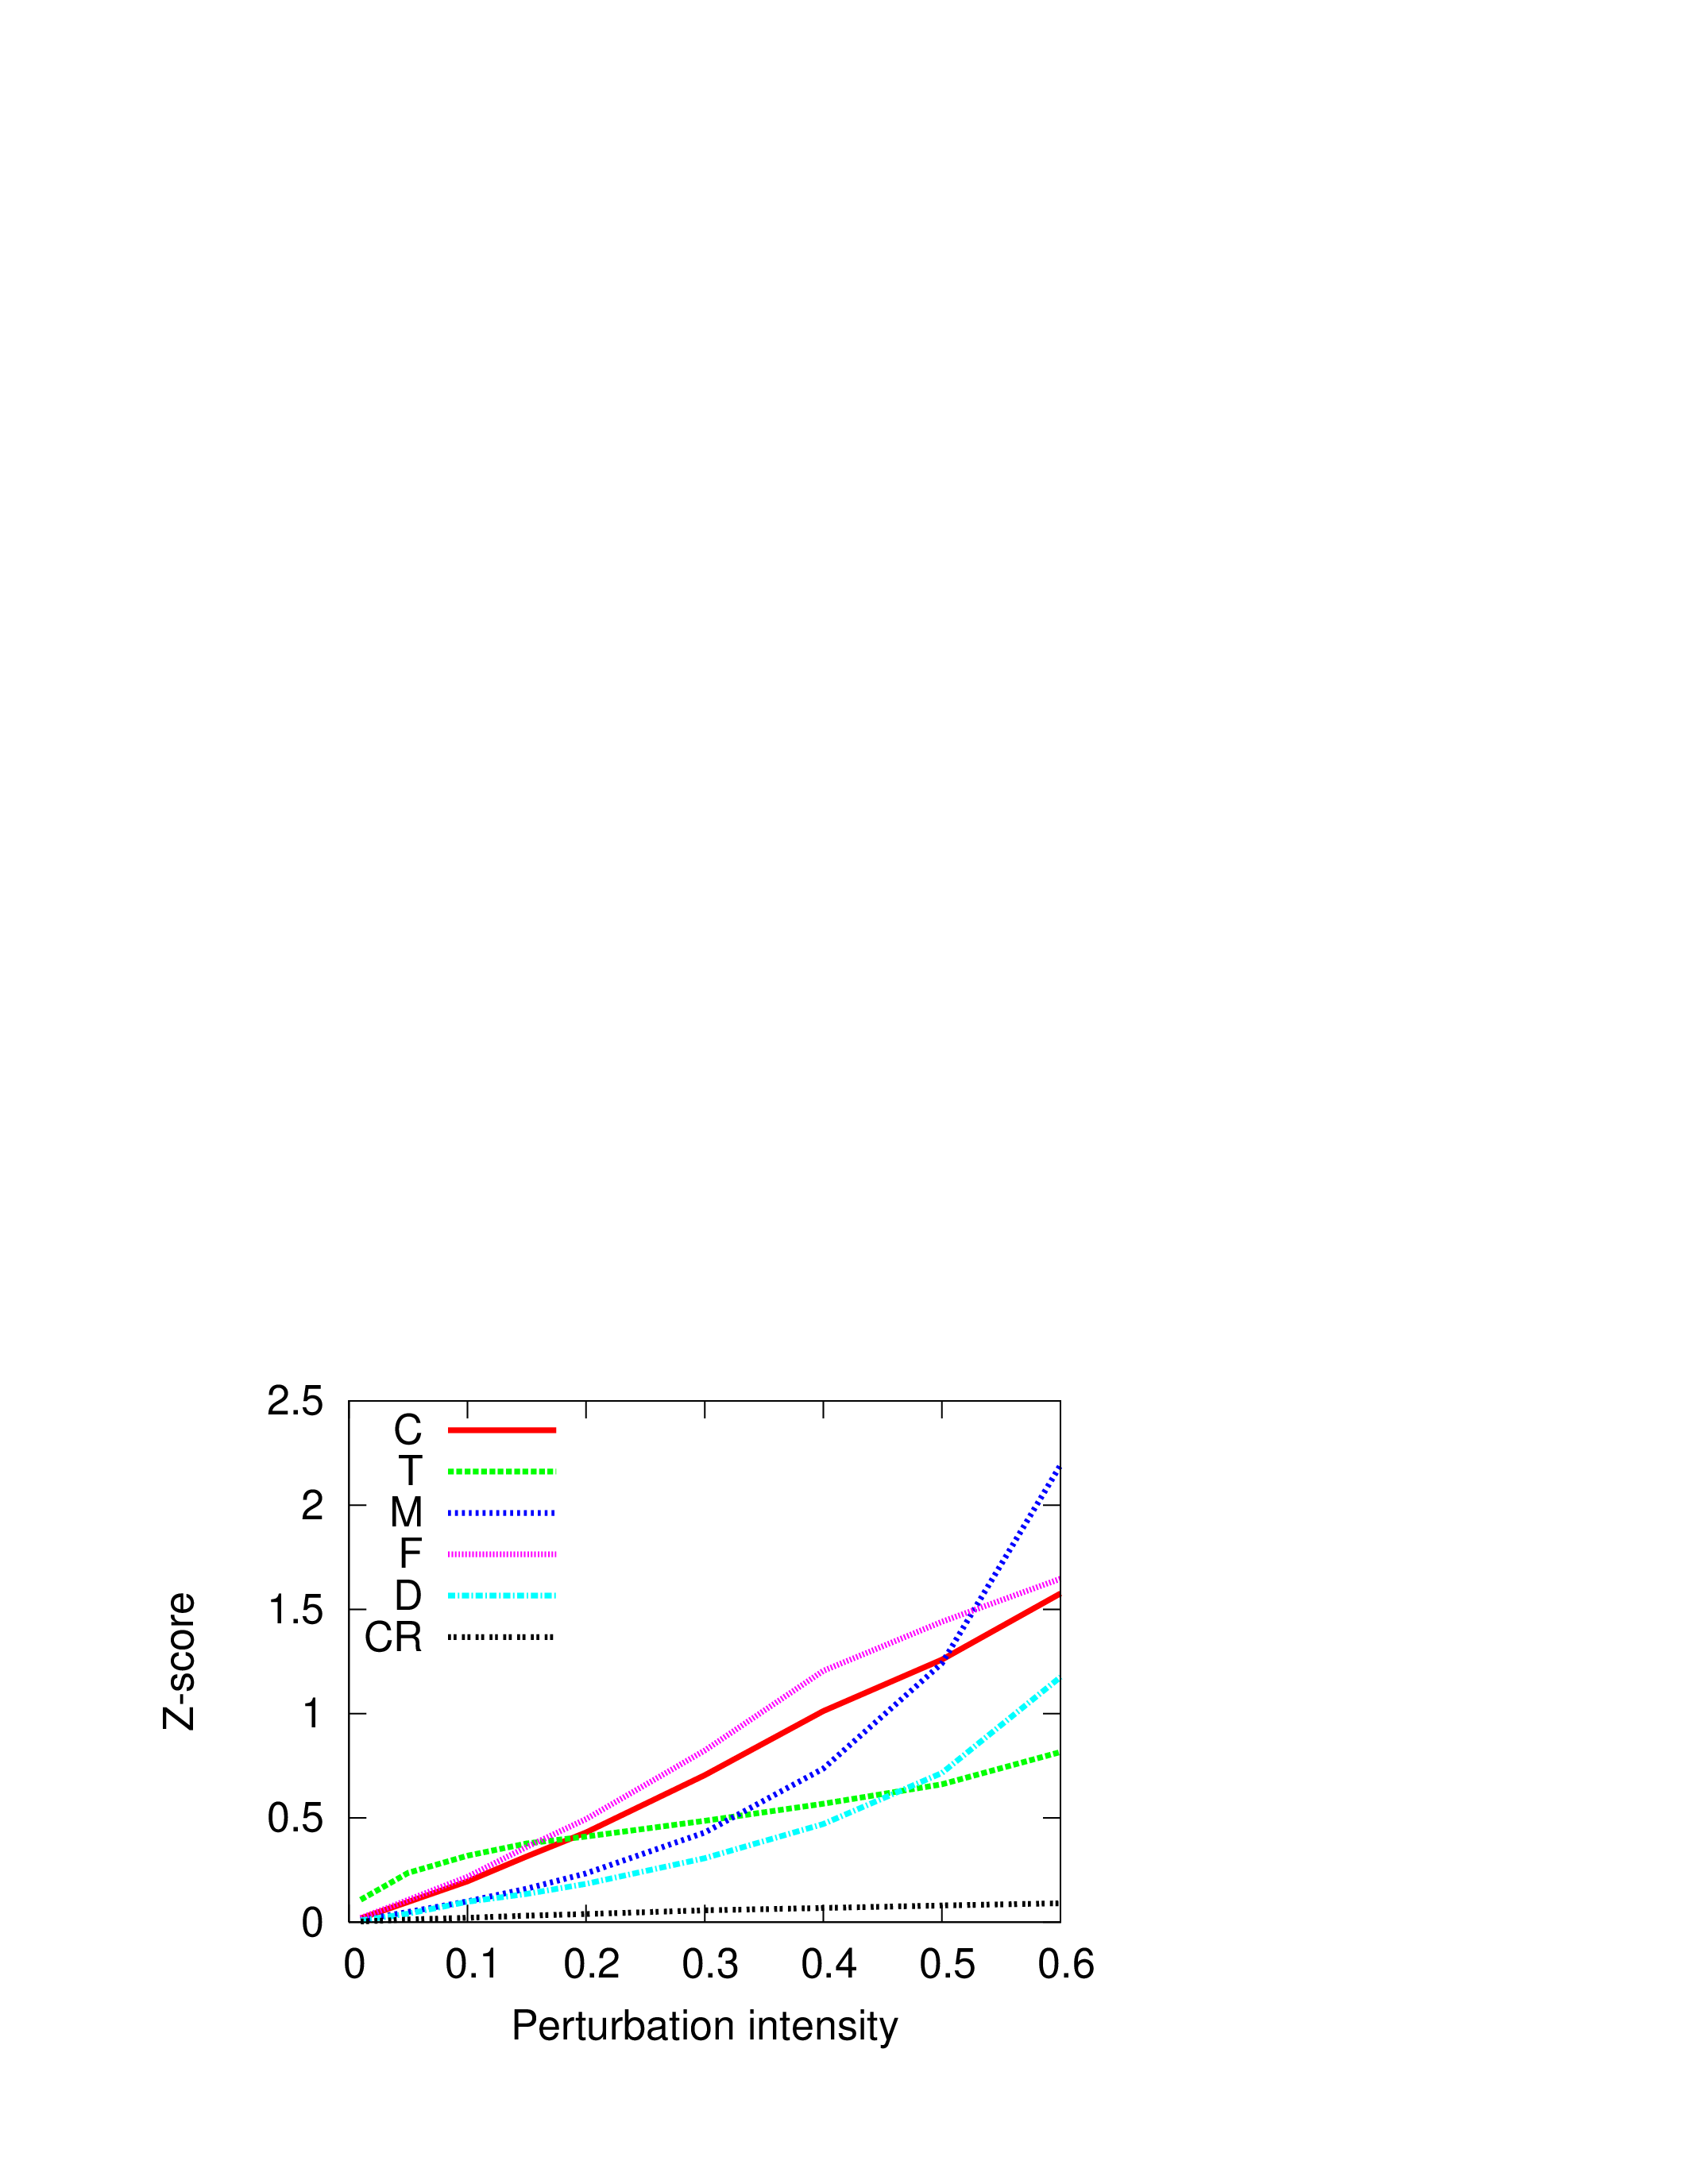}}
	\subfigure[SH	(Orkut)]{\includegraphics[width=0.15\textwidth]{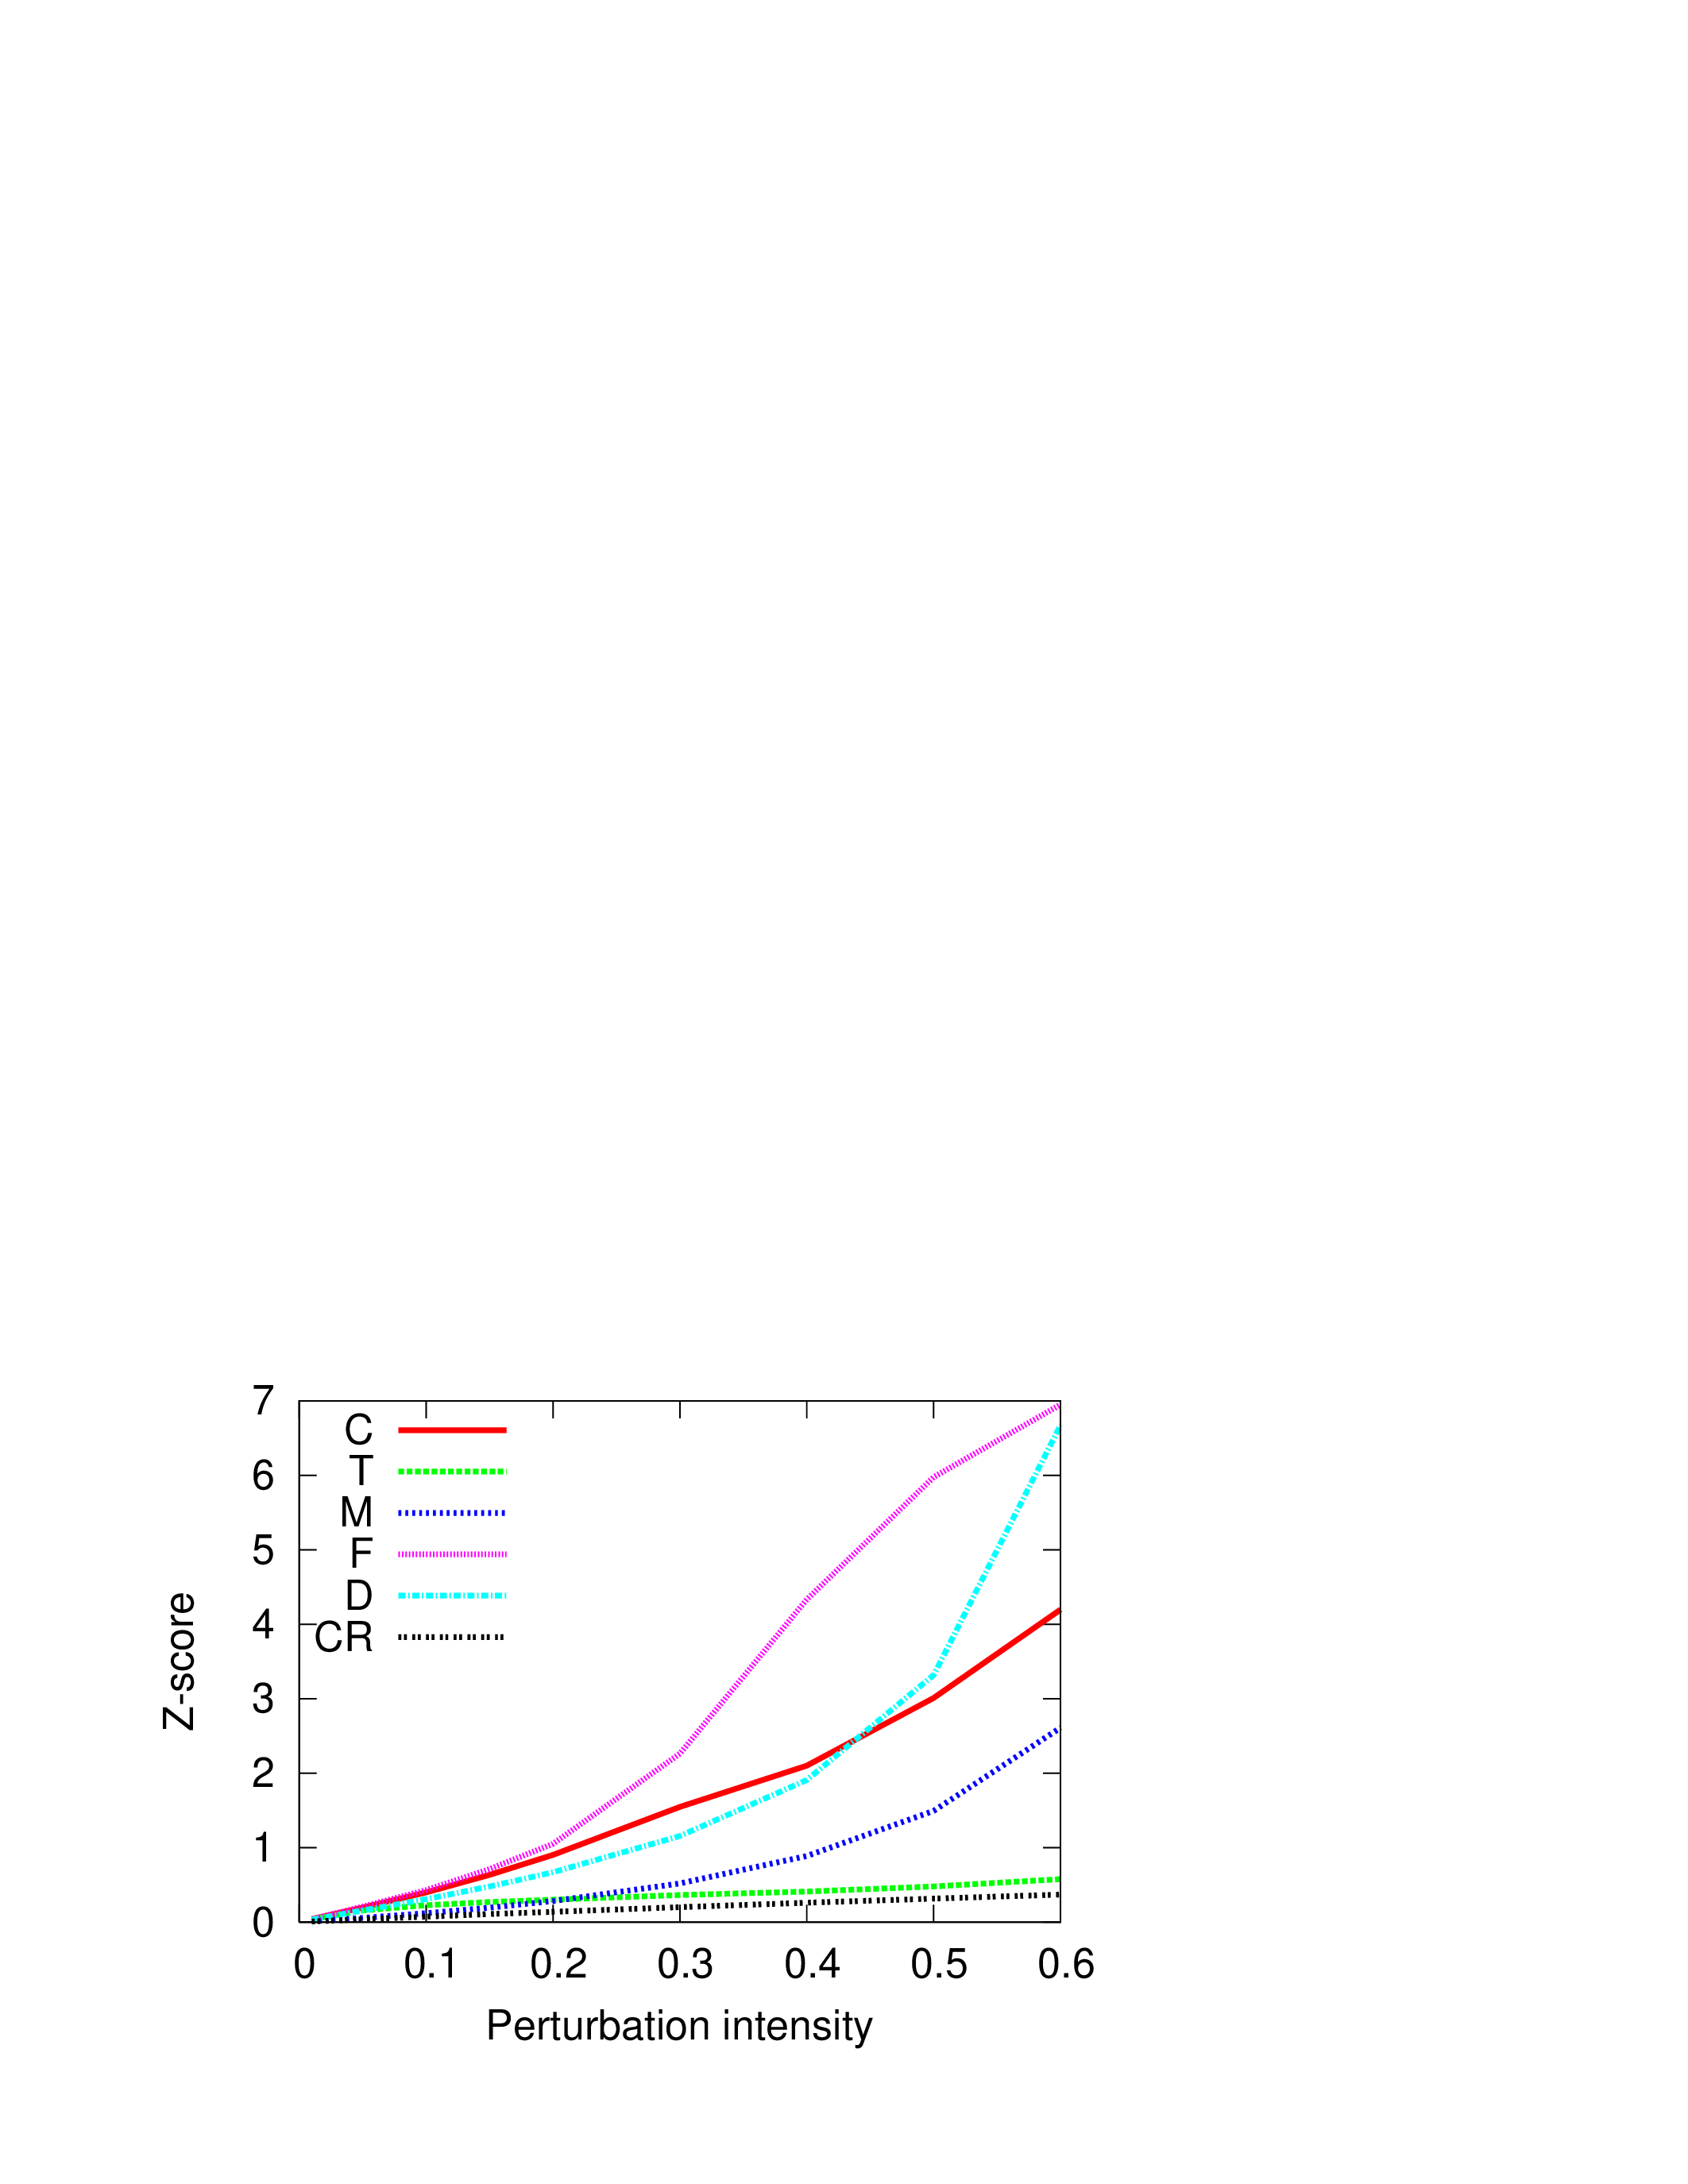}}
	\subfigure[SH	(Ning)]{\includegraphics[width=0.15\textwidth]{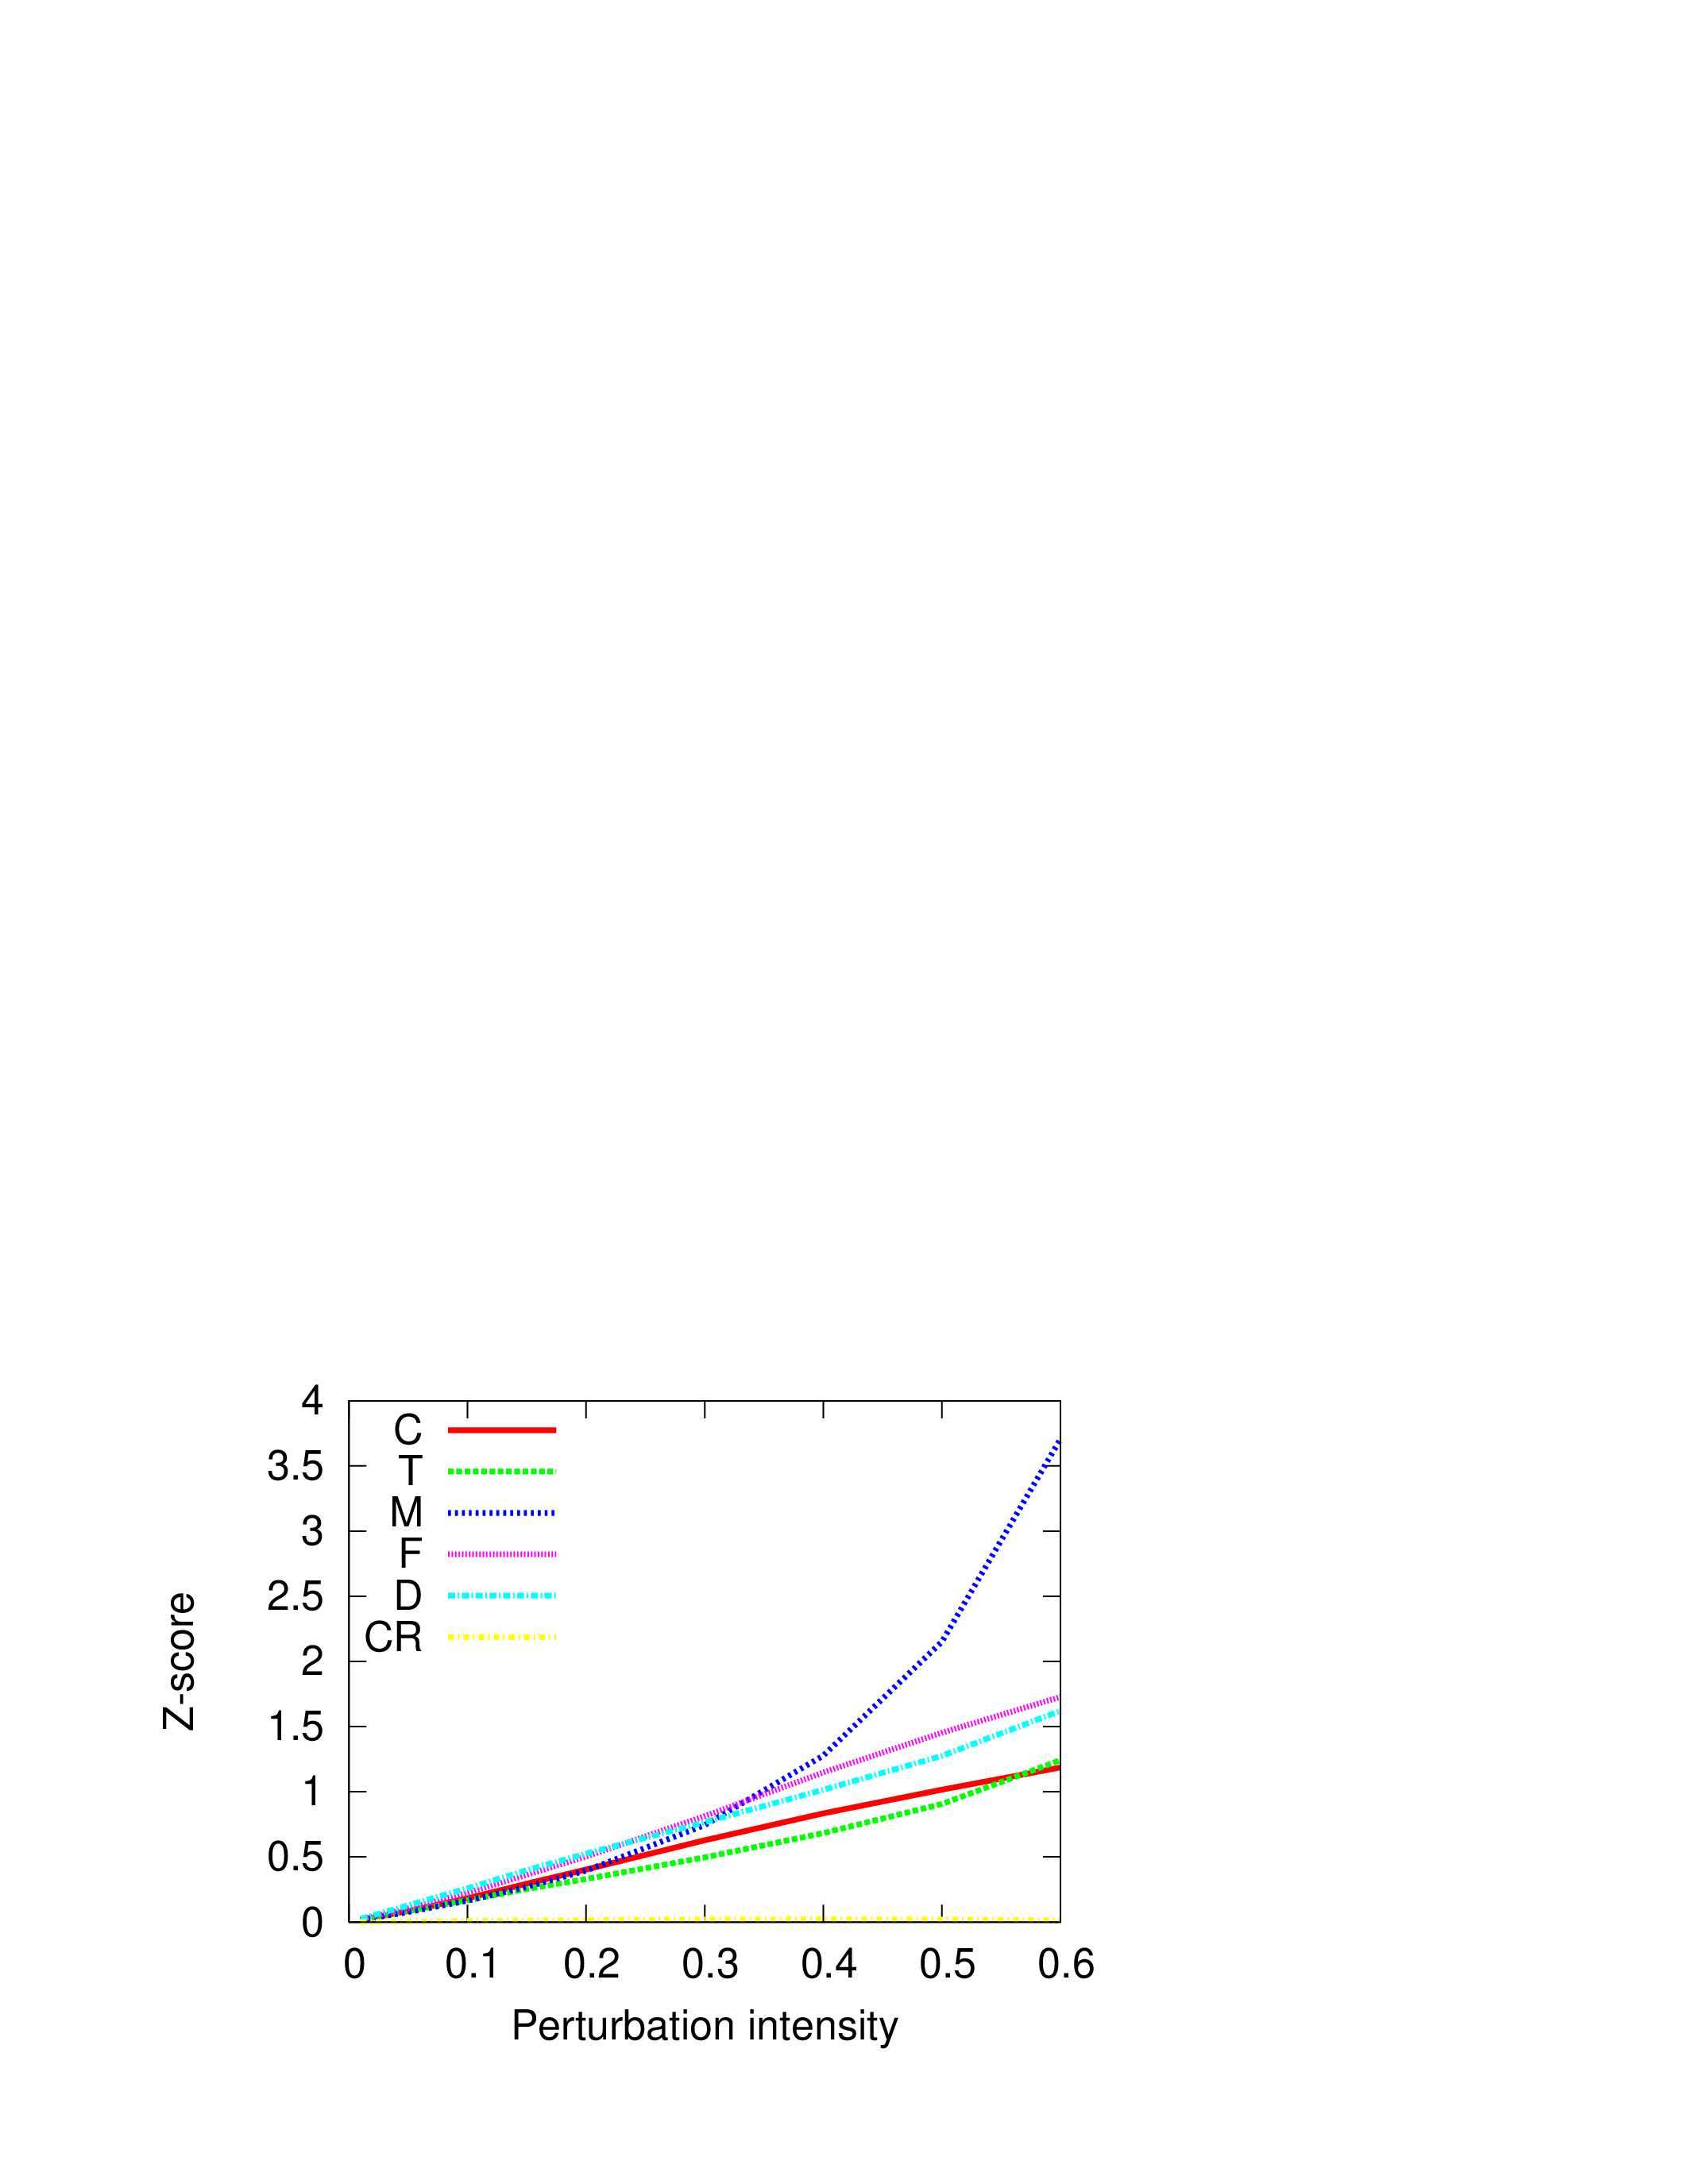}}
	\subfigure[SH	(Amazon)]{\includegraphics[width=0.15\textwidth]{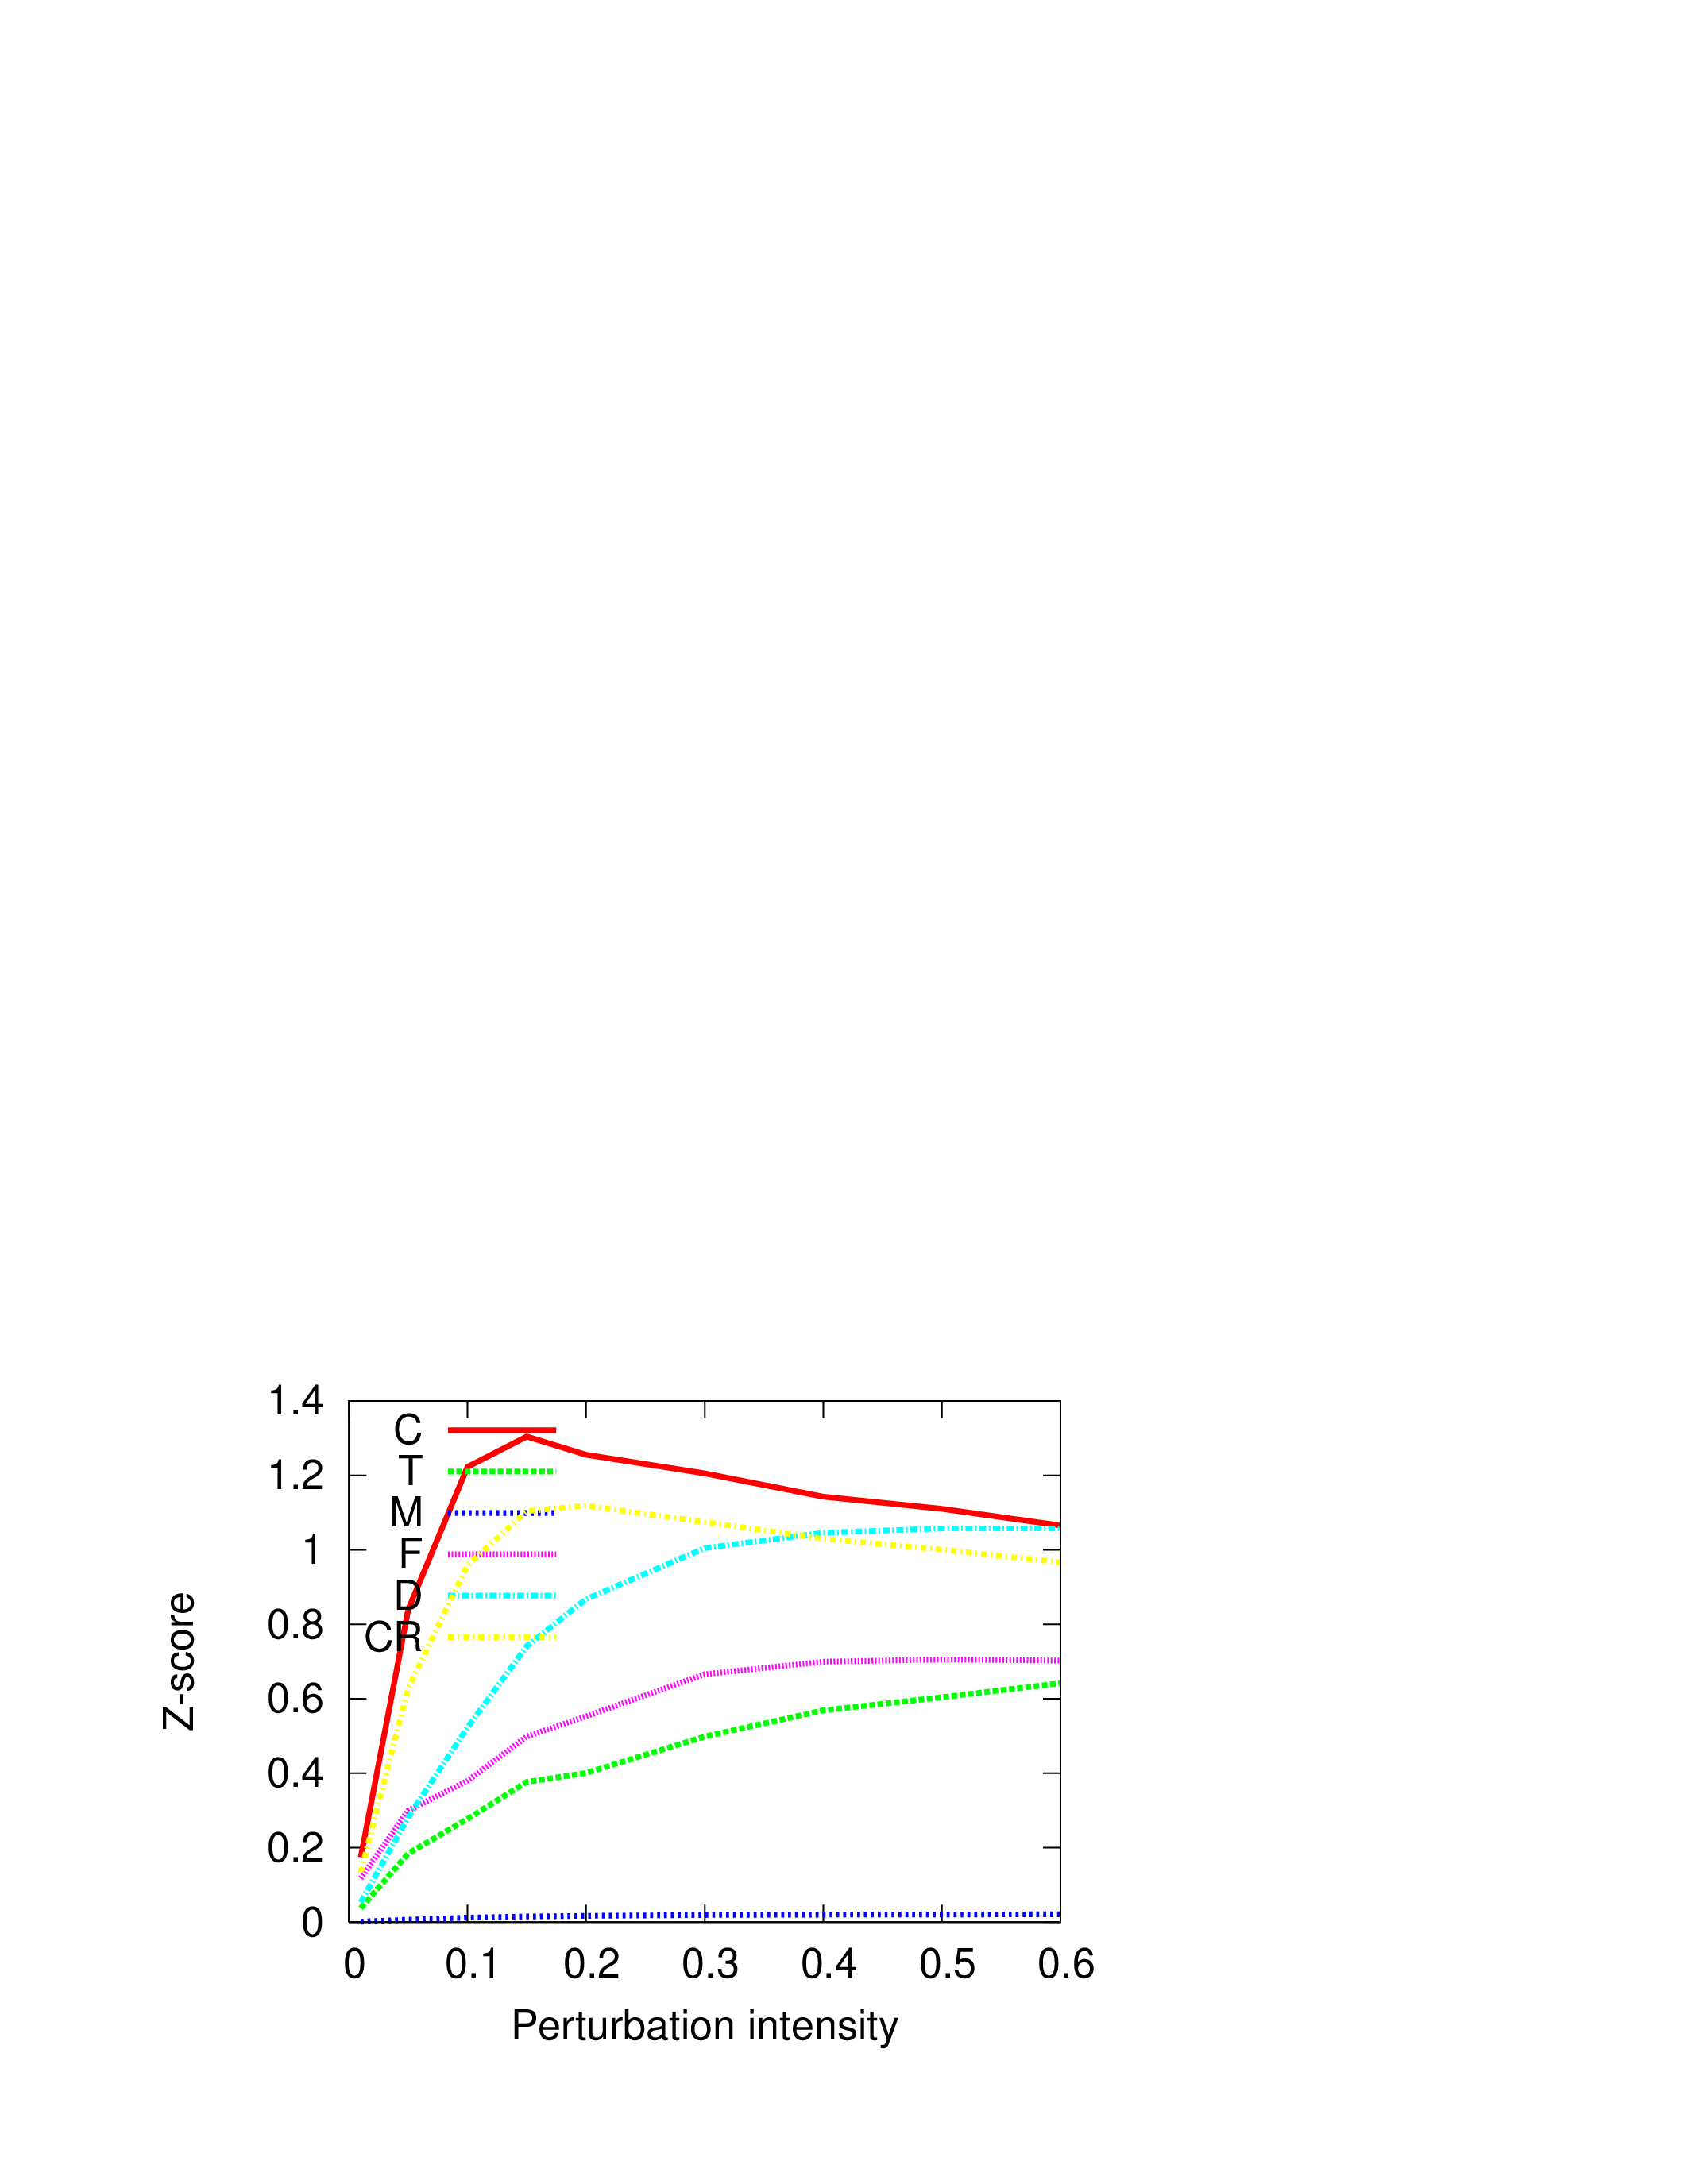}}
	\subfigure[SH	(DBLP)]{\includegraphics[width=0.15\textwidth]{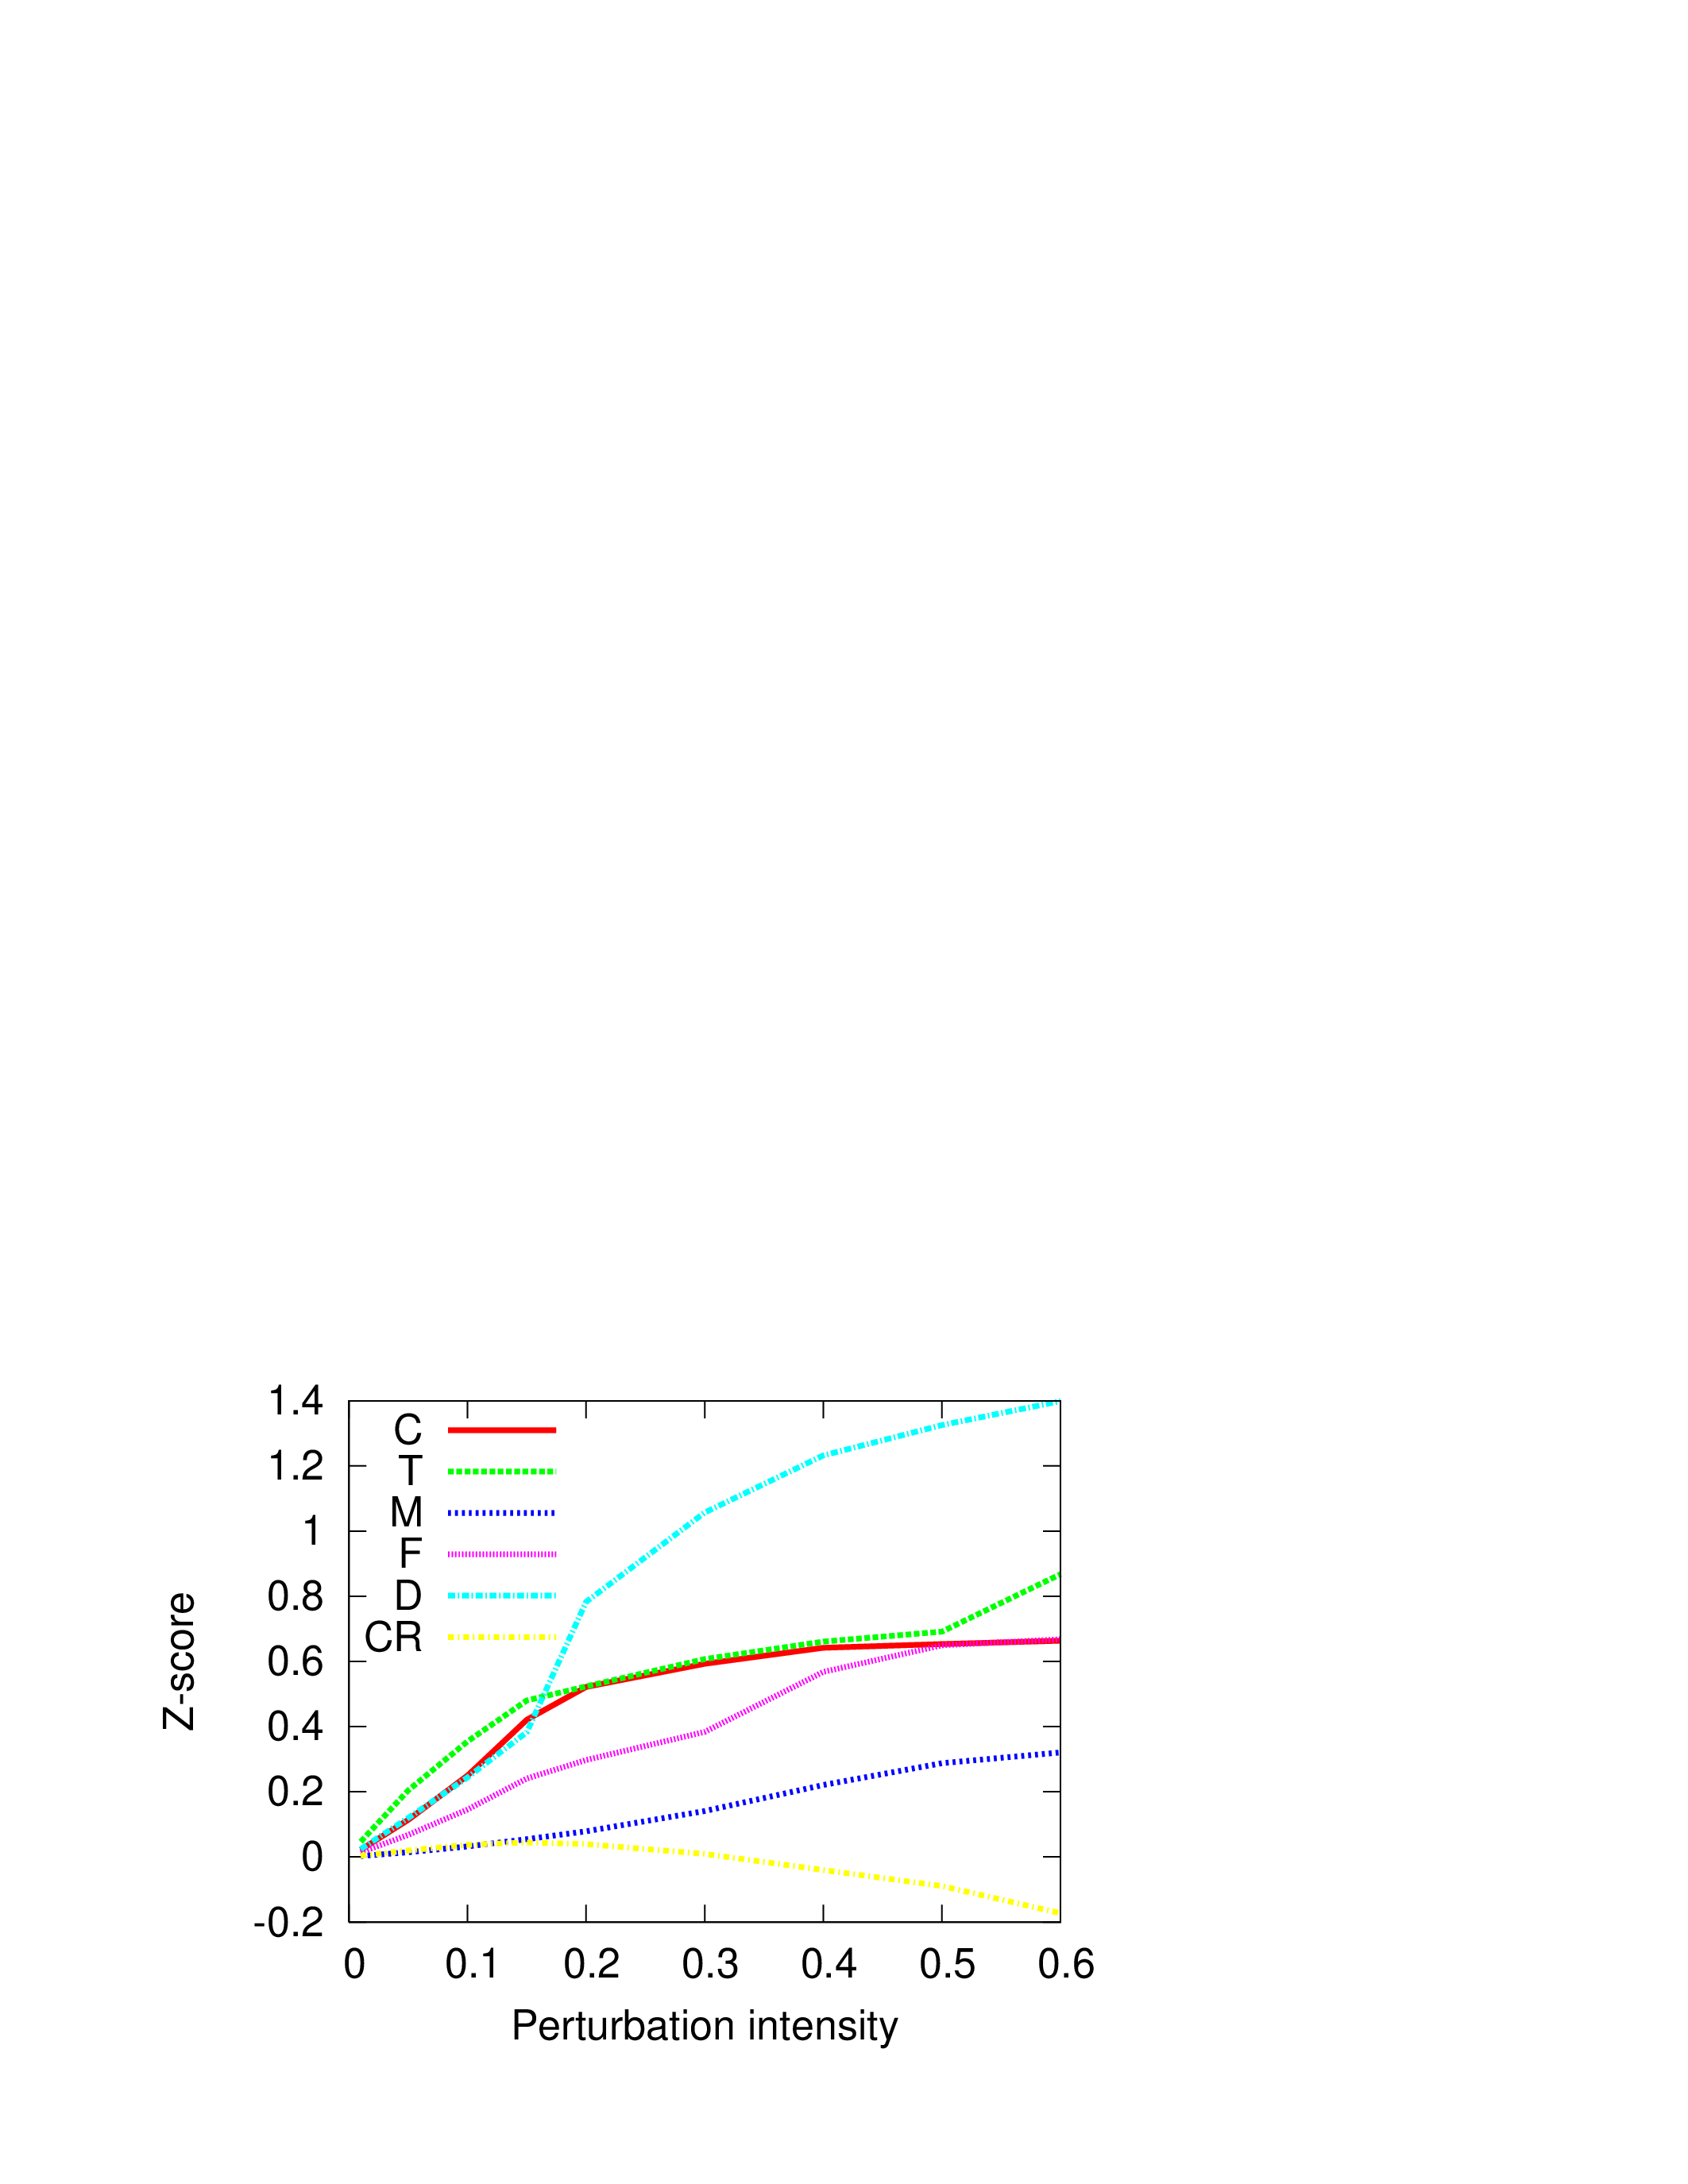}}
	\caption{Z-score of 6 scores versus the perturbation intensity for each null model. NS: NodeSwap, RA: Random, EX: Expand, SH: Shrink.}
\label{fig:All.Sensitivity}
\end{figure}

%% SUBMISSION TO KDD 2012. REVERT THIS FOR ICDM 2012
\hide{
\subsection{Size bias of community scoring functions}
\begin{figure}[t]
	\centering
	\subfigure[\NodeSwap]{\includegraphics[width=0.235\textwidth]{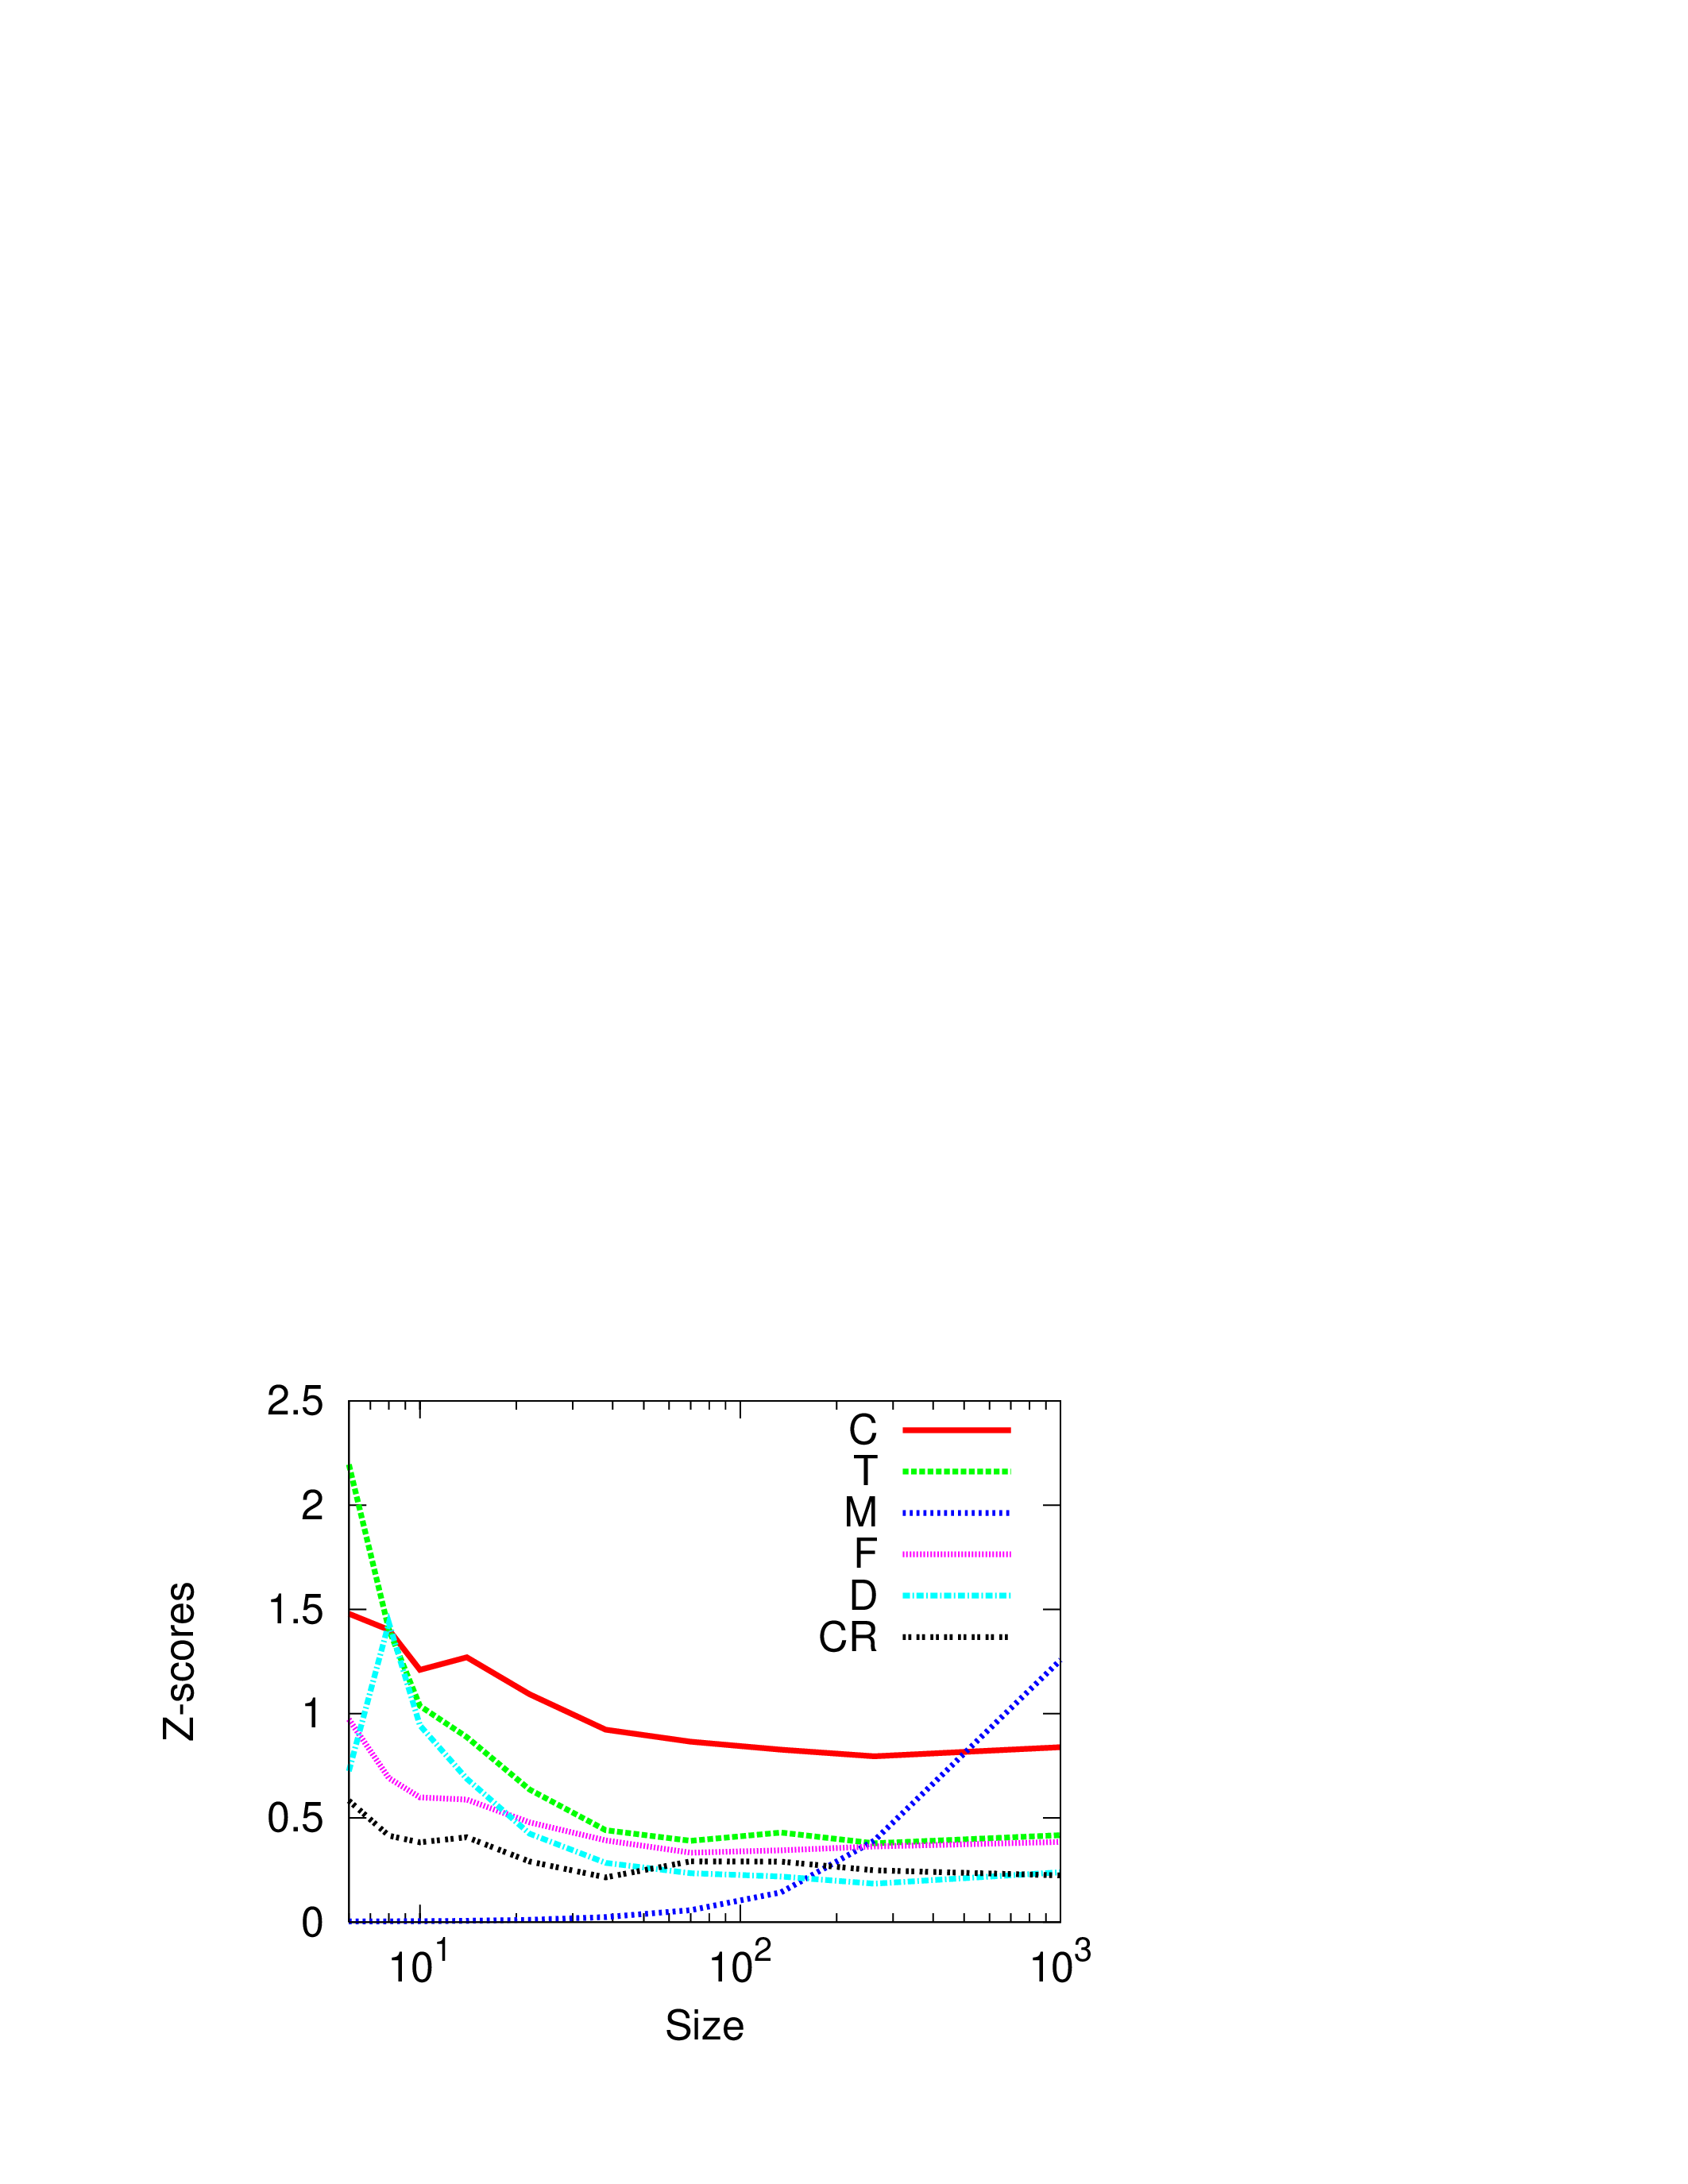}}
	\subfigure[\Random	]{\includegraphics[width=0.235\textwidth]{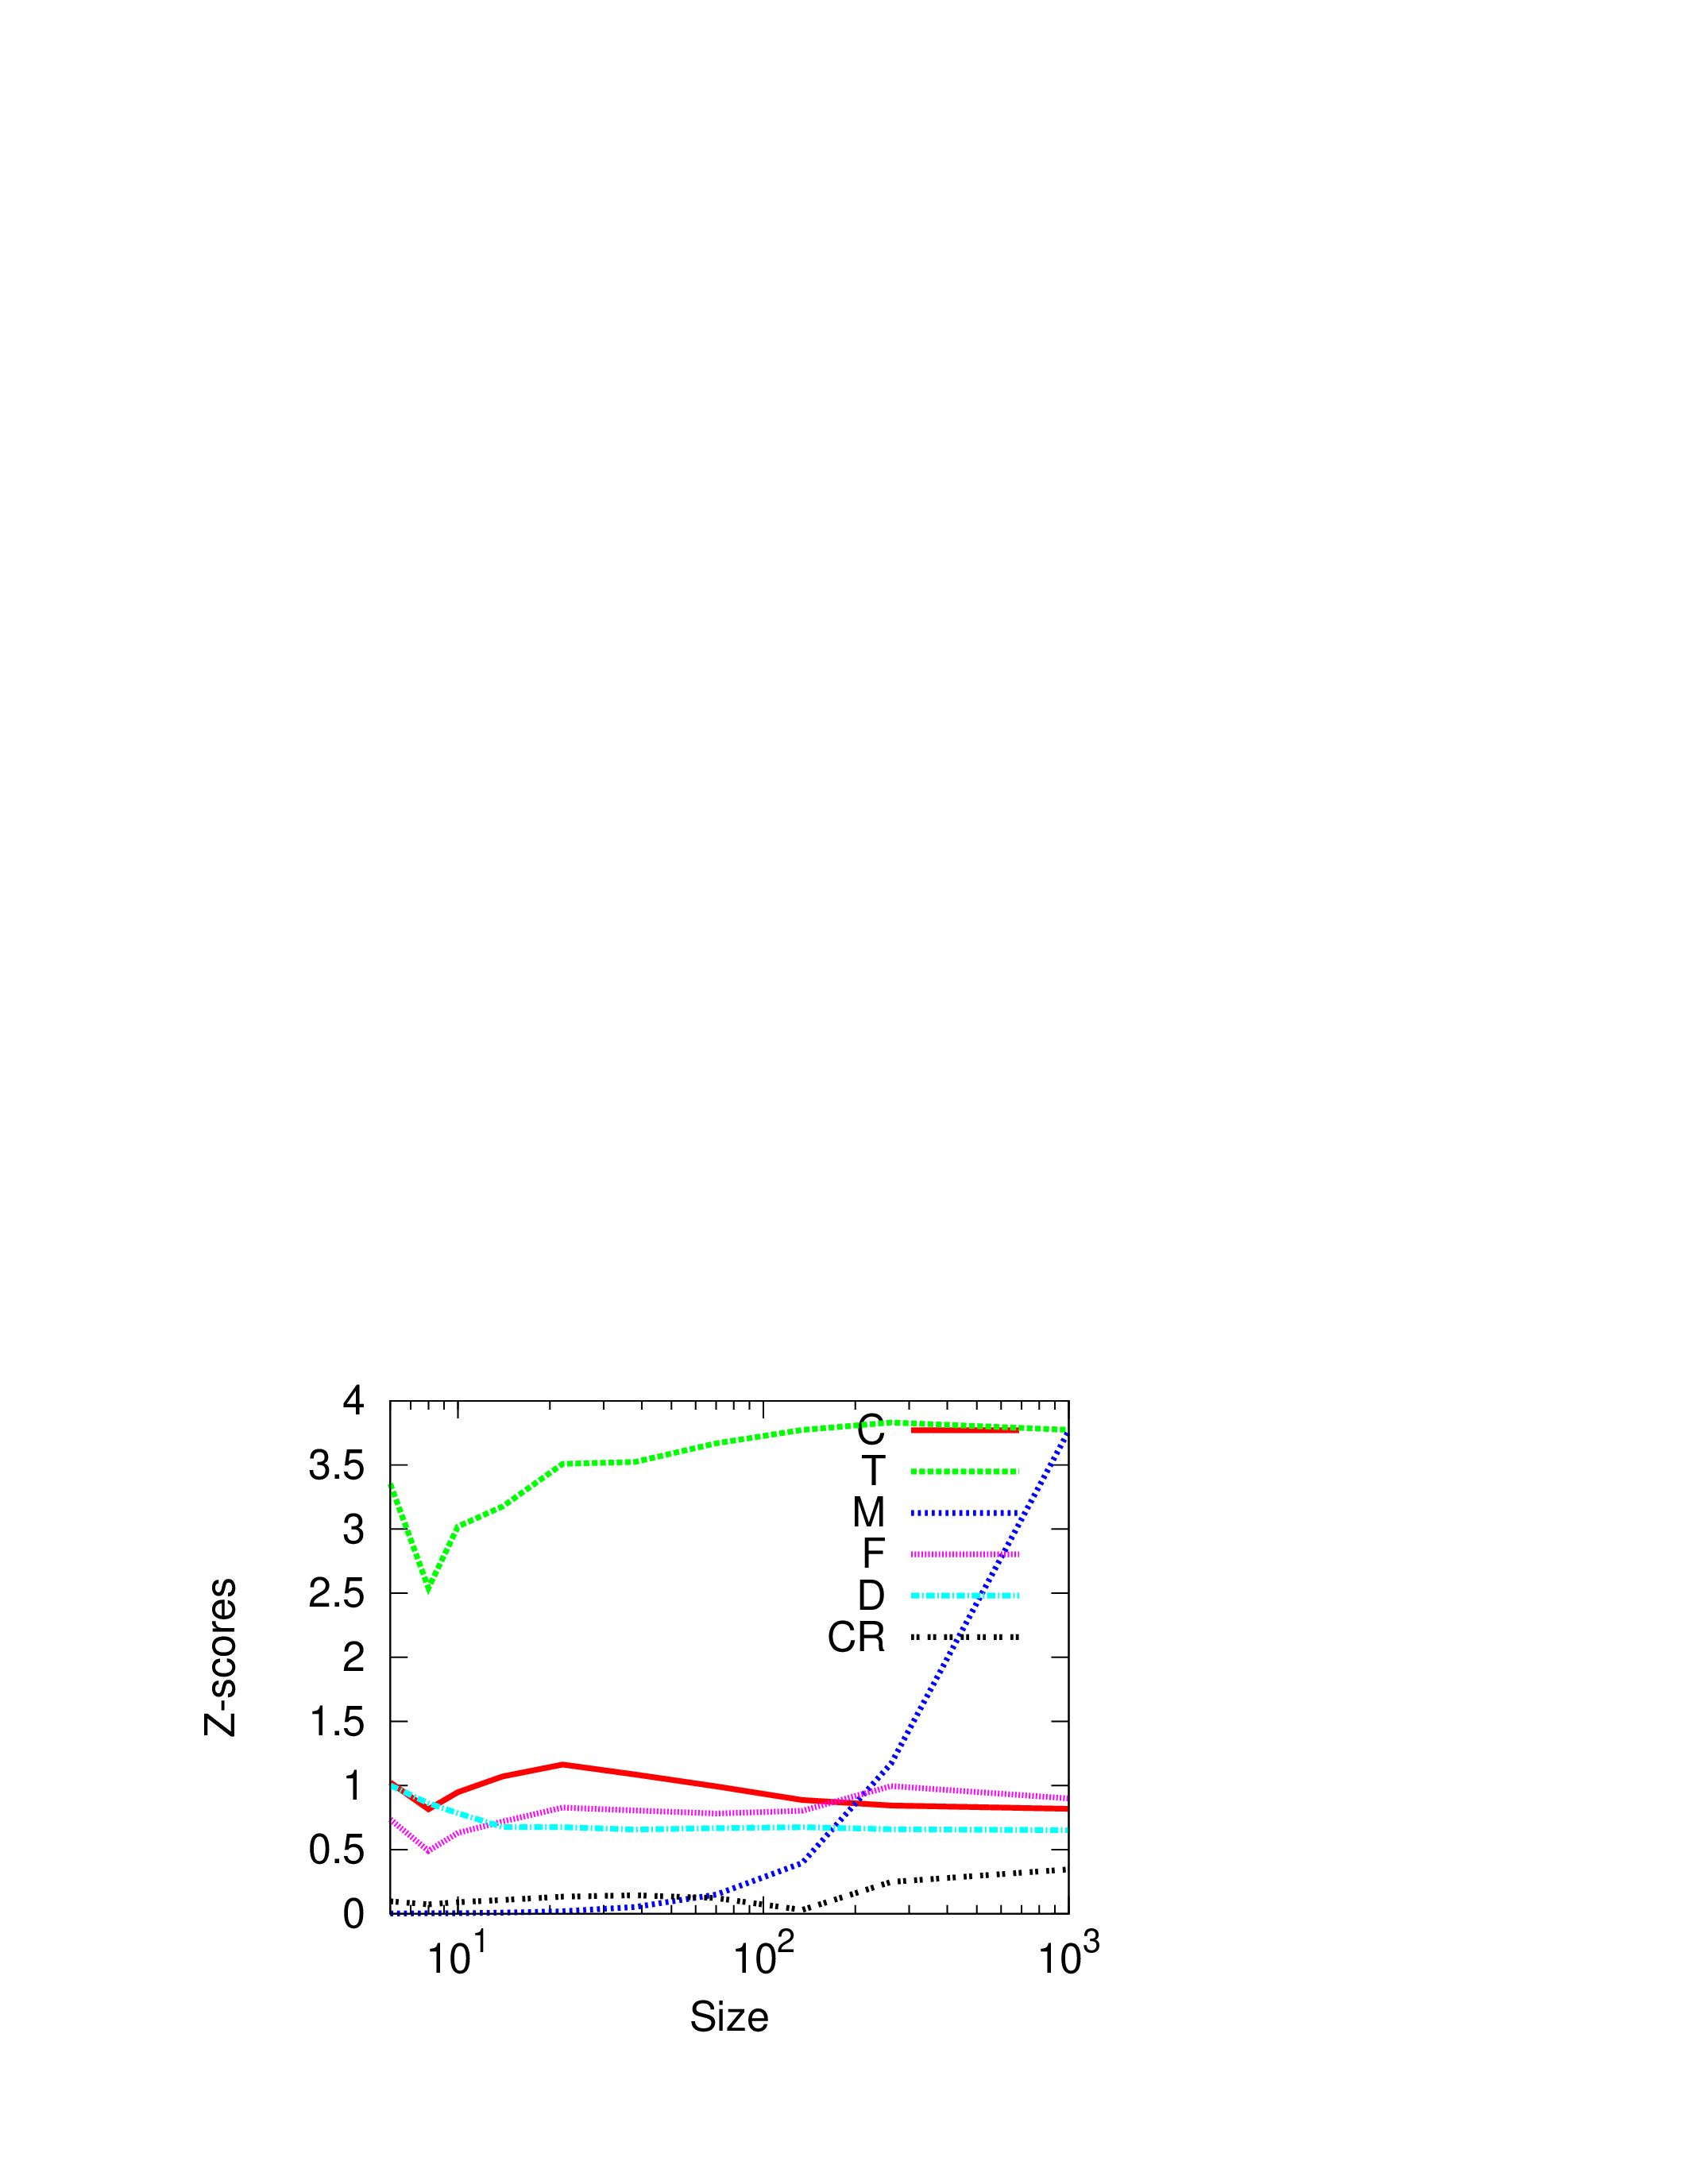}}
	\subfigure[\Expand	]{\includegraphics[width=0.235\textwidth]{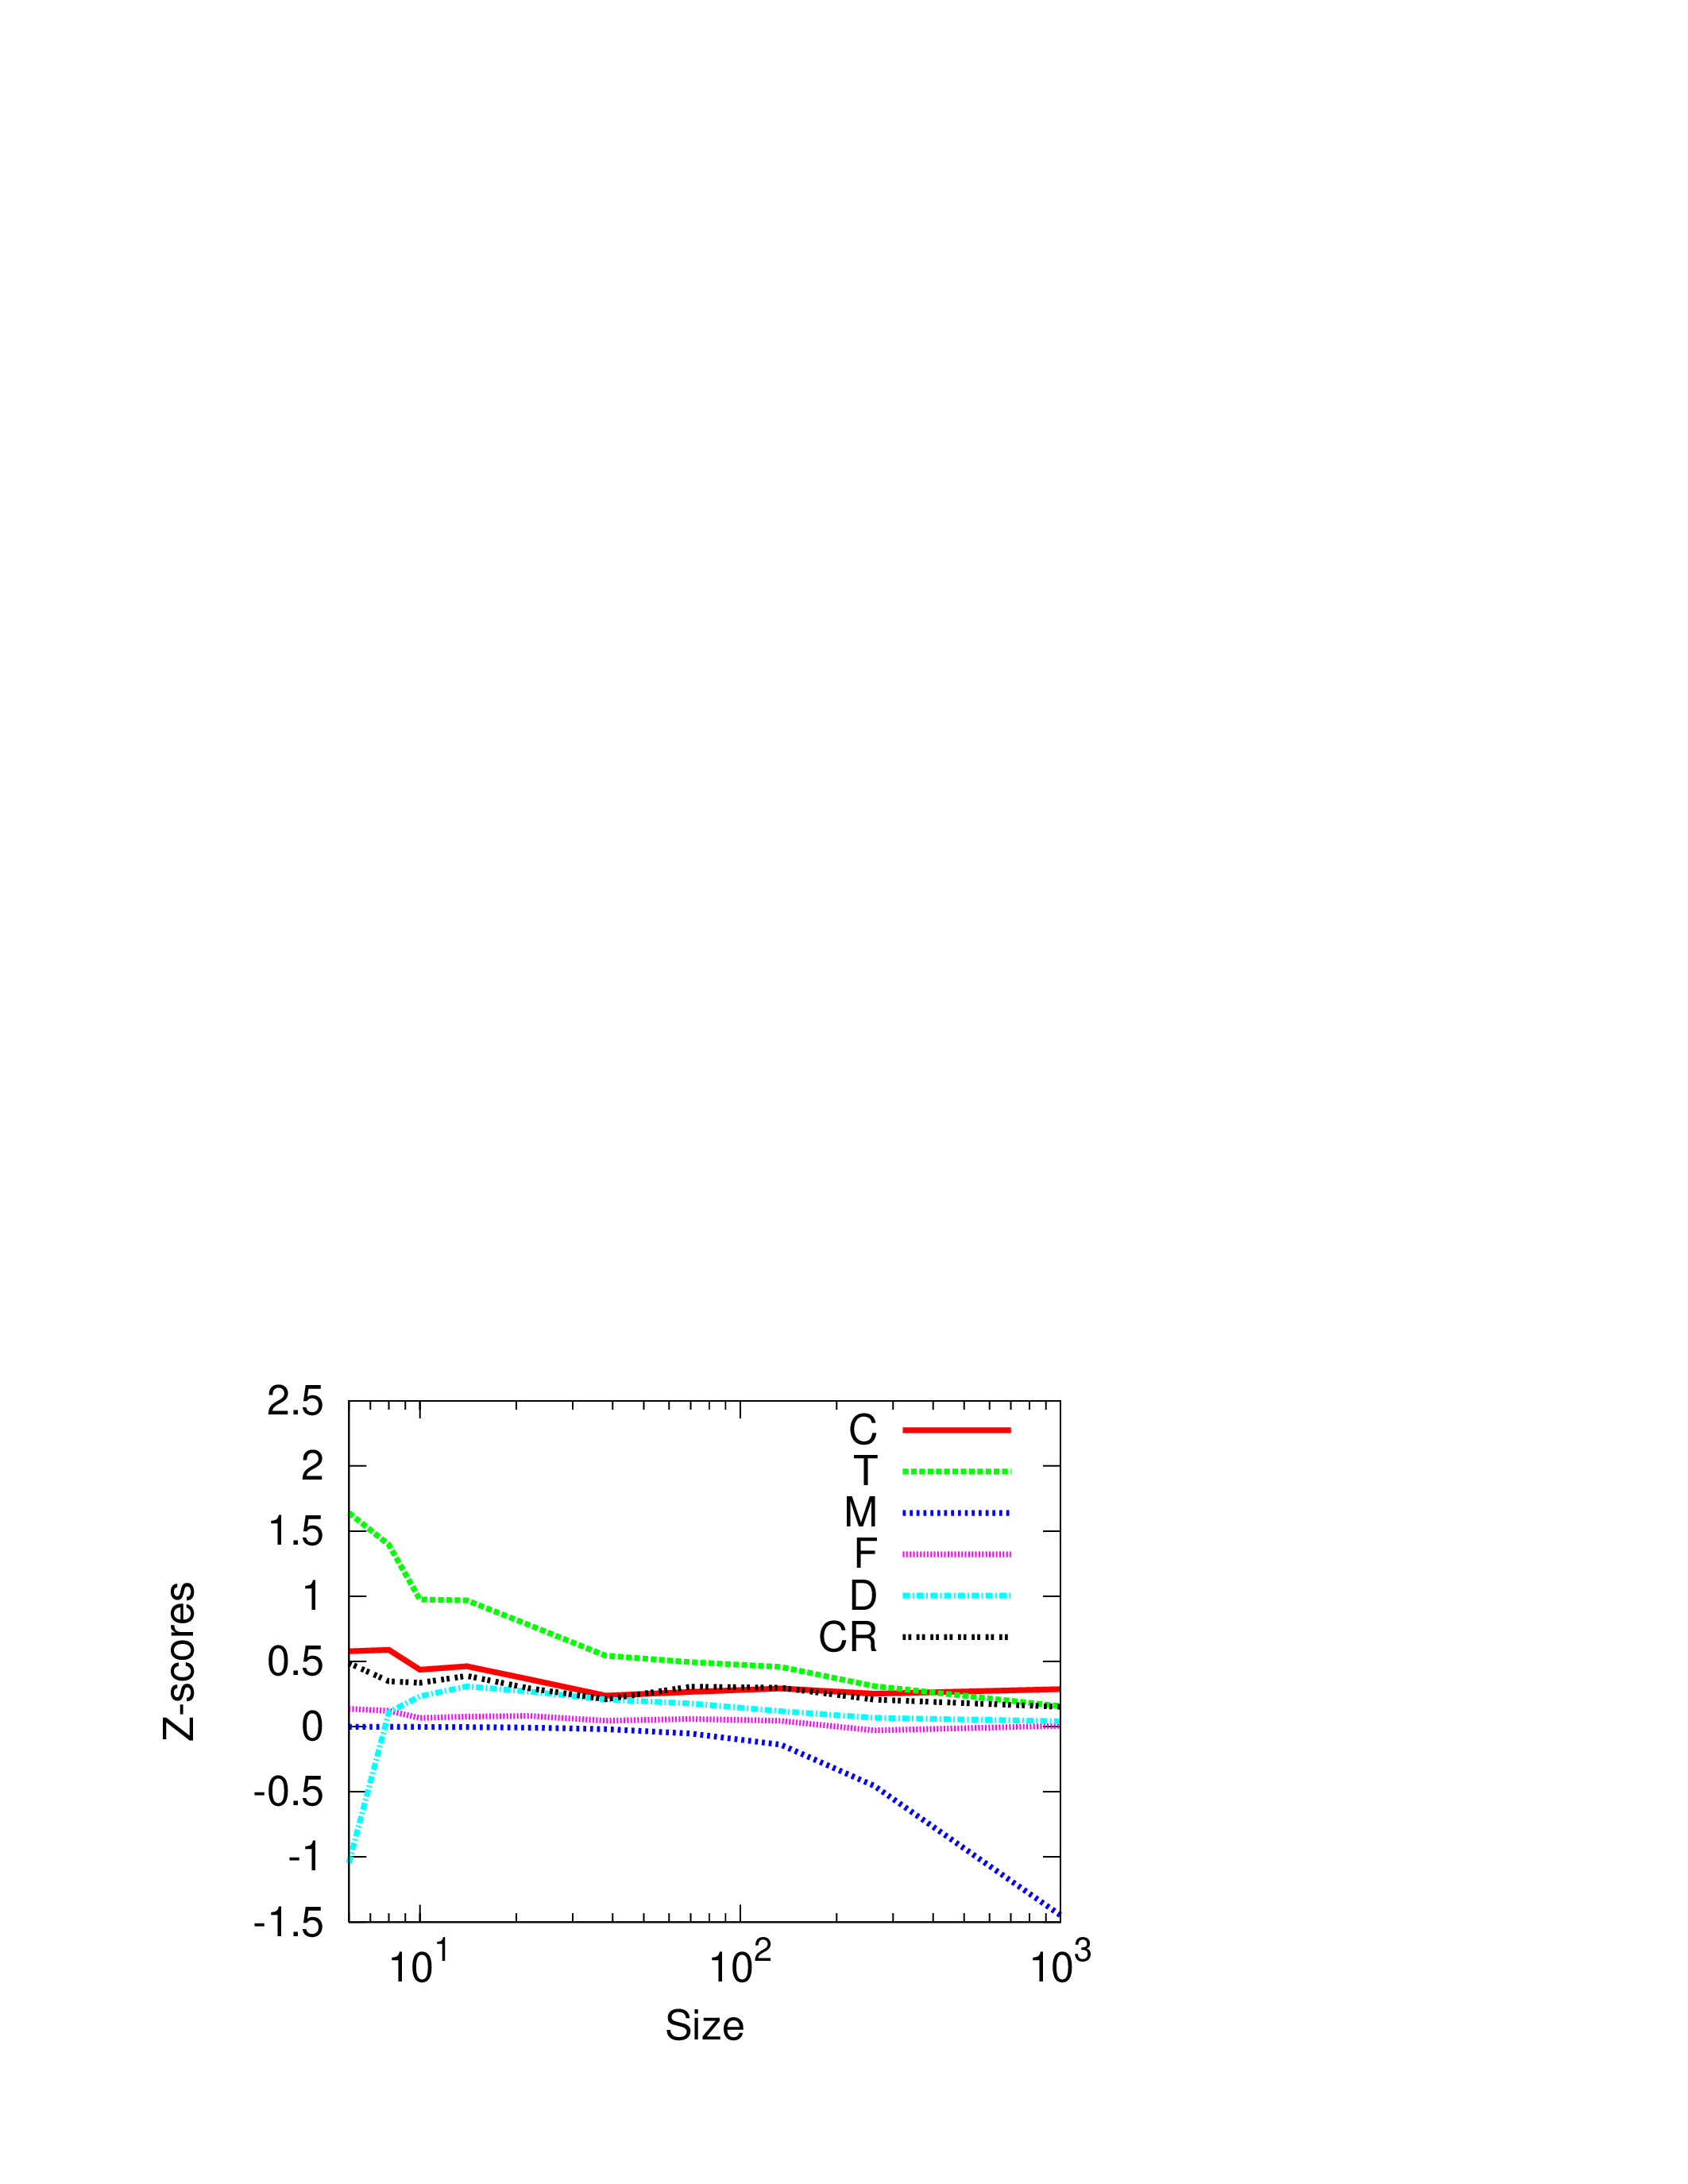}}
	\subfigure[\Shrink	]{\includegraphics[width=0.235\textwidth]{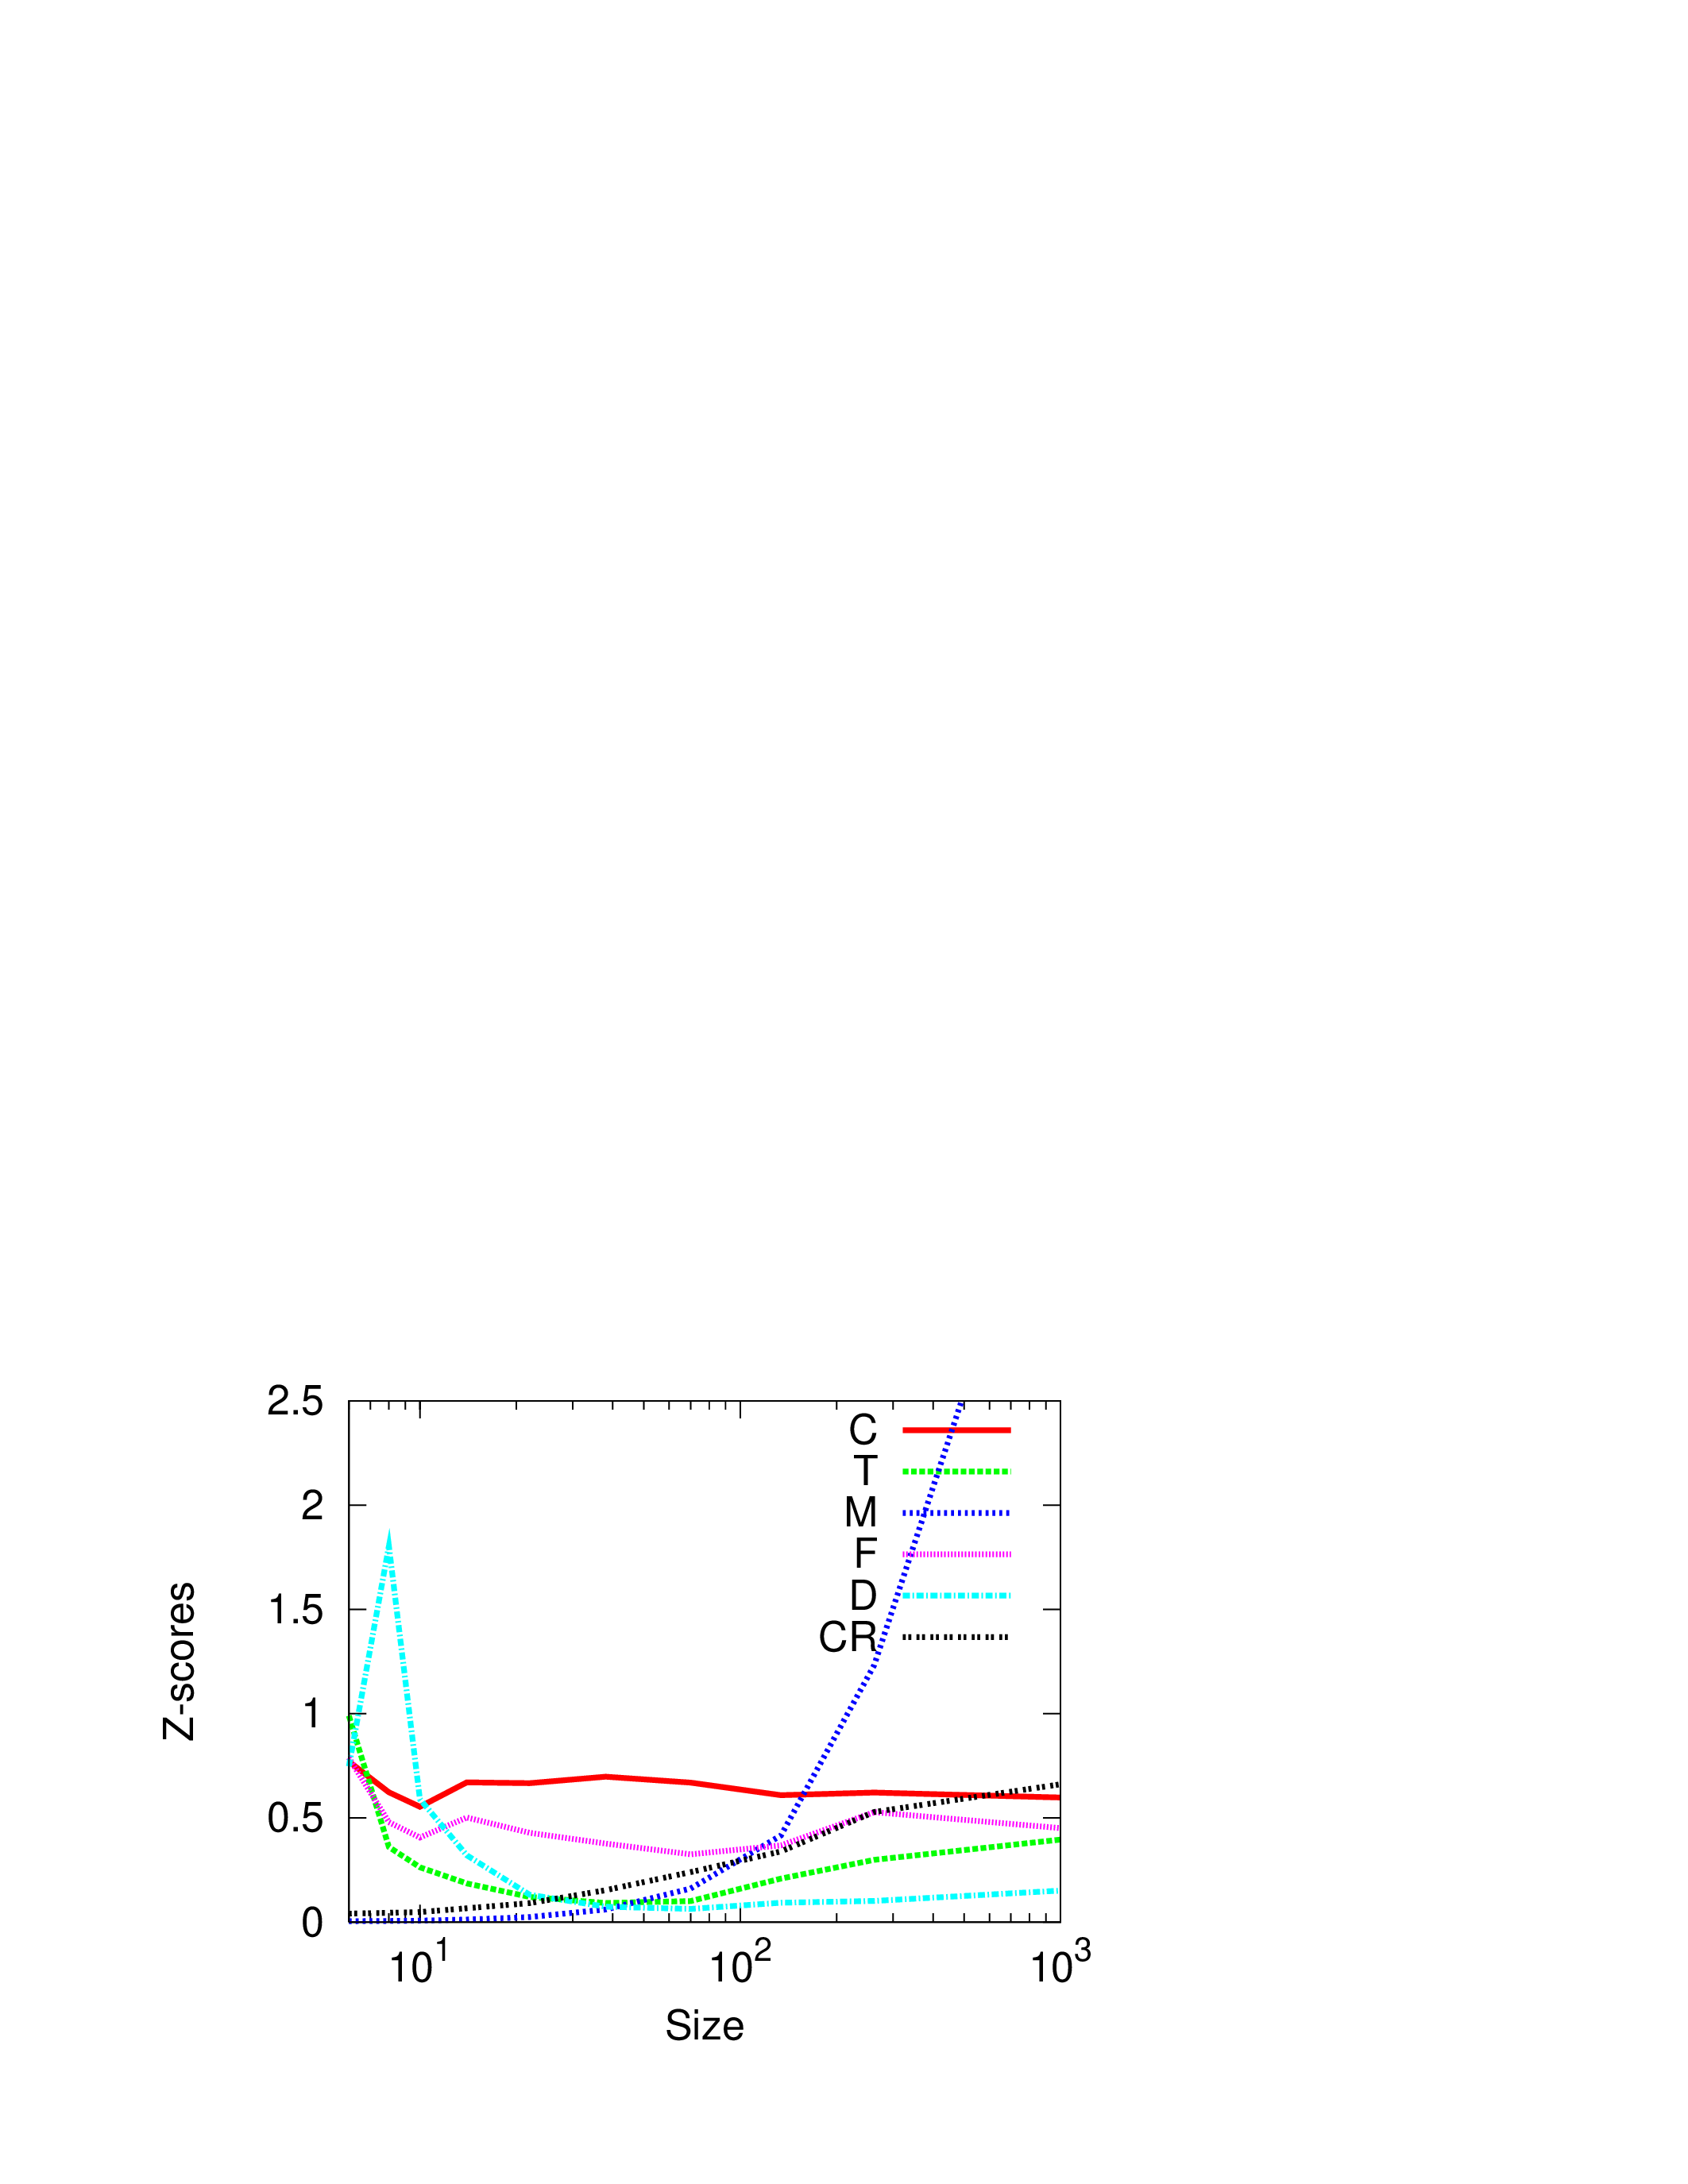}}
%    \vspace{-3mm}
	\caption{Z-score as a function of community size at perturbation intensity $p=0.2$ in LiveJournal.
Modularity (M) fails to detect perturbations of small communities (Z-score is 0). Conductance (C) and Triad participation ratio (T) best detect perturbations and their performance is independent of the community size.}
\label{fig:Zscore.Sz}
  \vspace{-2mm}
\end{figure}

\xhdr{Bias of scoring functions}
The experiments so far revealed surprisingly large differences in the robustness of different community scoring functions. Interestingly, we also observed that Modularity prefers large communities (score increases under \Expand). To further investigate the bias of different community scoring functions on the size of the underlying network community, we perform the following experiment.
%Community scores can show different characteristics depending on the size of communities~\cite{jure10community,Fortunato07_ResolutionPNAS}. Therefore,
We measure how the Z-score changes as a function of the size of the community while keeping perturbation intensity constant. In particular, we calculate the Z-score of each ground-truth community $S_i$ at perturbation intensity level $p = 0.2$, %., $\frac {f(S_i) - f(h(S_i, p))} { \sqrt{Var_i[f(h(S_i, p))]}}$,
and plot it as a function of the community size $|S_i|$. Figure~\ref{fig:Zscore.Sz} shows the results for the LiveJournal communities. Since $p=0.2$ represents relatively large perturbation, high Z-scores are desirable.

We observe that under \NodeSwap Conductance is the most robust score and that as the community size increases, robustness of Conductance slightly decreases. For \Random and \Expand, the Triad participation ratio score performs best over the whole range of network community sizes. Generally, best performing scores tend to be more sensitive on small communities. The exception is modularity.
The Z-score of modularity is very close to 0 for communities smaller than 100 members, \ie, modularity cannot distinguish a community and a perturbed community when the community is smaller than around 100 nodes. However, for large communities, modularity score shows high Z-scores, except under the \Expand perturbation, where it favors larger null communities.
We observe very similar results on all 229 remaining datasets considered in this study. Refer to extended version of the paper for the details~\cite{jaewon11comscore}.

\begin{figure*}[t]
	\centering
	\subfigure[Separability	(LJ)]{\includegraphics[width=0.16\textwidth]{rank_property.CutToEdgeIns.lj.eps}}
	\subfigure[Separability	 (FS)]{\includegraphics[width=0.16\textwidth]{rank_property.CutToEdgeIns.friendster.eps}}
	\subfigure[Separability	 (Orkut)]{\includegraphics[width=0.16\textwidth]{rank_property.CutToEdgeIns.orkut.eps}}
	\subfigure[Separability	 (Ning)]{\includegraphics[width=0.16\textwidth]{rank_property.CutToEdgeIns.Ning.eps}}
	\subfigure[Separability	 (Amazon)]{\includegraphics[width=0.16\textwidth]{rank_property.CutToEdgeIns.amazon.eps}}
	\subfigure[Separability	 (DBLP)]{\includegraphics[width=0.16\textwidth]{rank_property.CutToEdgeIns.dblp.eps}}
	\subfigure[Density	(LJ)]{\includegraphics[width=0.16\textwidth]{rank_property.Density.lj.eps}}
	\subfigure[Density	(FS)]{\includegraphics[width=0.16\textwidth]{rank_property.Density.friendster.eps}}
	\subfigure[Density	(Orkut)]{\includegraphics[width=0.16\textwidth]{rank_property.Density.orkut.eps}}
	\subfigure[Density	(Ning)]{\includegraphics[width=0.16\textwidth]{rank_property.Density.Ning.eps}}
	\subfigure[Density	(Amazon)]{\includegraphics[width=0.16\textwidth]{rank_property.Density.amazon.eps}}
	\subfigure[Density	(DBLP)]{\includegraphics[width=0.16\textwidth]{rank_property.Density.dblp.eps}}
	\subfigure[Cohesiveness	(LJ)]{\includegraphics[width=0.16\textwidth]{rank_property.InsidePhi.lj.eps}}
	\subfigure[Cohesiveness	 (FS)]{\includegraphics[width=0.16\textwidth]{rank_property.InsidePhi.friendster.eps}}
	\subfigure[Cohesiveness	(Orkut)]{\includegraphics[width=0.16\textwidth]{rank_property.InsidePhi.orkut.eps}}
	\subfigure[Cohesiveness	(Ning)]{\includegraphics[width=0.16\textwidth]{rank_property.InsidePhi.Ning.eps}}
	\subfigure[Cohesiveness	 (Amazon)]{\includegraphics[width=0.16\textwidth]{rank_property.InsidePhi.amazon.eps}}
	\subfigure[Cohesiveness	(DBLP)]{\includegraphics[width=0.16\textwidth]{rank_property.InsidePhi.dblp.eps}}
	\subfigure[CCF	(LJ)]{\includegraphics[width=0.16\textwidth]{rank_property.CCf.lj.eps}}
	\subfigure[CCF	(FS)]{\includegraphics[width=0.16\textwidth]{rank_property.CCf.friendster.eps}}
	\subfigure[CCF	(Orkut)]{\includegraphics[width=0.16\textwidth]{rank_property.CCf.orkut.eps}}
	\subfigure[CCF	(Ning)]{\includegraphics[width=0.16\textwidth]{rank_property.CCf.Ning.eps}}
	\subfigure[CCF	(Amazon)]{\includegraphics[width=0.16\textwidth]{rank_property.CCf.amazon.eps}}
	\subfigure[CCF	(DBLP)]{\includegraphics[width=0.16\textwidth]{rank_property.CCf.dblp.eps}}
	\caption{Average metrics of	top	k	communities	by 7 scores. C: Conductance, T: TPR, M: Modularity, R: Average Rank U: Practical upper bound for the metric}
\label{fig:rank.AvgPath}
\end{figure*}

\begin{figure*}[t]
	\centering
	\subfigure[NodeSwap	(LJ)]{\includegraphics[width=0.16\textwidth]{sens.NodeSwap.lj.eps}}
	\subfigure[NodeSwap	(FS)]{\includegraphics[width=0.16\textwidth]{sens.NodeSwap.friendster.eps}}
	\subfigure[NodeSwap	(Orkut)]{\includegraphics[width=0.16\textwidth]{sens.NodeSwap.orkut.eps}}
	\subfigure[NodeSwap	(Ning)]{\includegraphics[width=0.16\textwidth]{sens.NodeSwap.Ning.eps}}
	\subfigure[NodeSwap	(Amazon)]{\includegraphics[width=0.16\textwidth]{sens.NodeSwap.amazon.eps}}
	\subfigure[NodeSwap	(DBLP)]{\includegraphics[width=0.16\textwidth]{sens.NodeSwap.dblp.eps}}
	\subfigure[Random	(LJ)]{\includegraphics[width=0.16\textwidth]{sens.Random.lj.eps}}
	\subfigure[Random	(FS)]{\includegraphics[width=0.16\textwidth]{sens.Random.friendster.eps}}
	\subfigure[Random	(Orkut)]{\includegraphics[width=0.16\textwidth]{sens.Random.orkut.eps}}
	\subfigure[Random	(Ning)]{\includegraphics[width=0.16\textwidth]{sens.Random.Ning.eps}}
	\subfigure[Random	(Amazon)]{\includegraphics[width=0.16\textwidth]{sens.Random.amazon.eps}}
	\subfigure[Random	(DBLP)]{\includegraphics[width=0.16\textwidth]{sens.Random.dblp.eps}}
	\subfigure[Expand	(LJ)]{\includegraphics[width=0.16\textwidth]{sens.Expand.lj.eps}}
	\subfigure[Expand	(FS)]{\includegraphics[width=0.16\textwidth]{sens.Expand.friendster.eps}}
	\subfigure[Expand	(Orkut)]{\includegraphics[width=0.16\textwidth]{sens.Expand.orkut.eps}}
	\subfigure[Expand	(Ning)]{\includegraphics[width=0.16\textwidth]{sens.Expand.Ning.eps}}
	\subfigure[Expand	(Amazon)]{\includegraphics[width=0.16\textwidth]{sens.Expand.amazon.eps}}
	\subfigure[Expand	(DBLP)]{\includegraphics[width=0.16\textwidth]{sens.Expand.dblp.eps}}
	\subfigure[Shrink	(LJ)]{\includegraphics[width=0.16\textwidth]{sens.Shrink.lj.eps}}
	\subfigure[Shrink	(FS)]{\includegraphics[width=0.16\textwidth]{sens.Shrink.friendster.eps}}
	\subfigure[Shrink	(Orkut)]{\includegraphics[width=0.16\textwidth]{sens.Shrink.orkut.eps}}
	\subfigure[Shrink	(Ning)]{\includegraphics[width=0.16\textwidth]{sens.Shrink.Ning.eps}}
	\subfigure[Shrink	(Amazon)]{\includegraphics[width=0.16\textwidth]{sens.Shrink.amazon.eps}}
	\subfigure[Shrink	(DBLP)]{\includegraphics[width=0.16\textwidth]{sens.Shrink.dblp.eps}}
	\caption{Z-score of 6 scores versus the perturbation intensity for each null model. C: Conductance, T: TPR, M: Modularity, F: Flake-ODF, D: FOMD, CR: Cut-Ratio}
\label{fig:Sensitivity}
\end{figure*}

\begin{figure*}[t]
	\centering
	\subfigure[NodeSwap	(LJ)]{\includegraphics[width=0.16\textwidth]{zscore.sz.NodeSwap.lj.eps}}
	\subfigure[NodeSwap	(FS)]{\includegraphics[width=0.16\textwidth]{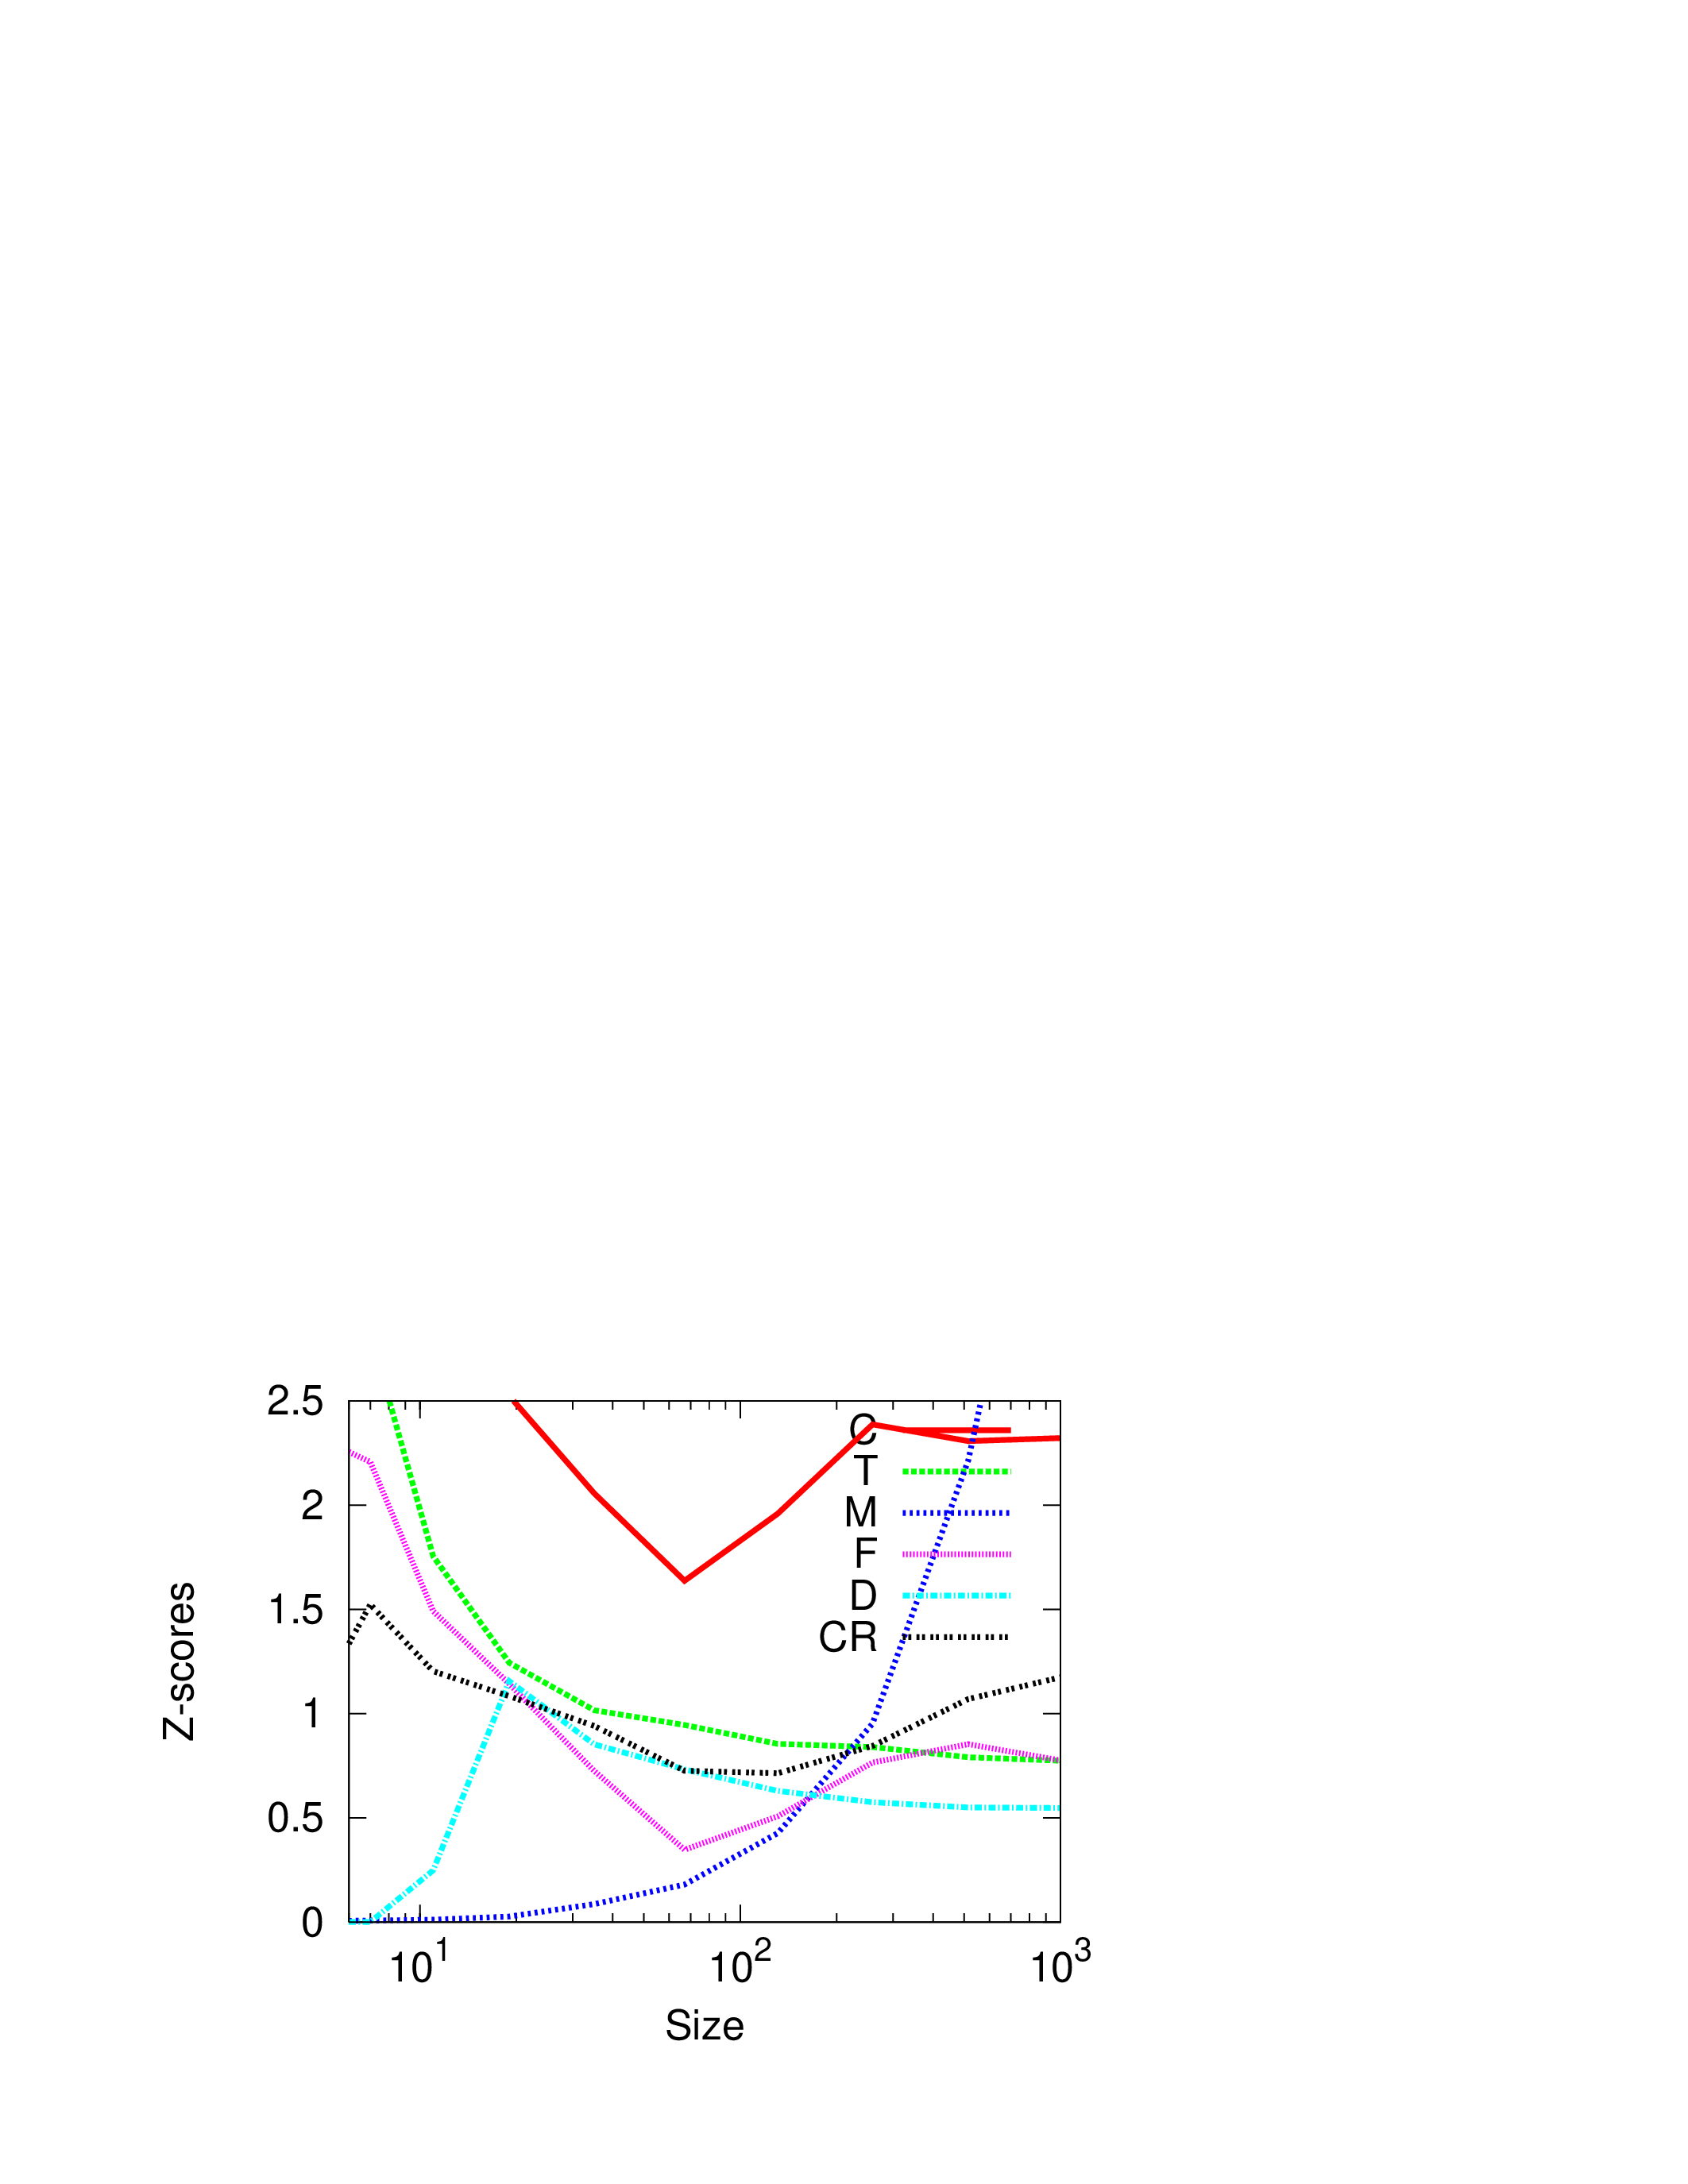}}
	\subfigure[NodeSwap	(Orkut)]{\includegraphics[width=0.16\textwidth]{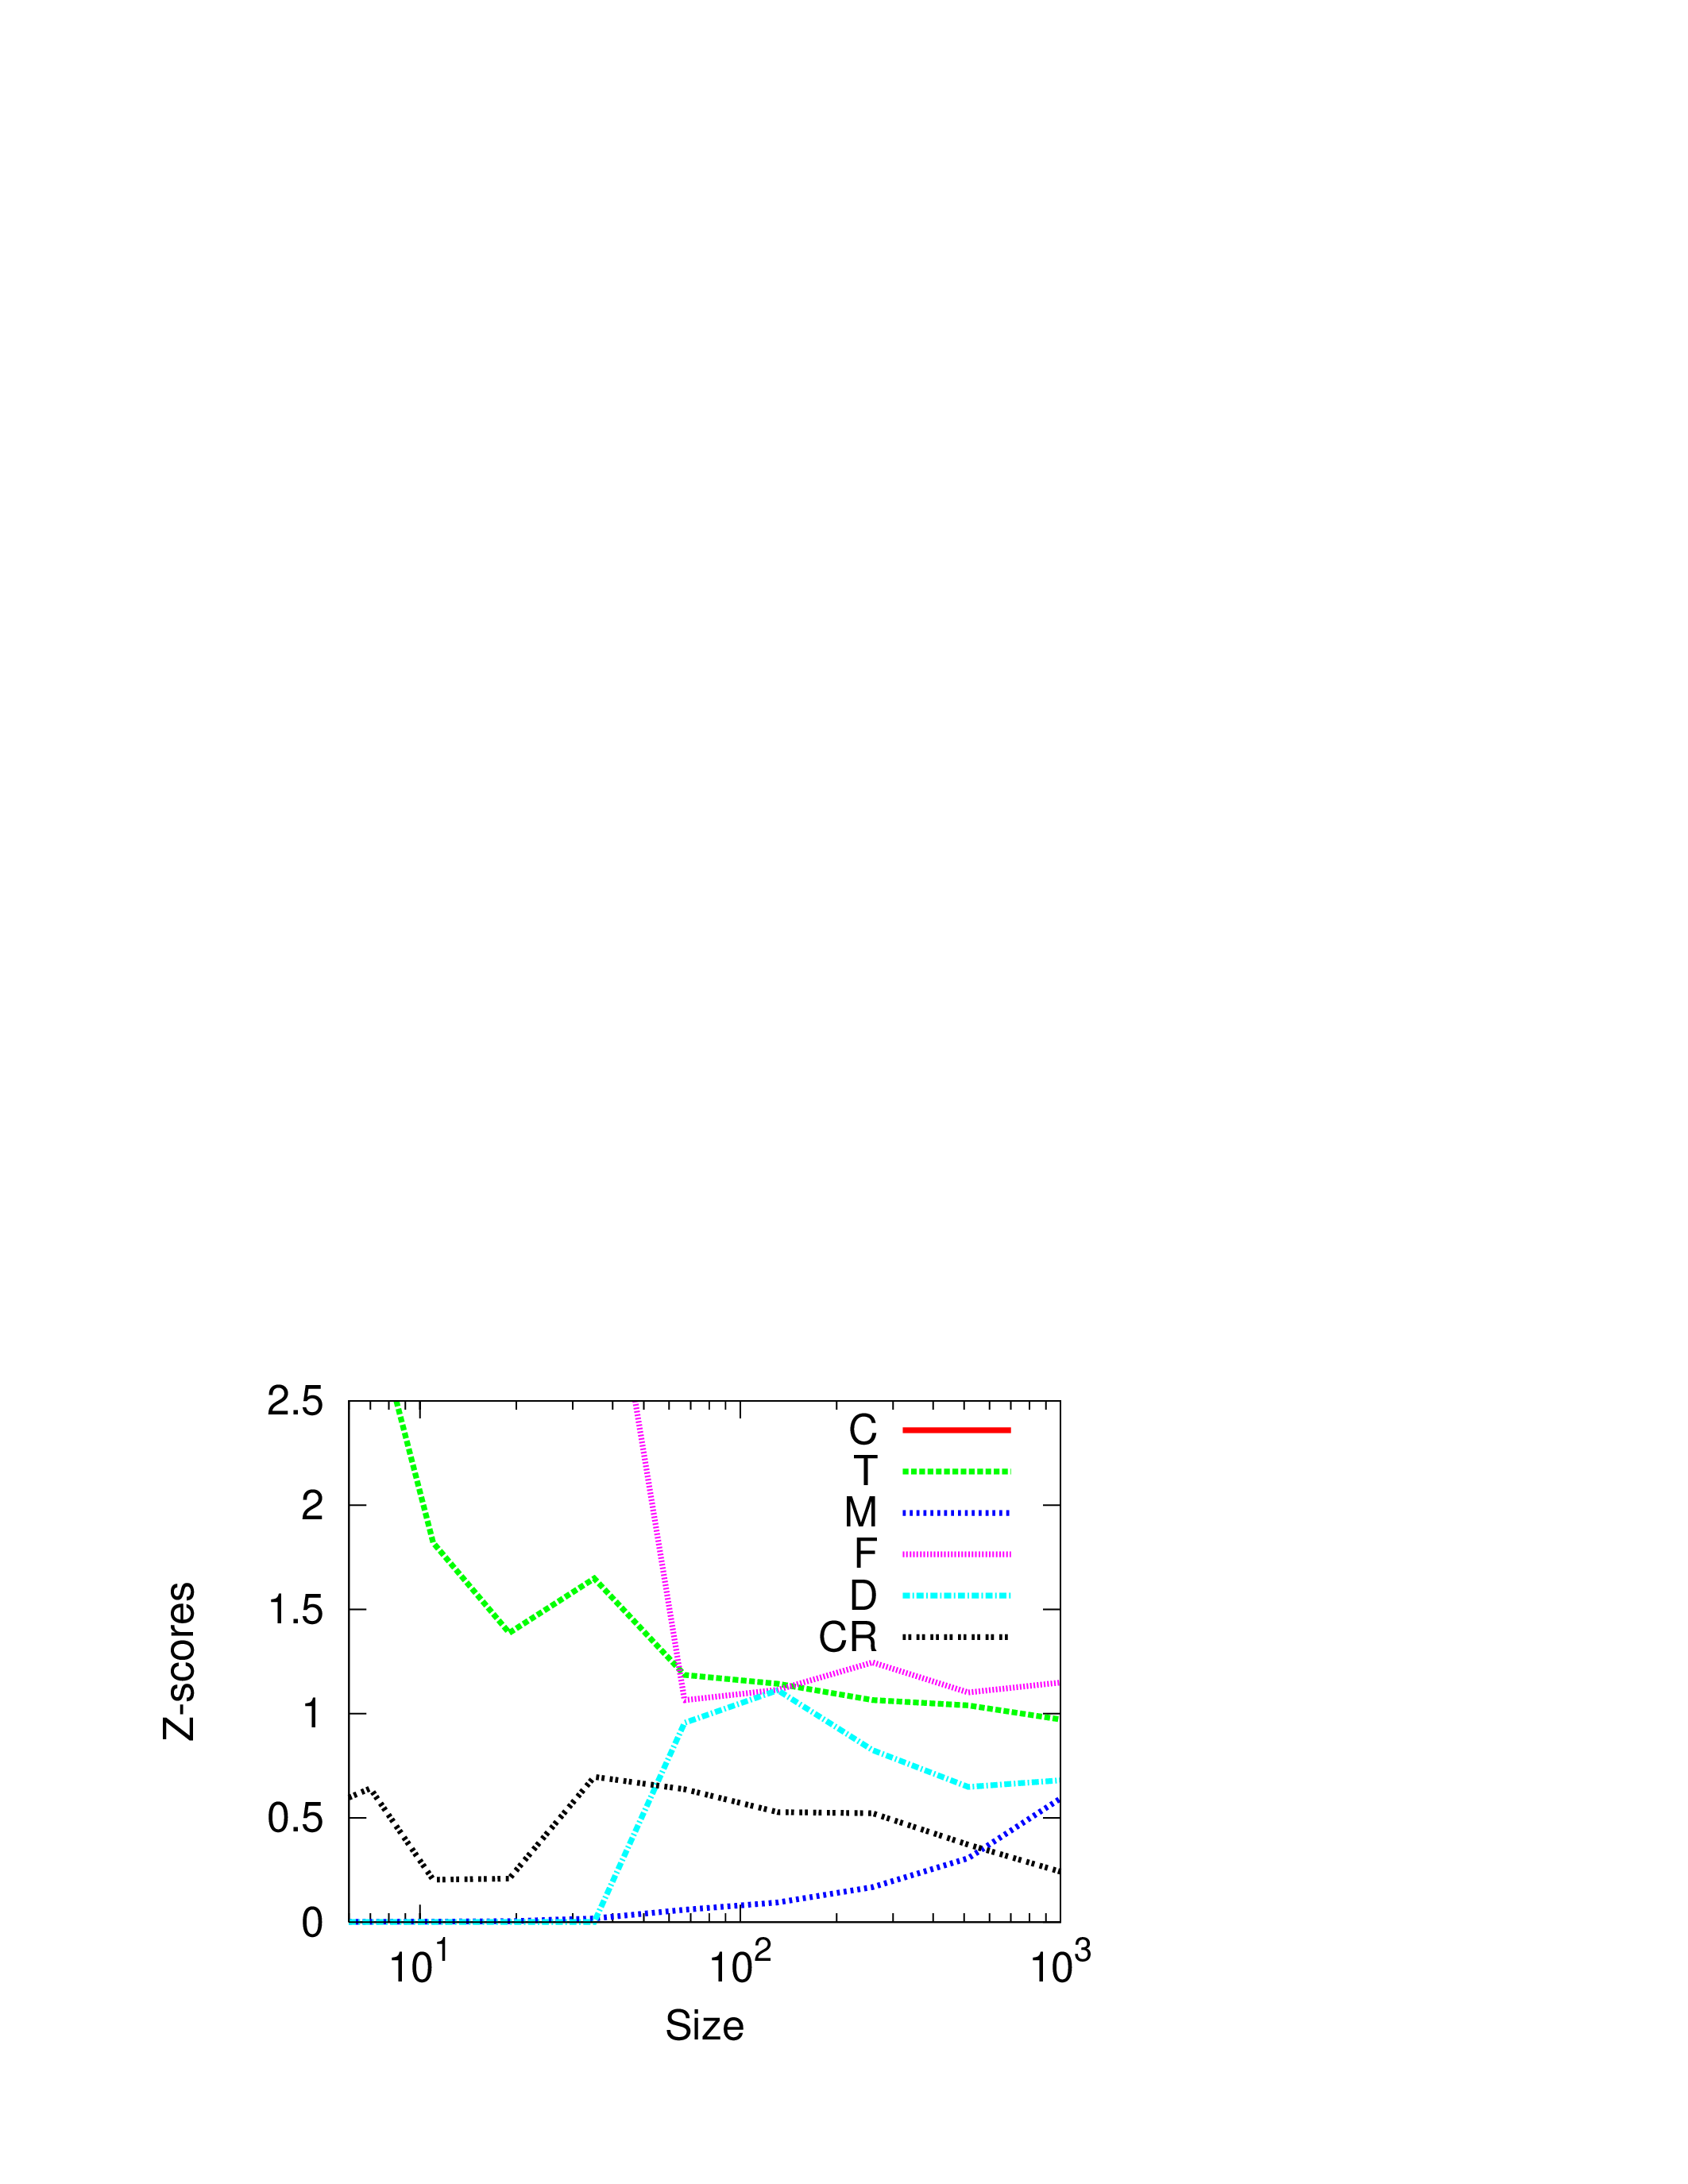}}
	\subfigure[NodeSwap	(Ning)]{\includegraphics[width=0.16\textwidth]{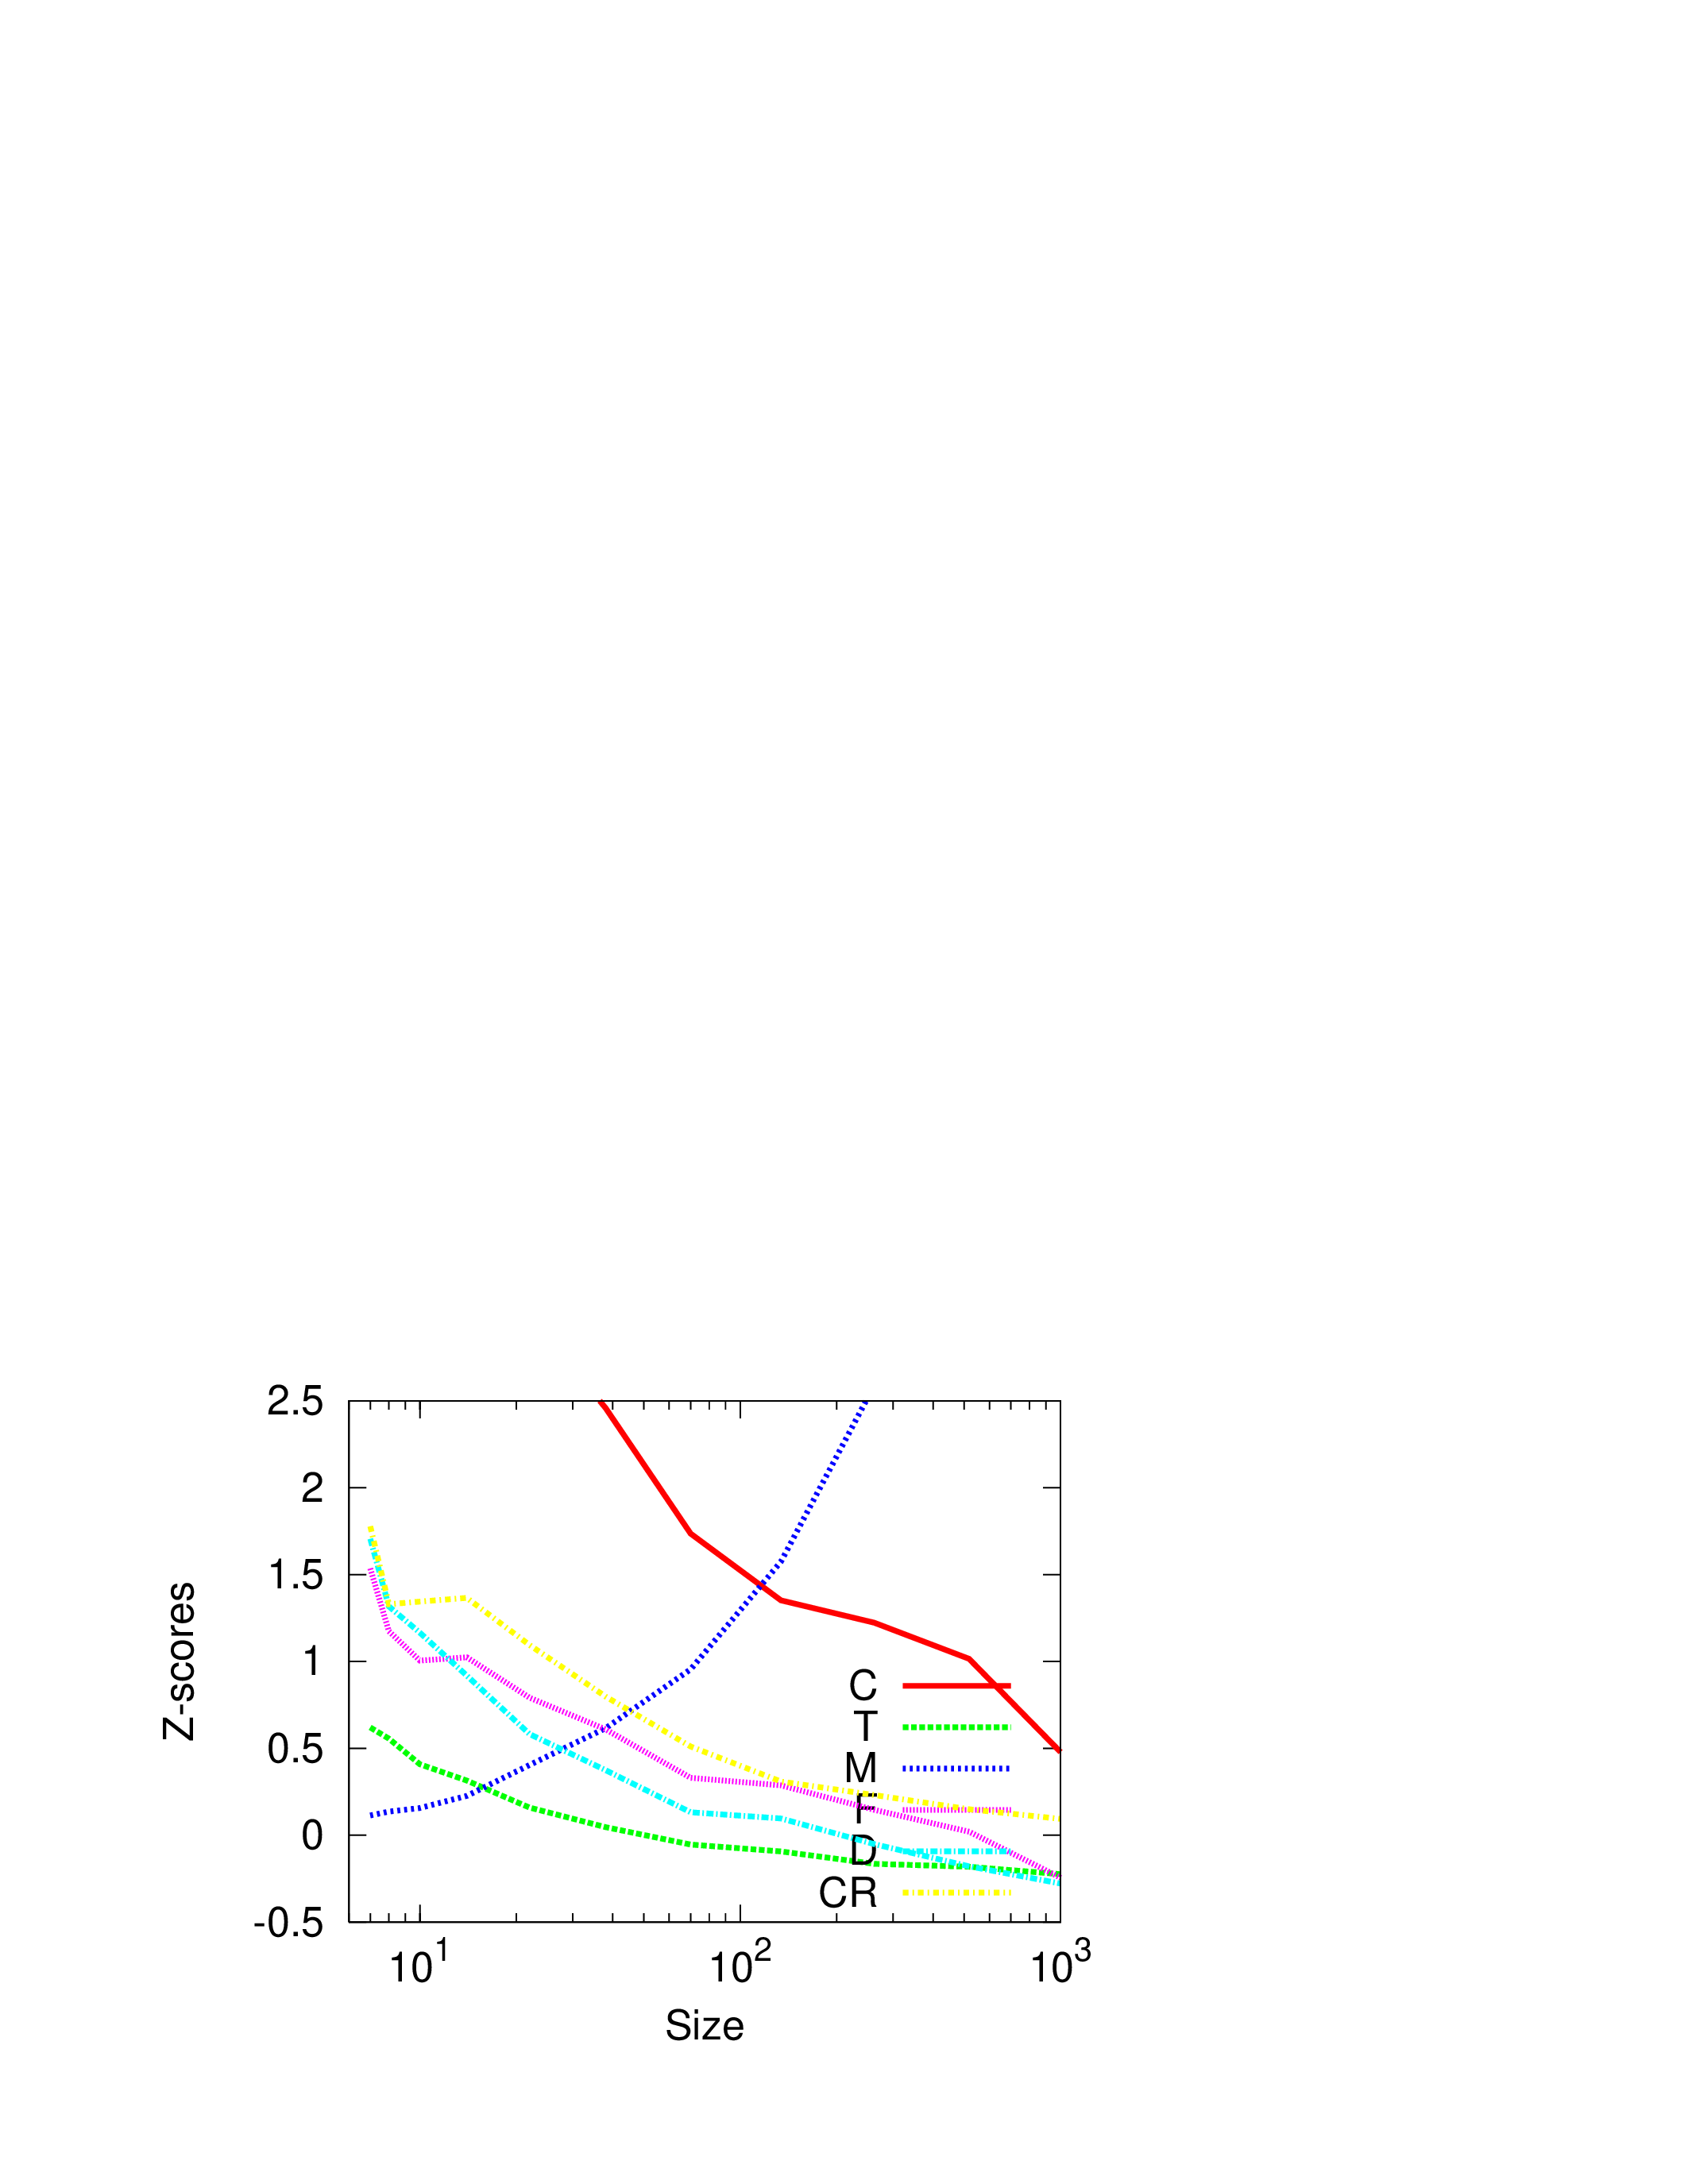}}
	\subfigure[NodeSwap	(Amazon)]{\includegraphics[width=0.16\textwidth]{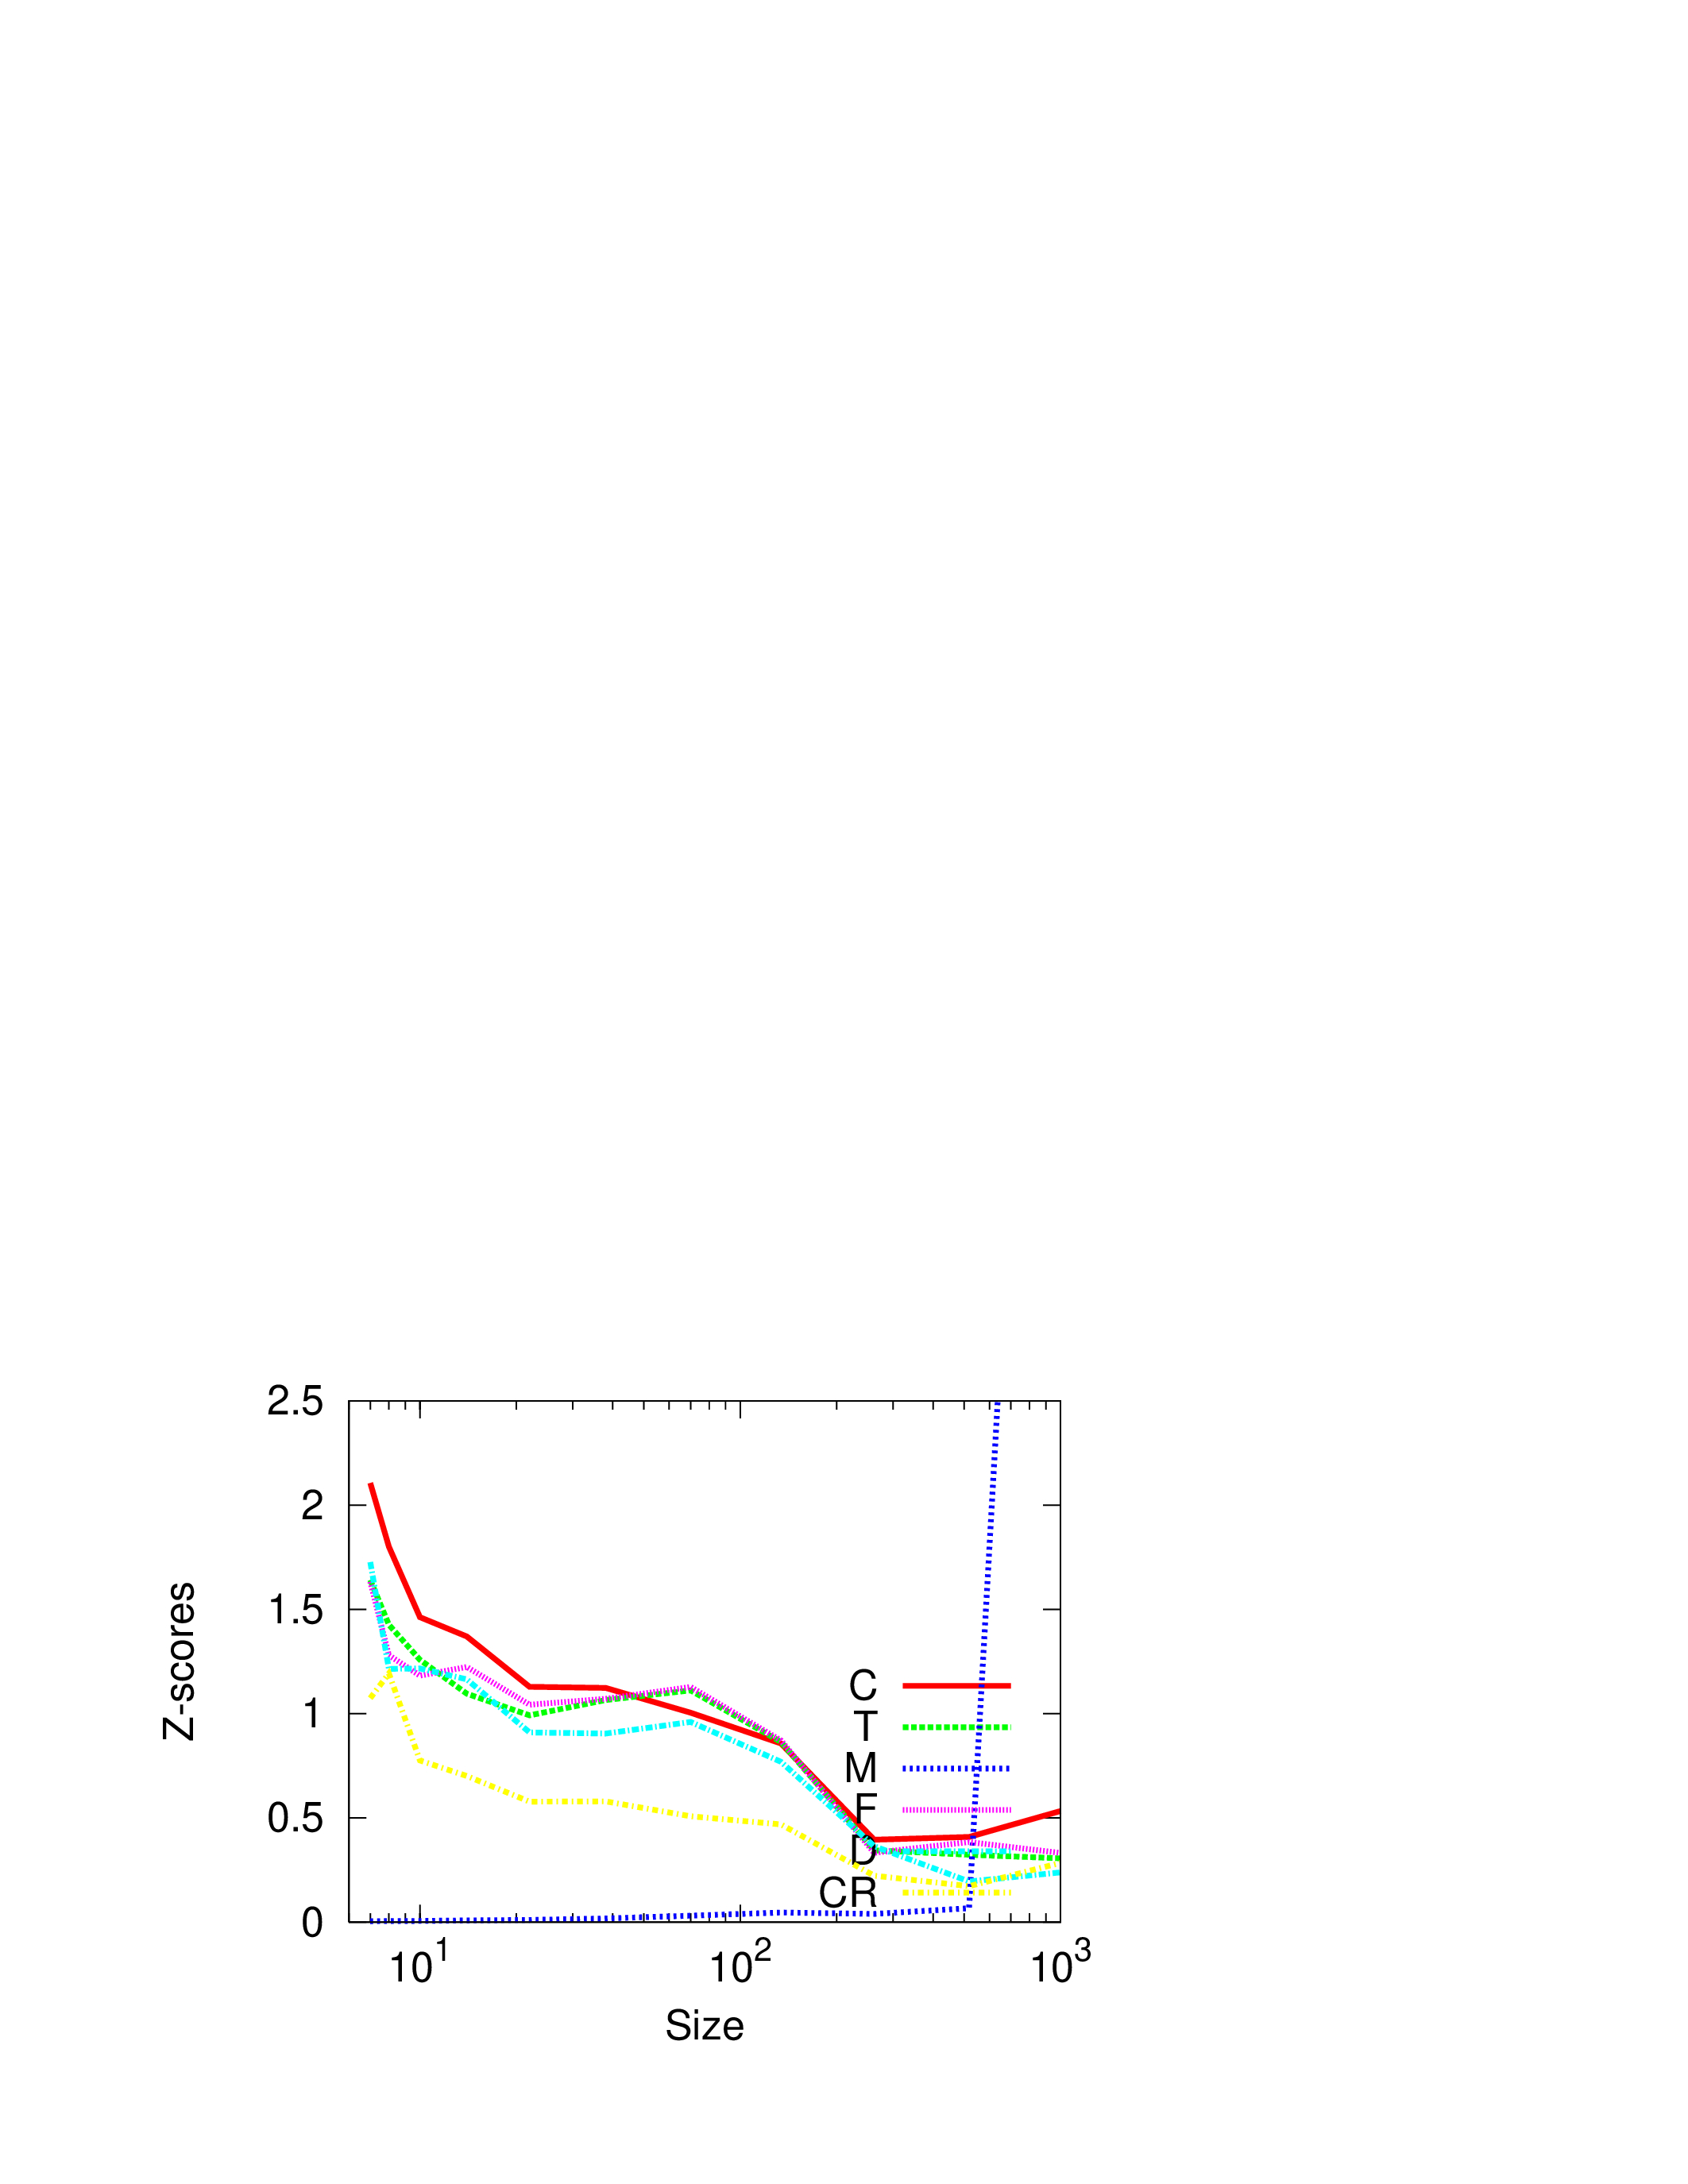}}
	\subfigure[NodeSwap	(DBLP)]{\includegraphics[width=0.16\textwidth]{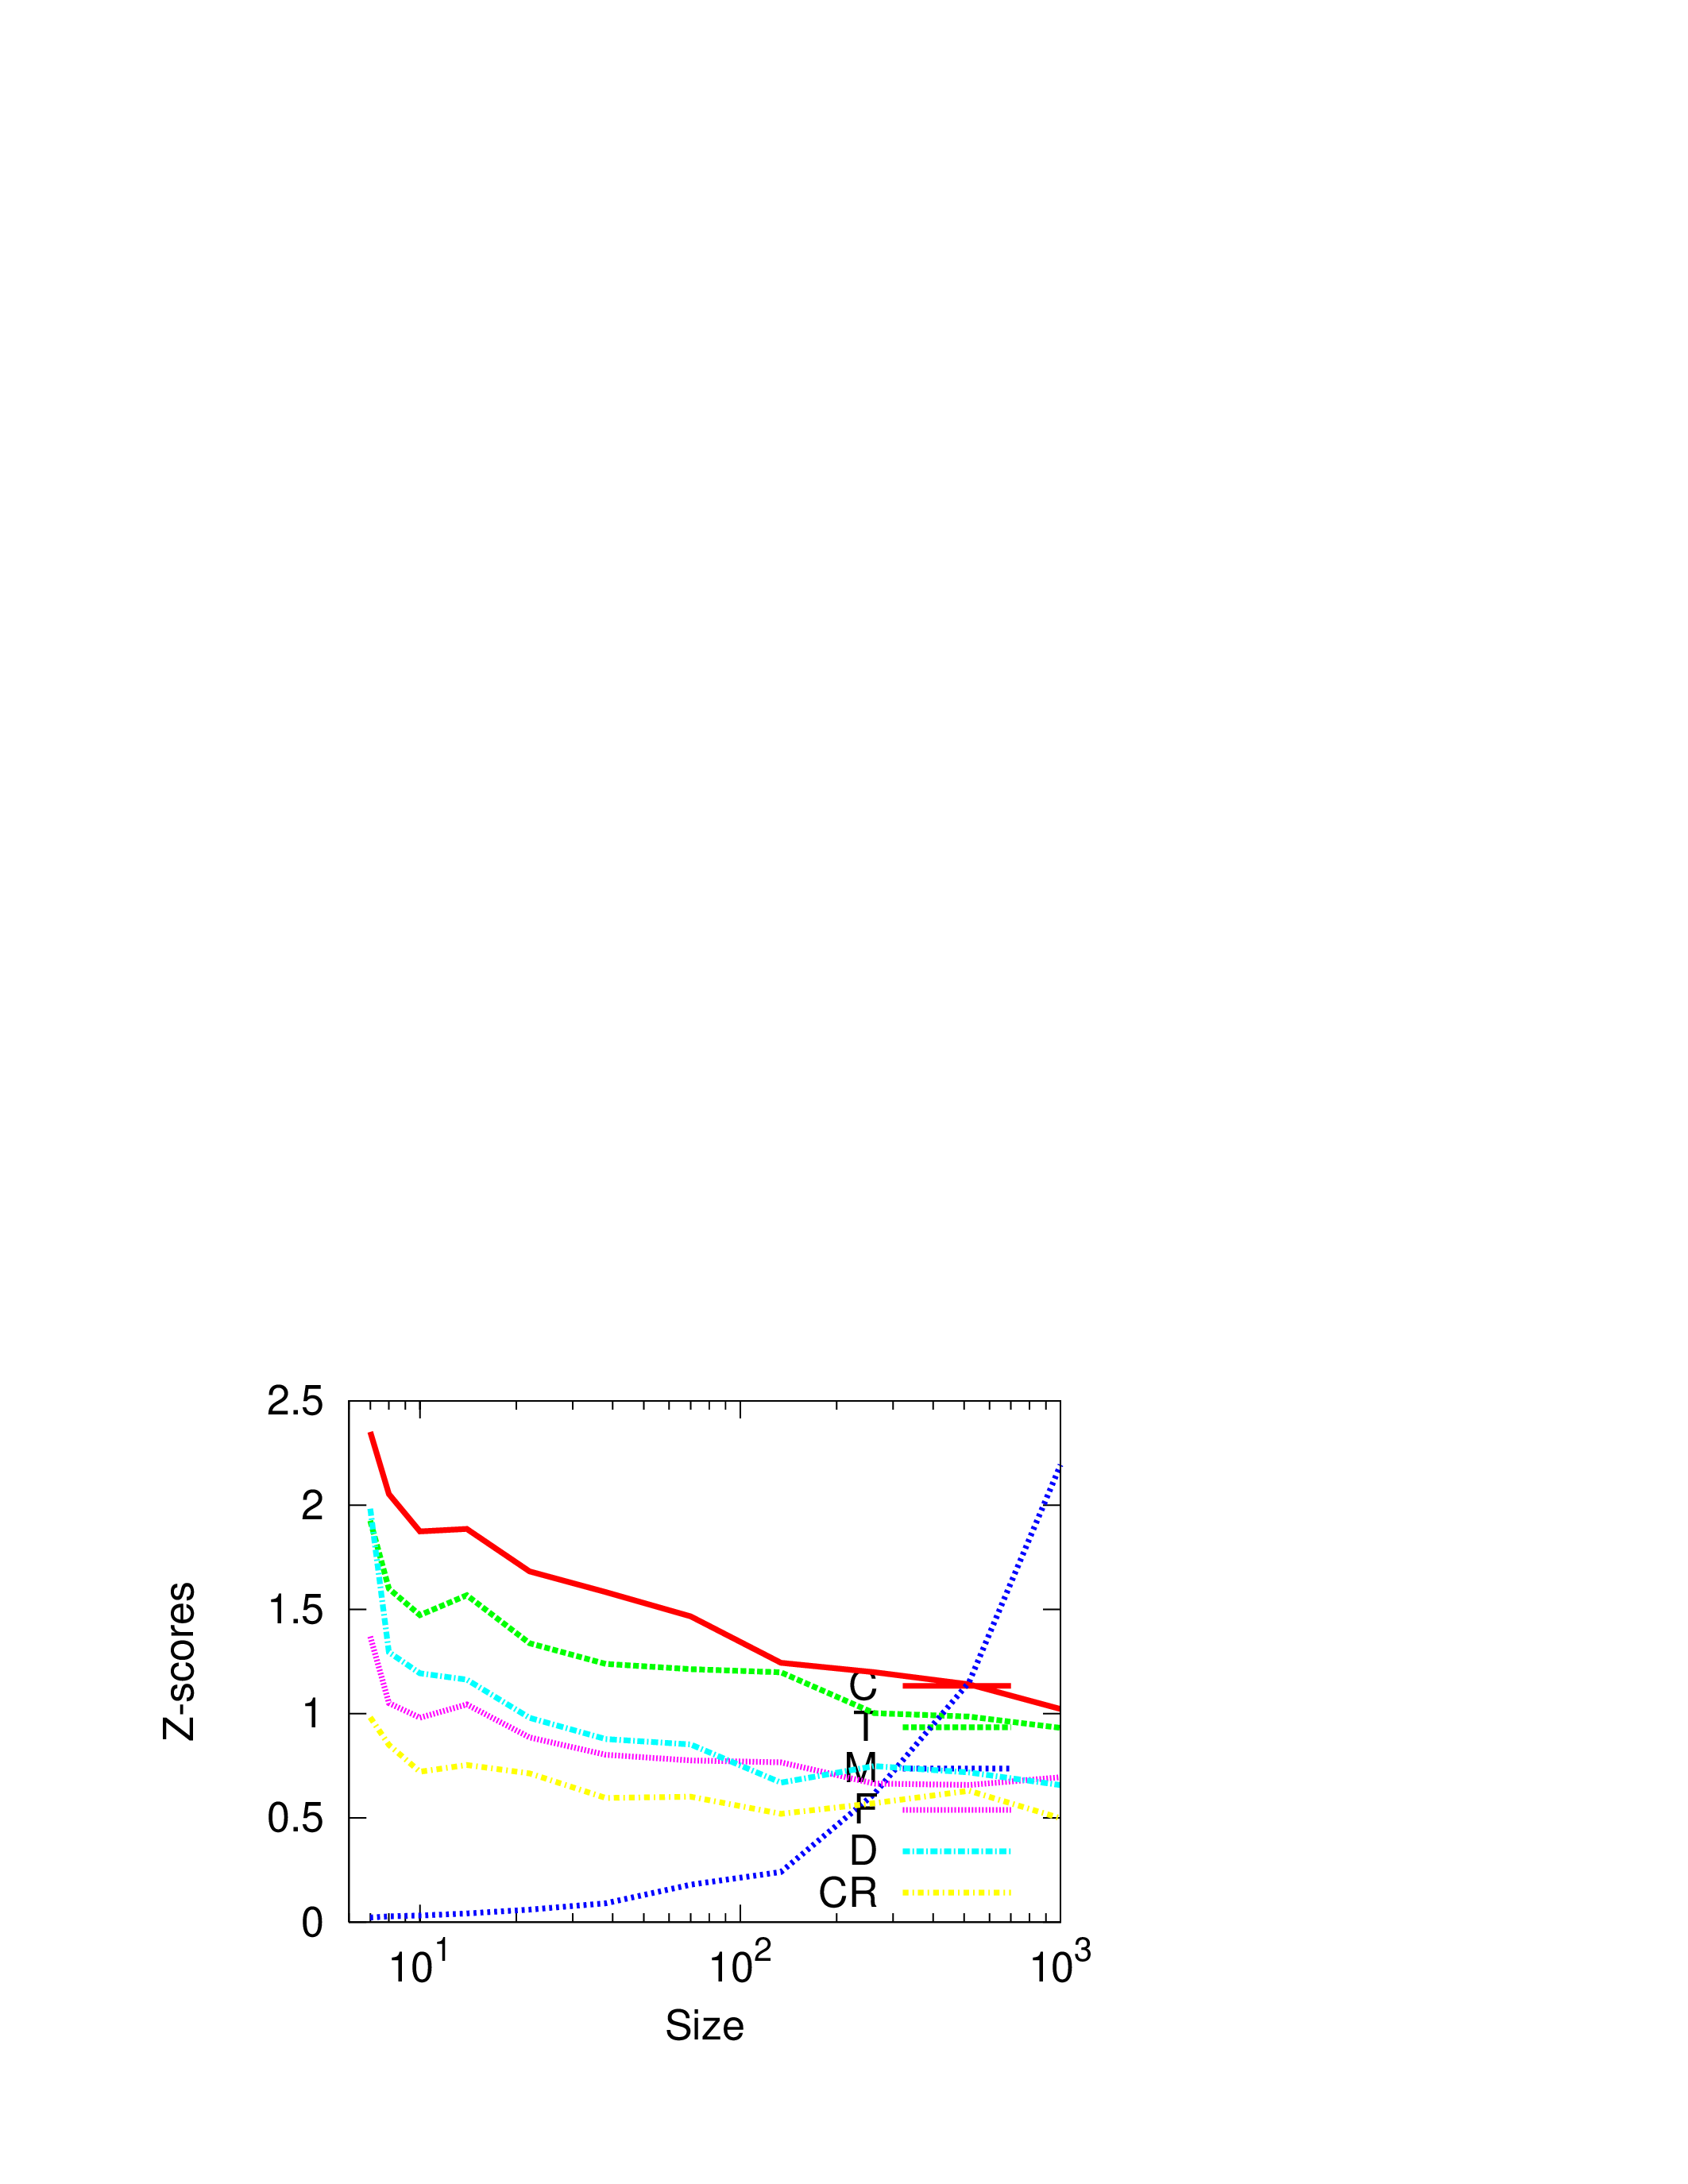}}
	\subfigure[Random	(LJ)]{\includegraphics[width=0.16\textwidth]{zscore.sz.Random.lj.eps}}
	\subfigure[Random	(FS)]{\includegraphics[width=0.16\textwidth]{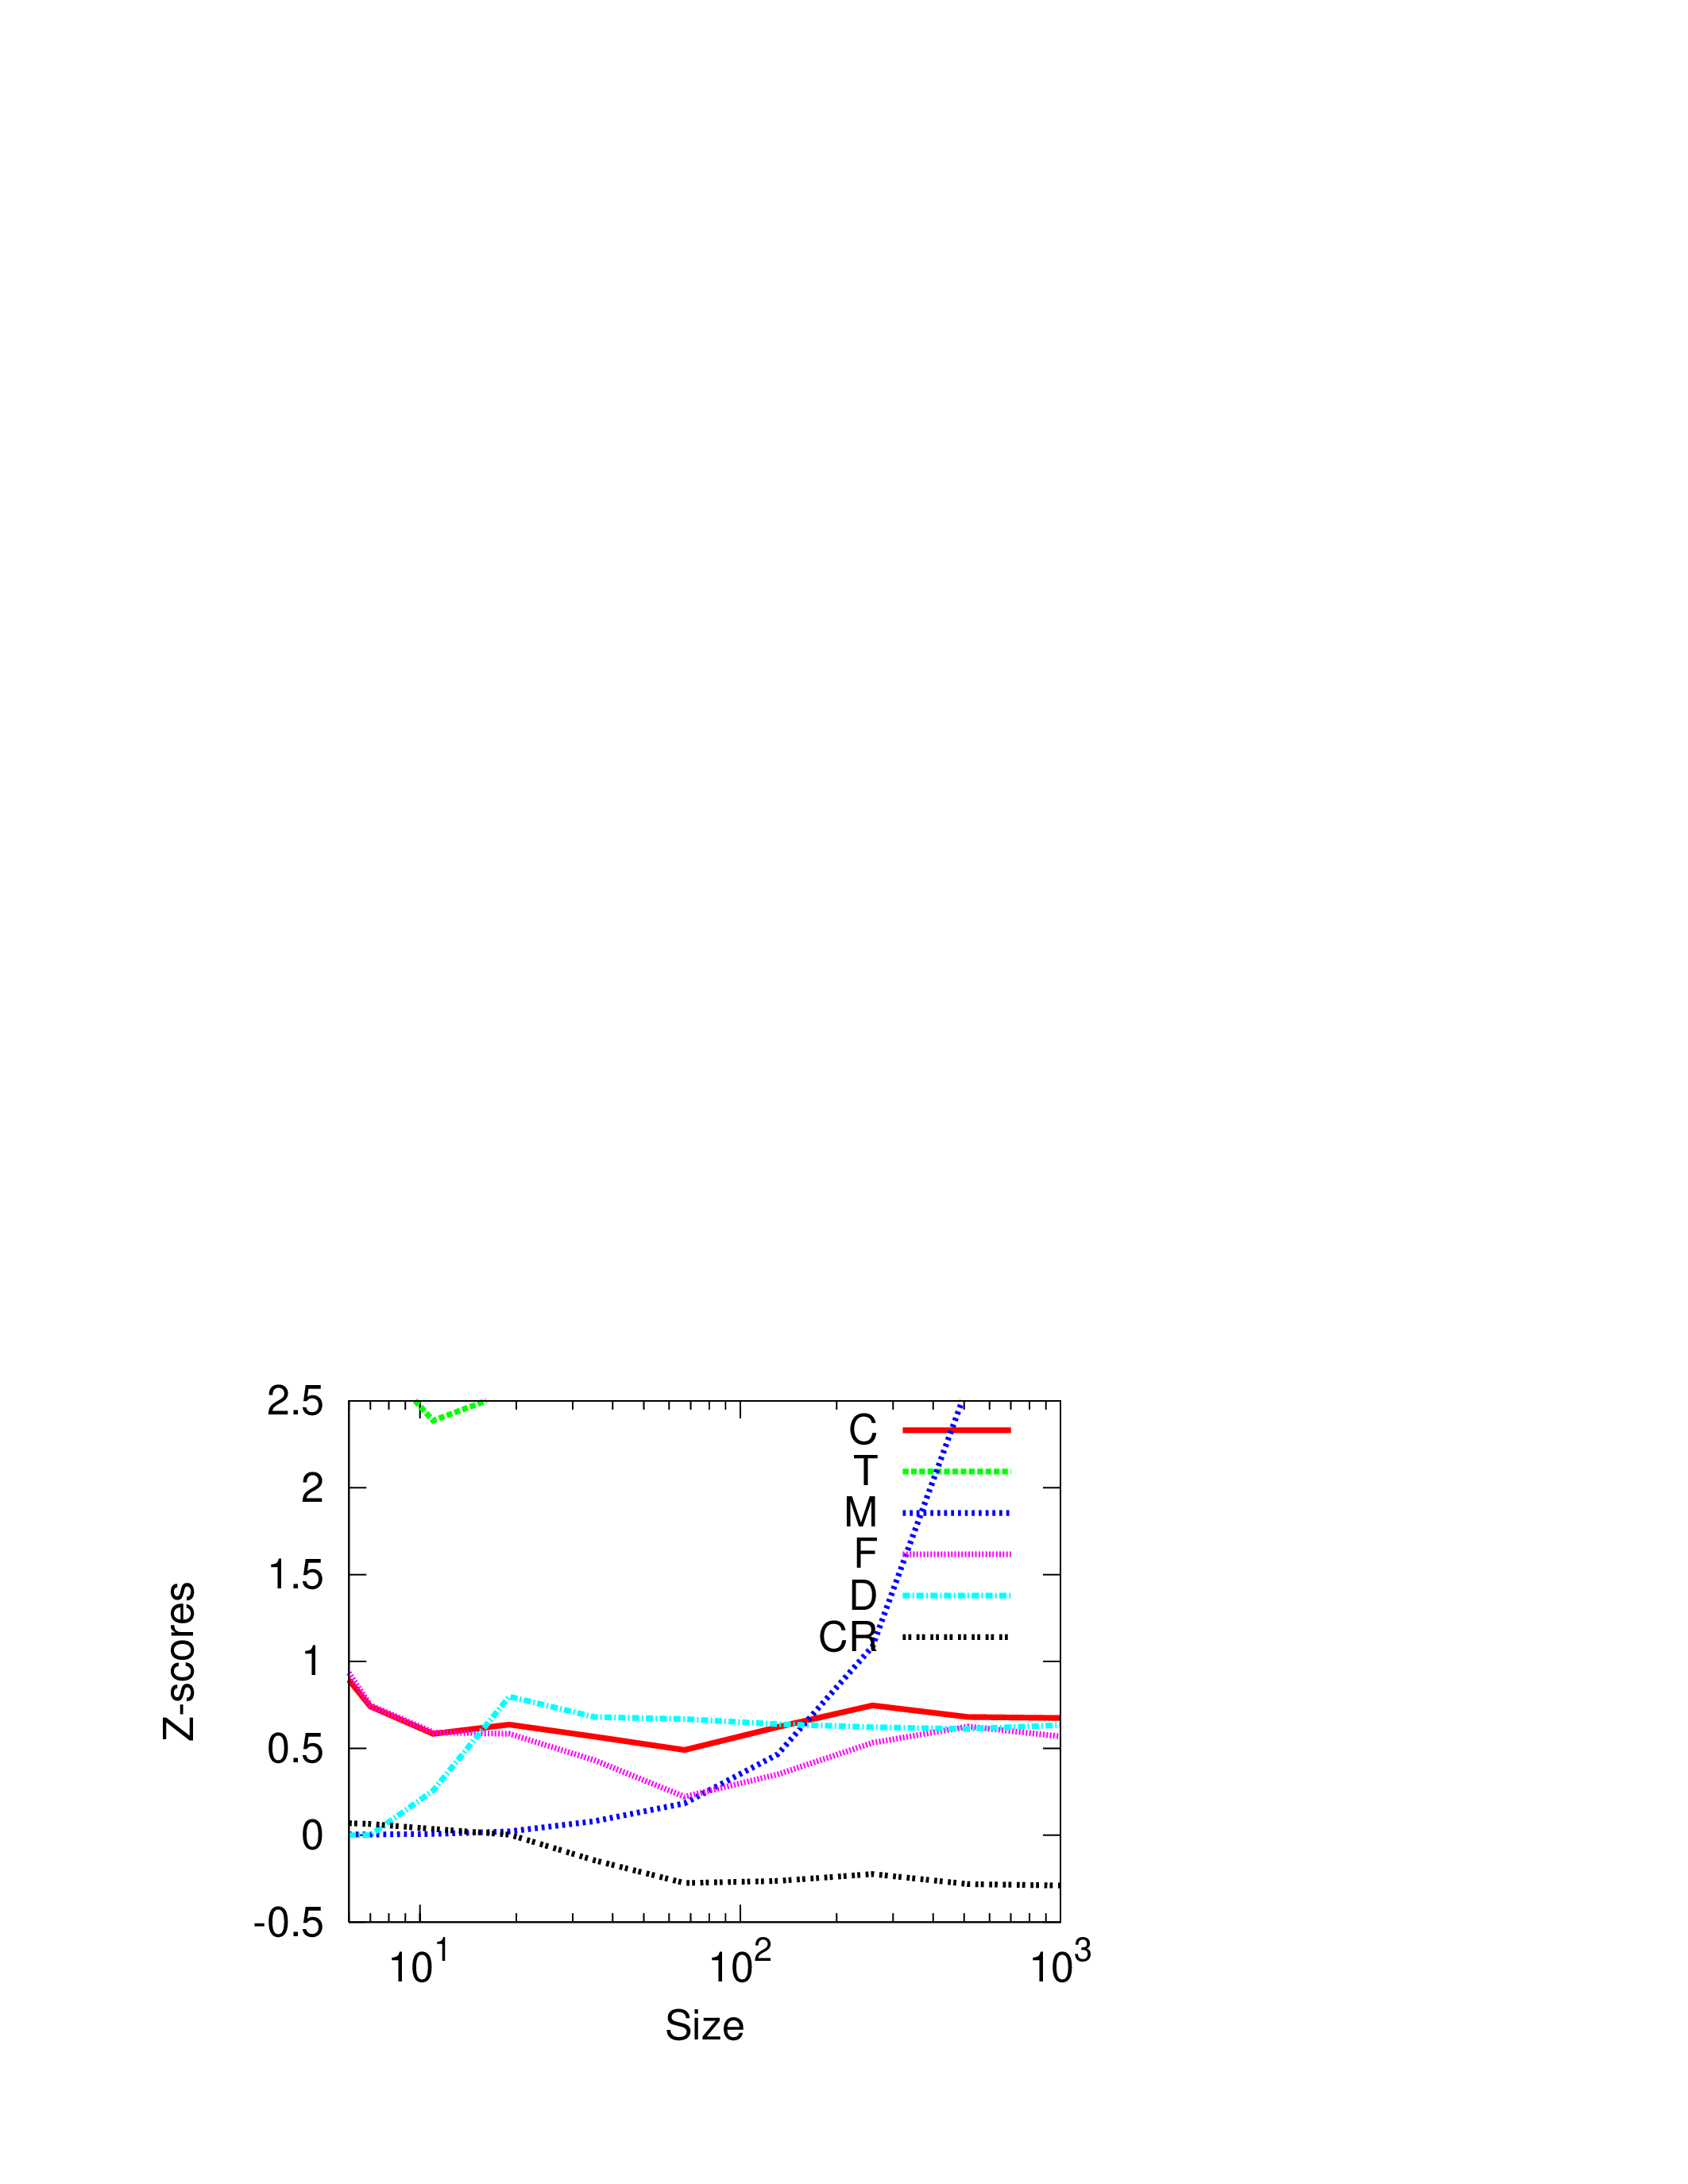}}
	\subfigure[Random	(Orkut)]{\includegraphics[width=0.16\textwidth]{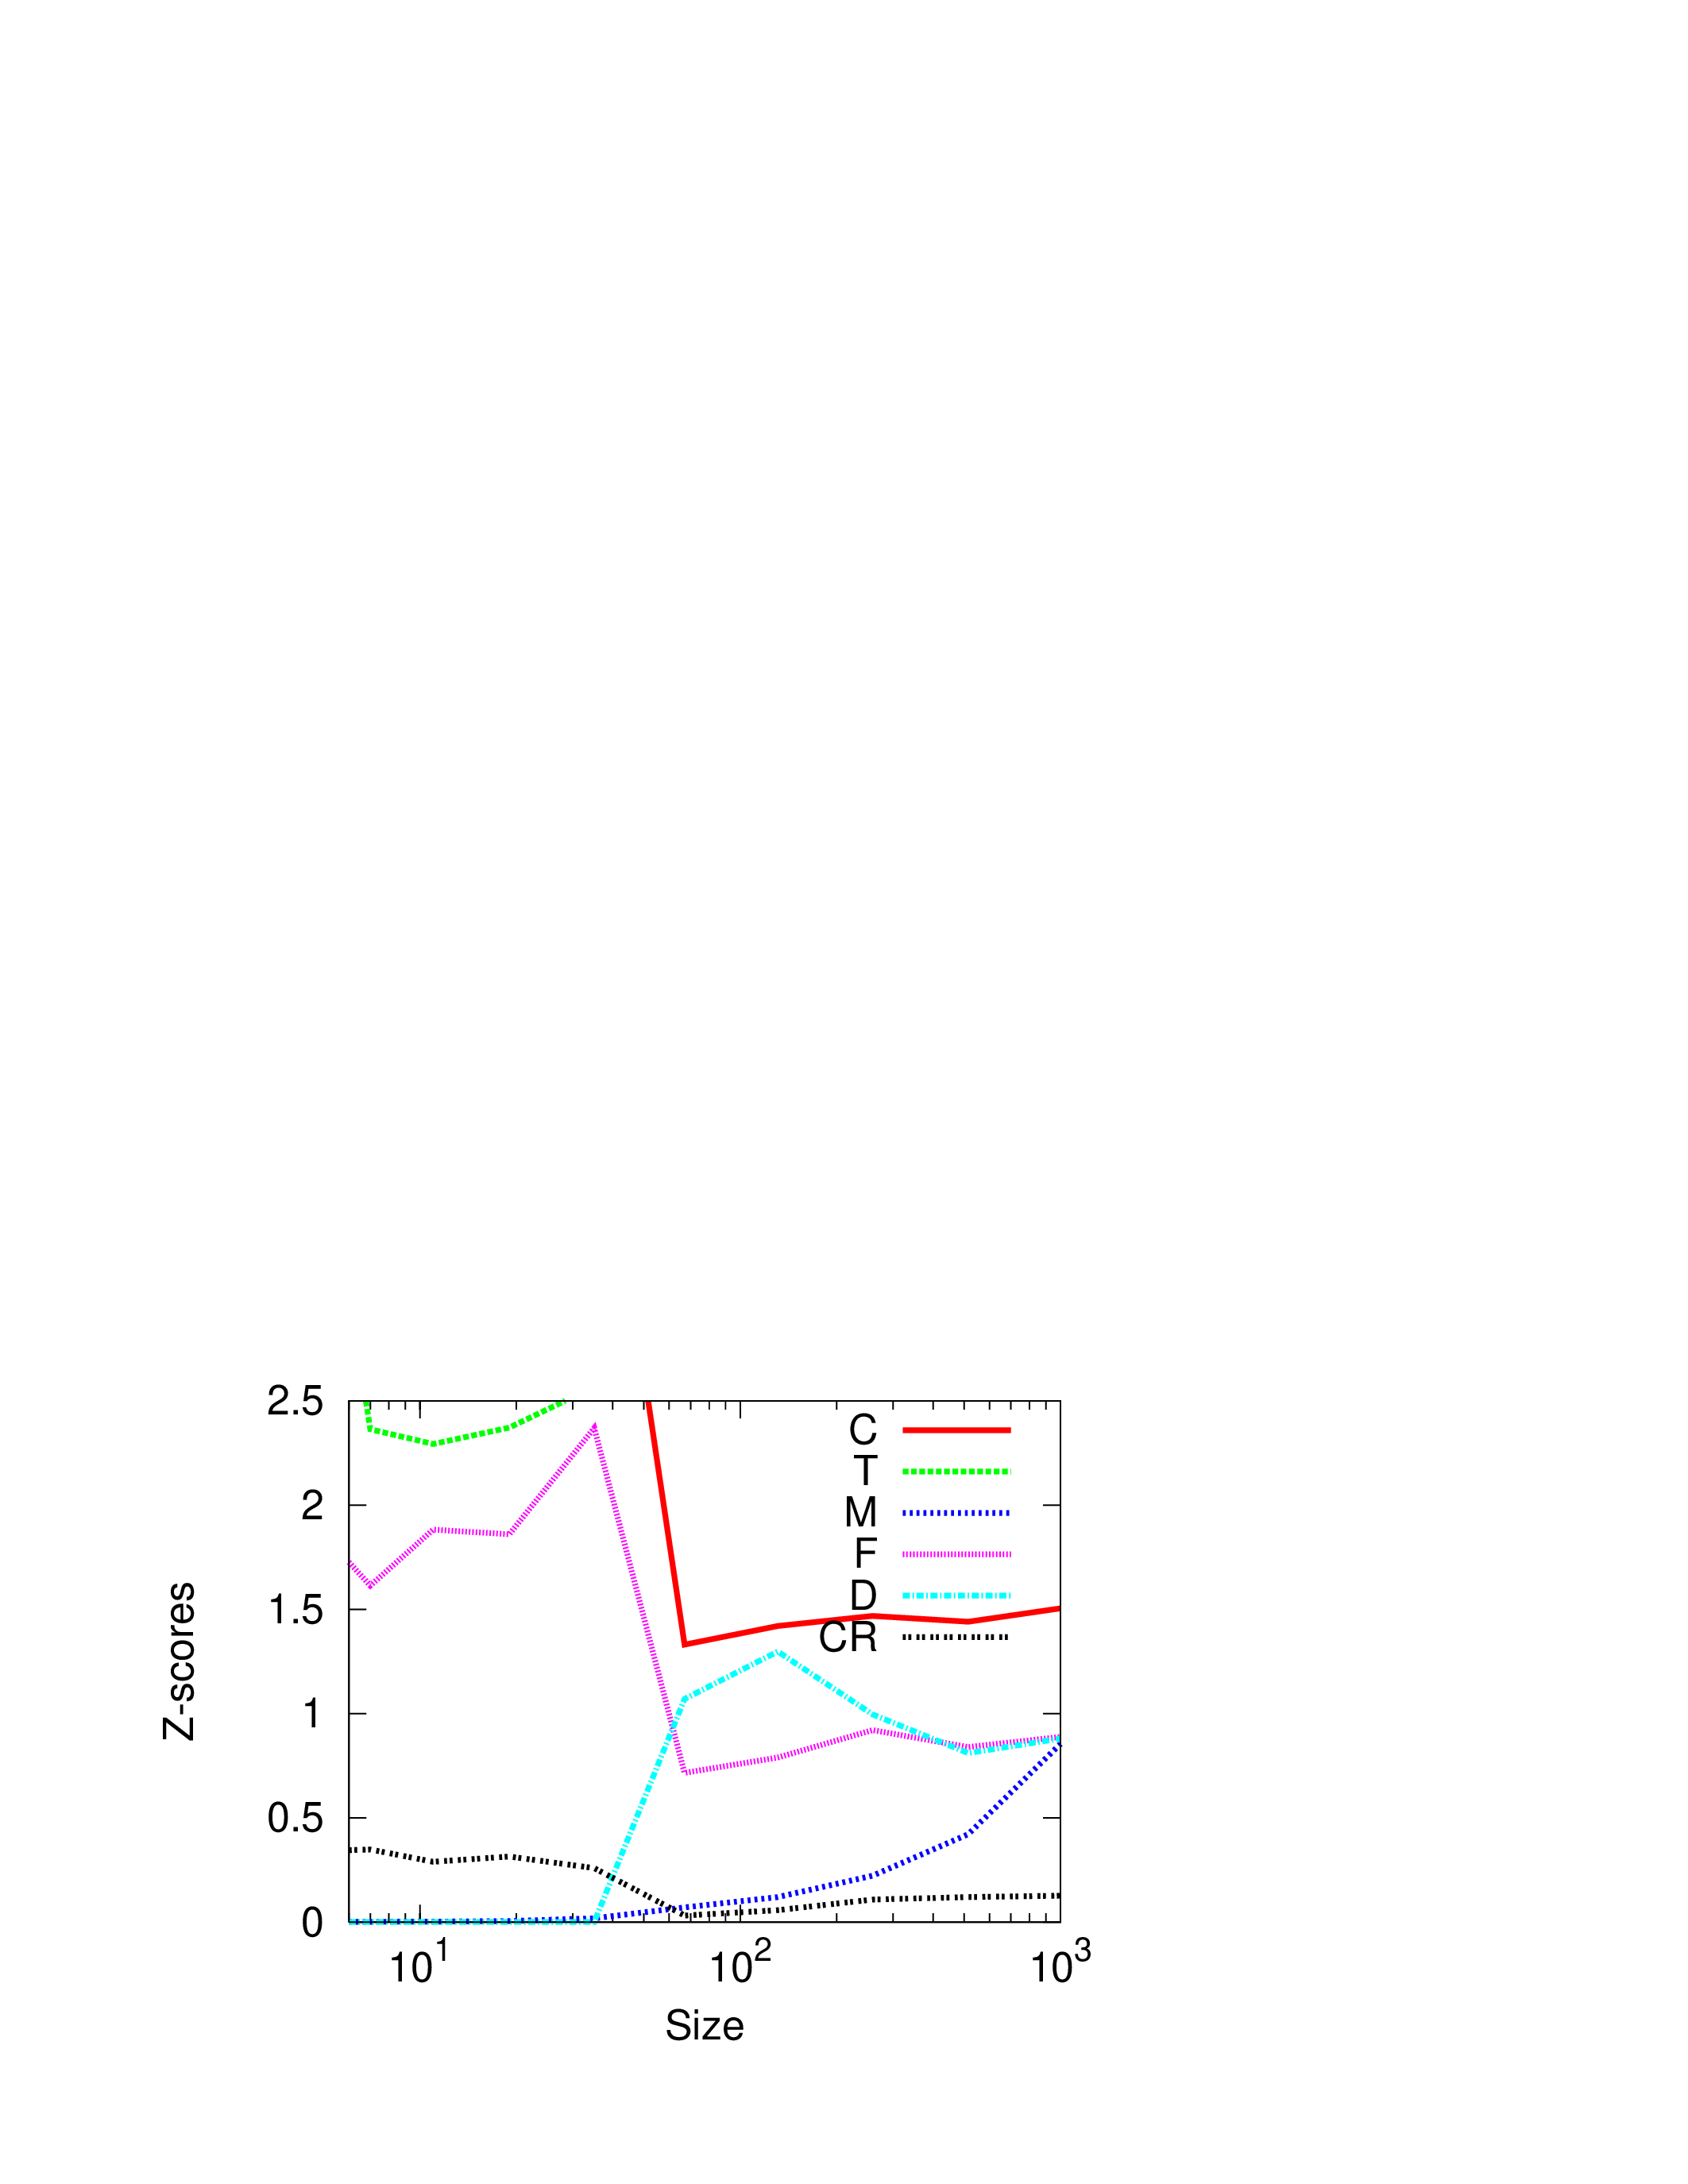}}
	\subfigure[Random	(Ning)]{\includegraphics[width=0.16\textwidth]{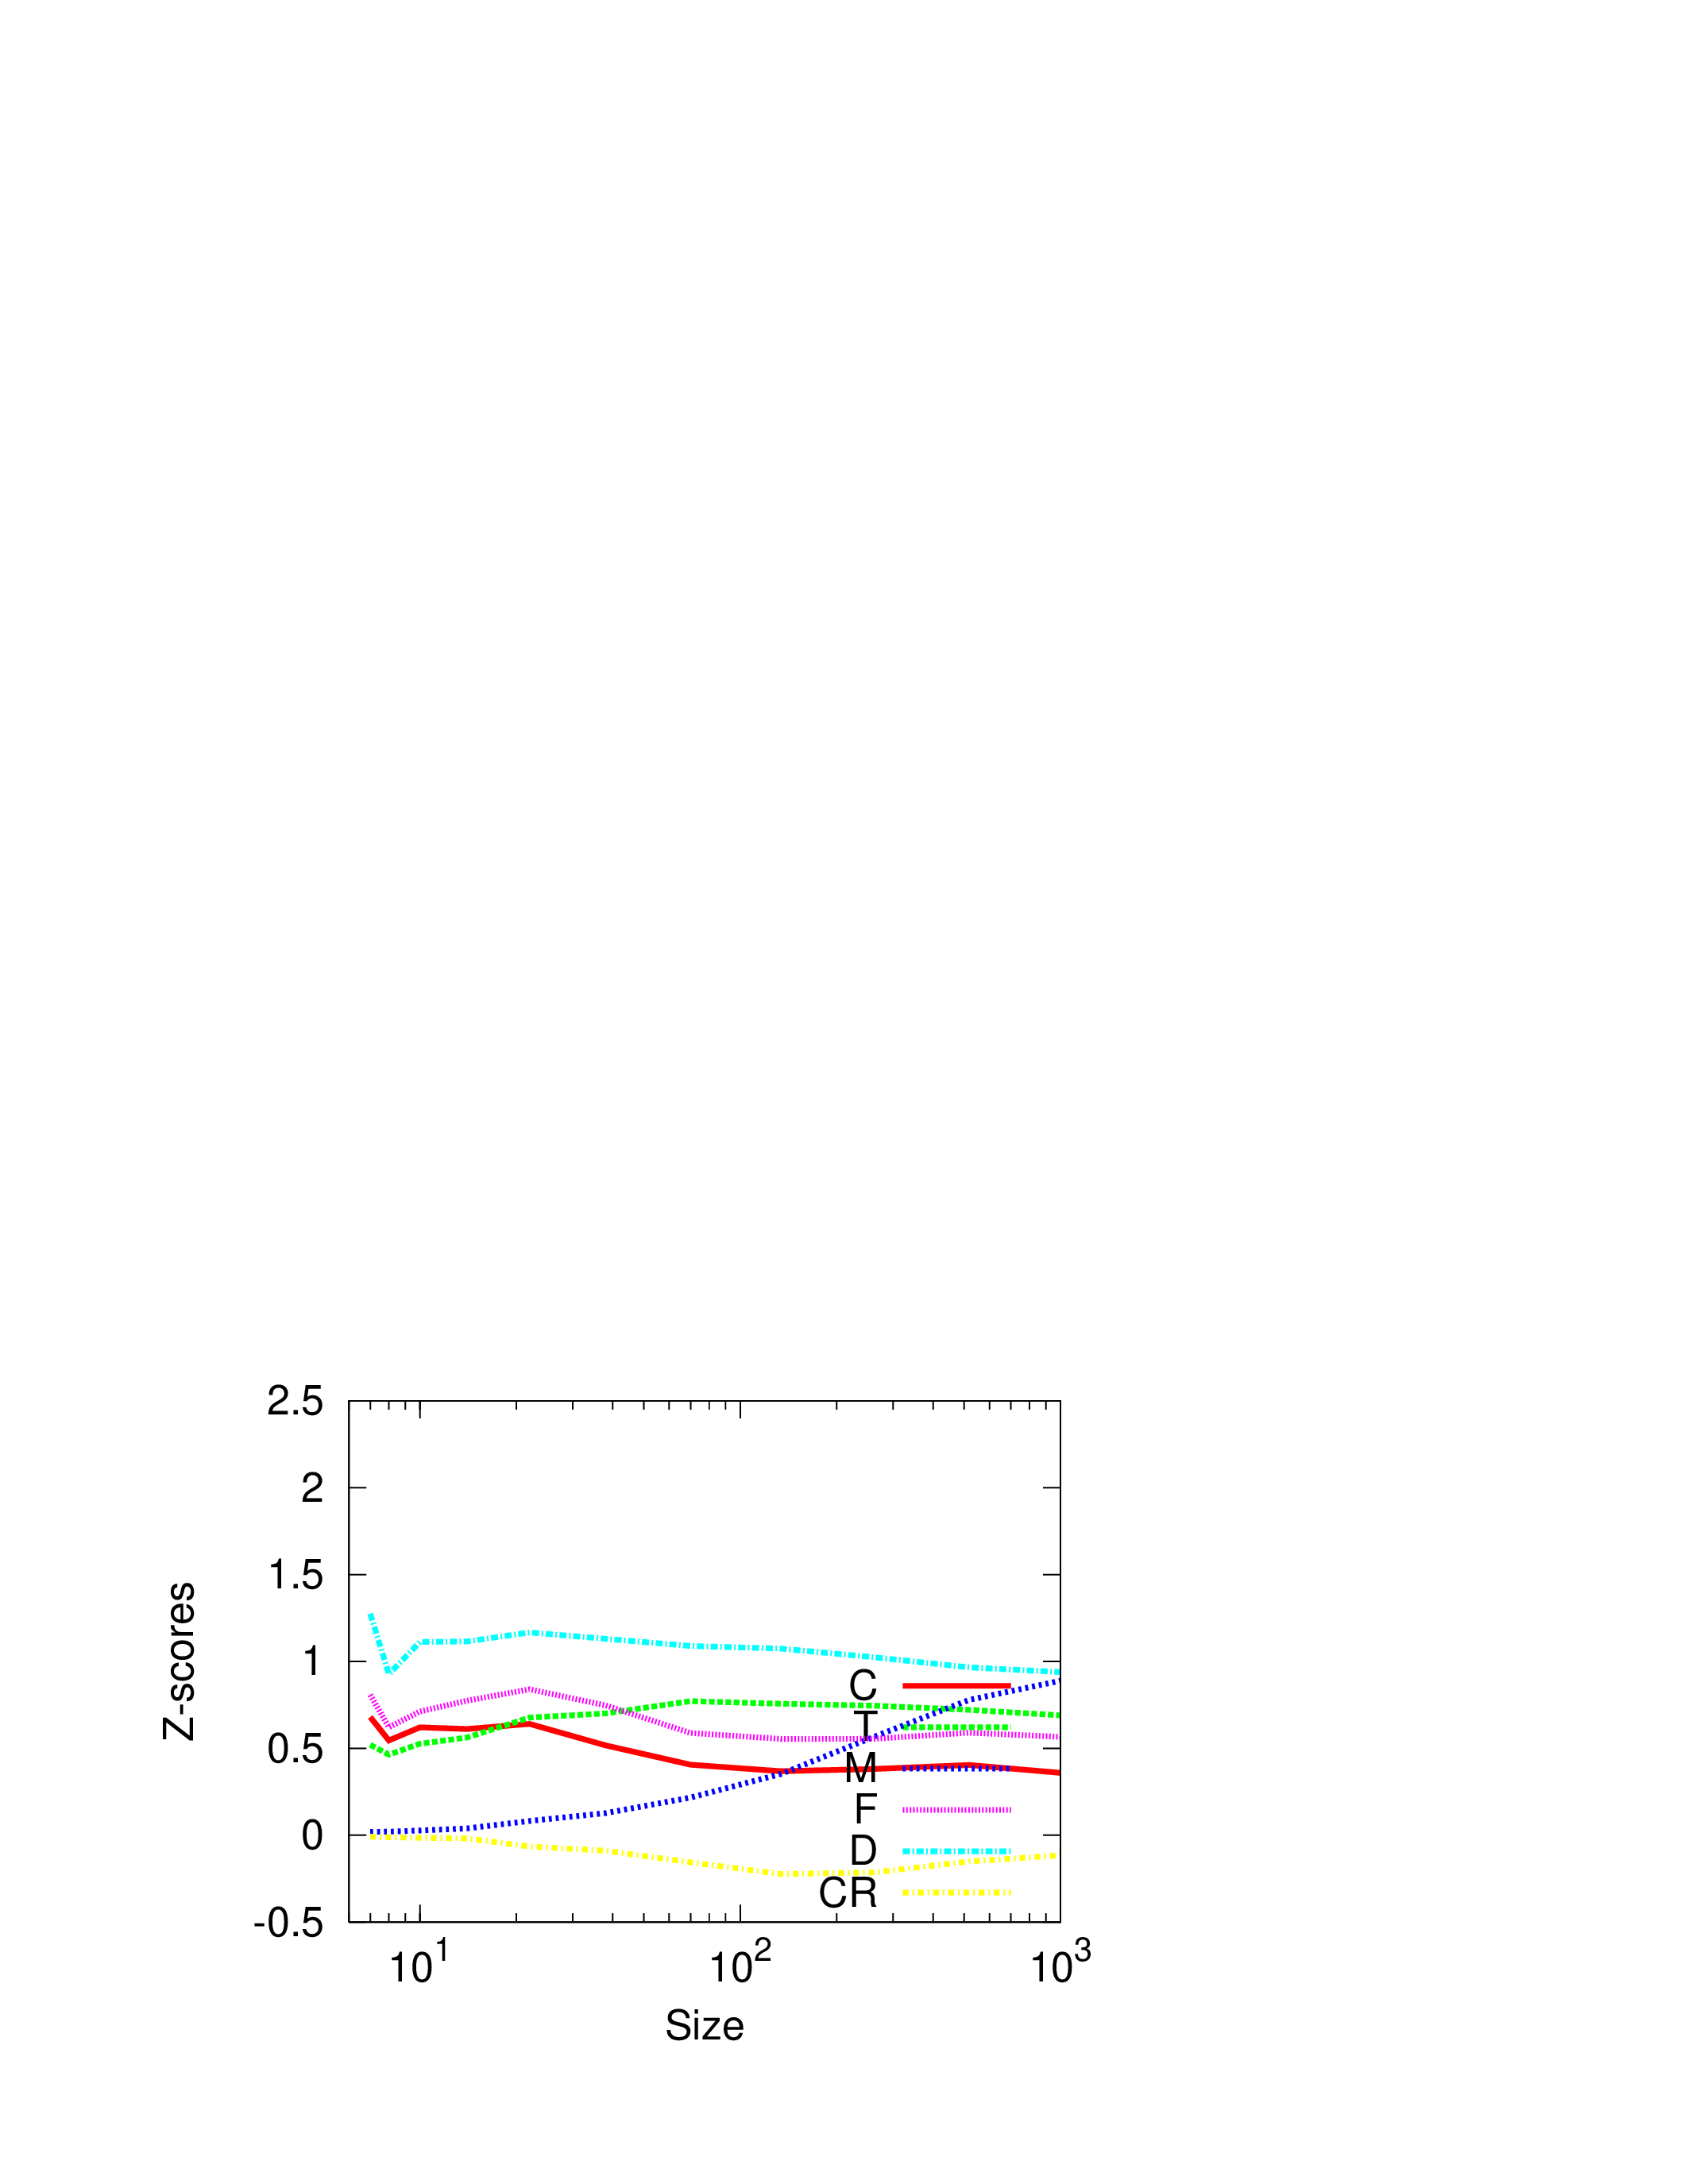}}
	\subfigure[Random	(Amazon)]{\includegraphics[width=0.16\textwidth]{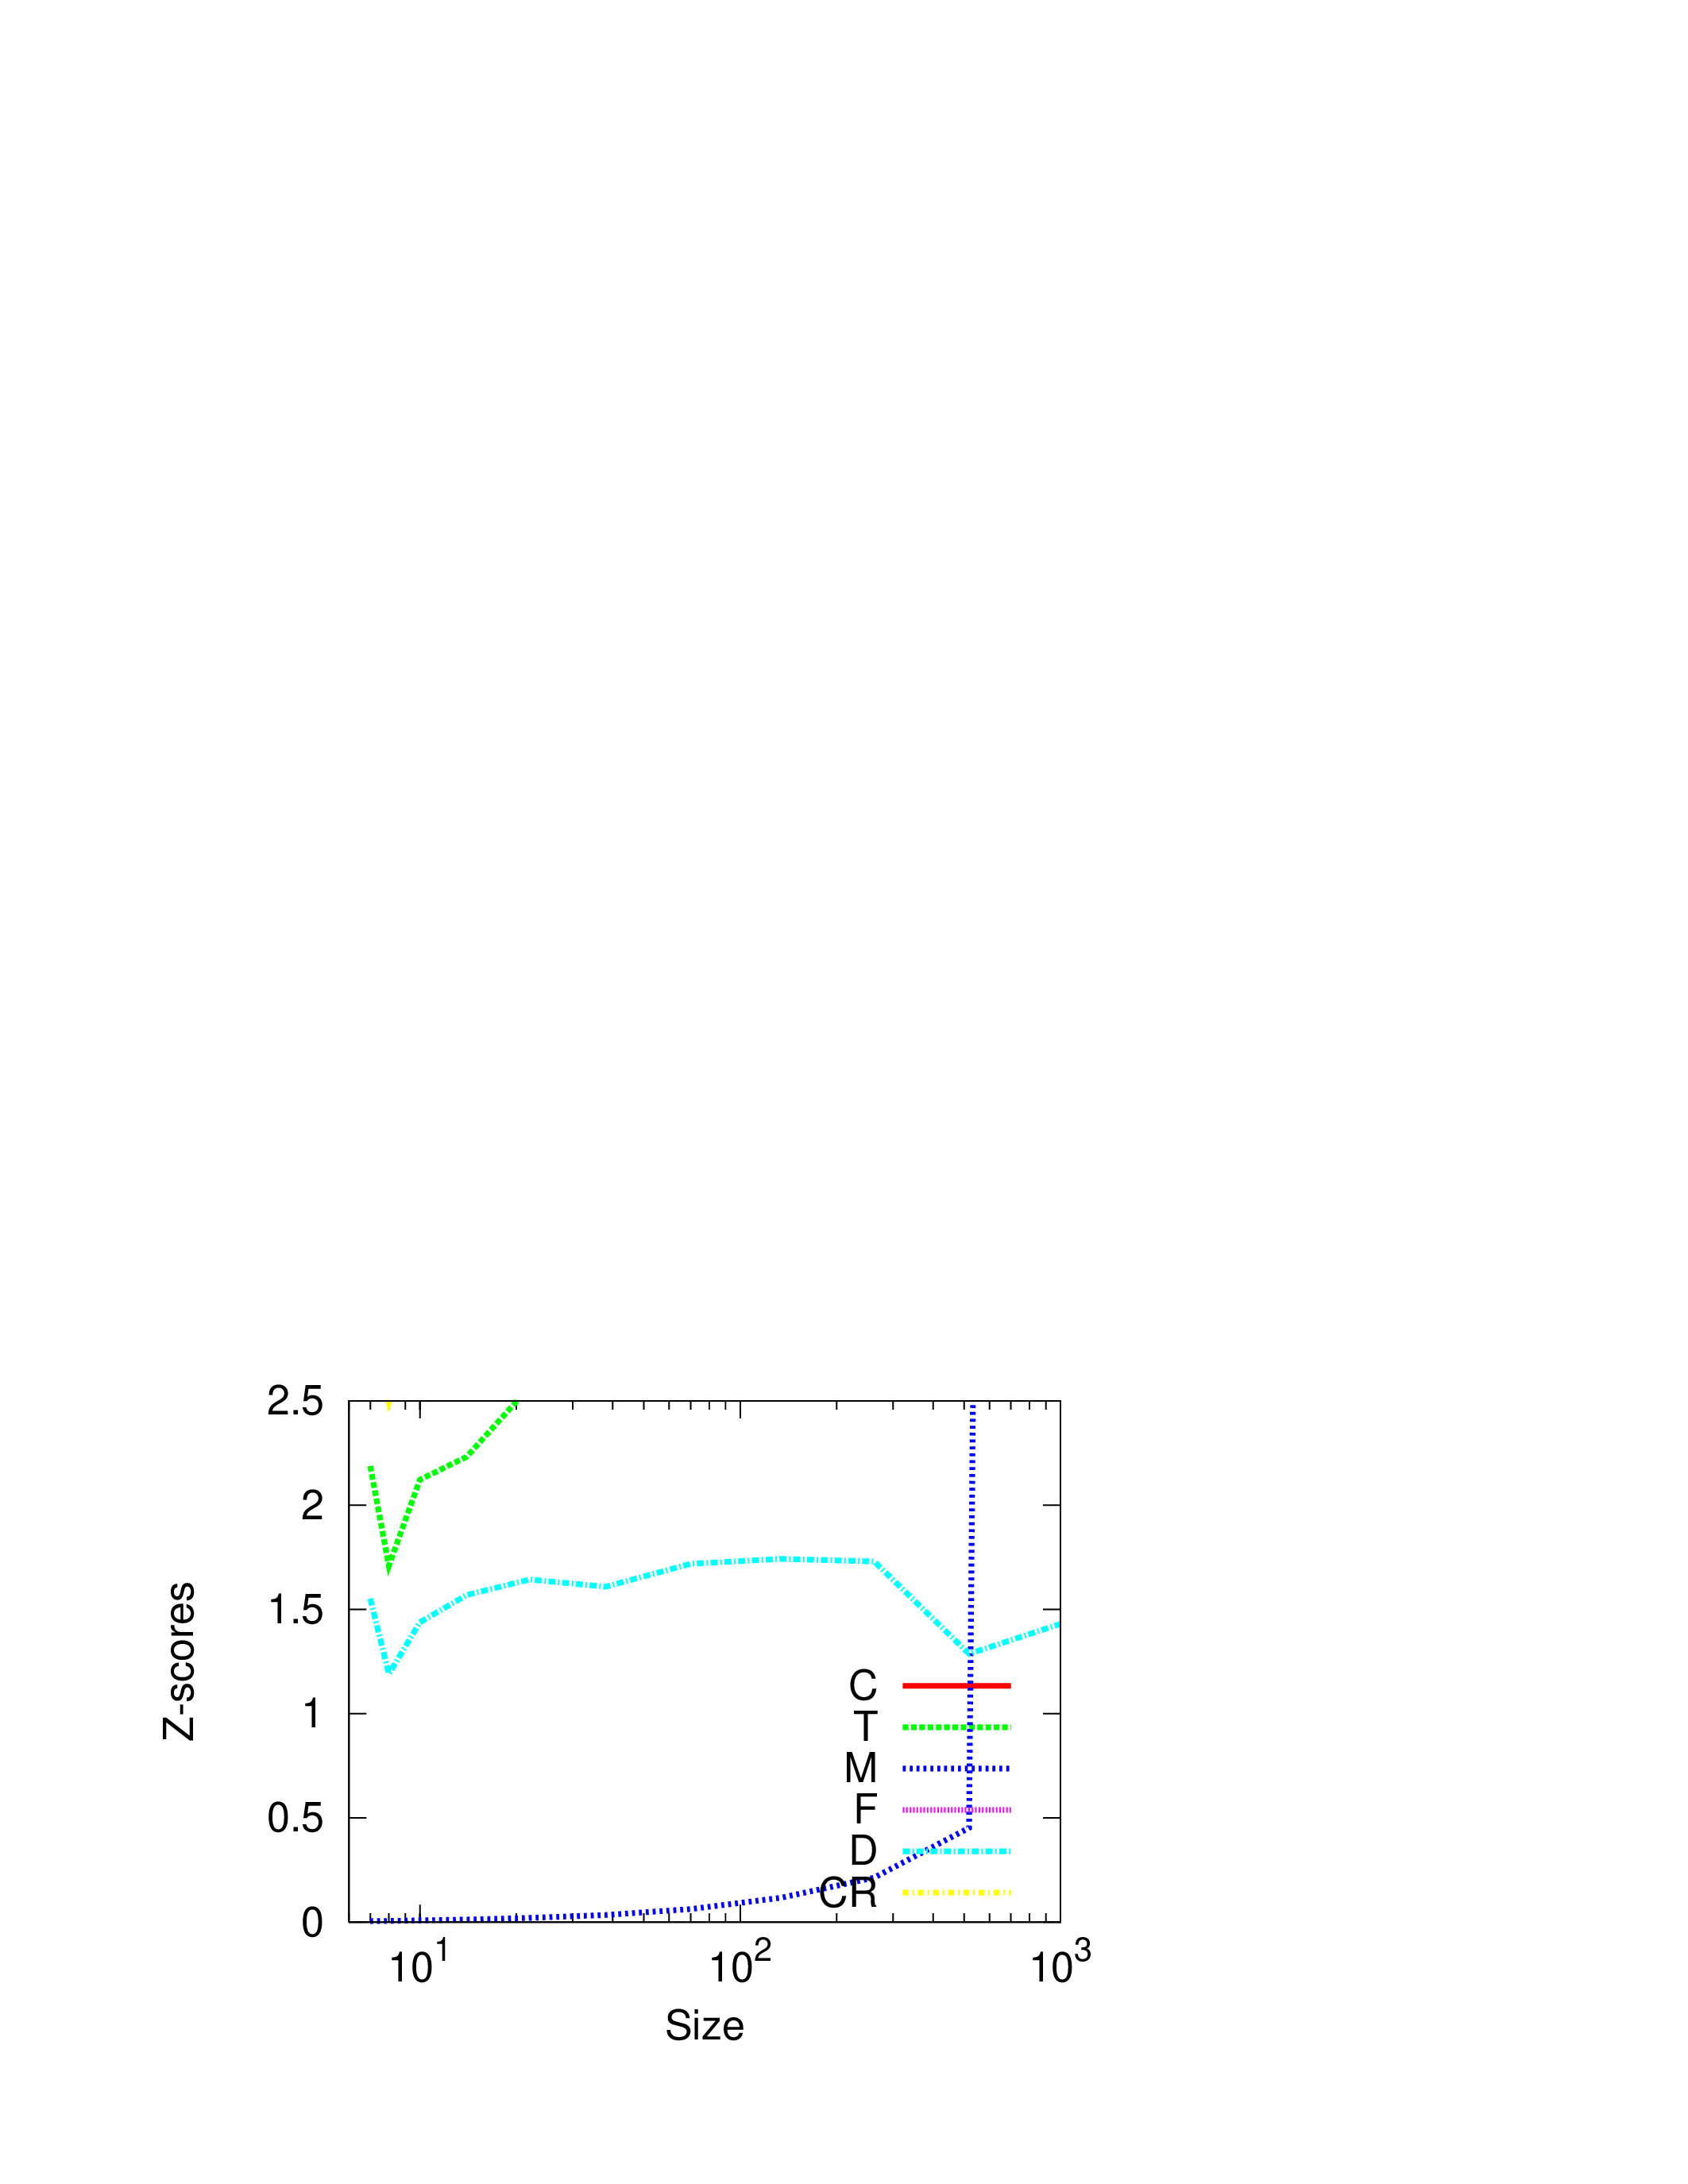}}
	\subfigure[Random	(DBLP)]{\includegraphics[width=0.16\textwidth]{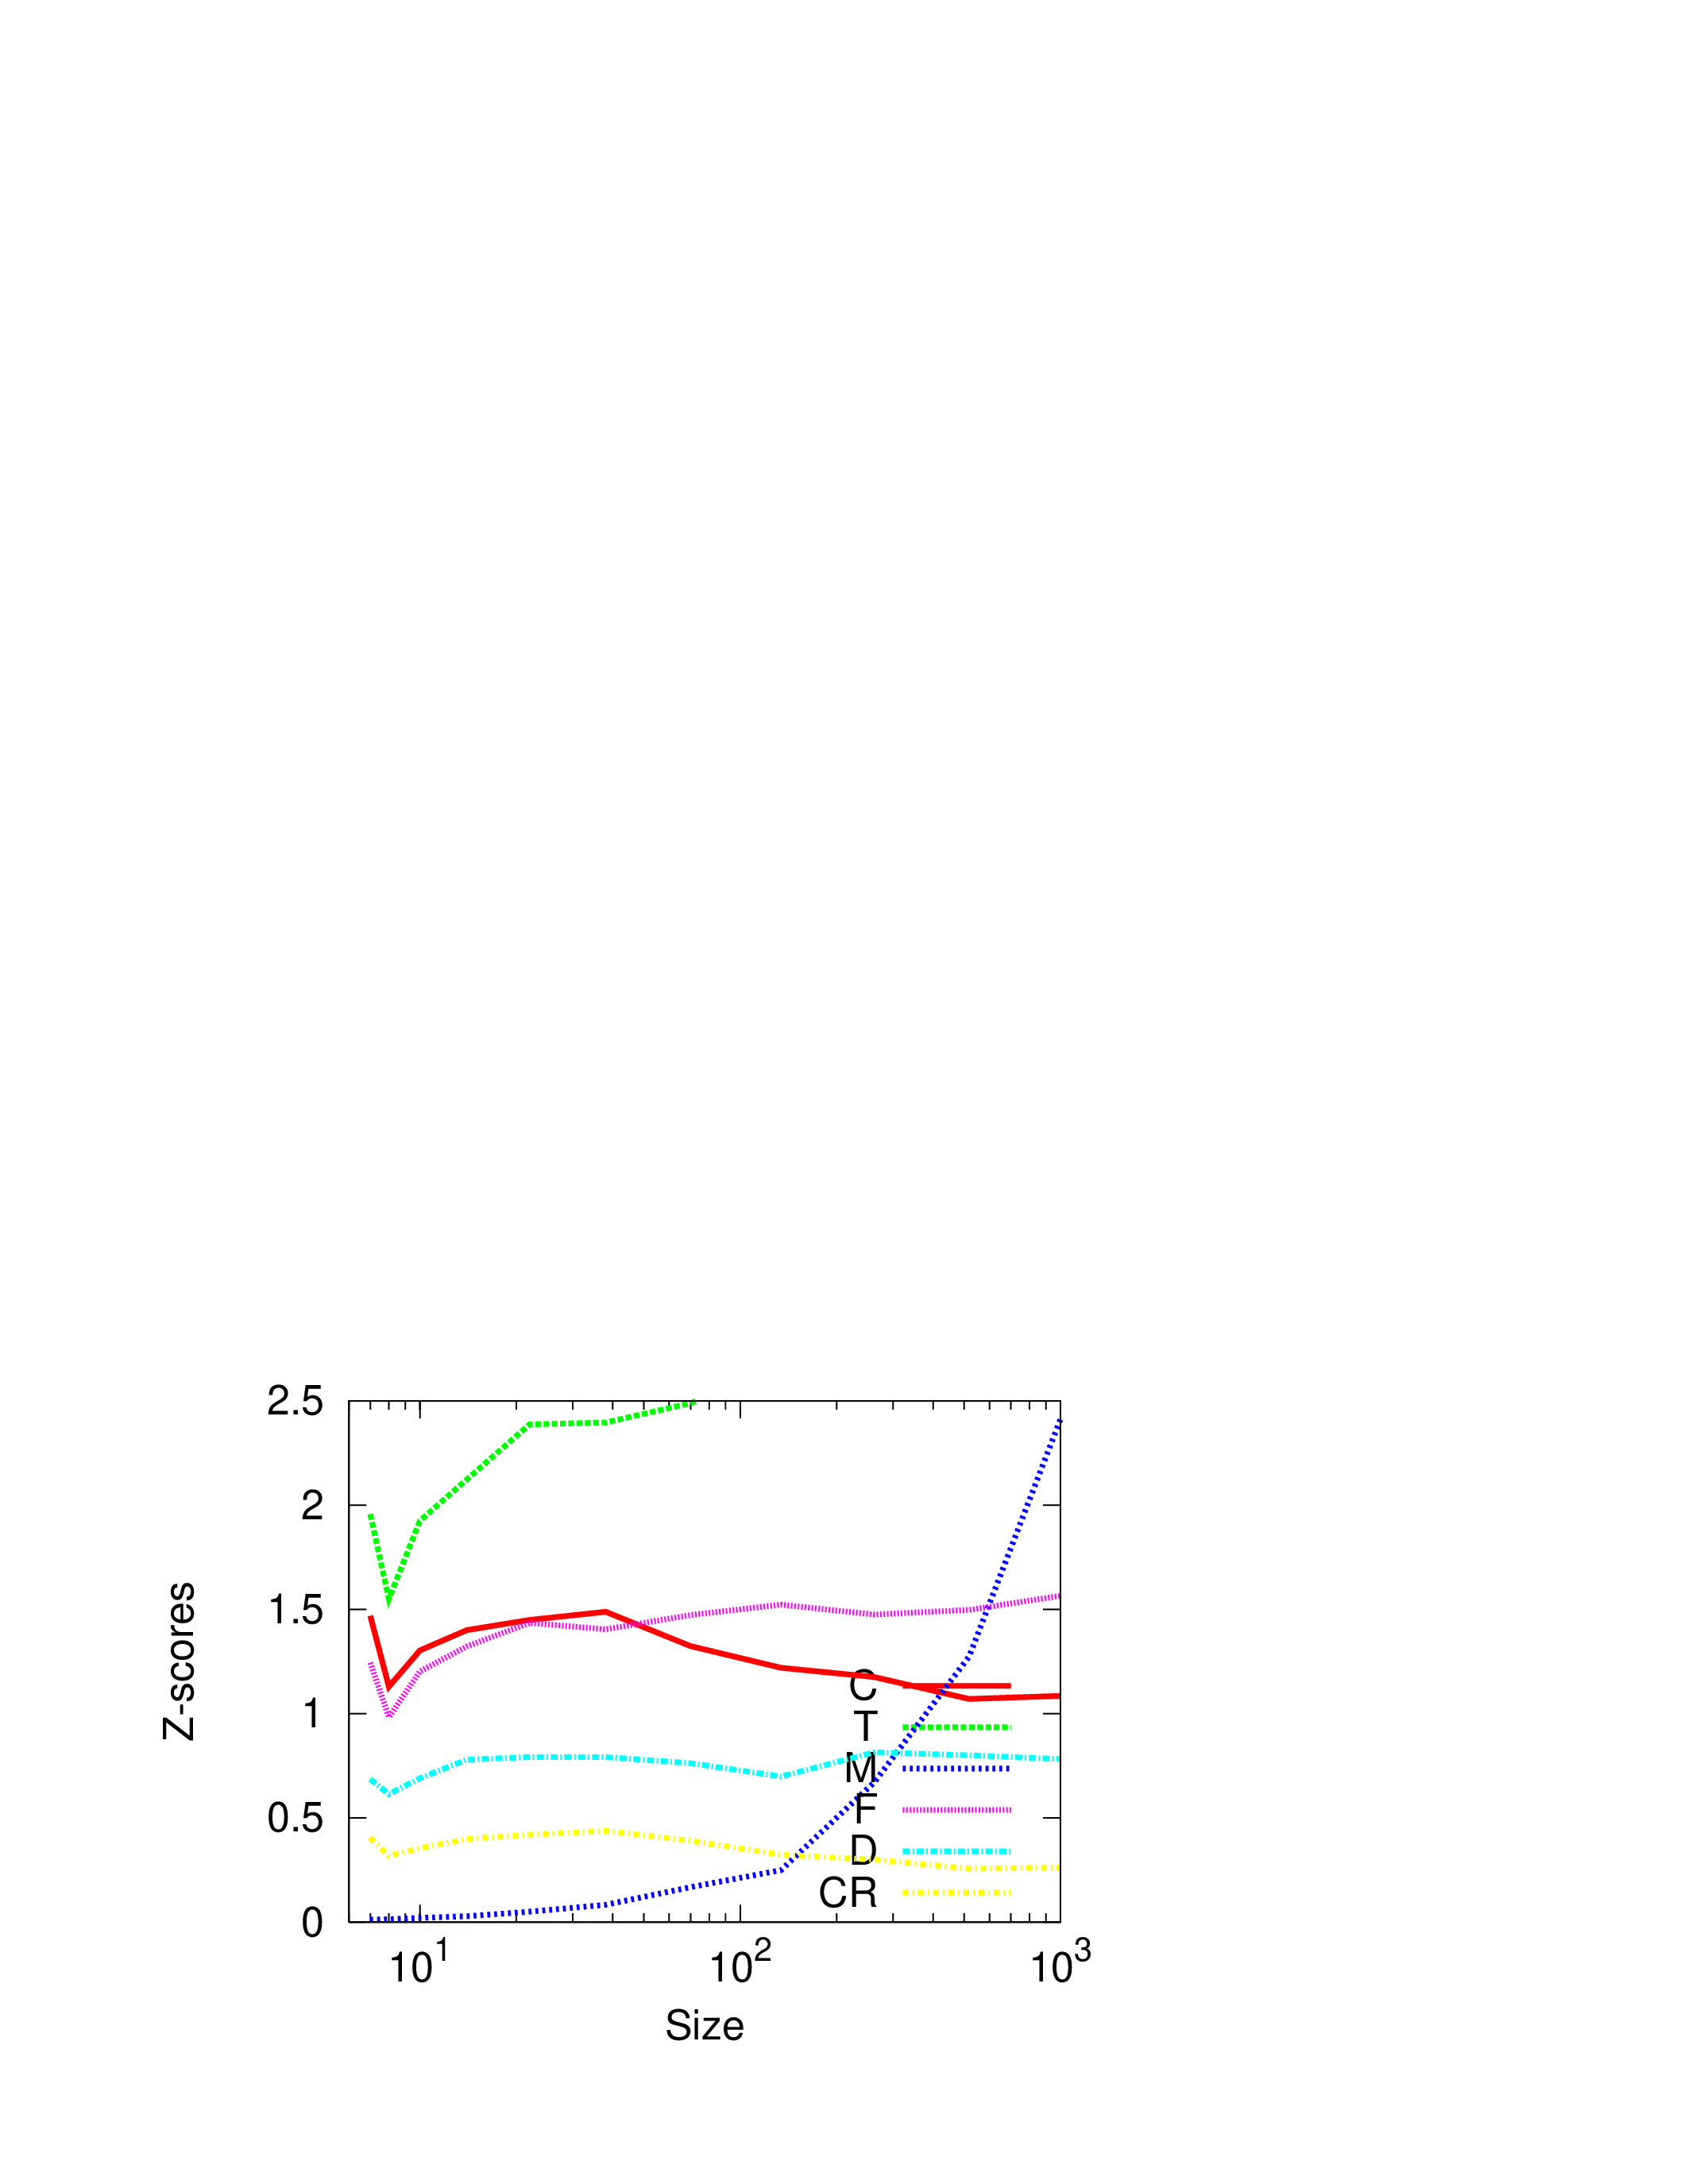}}
	\subfigure[Expand	(LJ)]{\includegraphics[width=0.16\textwidth]{zscore.sz.Expand.lj.eps}}
	\subfigure[Expand	(FS)]{\includegraphics[width=0.16\textwidth]{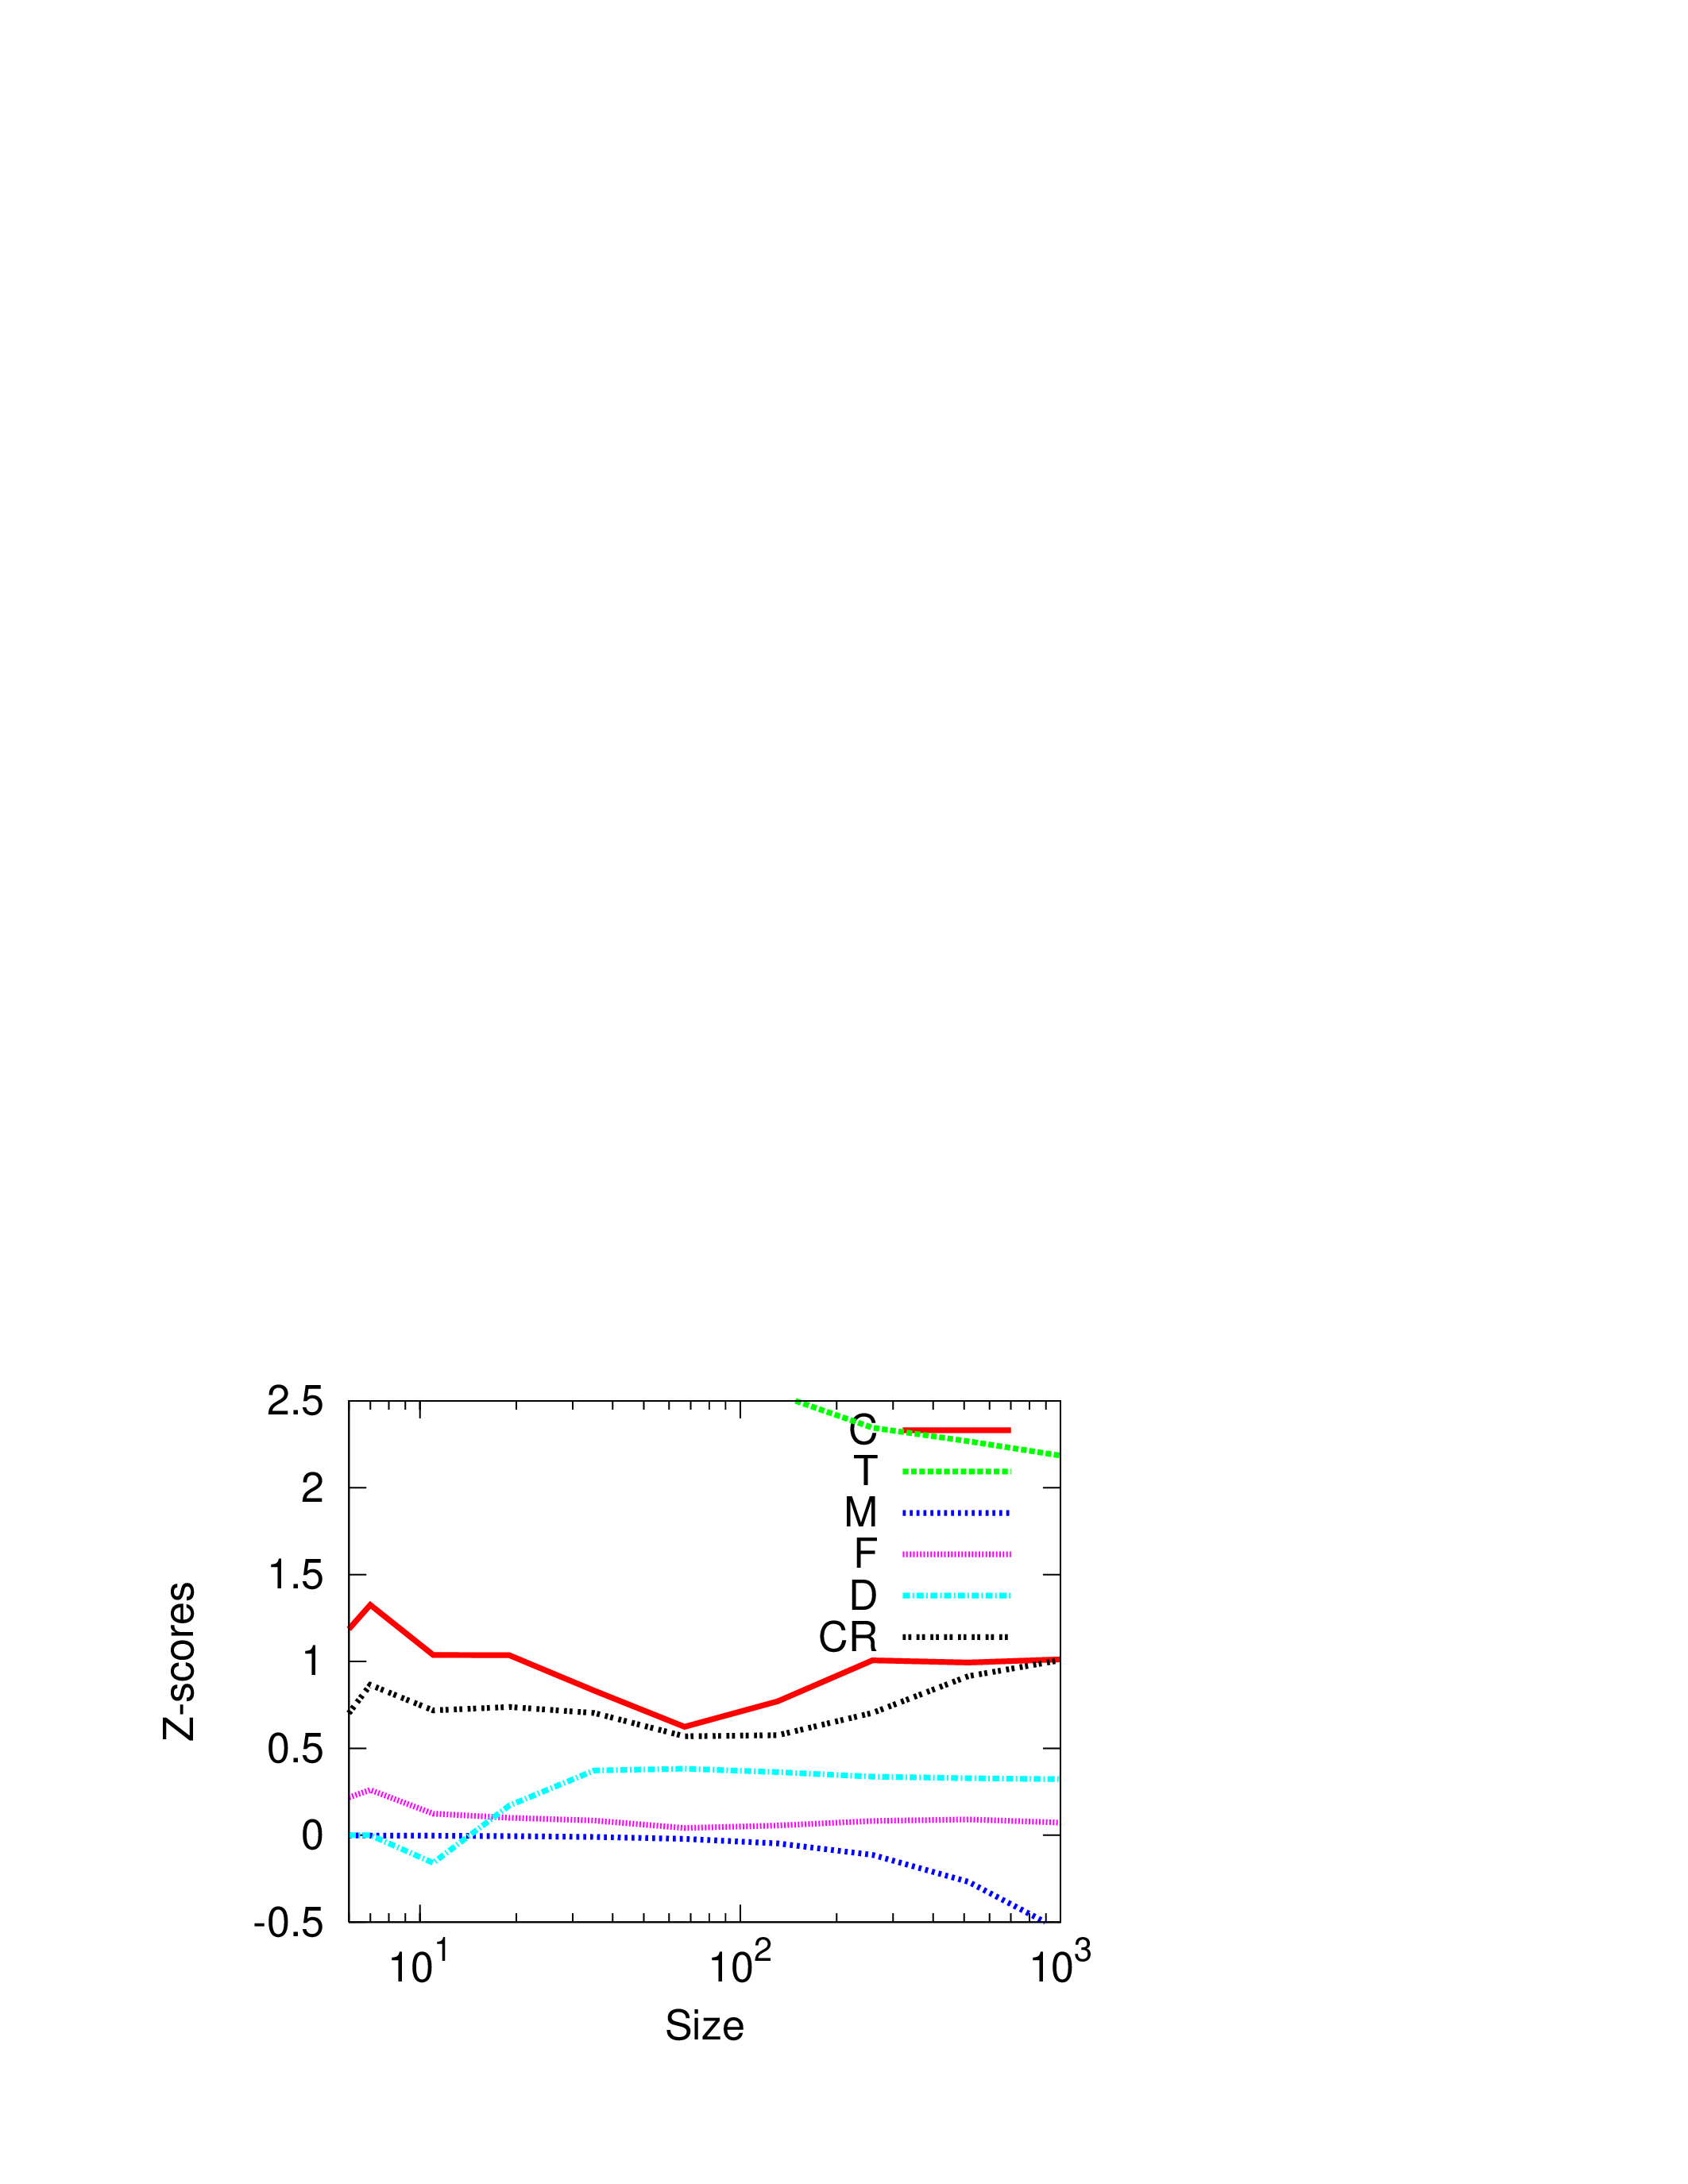}}
	\subfigure[Expand	(Orkut)]{\includegraphics[width=0.16\textwidth]{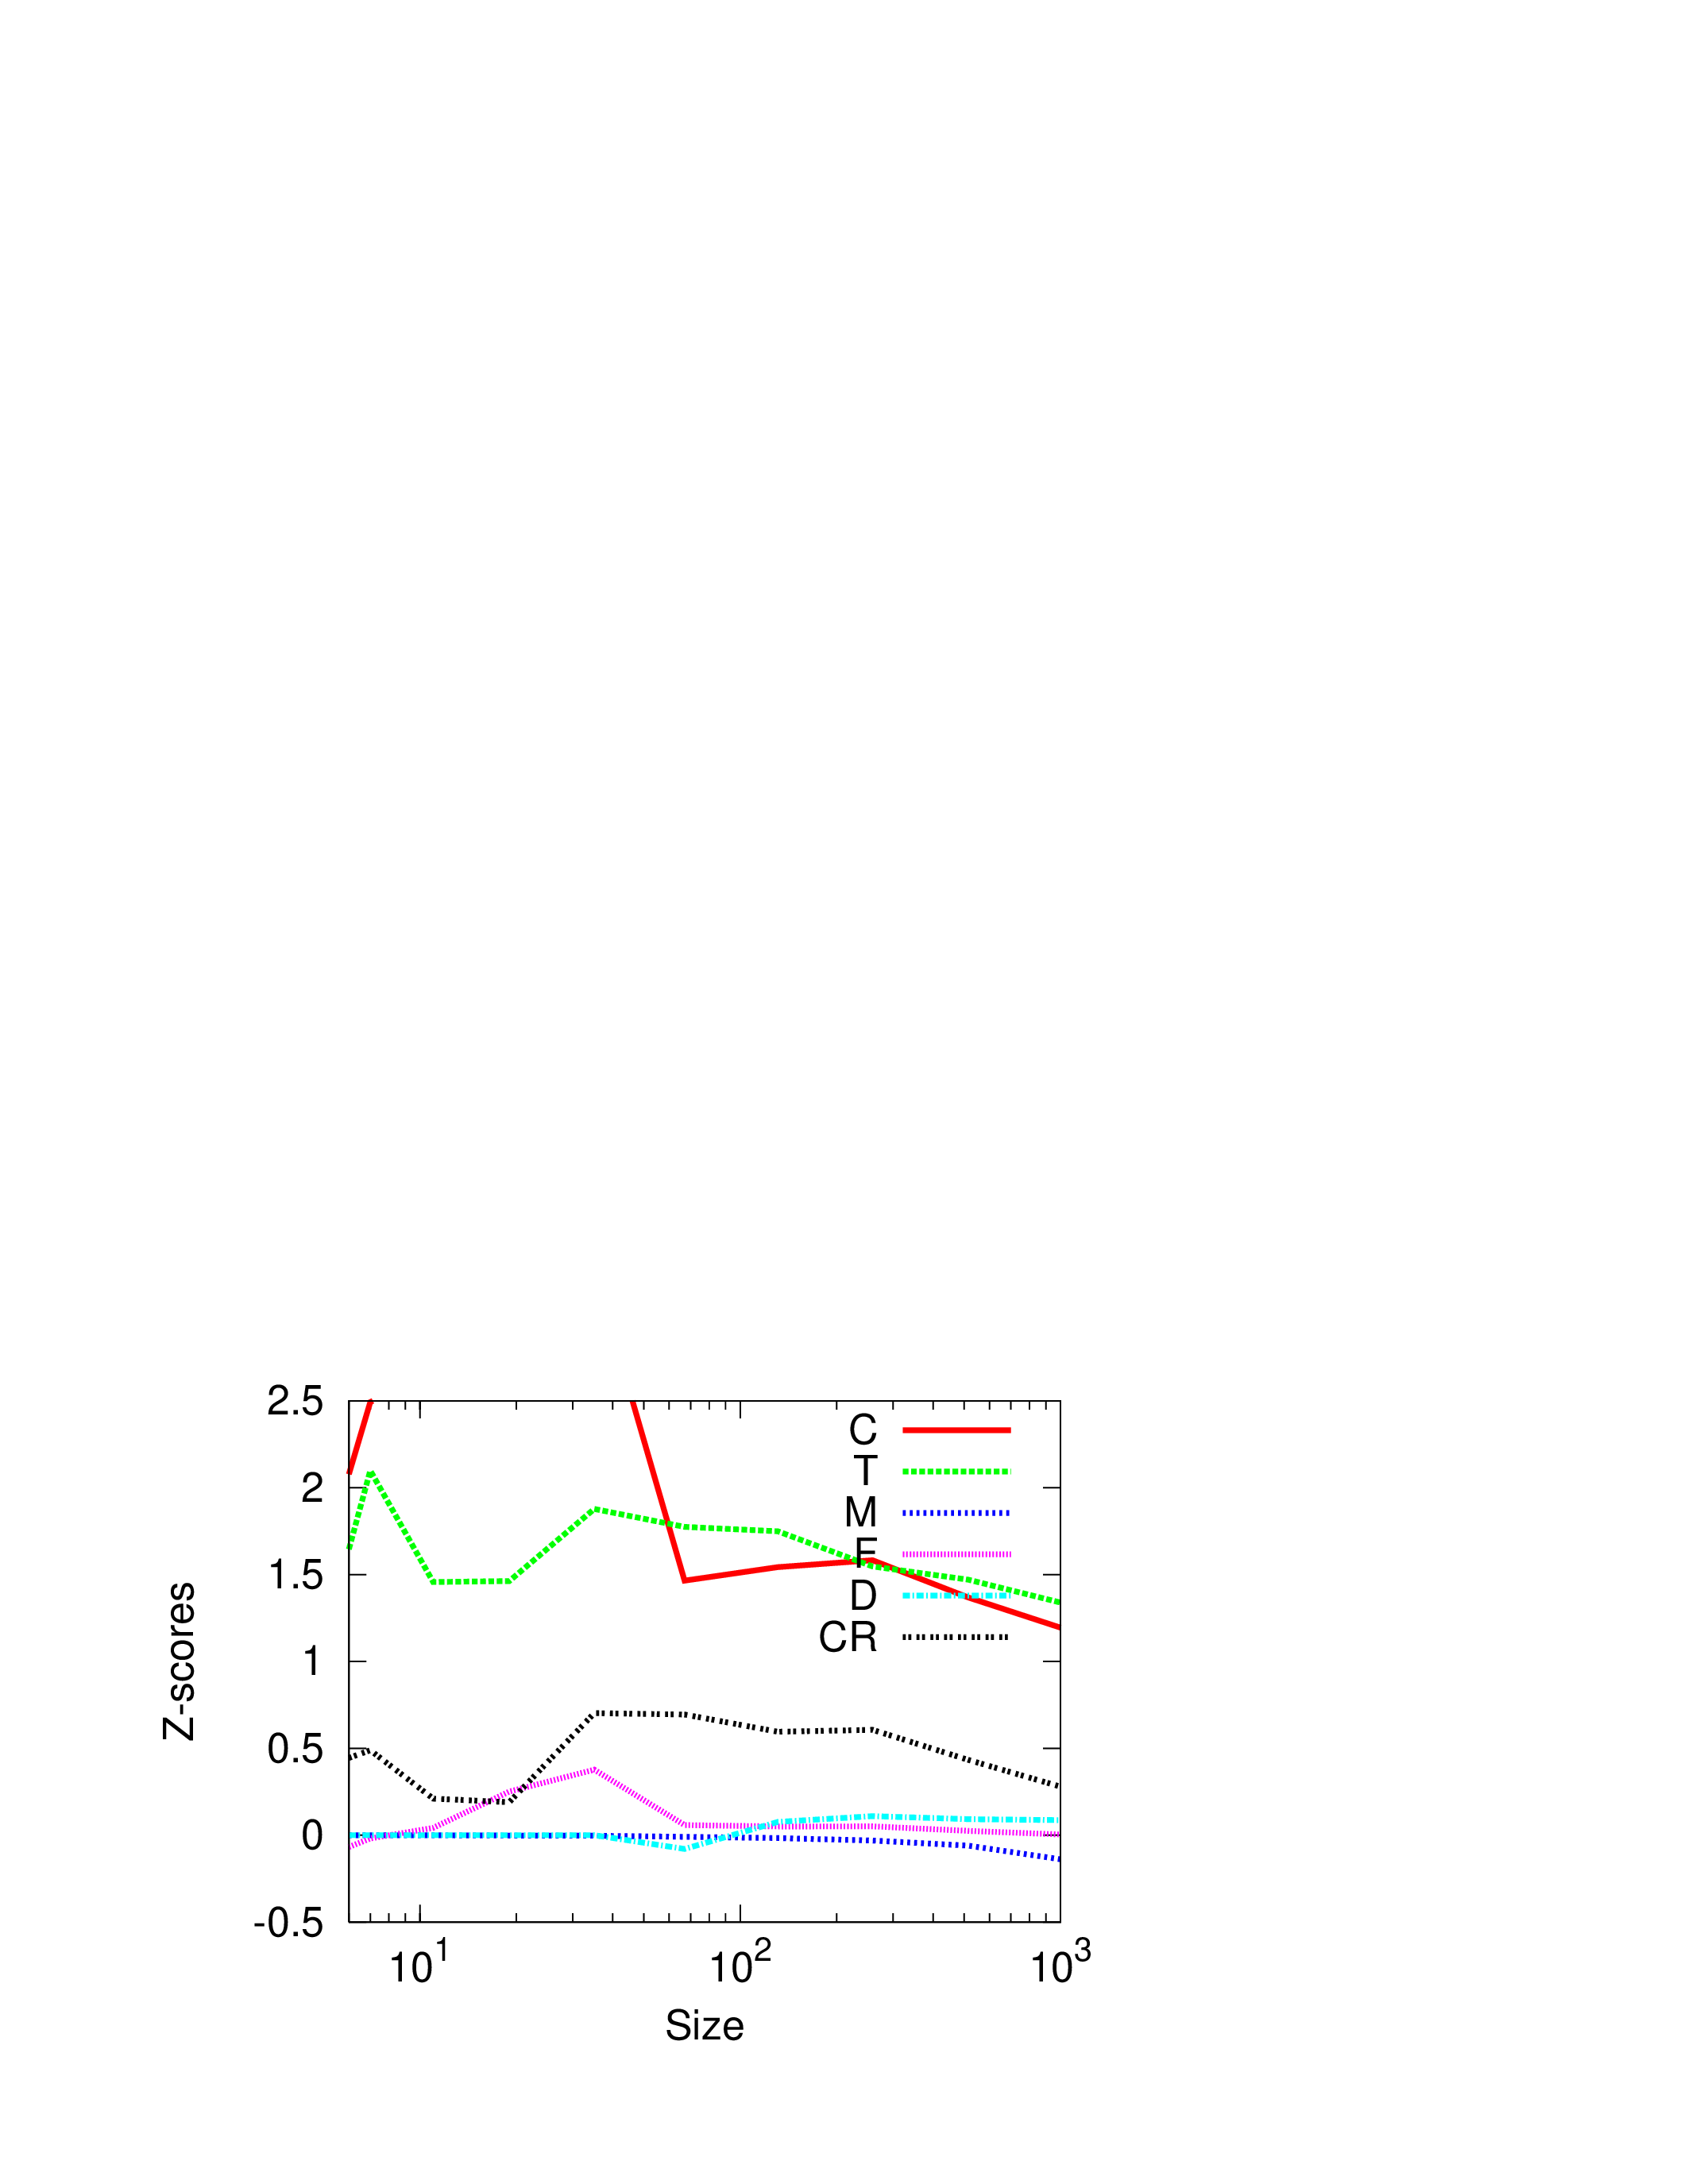}}
	\subfigure[Expand	(Ning)]{\includegraphics[width=0.16\textwidth]{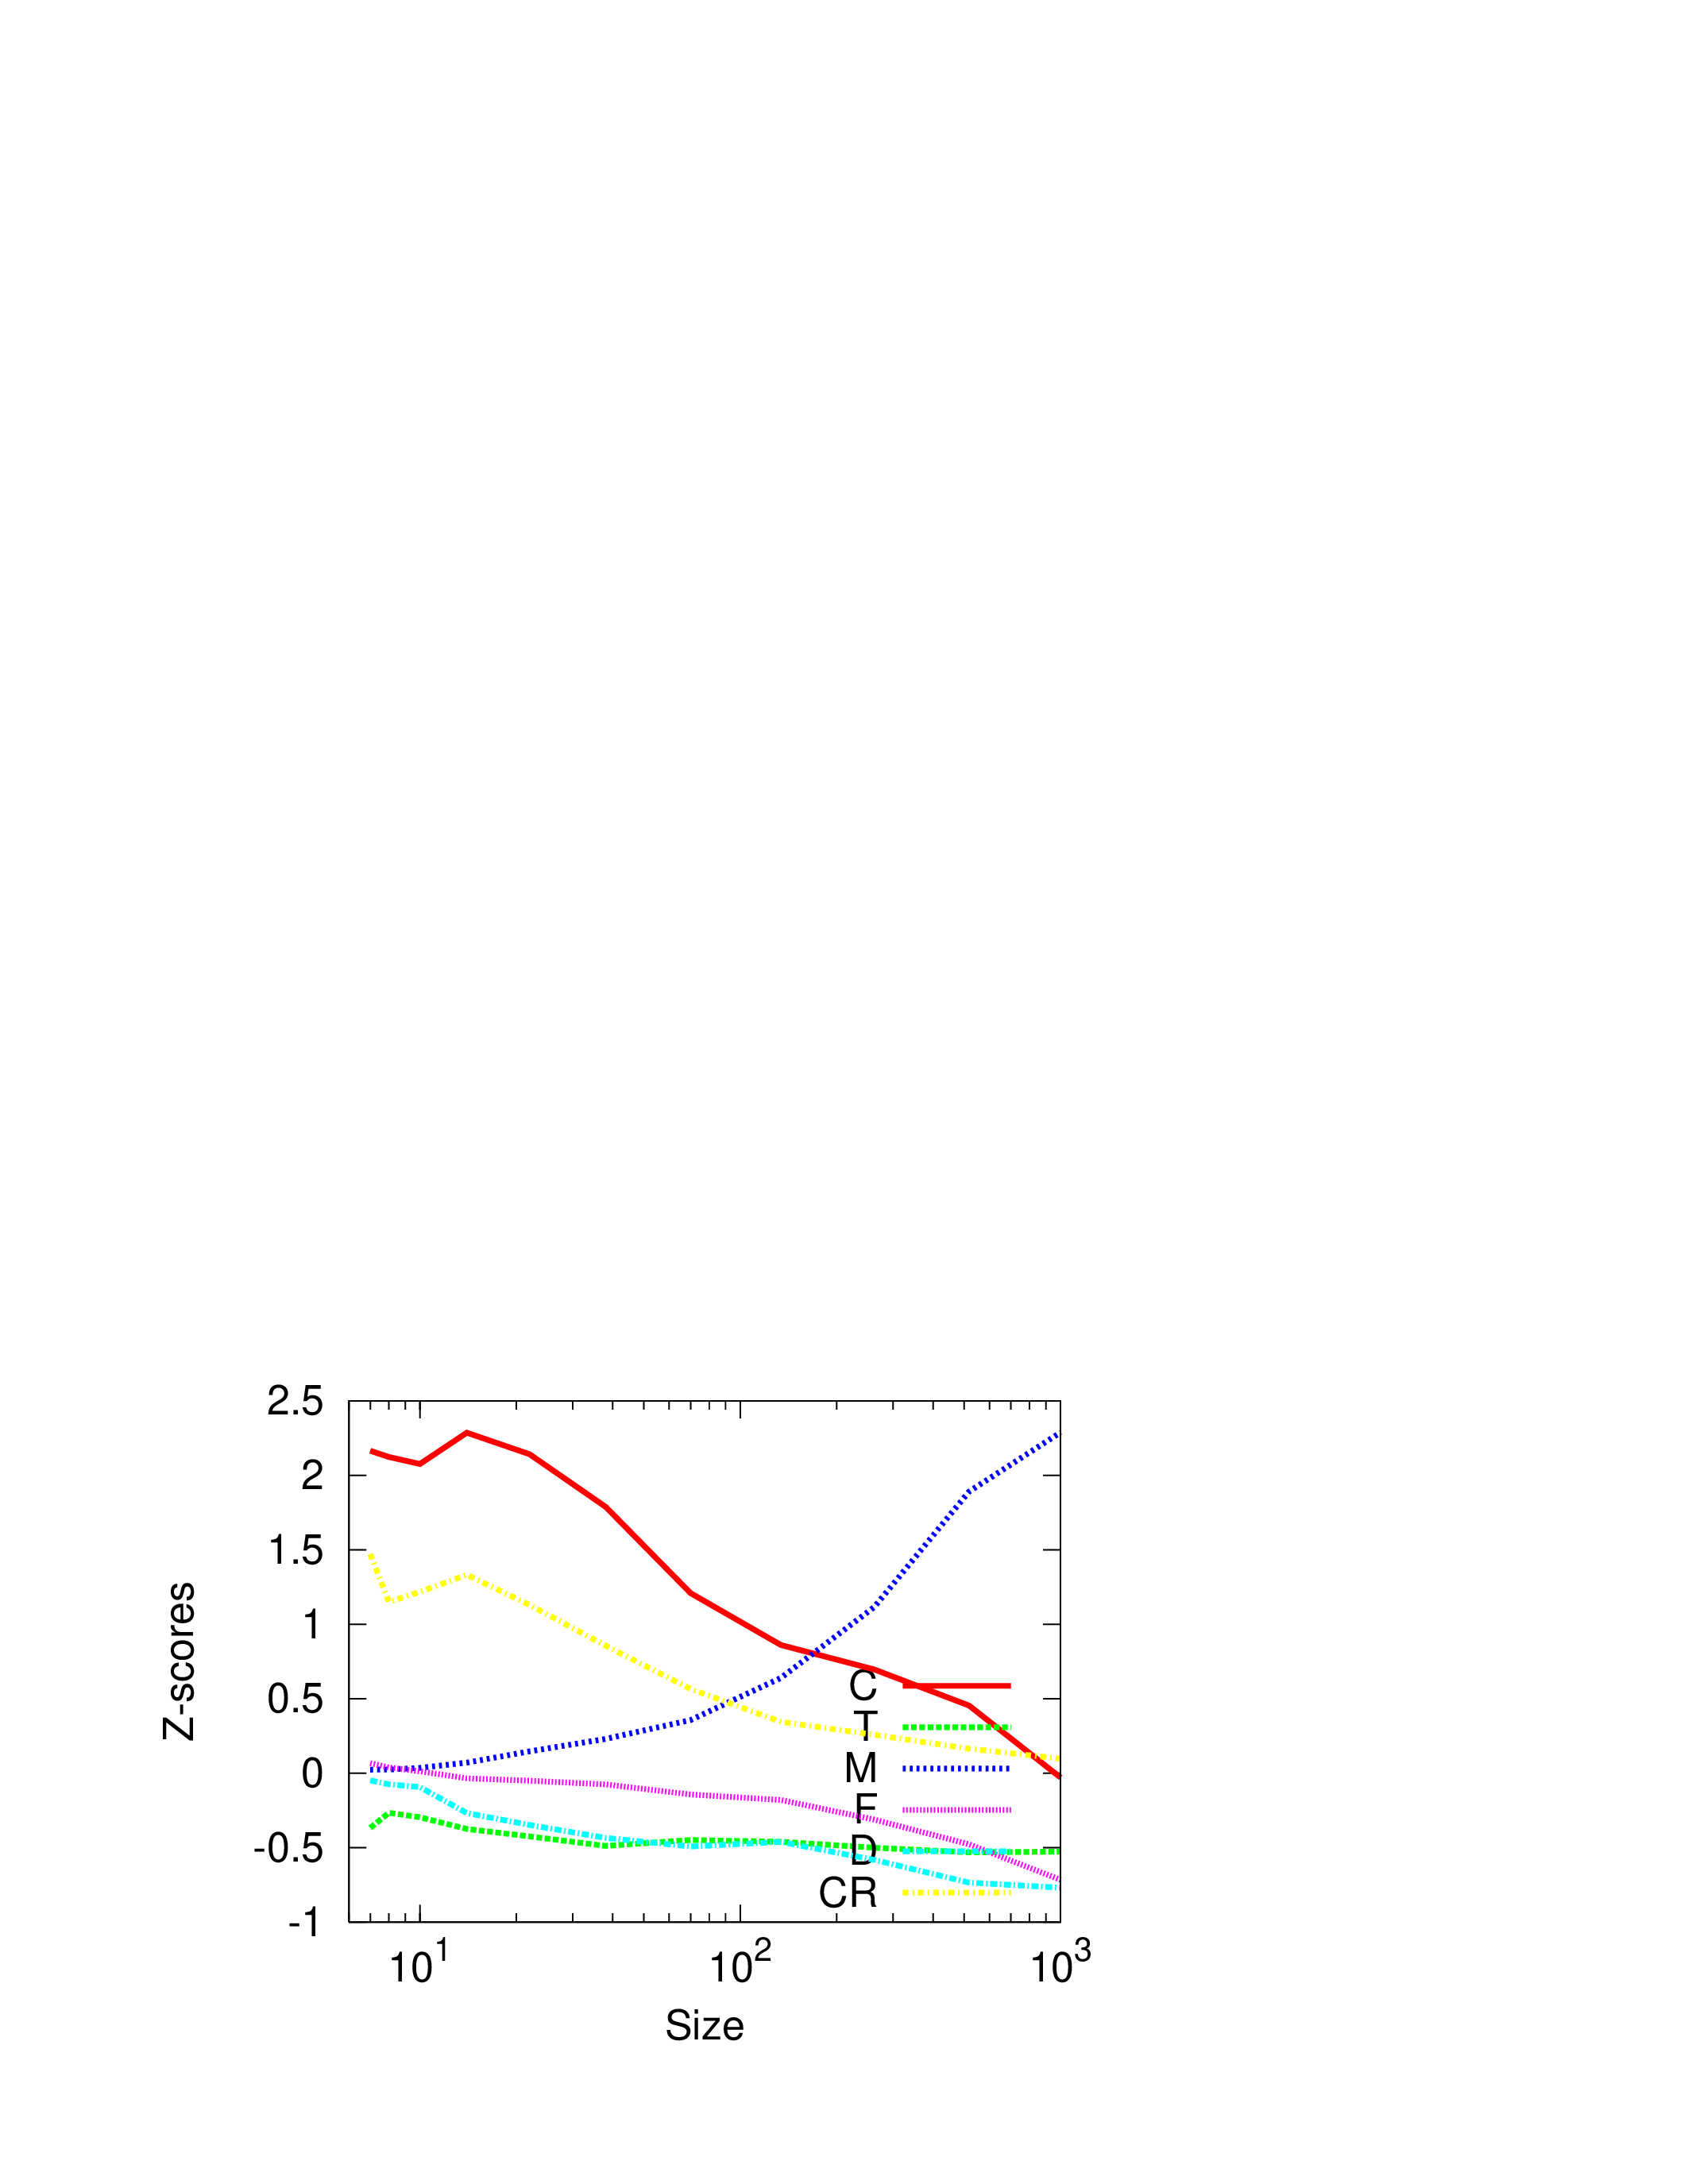}}
	\subfigure[Expand	(Amazon)]{\includegraphics[width=0.16\textwidth]{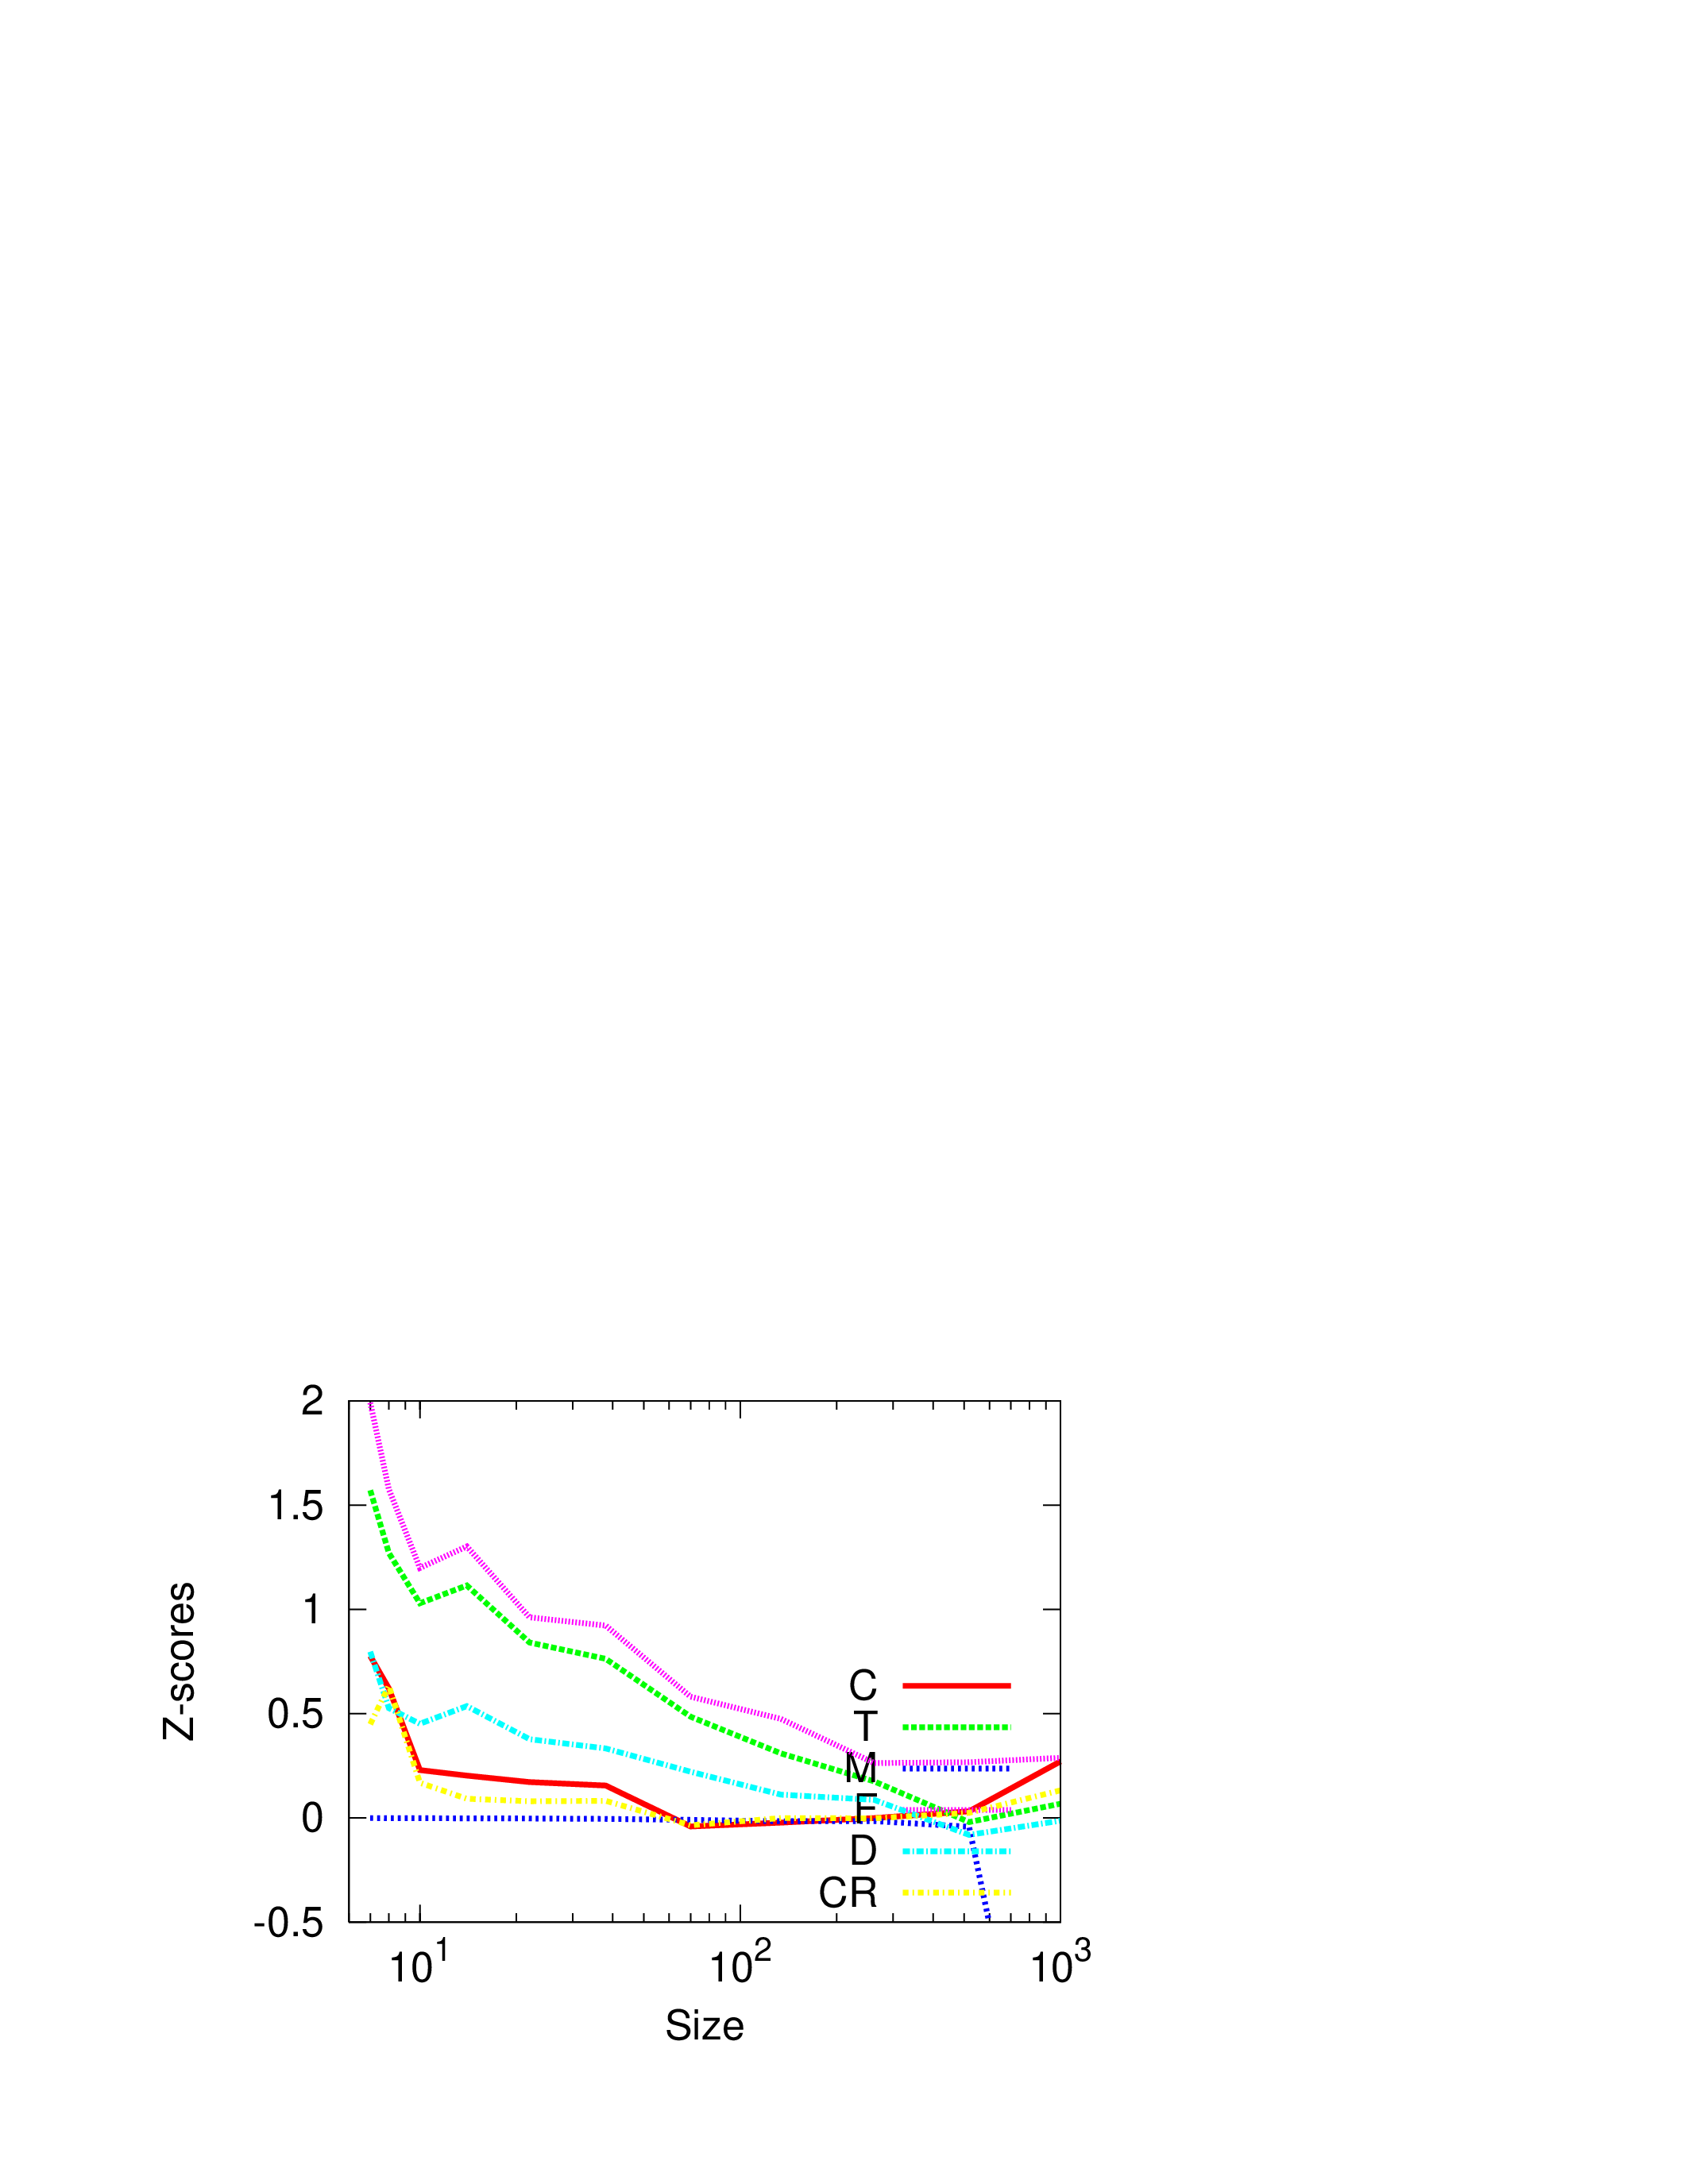}}
	\subfigure[Expand	(DBLP)]{\includegraphics[width=0.16\textwidth]{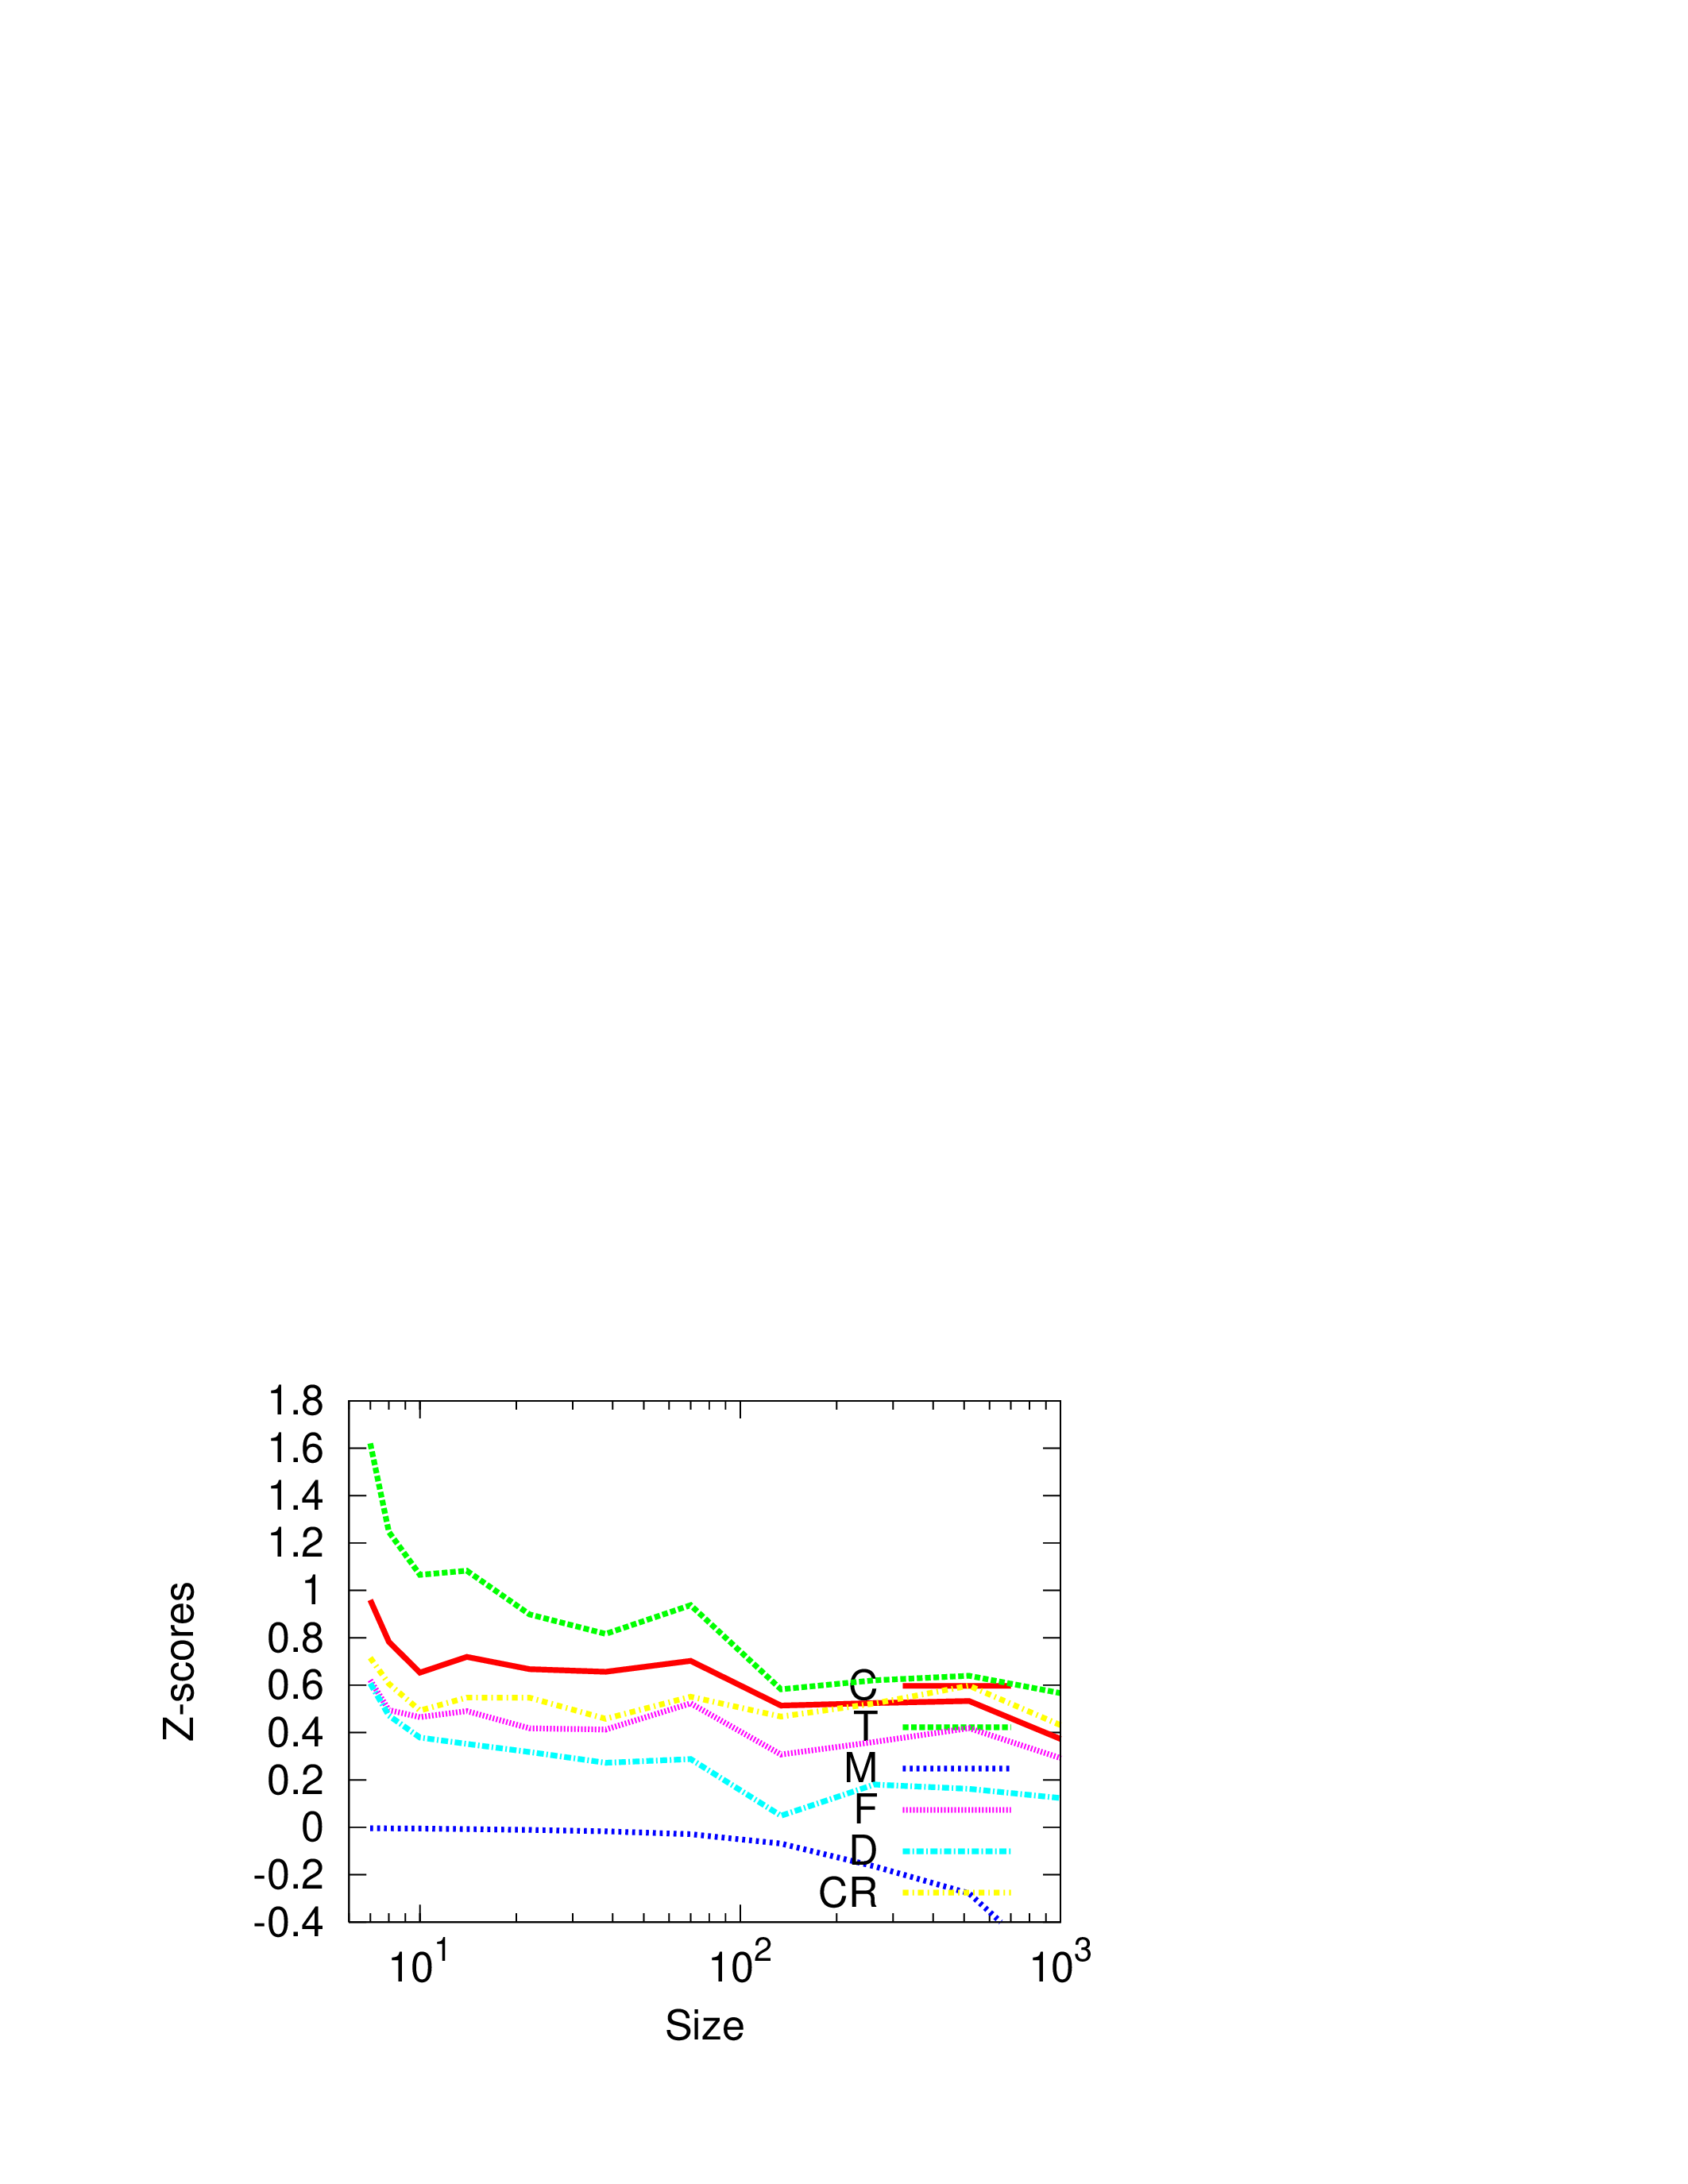}}
	\subfigure[Shrink	(LJ)]{\includegraphics[width=0.16\textwidth]{zscore.sz.Shrink.lj.eps}}
	\subfigure[Shrink	(FS)]{\includegraphics[width=0.16\textwidth]{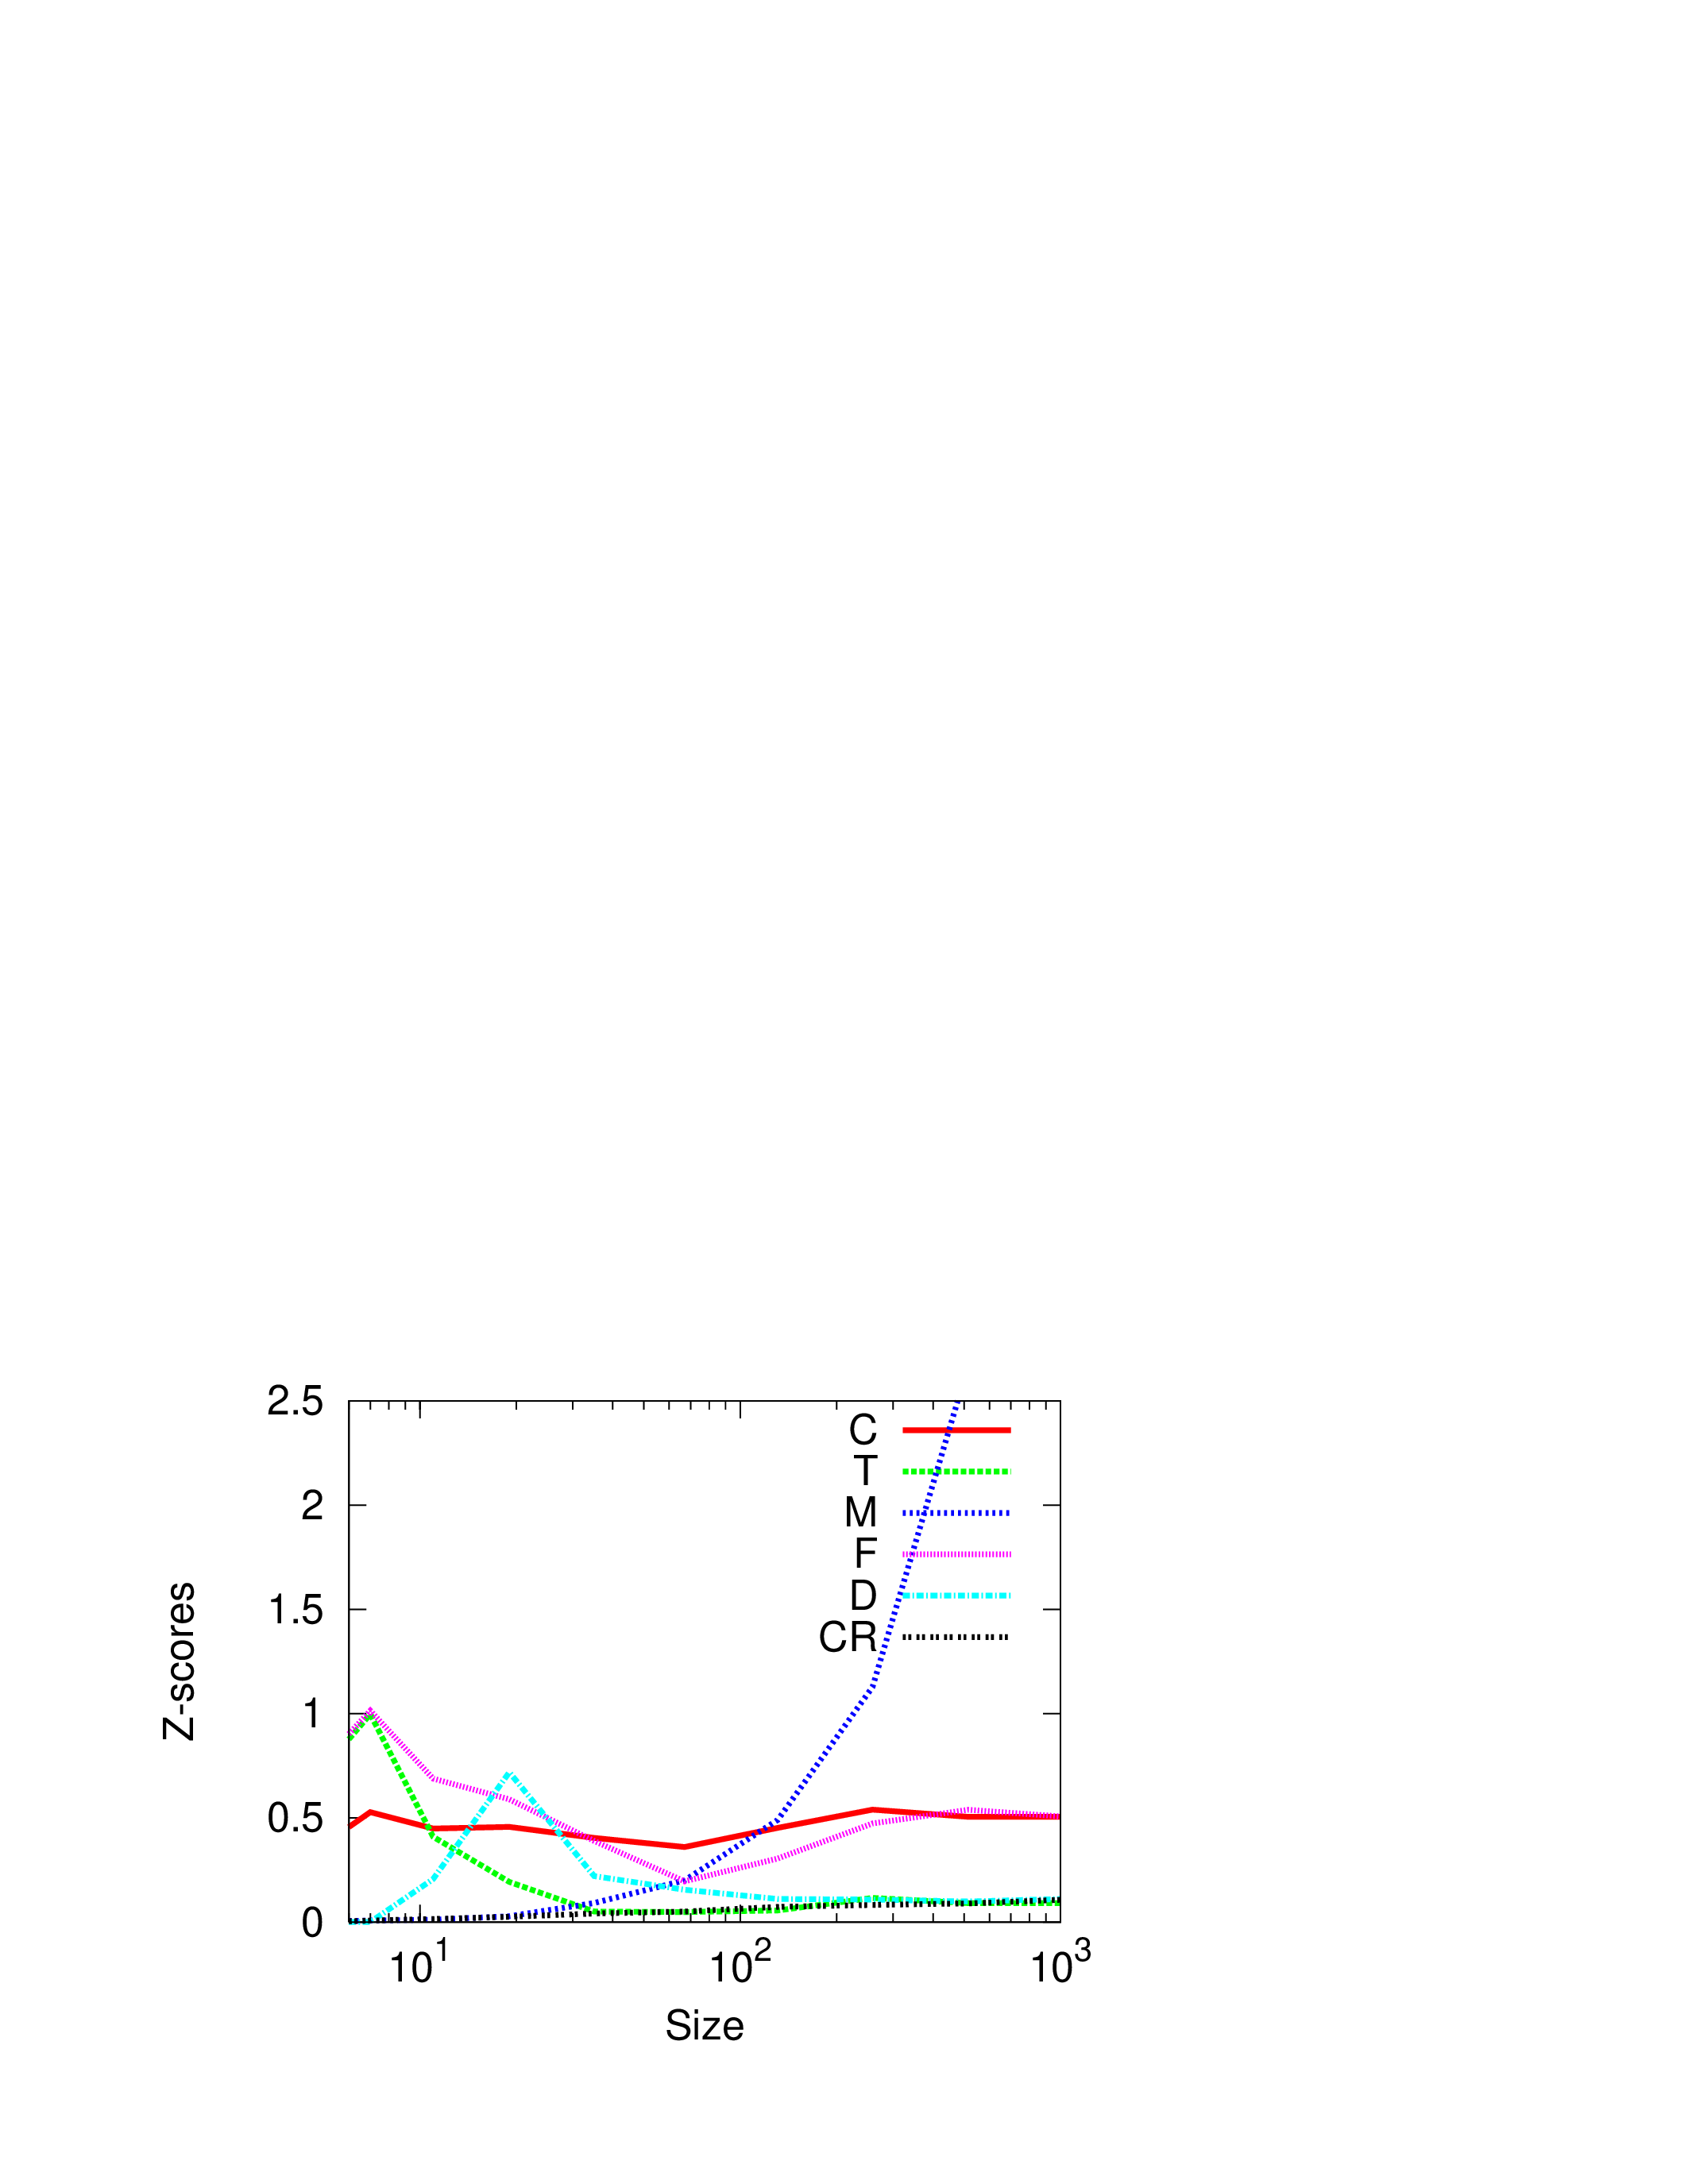}}
	\subfigure[Shrink	(Orkut)]{\includegraphics[width=0.16\textwidth]{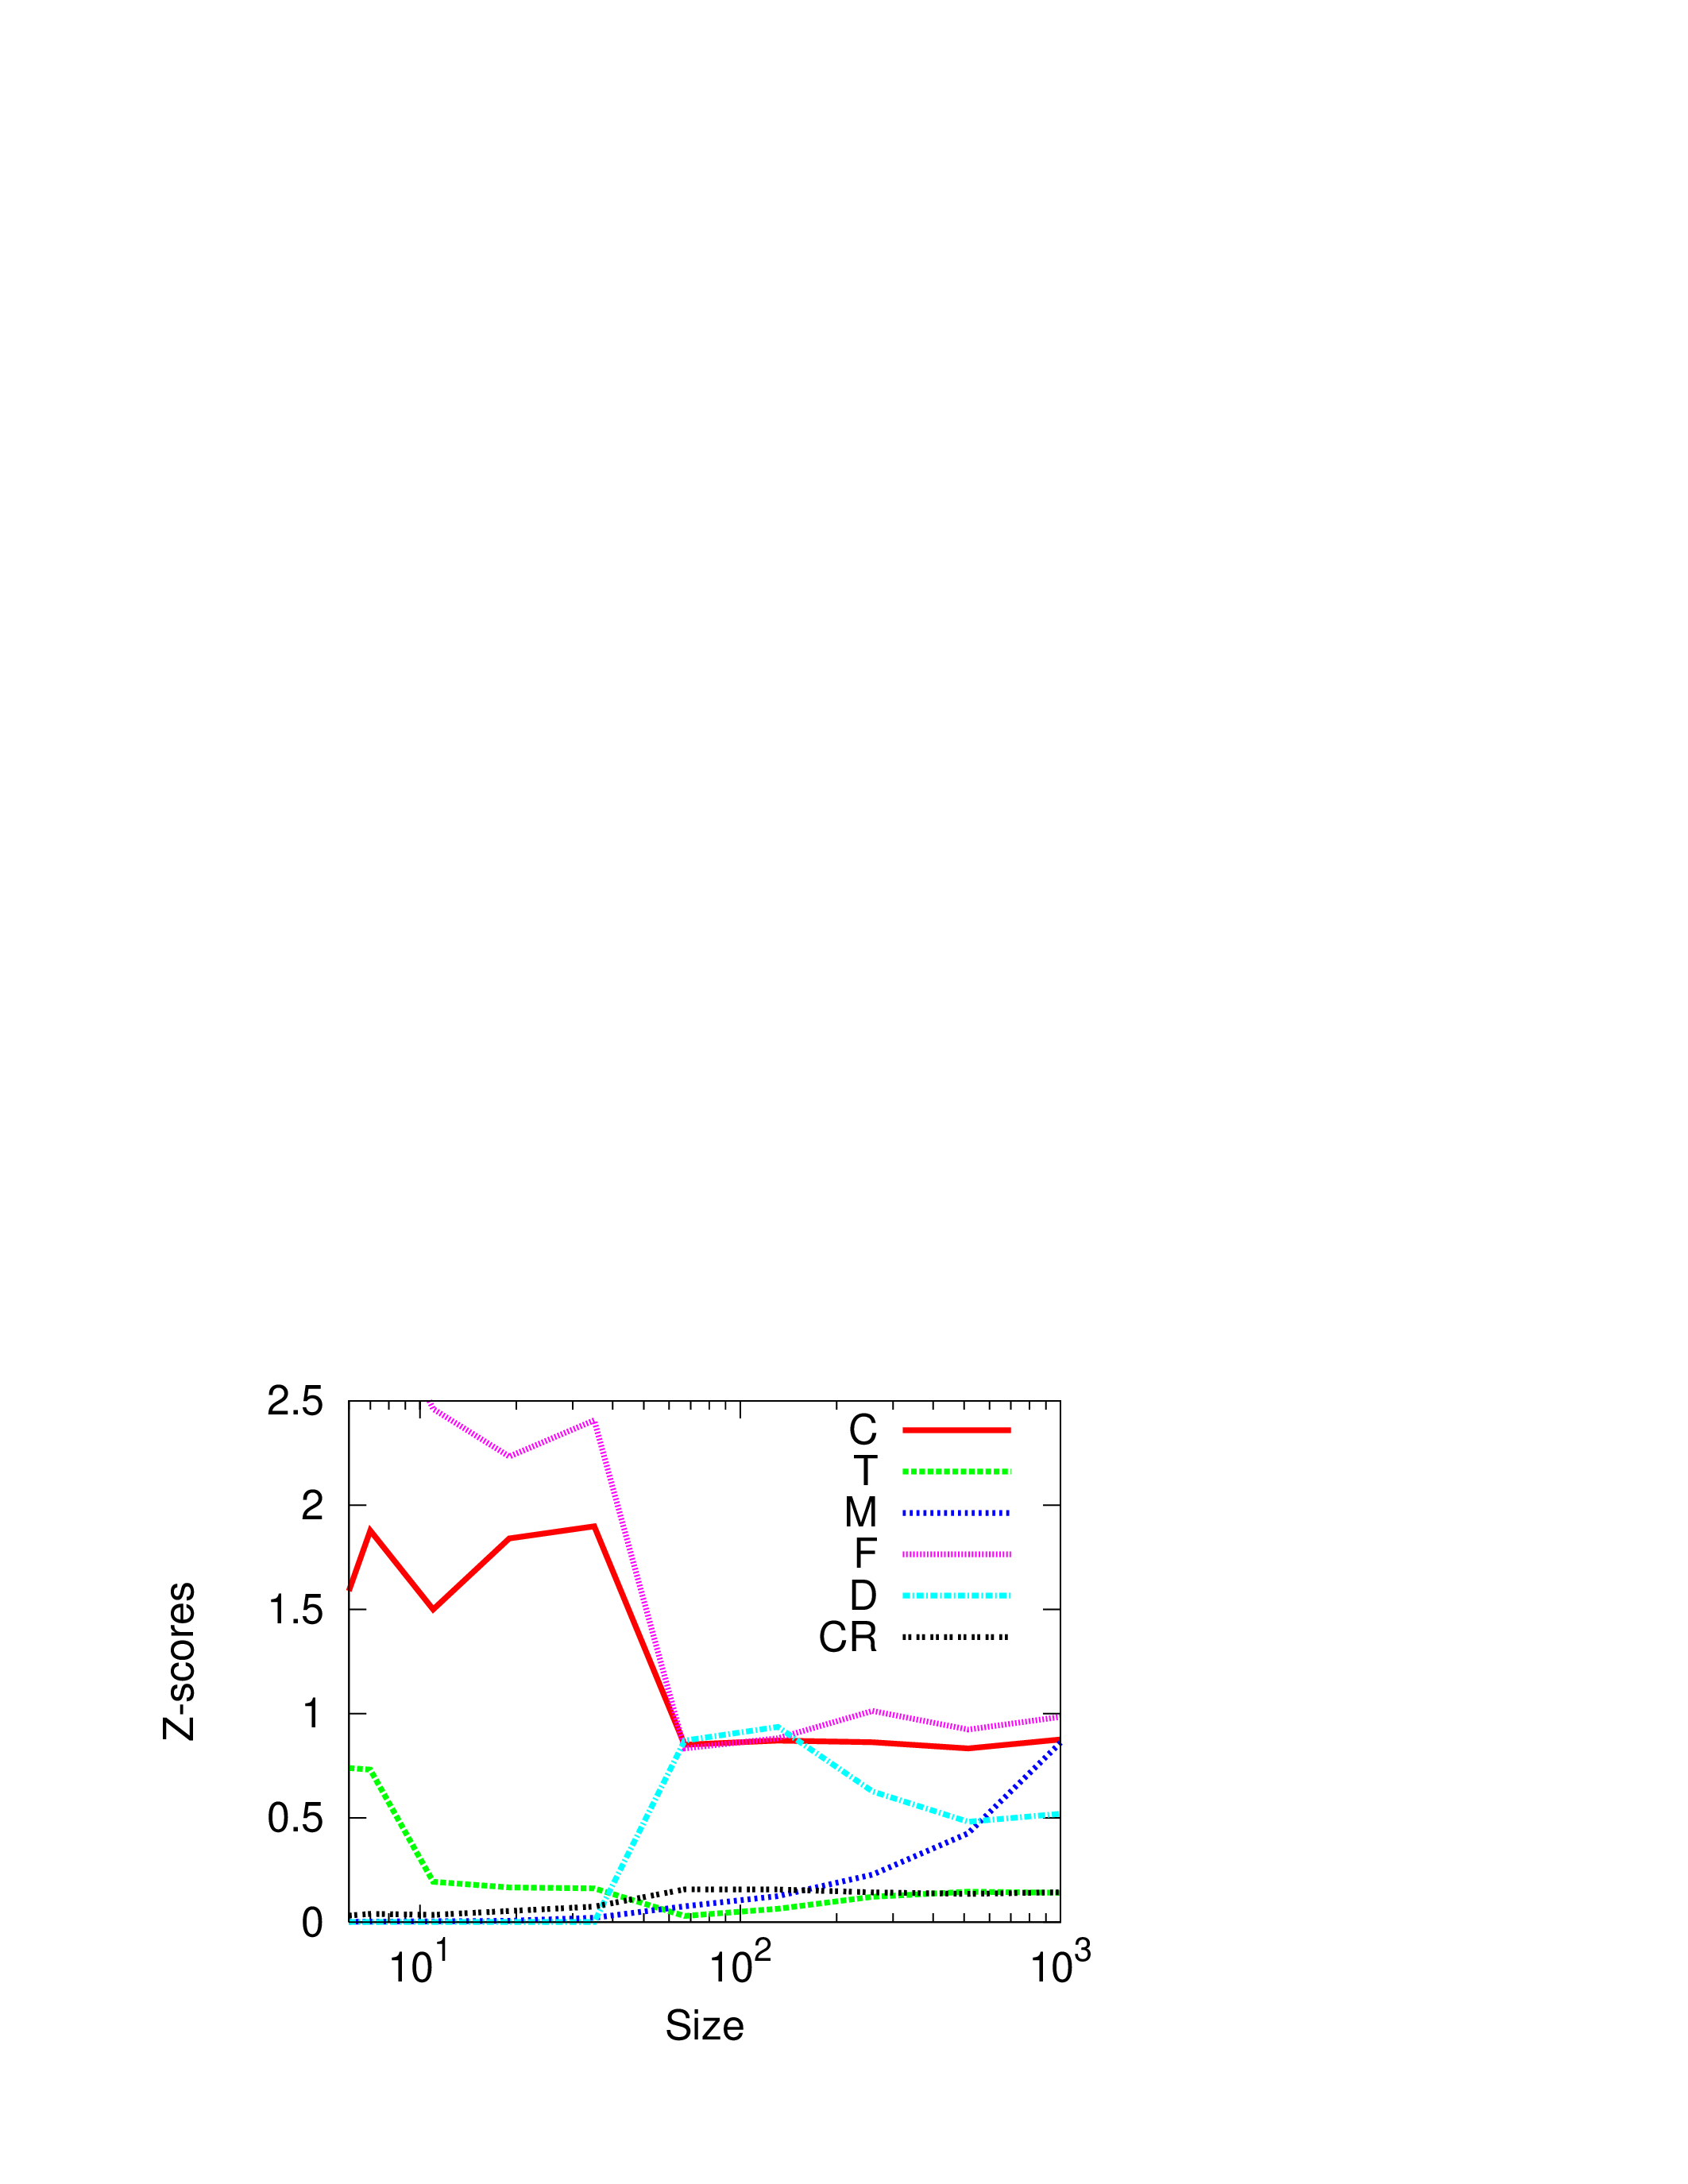}}
	\subfigure[Shrink	(Ning)]{\includegraphics[width=0.16\textwidth]{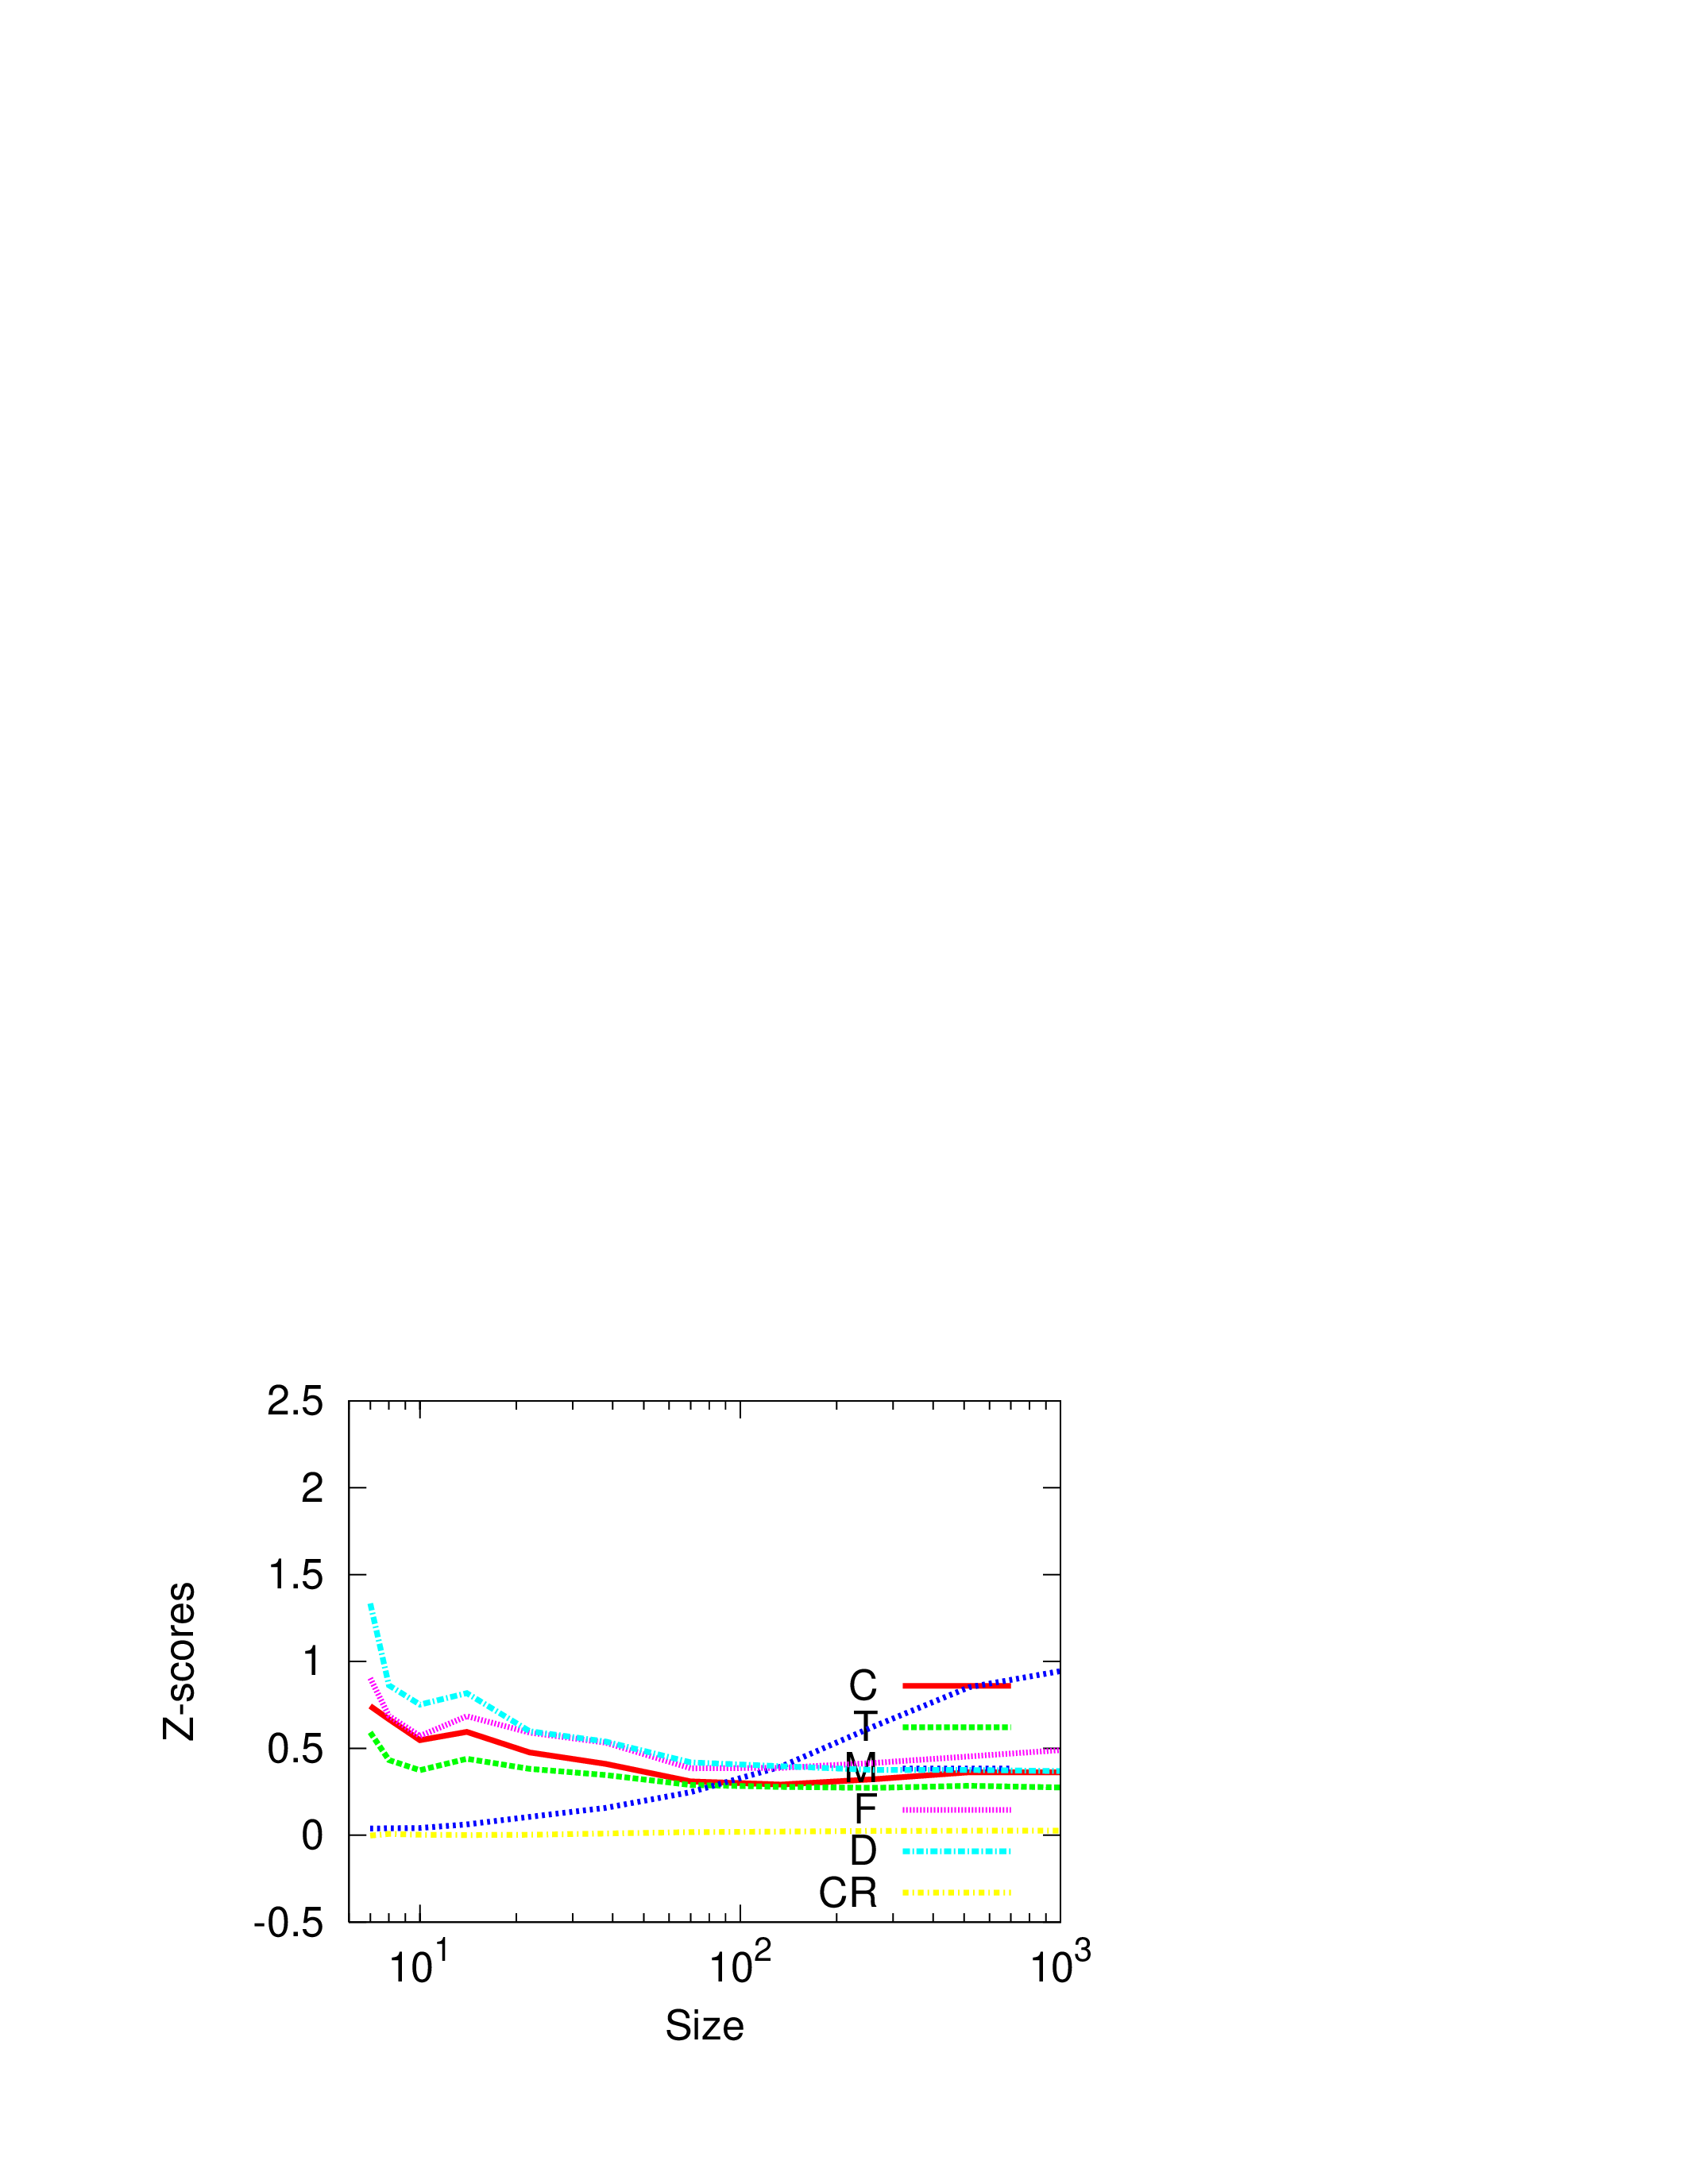}}
	\subfigure[Shrink	(Amazon)]{\includegraphics[width=0.16\textwidth]{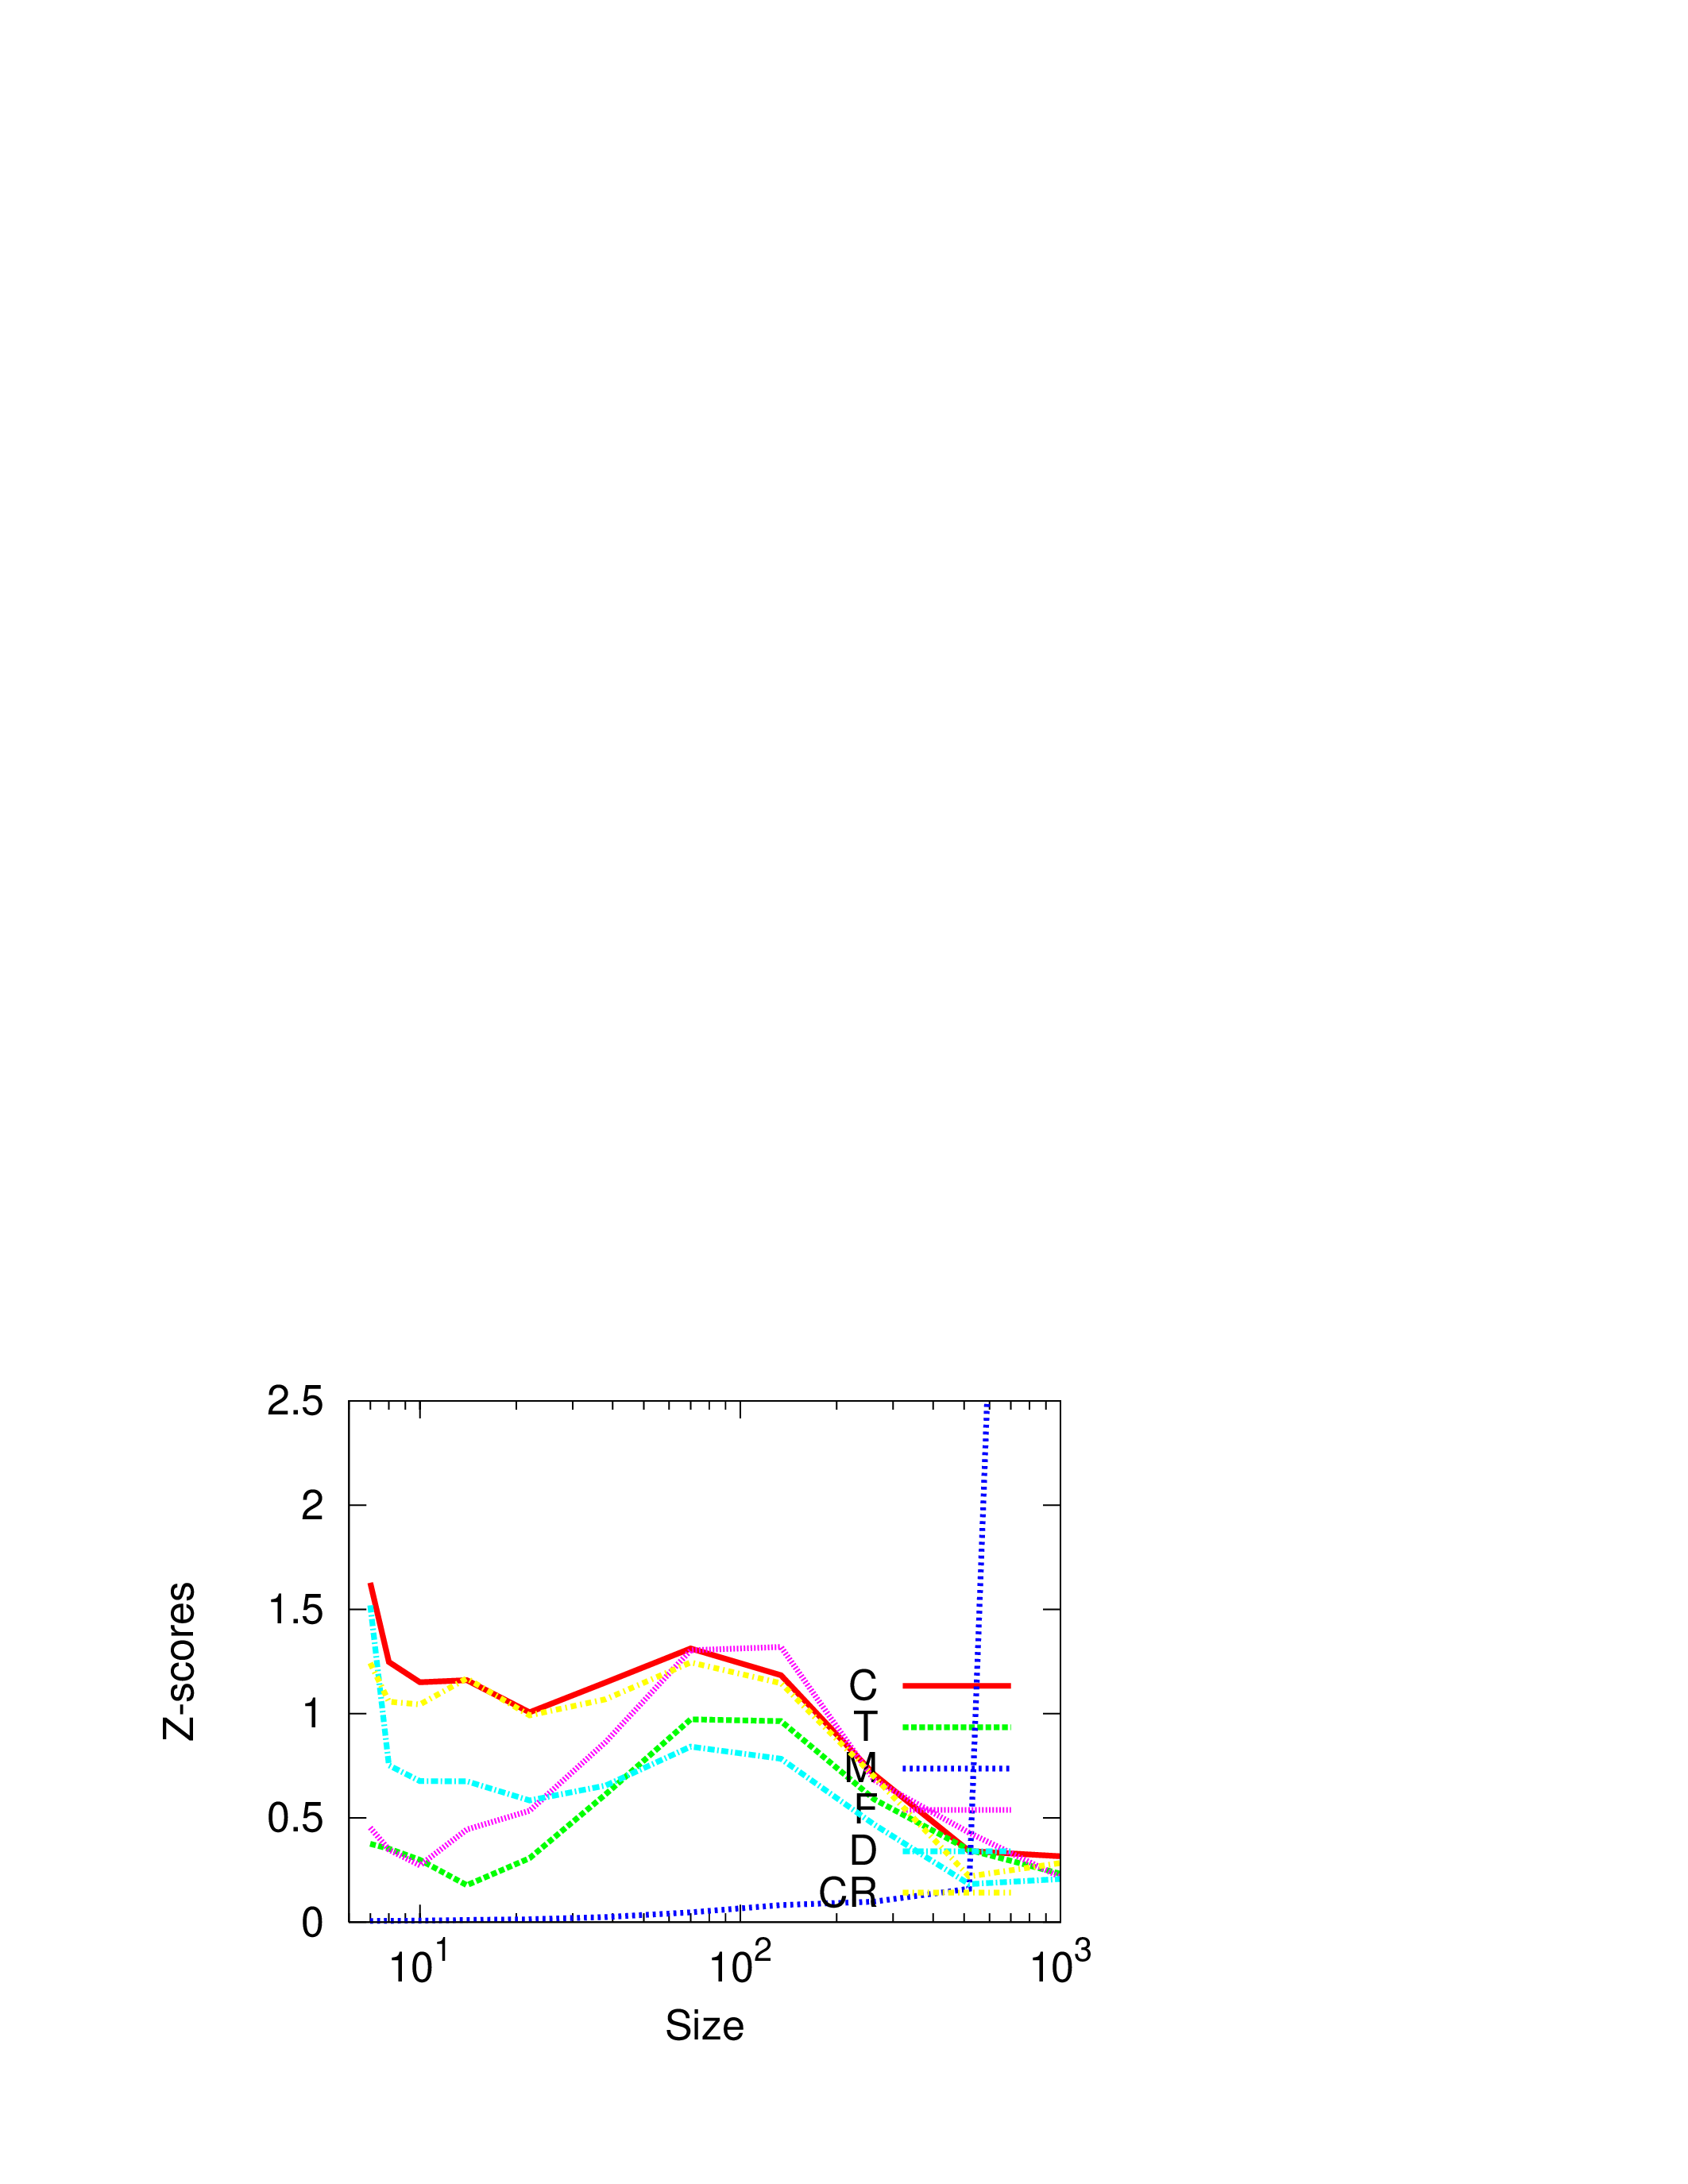}}
	\subfigure[Shrink	(DBLP)]{\includegraphics[width=0.16\textwidth]{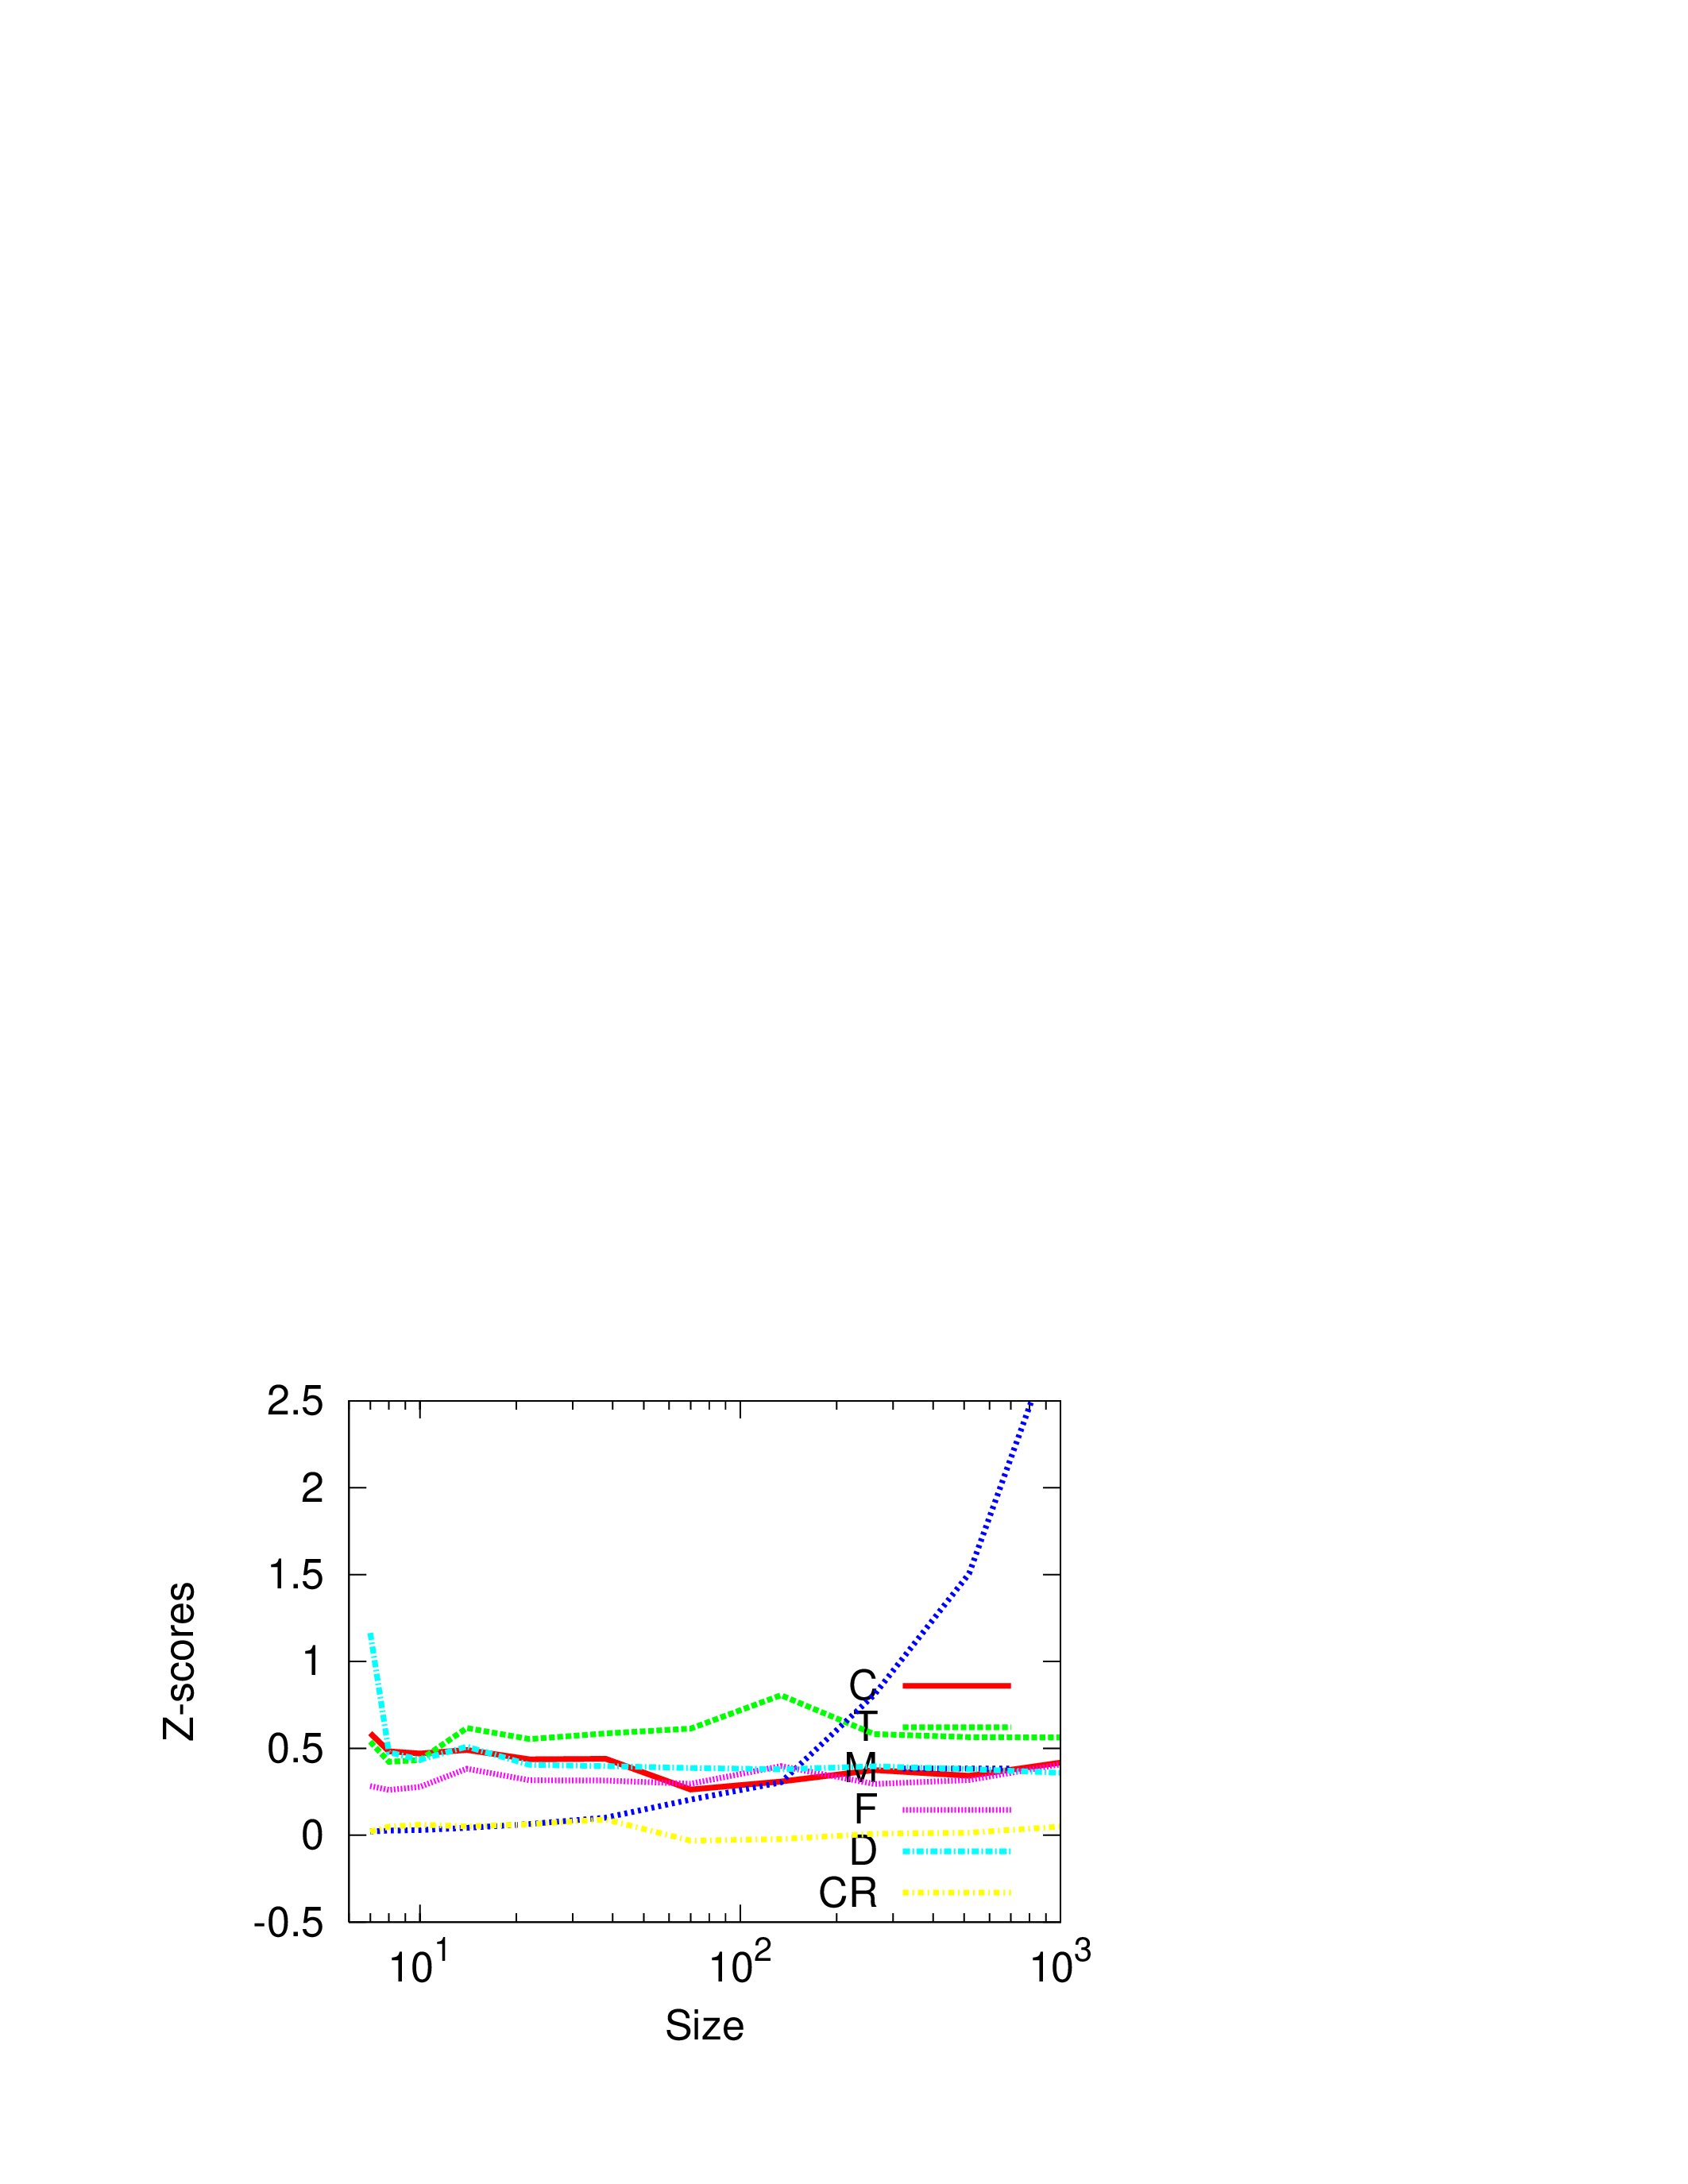}}
	\caption{Z-score of 6 scores versus the community size for each null model. C: Conductance, T: TPR, M: Modularity, F: Flake-ODF, D: FOMD, CR: Cut-Ratio}
\label{fig:Zscore.Sz}
\end{figure*}
}

\hide{
\begin{figure*}[t]
	\centering
	\subfigure[Separability	(LJ)]{\includegraphics[width=0.185\textwidth]{rank_property.CutToEdgeIns.lj.eps}}
	\subfigure[Separability	 (Ning)]{\includegraphics[width=0.185\textwidth]{rank_property.CutToEdgeIns.Ning.eps}}
	\subfigure[Separability	 (Amazon)]{\includegraphics[width=0.185\textwidth]{rank_property.CutToEdgeIns.amazon.eps}}
	\subfigure[Separability	 (DBLP)]{\includegraphics[width=0.185\textwidth]{rank_property.CutToEdgeIns.dblp.eps}}
	\subfigure[Separability	 (IMDB)]{\includegraphics[width=0.185\textwidth]{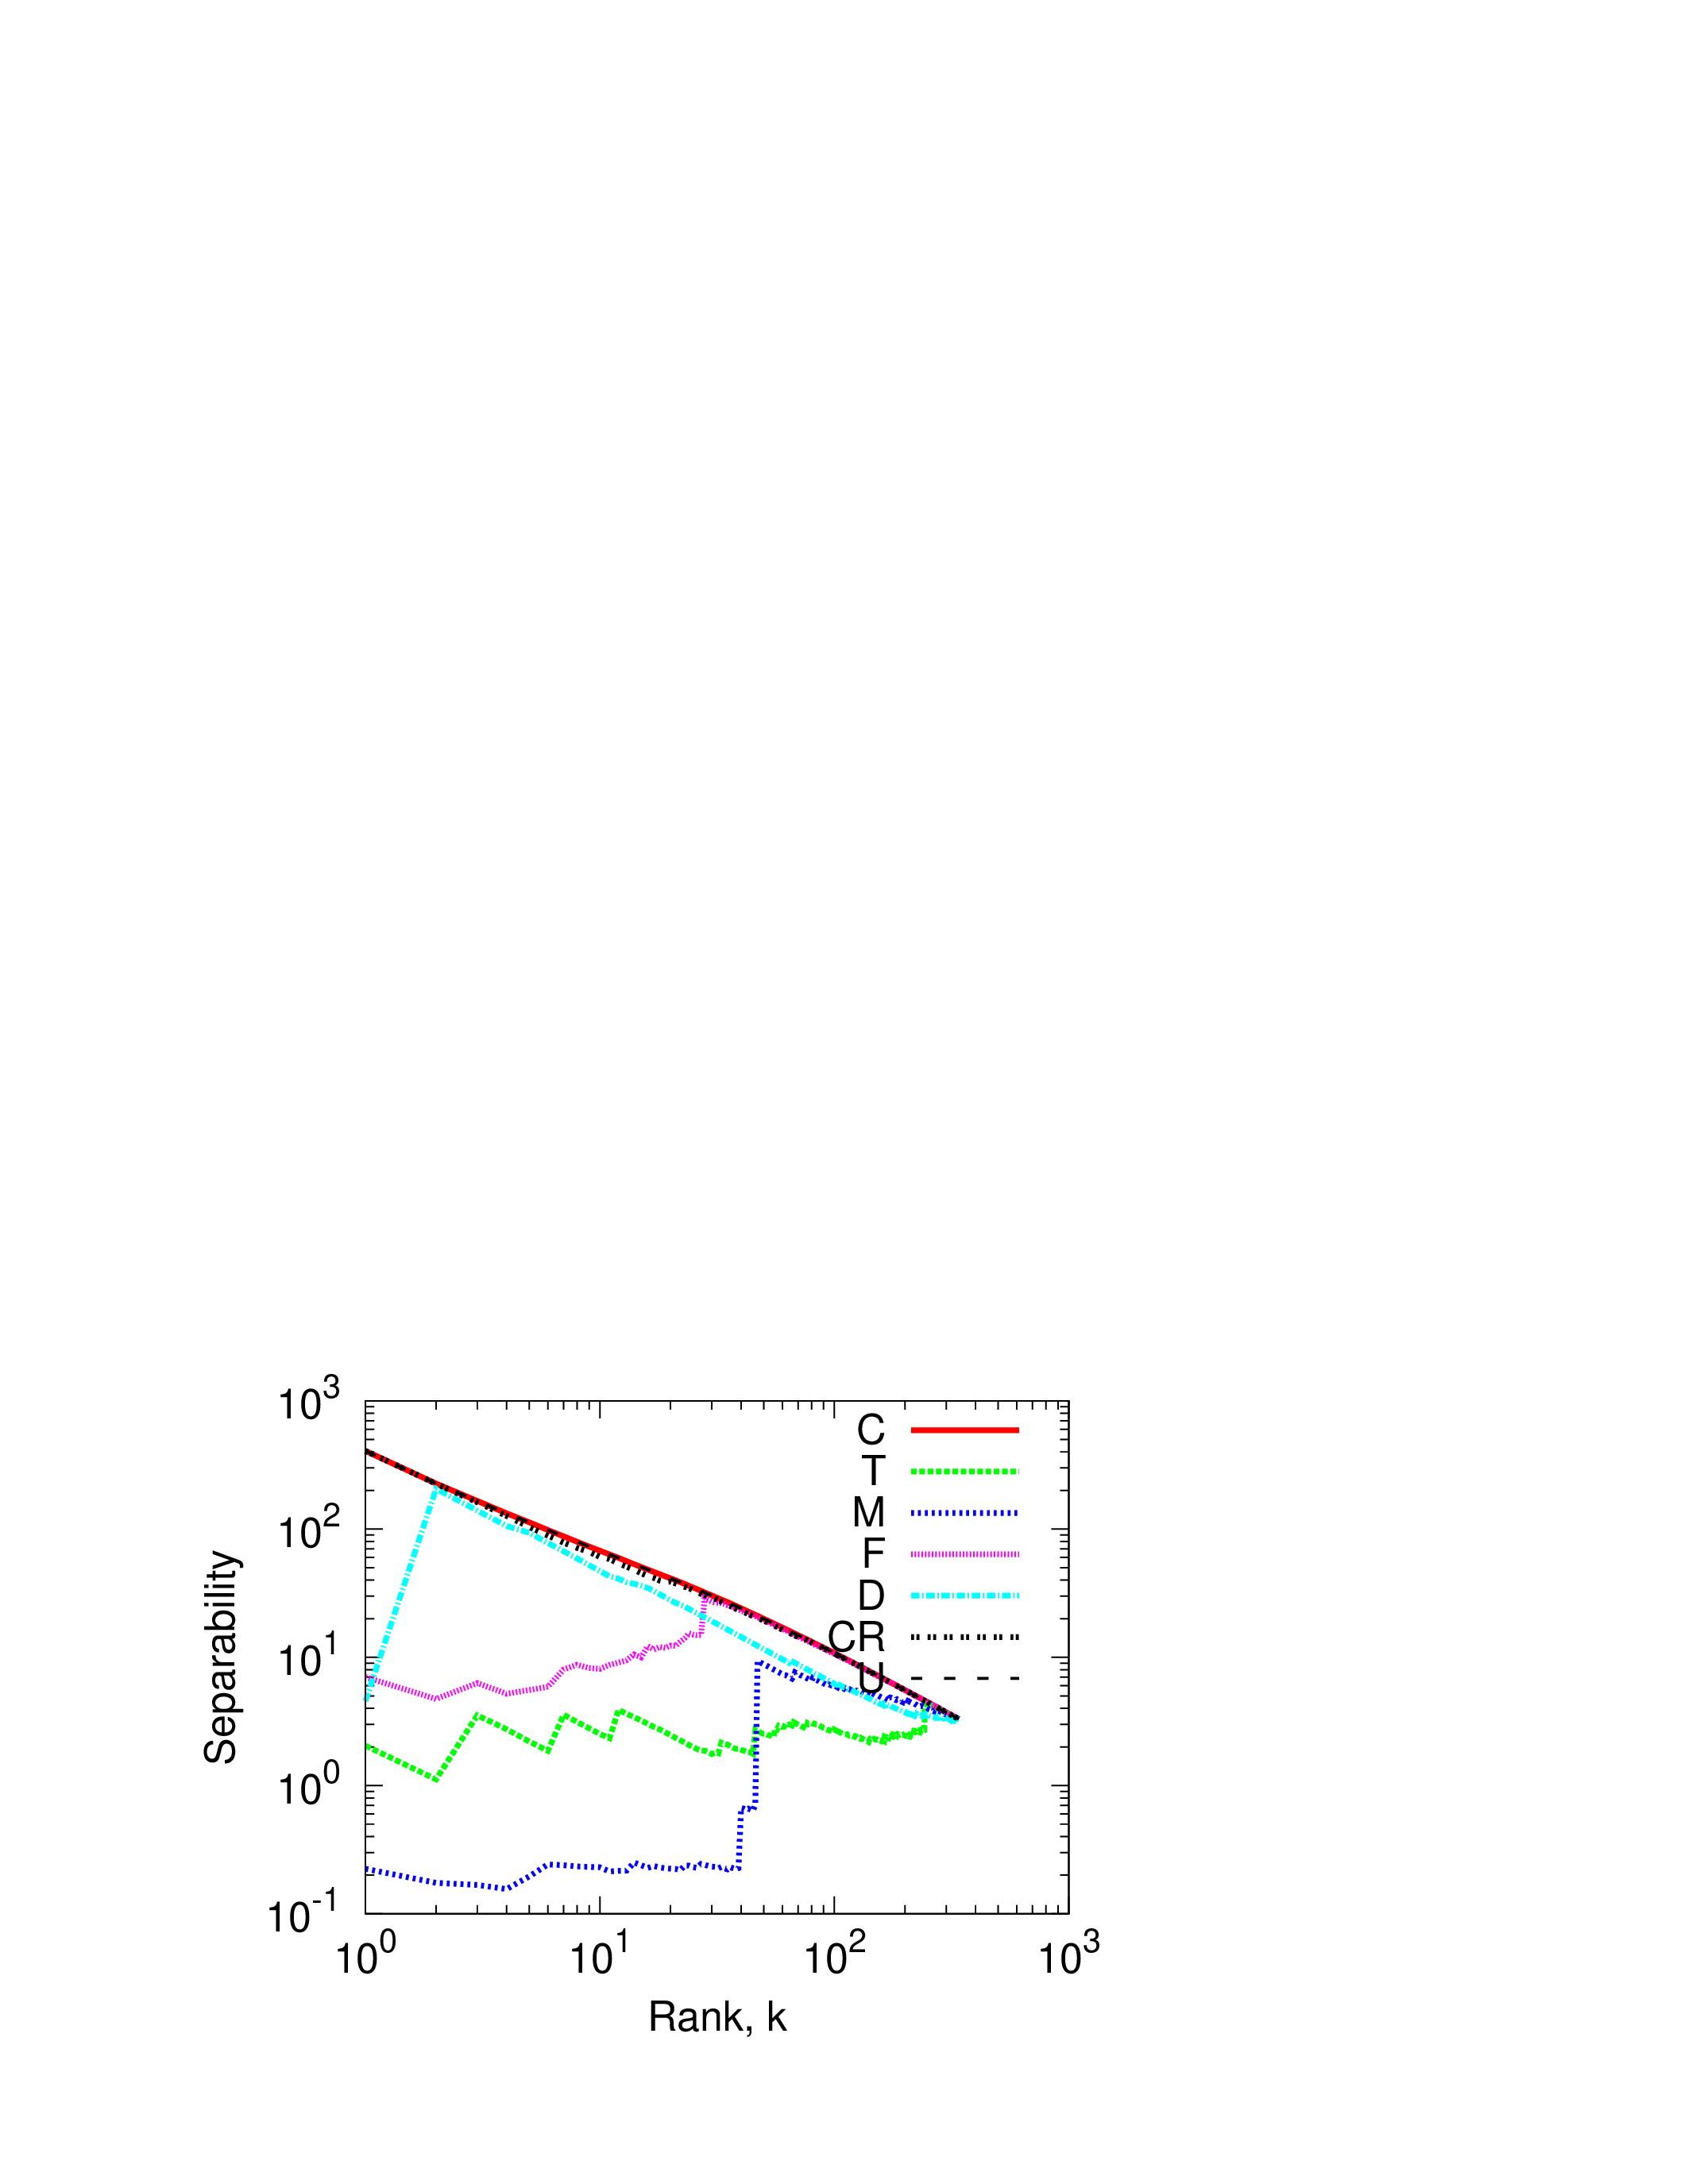}}
	\subfigure[Density	(LJ)]{\includegraphics[width=0.185\textwidth]{rank_property.Density.lj.eps}}
	\subfigure[Density	(Ning)]{\includegraphics[width=0.185\textwidth]{rank_property.Density.Ning.eps}}
	\subfigure[Density	(Amazon)]{\includegraphics[width=0.185\textwidth]{rank_property.Density.amazon.eps}}
	\subfigure[Density	(DBLP)]{\includegraphics[width=0.185\textwidth]{rank_property.Density.dblp.eps}}
	\subfigure[Density	(IMDB)]{\includegraphics[width=0.185\textwidth]{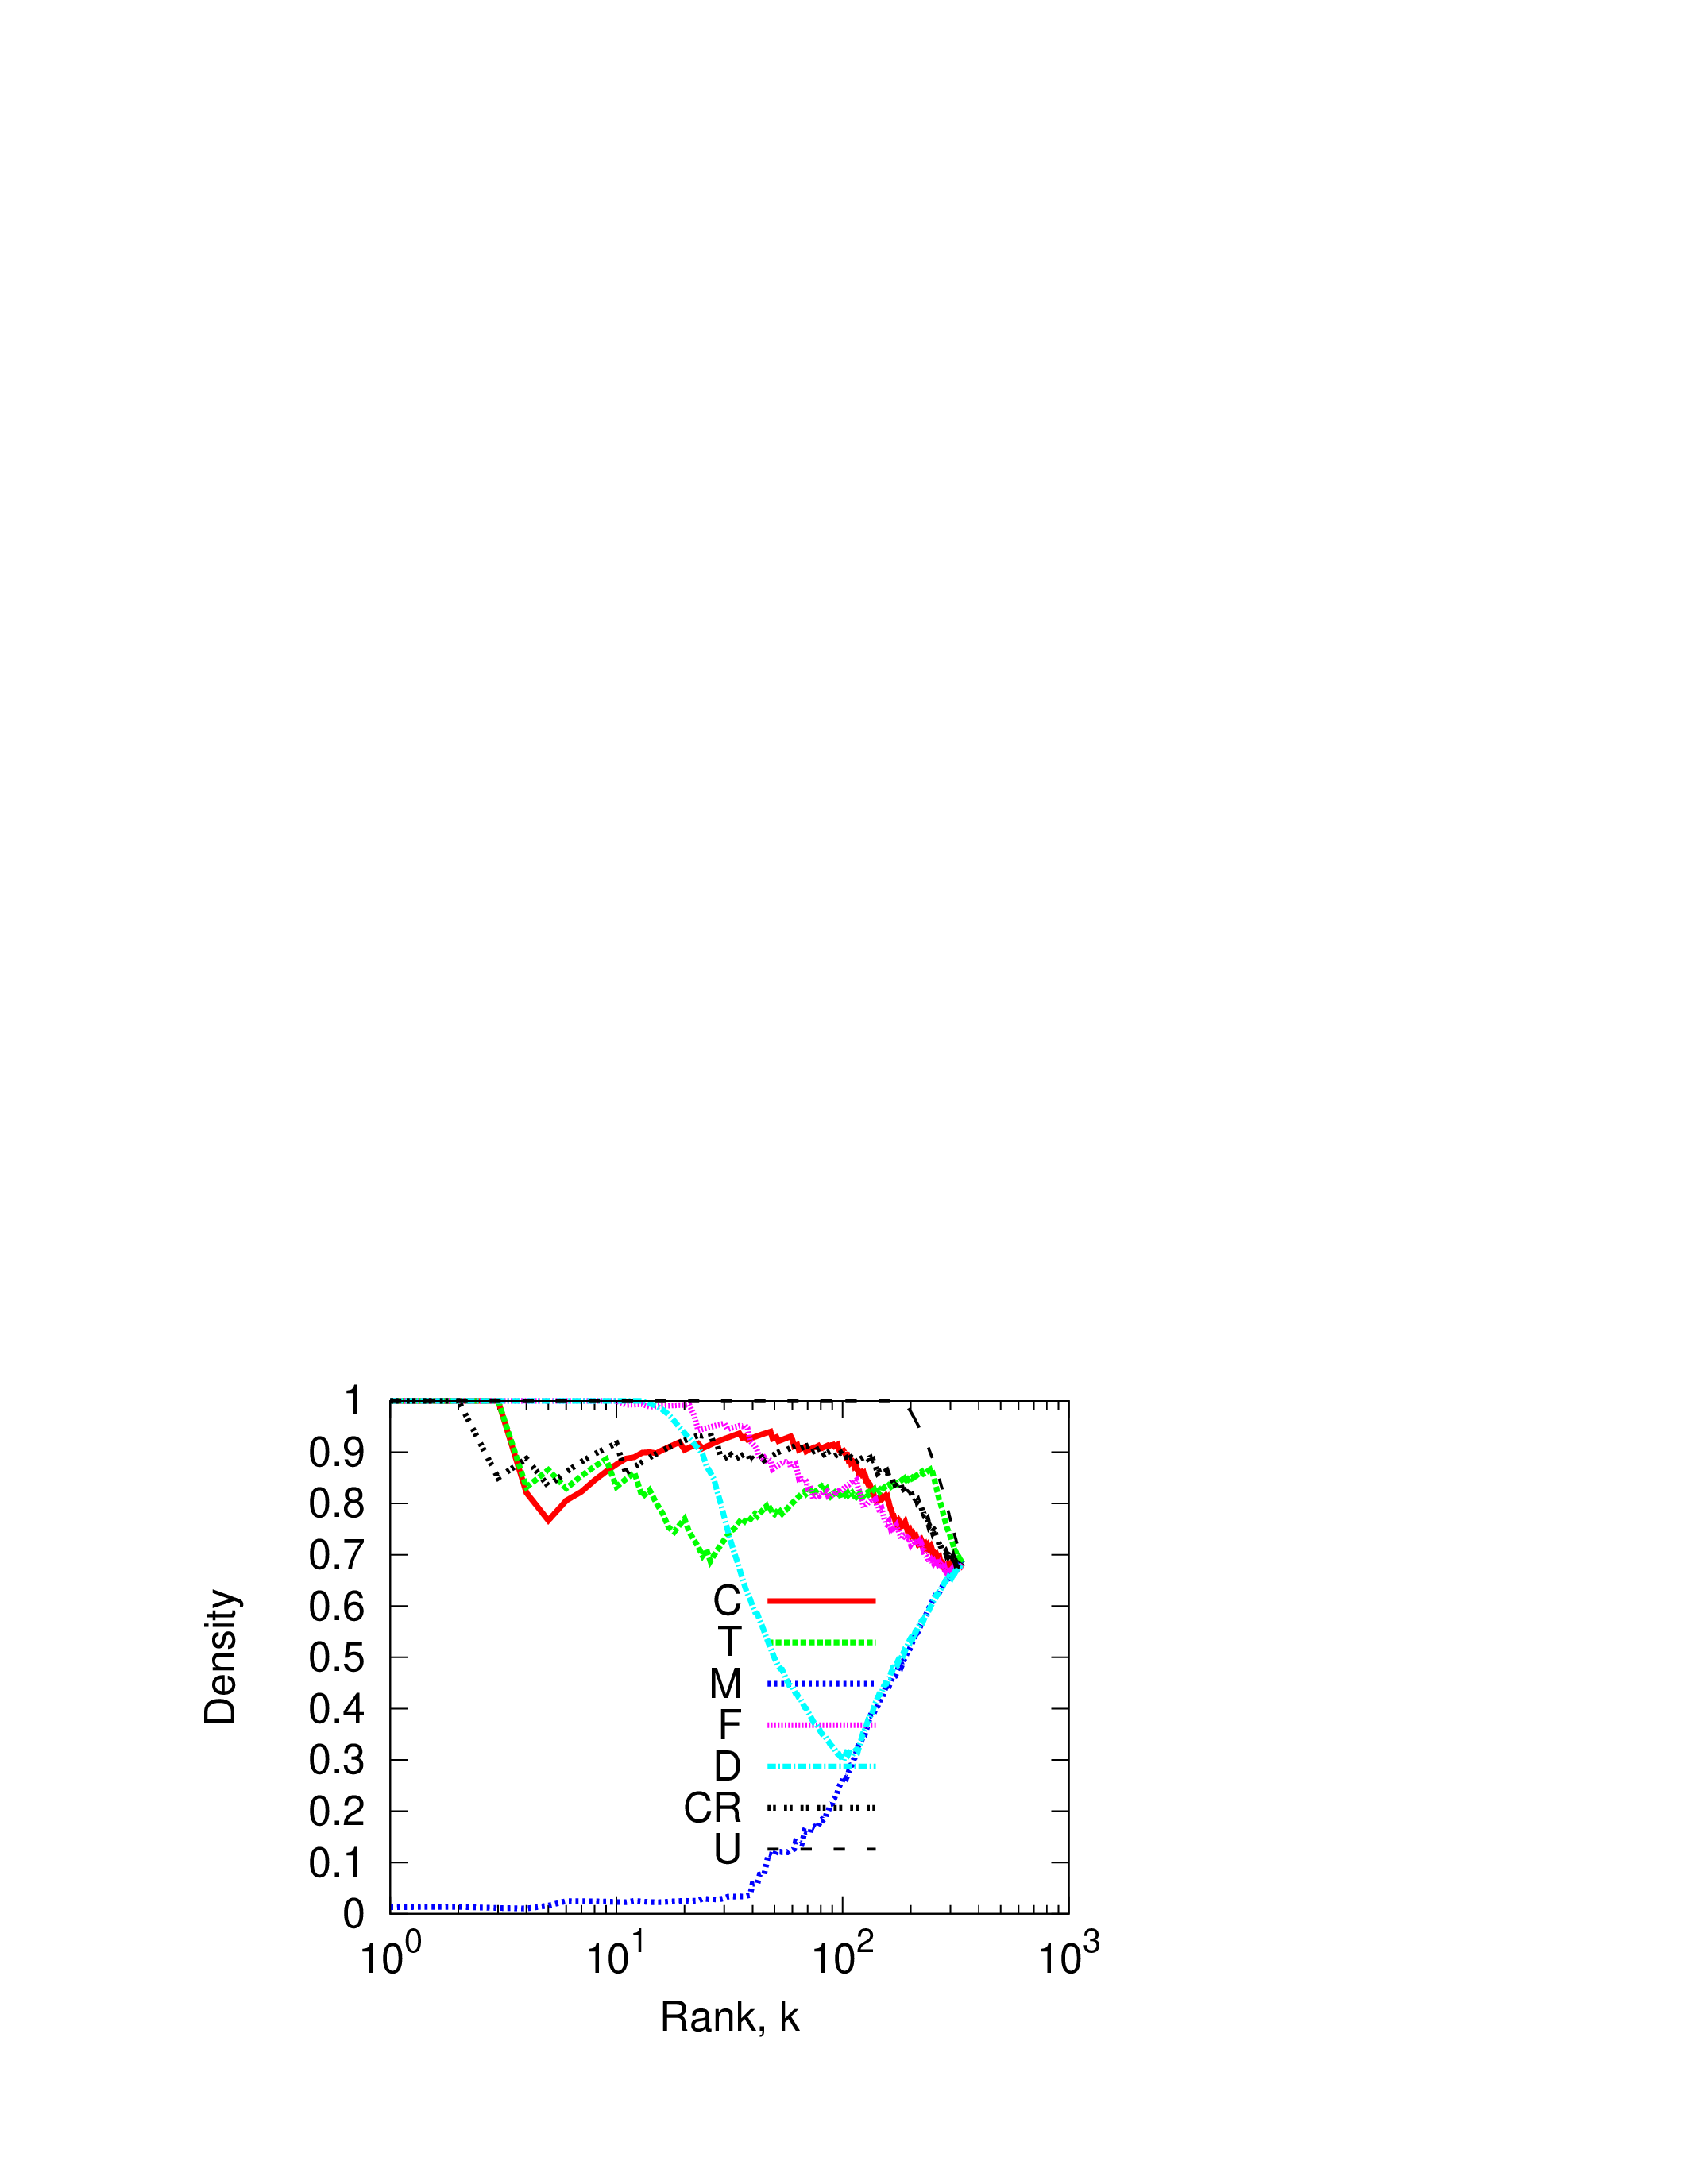}}
	\subfigure[Cohesiveness	(LJ)]{\includegraphics[width=0.185\textwidth]{rank_property.InsidePhi.lj.eps}}
	\subfigure[Cohesiveness	(Ning)]{\includegraphics[width=0.185\textwidth]{rank_property.InsidePhi.Ning.eps}}
	\subfigure[Cohesiveness	 (Amazon)]{\includegraphics[width=0.185\textwidth]{rank_property.InsidePhi.amazon.eps}}
	\subfigure[Cohesiveness	(DBLP)]{\includegraphics[width=0.185\textwidth]{rank_property.InsidePhi.dblp.eps}}
	\subfigure[Cohesiveness	(IMDB)]{\includegraphics[width=0.185\textwidth]{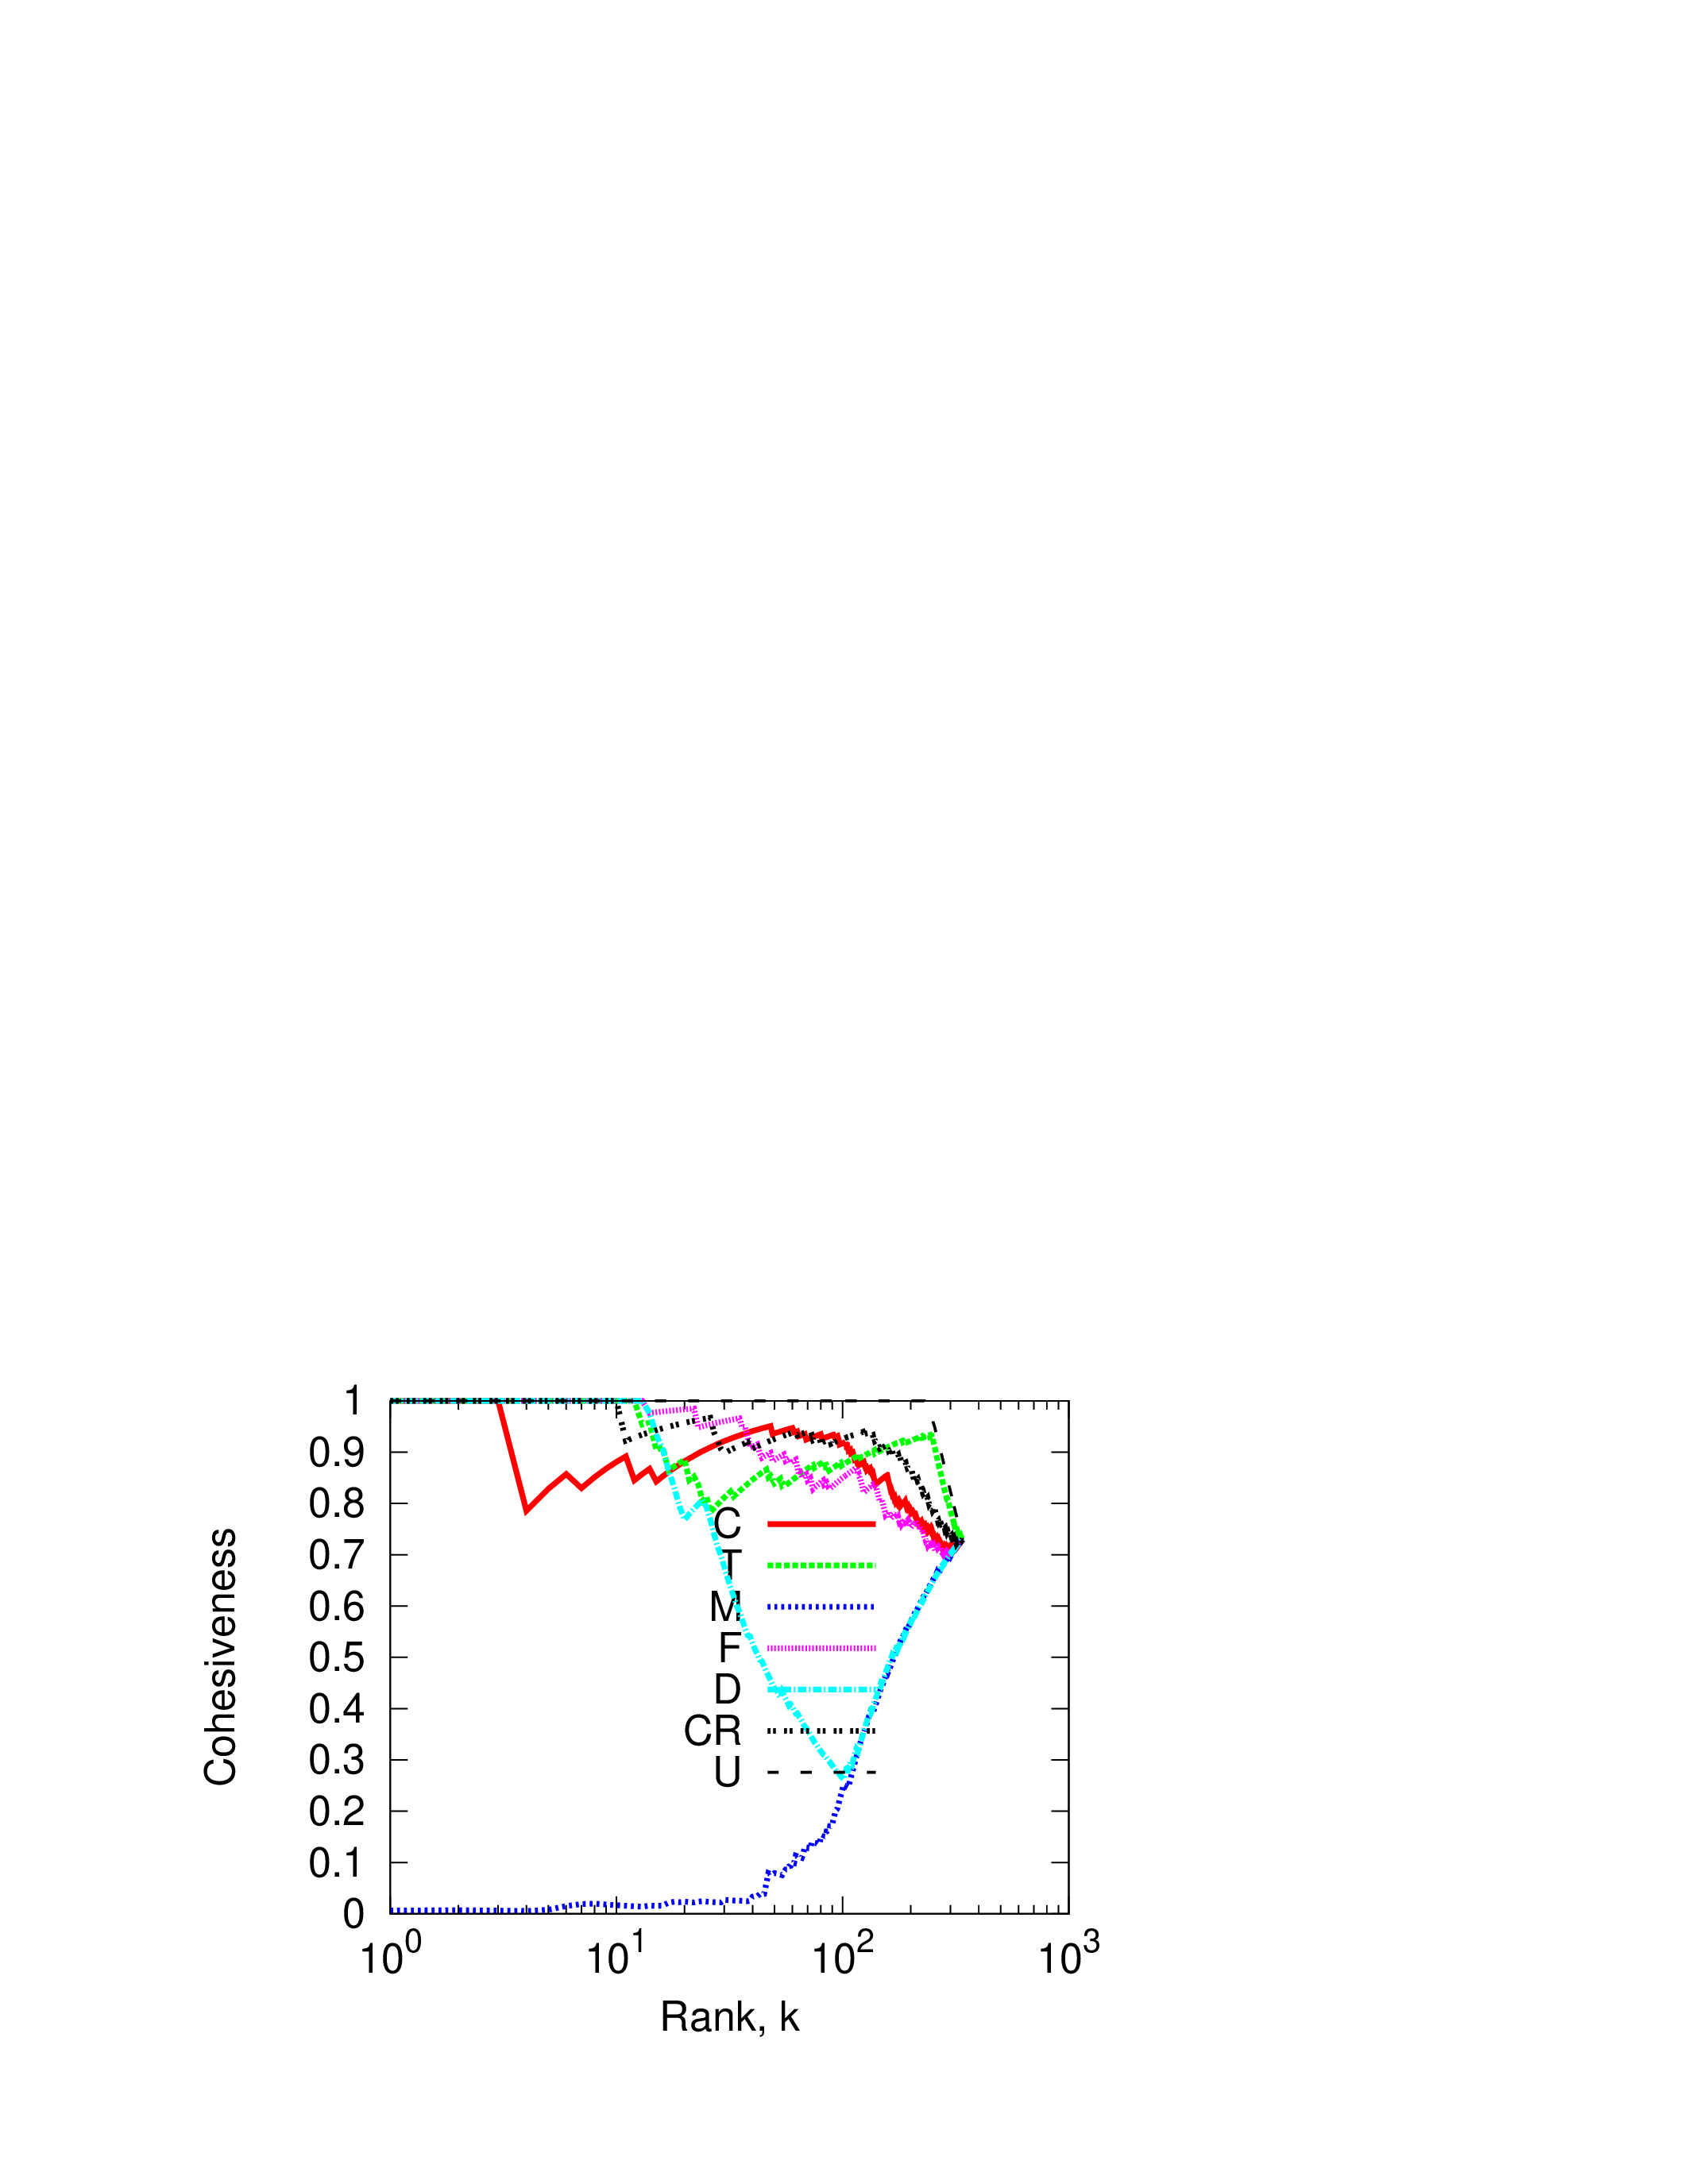}}
	\subfigure[CCF	(LJ)]{\includegraphics[width=0.185\textwidth]{rank_property.CCf.lj.eps}}
	\subfigure[CCF	(Ning)]{\includegraphics[width=0.185\textwidth]{rank_property.CCf.Ning.eps}}
	\subfigure[CCF	(Amazon)]{\includegraphics[width=0.185\textwidth]{rank_property.CCf.amazon.eps}}
	\subfigure[CCF	(DBLP)]{\includegraphics[width=0.185\textwidth]{rank_property.CCf.dblp.eps}}
	\subfigure[CCF	(IMDB)]{\includegraphics[width=0.185\textwidth]{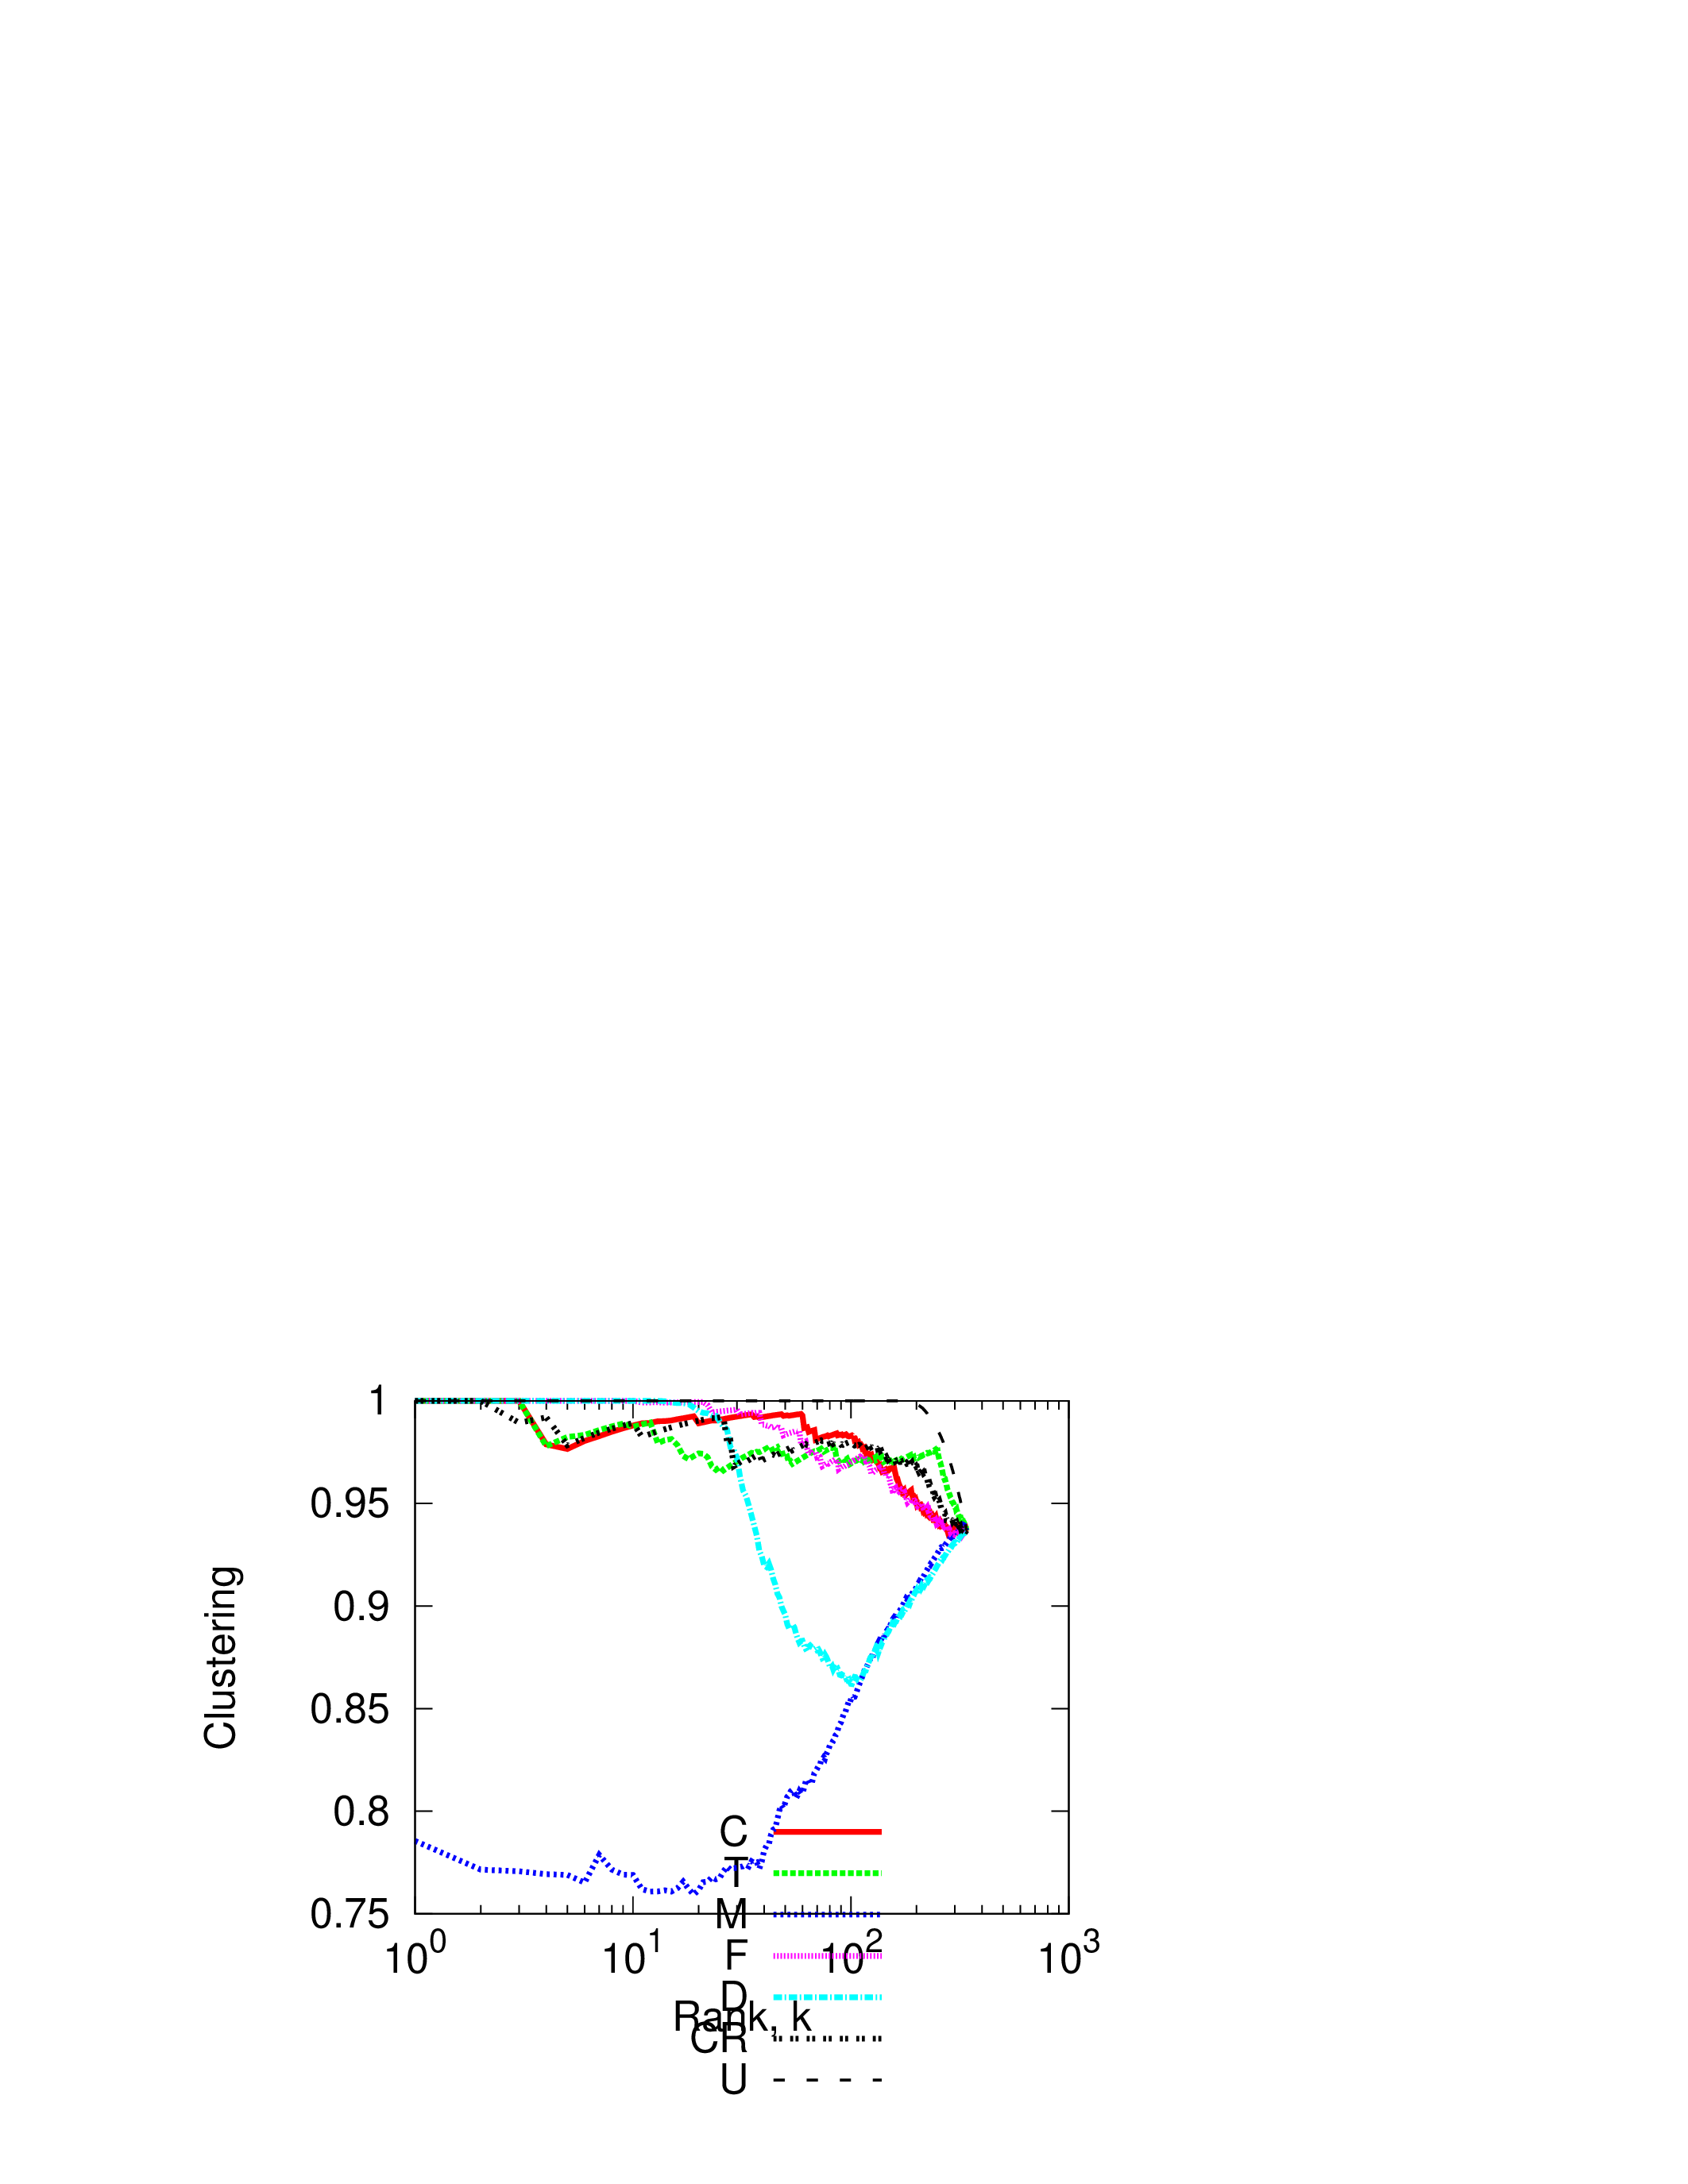}}
    \caption{Cumulative average of goodness metrics for the communities in each data set, ranked by each of the six community scoring functions. Scoring functions, like Conductance (C) and TPR (T), with high and monotonically decreasing values perform best.}
\label{fig:full.avgrank}
\end{figure*}

\begin{figure*}[t]
	\centering
	\subfigure[NodeSwap	(LJ)]{\includegraphics[width=0.185\textwidth]{sens.NodeSwap.lj.eps}}
	\subfigure[NodeSwap	(Ning)]{\includegraphics[width=0.185\textwidth]{sens.NodeSwap.Ning.eps}}
	\subfigure[NodeSwap	(Amazon)]{\includegraphics[width=0.185\textwidth]{sens.NodeSwap.amazon.eps}}
	\subfigure[NodeSwap	(DBLP)]{\includegraphics[width=0.185\textwidth]{sens.NodeSwap.dblp.eps}}
	\subfigure[NodeSwap	(IMDB)]{\includegraphics[width=0.185\textwidth]{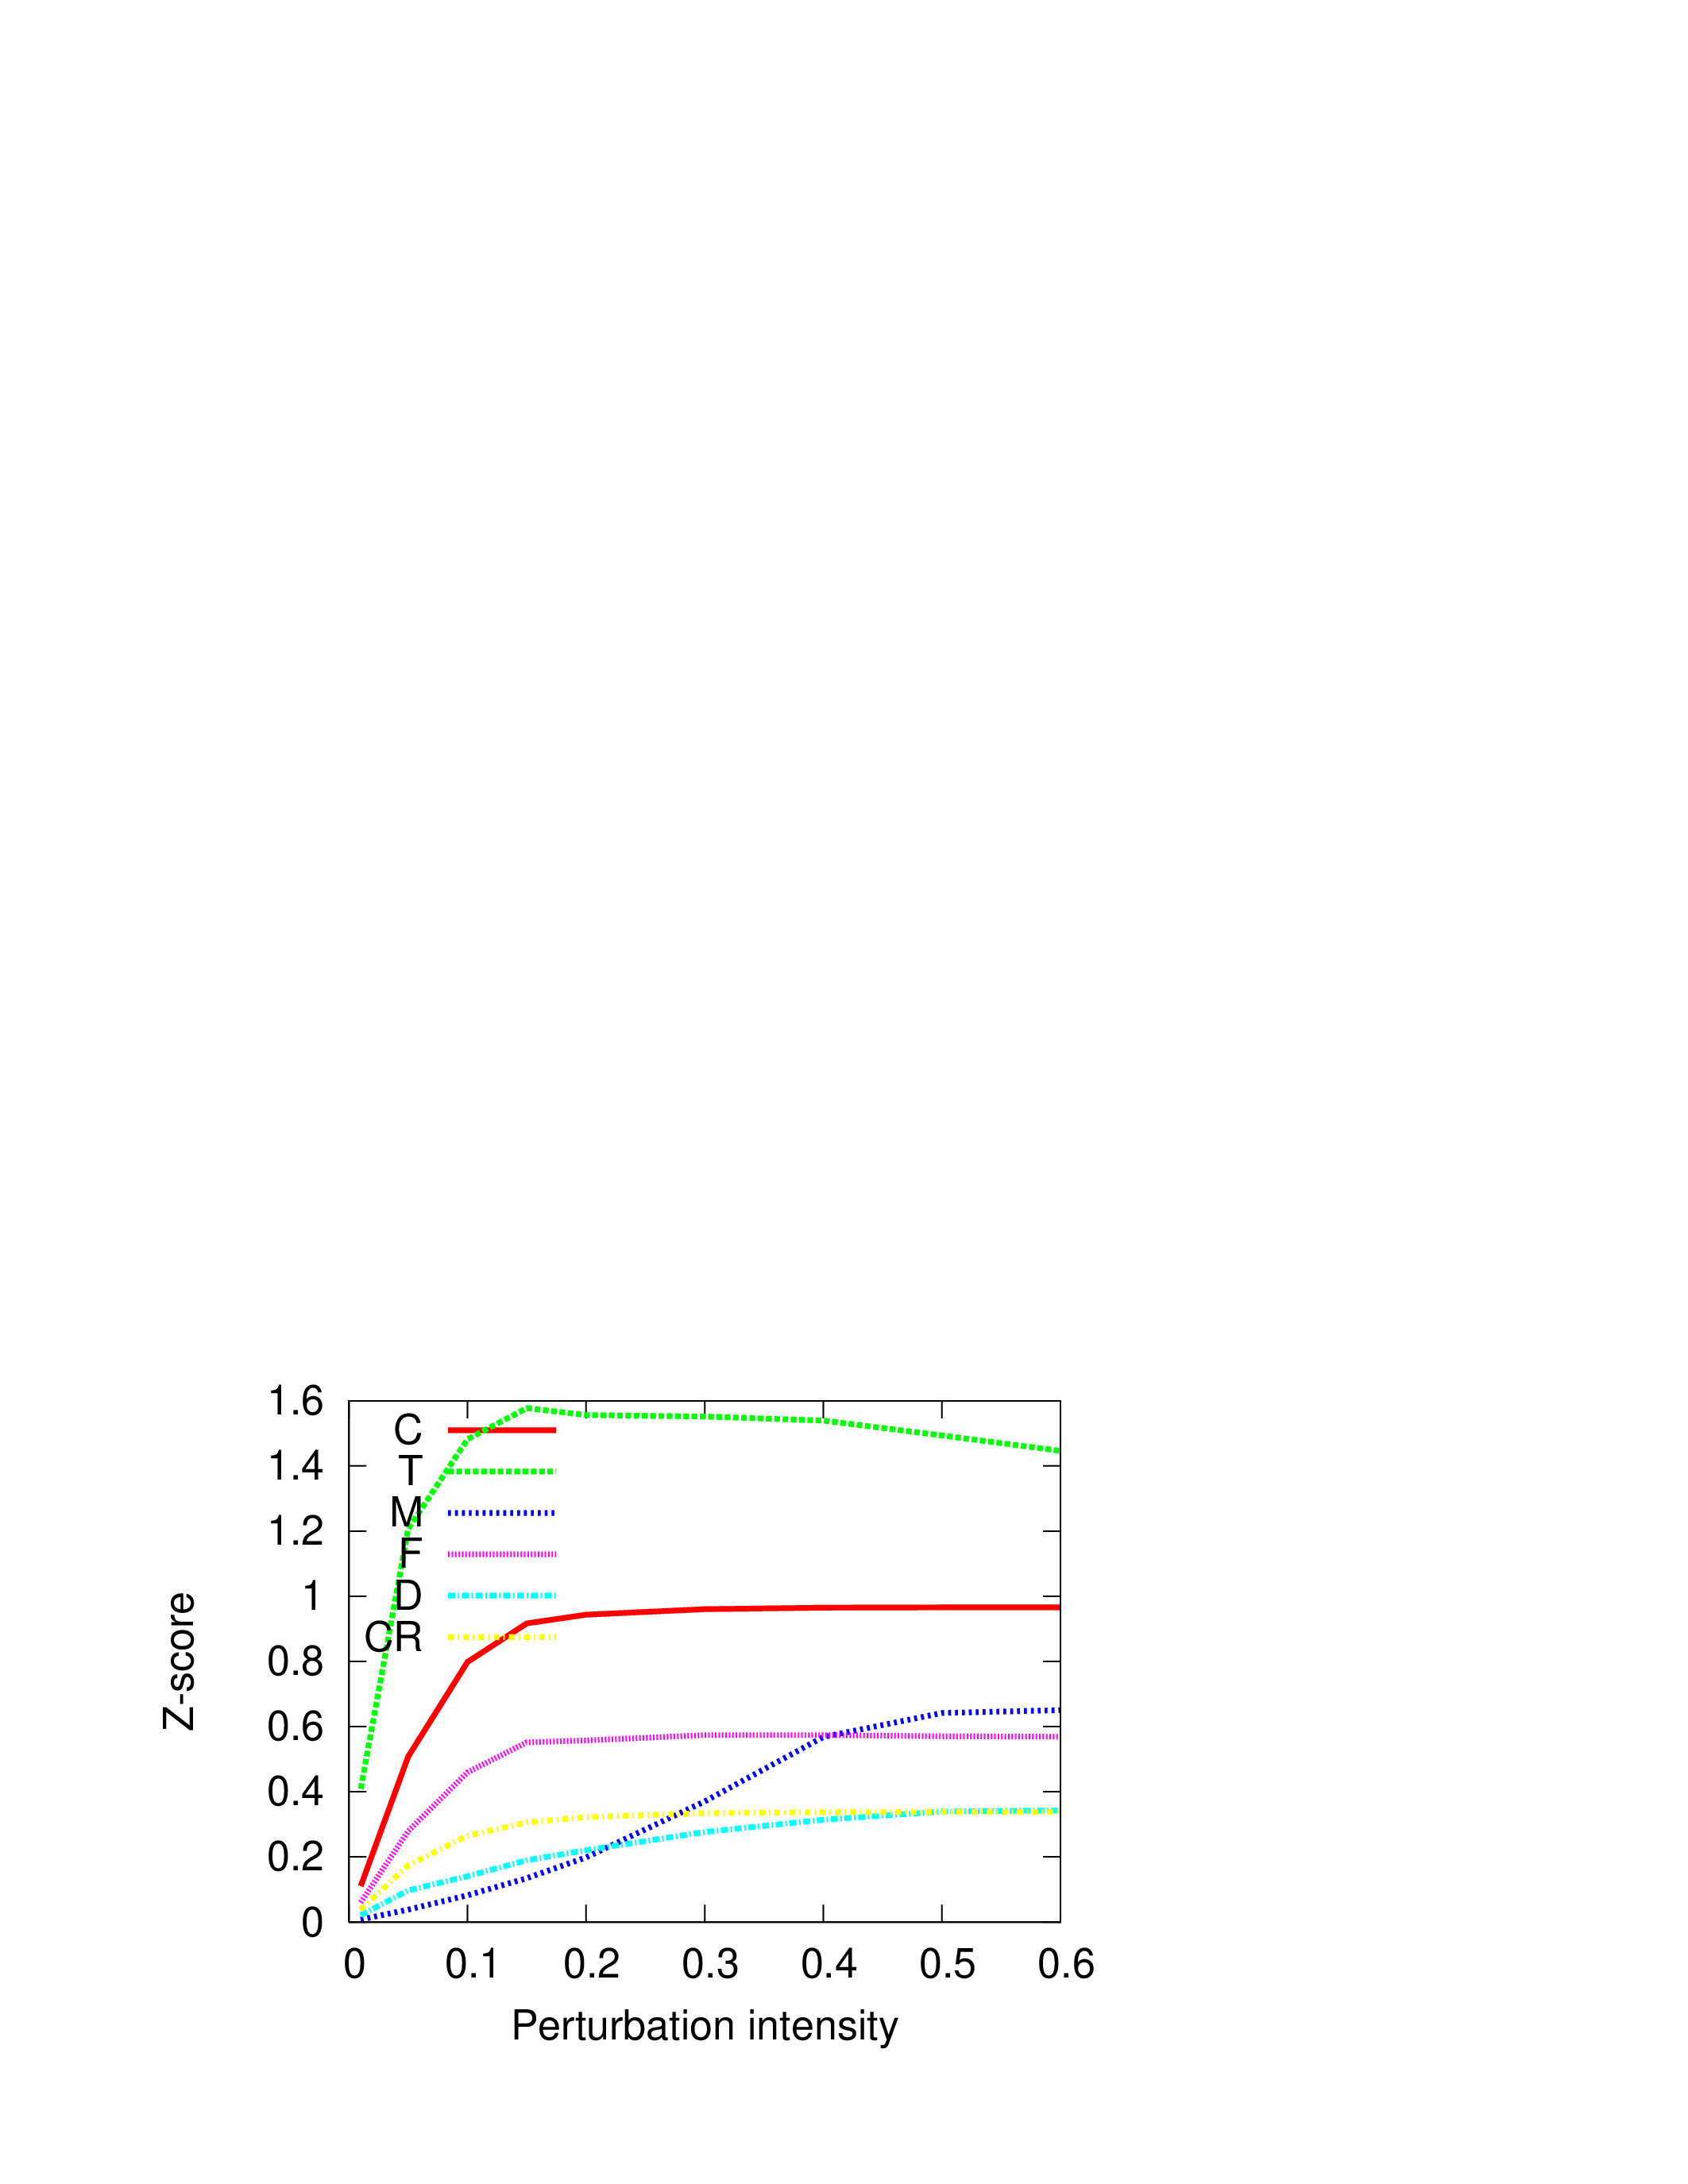}}
	\subfigure[Random	(LJ)]{\includegraphics[width=0.185\textwidth]{sens.Random.lj.eps}}
	\subfigure[Random	(Ning)]{\includegraphics[width=0.185\textwidth]{sens.Random.Ning.eps}}
	\subfigure[Random	(Amazon)]{\includegraphics[width=0.185\textwidth]{sens.Random.amazon.eps}}
	\subfigure[Random	(DBLP)]{\includegraphics[width=0.185\textwidth]{sens.Random.dblp.eps}}
	\subfigure[Random	(IMDB)]{\includegraphics[width=0.185\textwidth]{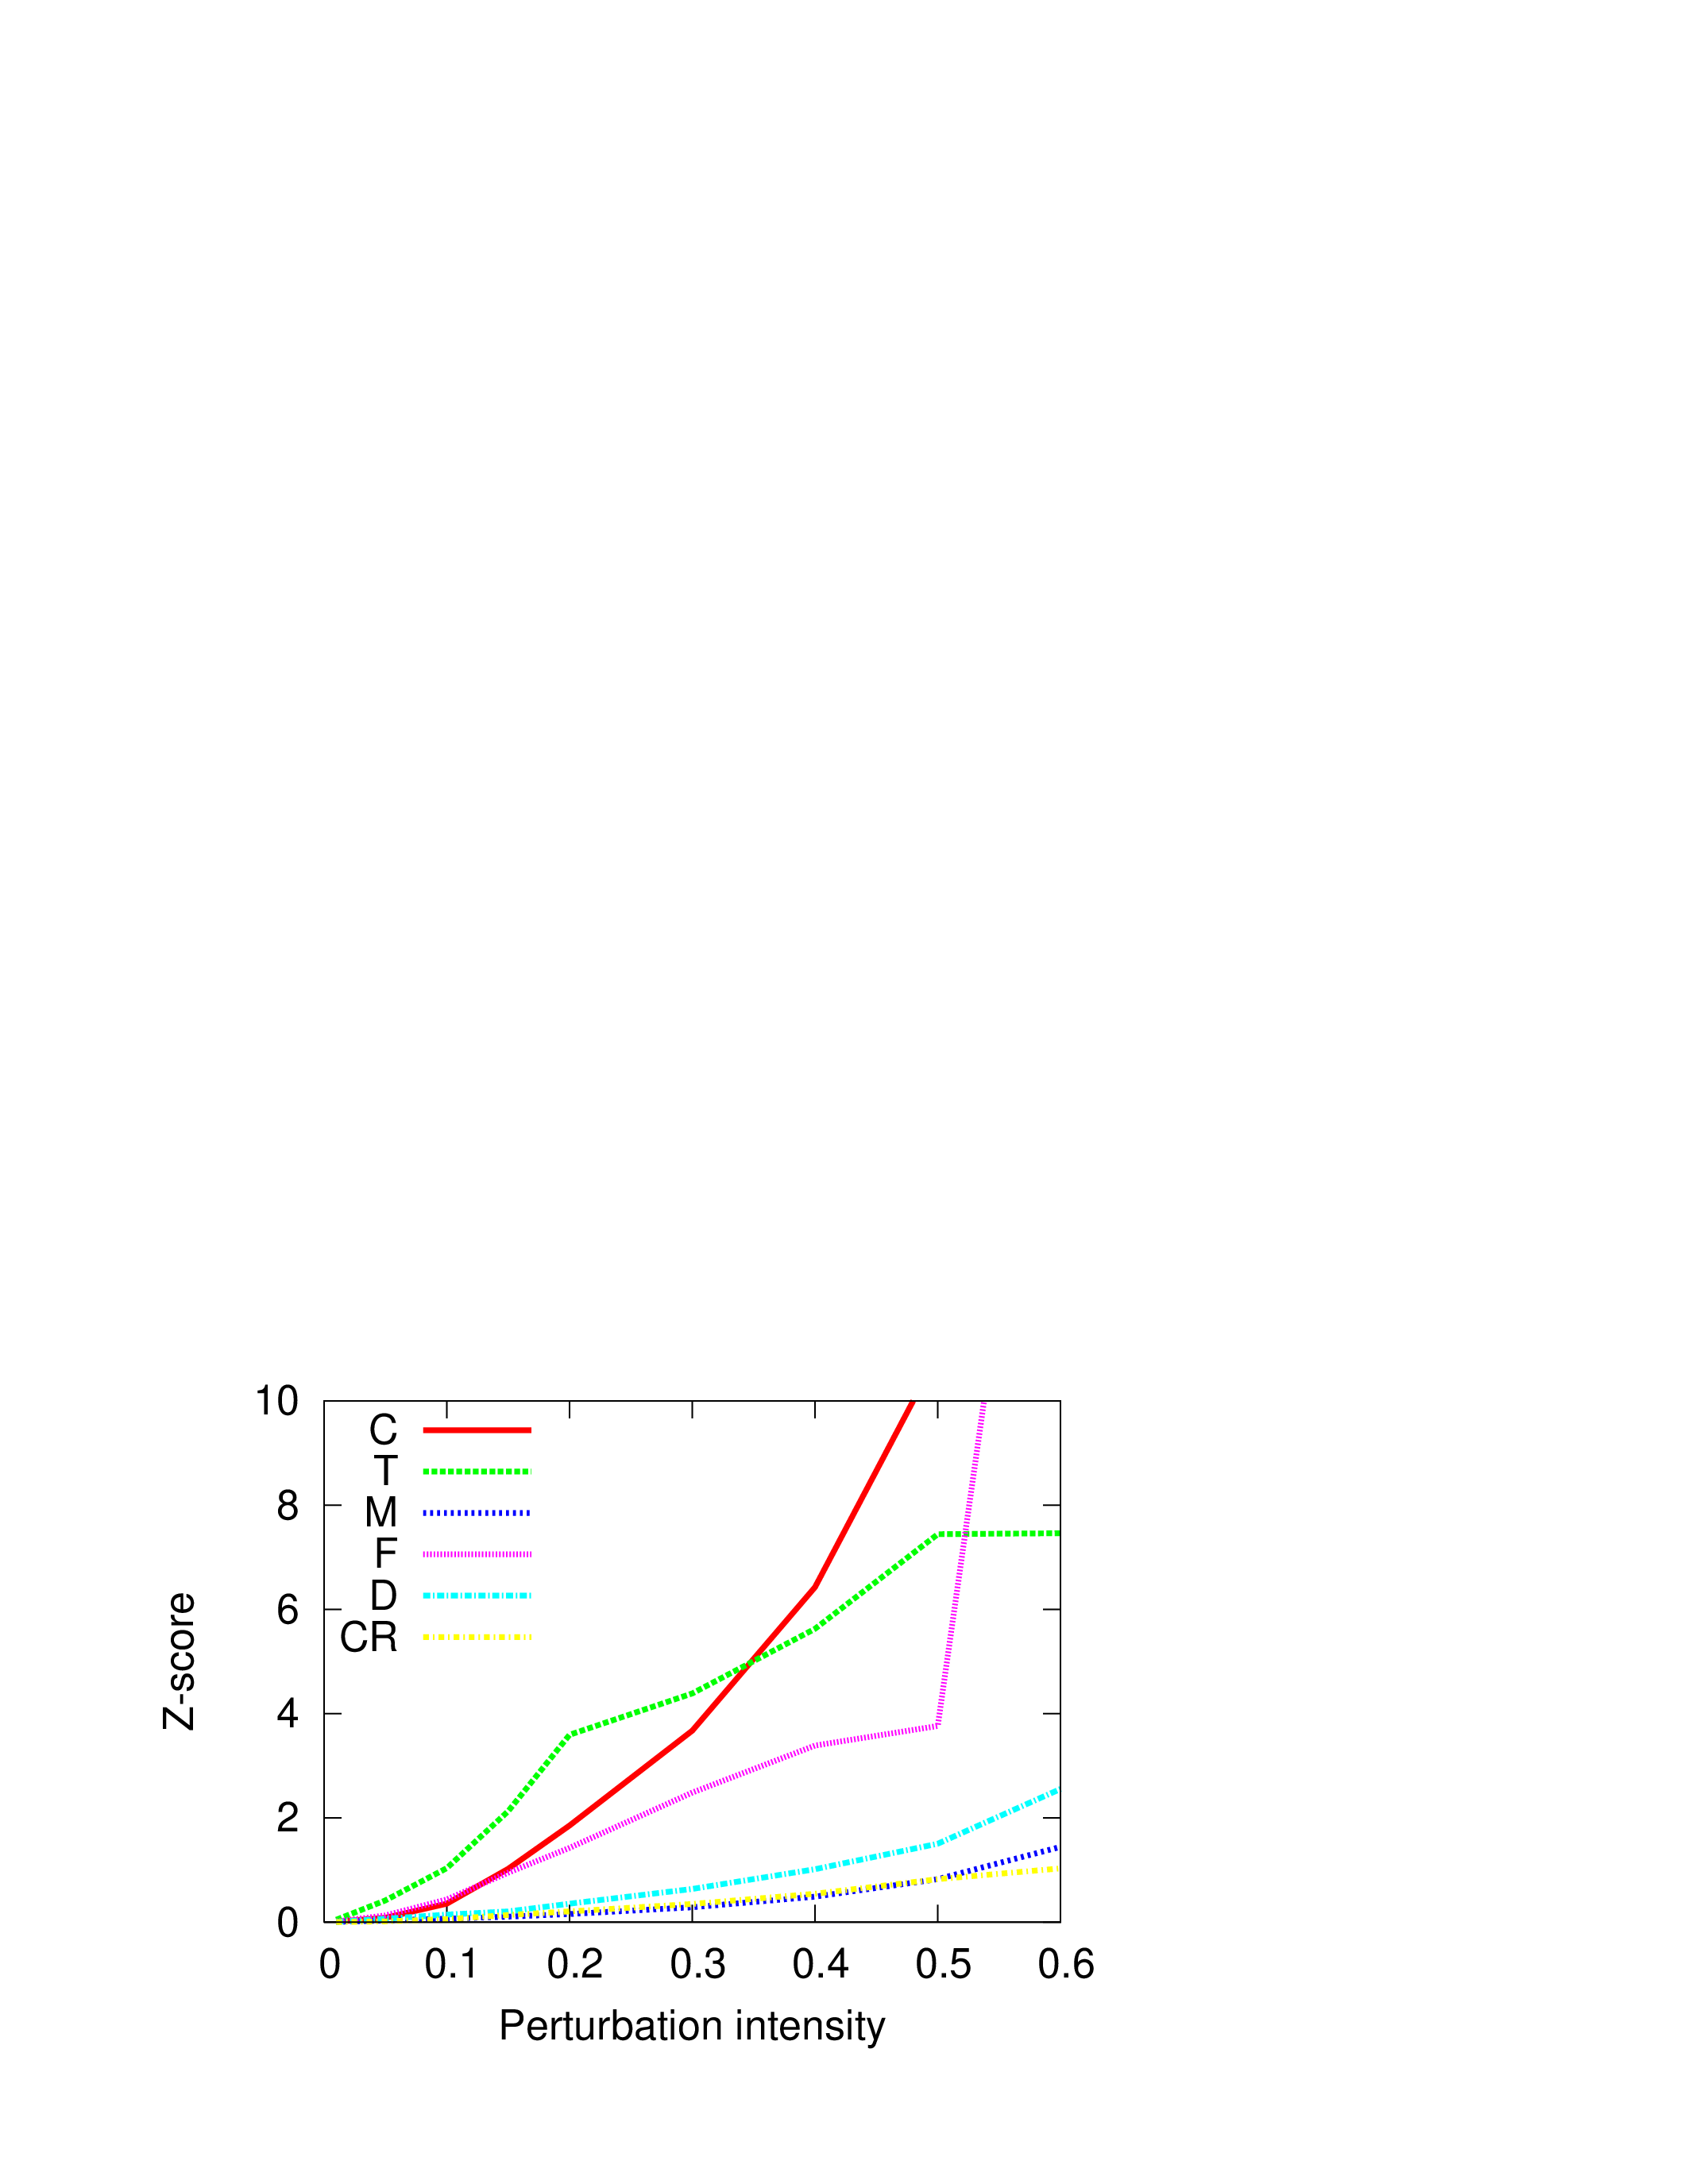}}
	\subfigure[Expand	(LJ)]{\includegraphics[width=0.185\textwidth]{sens.Expand.lj.eps}}
	\subfigure[Expand	(Ning)]{\includegraphics[width=0.185\textwidth]{sens.Expand.Ning.eps}}
	\subfigure[Expand	(Amazon)]{\includegraphics[width=0.185\textwidth]{sens.Expand.amazon.eps}}
	\subfigure[Expand	(DBLP)]{\includegraphics[width=0.185\textwidth]{sens.Expand.dblp.eps}}
	\subfigure[Expand	(IMDB)]{\includegraphics[width=0.185\textwidth]{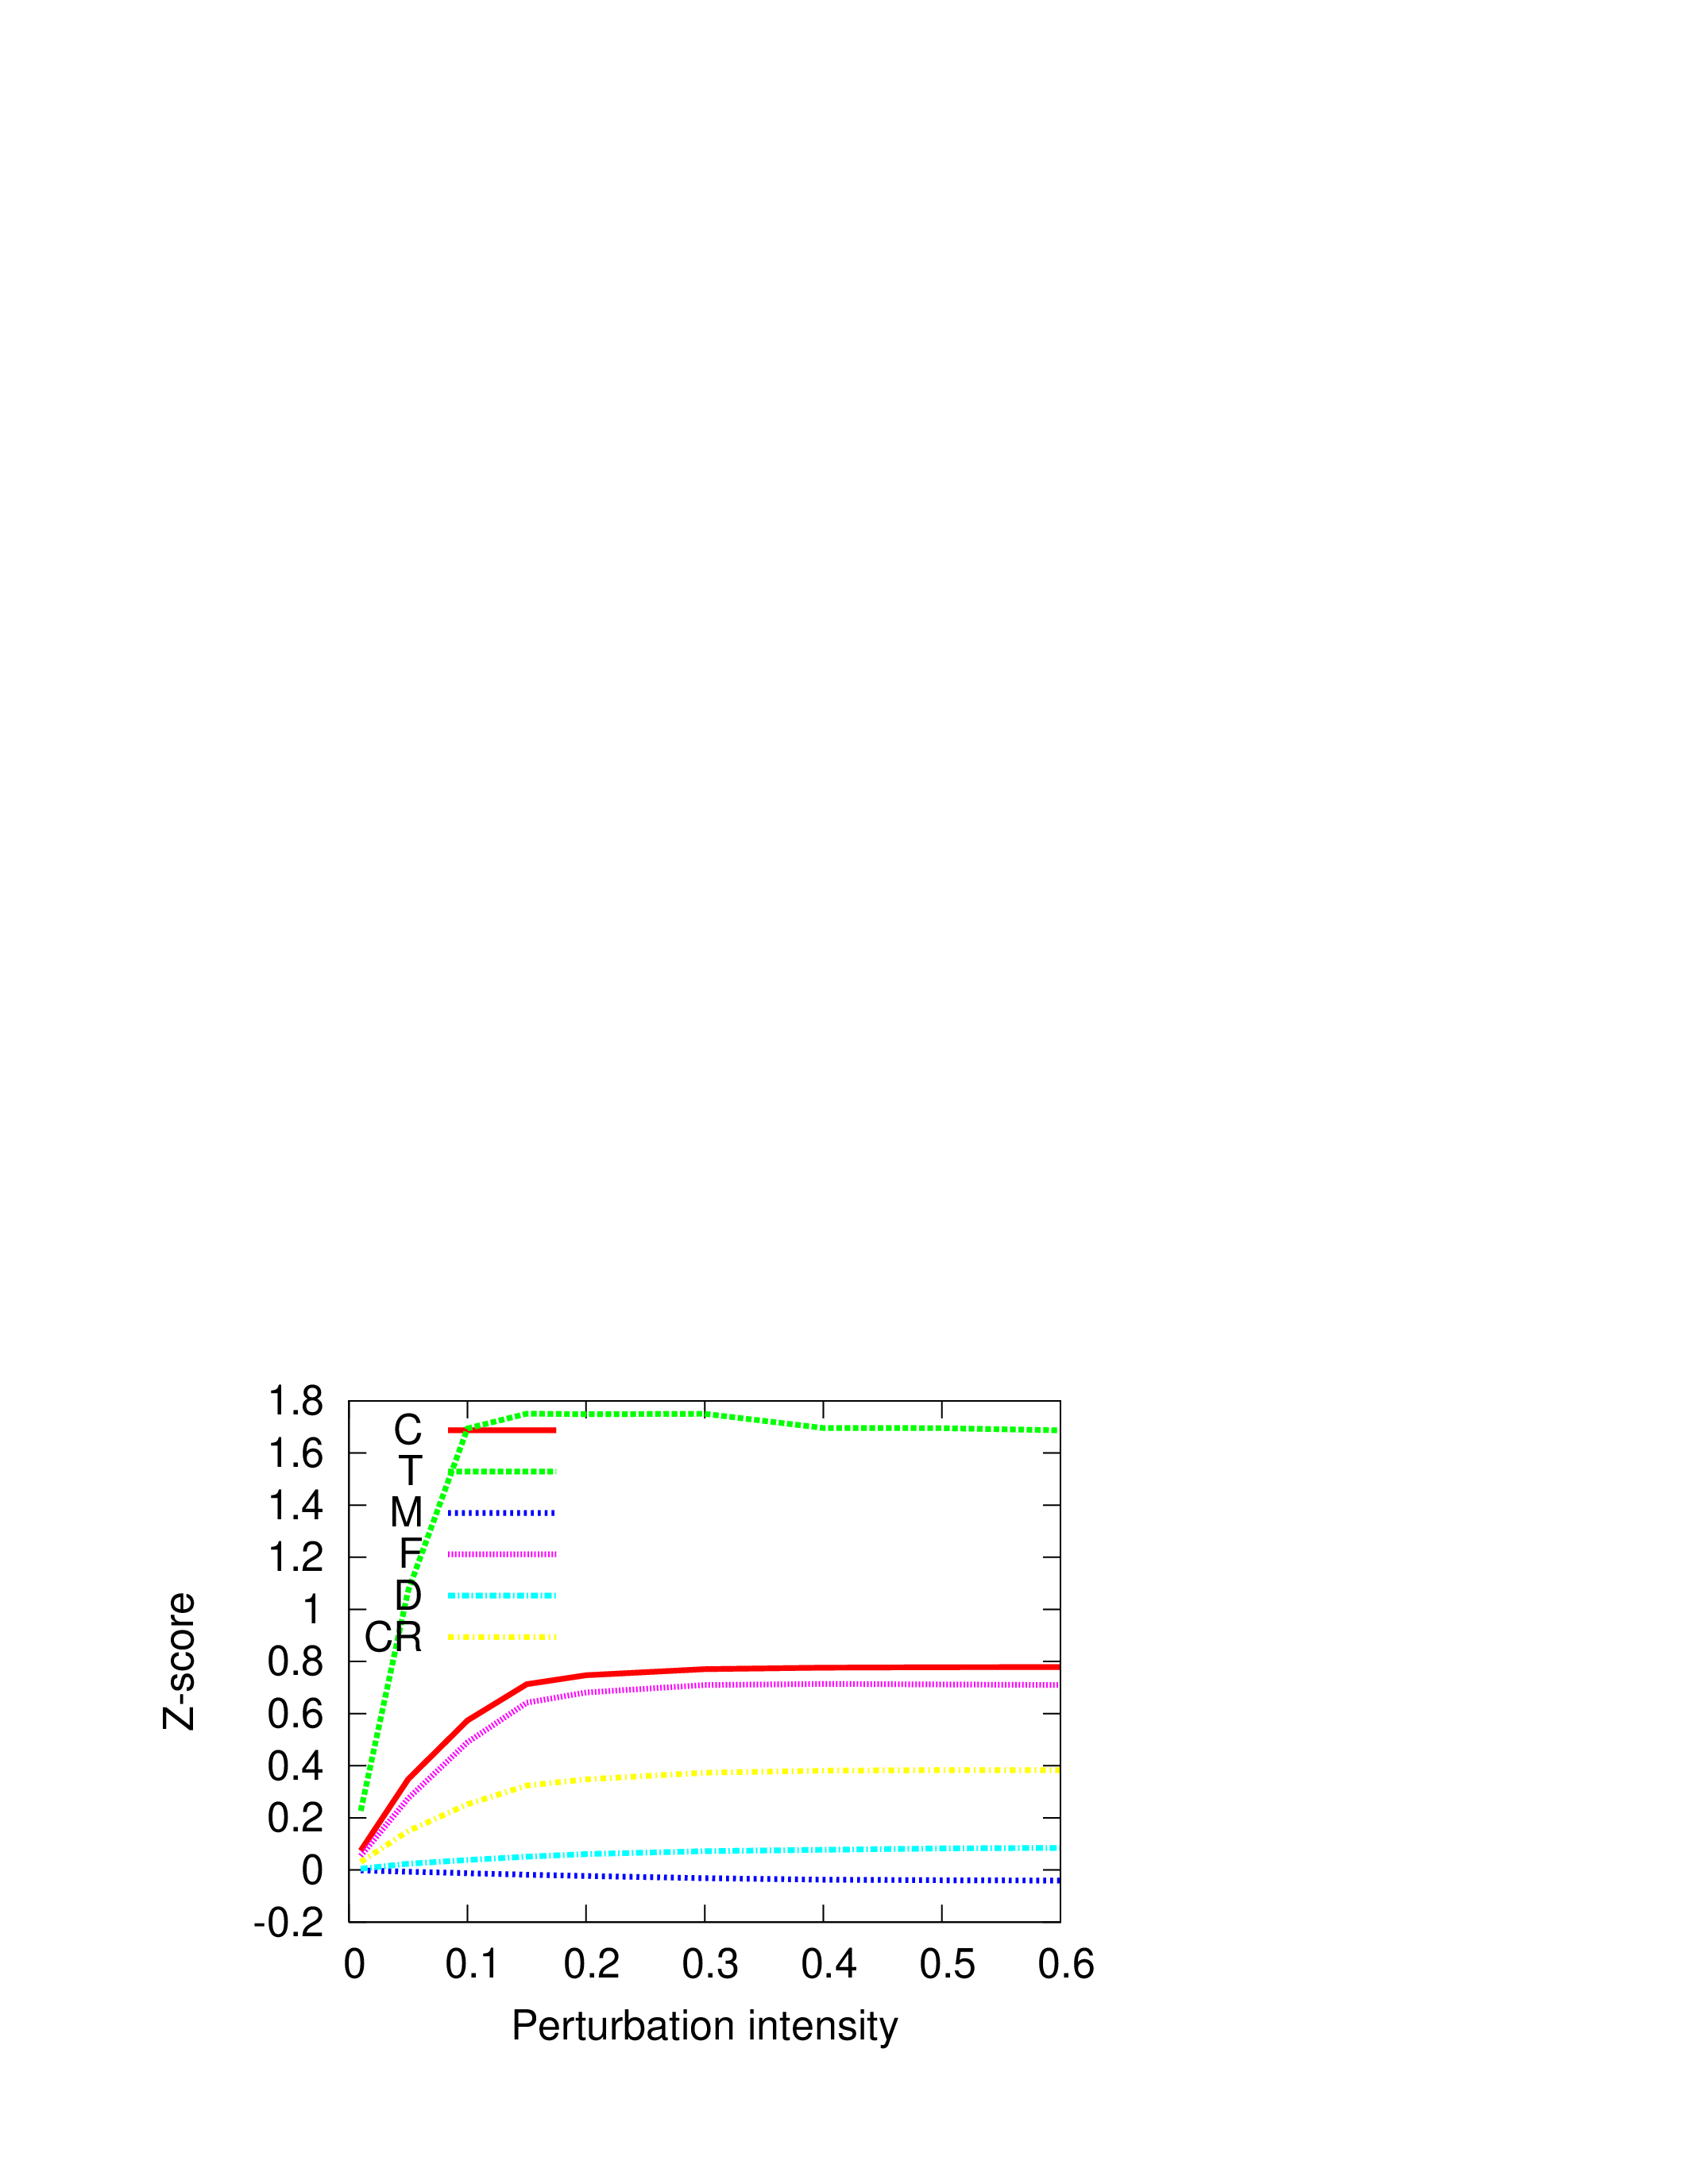}}
	\subfigure[Shrink	(LJ)]{\includegraphics[width=0.185\textwidth]{sens.Shrink.lj.eps}}
	\subfigure[Shrink	(Ning)]{\includegraphics[width=0.185\textwidth]{sens.Shrink.Ning.eps}}
	\subfigure[Shrink	(Amazon)]{\includegraphics[width=0.185\textwidth]{sens.Shrink.amazon.eps}}
	\subfigure[Shrink	(DBLP)]{\includegraphics[width=0.185\textwidth]{sens.Shrink.dblp.eps}}
	\subfigure[Shrink	(IMDB)]{\includegraphics[width=0.185\textwidth]{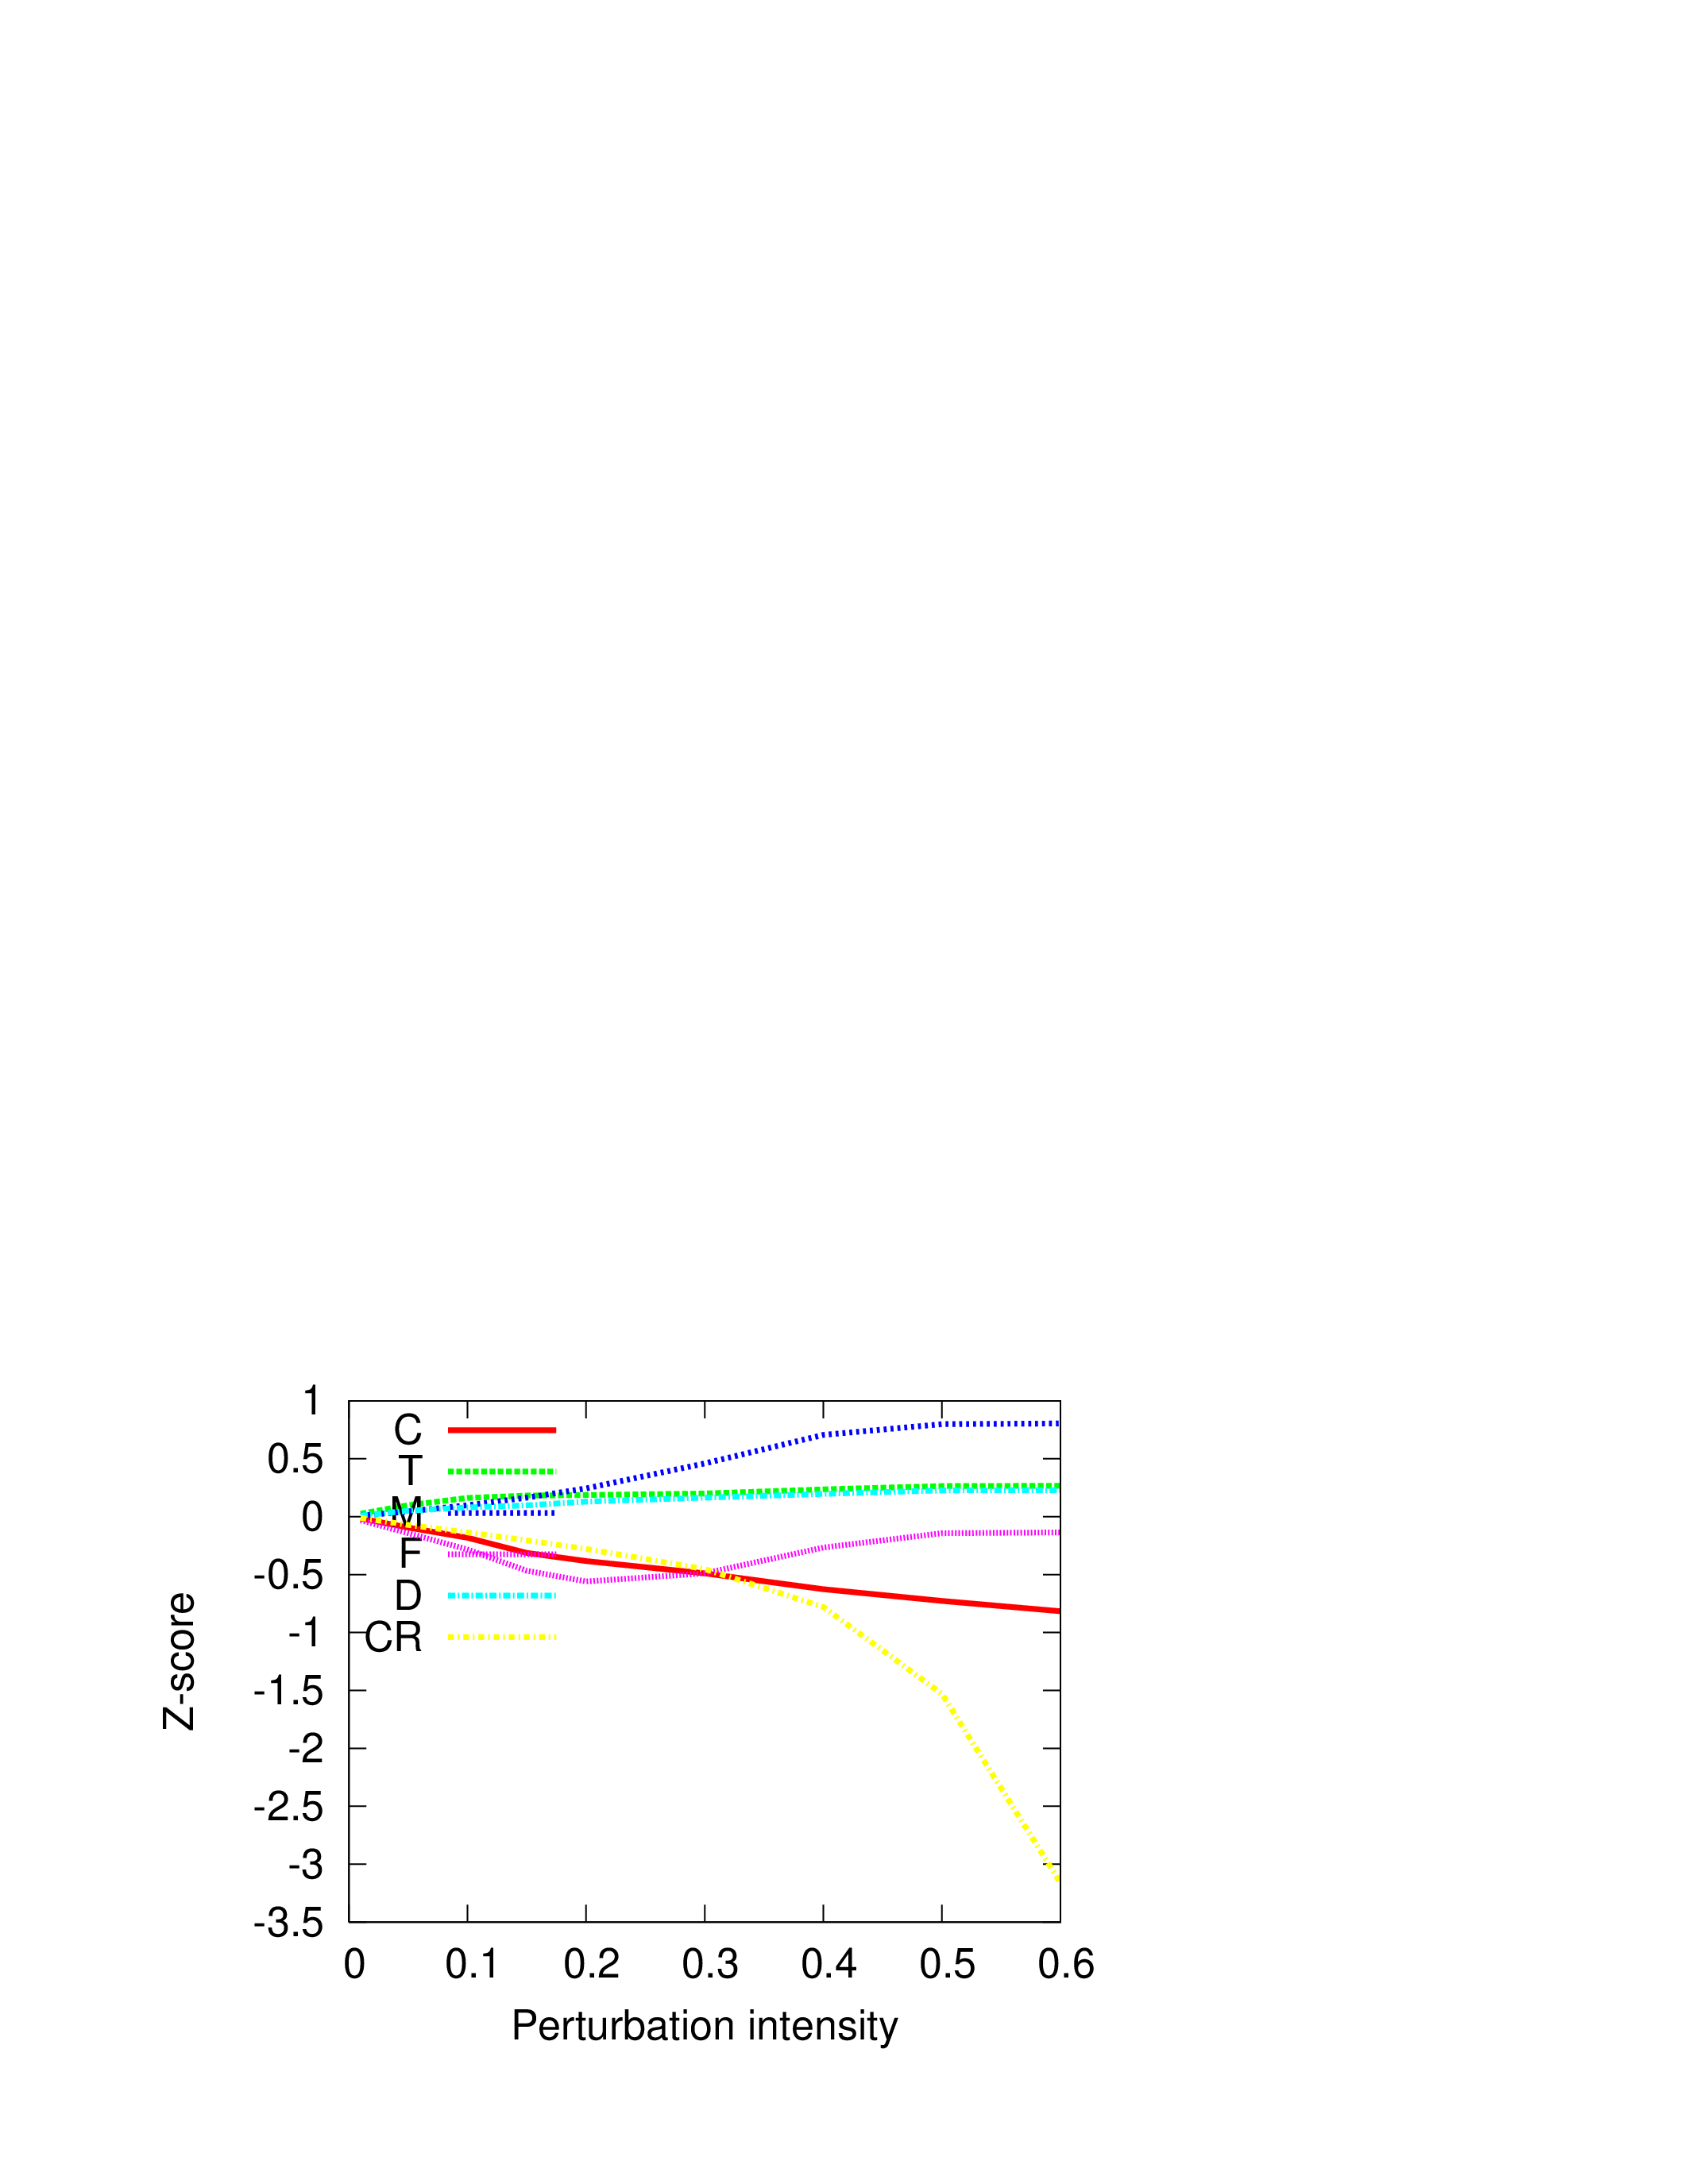}}
	\caption{Z-scores as a function of the perturbation intensity of each of the 6 scoring functions for the LiveJournal communities. Conductance (C) and Triad participation ratio (T) best detect random perturbations of community.}
\label{fig:full.Sensitivity}
\end{figure*}

\begin{figure*}[t]
	\centering
	\subfigure[NodeSwap	(LJ)]{\includegraphics[width=0.185\textwidth]{zscore.sz.NodeSwap.lj.eps}}
	\subfigure[NodeSwap	(Ning)]{\includegraphics[width=0.185\textwidth]{zscore.sz.NodeSwap.Ning.eps}}
	\subfigure[NodeSwap	(Amazon)]{\includegraphics[width=0.185\textwidth]{zscore.sz.NodeSwap.amazon.eps}}
	\subfigure[NodeSwap	(DBLP)]{\includegraphics[width=0.185\textwidth]{zscore.sz.NodeSwap.dblp.eps}}
	\subfigure[NodeSwap	(IMDB)]{\includegraphics[width=0.185\textwidth]{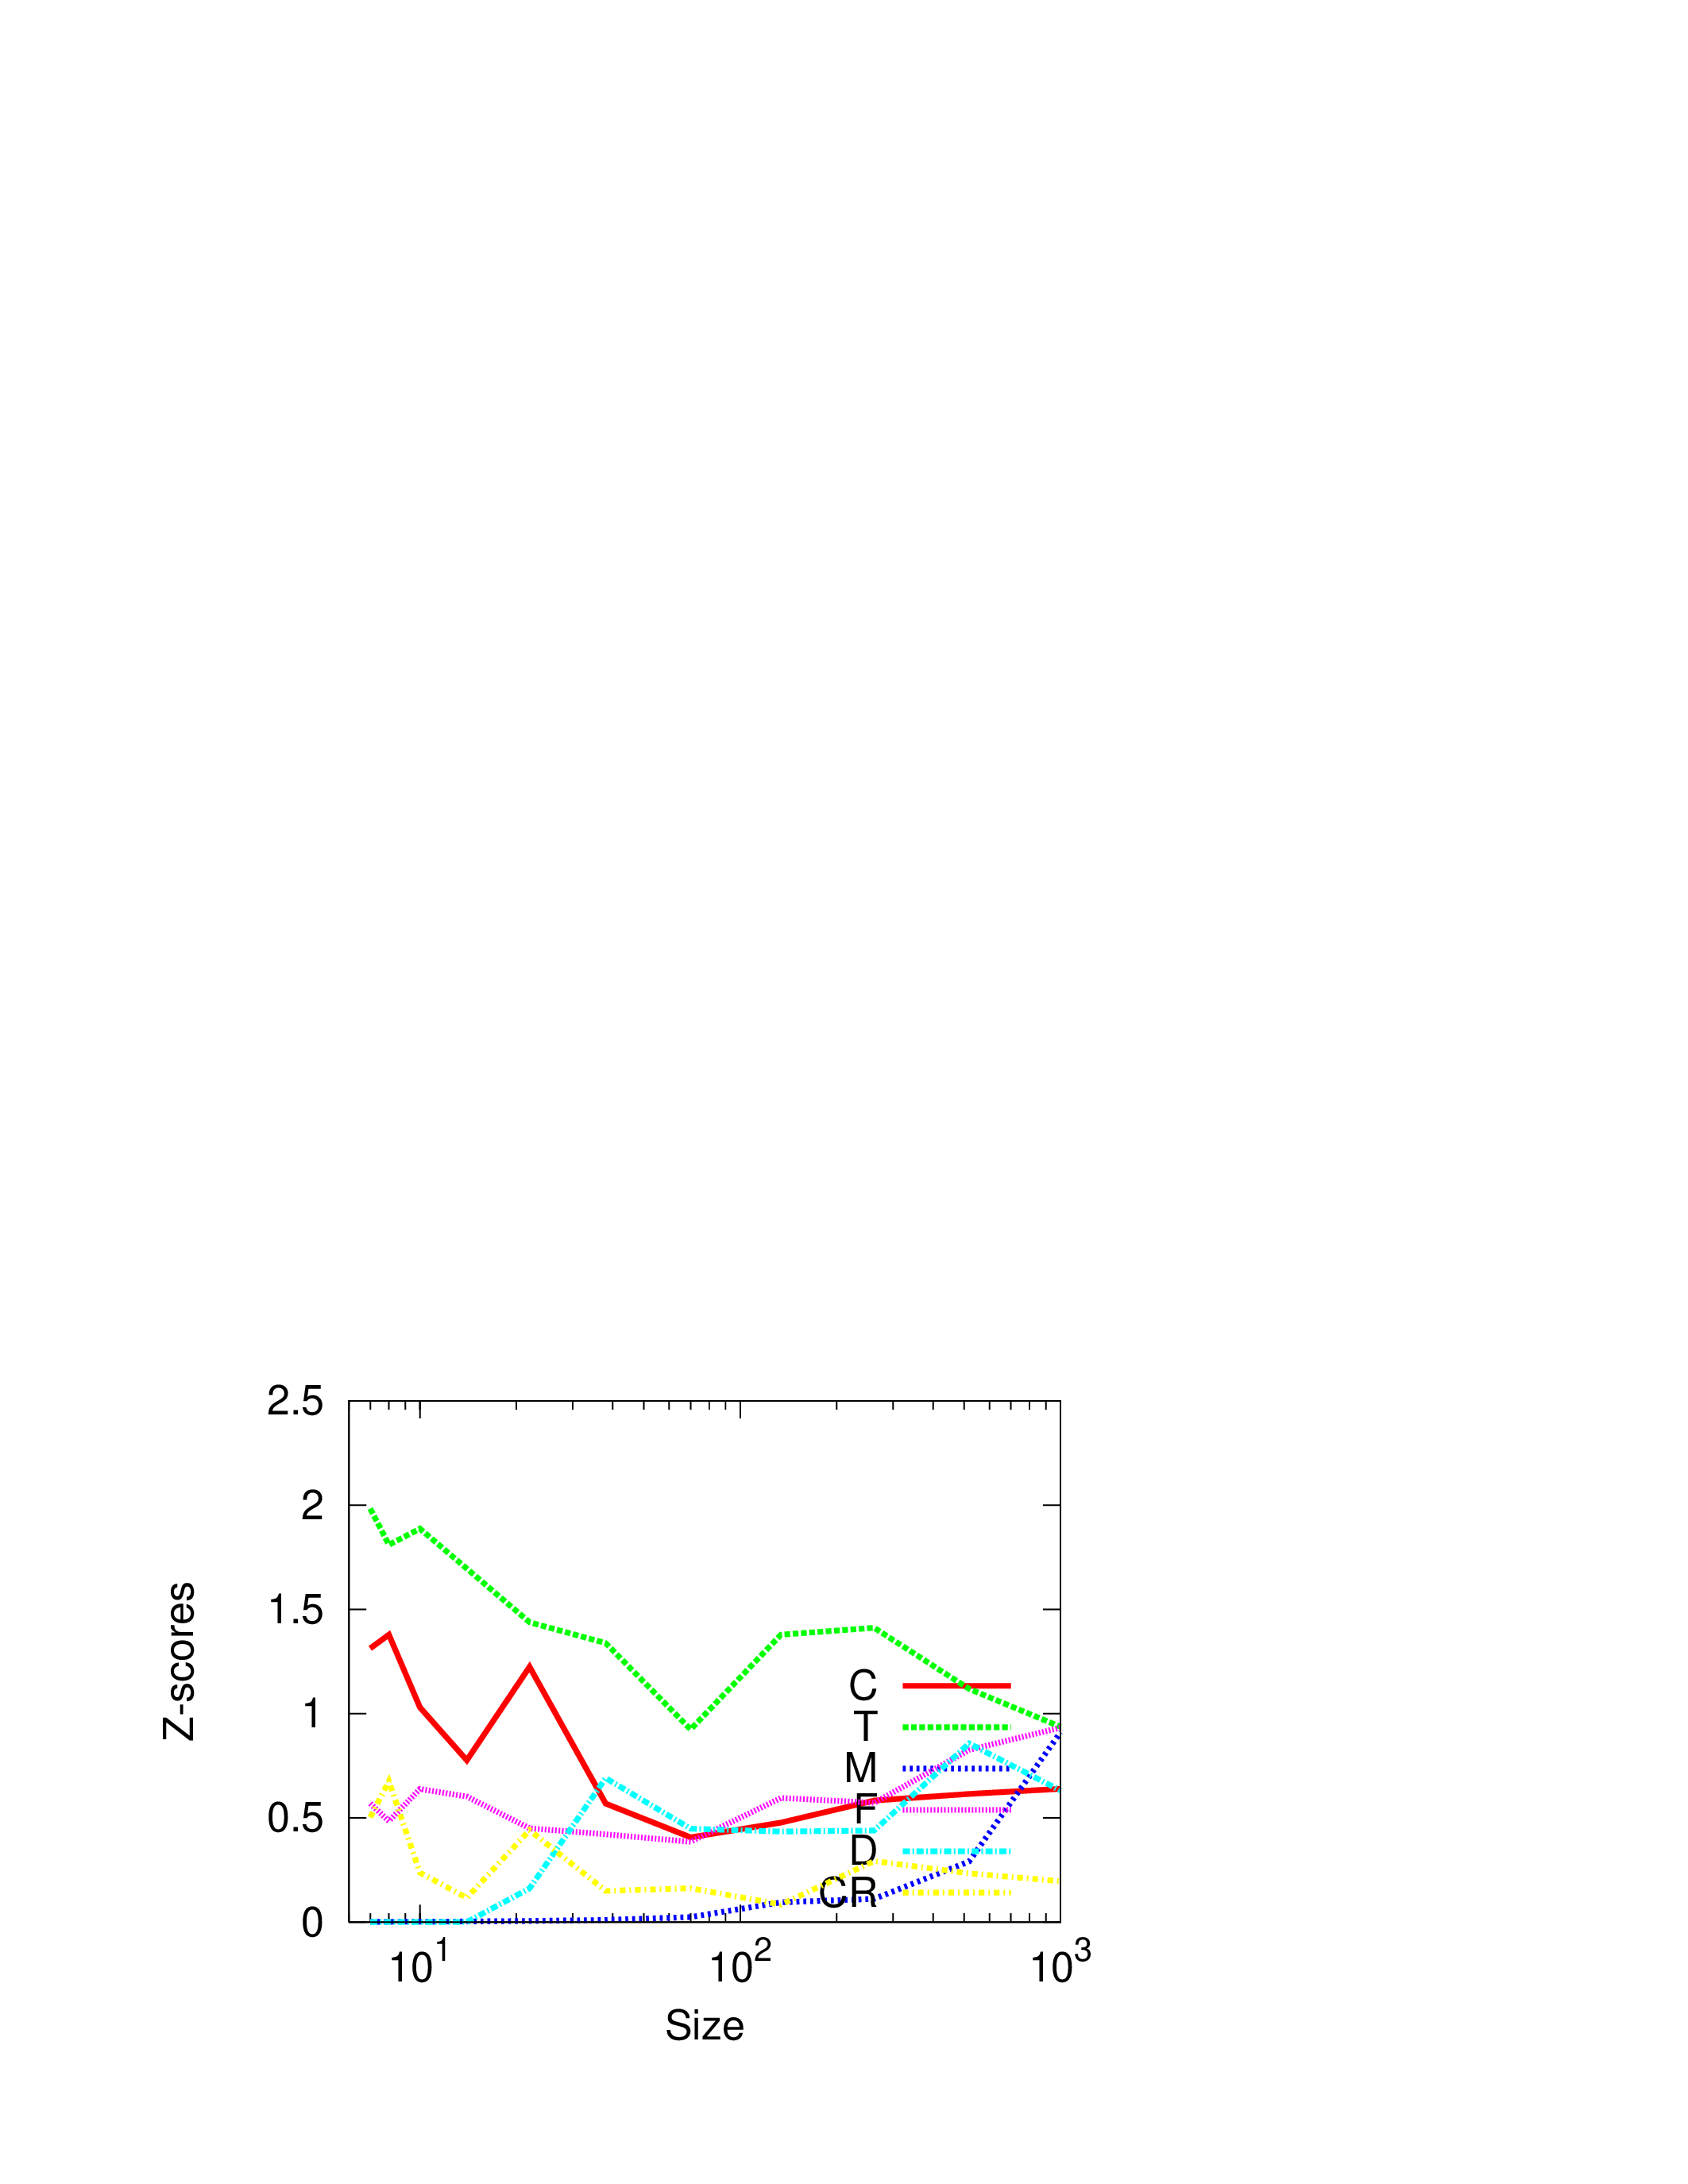}}
	\subfigure[Random	(LJ)]{\includegraphics[width=0.185\textwidth]{zscore.sz.Random.lj.eps}}
	\subfigure[Random	(Ning)]{\includegraphics[width=0.185\textwidth]{zscore.sz.Random.Ning.eps}}
	\subfigure[Random	(Amazon)]{\includegraphics[width=0.185\textwidth]{zscore.sz.Random.amazon.eps}}
	\subfigure[Random	(DBLP)]{\includegraphics[width=0.185\textwidth]{zscore.sz.Random.dblp.eps}}
	\subfigure[Random	(IMDB)]{\includegraphics[width=0.185\textwidth]{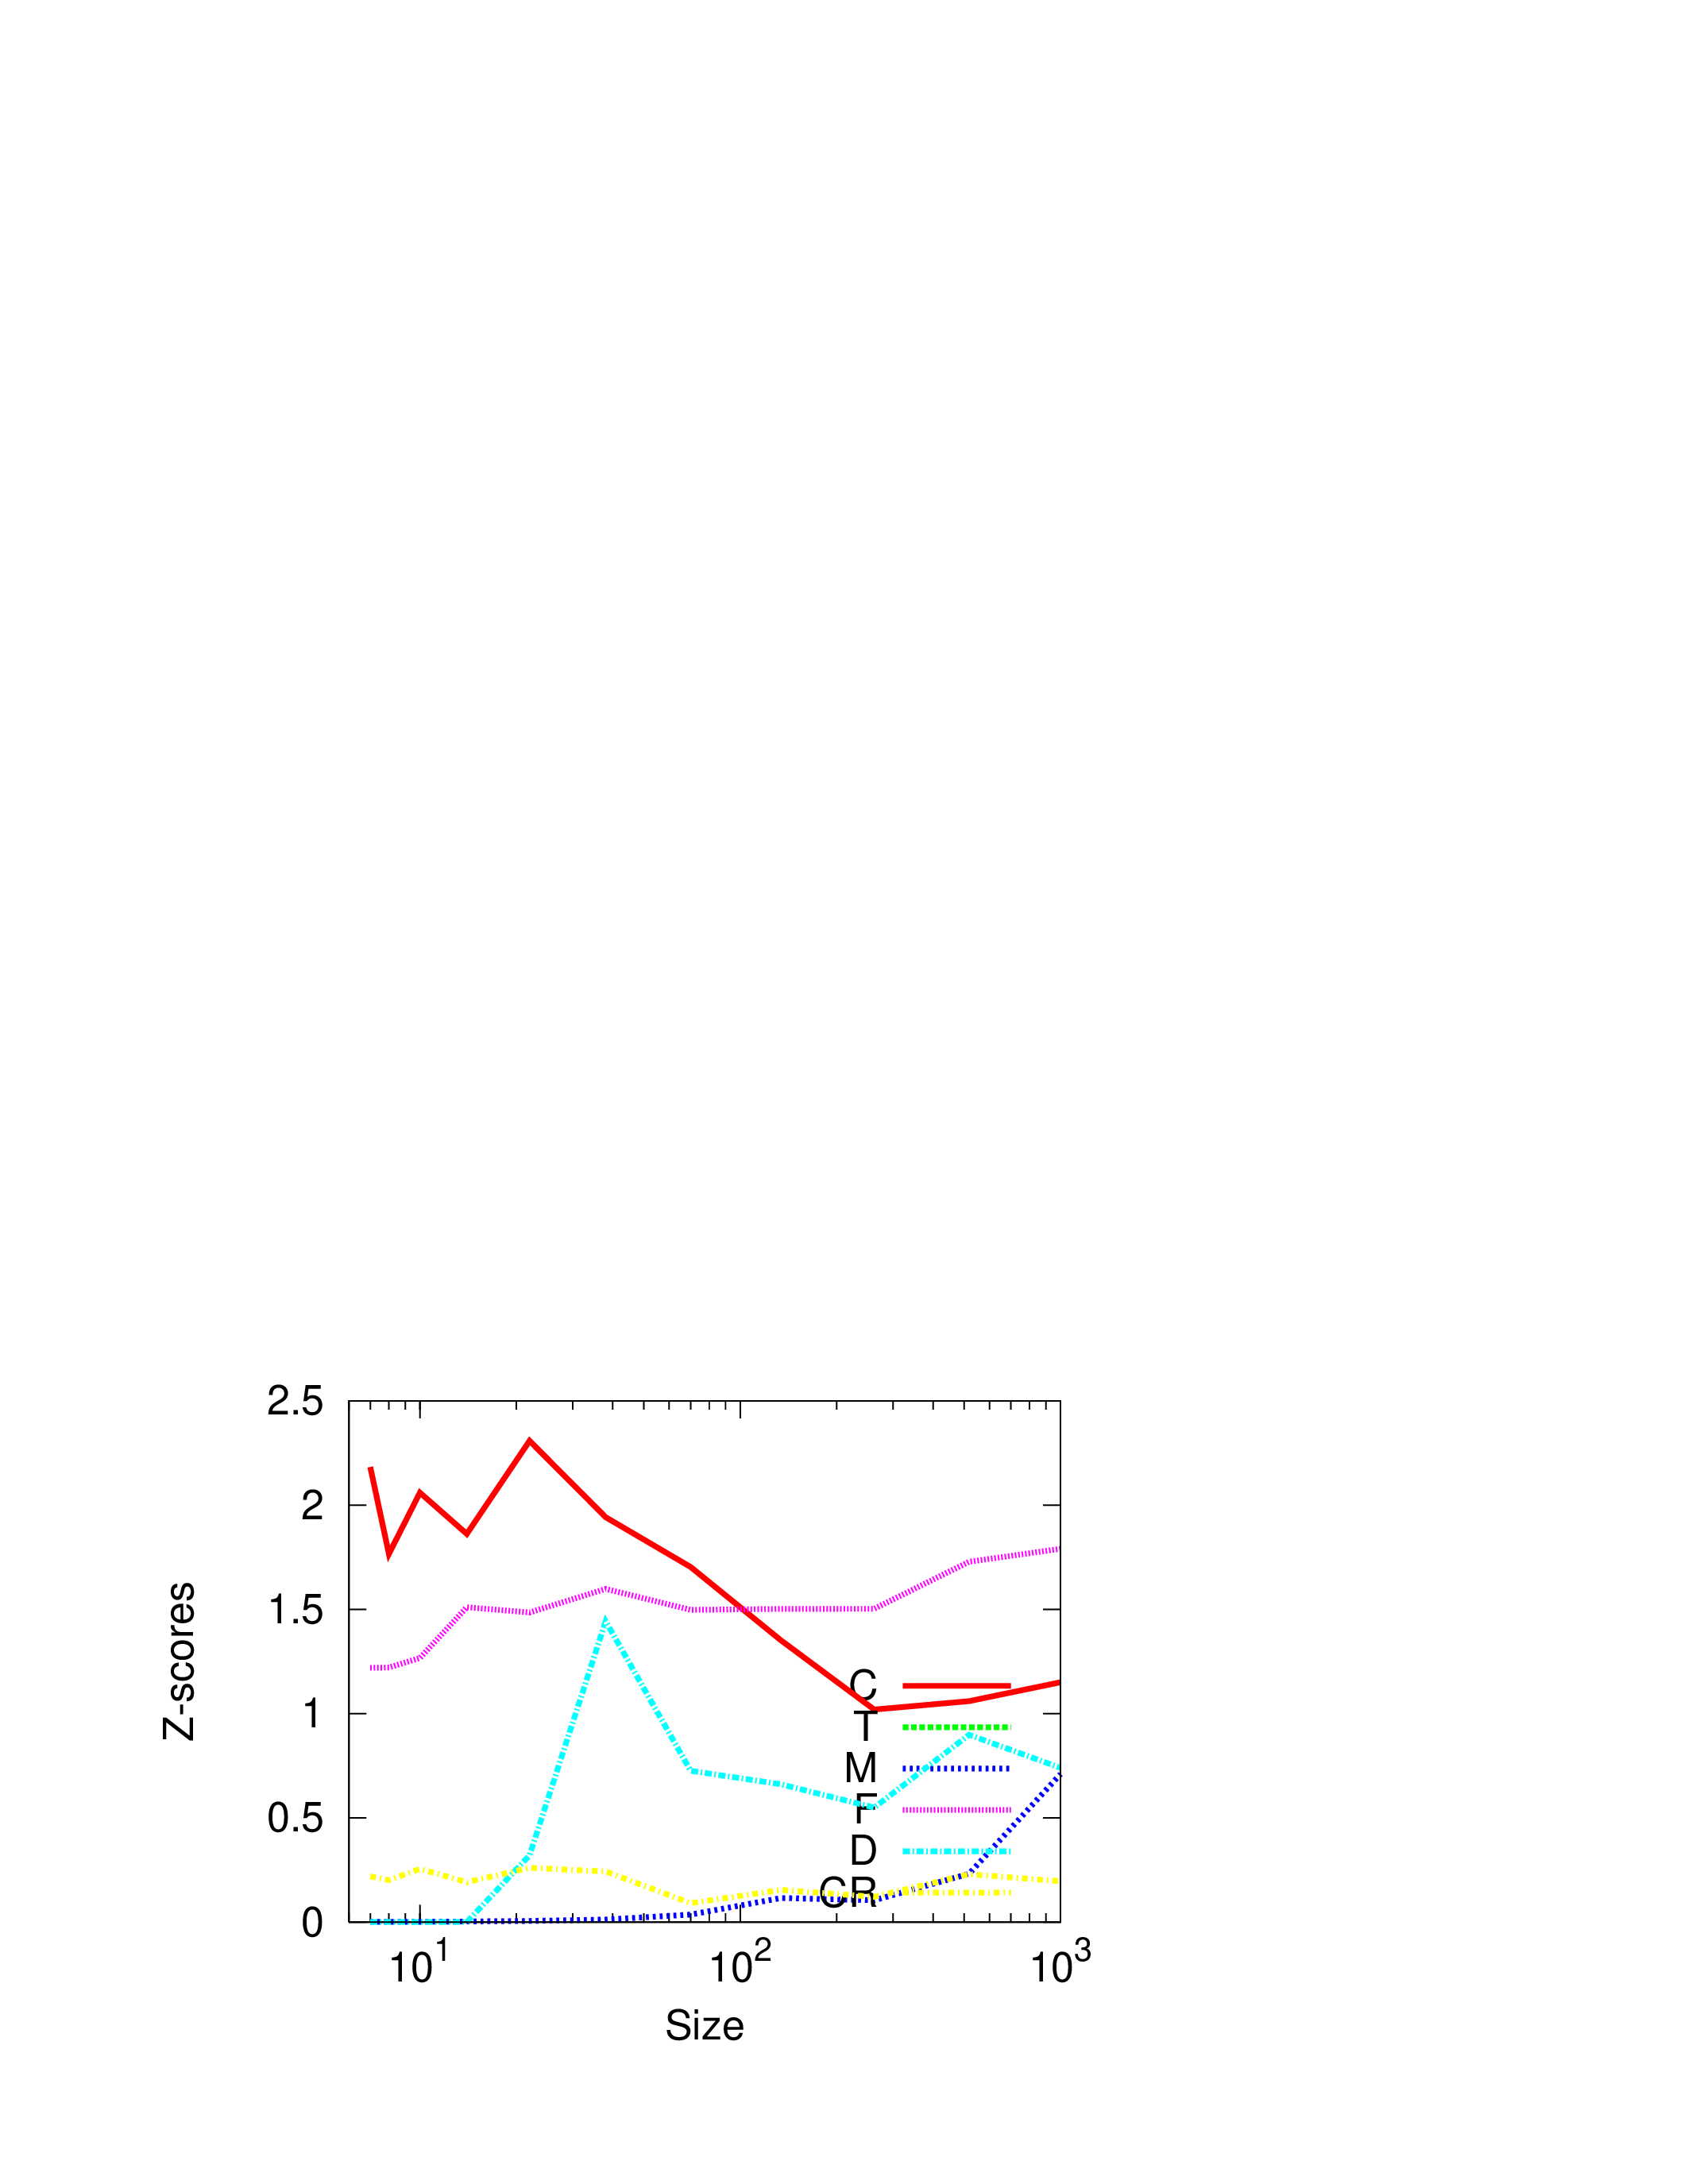}}
	\subfigure[Expand	(LJ)]{\includegraphics[width=0.185\textwidth]{zscore.sz.Expand.lj.eps}}
	\subfigure[Expand	(Ning)]{\includegraphics[width=0.185\textwidth]{zscore.sz.Expand.Ning.eps}}
	\subfigure[Expand	(Amazon)]{\includegraphics[width=0.185\textwidth]{zscore.sz.Expand.amazon.eps}}
	\subfigure[Expand	(DBLP)]{\includegraphics[width=0.185\textwidth]{zscore.sz.Expand.dblp.eps}}
	\subfigure[Expand	(IMDB)]{\includegraphics[width=0.185\textwidth]{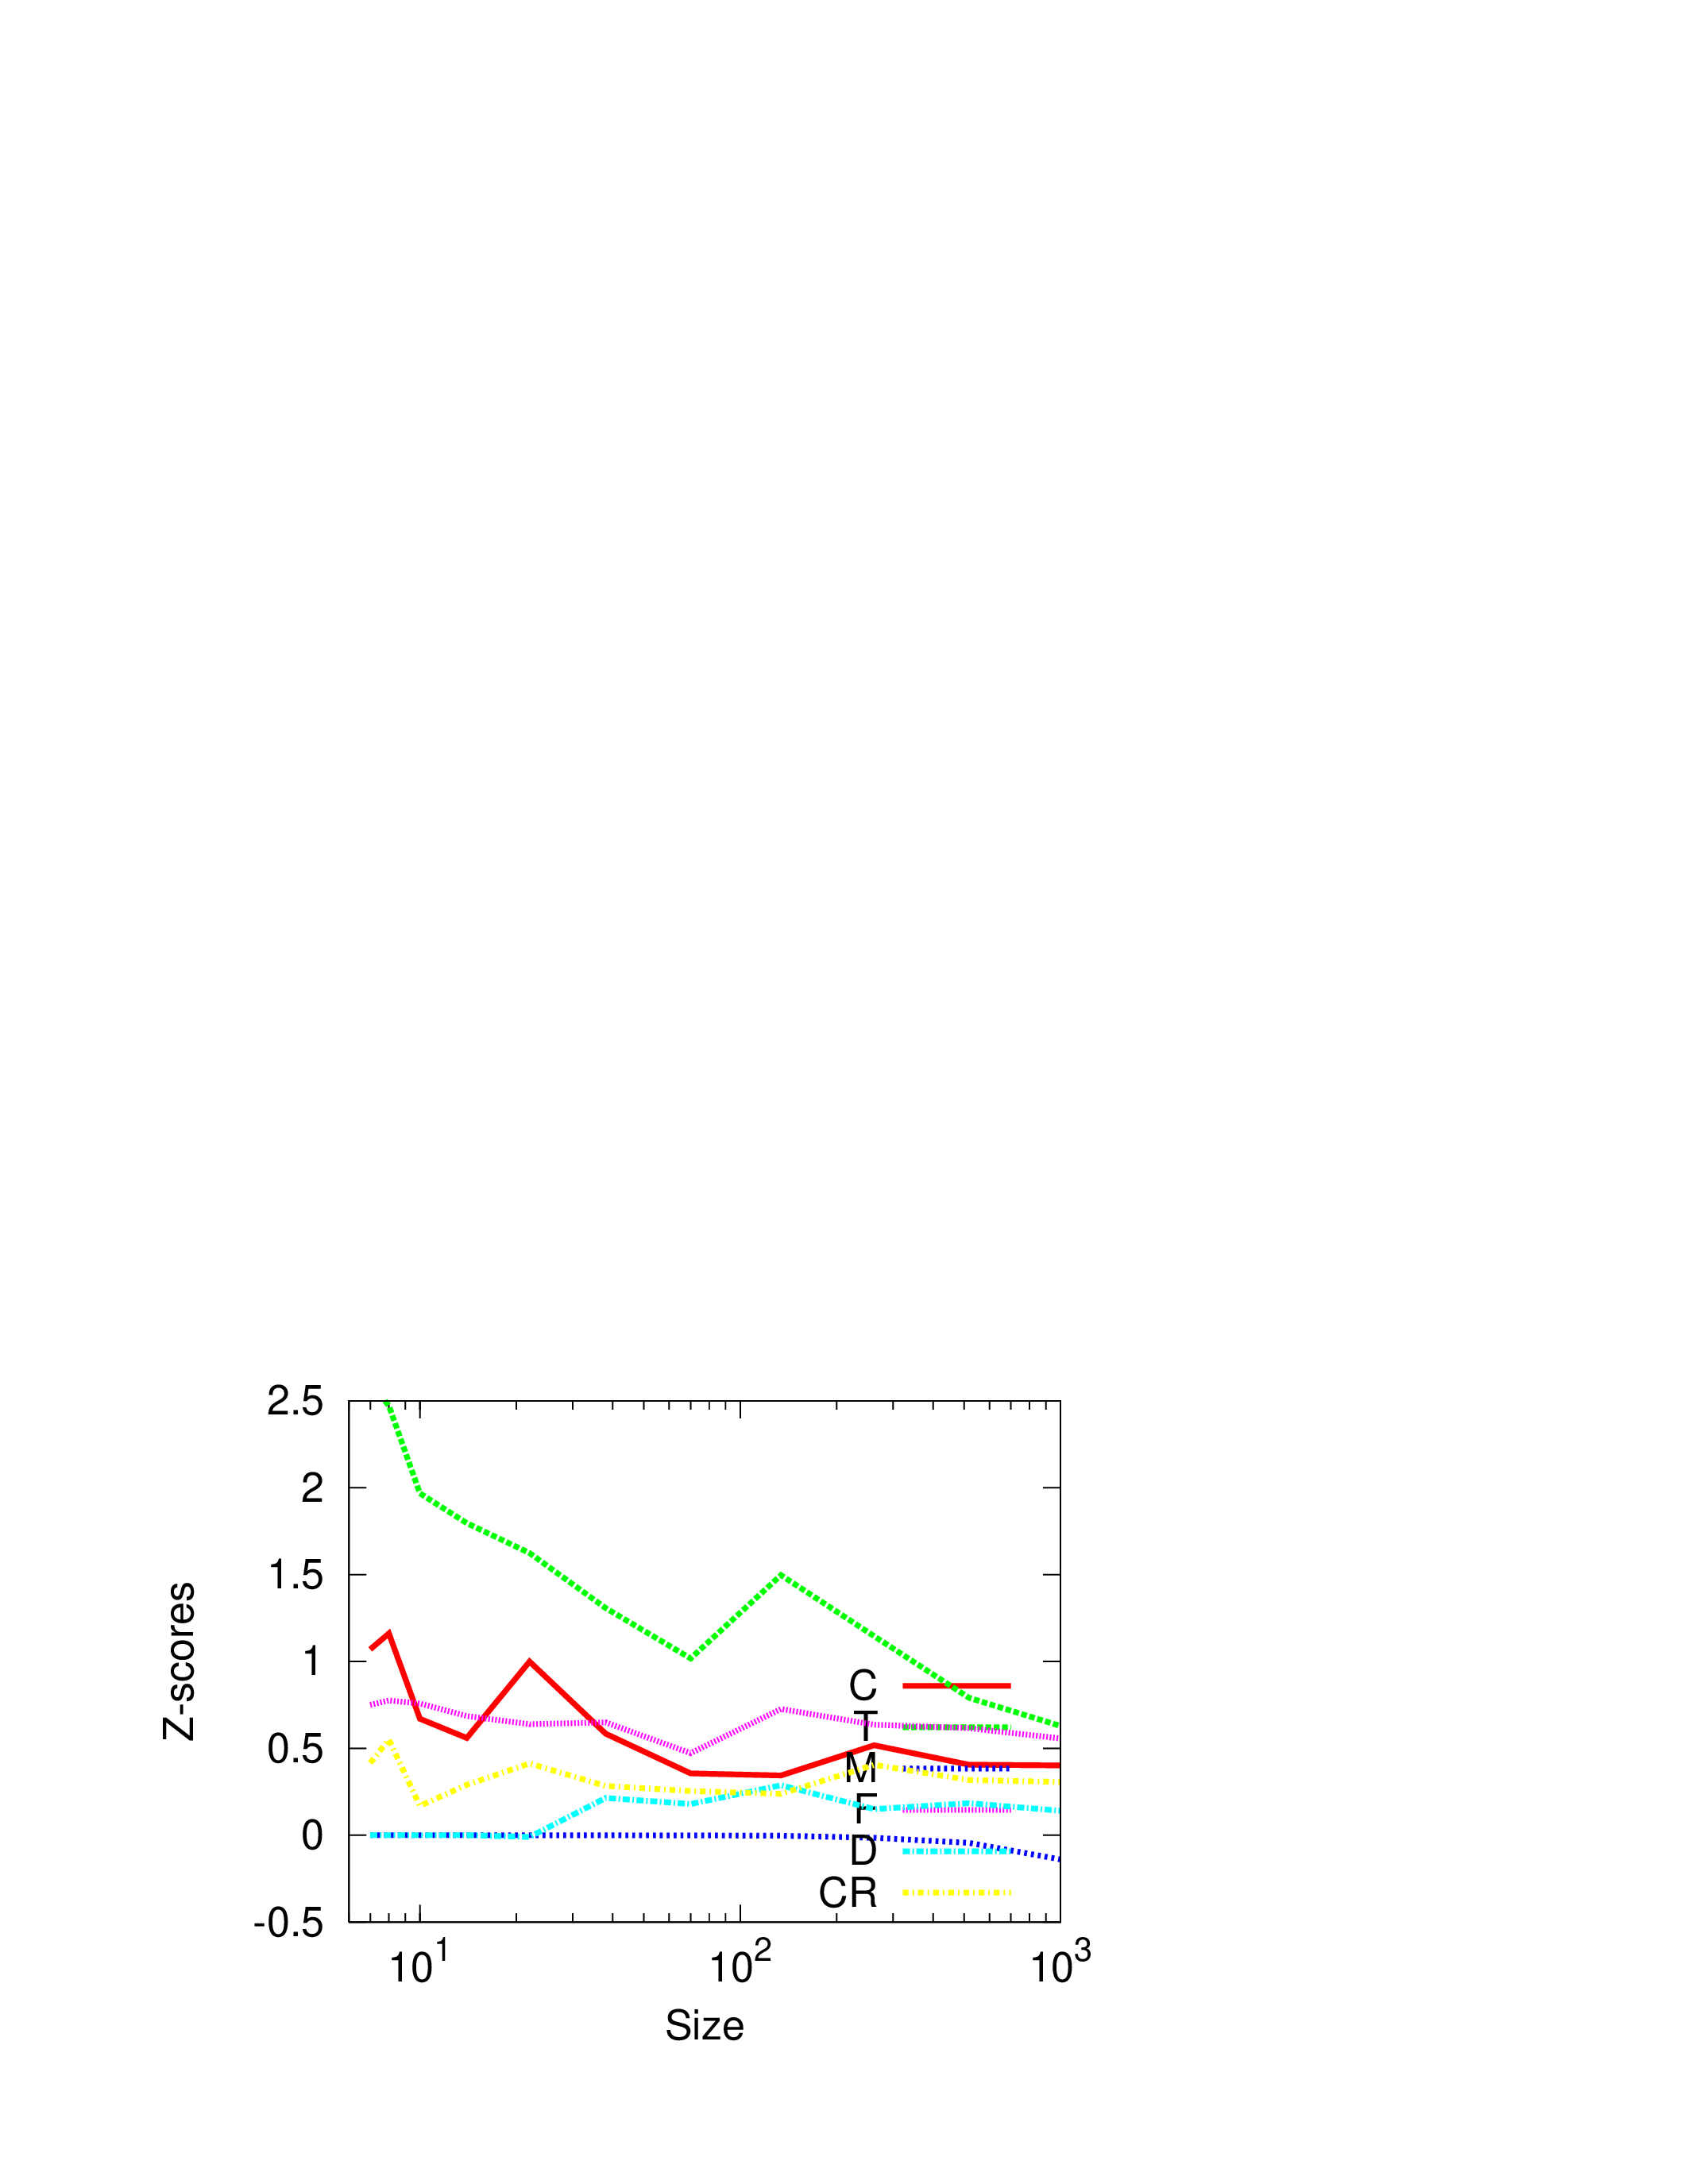}}
	\subfigure[Shrink	(LJ)]{\includegraphics[width=0.185\textwidth]{zscore.sz.Shrink.lj.eps}}
	\subfigure[Shrink	(Ning)]{\includegraphics[width=0.185\textwidth]{zscore.sz.Shrink.Ning.eps}}
	\subfigure[Shrink	(Amazon)]{\includegraphics[width=0.185\textwidth]{zscore.sz.Shrink.amazon.eps}}
	\subfigure[Shrink	(DBLP)]{\includegraphics[width=0.185\textwidth]{zscore.sz.Shrink.dblp.eps}}
	\subfigure[Shrink	(IMDB)]{\includegraphics[width=0.185\textwidth]{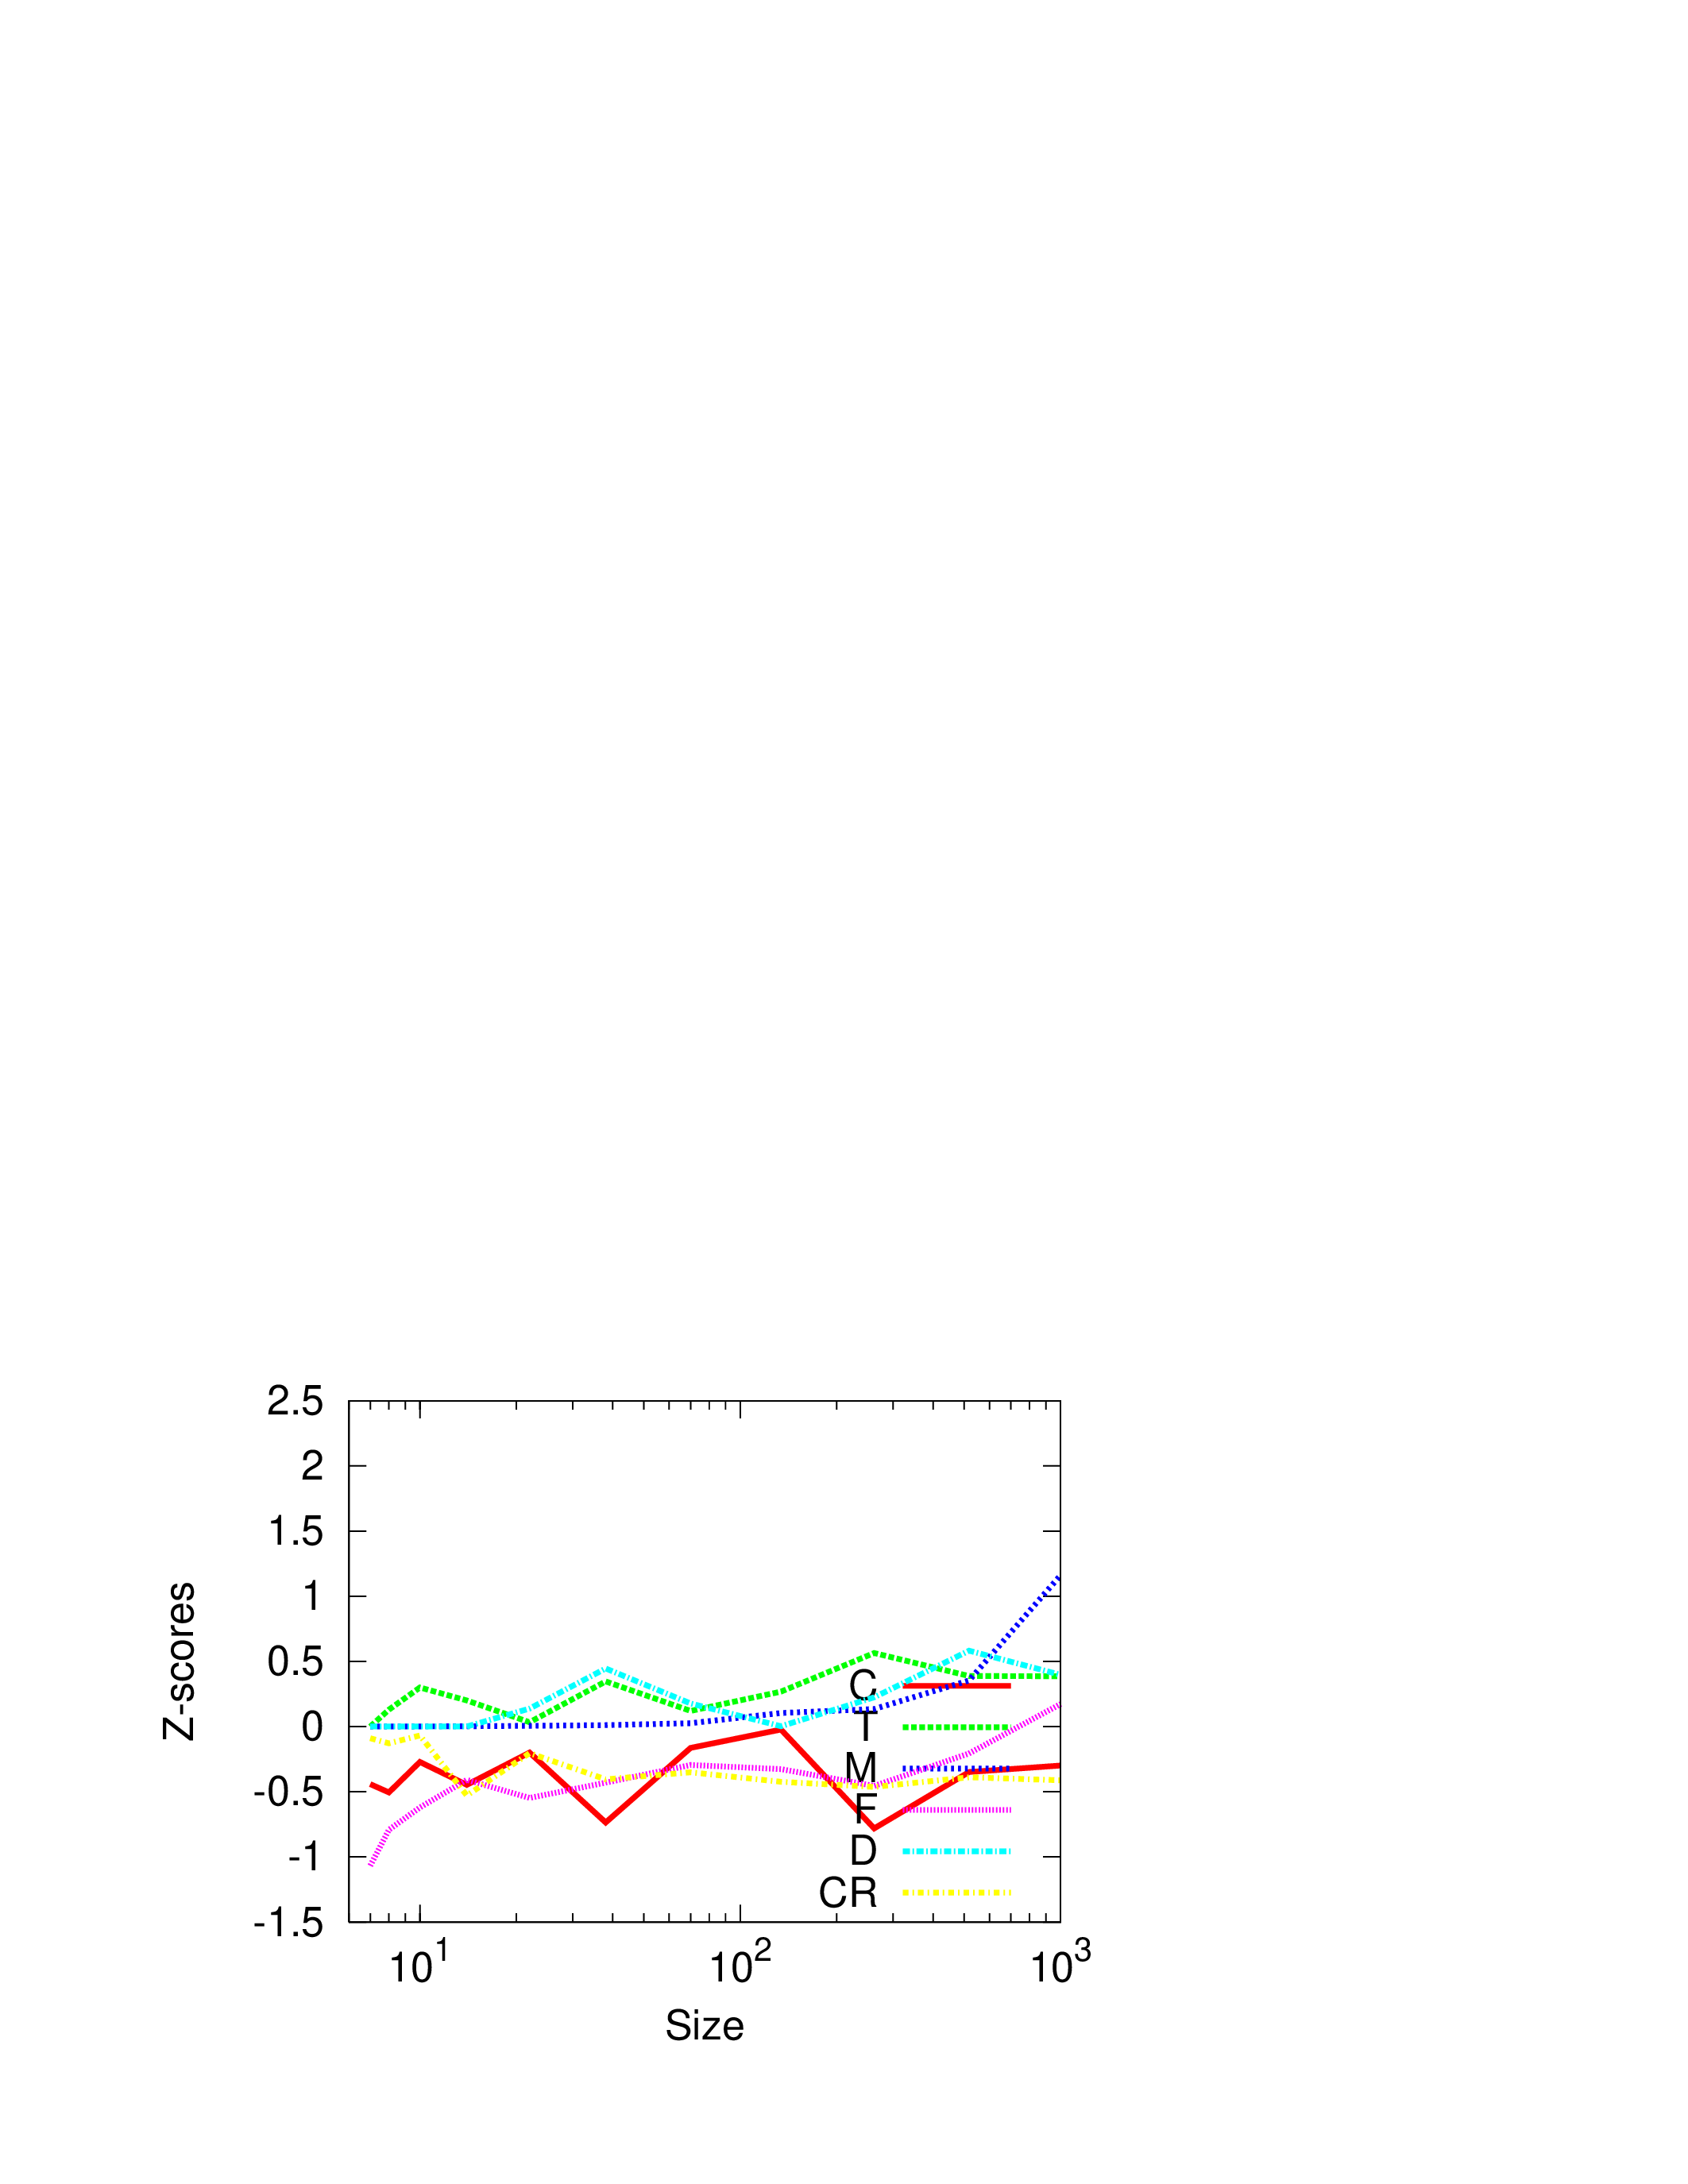}}
	\caption{Z-score as a function of community size at perturbation intensity $p=0.2$.}
\label{fig:Zscore.Sz}
\end{figure*}

\xhdr{Comparison to Local clustering}
It is interesting to compare the performance of the local clustering (LC) to
the generalized local clustering methods. The generalized local clustering method
with conductance finds a smaller community than the local clustering method,
because the generalized local clustering method includes the nodes just up to the first
 local minimum of conductance which is no later than the global minimum.
We confirm this from the fact that conductance always higher precision and smaller recall
than the local clustering (LC) in Table~\ref{table:lc.acc}.
The local clustering results very high recall, almost as high as modularity,
but shows much better precision than modularity.
This means that while modularity just reports a large community
regardless of the goodness of the community,
the local clustering finds a large community while keeping its quality.
Finally, CPM works poorer than our methods
 in IMDB, DBLP, Ning, and LiveJournal (all are social networks),
but shows good performance in the Amazon product network.

\begin{table}[t]
\centering
  \begin{tabular}{l|c|c|c|c|c|c||c}
      &&LJ&Ning&Amazon&DBLP&IMDB&Avg\\ \hline \hline
\multirow{3}{*}{Conductance}&Pr&0.56&0.27&0.91&0.55&0.84&0.62\\ \cline{2-8}
&Rc&0.90&0.50&0.88&0.82&0.71&0.76\\ \cline{2-8}
&F&0.64&0.24&0.87&0.60&0.71&0.61\\ \hline
\multirow{3}{*}{Flake-ODF}&Pr&0.61&0.33&0.88&0.66&0.89&0.67\\ \cline{2-8}
&Rc&0.77&0.27&0.77&0.65&0.66&0.62\\ \cline{2-8}
&F&0.64&0.19&0.75&0.61&0.70&0.58\\ \hline
\multirow{3}{*}{FOMD}&Pr&0.63&0.18&0.95&0.72&0.41&0.58\\ \cline{2-8}
&Rc&0.72&0.54&0.67&0.69&0.85&0.69\\ \cline{2-8}
&F&0.62&0.10&0.73&0.66&0.44&0.51\\ \hline
\multirow{3}{*}{TPR}&Pr&0.61&0.32&0.93&0.74&0.75&0.67\\ \cline{2-8}
&Rc&0.66&0.35&0.77&0.64&0.75&0.63\\ \cline{2-8}
&F&0.57&0.19&0.79&0.65&0.65&0.57\\ \hline
\multirow{3}{*}{Modularity}&Pr&0.09&0.04&0.03&0.02&0.19&0.07\\ \cline{2-8}
&Rc&0.98&0.82&1.00&0.99&0.94&0.95\\ \cline{2-8}
&F&0.15&0.08&0.06&0.04&0.29&0.12\\ \hline
\multirow{3}{*}{CutRatio}&Pr&0.57&0.36&0.90&0.59&0.85&0.65\\ \cline{2-8}
&Rc&0.78&0.26&0.86&0.76&0.69&0.67\\ \cline{2-8}
&F&0.61&0.19&0.85&0.61&0.69&0.59\\ \hline
\multirow{3}{*}{LC}&Pr&0.44&0.14&0.67&0.37&0.72&0.47\\ \cline{2-8}
&Rc&0.93&0.79&0.99&0.92&0.83&0.89\\ \cline{2-8}
&F&0.54&0.17&0.74&0.46&0.71&0.53\\ \hline
\multirow{3}{*}{CPM}&Pr&0.35&0.26&0.91&0.59&0.66&0.56\\ \cline{2-8}
&Rc&0.90&0.45&0.86&0.70&0.77&0.73\\ \cline{2-8}
&F&0.43&0.11&0.85&0.53&0.61&0.51\\ \hline

    \end{tabular}
  \caption{Performance of methods for detecting communities from a seed node.
  Refer to the main text for the naming convention.}
  \vspace{-8mm}
  \label{table:full.lc.acc}
\end{table}

\xhdr{Accuracy for each of multiple communities} Table~\ref{table:multicom.acc} gives the overall performance of our algorithm
for all the communities that a source node belongs to. Now we examine the performance
for each of ground-truth community. We ask the following question:
when a node $s$ belongs to several communities with different sizes,
are smaller communities easier to detect or not?
To investigate this, we conduct the following experiment. We choose a node $s$ that
belongs to $N \geq 5$ communities and detect $\hat{S}_j$'s by our generalized local clustering method.
We sort the ground-truth communities $S_i$ in the ascending order of the community size,
and measure $F(S_i)$ which is the best F1 score between $S_i$ and all $\hat{S}_j$'s.
For example, $F(S_1)$ denotes the best F1 score we can achieve for the smallest ground-truth community,
 \ie, the best performance that we can expect in detecting the smallest community that
 the source node belongs to.

Table~\ref{table:eachcom.acc} shows the results for $F(S_1)$ to $F(S_5)$
for LiveJournal, Amazon, and DBLP where we can find nodes that belong to at least 5 communities.
Note that the score is higher than the last column of Table~\ref{table:multicom.acc},
as the matching between $S_i$ and $S_j$ is not one-to-one in this experiment.
The trend happens differently depending on the data set. In LiveJournal,
the method records higher F1 score for larger ground-truth communities. However,
the performance decreases for larger communities in DBLP. In Amazon,
the score remain stable in very high value.

\begin{table}[t]
\centering
  \begin{tabular}{l||c|c|c}
    Ground-truth community&LJ&Amazon&DBLP\\ \hline \hline
    F($S_1$)&0.40&0.89&0.28\\ \hline
    F($S_2$)&0.47&0.90&0.27\\ \hline
    F($S_3$)&0.51&0.91&0.27\\ \hline
    F($S_4$)&0.55&0.91&0.24\\ \hline
    F($S_5$)&0.58&0.84&0.20\\ \hline
    \end{tabular}
  \caption{F($S_i$): The best F1 score for $S_i$ which is the $i$-th smallest community that a node belongs to}
  \vspace{-8mm}
  \label{table:eachcom.acc}
\end{table}

}
